# Supplementary material for: Ab initio spectroscopic studies of AlF and AlCl molecules
Source: arXiv:2303.08681 source file (2023-03-15)
Supplement: Supplementary file 1 [file AlCl_X1Sigma_S11.pdf]

## AlCl $X^1\Sigma$ --> Centrifugal distortion constants (in $cm^{-1}$)

| v | $D_v$ | $H_v$ | $L_v$ | $M_v$ | $N_v$ | $O_v$ |
|---|---|---|---|---|---|---|
| 0 | -2.4167547D-07 | -1.6916087D-14 | 4.3752060D-19 | -2.8631930D-23 | -2.3074486D-29 | 2.8438339D-33 |
| 1 | -2.3966463D-07 | -2.9785266D-13 | 9.1165424D-19 | 2.2269817D-23 | -4.4115422D-28 | 5.6057628D-33 |
| 2 | -2.3589804D-07 | -3.5382206D-13 | -1.0695411D-18 | 1.3344833D-22 | 1.1492259D-27 | -3.8248151D-32 |
| 3 | -2.3263098D-07 | 4.7880903D-14 | -3.0348954D-19 | -7.2040321D-23 | 5.7726846D-28 | 4.3005523D-32 |
| 4 | -2.2875263D-07 | 1.8727273D-13 | 2.5440609D-18 | -5.0589196D-23 | -3.1139044D-27 | 1.5788946D-32 |
| 5 | -2.2235930D-07 | 1.6863092D-13 | -2.7515995D-18 | 1.0240633D-22 | 3.3045426D-27 | -9.7440887D-32 |
| 6 | -2.1923696D-07 | 3.2612894D-13 | 5.3290465D-20 | -1.2543401D-22 | -1.4932166D-28 | 1.0374276D-31 |
| 7 | -2.1597600D-07 | 3.0233013D-13 | 1.5358049D-18 | -4.6757675D-23 | -2.4451917D-27 | 3.9777497D-32 |
| 8 | -2.1231627D-07 | 2.2203608D-13 | 7.4686735D-20 | 1.1856700D-22 | -2.1386279D-27 | -1.7430057D-31 |
| 9 | -2.0904497D-07 | 2.4983577D-13 | -5.3847583D-18 | -7.7084743D-23 | 6.4229668D-27 | 8.4543121D-32 |
| 10 | -2.0946114D-07 | 1.8684017D-13 | -1.4616586D-18 | -8.9314982D-23 | -3.6986757D-27 | 1.3984972D-31 |
| 11 | -2.1124879D-07 | 6.1719385D-14 | -1.9270428D-18 | 1.2519751D-22 | -1.1636939D-27 | -1.9909889D-31 |
| 12 | -2.1433056D-07 | 4.8534884D-14 | -3.1821792D-18 | 2.4224325D-23 | 5.4370870D-27 | -3.8122574D-32 |
| 13 | -2.1860449D-07 | 6.9931947D-14 | 3.6932239D-19 | -1.8607997D-22 | -5.9159396D-27 | 3.8281765D-31 |
| 14 | -2.2269083D-07 | -4.8591876D-14 | -1.9011118D-18 | 1.8677040D-22 | -2.8587330D-27 | -4.6804836D-31 |
| 15 | -2.2771737D-07 | -5.9529688D-14 | -6.1841324D-18 | -2.2819007D-23 | 1.2453070D-26 | 4.7986385D-32 |
| 16 | -2.3488959D-07 | -7.3503735D-14 | -2.7823468D-19 | -2.1564576D-22 | -8.7222775D-27 | 5.0778682D-31 |
| 17 | -2.4215690D-07 | -1.9589690D-13 | -1.6451859D-18 | 1.5029271D-22 | -4.0168318D-27 | -3.6976928D-31 |
| 18 | -2.5014596D-07 | -2.4034271D-13 | -3.6167033D-18 | 2.0072341D-22 | 9.9592582D-27 | -3.8700971D-31 |
| 19 | -2.5859064D-07 | -1.5912190D-13 | 4.2382588D-19 | -1.3652888D-22 | 5.9936695D-27 | 7.0078564D-31 |
| 20 | -2.6574532D-07 | -8.7392671D-14 | 8.2454867D-18 | 8.1643781D-23 | -1.5602292D-26 | -1.2099172D-31 |
| 21 | -2.6925555D-07 | 4.9032392D-14 | 6.0432532D-18 | 1.1197897D-22 | -3.4416181D-27 | -7.5373425D-31 |
| 22 | -2.6983411D-07 | 1.7800211D-13 | -1.1884111D-18 | -2.8363850D-22 | 2.0590375D-26 | 7.4092412D-31 |
| 23 | -2.7017563D-07 | 1.7217610D-13 | 4.0612831D-18 | -6.9998121D-23 | -8.1173157D-27 | 3.8843877D-31 |
| 24 | -2.6947332D-07 | 1.8672231D-13 | 7.4959131D-18 | 2.3059086D-22 | -8.4284895D-27 | -9.4725330D-31 |
| 25 | -2.6663350D-07 | 2.9615409D-13 | 5.4727191D-18 | -1.3979838D-22 | 3.3788046D-27 | 1.6967542D-32 |
| 26 | -2.6225452D-07 | 3.2003951D-13 | 1.8067334D-18 | -2.5473983D-22 | 1.9824616D-26 | 9.2324291D-31 |
| 27 | -2.5785623D-07 | 2.8500266D-13 | 9.8878963D-18 | -2.3776177D-23 | -3.2300493D-26 | -1.0060861D-31 |
| 28 | -2.5202594D-07 | 2.5414018D-13 | 3.0269972D-18 | -6.3388698D-23 | -5.5843133D-27 | -5.4338850D-31 |
| 29 | -2.4656540D-07 | 1.2278114D-13 | -5.3589926D-18 | 7.3443969D-23 | 2.9072233D-26 | -7.7482610D-31 |
| 30 | -2.4330758D-07 | -1.5135443D-15 | -2.1384891D-18 | -3.2699494D-22 | -3.2633196D-27 | 2.0769695D-30 |
| 31 | -2.4174679D-07 | -1.8817869D-13 | 7.1423438D-21 | 1.3932101D-22 | -2.1453834D-26 | 3.5707670D-31 |
| 32 | -2.4151245D-07 | -3.1977045D-13 | 1.2618625D-18 | 8.5822558D-22 | -3.3519604D-27 | -3.6989551D-30 |
| 33 | -2.4122853D-07 | -2.2744549D-13 | -1.5714280D-18 | -2.1845566D-22 | 2.2428922D-26 | 1.7927040D-30 |
| 34 | -2.4081376D-07 | -2.2374590D-13 | -2.0062091D-18 | -9.5531984D-23 | 1.1295374D-26 | 7.8113455D-31 |
| 35 | -2.4066905D-07 | -2.1593634D-13 | 2.9051265D-18 | -5.0677239D-23 | -2.5196566D-26 | 1.0919925D-30 |
| 36 | -2.4002852D-07 | -2.0464421D-13 | 2.4039884D-18 | 4.9002904D-22 | -8.2204732D-27 | -3.3579960D-30 |
| 37 | -2.3862750D-07 | -1.0584048D-13 | -2.8621301D-18 | -3.1799353D-22 | 2.0455613D-26 | 9.5563405D-31 |
| 38 | -2.3732575D-07 | -1.3009873D-13 | -6.2103428D-18 | -2.1168334D-22 | 4.1761889D-26 | 1.4472308D-30 |
| 39 | -2.3704138D-07 | -1.4364162D-13 | 6.2531357D-18 | -1.0725941D-22 | -5.1305013D-26 | 9.7439072D-31 |
| 40 | -2.3593583D-07 | -1.3054193D-13 | 3.0064990D-18 | 3.4060266D-23 | -1.1988344D-26 | -8.9148557D-31 |
| 41 | -2.3455702D-07 | -1.4684561D-13 | -1.7326961D-19 | 3.0672381D-22 | 9.4294808D-27 | -2.5289586D-30 |
| 42 | -2.3322588D-07 | -1.2647169D-13 | -2.1608848D-18 | -1.1981950D-22 | 3.8546055D-26 | 1.3391243D-30 |
| 43 | -2.3207223D-07 | -1.1021318D-13 | 3.2834610D-18 | -4.1094289D-22 | -3.5783471D-26 | 3.9703432D-30 |

| | | | | | | |
|---|---|---|---|---|---|---|
| 44 | -2.3069235D-07 | -1.5635889D-13 | 2.3845663D-18 | 5.1518741D-22 | -2.5806904D-26 | -4.2735264D-30 |
| 45 | -2.2916536D-07 | -1.3107114D-13 | -2.4172120D-18 | 7.6189658D-23 | 2.0769978D-26 | 1.9022588D-31 |
| 46 | -2.2783418D-07 | -1.3119504D-13 | -2.7018497D-18 | 3.1255512D-22 | 2.4591633D-26 | -2.6388195D-30 |
| 47 | -2.2652325D-07 | -6.7356636D-14 | -2.3369388D-18 | -6.7907578D-22 | 1.4249390D-26 | 5.9303886D-30 |
| 48 | -2.2537869D-07 | -1.0764090D-13 | 1.4473854D-18 | 2.0693242D-22 | -2.9446679D-26 | -2.0198434D-30 |
| 49 | -2.2415127D-07 | -8.2414404D-14 | 1.4179595D-18 | -8.9349274D-23 | -2.2218398D-26 | 3.1756176D-31 |
| 50 | -2.2277819D-07 | -1.0275477D-13 | -2.8329135D-18 | 3.8308428D-22 | 3.0486337D-26 | -3.9911003D-30 |
| 51 | -2.2164477D-07 | -6.7558705D-14 | -1.0352386D-18 | -2.6609415D-22 | 2.0912859D-26 | 2.1009378D-30 |
| 52 | -2.2044517D-07 | -5.9715786D-14 | -7.4891160D-20 | -4.3600976D-22 | 3.2397780D-27 | 4.2500087D-30 |
| 53 | -2.1937953D-07 | -8.5776213D-14 | 4.9995473D-18 | 1.1389607D-22 | -6.1386309D-26 | -1.4461876D-30 |
| 54 | -2.1800615D-07 | -9.2244567D-14 | -2.6320423D-19 | 1.7383575D-22 | 1.0552809D-26 | -6.4287774D-31 |
| 55 | -2.1679522D-07 | -1.0135375D-13 | 1.0953432D-18 | 4.6440364D-22 | -2.7727731D-26 | -4.4724416D-30 |
| 56 | -2.1540257D-07 | -7.9754892D-14 | -6.4233191D-18 | 1.1840147D-22 | 9.4647401D-26 | -1.2251699D-30 |
| 57 | -2.1436698D-07 | -4.2920071D-14 | -1.0704733D-20 | -6.8611481D-22 | -1.5948700D-26 | 8.4503114D-30 |
| 58 | -2.1325133D-07 | -6.4746032D-14 | 1.8203882D-18 | 7.9072989D-23 | -4.2885274D-26 | -1.8190230D-30 |
| 59 | -2.1208550D-07 | -6.5272020D-14 | 4.1646247D-19 | 1.3876540D-22 | -1.1440595D-26 | -1.4858653D-30 |
| 60 | -2.1091779D-07 | -6.6704556D-14 | -1.0135226D-18 | 2.9301563D-22 | 4.2356538D-27 | -3.4458108D-30 |
| 61 | -2.0976367D-07 | -5.0484022D-14 | -3.2914731D-18 | 1.4196535D-23 | 4.8210693D-26 | -6.1062802D-31 |
| 62 | -2.0872584D-07 | -3.0453777D-14 | -1.0787317D-18 | -4.2377988D-22 | 1.2958556D-26 | 4.6872360D-30 |
| 63 | -2.0771719D-07 | -3.5957355D-14 | 1.7699467D-18 | -2.1865503D-22 | -2.8259471D-26 | 1.7771181D-30 |
| 64 | -2.0665732D-07 | -4.5423136D-14 | 2.2897764D-18 | -4.8987164D-24 | -3.0083188D-26 | -2.1641100D-31 |
| 65 | -2.0555602D-07 | -5.7870703D-14 | 1.3665253D-18 | 2.7083259D-22 | -1.5709391D-26 | -2.7327333D-30 |
| 66 | -2.0442553D-07 | -5.5197780D-14 | -5.7457576D-19 | 1.9987661D-22 | 7.1245421D-27 | -1.5241120D-30 |
| 67 | -2.0332597D-07 | -5.1916975D-14 | -1.7503711D-18 | 2.3013947D-22 | 2.5467899D-26 | -2.9694425D-30 |
| 68 | -2.0224603D-07 | -3.1275060D-14 | -2.7633469D-18 | -3.1476654D-22 | 4.4272123D-26 | 5.3437064D-30 |
| 69 | -2.0128688D-07 | -2.9267154D-14 | 2.0062142D-18 | -2.0327551D-22 | -6.1967768D-26 | 2.5181348D-30 |
| 70 | -2.0020971D-07 | -4.2643752D-14 | -9.9728414D-19 | 3.6780257D-22 | 1.7835575D-26 | -6.5812850D-30 |
| 71 | -1.9918860D-07 | -2.0855758D-14 | -9.5104880D-19 | -3.5516897D-22 | 1.3884290D-26 | 6.7574905D-30 |
| 72 | -1.9821716D-07 | -3.3928782D-14 | 1.7746064D-18 | 2.5428861D-22 | -5.9592037D-26 | -4.2813055D-30 |
| 73 | -1.9713602D-07 | -3.0200662D-14 | -3.2598586D-18 | 2.8209212D-22 | 6.7355421D-26 | -5.5759797D-30 |
| 74 | -1.9617949D-07 | -7.0060460D-15 | -1.2807159D-18 | -4.7501604D-22 | 2.4171089D-26 | 7.5049766D-30 |
| 75 | -1.9523863D-07 | -1.3567877D-14 | 1.2809305D-18 | -1.4586931D-22 | -2.9829507D-26 | 1.0527944D-30 |
| 76 | -1.9425712D-07 | -1.5240857D-14 | 1.1126256D-18 | -1.0806019D-22 | -1.2760606D-26 | 1.2606775D-30 |
| 77 | -1.9328338D-07 | -2.2810525D-14 | 2.1259389D-18 | 1.1150006D-22 | -4.0494428D-26 | -1.3170810D-30 |
| 78 | -1.9225252D-07 | -2.8722396D-14 | -1.4951843D-19 | 3.3052542D-22 | 9.3651432D-27 | -4.6598249D-30 |
| 79 | -1.9124114D-07 | -1.9721862D-14 | -1.0669785D-18 | 3.4238068D-23 | 2.0120737D-26 | 9.1567080D-31 |
| 80 | -1.9025326D-07 | -1.7063316D-14 | -8.2662540D-19 | 8.4633829D-23 | 5.8104077D-27 | -1.3337635D-30 |
| 81 | -1.8926022D-07 | -9.1192749D-15 | -1.7703628D-18 | -9.4253400D-23 | 3.5339167D-26 | 1.4606851D-30 |
| 82 | -1.8831784D-07 | -1.8064988D-15 | 2.5347885D-19 | -3.1190496D-22 | -1.9678059D-26 | 5.8497170D-30 |
| 83 | -1.8737104D-07 | -1.1197983D-14 | 1.0586793D-18 | 1.4024838D-22 | -4.2111148D-26 | -3.4829598D-30 |
| 84 | -1.8640410D-07 | -1.3011553D-14 | -1.3441853D-18 | 1.6882252D-22 | 2.6525565D-26 | -3.3453640D-30 |
| 85 | -1.8551157D-07 | -8.4884205D-15 | -9.4224240D-19 | -1.5023772D-22 | 3.7871557D-27 | 4.0800926D-30 |
| 86 | -1.8467748D-07 | -1.6647601D-14 | -1.4716640D-19 | 1.4076515D-22 | -2.7019478D-26 | -3.0615528D-30 |
| 87 | -1.8386388D-07 | -1.8393312D-14 | -2.1341650D-18 | 1.9598427D-22 | 4.4128964D-26 | -5.4265342D-30 |
| 88 | -1.8311572D-07 | -6.4831885D-15 | -1.7800939D-18 | -3.6118928D-22 | 4.9961017D-26 | 6.6985825D-30 |
| 89 | -1.8241588D-07 | -5.4631500D-15 | 1.3775903D-18 | -4.3583146D-22 | -3.8970669D-26 | 7.8927402D-30 |
| 90 | -1.8169870D-07 | -1.9183371D-14 | 2.1886656D-18 | 6.1080468D-23 | -5.8448849D-26 | -2.4052499D-30 |

| | | | | | | |
|---|---|---|---|---|---|---|
| 91 | -1.8097367D-07 | -2.8792125D-14 | 5.2561172D-19 | 2.7556781D-22 | -2.1101290D-27 | -5.3940964D-30 |
| 92 | -1.8027793D-07 | -2.8236410D-14 | -2.2813174D-19 | 7.8345416D-23 | 1.4090772D-26 | 8.2952597D-31 |
| 93 | -1.7960516D-07 | -2.8630659D-14 | 9.3169409D-20 | 5.3714482D-23 | -1.8158622D-26 | 1.5333141D-30 |
| 94 | -1.7894003D-07 | -3.3371405D-14 | -7.9671017D-19 | 2.9673852D-22 | -6.0806437D-27 | -5.4626780D-30 |
| 95 | -1.7829765D-07 | -3.0018937D-14 | -2.5547989D-18 | 1.9023030D-22 | 5.2119197D-26 | -4.4144211D-30 |
| 96 | -1.7770167D-07 | -1.8957065D-14 | -2.4235807D-18 | -2.8179902D-22 | 5.1747042D-26 | 5.4527400D-30 |
| 97 | -1.7715190D-07 | -1.6803562D-14 | -3.0039093D-19 | -3.9022773D-22 | -1.1914929D-26 | 7.3981245D-30 |
| 98 | -1.7661917D-07 | -2.3181706D-14 | 1.0879337D-18 | -1.2795004D-22 | -4.2130644D-26 | 1.3463617D-30 |
| 99 | -1.7608231D-07 | -2.8634843D-14 | 9.2048202D-19 | 3.4455292D-23 | -3.0627757D-26 | -1.0340091D-30 |
| 100 | -1.7555682D-07 | -3.4548847D-14 | 5.3642143D-19 | 1.8865321D-22 | -2.5852296D-26 | -3.0497476D-30 |
| 101 | -1.7504240D-07 | -3.7999841D-14 | -5.6000230D-19 | 3.1634071D-22 | 2.3284352D-27 | -6.4348741D-30 |
| 102 | -1.7454071D-07 | -3.4965685D-14 | -2.1972678D-18 | 1.4224985D-22 | 5.1041914D-26 | -2.9239981D-30 |
| 103 | -1.7408524D-07 | -2.9211091D-14 | -1.8443498D-18 | -1.7450056D-22 | 3.7677814D-26 | 3.9920917D-30 |
| 104 | -1.7366117D-07 | -2.7803490D-14 | -6.1473917D-19 | -2.3376947D-22 | 2.6259046D-29 | 3.4111323D-30 |
| 105 | -1.7325017D-07 | -3.0850820D-14 | -2.0902162D-19 | -1.4945007D-22 | 4.7966496D-27 | 6.3961476D-31 |
| 106 | -1.7285957D-07 | -3.1680982D-14 | 4.9442912D-19 | -2.8910029D-22 | -3.0358474D-27 | 5.9079746D-30 |
| 107 | -1.7248803D-07 | -3.8015421D-14 | 2.0165771D-18 | -1.8643562D-22 | -6.0938904D-26 | 5.7551583D-30 |
| 108 | -1.7211623D-07 | -5.0289885D-14 | 2.2105880D-18 | 3.0979696D-22 | -7.7048520D-26 | -6.5340370D-30 |
| 109 | -1.7172948D-07 | -5.7407180D-14 | -4.6373554D-19 | 5.5863750D-22 | 1.3124806D-26 | -1.2647132D-29 |
| 110 | -1.7136940D-07 | -5.3146601D-14 | -2.3105799D-18 | 1.8251413D-22 | 7.0345356D-26 | -1.3787226D-30 |
| 111 | -1.7105244D-07 | -4.7783848D-14 | -1.6591044D-18 | -1.7570405D-22 | 2.2681889D-26 | 8.0177805D-30 |
| 112 | -1.7076347D-07 | -5.0171648D-14 | -5.7051945D-19 | 1.1215249D-23 | -3.0991402D-26 | -3.3908236D-33 |
| 113 | -1.7047775D-07 | -5.2376645D-14 | -1.6617742D-18 | 1.9651526D-22 | 1.9811429D-26 | -8.1085194D-30 |
| 114 | -1.7021813D-07 | -4.8001778D-14 | -2.5186909D-18 | -1.1209167D-22 | 7.2836808D-26 | 2.9053248D-31 |
| 115 | -1.6999937D-07 | -4.3076293D-14 | -1.0804952D-18 | -5.3406305D-22 | 2.5688914D-26 | 1.3411295D-29 |
| 116 | -1.6980967D-07 | -4.8047648D-14 | 1.5314419D-18 | -3.8092307D-22 | -7.4816022D-26 | 9.5614212D-30 |
| 117 | -1.6961520D-07 | -5.9313585D-14 | 1.8676392D-18 | 1.4972077D-22 | -8.3406098D-26 | -5.6879304D-30 |
| 118 | -1.6941904D-07 | -6.6726433D-14 | 2.1325677D-19 | 4.0720566D-22 | -1.0267690D-26 | -1.2030229D-29 |
| 119 | -1.6923928D-07 | -6.6829447D-14 | -1.3577976D-18 | 1.9862540D-22 | 4.9097412D-26 | -4.1305713D-30 |
| 120 | -1.6909309D-07 | -6.5251447D-14 | -1.1797538D-18 | -6.8704330D-23 | 2.8761695D-26 | 4.1418421D-30 |
| 121 | -1.6896945D-07 | -6.7073415D-14 | -6.4948128D-19 | -6.5081122D-23 | -2.8792661D-27 | 2.6082164D-30 |
| 122 | -1.6886249D-07 | -6.9868395D-14 | -5.9944974D-19 | 9.8274028D-24 | -3.0203466D-27 | -1.3271726D-30 |
| 123 | -1.6877253D-07 | -7.1914143D-14 | -9.0629013D-19 | -8.5973061D-24 | 1.7034276D-26 | -1.1854094D-30 |
| 124 | -1.6870681D-07 | -7.2904779D-14 | -7.1985617D-19 | -1.4115878D-22 | 1.2840014D-26 | 3.1442410D-30 |
| 125 | -1.6866651D-07 | -7.6709951D-14 | -1.4644658D-19 | -1.3643906D-22 | -1.2311303D-26 | 3.0141224D-30 |
| 126 | -1.6865032D-07 | -8.2945260D-14 | -7.5211887D-20 | -5.7927517D-23 | -1.7793217D-26 | 4.3934484D-31 |
| 127 | -1.6867239D-07 | -9.1229115D-14 | -3.4554666D-19 | -6.7819035D-24 | -1.2164952D-26 | -4.8693212D-31 |
| 128 | -1.6875345D-07 | -1.0174329D-13 | -7.4346816D-19 | -3.7972476D-24 | -7.7365890D-27 | 1.1754483D-30 |
| 129 | -1.6891803D-07 | -1.1452927D-13 | -7.1040713D-19 | 3.8831367D-23 | -2.4902258D-26 | 1.6535032D-30 |
| 130 | -1.6916894D-07 | -1.2824664D-13 | -7.4145425D-19 | 2.2787486D-22 | -3.1203677D-26 | -3.9417341D-30 |
| 131 | -1.6948737D-07 | -1.3742609D-13 | -1.4337370D-18 | 3.3001163D-22 | 2.9443100D-28 | -8.5102156D-30 |
| 132 | -1.6985564D-07 | -1.4175576D-13 | -2.5271091D-18 | 2.1635734D-22 | 4.3818784D-26 | -6.8355738D-30 |
| 133 | -1.7028083D-07 | -1.4600345D-13 | -3.3896453D-18 | -4.5533492D-23 | 6.9485913D-26 | 8.1996598D-31 |
| 134 | -1.7079273D-07 | -1.5316082D-13 | -2.8645164D-18 | -2.7231014D-22 | 4.1786425D-26 | 8.4059264D-30 |
| 135 | -1.7139092D-07 | -1.6229210D-13 | -1.4820276D-18 | -2.9710188D-22 | -1.2331237D-26 | 7.8381385D-30 |
| 136 | -1.7204878D-07 | -1.7290536D-13 | -9.7126187D-19 | -1.9888085D-22 | -3.2323155D-26 | 2.4779402D-30 |
| 137 | -1.7277418D-07 | -1.8732768D-13 | -1.1856022D-18 | -4.9405910D-23 | -1.9888379D-26 | -2.2083001D-30 |

| | | | | | | |
|---|---|---|---|---|---|---|
| 138 | -1.7358799D-07 | -2.0182565D-13 | -1.2310022D-18 | 5.9828546D-24 | -2.8387324D-27 | -2.6198361D-30 |
| 139 | -1.7448214D-07 | -2.1393739D-13 | -1.3449467D-18 | -1.1281399D-22 | 2.1676325D-27 | 2.5759289D-30 |
| 140 | -1.7546382D-07 | -2.3006447D-13 | -1.2708094D-18 | -1.0320370D-22 | -1.7990835D-26 | 4.4544541D-30 |
| 141 | -1.7654842D-07 | -2.4844237D-13 | -8.9887284D-19 | 3.9283560D-23 | -4.4446761D-26 | 1.6456181D-31 |
| 142 | -1.7772523D-07 | -2.6663128D-13 | -1.5270972D-18 | 1.5486213D-22 | -3.2512986D-26 | -4.7749307D-30 |
| 143 | -1.7901173D-07 | -2.8727551D-13 | -2.4884336D-18 | 2.8883828D-22 | -6.6726324D-28 | -9.3497042D-30 |
| 144 | -1.8042173D-07 | -3.0551888D-13 | -3.3744741D-18 | 2.0108254D-22 | 3.4661670D-26 | -7.5180829D-30 |
| 145 | -1.8195975D-07 | -3.2463214D-13 | -4.3429096D-18 | 6.5739699D-24 | 6.5528056D-26 | -7.1390694D-31 |
| 146 | -1.8365249D-07 | -3.4575571D-13 | -4.0699917D-18 | -1.9204766D-22 | 4.1411800D-26 | 6.1437560D-30 |
| 147 | -1.8549846D-07 | -3.6981521D-13 | -3.8810809D-18 | -3.1608863D-22 | 1.3092499D-26 | 9.5077422D-30 |
| 148 | -1.8751856D-07 | -3.9969210D-13 | -3.4003944D-18 | -2.4379165D-22 | -2.4450866D-26 | 6.7704548D-30 |
| 149 | -1.8972196D-07 | -4.3213819D-13 | -3.3972667D-18 | -1.8237278D-22 | -4.3813549D-26 | 3.7005647D-30 |
| 150 | -1.9212957D-07 | -4.7060736D-13 | -3.8238402D-18 | 3.0434685D-23 | -4.2470255D-26 | -4.0232345D-30 |
| 151 | -1.9476378D-07 | -5.1066236D-13 | -4.7640075D-18 | 6.2845507D-23 | -1.8225950D-26 | -5.5423985D-30 |
| 152 | -1.9765333D-07 | -5.5603920D-13 | -5.9039087D-18 | 9.4974336D-23 | 8.6807905D-27 | -5.7474747D-30 |
| 153 | -2.0083293D-07 | -6.0465933D-13 | -6.8752770D-18 | -4.4359448D-23 | 1.6768869D-26 | -3.0670749D-31 |
| 154 | -2.0433883D-07 | -6.6152387D-13 | -7.8479249D-18 | -7.2150870D-23 | 1.5237118D-26 | 1.0965482D-30 |
| 155 | -2.0821633D-07 | -7.2498776D-13 | -8.8016568D-18 | -2.0139748D-22 | 3.3741417D-28 | 5.8164878D-30 |
| 156 | -2.1251870D-07 | -8.0037304D-13 | -9.8308480D-18 | -1.4713233D-22 | -2.5621132D-26 | 2.9735742D-30 |
| 157 | -2.1730811D-07 | -8.8687182D-13 | -1.1492075D-17 | -1.3259033D-22 | -3.3779700D-26 | 2.9367760D-31 |
