# Supplementary material for: Ab initio spectroscopic studies of AlF and AlCl molecules
Source: arXiv:2303.08681 source file (2023-03-15)
Supplement: Supplementary file 2 [file AlCl_singlet_pi_-_S18.pdf]

# AlCl $A^1\Pi$: Rotational parameters

Note that (v',J') & (v",J") strictly label the upper and lower levels, resp., and E(lower)=E"

but E(2)-E(1) is: (energy of State-2 level) - (energy of State-1 level)

In the following table, E is expressed in $cm^{-1}$, A in $s^{-1}$ and transition dipole moment in debye.

| dJ(J") | Band v' v" | E(lower) | E(2)-E(1) | A(Einstein) | F-C Factor | <v'j'\|M\|v"j"> |
|---|---|---|---|---|---|---|
| ------ | ------- | -------- | -------- | ----------- | ----------- | ----------- |
| R( 0) | 0 - 0 | 217.67 | -0.48 | 1.34576D-08 | 1.00000D+00 | -1.08551D+00 |
| R( 1) | 0 - 0 | 218.15 | -0.96 | 1.29195D-07 | 1.00000D+00 | -1.08553D+00 |
| R( 2) | 0 - 0 | 219.10 | -1.43 | 4.67173D-07 | 1.00000D+00 | -1.08555D+00 |
| R( 3) | 0 - 0 | 220.54 | -1.91 | 1.14840D-06 | 1.00000D+00 | -1.08559D+00 |
| R( 4) | 0 - 0 | 222.45 | -2.39 | 2.29398D-06 | 1.00000D+00 | -1.08563D+00 |
| R( 5) | 0 - 0 | 224.84 | -2.87 | 4.02505D-06 | 1.00000D+00 | -1.08568D+00 |
| R( 6) | 0 - 0 | 227.71 | -3.35 | 6.46279D-06 | 1.00000D+00 | -1.08575D+00 |
| R( 7) | 0 - 0 | 231.05 | -3.82 | 9.72838D-06 | 1.00000D+00 | -1.08582D+00 |
| R( 8) | 0 - 0 | 234.88 | -4.30 | 1.39431D-05 | 1.00000D+00 | -1.08590D+00 |
| R( 9) | 0 - 0 | 239.18 | -4.78 | 1.92281D-05 | 1.00000D+00 | -1.08600D+00 |
| R( 10) | 0 - 0 | 243.96 | -5.26 | 2.57047D-05 | 1.00000D+00 | -1.08610D+00 |
| R( 11) | 0 - 0 | 249.22 | -5.73 | 3.34942D-05 | 1.00000D+00 | -1.08621D+00 |
| R( 12) | 0 - 0 | 254.95 | -6.21 | 4.27181D-05 | 1.00000D+00 | -1.08633D+00 |
| R( 13) | 0 - 0 | 261.16 | -6.69 | 5.34977D-05 | 9.99999D-01 | -1.08647D+00 |
| R( 14) | 0 - 0 | 267.85 | -7.17 | 6.59545D-05 | 9.99999D-01 | -1.08661D+00 |
| R( 15) | 0 - 0 | 275.02 | -7.64 | 8.02099D-05 | 9.99999D-01 | -1.08676D+00 |
| R( 16) | 0 - 0 | 282.66 | -8.12 | 9.63856D-05 | 9.99999D-01 | -1.08692D+00 |
| R( 17) | 0 - 0 | 290.78 | -8.60 | 1.14603D-04 | 9.99999D-01 | -1.08709D+00 |
| R( 18) | 0 - 0 | 299.38 | -9.07 | 1.34984D-04 | 9.99999D-01 | -1.08727D+00 |

| | | | | | | | |
|---|---|---|---|---|---|---|---|
| R( 19) | 0 - 0 | 308.46 | -9.55 | 1.57651D-04 | 9.99999D-01 | -1.08746D+00 |
| P( 1) | 1 - 0 | 218.15 | -425.90 | 2.03908D-01 | 2.74664D-09 | 9.17377D-02 |
| R( 0) | 1 - 0 | 217.67 | -426.85 | 6.82533D-02 | 2.74707D-09 | 9.16222D-02 |
| P( 2) | 1 - 0 | 219.10 | -425.42 | 1.35636D-01 | 1.09870D-08 | 9.17917D-02 |
| R( 0) | 1 - 1 | 644.05 | -0.47 | 1.29777D-08 | 1.00000D+00 | 1.08569D+00 |
| R( 1) | 1 - 0 | 218.15 | -427.32 | 8.20624D-02 | 1.09892D-08 | 9.15607D-02 |
| P( 3) | 1 - 0 | 220.54 | -424.93 | 1.21787D-01 | 2.47212D-08 | 9.18431D-02 |
| R( 1) | 1 - 1 | 644.53 | -0.94 | 1.24587D-07 | 1.00000D+00 | 1.08570D+00 |
| R( 2) | 1 - 0 | 219.10 | -427.78 | 8.80852D-02 | 2.47236D-08 | 9.14966D-02 |
| P( 4) | 1 - 0 | 222.45 | -424.44 | 1.15706D-01 | 4.39570D-08 | 9.18921D-02 |
| R( 2) | 1 - 1 | 645.47 | -1.42 | 4.50508D-07 | 1.00000D+00 | 1.08572D+00 |
| R( 3) | 1 - 0 | 220.54 | -428.24 | 9.15059D-02 | 4.39565D-08 | 9.14300D-02 |
| P( 5) | 1 - 0 | 224.84 | -423.93 | 1.12207D-01 | 6.86911D-08 | 9.19385D-02 |
| R( 3) | 1 - 1 | 646.89 | -1.89 | 1.10742D-06 | 1.00000D+00 | 1.08575D+00 |
| R( 4) | 1 - 0 | 222.45 | -428.69 | 9.37383D-02 | 6.86893D-08 | 9.13609D-02 |
| P( 6) | 1 - 0 | 227.71 | -423.43 | 1.09877D-01 | 9.89296D-08 | 9.19824D-02 |
| R( 4) | 1 - 1 | 648.78 | -2.36 | 2.21209D-06 | 1.00000D+00 | 1.08579D+00 |
| R( 5) | 1 - 0 | 224.84 | -429.13 | 9.53261D-02 | 9.89256D-08 | 9.12892D-02 |
| P( 7) | 1 - 0 | 231.05 | -422.91 | 1.08172D-01 | 1.34677D-07 | 9.20238D-02 |
| R( 5) | 1 - 1 | 651.14 | -2.83 | 3.88131D-06 | 1.00000D+00 | 1.08584D+00 |
| R( 6) | 1 - 0 | 227.71 | -429.57 | 9.65230D-02 | 1.34670D-07 | 9.12149D-02 |
| P( 8) | 1 - 0 | 234.88 | -422.40 | 1.06839D-01 | 1.75939D-07 | 9.20627D-02 |
| R( 6) | 1 - 1 | 653.97 | -3.31 | 6.23187D-06 | 1.00000D+00 | 1.08590D+00 |
| R( 7) | 1 - 0 | 231.05 | -430.00 | 9.74633D-02 | 1.75927D-07 | 9.11381D-02 |
| P( 9) | 1 - 0 | 239.18 | -421.87 | 1.05742D-01 | 2.22722D-07 | 9.20991D-02 |
| R( 7) | 1 - 1 | 657.27 | -3.78 | 9.38057D-06 | 9.99999D-01 | 1.08596D+00 |
| R( 8) | 1 - 0 | 234.88 | -430.42 | 9.82247D-02 | 2.22705D-07 | 9.10587D-02 |
| P( 10) | 1 - 0 | 243.96 | -421.34 | 1.04805D-01 | 2.75032D-07 | 9.21330D-02 |
| R( 8) | 1 - 1 | 661.05 | -4.25 | 1.34442D-05 | 9.99999D-01 | 1.08604D+00 |

| | | | | | | | |
|---|---|---|---|---|---|---|---|
| R( 9) | 1 - 0 | 239.18 | -430.84 | 9.88554D-02 | 2.75008D-07 | 9.09768D-02 |
| P( 11) | 1 - 0 | 249.22 | -420.81 | 1.03980D-01 | 3.32879D-07 | 9.21644D-02 |
| R( 9) | 1 - 1 | 665.30 | -4.72 | 1.85396D-05 | 9.99999D-01 | 1.08612D+00 |
| R( 10) | 1 - 0 | 243.96 | -431.26 | 9.93866D-02 | 3.32846D-07 | 9.08923D-02 |
| P( 12) | 1 - 0 | 254.95 | -420.26 | 1.03234D-01 | 3.96270D-07 | 9.21932D-02 |
| R( 10) | 1 - 1 | 670.02 | -5.19 | 2.47836D-05 | 9.99999D-01 | 1.08621D+00 |
| R( 11) | 1 - 0 | 249.22 | -431.66 | 9.98396D-02 | 3.96227D-07 | 9.08051D-02 |
| P( 13) | 1 - 0 | 261.16 | -419.72 | 1.02547D-01 | 4.65217D-07 | 9.22196D-02 |
| R( 11) | 1 - 1 | 675.22 | -5.66 | 3.22929D-05 | 9.99999D-01 | 1.08631D+00 |
| R( 12) | 1 - 0 | 254.95 | -432.07 | 1.00229D-01 | 4.65160D-07 | 9.07154D-02 |
| P( 14) | 1 - 0 | 267.85 | -419.16 | 1.01904D-01 | 5.39728D-07 | 9.22435D-02 |
| R( 12) | 1 - 1 | 680.88 | -6.14 | 4.11844D-05 | 9.99999D-01 | 1.08642D+00 |
| R( 13) | 1 - 0 | 261.16 | -432.46 | 1.00567D-01 | 5.39657D-07 | 9.06231D-02 |
| P( 15) | 1 - 0 | 275.02 | -418.61 | 1.01294D-01 | 6.19816D-07 | 9.22648D-02 |
| R( 13) | 1 - 1 | 687.02 | -6.61 | 5.15749D-05 | 9.99998D-01 | 1.08654D+00 |
| R( 14) | 1 - 0 | 267.85 | -432.85 | 1.00860D-01 | 6.19728D-07 | 9.05282D-02 |
| P( 16) | 1 - 0 | 282.66 | -418.04 | 1.00709D-01 | 7.05492D-07 | 9.22837D-02 |
| R( 14) | 1 - 1 | 693.62 | -7.08 | 6.35811D-05 | 9.99998D-01 | 1.08667D+00 |
| R( 15) | 1 - 0 | 275.02 | -433.24 | 1.01115D-01 | 7.05385D-07 | 9.04307D-02 |
| P( 17) | 1 - 0 | 290.78 | -417.47 | 1.00143D-01 | 7.96771D-07 | 9.23000D-02 |
| R( 15) | 1 - 1 | 700.70 | -7.55 | 7.73200D-05 | 9.99998D-01 | 1.08680D+00 |
| R( 16) | 1 - 0 | 282.66 | -433.61 | 1.01336D-01 | 7.96641D-07 | 9.03305D-02 |
| P( 18) | 1 - 0 | 299.38 | -416.90 | 9.95914D-02 | 8.93667D-07 | 9.23139D-02 |
| R( 16) | 1 - 1 | 708.26 | -8.02 | 9.29083D-05 | 9.99998D-01 | 1.08695D+00 |
| R( 17) | 1 - 0 | 290.78 | -433.99 | 1.01527D-01 | 8.93512D-07 | 9.02277D-02 |
| P( 19) | 1 - 0 | 308.46 | -416.31 | 9.90504D-02 | 9.96193D-07 | 9.23252D-02 |
| R( 17) | 1 - 1 | 716.28 | -8.49 | 1.10463D-04 | 9.99997D-01 | 1.08710D+00 |
| R( 18) | 1 - 0 | 299.38 | -434.35 | 1.01691D-01 | 9.96010D-07 | 9.01222D-02 |
| P( 20) | 1 - 0 | 318.01 | -415.73 | 9.85174D-02 | 1.10437D-06 | 9.23340D-02 |

| | | | | | | | |
|---|---|---|---|---|---|---|---|
| R( 18) | 1 - 1 | 724.77 | -8.96 | 1.30100D-04 | 9.99997D-01 | 1.08726D+00 |
| R( 19) | 1 - 0 | 308.46 | -434.71 | 1.01830D-01 | 1.10415D-06 | 9.00141D-02 |
| P( 21) | 1 - 0 | 328.04 | -415.13 | 9.79900D-02 | 1.21820D-06 | 9.23403D-02 |
| R( 19) | 1 - 1 | 733.73 | -9.43 | 1.51938D-04 | 9.99997D-01 | 1.08743D+00 |
| P( 1) | 2 - 0 | 218.15 | -838.06 | 1.39932D-01 | 1.14501D-11 | 2.75325D-02 |
| P( 1) | 2 - 1 | 644.53 | -411.68 | 2.98458D-01 | 5.80279D-09 | -1.16787D-01 |
| R( 0) | 2 - 0 | 217.67 | -839.00 | 4.68205D-02 | 1.14782D-11 | 2.75380D-02 |
| P( 2) | 2 - 0 | 219.10 | -837.57 | 9.31108D-02 | 4.57439D-11 | 2.75304D-02 |
| R( 0) | 2 - 1 | 644.05 | -412.62 | 9.98760D-02 | 5.80297D-09 | -1.16617D-01 |
| P( 2) | 2 - 1 | 645.47 | -411.20 | 1.98547D-01 | 2.32118D-08 | -1.16866D-01 |
| R( 0) | 2 - 2 | 1056.21 | -0.47 | 1.23826D-08 | 1.00000D+00 | -1.08195D+00 |
| R( 1) | 2 - 0 | 218.15 | -839.46 | 5.62899D-02 | 4.59874D-11 | 2.75414D-02 |
| P( 3) | 2 - 0 | 220.54 | -837.07 | 8.36394D-02 | 1.02789D-10 | 2.75289D-02 |
| R( 1) | 2 - 1 | 644.53 | -413.08 | 1.20064D-01 | 2.32144D-08 | -1.16526D-01 |
| P( 3) | 2 - 1 | 646.89 | -410.72 | 1.78289D-01 | 5.22276D-08 | -1.16941D-01 |
| R( 1) | 2 - 2 | 1056.67 | -0.93 | 1.18874D-07 | 1.00000D+00 | -1.08196D+00 |
| R( 2) | 2 - 0 | 219.10 | -839.90 | 6.04229D-02 | 1.03548D-10 | 2.75453D-02 |
| P( 4) | 2 - 0 | 222.45 | -836.55 | 7.95034D-02 | 1.82627D-10 | 2.75277D-02 |
| R( 2) | 2 - 1 | 645.47 | -413.53 | 1.28853D-01 | 5.22289D-08 | -1.16431D-01 |
| P( 4) | 2 - 1 | 648.78 | -410.23 | 1.69396D-01 | 9.28672D-08 | -1.17012D-01 |
| R( 2) | 2 - 2 | 1057.61 | -1.40 | 4.29843D-07 | 1.00000D+00 | -1.08198D+00 |
| R( 3) | 2 - 0 | 220.54 | -840.33 | 6.27767D-02 | 1.84337D-10 | 2.75496D-02 |
| P( 5) | 2 - 0 | 224.84 | -836.03 | 7.71455D-02 | 2.85091D-10 | 2.75271D-02 |
| R( 3) | 2 - 1 | 646.89 | -413.98 | 1.33831D-01 | 9.28595D-08 | -1.16331D-01 |
| P( 5) | 2 - 1 | 651.14 | -409.73 | 1.64279D-01 | 1.45125D-07 | -1.17079D-01 |
| R( 3) | 2 - 2 | 1059.00 | -1.86 | 1.05661D-06 | 1.00000D+00 | -1.08200D+00 |
| R( 4) | 2 - 0 | 222.45 | -840.75 | 6.43216D-02 | 2.88435D-10 | 2.75544D-02 |
| P( 6) | 2 - 0 | 227.71 | -835.49 | 7.55955D-02 | 4.10174D-10 | 2.75269D-02 |
| R( 4) | 2 - 1 | 648.78 | -414.42 | 1.37066D-01 | 1.45110D-07 | -1.16228D-01 |

| | | | | | | | |
|---|---|---|---|---|---|---|---|
| P( 6) | 2 - 1 | 653.97 | -409.23 | 1.60871D-01 | 2.09014D-07 | -1.17141D-01 |
| R( 4) | 2 - 2 | 1060.87 | -2.33 | 2.11056D-06 | 1.00000D+00 | -1.08204D+00 |
| R( 5) | 2 - 0 | 224.84 | -841.15 | 6.54307D-02 | 4.15958D-10 | 2.75596D-02 |
| P( 7) | 2 - 0 | 231.05 | -834.94 | 7.44804D-02 | 5.57838D-10 | 2.75271D-02 |
| R( 5) | 2 - 1 | 651.14 | -414.86 | 1.39354D-01 | 2.08989D-07 | -1.16120D-01 |
| P( 7) | 2 - 1 | 657.27 | -408.72 | 1.58374D-01 | 2.84547D-07 | -1.17200D-01 |
| R( 5) | 2 - 2 | 1063.20 | -2.80 | 3.70310D-06 | 9.99999D-01 | -1.08208D+00 |
| R( 6) | 2 - 0 | 227.71 | -841.55 | 6.62780D-02 | 5.67029D-10 | 2.75653D-02 |
| P( 8) | 2 - 0 | 234.88 | -834.38 | 7.36260D-02 | 7.28052D-10 | 2.75279D-02 |
| R( 6) | 2 - 1 | 653.97 | -415.28 | 1.41067D-01 | 2.84506D-07 | -1.16008D-01 |
| P( 8) | 2 - 1 | 661.05 | -408.20 | 1.56418D-01 | 3.71736D-07 | -1.17254D-01 |
| R( 6) | 2 - 2 | 1065.99 | -3.26 | 5.94559D-06 | 9.99999D-01 | -1.08213D+00 |
| R( 7) | 2 - 0 | 231.05 | -841.93 | 6.69557D-02 | 7.41780D-10 | 2.75715D-02 |
| P( 9) | 2 - 0 | 239.18 | -833.80 | 7.29401D-02 | 9.20792D-10 | 2.75291D-02 |
| R( 7) | 2 - 1 | 657.27 | -415.71 | 1.42402D-01 | 3.71675D-07 | -1.15892D-01 |
| P( 9) | 2 - 1 | 665.30 | -407.68 | 1.54806D-01 | 4.70596D-07 | -1.17305D-01 |
| R( 7) | 2 - 2 | 1069.25 | -3.73 | 8.94940D-06 | 9.99999D-01 | -1.08218D+00 |
| R( 8) | 2 - 0 | 234.88 | -842.30 | 6.75172D-02 | 9.40351D-10 | 2.75781D-02 |
| P( 10) | 2 - 0 | 243.96 | -833.22 | 7.23694D-02 | 1.13604D-09 | 2.75307D-02 |
| R( 8) | 2 - 1 | 661.05 | -416.12 | 1.43471D-01 | 4.70509D-07 | -1.15772D-01 |
| P( 10) | 2 - 1 | 670.02 | -407.15 | 1.53424D-01 | 5.81145D-07 | -1.17351D-01 |
| R( 8) | 2 - 2 | 1072.98 | -4.19 | 1.28259D-05 | 9.99999D-01 | -1.08225D+00 |
| R( 9) | 2 - 0 | 239.18 | -842.65 | 6.79956D-02 | 1.16289D-09 | 2.75852D-02 |
| P( 11) | 2 - 0 | 249.22 | -832.62 | 7.18809D-02 | 1.37380D-09 | 2.75328D-02 |
| R( 9) | 2 - 1 | 665.30 | -416.53 | 1.44345D-01 | 5.81026D-07 | -1.15648D-01 |
| P( 11) | 2 - 1 | 675.22 | -406.62 | 1.52202D-01 | 7.03402D-07 | -1.17394D-01 |
| R( 9) | 2 - 2 | 1077.17 | -4.66 | 1.76863D-05 | 9.99998D-01 | -1.08232D+00 |
| R( 10) | 2 - 0 | 243.96 | -843.00 | 6.84123D-02 | 1.40955D-09 | 2.75927D-02 |
| P( 12) | 2 - 0 | 254.95 | -832.01 | 7.14528D-02 | 1.63405D-09 | 2.75354D-02 |

| | | | | | | | |
|---|---|---|---|---|---|---|---|
| R( 10) | 2 - 1 | 670.02 | -416.93 | 1.45071D-01 | 7.03243D-07 | -1.15520D-01 |
| P( 12) | 2 - 1 | 680.88 | -406.08 | 1.51095D-01 | 8.37388D-07 | -1.17432D-01 |
| R( 10) | 2 - 2 | 1081.83 | -5.12 | 2.36420D-05 | 9.99998D-01 | -1.08240D+00 |
| R( 11) | 2 - 0 | 249.22 | -843.33 | 6.87821D-02 | 1.68050D-09 | 2.76007D-02 |
| P( 13) | 2 - 0 | 261.16 | -831.38 | 7.10708D-02 | 1.91681D-09 | 2.75385D-02 |
| R( 11) | 2 - 1 | 675.22 | -417.33 | 1.45679D-01 | 8.37182D-07 | -1.15387D-01 |
| P( 13) | 2 - 1 | 687.02 | -405.53 | 1.50071D-01 | 9.83127D-07 | -1.17466D-01 |
| R( 11) | 2 - 2 | 1086.96 | -5.59 | 3.08041D-05 | 9.99998D-01 | -1.08248D+00 |
| R( 12) | 2 - 0 | 254.95 | -843.65 | 6.91152D-02 | 1.97592D-09 | 2.76091D-02 |
| P( 14) | 2 - 0 | 267.85 | -830.75 | 7.07243D-02 | 2.22210D-09 | 2.75420D-02 |
| R( 12) | 2 - 1 | 680.88 | -417.72 | 1.46192D-01 | 9.82864D-07 | -1.15250D-01 |
| P( 14) | 2 - 1 | 693.62 | -404.98 | 1.49109D-01 | 1.14064D-06 | -1.17496D-01 |
| R( 12) | 2 - 2 | 1092.55 | -6.05 | 3.92839D-05 | 9.99997D-01 | -1.08258D+00 |
| R( 13) | 2 - 0 | 261.16 | -843.96 | 6.94190D-02 | 2.29598D-09 | 2.76179D-02 |
| P( 15) | 2 - 0 | 275.02 | -830.10 | 7.04060D-02 | 2.54993D-09 | 2.75461D-02 |
| R( 13) | 2 - 1 | 687.02 | -418.10 | 1.46624D-01 | 1.14031D-06 | -1.15109D-01 |
| P( 15) | 2 - 1 | 700.70 | -404.42 | 1.48191D-01 | 1.30996D-06 | -1.17522D-01 |
| R( 13) | 2 - 2 | 1098.60 | -6.52 | 4.91925D-05 | 9.99997D-01 | -1.08268D+00 |
| R( 14) | 2 - 0 | 267.85 | -844.25 | 6.96992D-02 | 2.64087D-09 | 2.76273D-02 |
| P( 16) | 2 - 0 | 282.66 | -829.44 | 7.01103D-02 | 2.90034D-09 | 2.75505D-02 |
| R( 14) | 2 - 1 | 693.62 | -418.48 | 1.46988D-01 | 1.30956D-06 | -1.14964D-01 |
| P( 16) | 2 - 1 | 708.26 | -403.85 | 1.47308D-01 | 1.49112D-06 | -1.17544D-01 |
| R( 14) | 2 - 2 | 1105.12 | -6.99 | 6.06411D-05 | 9.99997D-01 | -1.08279D+00 |
| R( 15) | 2 - 0 | 275.02 | -844.54 | 6.99598D-02 | 3.01080D-09 | 2.76370D-02 |
| P( 17) | 2 - 0 | 290.78 | -828.77 | 6.98330D-02 | 3.27336D-09 | 2.75555D-02 |
| R( 15) | 2 - 1 | 700.70 | -418.85 | 1.47293D-01 | 1.49063D-06 | -1.14814D-01 |
| P( 17) | 2 - 1 | 716.28 | -403.28 | 1.46450D-01 | 1.68414D-06 | -1.17562D-01 |
| R( 15) | 2 - 2 | 1112.11 | -7.45 | 7.37405D-05 | 9.99996D-01 | -1.08290D+00 |
| R( 16) | 2 - 0 | 282.66 | -844.81 | 7.02042D-02 | 3.40597D-09 | 2.76472D-02 |

| | | | | | | | |
|---|---|---|---|---|---|---|---|
| P( 18) | 2 - 0 | 299.38 | -828.09 | 6.95709D-02 | 3.66904D-09 | 2.75609D-02 |
| R( 16) | 2 - 1 | 708.26 | -419.22 | 1.47546D-01 | 1.68355D-06 | -1.14660D-01 |
| P( 18) | 2 - 1 | 724.77 | -402.70 | 1.45611D-01 | 1.88907D-06 | -1.17576D-01 |
| R( 16) | 2 - 2 | 1119.56 | -7.92 | 8.86018D-05 | 9.99996D-01 | -1.08303D+00 |
| R( 17) | 2 - 0 | 290.78 | -845.07 | 7.04348D-02 | 3.82661D-09 | 2.76579D-02 |
| P( 19) | 2 - 0 | 308.46 | -827.40 | 6.93215D-02 | 4.08743D-09 | 2.75669D-02 |
| R( 17) | 2 - 1 | 716.28 | -419.57 | 1.47751D-01 | 1.88836D-06 | -1.14502D-01 |
| P( 19) | 2 - 1 | 733.73 | -402.12 | 1.44784D-01 | 2.10592D-06 | -1.17585D-01 |
| R( 17) | 2 - 2 | 1127.47 | -8.38 | 1.05336D-04 | 9.99995D-01 | -1.08316D+00 |
| R( 18) | 2 - 0 | 299.38 | -845.31 | 7.06536D-02 | 4.27294D-09 | 2.76690D-02 |
| P( 20) | 2 - 0 | 318.01 | -826.69 | 6.90827D-02 | 4.52859D-09 | 2.75732D-02 |
| R( 18) | 2 - 1 | 724.77 | -419.93 | 1.47913D-01 | 2.10510D-06 | -1.14340D-01 |
| P( 20) | 2 - 1 | 743.17 | -401.53 | 1.43967D-01 | 2.33476D-06 | -1.17591D-01 |
| R( 18) | 2 - 2 | 1135.85 | -8.84 | 1.24054D-04 | 9.99995D-01 | -1.08329D+00 |
| R( 19) | 2 - 0 | 308.46 | -845.55 | 7.08623D-02 | 4.74519D-09 | 2.76806D-02 |
| P( 21) | 2 - 0 | 328.04 | -825.97 | 6.88528D-02 | 4.99259D-09 | 2.75801D-02 |
| R( 19) | 2 - 1 | 733.73 | -420.27 | 1.48036D-01 | 2.33379D-06 | -1.14173D-01 |
| P( 21) | 2 - 1 | 753.07 | -400.93 | 1.43155D-01 | 2.57560D-06 | -1.17593D-01 |
| R( 19) | 2 - 2 | 1144.70 | -9.31 | 1.44866D-04 | 9.99994D-01 | -1.08344D+00 |
| P( 1) | 3 - 0 | 218.15 | -1235.39 | 7.34557D-03 | 1.39931D-13 | 3.52455D-03 |
| P( 1) | 3 - 1 | 644.53 | -809.02 | 3.88565D-01 | 3.84734D-11 | -4.83721D-02 |
| P( 1) | 3 - 2 | 1056.67 | -396.87 | 3.11107D-01 | 9.23979D-09 | 1.25975D-01 |
| R( 0) | 3 - 0 | 217.67 | -1236.33 | 2.46156D-03 | 1.39947D-13 | 3.52990D-03 |
| P( 2) | 3 - 0 | 219.10 | -1234.90 | 4.88461D-03 | 5.58048D-13 | 3.52220D-03 |
| R( 0) | 3 - 1 | 644.05 | -809.95 | 1.30005D-01 | 3.85703D-11 | -4.83786D-02 |
| P( 2) | 3 - 1 | 645.47 | -808.53 | 2.58555D-01 | 1.53714D-10 | -4.83700D-02 |
| R( 0) | 3 - 2 | 1056.21 | -397.79 | 1.04071D-01 | 9.23994D-09 | 1.25759D-01 |
| P( 2) | 3 - 2 | 1057.61 | -396.39 | 2.06993D-01 | 3.69605D-08 | 1.26075D-01 |
| R( 0) | 3 - 3 | 1453.54 | -0.46 | 1.16678D-08 | 1.00000D+00 | 1.07218D+00 |

| | | | | | | | |
|---|---|---|---|---|---|---|---|
| R( 1) | 3 - 0 | 218.15 | -1236.77 | 2.96206D-03 | 5.62039D-13 | 3.53290D-03 |
| P( 3) | 3 - 0 | 220.54 | -1234.38 | 4.38532D-03 | 1.25217D-12 | 3.52006D-03 |
| R( 1) | 3 - 1 | 644.53 | -810.39 | 1.56292D-01 | 1.54519D-10 | -4.83830D-02 |
| P( 3) | 3 - 1 | 646.89 | -808.03 | 2.32258D-01 | 3.45427D-10 | -4.83687D-02 |
| R( 1) | 3 - 2 | 1056.67 | -398.25 | 1.25079D-01 | 3.69635D-08 | 1.25642D-01 |
| P( 3) | 3 - 2 | 1059.00 | -395.92 | 1.85896D-01 | 8.31638D-08 | 1.26169D-01 |
| R( 1) | 3 - 3 | 1454.00 | -0.92 | 1.12011D-07 | 1.00000D+00 | 1.07219D+00 |
| R( 2) | 3 - 0 | 219.10 | -1237.19 | 3.18267D-03 | 1.26507D-12 | 3.53611D-03 |
| P( 4) | 3 - 0 | 222.45 | -1233.85 | 4.16653D-03 | 2.22536D-12 | 3.51813D-03 |
| R( 2) | 3 - 1 | 645.47 | -810.83 | 1.67761D-01 | 3.47955D-10 | -4.83881D-02 |
| P( 4) | 3 - 1 | 648.78 | -807.52 | 2.20773D-01 | 6.13703D-10 | -4.83680D-02 |
| R( 2) | 3 - 2 | 1057.61 | -398.69 | 1.34202D-01 | 8.31626D-08 | 1.25519D-01 |
| P( 4) | 3 - 2 | 1060.87 | -395.43 | 1.76641D-01 | 1.47876D-07 | 1.26257D-01 |
| R( 2) | 3 - 3 | 1454.92 | -1.38 | 4.05022D-07 | 1.00000D+00 | 1.07220D+00 |
| R( 3) | 3 - 0 | 220.54 | -1237.60 | 3.31020D-03 | 2.25394D-12 | 3.53954D-03 |
| P( 5) | 3 - 0 | 224.84 | -1233.30 | 4.04143D-03 | 3.47212D-12 | 3.51642D-03 |
| R( 3) | 3 - 1 | 646.89 | -811.25 | 1.74288D-01 | 6.19433D-10 | -4.83939D-02 |
| P( 5) | 3 - 1 | 651.14 | -807.00 | 2.14226D-01 | 9.58051D-10 | -4.83682D-02 |
| R( 3) | 3 - 2 | 1059.00 | -399.13 | 1.39348D-01 | 1.47857D-07 | 1.25390D-01 |
| P( 5) | 3 - 2 | 1063.20 | -394.94 | 1.71318D-01 | 2.31091D-07 | 1.26340D-01 |
| R( 3) | 3 - 3 | 1456.30 | -1.84 | 9.95583D-07 | 1.00000D+00 | 1.07222D+00 |
| R( 4) | 3 - 0 | 222.45 | -1237.98 | 3.39558D-03 | 3.52957D-12 | 3.54319D-03 |
| P( 6) | 3 - 0 | 227.71 | -1232.73 | 3.95908D-03 | 4.99325D-12 | 3.51493D-03 |
| R( 4) | 3 - 1 | 648.78 | -811.66 | 1.78567D-01 | 9.69244D-10 | -4.84005D-02 |
| P( 6) | 3 - 1 | 653.97 | -806.47 | 2.09920D-01 | 1.37844D-09 | -4.83691D-02 |
| R( 4) | 3 - 2 | 1060.87 | -399.57 | 1.42674D-01 | 2.31054D-07 | 1.25256D-01 |
| P( 6) | 3 - 2 | 1065.99 | -394.44 | 1.67772D-01 | 3.32830D-07 | 1.26417D-01 |
| R( 4) | 3 - 3 | 1458.14 | -2.30 | 1.98862D-06 | 9.99999D-01 | 1.07225D+00 |
| R( 5) | 3 - 0 | 224.84 | -1238.35 | 3.45841D-03 | 5.09408D-12 | 3.54705D-03 |

| | | | | | | |
|---|---|---|---|---|---|---|
| P( 7) | 3 - 0 | 231.05 | -1232.14 | 3.89988D-03 | 6.78810D-12 | 3.51365D-03 |
| R( 5) | 3 - 1 | 651.14 | -812.06 | 1.81635D-01 | 1.39779D-09 | -4.84078D-02 |
| P( 7) | 3 - 1 | 657.27 | -805.92 | 2.06821D-01 | 1.87474D-09 | -4.83707D-02 |
| R( 5) | 3 - 2 | 1063.20 | -400.00 | 1.45009D-01 | 3.32766D-07 | 1.25115D-01 |
| P( 7) | 3 - 2 | 1069.25 | -393.94 | 1.65172D-01 | 4.53112D-07 | 1.26488D-01 |
| R( 5) | 3 - 3 | 1460.43 | -2.76 | 3.48906D-06 | 9.99999D-01 | 1.07228D+00 |
| R( 6) | 3 - 0 | 227.71 | -1238.70 | 3.50784D-03 | 6.94976D-12 | 3.55113D-03 |
| P( 8) | 3 - 0 | 234.88 | -1231.53 | 3.85469D-03 | 8.85617D-12 | 3.51258D-03 |
| R( 6) | 3 - 1 | 653.97 | -812.44 | 1.83975D-01 | 1.90548D-09 | -4.84159D-02 |
| P( 8) | 3 - 1 | 661.05 | -805.36 | 2.04444D-01 | 2.44688D-09 | -4.83732D-02 |
| R( 6) | 3 - 2 | 1065.99 | -400.42 | 1.46741D-01 | 4.53011D-07 | 1.24969D-01 |
| P( 8) | 3 - 2 | 1072.98 | -393.43 | 1.63132D-01 | 5.91959D-07 | 1.26553D-01 |
| R( 6) | 3 - 3 | 1463.19 | -3.22 | 5.60177D-06 | 9.99999D-01 | 1.07232D+00 |
| R( 7) | 3 - 0 | 231.05 | -1239.03 | 3.54872D-03 | 9.09905D-12 | 3.55542D-03 |
| P( 9) | 3 - 0 | 239.18 | -1230.91 | 3.81867D-03 | 1.11971D-11 | 3.51173D-03 |
| R( 7) | 3 - 1 | 657.27 | -812.81 | 1.85843D-01 | 2.49278D-09 | -4.84247D-02 |
| P( 9) | 3 - 1 | 665.30 | -804.78 | 2.02535D-01 | 3.09479D-09 | -4.83763D-02 |
| R( 7) | 3 - 2 | 1069.25 | -400.83 | 1.48073D-01 | 5.91808D-07 | 1.24817D-01 |
| P( 9) | 3 - 2 | 1077.17 | -392.91 | 1.61447D-01 | 7.49398D-07 | 1.26612D-01 |
| R( 7) | 3 - 3 | 1466.41 | -3.68 | 8.43161D-06 | 9.99999D-01 | 1.07236D+00 |
| R( 8) | 3 - 0 | 234.88 | -1239.34 | 3.58384D-03 | 1.15445D-11 | 3.55993D-03 |
| P( 10) | 3 - 0 | 243.96 | -1230.26 | 3.78902D-03 | 1.38107D-11 | 3.51110D-03 |
| R( 8) | 3 - 1 | 661.05 | -813.17 | 1.87386D-01 | 3.16017D-09 | -4.84342D-02 |
| P( 10) | 3 - 1 | 670.02 | -804.20 | 2.00944D-01 | 3.81842D-09 | -4.83803D-02 |
| R( 8) | 3 - 2 | 1072.98 | -401.24 | 1.49126D-01 | 7.49182D-07 | 1.24660D-01 |
| P( 10) | 3 - 2 | 1081.83 | -392.39 | 1.59998D-01 | 9.25455D-07 | 1.26666D-01 |
| R( 8) | 3 - 3 | 1470.09 | -4.14 | 1.20833D-05 | 9.99998D-01 | 1.07241D+00 |
| R( 9) | 3 - 0 | 239.18 | -1239.64 | 3.61494D-03 | 1.42890D-11 | 3.56466D-03 |
| P( 11) | 3 - 0 | 249.22 | -1229.60 | 3.76399D-03 | 1.66968D-11 | 3.51068D-03 |

| | | | | | | | |
|---|---|---|---|---|---|---|---|
| R( 9) | 3 - 1 | 665.30 | -813.51 | 1.88698D-01 | 3.90817D-09 | -4.84445D-02 |
| P( 11) | 3 - 1 | 675.22 | -803.60 | 1.99580D-01 | 4.61778D-09 | -4.83850D-02 |
| R( 9) | 3 - 2 | 1077.17 | -401.64 | 1.49971D-01 | 9.25160D-07 | 1.24496D-01 |
| P( 11) | 3 - 2 | 1086.96 | -391.86 | 1.58713D-01 | 1.12016D-06 | 1.26714D-01 |
| R( 9) | 3 - 3 | 1474.22 | -4.59 | 1.66617D-05 | 9.99998D-01 | 1.07246D+00 |
| R( 10) | 3 - 0 | 243.96 | -1239.91 | 3.64317D-03 | 1.73354D-11 | 3.56961D-03 |
| P( 12) | 3 - 0 | 254.95 | -1228.92 | 3.74245D-03 | 1.98556D-11 | 3.51047D-03 |
| R( 10) | 3 - 1 | 670.02 | -813.85 | 1.89837D-01 | 4.73730D-09 | -4.84555D-02 |
| P( 12) | 3 - 1 | 680.88 | -802.99 | 1.98383D-01 | 5.49288D-09 | -4.83905D-02 |
| R( 10) | 3 - 2 | 1081.83 | -402.04 | 1.50657D-01 | 1.11977D-06 | 1.24326D-01 |
| P( 12) | 3 - 2 | 1092.55 | -391.32 | 1.57543D-01 | 1.33356D-06 | 1.26756D-01 |
| R( 10) | 3 - 3 | 1478.82 | -5.05 | 2.22713D-05 | 9.99997D-01 | 1.07252D+00 |
| R( 11) | 3 - 0 | 249.22 | -1240.17 | 3.66928D-03 | 2.06868D-11 | 3.57478D-03 |
| P( 13) | 3 - 0 | 261.16 | -1228.22 | 3.72364D-03 | 2.32872D-11 | 3.51048D-03 |
| R( 11) | 3 - 1 | 675.22 | -814.17 | 1.90845D-01 | 5.64815D-09 | -4.84672D-02 |
| P( 13) | 3 - 1 | 687.02 | -802.37 | 1.97312D-01 | 6.44376D-09 | -4.83967D-02 |
| R( 11) | 3 - 2 | 1086.96 | -402.43 | 1.51216D-01 | 1.33305D-06 | 1.24151D-01 |
| P( 13) | 3 - 2 | 1098.60 | -390.78 | 1.56456D-01 | 1.56568D-06 | 1.26793D-01 |
| R( 11) | 3 - 3 | 1483.87 | -5.51 | 2.90168D-05 | 9.99997D-01 | 1.07258D+00 |
| R( 12) | 3 - 0 | 254.95 | -1240.40 | 3.69383D-03 | 2.43464D-11 | 3.58016D-03 |
| P( 14) | 3 - 0 | 267.85 | -1227.50 | 3.70701D-03 | 2.69921D-11 | 3.51071D-03 |
| R( 12) | 3 - 1 | 680.88 | -814.47 | 1.91749D-01 | 6.64132D-09 | -4.84797D-02 |
| P( 14) | 3 - 1 | 693.62 | -801.73 | 1.96339D-01 | 7.47050D-09 | -4.84037D-02 |
| R( 12) | 3 - 2 | 1092.55 | -402.81 | 1.51671D-01 | 1.56503D-06 | 1.23969D-01 |
| P( 14) | 3 - 2 | 1105.12 | -390.23 | 1.55430D-01 | 1.81657D-06 | 1.26823D-01 |
| R( 12) | 3 - 3 | 1489.38 | -5.97 | 3.70025D-05 | 9.99996D-01 | 1.07265D+00 |
| R( 13) | 3 - 0 | 261.16 | -1240.62 | 3.71720D-03 | 2.83178D-11 | 3.58577D-03 |
| P( 15) | 3 - 0 | 275.02 | -1226.77 | 3.69216D-03 | 3.09706D-11 | 3.51116D-03 |
| R( 13) | 3 - 1 | 687.02 | -814.77 | 1.92571D-01 | 7.71744D-09 | -4.84929D-02 |

| | | | | | | | |
|---|---|---|---|---|---|---|---|
| P( 15) | 3 - 1 | 700.70 | -801.08 | 1.95443D-01 | 8.57320D-09 | -4.84115D-02 |
| R( 13) | 3 - 2 | 1098.60 | -403.18 | 1.52039D-01 | 1.81576D-06 | 1.23782D-01 |
| P( 15) | 3 - 2 | 1112.11 | -389.68 | 1.54448D-01 | 2.08627D-06 | 1.26848D-01 |
| R( 13) | 3 - 3 | 1495.35 | -6.43 | 4.63329D-05 | 9.99996D-01 | 1.07273D+00 |
| R( 14) | 3 - 0 | 267.85 | -1240.82 | 3.73969D-03 | 3.26044D-11 | 3.59160D-03 |
| P( 16) | 3 - 0 | 282.66 | -1226.01 | 3.67882D-03 | 3.52234D-11 | 3.51182D-03 |
| R( 14) | 3 - 1 | 693.62 | -815.05 | 1.93325D-01 | 8.87718D-09 | -4.85068D-02 |
| P( 16) | 3 - 1 | 708.26 | -800.42 | 1.94609D-01 | 9.75198D-09 | -4.84200D-02 |
| R( 14) | 3 - 2 | 1105.12 | -403.55 | 1.52332D-01 | 2.08527D-06 | 1.23589D-01 |
| P( 16) | 3 - 2 | 1119.56 | -389.12 | 1.53498D-01 | 2.37484D-06 | 1.26867D-01 |
| R( 14) | 3 - 3 | 1501.78 | -6.89 | 5.71122D-05 | 9.99995D-01 | 1.07281D+00 |
| R( 15) | 3 - 0 | 275.02 | -1241.00 | 3.76153D-03 | 3.72102D-11 | 3.59765D-03 |
| P( 17) | 3 - 0 | 290.78 | -1225.24 | 3.66674D-03 | 3.97514D-11 | 3.51270D-03 |
| R( 15) | 3 - 1 | 700.70 | -815.32 | 1.94025D-01 | 1.01212D-08 | -4.85214D-02 |
| P( 17) | 3 - 1 | 716.28 | -799.75 | 1.93825D-01 | 1.10070D-08 | -4.84294D-02 |
| R( 15) | 3 - 2 | 1112.11 | -403.92 | 1.52558D-01 | 2.37362D-06 | 1.23389D-01 |
| P( 17) | 3 - 2 | 1127.47 | -388.55 | 1.52571D-01 | 2.68232D-06 | 1.26881D-01 |
| R( 15) | 3 - 3 | 1508.67 | -7.35 | 6.94446D-05 | 9.99994D-01 | 1.07289D+00 |
| R( 16) | 3 - 0 | 282.66 | -1241.17 | 3.78289D-03 | 4.21391D-11 | 3.60392D-03 |
| P( 18) | 3 - 0 | 299.38 | -1224.45 | 3.65578D-03 | 4.45554D-11 | 3.51380D-03 |
| R( 16) | 3 - 1 | 708.26 | -815.57 | 1.94677D-01 | 1.14503D-08 | -4.85368D-02 |
| P( 18) | 3 - 1 | 724.77 | -799.06 | 1.93082D-01 | 1.23384D-08 | -4.84395D-02 |
| R( 16) | 3 - 2 | 1119.56 | -404.27 | 1.52726D-01 | 2.68086D-06 | 1.23184D-01 |
| P( 18) | 3 - 2 | 1135.85 | -387.98 | 1.51659D-01 | 3.00877D-06 | 1.26889D-01 |
| R( 16) | 3 - 3 | 1516.02 | -7.81 | 8.34341D-05 | 9.99994D-01 | 1.07298D+00 |
| R( 17) | 3 - 0 | 290.78 | -1241.31 | 3.80390D-03 | 4.73953D-11 | 3.61042D-03 |
| P( 19) | 3 - 0 | 308.46 | -1223.64 | 3.64578D-03 | 4.96366D-11 | 3.51511D-03 |
| R( 17) | 3 - 1 | 716.28 | -815.82 | 1.95290D-01 | 1.28652D-08 | -4.85529D-02 |
| P( 19) | 3 - 1 | 733.73 | -798.36 | 1.92373D-01 | 1.37465D-08 | -4.84504D-02 |

| | | | | | | | |
|---|---|---|---|---|---|---|---|
| R( 17) | 3 - 2 | 1127.47 | -404.62 | 1.52841D-01 | 3.00703D-06 | 1.22973D-01 |
| P( 19) | 3 - 2 | 1144.70 | -387.40 | 1.50758D-01 | 3.35425D-06 | 1.26890D-01 |
| R( 17) | 3 - 3 | 1523.83 | -8.26 | 9.91845D-05 | 9.99993D-01 | 1.07308D+00 |
| R( 18) | 3 - 0 | 299.38 | -1241.43 | 3.82467D-03 | 5.29832D-11 | 3.61714D-03 |
| P( 20) | 3 - 0 | 318.01 | -1222.81 | 3.63665D-03 | 5.49961D-11 | 3.51665D-03 |
| R( 18) | 3 - 1 | 724.77 | -816.05 | 1.95869D-01 | 1.43668D-08 | -4.85697D-02 |
| P( 20) | 3 - 1 | 743.17 | -797.65 | 1.91692D-01 | 1.52315D-08 | -4.84621D-02 |
| R( 18) | 3 - 2 | 1135.85 | -404.96 | 1.52906D-01 | 3.35221D-06 | 1.22756D-01 |
| P( 20) | 3 - 2 | 1154.01 | -386.81 | 1.49863D-01 | 3.71882D-06 | 1.26886D-01 |
| R( 18) | 3 - 3 | 1532.09 | -8.72 | 1.16800D-04 | 9.99992D-01 | 1.07318D+00 |
| R( 19) | 3 - 0 | 308.46 | -1241.54 | 3.84529D-03 | 5.89072D-11 | 3.62409D-03 |
| P( 21) | 3 - 0 | 328.04 | -1221.96 | 3.62829D-03 | 6.06354D-11 | 3.51841D-03 |
| R( 19) | 3 - 1 | 733.73 | -816.26 | 1.96419D-01 | 1.59557D-08 | -4.85872D-02 |
| P( 21) | 3 - 1 | 753.07 | -796.92 | 1.91035D-01 | 1.67935D-08 | -4.84745D-02 |
| R( 19) | 3 - 2 | 1144.70 | -405.30 | 1.52926D-01 | 3.71644D-06 | 1.22532D-01 |
| P( 21) | 3 - 2 | 1163.78 | -386.22 | 1.48971D-01 | 4.10255D-06 | 1.26877D-01 |
| R( 19) | 3 - 3 | 1540.82 | -9.18 | 1.36383D-04 | 9.99991D-01 | 1.07329D+00 |
| P( 1) | 4 - 0 | 218.15 | -1619.44 | 7.36930D-05 | 3.00679D-15 | 2.35214D-04 |
| P( 1) | 4 - 1 | 644.53 | -1193.06 | 3.22589D-02 | 6.49070D-13 | -7.78266D-03 |
| P( 1) | 4 - 2 | 1056.67 | -780.92 | 7.09796D-01 | 8.33806D-11 | 6.89381D-02 |
| P( 1) | 4 - 3 | 1454.00 | -383.59 | 2.71386D-01 | 1.29646D-08 | -1.23821D-01 |
| R( 0) | 4 - 0 | 217.67 | -1620.37 | 2.48799D-05 | 3.03072D-15 | 2.36516D-04 |
| P( 2) | 4 - 0 | 219.10 | -1618.94 | 4.88364D-05 | 1.19950D-14 | 2.34623D-04 |
| R( 0) | 4 - 1 | 644.05 | -1193.99 | 1.08079D-02 | 6.51710D-13 | -7.79342D-03 |
| P( 2) | 4 - 1 | 645.47 | -1192.57 | 2.14532D-02 | 2.59139D-12 | -7.77790D-03 |
| R( 0) | 4 - 2 | 1056.21 | -781.84 | 2.37467D-01 | 8.35909D-11 | 6.89428D-02 |
| P( 2) | 4 - 2 | 1057.61 | -780.44 | 4.72316D-01 | 3.33130D-10 | 6.89372D-02 |
| R( 0) | 4 - 3 | 1453.54 | -384.50 | 9.07298D-02 | 1.29646D-08 | -1.23562D-01 |
| P( 2) | 4 - 3 | 1454.92 | -383.12 | 1.80607D-01 | 5.18605D-08 | -1.23938D-01 |

| | | | | | | | |
|---|---|---|---|---|---|---|---|
| R( 0) | 4 - 4 | 1837.59 | -0.45 | 1.08253D-08 | 1.00000D+00 | -1.05459D+00 |
| R( 1) | 4 - 0 | 218.15 | -1620.80 | 3.00594D-05 | 1.21872D-14 | 2.37227D-04 |
| P( 3) | 4 - 0 | 220.54 | -1618.41 | 4.37035D-05 | 2.68720D-14 | 2.34071D-04 |
| R( 1) | 4 - 1 | 644.53 | -1194.42 | 1.30036D-02 | 2.61414D-12 | -7.79943D-03 |
| P( 3) | 4 - 1 | 646.89 | -1192.06 | 1.92616D-02 | 5.81776D-12 | -7.77356D-03 |
| R( 1) | 4 - 2 | 1056.67 | -782.28 | 2.85474D-01 | 3.34871D-10 | 6.89466D-02 |
| P( 3) | 4 - 2 | 1059.00 | -779.95 | 4.24283D-01 | 7.48613D-10 | 6.89373D-02 |
| R( 1) | 4 - 3 | 1454.00 | -384.95 | 1.09007D-01 | 5.18634D-08 | -1.23422D-01 |
| P( 3) | 4 - 3 | 1456.30 | -382.65 | 1.62232D-01 | 1.16691D-07 | -1.24048D-01 |
| R( 1) | 4 - 4 | 1838.04 | -0.91 | 1.03922D-07 | 1.00000D+00 | -1.05459D+00 |
| R( 2) | 4 - 0 | 219.10 | -1621.20 | 3.24349D-05 | 2.73273D-14 | 2.37978D-04 |
| P( 4) | 4 - 0 | 222.45 | -1617.86 | 4.13980D-05 | 4.78776D-14 | 2.33559D-04 |
| R( 2) | 4 - 1 | 645.47 | -1194.84 | 1.39700D-02 | 5.88408D-12 | -7.80586D-03 |
| P( 4) | 4 - 1 | 648.78 | -1191.53 | 1.83014D-02 | 1.03393D-11 | -7.76964D-03 |
| R( 2) | 4 - 2 | 1057.61 | -782.70 | 3.06410D-01 | 7.54112D-10 | 6.89513D-02 |
| P( 4) | 4 - 2 | 1060.87 | -779.44 | 4.03309D-01 | 1.32995D-09 | 6.89384D-02 |
| R( 2) | 4 - 3 | 1454.92 | -385.39 | 1.16913D-01 | 1.16685D-07 | -1.23273D-01 |
| P( 4) | 4 - 3 | 1458.14 | -382.17 | 1.54181D-01 | 2.07492D-07 | -1.24149D-01 |
| R( 2) | 4 - 4 | 1838.95 | -1.36 | 3.75767D-07 | 1.00000D+00 | -1.05460D+00 |
| R( 3) | 4 - 0 | 220.54 | -1621.58 | 3.38839D-05 | 4.87002D-14 | 2.38769D-04 |
| P( 5) | 4 - 0 | 224.84 | -1617.28 | 4.00425D-05 | 7.46952D-14 | 2.33086D-04 |
| R( 3) | 4 - 1 | 646.89 | -1195.24 | 1.45272D-02 | 1.04820D-11 | -7.81271D-03 |
| P( 5) | 4 - 1 | 651.14 | -1190.99 | 1.77525D-02 | 1.61344D-11 | -7.76613D-03 |
| R( 3) | 4 - 2 | 1059.00 | -783.12 | 3.18317D-01 | 1.34247D-09 | 6.89571D-02 |
| P( 5) | 4 - 2 | 1063.20 | -778.92 | 3.91350D-01 | 2.07612D-09 | 6.89405D-02 |
| R( 3) | 4 - 3 | 1456.30 | -385.82 | 1.21344D-01 | 2.07456D-07 | -1.23117D-01 |
| P( 5) | 4 - 3 | 1460.43 | -381.69 | 1.49554D-01 | 3.24257D-07 | -1.24243D-01 |
| R( 3) | 4 - 4 | 1840.31 | -1.81 | 9.23651D-07 | 1.00000D+00 | -1.05461D+00 |
| R( 4) | 4 - 0 | 222.45 | -1621.94 | 3.49186D-05 | 7.62902D-14 | 2.39600D-04 |

| | | | | | | |
|---|---|---|---|---|---|---|
| P( 6) | 4 - 0 | 227.71 | -1616.68 | 3.91247D-05 | 1.07409D-13 | 2.32653D-04 |
| R( 4) | 4 - 1 | 648.78 | -1195.61 | 1.48991D-02 | 1.64134D-11 | -7.81997D-03 |
| P( 6) | 4 - 1 | 653.97 | -1190.42 | 1.73910D-02 | 2.32059D-11 | -7.76304D-03 |
| R( 4) | 4 - 2 | 1060.87 | -783.52 | 3.26117D-01 | 2.10058D-09 | 6.89638D-02 |
| P( 6) | 4 - 2 | 1065.99 | -778.40 | 3.83486D-01 | 2.98700D-09 | 6.89436D-02 |
| R( 4) | 4 - 3 | 1458.14 | -386.25 | 1.24183D-01 | 3.24185D-07 | -1.22952D-01 |
| P( 6) | 4 - 3 | 1463.19 | -381.20 | 1.46472D-01 | 4.67015D-07 | -1.24330D-01 |
| R( 4) | 4 - 4 | 1842.12 | -2.27 | 1.84489D-06 | 9.99999D-01 | -1.05463D+00 |
| R( 5) | 4 - 0 | 224.84 | -1622.27 | 3.57361D-05 | 1.10155D-13 | 2.40472D-04 |
| P( 7) | 4 - 0 | 231.05 | -1616.05 | 3.84478D-05 | 1.46005D-13 | 2.32260D-04 |
| R( 5) | 4 - 1 | 651.14 | -1195.97 | 1.51717D-02 | 2.36882D-11 | -7.82765D-03 |
| P( 7) | 4 - 1 | 657.27 | -1189.83 | 1.71308D-02 | 3.15514D-11 | -7.76037D-03 |
| R( 5) | 4 - 2 | 1063.20 | -783.91 | 3.31702D-01 | 3.02928D-09 | 6.89715D-02 |
| P( 7) | 4 - 2 | 1069.25 | -777.85 | 3.77824D-01 | 4.06231D-09 | 6.89477D-02 |
| R( 5) | 4 - 3 | 1460.43 | -386.67 | 1.26153D-01 | 4.66891D-07 | -1.22780D-01 |
| P( 7) | 4 - 3 | 1466.41 | -380.70 | 1.44210D-01 | 6.35794D-07 | -1.24408D-01 |
| R( 5) | 4 - 4 | 1844.39 | -2.72 | 3.23678D-06 | 9.99999D-01 | -1.05465D+00 |
| R( 6) | 4 - 0 | 227.71 | -1622.57 | 3.64285D-05 | 1.50358D-13 | 2.41385D-04 |
| P( 8) | 4 - 0 | 234.88 | -1615.40 | 3.79197D-05 | 1.90474D-13 | 2.31906D-04 |
| R( 6) | 4 - 1 | 653.97 | -1196.31 | 1.53851D-02 | 3.23177D-11 | -7.83575D-03 |
| P( 8) | 4 - 1 | 661.05 | -1189.23 | 1.69320D-02 | 4.11689D-11 | -7.75811D-03 |
| R( 6) | 4 - 2 | 1065.99 | -784.29 | 3.35955D-01 | 4.12947D-09 | 6.89801D-02 |
| P( 8) | 4 - 2 | 1072.98 | -777.30 | 3.73480D-01 | 5.30182D-09 | 6.89528D-02 |
| R( 6) | 4 - 3 | 1463.19 | -387.09 | 1.27591D-01 | 6.35597D-07 | -1.22600D-01 |
| P( 8) | 4 - 3 | 1470.09 | -380.19 | 1.42432D-01 | 8.30625D-07 | -1.24479D-01 |
| R( 6) | 4 - 4 | 1847.11 | -3.17 | 5.19653D-06 | 9.99999D-01 | -1.05467D+00 |
| R( 7) | 4 - 0 | 231.05 | -1622.85 | 3.70447D-05 | 1.96966D-13 | 2.42339D-04 |
| P( 9) | 4 - 0 | 239.18 | -1614.72 | 3.74918D-05 | 2.40809D-13 | 2.31592D-04 |
| R( 7) | 4 - 1 | 657.27 | -1196.63 | 1.55607D-02 | 4.23137D-11 | -7.84427D-03 |

| | | | | | | | |
|---|---|---|---|---|---|---|---|
| P( 9) | 4 - 1 | 665.30 | -1188.60 | 1.67730D-02 | 5.20576D-11 | -7.75627D-03 |
| R( 7) | 4 - 2 | 1069.25 | -784.65 | 3.39344D-01 | 5.40210D-09 | 6.89897D-02 |
| P( 9) | 4 - 2 | 1077.17 | -776.73 | 3.69987D-01 | 6.70535D-09 | 6.89589D-02 |
| R( 7) | 4 - 3 | 1466.41 | -387.50 | 1.28675D-01 | 8.30331D-07 | -1.22413D-01 |
| P( 9) | 4 - 3 | 1474.22 | -379.68 | 1.40959D-01 | 1.05154D-06 | -1.24542D-01 |
| R( 7) | 4 - 4 | 1850.28 | -3.63 | 7.82131D-06 | 9.99998D-01 | -1.05469D+00 |
| R( 8) | 4 - 0 | 234.88 | -1623.10 | 3.76131D-05 | 2.50051D-13 | 2.43335D-04 |
| P( 10) | 4 - 0 | 243.96 | -1614.02 | 3.71359D-05 | 2.97009D-13 | 2.31317D-04 |
| R( 8) | 4 - 1 | 661.05 | -1196.93 | 1.57106D-02 | 5.36888D-11 | -7.85322D-03 |
| P( 10) | 4 - 1 | 670.02 | -1187.96 | 1.66418D-02 | 6.42170D-11 | -7.75484D-03 |
| R( 8) | 4 - 2 | 1072.98 | -785.00 | 3.42140D-01 | 6.84820D-09 | 6.90003D-02 |
| P( 10) | 4 - 2 | 1081.83 | -776.15 | 3.67075D-01 | 8.27277D-09 | 6.89660D-02 |
| R( 8) | 4 - 3 | 1470.09 | -387.90 | 1.29510D-01 | 1.05113D-06 | -1.22217D-01 |
| P( 10) | 4 - 3 | 1478.82 | -379.17 | 1.39687D-01 | 1.29859D-06 | -1.24597D-01 |
| R( 8) | 4 - 4 | 1853.90 | -4.08 | 1.12082D-05 | 9.99998D-01 | -1.05472D+00 |
| R( 9) | 4 - 0 | 239.18 | -1623.33 | 3.81513D-05 | 3.09690D-13 | 2.44372D-04 |
| P( 11) | 4 - 0 | 249.22 | -1613.30 | 3.68344D-05 | 3.59076D-13 | 2.31083D-04 |
| R( 9) | 4 - 1 | 665.30 | -1197.21 | 1.58426D-02 | 6.64565D-11 | -7.86258D-03 |
| P( 11) | 4 - 1 | 675.22 | -1187.30 | 1.65306D-02 | 7.76477D-11 | -7.75383D-03 |
| R( 9) | 4 - 2 | 1077.17 | -785.34 | 3.44510D-01 | 8.46883D-09 | 6.90118D-02 |
| P( 11) | 4 - 2 | 1086.96 | -775.56 | 3.64576D-01 | 1.00040D-08 | 6.89741D-02 |
| R( 9) | 4 - 3 | 1474.22 | -388.29 | 1.30159D-01 | 1.29802D-06 | -1.22013D-01 |
| P( 11) | 4 - 3 | 1483.87 | -378.64 | 1.38552D-01 | 1.57181D-06 | -1.24644D-01 |
| R( 9) | 4 - 4 | 1857.98 | -4.53 | 1.54540D-05 | 9.99997D-01 | -1.05475D+00 |
| R( 10) | 4 - 0 | 243.96 | -1623.54 | 3.86711D-05 | 3.75966D-13 | 2.45452D-04 |
| P( 12) | 4 - 0 | 254.95 | -1612.55 | 3.65759D-05 | 4.27018D-13 | 2.30888D-04 |
| R( 10) | 4 - 1 | 670.02 | -1197.47 | 1.59616D-02 | 8.06313D-11 | -7.87236D-03 |
| P( 12) | 4 - 1 | 680.88 | -1186.62 | 1.64344D-02 | 9.23507D-11 | -7.75324D-03 |
| R( 10) | 4 - 2 | 1081.83 | -785.66 | 3.46563D-01 | 1.02651D-08 | 6.90243D-02 |

| | | | | | | | |
|---|---|---|---|---|---|---|---|
| P( 12) | 4 - 2 | 1092.55 | -774.95 | 3.62380D-01 | 1.18991D-08 | 6.89832D-02 |
| R( 10) | 4 - 3 | 1478.82 | -388.68 | 1.30664D-01 | 1.57105D-06 | -1.21801D-01 |
| P( 12) | 4 - 3 | 1489.38 | -378.11 | 1.37514D-01 | 1.87126D-06 | -1.24684D-01 |
| R( 10) | 4 - 4 | 1862.51 | -4.98 | 2.06558D-05 | 9.99996D-01 | -1.05478D+00 |
| R( 11) | 4 - 0 | 249.22 | -1623.72 | 3.91803D-05 | 4.48966D-13 | 2.46573D-04 |
| P( 13) | 4 - 0 | 261.16 | -1611.77 | 3.63528D-05 | 5.00846D-13 | 2.30734D-04 |
| R( 11) | 4 - 1 | 675.22 | -1197.72 | 1.60710D-02 | 9.62283D-11 | -7.88256D-03 |
| P( 13) | 4 - 1 | 687.02 | -1185.92 | 1.63499D-02 | 1.08328D-10 | -7.75306D-03 |
| R( 11) | 4 - 2 | 1086.96 | -785.98 | 3.48373D-01 | 1.22383D-08 | 6.90377D-02 |
| P( 13) | 4 - 2 | 1098.60 | -774.33 | 3.60414D-01 | 1.39580D-08 | 6.89933D-02 |
| R( 11) | 4 - 3 | 1483.87 | -389.06 | 1.31052D-01 | 1.87027D-06 | -1.21582D-01 |
| P( 13) | 4 - 3 | 1495.35 | -377.58 | 1.36544D-01 | 2.19698D-06 | -1.24716D-01 |
| R( 11) | 4 - 4 | 1867.50 | -5.44 | 2.69101D-05 | 9.99996D-01 | -1.05482D+00 |
| R( 12) | 4 - 0 | 254.95 | -1623.87 | 3.96847D-05 | 5.28780D-13 | 2.47738D-04 |
| P( 14) | 4 - 0 | 267.85 | -1610.97 | 3.61595D-05 | 5.80557D-13 | 2.30620D-04 |
| R( 12) | 4 - 1 | 680.88 | -1197.94 | 1.61731D-02 | 1.13264D-10 | -7.89319D-03 |
| P( 14) | 4 - 1 | 693.62 | -1185.20 | 1.62746D-02 | 1.25583D-10 | -7.75330D-03 |
| R( 12) | 4 - 2 | 1092.55 | -786.28 | 3.49994D-01 | 1.43896D-08 | 6.90521D-02 |
| P( 14) | 4 - 2 | 1105.12 | -773.70 | 3.58624D-01 | 1.61808D-08 | 6.90045D-02 |
| R( 12) | 4 - 3 | 1489.38 | -389.44 | 1.31345D-01 | 2.19572D-06 | -1.21354D-01 |
| P( 14) | 4 - 3 | 1501.78 | -377.04 | 1.35621D-01 | 2.54905D-06 | -1.24739D-01 |
| R( 12) | 4 - 4 | 1872.93 | -5.89 | 3.43135D-05 | 9.99995D-01 | -1.05486D+00 |
| R( 13) | 4 - 0 | 261.16 | -1624.00 | 4.01885D-05 | 6.15508D-13 | 2.48946D-04 |
| P( 15) | 4 - 0 | 275.02 | -1610.14 | 3.59922D-05 | 6.66203D-13 | 2.30547D-04 |
| R( 13) | 4 - 1 | 687.02 | -1198.15 | 1.62698D-02 | 1.31755D-10 | -7.90424D-03 |
| P( 15) | 4 - 1 | 700.70 | -1184.46 | 1.62070D-02 | 1.44118D-10 | -7.75395D-03 |
| R( 13) | 4 - 2 | 1098.60 | -786.56 | 3.51461D-01 | 1.67203D-08 | 6.90674D-02 |
| P( 15) | 4 - 2 | 1112.11 | -773.06 | 3.56974D-01 | 1.85678D-08 | 6.90166D-02 |
| R( 13) | 4 - 3 | 1495.35 | -389.81 | 1.31556D-01 | 2.54747D-06 | -1.21119D-01 |

| | | | | | | | |
|---|---|---|---|---|---|---|---|
| P( 15) | 4 - 3 | 1508.67 | -376.49 | 1.34733D-01 | 2.92751D-06 | -1.24756D-01 |
| R( 13) | 4 - 4 | 1878.82 | -6.34 | 4.29624D-05 | 9.99994D-01 | -1.05491D+00 |
| R( 14) | 4 - 0 | 267.85 | -1624.10 | 4.06951D-05 | 7.09269D-13 | 2.50198D-04 |
| P( 16) | 4 - 0 | 282.66 | -1609.29 | 3.58479D-05 | 7.57790D-13 | 2.30515D-04 |
| R( 14) | 4 - 1 | 693.62 | -1198.33 | 1.63622D-02 | 1.51719D-10 | -7.91571D-03 |
| P( 16) | 4 - 1 | 708.26 | -1183.70 | 1.61456D-02 | 1.63937D-10 | -7.75502D-03 |
| R( 14) | 4 - 2 | 1105.12 | -786.84 | 3.52805D-01 | 1.92318D-08 | 6.90836D-02 |
| P( 16) | 4 - 2 | 1119.56 | -772.40 | 3.55435D-01 | 2.11190D-08 | 6.90298D-02 |
| R( 14) | 4 - 3 | 1501.78 | -390.17 | 1.31696D-01 | 2.92557D-06 | -1.20875D-01 |
| P( 16) | 4 - 3 | 1516.02 | -375.93 | 1.33868D-01 | 3.33245D-06 | -1.24764D-01 |
| R( 14) | 4 - 4 | 1885.16 | -6.79 | 5.29530D-05 | 9.99993D-01 | -1.05495D+00 |
| R( 15) | 4 - 0 | 275.02 | -1624.18 | 4.12068D-05 | 8.10137D-13 | 2.51494D-04 |
| P( 17) | 4 - 0 | 290.78 | -1608.42 | 3.57244D-05 | 8.55348D-13 | 2.30523D-04 |
| R( 15) | 4 - 1 | 700.70 | -1198.50 | 1.64515D-02 | 1.73176D-10 | -7.92760D-03 |
| P( 17) | 4 - 1 | 716.28 | -1182.93 | 1.60895D-02 | 1.85047D-10 | -7.75651D-03 |
| R( 15) | 4 - 2 | 1112.11 | -787.10 | 3.54045D-01 | 2.19256D-08 | 6.91008D-02 |
| P( 17) | 4 - 2 | 1127.47 | -771.73 | 3.53986D-01 | 2.38348D-08 | 6.90440D-02 |
| R( 15) | 4 - 3 | 1508.67 | -390.53 | 1.31774D-01 | 3.33008D-06 | -1.20623D-01 |
| P( 17) | 4 - 3 | 1523.83 | -375.37 | 1.33018D-01 | 3.76393D-06 | -1.24764D-01 |
| R( 15) | 4 - 4 | 1891.96 | -7.25 | 6.43813D-05 | 9.99992D-01 | -1.05500D+00 |
| R( 16) | 4 - 0 | 282.66 | -1624.24 | 4.17259D-05 | 9.18242D-13 | 2.52835D-04 |
| P( 18) | 4 - 0 | 299.38 | -1607.52 | 3.56201D-05 | 9.58906D-13 | 2.30574D-04 |
| R( 16) | 4 - 1 | 708.26 | -1198.65 | 1.65382D-02 | 1.96144D-10 | -7.93992D-03 |
| P( 18) | 4 - 1 | 724.77 | -1182.13 | 1.60379D-02 | 2.07451D-10 | -7.75841D-03 |
| R( 16) | 4 - 2 | 1119.56 | -787.34 | 3.55198D-01 | 2.48031D-08 | 6.91190D-02 |
| P( 18) | 4 - 2 | 1135.85 | -771.05 | 3.52611D-01 | 2.67154D-08 | 6.90593D-02 |
| R( 16) | 4 - 3 | 1516.02 | -390.88 | 1.31794D-01 | 3.76109D-06 | -1.20363D-01 |
| P( 18) | 4 - 3 | 1532.09 | -374.81 | 1.32177D-01 | 4.22204D-06 | -1.24757D-01 |
| R( 16) | 4 - 4 | 1899.20 | -7.70 | 7.73431D-05 | 9.99991D-01 | -1.05505D+00 |

| | | | | | | | |
|---|---|---|---|---|---|---|---|
| R( 17) | 4 - 0 | 290.78 | -1624.27 | 4.22539D-05 | 1.03370D-12 | 2.54221D-04 |
| P( 19) | 4 - 0 | 308.46 | -1606.59 | 3.55337D-05 | 1.06850D-12 | 2.30666D-04 |
| R( 17) | 4 - 1 | 716.28 | -1198.77 | 1.66230D-02 | 2.20646D-10 | -7.95266D-03 |
| P( 19) | 4 - 1 | 733.73 | -1181.32 | 1.59903D-02 | 2.31158D-10 | -7.76073D-03 |
| R( 17) | 4 - 2 | 1127.47 | -787.58 | 3.56277D-01 | 2.78660D-08 | 6.91381D-02 |
| P( 19) | 4 - 2 | 1144.70 | -770.35 | 3.51296D-01 | 2.97613D-08 | 6.90755D-02 |
| R( 17) | 4 - 3 | 1523.83 | -391.22 | 1.31763D-01 | 4.21866D-06 | -1.20095D-01 |
| P( 19) | 4 - 3 | 1540.82 | -374.23 | 1.31342D-01 | 4.70686D-06 | -1.24741D-01 |
| R( 17) | 4 - 4 | 1906.90 | -8.15 | 9.19341D-05 | 9.99990D-01 | -1.05511D+00 |
| R( 18) | 4 - 0 | 299.38 | -1624.27 | 4.27924D-05 | 1.15665D-12 | 2.55653D-04 |
| P( 20) | 4 - 0 | 318.01 | -1605.64 | 3.54641D-05 | 1.18417D-12 | 2.30801D-04 |
| R( 18) | 4 - 1 | 724.77 | -1198.88 | 1.67063D-02 | 2.46702D-10 | -7.96583D-03 |
| P( 20) | 4 - 1 | 743.17 | -1180.48 | 1.59462D-02 | 2.56173D-10 | -7.76346D-03 |
| R( 18) | 4 - 2 | 1135.85 | -787.80 | 3.57292D-01 | 3.11159D-08 | 6.91581D-02 |
| P( 20) | 4 - 2 | 1154.01 | -769.65 | 3.50031D-01 | 3.29727D-08 | 6.90928D-02 |
| R( 18) | 4 - 3 | 1532.09 | -391.56 | 1.31683D-01 | 4.70288D-06 | -1.19819D-01 |
| P( 20) | 4 - 3 | 1550.00 | -373.65 | 1.30507D-01 | 5.21847D-06 | -1.24718D-01 |
| R( 18) | 4 - 4 | 1915.05 | -8.60 | 1.08249D-04 | 9.99989D-01 | -1.05517D+00 |
| R( 19) | 4 - 0 | 308.46 | -1624.25 | 4.33425D-05 | 1.28720D-12 | 2.57131D-04 |
| P( 21) | 4 - 0 | 328.04 | -1604.67 | 3.54106D-05 | 1.30596D-12 | 2.30978D-04 |
| R( 19) | 4 - 1 | 733.73 | -1198.97 | 1.67887D-02 | 2.74336D-10 | -7.97942D-03 |
| P( 21) | 4 - 1 | 753.07 | -1179.63 | 1.59051D-02 | 2.82506D-10 | -7.76661D-03 |
| R( 19) | 4 - 2 | 1144.70 | -788.01 | 3.58252D-01 | 3.45545D-08 | 6.91790D-02 |
| P( 21) | 4 - 2 | 1163.78 | -768.93 | 3.48808D-01 | 3.63503D-08 | 6.91112D-02 |
| R( 19) | 4 - 3 | 1540.82 | -391.89 | 1.31559D-01 | 5.21383D-06 | -1.19535D-01 |
| P( 21) | 4 - 3 | 1559.64 | -373.07 | 1.29671D-01 | 5.75698D-06 | -1.24687D-01 |
| R( 19) | 4 - 4 | 1923.65 | -9.05 | 1.26384D-04 | 9.99988D-01 | -1.05523D+00 |
| P( 1) | 5 - 0 | 218.15 | -1988.68 | 2.08510D-06 | 9.12363D-17 | -2.90748D-05 |
| P( 1) | 5 - 1 | 644.53 | -1562.30 | 9.13122D-04 | 1.65698D-14 | -8.73810D-04 |

| | | | | | | | |
|---|---|---|---|---|---|---|---|
| P( 1) | 5 - 2 | 1056.67 | -1150.15 | 7.77546D-02 | 1.86361D-12 | 1.27653D-02 |
| P( 1) | 5 - 3 | 1454.00 | -752.82 | 1.07394D+00 | 1.48198D-10 | -8.95878D-02 |
| P( 1) | 5 - 4 | 1838.04 | -368.78 | 1.92660D-01 | 1.71857D-08 | 1.10673D-01 |
| R( 0) | 5 - 0 | 217.67 | -1989.60 | 6.85225D-07 | 1.00356D-16 | -2.88488D-05 |
| P( 2) | 5 - 0 | 219.10 | -1988.17 | 1.40146D-06 | 3.70715D-16 | -2.92050D-05 |
| R( 0) | 5 - 1 | 644.05 | -1563.22 | 3.07109D-04 | 1.66781D-14 | -8.76955D-04 |
| P( 2) | 5 - 1 | 645.47 | -1561.80 | 6.06322D-04 | 6.60765D-14 | -8.72485D-04 |
| R( 0) | 5 - 2 | 1056.21 | -1151.06 | 2.60490D-02 | 1.87110D-12 | 1.27822D-02 |
| P( 2) | 5 - 2 | 1057.61 | -1149.66 | 5.17093D-02 | 7.44063D-12 | 1.27577D-02 |
| R( 0) | 5 - 3 | 1453.54 | -753.73 | 3.59267D-01 | 1.48579D-10 | -8.95872D-02 |
| P( 2) | 5 - 3 | 1454.92 | -752.35 | 7.14643D-01 | 5.92089D-10 | -8.95900D-02 |
| R( 0) | 5 - 4 | 1837.59 | -369.68 | 6.43432D-02 | 1.71856D-08 | 1.10375D-01 |
| P( 2) | 5 - 4 | 1838.95 | -368.32 | 1.28266D-01 | 6.87467D-08 | 1.10806D-01 |
| R( 0) | 5 - 5 | 2206.82 | -0.45 | 9.79656D-09 | 1.00000D+00 | 1.02931D+00 |
| R( 1) | 5 - 0 | 218.15 | -1990.01 | 8.17323D-07 | 3.98411D-16 | -2.87529D-05 |
| P( 3) | 5 - 0 | 220.54 | -1987.62 | 1.27255D-06 | 8.31557D-16 | -2.93467D-05 |
| R( 1) | 5 - 1 | 644.53 | -1563.64 | 3.70360D-04 | 6.70874D-14 | -8.78774D-04 |
| P( 3) | 5 - 1 | 646.89 | -1561.27 | 5.43690D-04 | 1.48024D-13 | -8.71325D-04 |
| R( 1) | 5 - 2 | 1056.67 | -1151.49 | 3.13394D-02 | 7.50515D-12 | 1.27916D-02 |
| P( 3) | 5 - 2 | 1059.00 | -1149.16 | 4.64261D-02 | 1.67052D-11 | 1.27507D-02 |
| R( 1) | 5 - 3 | 1454.00 | -754.16 | 4.31876D-01 | 5.95247D-10 | -8.95888D-02 |
| P( 3) | 5 - 3 | 1456.30 | -751.86 | 6.41978D-01 | 1.33053D-09 | -8.95935D-02 |
| R( 1) | 5 - 4 | 1838.04 | -370.12 | 7.72554D-02 | 6.87499D-08 | 1.10211D-01 |
| P( 3) | 5 - 4 | 1840.31 | -367.85 | 1.15253D-01 | 1.54689D-07 | 1.10928D-01 |
| R( 1) | 5 - 5 | 2207.27 | -0.89 | 9.40453D-08 | 1.00000D+00 | 1.02931D+00 |
| R( 2) | 5 - 0 | 219.10 | -1990.39 | 8.71059D-07 | 8.77508D-16 | -2.86684D-05 |
| P( 4) | 5 - 0 | 222.45 | -1987.05 | 1.22357D-06 | 1.49884D-15 | -2.94999D-05 |
| R( 2) | 5 - 1 | 645.47 | -1564.03 | 3.98909D-04 | 1.50514D-13 | -8.80760D-04 |
| P( 4) | 5 - 1 | 648.78 | -1560.72 | 5.16069D-04 | 2.63652D-13 | -8.70329D-04 |

| | | | | | | | |
|---|---|---|---|---|---|---|---|
| R( 2) | 5 - 2 | 1057.61 | -1151.89 | 3.36659D-02 | 1.68936D-11 | 1.28016D-02 |
| P( 4) | 5 - 2 | 1060.87 | -1148.63 | 4.41105D-02 | 2.96886D-11 | 1.27444D-02 |
| R( 2) | 5 - 3 | 1454.92 | -754.58 | 4.63523D-01 | 1.34047D-09 | -8.95916D-02 |
| P( 4) | 5 - 3 | 1458.14 | -751.36 | 6.10249D-01 | 2.36385D-09 | -8.95982D-02 |
| R( 2) | 5 - 4 | 1838.95 | -370.55 | 8.27984D-02 | 1.54675D-07 | 1.10035D-01 |
| P( 4) | 5 - 4 | 1842.12 | -367.38 | 1.09559D-01 | 2.75071D-07 | 1.11040D-01 |
| R( 2) | 5 - 5 | 2208.16 | -1.34 | 3.40043D-07 | 1.00000D+00 | 1.02931D+00 |
| R( 3) | 5 - 0 | 220.54 | -1990.74 | 8.99185D-07 | 1.55942D-15 | -2.85952D-05 |
| P( 5) | 5 - 0 | 224.84 | -1986.44 | 1.20182D-06 | 2.34365D-15 | -2.96648D-05 |
| R( 3) | 5 - 1 | 646.89 | -1564.39 | 4.15998D-04 | 2.68290D-13 | -8.82911D-04 |
| P( 5) | 5 - 1 | 651.14 | -1560.14 | 5.00218D-04 | 4.11307D-13 | -8.69497D-04 |
| R( 3) | 5 - 2 | 1059.00 | -1152.28 | 3.50057D-02 | 3.00945D-11 | 1.28122D-02 |
| P( 5) | 5 - 2 | 1063.20 | -1148.08 | 4.27853D-02 | 4.63306D-11 | 1.27386D-02 |
| R( 3) | 5 - 3 | 1456.30 | -754.98 | 4.81505D-01 | 2.38642D-09 | -8.95956D-02 |
| P( 5) | 5 - 3 | 1460.43 | -750.84 | 5.92156D-01 | 3.69016D-09 | -8.96042D-02 |
| R( 3) | 5 - 4 | 1840.31 | -370.97 | 8.58677D-02 | 2.75006D-07 | 1.09849D-01 |
| P( 5) | 5 - 4 | 1844.39 | -366.89 | 1.06288D-01 | 4.29883D-07 | 1.11141D-01 |
| R( 3) | 5 - 5 | 2209.50 | -1.78 | 8.35811D-07 | 9.99999D-01 | 1.02931D+00 |
| R( 4) | 5 - 0 | 222.45 | -1991.06 | 9.16082D-07 | 2.43955D-15 | -2.85333D-05 |
| P( 6) | 5 - 0 | 227.71 | -1985.80 | 1.19290D-06 | 3.37568D-15 | -2.98414D-05 |
| R( 4) | 5 - 1 | 648.78 | -1564.73 | 4.27967D-04 | 4.20370D-13 | -8.85229D-04 |
| P( 6) | 5 - 1 | 653.97 | -1559.54 | 4.89799D-04 | 5.91427D-13 | -8.68830D-04 |
| R( 4) | 5 - 2 | 1060.87 | -1152.64 | 3.58980D-02 | 4.71238D-11 | 1.28235D-02 |
| P( 6) | 5 - 2 | 1065.99 | -1147.51 | 4.19112D-02 | 6.66396D-11 | 1.27335D-02 |
| R( 4) | 5 - 3 | 1458.14 | -755.37 | 4.93268D-01 | 3.73426D-09 | -8.96009D-02 |
| P( 6) | 5 - 3 | 1463.19 | -750.31 | 5.80254D-01 | 5.30936D-09 | -8.96115D-02 |
| R( 4) | 5 - 4 | 1842.12 | -371.38 | 8.77986D-02 | 4.29754D-07 | 1.09652D-01 |
| P( 6) | 5 - 4 | 1847.11 | -366.40 | 1.04106D-01 | 6.19175D-07 | 1.11231D-01 |
| R( 4) | 5 - 5 | 2211.28 | -2.23 | 1.66936D-06 | 9.99999D-01 | 1.02931D+00 |

| | | | | | | | | |
|---|---|---|---|---|---|---|---|---|
| R( 5) | 5 - 0 | 224.84 | -1991.34 | 9.27279D-07 | 3.52041D-15 | -2.84828D-05 |
| P( 7) | 5 - 0 | 231.05 | -1985.13 | 1.19130D-06 | 4.59494D-15 | -3.00297D-05 |
| R( 5) | 5 - 1 | 651.14 | -1565.04 | 4.37255D-04 | 6.07100D-13 | -8.87714D-04 |
| P( 7) | 5 - 1 | 657.27 | -1558.90 | 4.82373D-04 | 8.03943D-13 | -8.68327D-04 |
| R( 5) | 5 - 2 | 1063.20 | -1152.98 | 3.65502D-02 | 6.80110D-11 | 1.28353D-02 |
| P( 7) | 5 - 2 | 1069.25 | -1146.93 | 4.12808D-02 | 9.06090D-11 | 1.27290D-02 |
| R( 5) | 5 - 3 | 1460.43 | -755.74 | 5.01676D-01 | 5.38557D-09 | -8.96074D-02 |
| P( 7) | 5 - 3 | 1466.41 | -749.77 | 5.71679D-01 | 7.22098D-09 | -8.96200D-02 |
| R( 5) | 5 - 4 | 1844.39 | -371.79 | 8.91044D-02 | 6.18952D-07 | 1.09445D-01 |
| P( 7) | 5 - 4 | 1850.28 | -365.90 | 1.02498D-01 | 8.42992D-07 | 1.11310D-01 |
| R( 5) | 5 - 5 | 2213.51 | -2.67 | 2.92865D-06 | 9.99999D-01 | 1.02931D+00 |
| R( 6) | 5 - 0 | 227.71 | -1991.59 | 9.35354D-07 | 4.80476D-15 | -2.84435D-05 |
| P( 8) | 5 - 0 | 234.88 | -1984.42 | 1.19446D-06 | 6.00169D-15 | -3.02298D-05 |
| R( 6) | 5 - 1 | 653.97 | -1565.33 | 4.45002D-04 | 8.28852D-13 | -8.90366D-04 |
| P( 8) | 5 - 1 | 661.05 | -1558.25 | 4.76802D-04 | 1.04881D-12 | -8.67990D-04 |
| R( 6) | 5 - 2 | 1065.99 | -1153.30 | 3.70591D-02 | 9.27881D-11 | 1.28477D-02 |
| P( 8) | 5 - 2 | 1072.98 | -1146.32 | 4.07974D-02 | 1.18235D-10 | 1.27250D-02 |
| R( 6) | 5 - 3 | 1463.19 | -756.11 | 5.08065D-01 | 7.34206D-09 | -8.96152D-02 |
| P( 8) | 5 - 3 | 1470.09 | -749.21 | 5.65095D-01 | 9.42472D-09 | -8.96299D-02 |
| R( 6) | 5 - 4 | 1847.11 | -372.19 | 9.00246D-02 | 8.42639D-07 | 1.09226D-01 |
| P( 8) | 5 - 4 | 1853.90 | -365.39 | 1.01226D-01 | 1.10139D-06 | 1.11379D-01 |
| R( 6) | 5 - 5 | 2216.18 | -3.12 | 4.70152D-06 | 9.99998D-01 | 1.02932D+00 |
| R( 7) | 5 - 0 | 231.05 | -1991.81 | 9.41672D-07 | 6.29564D-15 | -2.84156D-05 |
| P( 9) | 5 - 0 | 239.18 | -1983.68 | 1.20103D-06 | 7.59642D-15 | -3.04419D-05 |
| R( 7) | 5 - 1 | 657.27 | -1565.59 | 4.51813D-04 | 1.08603D-12 | -8.93186D-04 |
| P( 9) | 5 - 1 | 665.30 | -1557.56 | 4.72483D-04 | 1.32602D-12 | -8.67817D-04 |
| R( 7) | 5 - 2 | 1069.25 | -1153.61 | 3.74760D-02 | 1.21490D-10 | 1.28608D-02 |
| P( 9) | 5 - 2 | 1077.17 | -1145.69 | 4.04097D-02 | 1.49514D-10 | 1.27217D-02 |
| R( 7) | 5 - 3 | 1466.41 | -756.45 | 5.13142D-01 | 9.60554D-09 | -8.96241D-02 |

| | | | | | | | |
|---|---|---|---|---|---|---|---|
| P( 9) | 5 - 3 | 1474.22 | -748.64 | 5.59796D-01 | 1.19203D-08 | -8.96410D-02 |
| R( 7) | 5 - 4 | 1850.28 | -372.58 | 9.06861D-02 | 1.10086D-06 | 1.08997D-01 |
| P( 9) | 5 - 4 | 1857.98 | -364.88 | 1.00163D-01 | 1.39442D-06 | 1.11438D-01 |
| R( 7) | 5 - 5 | 2219.30 | -3.56 | 7.07571D-06 | 9.99997D-01 | 1.02932D+00 |
| R( 8) | 5 - 0 | 234.88 | -1991.99 | 9.47024D-07 | 7.99638D-15 | -2.83990D-05 |
| P( 10) | 5 - 0 | 243.96 | -1982.91 | 1.21024D-06 | 9.37987D-15 | -3.06659D-05 |
| R( 8) | 5 - 1 | 661.05 | -1565.82 | 4.58037D-04 | 1.37907D-12 | -8.96175D-04 |
| P( 10) | 5 - 1 | 670.02 | -1556.85 | 4.69067D-04 | 1.63558D-12 | -8.67809D-04 |
| R( 8) | 5 - 2 | 1072.98 | -1153.89 | 3.78304D-02 | 1.54153D-10 | 1.28745D-02 |
| P( 10) | 5 - 2 | 1081.83 | -1145.04 | 4.00880D-02 | 1.84448D-10 | 1.27190D-02 |
| R( 8) | 5 - 3 | 1470.09 | -756.78 | 5.17317D-01 | 1.21779D-08 | -8.96343D-02 |
| P( 10) | 5 - 3 | 1478.82 | -748.05 | 5.55370D-01 | 1.47078D-08 | -8.96534D-02 |
| R( 8) | 5 - 4 | 1853.90 | -372.97 | 9.11623D-02 | 1.39367D-06 | 1.08757D-01 |
| P( 10) | 5 - 4 | 1862.51 | -364.36 | 9.92351D-02 | 1.72216D-06 | 1.11486D-01 |
| R( 8) | 5 - 5 | 2222.86 | -4.01 | 1.01388D-05 | 9.99997D-01 | 1.02932D+00 |
| R( 9) | 5 - 0 | 239.18 | -1992.14 | 9.51899D-07 | 9.91057D-15 | -2.83938D-05 |
| P( 11) | 5 - 0 | 249.22 | -1982.11 | 1.22161D-06 | 1.13530D-14 | -3.09020D-05 |
| R( 9) | 5 - 1 | 665.30 | -1566.02 | 4.63894D-04 | 1.70844D-12 | -8.99334D-04 |
| P( 11) | 5 - 1 | 675.22 | -1556.11 | 4.66338D-04 | 1.97752D-12 | -8.67966D-04 |
| R( 9) | 5 - 2 | 1077.17 | -1154.15 | 3.81409D-02 | 1.90817D-10 | 1.28888D-02 |
| P( 11) | 5 - 2 | 1086.96 | -1144.37 | 3.98139D-02 | 2.23038D-10 | 1.27169D-02 |
| R( 9) | 5 - 3 | 1474.22 | -757.10 | 5.20843D-01 | 1.50613D-08 | -8.96457D-02 |
| P( 11) | 5 - 3 | 1483.87 | -747.45 | 5.51565D-01 | 1.77870D-08 | -8.96672D-02 |
| R( 9) | 5 - 4 | 1857.98 | -373.34 | 9.14984D-02 | 1.72113D-06 | 1.08507D-01 |
| P( 11) | 5 - 4 | 1867.50 | -363.83 | 9.83975D-02 | 2.08469D-06 | 1.11523D-01 |
| R( 9) | 5 - 5 | 2226.87 | -4.45 | 1.39782D-05 | 9.99996D-01 | 1.02932D+00 |
| R( 10) | 5 - 0 | 243.96 | -1992.26 | 9.56618D-07 | 1.20421D-14 | -2.83998D-05 |
| P( 12) | 5 - 0 | 254.95 | -1981.27 | 1.23484D-06 | 1.35171D-14 | -3.11503D-05 |
| R( 10) | 5 - 1 | 670.02 | -1566.20 | 4.69526D-04 | 2.07463D-12 | -9.02663D-04 |

| | | | | | | |
|---|---|---|---|---|---|---|
| P( 12) | 5 - 1 | 680.88 | -1555.34 | 4.64155D-04 | 2.35191D-12 | -8.68290D-04 |
| R( 10) | 5 - 2 | 1081.83 | -1154.39 | 3.84193D-02 | 2.31524D-10 | 1.29037D-02 |
| P( 12) | 5 - 2 | 1092.55 | -1143.68 | 3.95755D-02 | 2.65290D-10 | 1.27154D-02 |
| R( 10) | 5 - 3 | 1478.82 | -757.41 | 5.23885D-01 | 1.82579D-08 | -8.96583D-02 |
| P( 12) | 5 - 3 | 1489.38 | -746.84 | 5.48215D-01 | 2.11582D-08 | -8.96822D-02 |
| R( 10) | 5 - 4 | 1862.51 | -373.71 | 9.17240D-02 | 2.08331D-06 | 1.08245D-01 |
| P( 12) | 5 - 4 | 1872.93 | -363.29 | 9.76208D-02 | 2.48208D-06 | 1.11549D-01 |
| R( 10) | 5 - 5 | 2231.32 | -4.90 | 1.86811D-05 | 9.99995D-01 | 1.02932D+00 |
| R( 11) | 5 - 0 | 249.22 | -1992.35 | 9.61401D-07 | 1.43951D-14 | -2.84173D-05 |
| P( 13) | 5 - 0 | 261.16 | -1980.40 | 1.24976D-06 | 1.58736D-14 | -3.14109D-05 |
| R( 11) | 5 - 1 | 675.22 | -1566.35 | 4.75033D-04 | 2.47818D-12 | -9.06164D-04 |
| P( 13) | 5 - 1 | 687.02 | -1554.55 | 4.62422D-04 | 2.75883D-12 | -8.68780D-04 |
| R( 11) | 5 - 2 | 1086.96 | -1154.61 | 3.86739D-02 | 2.76318D-10 | 1.29192D-02 |
| P( 13) | 5 - 2 | 1098.60 | -1142.96 | 3.93646D-02 | 3.11210D-10 | 1.27146D-02 |
| R( 11) | 5 - 3 | 1483.87 | -757.70 | 5.26556D-01 | 2.17700D-08 | -8.96721D-02 |
| P( 13) | 5 - 3 | 1495.35 | -746.21 | 5.45208D-01 | 2.48216D-08 | -8.96985D-02 |
| R( 11) | 5 - 4 | 1867.50 | -374.07 | 9.18593D-02 | 2.48029D-06 | 1.07972D-01 |
| P( 13) | 5 - 4 | 1878.82 | -362.74 | 9.68850D-02 | 2.91443D-06 | 1.11564D-01 |
| R( 11) | 5 - 5 | 2236.22 | -5.34 | 2.43345D-05 | 9.99994D-01 | 1.02933D+00 |
| R( 12) | 5 - 0 | 254.95 | -1992.40 | 9.66403D-07 | 1.69742D-14 | -2.84461D-05 |
| P( 14) | 5 - 0 | 267.85 | -1979.50 | 1.26622D-06 | 1.84231D-14 | -3.16838D-05 |
| R( 12) | 5 - 1 | 680.88 | -1566.47 | 4.80483D-04 | 2.91964D-12 | -9.09836D-04 |
| P( 14) | 5 - 1 | 693.62 | -1553.73 | 4.61071D-04 | 3.19842D-12 | -8.69436D-04 |
| R( 12) | 5 - 2 | 1092.55 | -1154.81 | 3.89103D-02 | 3.25248D-10 | 1.29353D-02 |
| P( 14) | 5 - 2 | 1105.12 | -1142.23 | 3.91755D-02 | 3.60807D-10 | 1.27143D-02 |
| R( 12) | 5 - 3 | 1489.38 | -757.97 | 5.28934D-01 | 2.56001D-08 | -8.96871D-02 |
| P( 14) | 5 - 3 | 1501.78 | -745.57 | 5.42465D-01 | 2.87775D-08 | -8.97162D-02 |
| R( 12) | 5 - 4 | 1872.93 | -374.42 | 9.19184D-02 | 2.91215D-06 | 1.07689D-01 |
| P( 14) | 5 - 4 | 1885.16 | -362.19 | 9.61761D-02 | 3.38184D-06 | 1.11569D-01 |

| | | | | | | | |
|---|---|---|---|---|---|---|---|
| R( 12) | 5 - 5 | 2241.57 | -5.79 | 3.10252D-05 | 9.99993D-01 | 1.02933D+00 |
| R( 13) | 5 - 0 | 261.16 | -1992.42 | 9.71738D-07 | 1.97840D-14 | -2.84863D-05 |
| P( 15) | 5 - 0 | 275.02 | -1978.57 | 1.28414D-06 | 2.11696D-14 | -3.19692D-05 |
| R( 13) | 5 - 1 | 687.02 | -1566.57 | 4.85928D-04 | 3.39962D-12 | -9.13682D-04 |
| P( 15) | 5 - 1 | 700.70 | -1552.88 | 4.60055D-04 | 3.67080D-12 | -8.70260D-04 |
| R( 13) | 5 - 2 | 1098.60 | -1154.99 | 3.91328D-02 | 3.78363D-10 | 1.29521D-02 |
| P( 15) | 5 - 2 | 1112.11 | -1141.48 | 3.90040D-02 | 4.14093D-10 | 1.27147D-02 |
| R( 13) | 5 - 3 | 1495.35 | -758.23 | 5.31076D-01 | 2.97506D-08 | -8.97033D-02 |
| P( 15) | 5 - 3 | 1508.67 | -744.91 | 5.39929D-01 | 3.30264D-08 | -8.97352D-02 |
| R( 13) | 5 - 4 | 1878.82 | -374.76 | 9.19116D-02 | 3.37899D-06 | 1.07394D-01 |
| P( 15) | 5 - 4 | 1891.96 | -361.63 | 9.54841D-02 | 3.88442D-06 | 1.11563D-01 |
| R( 13) | 5 - 5 | 2247.35 | -6.23 | 3.88396D-05 | 9.99992D-01 | 1.02933D+00 |
| R( 14) | 5 - 0 | 267.85 | -1992.41 | 9.77496D-07 | 2.28309D-14 | -2.85380D-05 |
| P( 16) | 5 - 0 | 282.66 | -1977.60 | 1.30347D-06 | 2.41144D-14 | -3.22673D-05 |
| R( 14) | 5 - 1 | 693.62 | -1566.64 | 4.91408D-04 | 3.91875D-12 | -9.17703D-04 |
| P( 16) | 5 - 1 | 708.26 | -1552.01 | 4.59336D-04 | 4.17615D-12 | -8.71252D-04 |
| R( 14) | 5 - 2 | 1105.12 | -1155.14 | 3.93444D-02 | 4.35716D-10 | 1.29695D-02 |
| P( 16) | 5 - 2 | 1119.56 | -1140.71 | 3.88470D-02 | 4.71081D-10 | 1.27156D-02 |
| R( 14) | 5 - 3 | 1501.78 | -758.48 | 5.33026D-01 | 3.42244D-08 | -8.97207D-02 |
| P( 16) | 5 - 3 | 1516.02 | -744.24 | 5.37557D-01 | 3.75689D-08 | -8.97555D-02 |
| R( 14) | 5 - 4 | 1885.16 | -375.10 | 9.18463D-02 | 3.88092D-06 | 1.07089D-01 |
| P( 16) | 5 - 4 | 1899.20 | -361.06 | 9.48017D-02 | 4.42229D-06 | 1.11547D-01 |
| R( 14) | 5 - 5 | 2253.59 | -6.68 | 4.78641D-05 | 9.99991D-01 | 1.02934D+00 |
| R( 15) | 5 - 0 | 275.02 | -1992.37 | 9.83742D-07 | 2.61180D-14 | -2.86011D-05 |
| P( 17) | 5 - 0 | 290.78 | -1976.60 | 1.32417D-06 | 2.72599D-14 | -3.25780D-05 |
| R( 15) | 5 - 1 | 700.70 | -1566.68 | 4.96954D-04 | 4.47768D-12 | -9.21899D-04 |
| P( 17) | 5 - 1 | 716.28 | -1551.11 | 4.58889D-04 | 4.71467D-12 | -8.72413D-04 |
| R( 15) | 5 - 2 | 1112.11 | -1155.28 | 3.95474D-02 | 4.97363D-10 | 1.29875D-02 |
| P( 17) | 5 - 2 | 1127.47 | -1139.91 | 3.87022D-02 | 5.31788D-10 | 1.27172D-02 |

| | | | | | | | |
|---|---|---|---|---|---|---|---|
| R( 15) | 5 - 3 | 1508.67 | -758.71 | 5.34814D-01 | 3.90243D-08 | -8.97393D-02 |
| P( 17) | 5 - 3 | 1523.83 | -743.56 | 5.35316D-01 | 4.24058D-08 | -8.97771D-02 |
| R( 15) | 5 - 4 | 1891.96 | -375.43 | 9.17283D-02 | 4.41803D-06 | 1.06772D-01 |
| P( 17) | 5 - 4 | 1906.90 | -360.48 | 9.41232D-02 | 4.99557D-06 | 1.11519D-01 |
| R( 15) | 5 - 5 | 2260.26 | -7.12 | 5.81845D-05 | 9.99989D-01 | 1.02934D+00 |
| R( 16) | 5 - 0 | 282.66 | -1992.29 | 9.90533D-07 | 2.96522D-14 | -2.86758D-05 |
| P( 18) | 5 - 0 | 299.38 | -1975.57 | 1.34623D-06 | 3.06088D-14 | -3.29016D-05 |
| R( 16) | 5 - 1 | 708.26 | -1566.70 | 5.02589D-04 | 5.07714D-12 | -9.26271D-04 |
| P( 18) | 5 - 1 | 724.77 | -1550.18 | 4.58692D-04 | 5.28659D-12 | -8.73743D-04 |
| R( 16) | 5 - 2 | 1119.56 | -1155.39 | 3.97438D-02 | 5.63362D-10 | 1.30061D-02 |
| P( 18) | 5 - 2 | 1135.85 | -1139.10 | 3.85678D-02 | 5.96231D-10 | 1.27194D-02 |
| R( 16) | 5 - 3 | 1516.02 | -758.93 | 5.36466D-01 | 4.41534D-08 | -8.97591D-02 |
| P( 18) | 5 - 3 | 1532.09 | -742.86 | 5.33182D-01 | 4.75379D-08 | -8.98001D-02 |
| R( 16) | 5 - 4 | 1899.20 | -375.75 | 9.15621D-02 | 4.99045D-06 | 1.06444D-01 |
| P( 18) | 5 - 4 | 1915.05 | -359.90 | 9.34446D-02 | 5.60440D-06 | 1.11481D-01 |
| R( 16) | 5 - 5 | 2267.39 | -7.57 | 6.98863D-05 | 9.99988D-01 | 1.02934D+00 |
| R( 17) | 5 - 0 | 290.78 | -1992.18 | 9.97914D-07 | 3.34394D-14 | -2.87620D-05 |
| P( 19) | 5 - 0 | 308.46 | -1974.50 | 1.36963D-06 | 3.41640D-14 | -3.32382D-05 |
| R( 17) | 5 - 1 | 716.28 | -1566.68 | 5.08334D-04 | 5.71785D-12 | -9.30821D-04 |
| P( 19) | 5 - 1 | 733.73 | -1549.23 | 4.58729D-04 | 5.89215D-12 | -8.75244D-04 |
| R( 17) | 5 - 2 | 1127.47 | -1155.49 | 3.99348D-02 | 6.33774D-10 | 1.30254D-02 |
| P( 19) | 5 - 2 | 1144.70 | -1138.26 | 3.84424D-02 | 6.64432D-10 | 1.27223D-02 |
| R( 17) | 5 - 3 | 1523.83 | -759.13 | 5.38000D-01 | 4.96146D-08 | -8.97800D-02 |
| P( 19) | 5 - 3 | 1540.82 | -742.14 | 5.31136D-01 | 5.29661D-08 | -8.98244D-02 |
| R( 17) | 5 - 4 | 1906.90 | -376.06 | 9.13512D-02 | 5.59831D-06 | 1.06105D-01 |
| P( 19) | 5 - 4 | 1923.65 | -359.31 | 9.27625D-02 | 6.24892D-06 | 1.11432D-01 |
| R( 17) | 5 - 5 | 2274.95 | -8.01 | 8.30548D-05 | 9.99987D-01 | 1.02934D+00 |
| R( 18) | 5 - 0 | 299.38 | -1992.03 | 1.00592D-06 | 3.74863D-14 | -2.88598D-05 |
| P( 20) | 5 - 0 | 318.01 | -1973.40 | 1.39438D-06 | 3.79288D-14 | -3.35879D-05 |

| | | | | | | | |
|---|---|---|---|---|---|---|---|
| R( 18) | 5 - 1 | 724.77 | -1566.64 | 5.14204D-04 | 6.40061D-12 | -9.35551D-04 |
| P( 20) | 5 - 1 | 743.17 | -1548.24 | 4.58987D-04 | 6.53165D-12 | -8.76915D-04 |
| R( 18) | 5 - 2 | 1135.85 | -1155.56 | 4.01216D-02 | 7.08665D-10 | 1.30453D-02 |
| P( 20) | 5 - 2 | 1154.01 | -1137.41 | 3.83247D-02 | 7.36413D-10 | 1.27257D-02 |
| R( 18) | 5 - 3 | 1532.09 | -759.32 | 5.39433D-01 | 5.54115D-08 | -8.98022D-02 |
| P( 20) | 5 - 3 | 1550.00 | -741.41 | 5.29162D-01 | 5.86915D-08 | -8.98501D-02 |
| R( 18) | 5 - 4 | 1915.05 | -376.36 | 9.10983D-02 | 6.24175D-06 | 1.05755D-01 |
| P( 20) | 5 - 4 | 1932.70 | -358.71 | 9.20745D-02 | 6.92929D-06 | 1.11371D-01 |
| R( 18) | 5 - 5 | 2282.96 | -8.45 | 9.77748D-05 | 9.99985D-01 | 1.02934D+00 |
| R( 19) | 5 - 0 | 308.46 | -1991.85 | 1.01460D-06 | 4.17994D-14 | -2.89692D-05 |
| P( 21) | 5 - 0 | 328.04 | -1972.27 | 1.42049D-06 | 4.19066D-14 | -3.39508D-05 |
| R( 19) | 5 - 1 | 733.73 | -1566.57 | 5.20216D-04 | 7.12622D-12 | -9.40461D-04 |
| P( 21) | 5 - 1 | 753.07 | -1547.23 | 4.59457D-04 | 7.20539D-12 | -8.78759D-04 |
| R( 19) | 5 - 2 | 1144.70 | -1155.61 | 4.03052D-02 | 7.88101D-10 | 1.30659D-02 |
| P( 21) | 5 - 2 | 1163.78 | -1136.53 | 3.82140D-02 | 8.12201D-10 | 1.27298D-02 |
| R( 19) | 5 - 3 | 1540.82 | -759.49 | 5.40776D-01 | 6.15473D-08 | -8.98255D-02 |
| P( 21) | 5 - 3 | 1559.64 | -740.67 | 5.27247D-01 | 6.47154D-08 | -8.98771D-02 |
| R( 19) | 5 - 4 | 1923.65 | -376.66 | 9.08056D-02 | 6.92091D-06 | 1.05393D-01 |
| P( 21) | 5 - 4 | 1942.21 | -358.10 | 9.13786D-02 | 7.64566D-06 | 1.11300D-01 |
| R( 19) | 5 - 5 | 2291.41 | -8.90 | 1.14131D-04 | 9.99984D-01 | 1.02935D+00 |
| Q( 0) | 0 - 0 | 217.67 | 0.00 | 0.00000D+00 | 1.00000D+00 | -1.08551D+00 |
| Q( 1) | 0 - 0 | 218.15 | -0.00 | 0.00000D+00 | 1.00000D+00 | -1.08552D+00 |
| Q( 2) | 0 - 0 | 219.10 | -0.00 | 0.00000D+00 | 1.00000D+00 | -1.08554D+00 |
| Q( 3) | 0 - 0 | 220.54 | 0.00 | 0.00000D+00 | 1.00000D+00 | -1.08557D+00 |
| Q( 4) | 0 - 0 | 222.45 | 0.00 | 0.00000D+00 | 1.00000D+00 | -1.08561D+00 |
| Q( 5) | 0 - 0 | 224.84 | 0.00 | 0.00000D+00 | 1.00000D+00 | -1.08565D+00 |
| Q( 6) | 0 - 0 | 227.71 | 0.00 | 0.00000D+00 | 1.00000D+00 | -1.08571D+00 |
| Q( 7) | 0 - 0 | 231.05 | 0.00 | 0.00000D+00 | 1.00000D+00 | -1.08578D+00 |
| Q( 8) | 0 - 0 | 234.88 | 0.00 | 0.00000D+00 | 1.00000D+00 | -1.08586D+00 |

| | | | | | | |
|---|---|---|---|---|---|---|
| Q( 9) | 0 - 0 | 239.18 | 0.00 | 0.00000D+00 | 1.00000D+00 | -1.08595D+00 |
| Q( 10) | 0 - 0 | 243.96 | 0.00 | 0.00000D+00 | 1.00000D+00 | -1.08605D+00 |
| Q( 11) | 0 - 0 | 249.22 | 0.00 | 0.00000D+00 | 1.00000D+00 | -1.08615D+00 |
| Q( 12) | 0 - 0 | 254.95 | 0.00 | 0.00000D+00 | 1.00000D+00 | -1.08627D+00 |
| Q( 13) | 0 - 0 | 261.16 | 0.00 | 0.00000D+00 | 1.00000D+00 | -1.08640D+00 |
| Q( 14) | 0 - 0 | 267.85 | 0.00 | 0.00000D+00 | 1.00000D+00 | -1.08654D+00 |
| Q( 15) | 0 - 0 | 275.02 | 0.00 | 0.00000D+00 | 1.00000D+00 | -1.08668D+00 |
| Q( 16) | 0 - 0 | 282.66 | 0.00 | 0.00000D+00 | 1.00000D+00 | -1.08684D+00 |
| Q( 17) | 0 - 0 | 290.78 | 0.00 | 0.00000D+00 | 1.00000D+00 | -1.08701D+00 |
| Q( 18) | 0 - 0 | 299.38 | 0.00 | 0.00000D+00 | 1.00000D+00 | -1.08718D+00 |
| Q( 19) | 0 - 0 | 308.46 | 0.00 | 0.00000D+00 | 1.00000D+00 | -1.08737D+00 |
| Q( 20) | 0 - 0 | 318.01 | 0.00 | 0.00000D+00 | 1.00000D+00 | -1.08756D+00 |
| Q( 0) | 1 - 0 | 217.67 | -426.38 | 0.00000D+00 | 2.20151D-18 | 9.16812D-02 |
| Q( 0) | 1 - 1 | 644.05 | 0.00 | 0.00000D+00 | 1.00000D+00 | 1.08568D+00 |
| Q( 1) | 1 - 0 | 218.15 | -426.38 | 0.00000D+00 | 8.45434D-18 | 9.16787D-02 |
| Q( 1) | 1 - 1 | 644.53 | -0.00 | 0.00000D+00 | 1.00000D+00 | 1.08569D+00 |
| Q( 2) | 1 - 0 | 219.10 | -426.37 | 0.00000D+00 | 7.40171D-17 | 9.16737D-02 |
| Q( 2) | 1 - 1 | 645.47 | -0.00 | 0.00000D+00 | 1.00000D+00 | 1.08571D+00 |
| Q( 3) | 1 - 0 | 220.54 | -426.35 | 0.00000D+00 | 2.19442D-18 | 9.16661D-02 |
| Q( 3) | 1 - 1 | 646.89 | 0.00 | 0.00000D+00 | 1.00000D+00 | 1.08573D+00 |
| Q( 4) | 1 - 0 | 222.45 | -426.32 | 0.00000D+00 | 2.19042D-18 | 9.16560D-02 |
| Q( 4) | 1 - 1 | 648.78 | 0.00 | 0.00000D+00 | 1.00000D+00 | 1.08577D+00 |
| Q( 5) | 1 - 0 | 224.84 | -426.30 | 0.00000D+00 | 2.18548D-18 | 9.16434D-02 |
| Q( 5) | 1 - 1 | 651.14 | 0.00 | 0.00000D+00 | 1.00000D+00 | 1.08581D+00 |
| Q( 6) | 1 - 0 | 227.71 | -426.26 | 0.00000D+00 | 2.17949D-18 | 9.16282D-02 |
| Q( 6) | 1 - 1 | 653.97 | 0.00 | 0.00000D+00 | 1.00000D+00 | 1.08587D+00 |
| Q( 7) | 1 - 0 | 231.05 | -426.22 | 0.00000D+00 | 2.17257D-18 | 9.16105D-02 |
| Q( 7) | 1 - 1 | 657.27 | 0.00 | 0.00000D+00 | 1.00000D+00 | 1.08593D+00 |
| Q( 8) | 1 - 0 | 234.88 | -426.17 | 0.00000D+00 | 2.16468D-18 | 9.15903D-02 |

| | | | | | | |
|---|---|---|---|---|---|---|
| Q( 8) | 1 - 1 | 661.05 | 0.00 | 0.00000D+00 | 1.00000D+00 | 1.08600D+00 |
| Q( 9) | 1 - 0 | 239.18 | -426.12 | 0.00000D+00 | 2.15612D-18 | 9.15675D-02 |
| Q( 9) | 1 - 1 | 665.30 | 0.00 | 0.00000D+00 | 1.00000D+00 | 1.08608D+00 |
| Q( 10) | 1 - 0 | 243.96 | -426.06 | 0.00000D+00 | 2.14638D-18 | 9.15422D-02 |
| Q( 10) | 1 - 1 | 670.02 | 0.00 | 0.00000D+00 | 1.00000D+00 | 1.08616D+00 |
| Q( 11) | 1 - 0 | 249.22 | -426.00 | 0.00000D+00 | 2.13579D-18 | 9.15144D-02 |
| Q( 11) | 1 - 1 | 675.22 | -0.00 | 0.00000D+00 | 1.00000D+00 | 1.08626D+00 |
| Q( 12) | 1 - 0 | 254.95 | -425.93 | 0.00000D+00 | 2.12469D-18 | 9.14840D-02 |
| Q( 12) | 1 - 1 | 680.88 | -0.00 | 0.00000D+00 | 1.00000D+00 | 1.08637D+00 |
| Q( 13) | 1 - 0 | 261.16 | -425.85 | 0.00000D+00 | 2.11266D-18 | 9.14511D-02 |
| Q( 13) | 1 - 1 | 687.02 | -0.00 | 0.00000D+00 | 1.00000D+00 | 1.08648D+00 |
| Q( 14) | 1 - 0 | 267.85 | -425.77 | 0.00000D+00 | 2.17013D-18 | 9.14156D-02 |
| Q( 14) | 1 - 1 | 693.62 | -0.00 | 0.00000D+00 | 1.00000D+00 | 1.08660D+00 |
| Q( 15) | 1 - 0 | 275.02 | -425.69 | 0.00000D+00 | 2.15632D-18 | 9.13775D-02 |
| Q( 15) | 1 - 1 | 700.70 | -0.00 | 0.00000D+00 | 1.00000D+00 | 1.08673D+00 |
| Q( 16) | 1 - 0 | 282.66 | -425.59 | 0.00000D+00 | 2.14205D-18 | 9.13369D-02 |
| Q( 16) | 1 - 1 | 708.26 | -0.00 | 0.00000D+00 | 1.00000D+00 | 1.08687D+00 |
| Q( 17) | 1 - 0 | 290.78 | -425.49 | 0.00000D+00 | 2.12709D-18 | 9.12937D-02 |
| Q( 17) | 1 - 1 | 716.28 | -0.00 | 0.00000D+00 | 1.00000D+00 | 1.08702D+00 |
| Q( 18) | 1 - 0 | 299.38 | -425.39 | 0.00000D+00 | 2.11153D-18 | 9.12479D-02 |
| Q( 18) | 1 - 1 | 724.77 | -0.00 | 0.00000D+00 | 1.00000D+00 | 1.08718D+00 |
| Q( 19) | 1 - 0 | 308.46 | -425.28 | 0.00000D+00 | 2.09560D-18 | 9.11995D-02 |
| Q( 19) | 1 - 1 | 733.73 | -0.00 | 0.00000D+00 | 1.00000D+00 | 1.08735D+00 |
| Q( 20) | 1 - 0 | 318.01 | -425.16 | 0.00000D+00 | 2.07929D-18 | 9.11486D-02 |
| Q( 20) | 1 - 1 | 743.17 | -0.00 | 0.00000D+00 | 1.00000D+00 | 1.08752D+00 |
| Q( 0) | 2 - 0 | 217.67 | -838.54 | 0.00000D+00 | 8.81088D-21 | 2.75350D-02 |
| Q( 0) | 2 - 1 | 644.05 | -412.15 | 0.00000D+00 | 1.85856D-24 | -1.16704D-01 |
| Q( 0) | 2 - 2 | 1056.21 | 0.00 | 0.00000D+00 | 1.00000D+00 | -1.08194D+00 |
| Q( 1) | 2 - 0 | 218.15 | -838.53 | 0.00000D+00 | 8.77546D-20 | 2.75355D-02 |

| | | | | | | | |
|---|---|---|---|---|---|---|---|
| Q( 1) | 2 - 1 | 644.53 | -412.15 | 0.00000D+00 | 3.78065D-18 | -1.16700D-01 |
| Q( 1) | 2 - 2 | 1056.67 | -0.00 | 0.00000D+00 | 1.00000D+00 | -1.08195D+00 |
| Q( 2) | 2 - 0 | 219.10 | -838.50 | 0.00000D+00 | 3.44507D-18 | 2.75364D-02 |
| Q( 2) | 2 - 1 | 645.47 | -412.14 | 0.00000D+00 | 9.43965D-17 | -1.16692D-01 |
| Q( 2) | 2 - 2 | 1057.61 | -0.00 | 0.00000D+00 | 1.00000D+00 | -1.08197D+00 |
| Q( 3) | 2 - 0 | 220.54 | -838.47 | 0.00000D+00 | 8.67738D-21 | 2.75378D-02 |
| Q( 3) | 2 - 1 | 646.89 | -412.12 | 0.00000D+00 | 1.09520D-24 | -1.16680D-01 |
| Q( 3) | 2 - 2 | 1059.00 | 0.00 | 0.00000D+00 | 1.00000D+00 | -1.08199D+00 |
| Q( 4) | 2 - 0 | 222.45 | -838.42 | 0.00000D+00 | 8.58342D-21 | 2.75396D-02 |
| Q( 4) | 2 - 1 | 648.78 | -412.09 | 0.00000D+00 | 1.13032D-24 | -1.16664D-01 |
| Q( 4) | 2 - 2 | 1060.87 | 0.00 | 0.00000D+00 | 1.00000D+00 | -1.08202D+00 |
| Q( 5) | 2 - 0 | 224.84 | -838.36 | 0.00000D+00 | 8.46483D-21 | 2.75419D-02 |
| Q( 5) | 2 - 1 | 651.14 | -412.06 | 0.00000D+00 | 1.11799D-24 | -1.16643D-01 |
| Q( 5) | 2 - 2 | 1063.20 | 0.00 | 0.00000D+00 | 1.00000D+00 | -1.08206D+00 |
| Q( 6) | 2 - 0 | 227.71 | -838.28 | 0.00000D+00 | 8.32254D-21 | 2.75447D-02 |
| Q( 6) | 2 - 1 | 653.97 | -412.02 | 0.00000D+00 | 1.26586D-24 | -1.16618D-01 |
| Q( 6) | 2 - 2 | 1065.99 | 0.00 | 0.00000D+00 | 1.00000D+00 | -1.08210D+00 |
| Q( 7) | 2 - 0 | 231.05 | -838.20 | 0.00000D+00 | 8.15974D-21 | 2.75480D-02 |
| Q( 7) | 2 - 1 | 657.27 | -411.98 | 0.00000D+00 | 1.36781D-24 | -1.16590D-01 |
| Q( 7) | 2 - 2 | 1069.25 | 0.00 | 0.00000D+00 | 1.00000D+00 | -1.08215D+00 |
| Q( 8) | 2 - 0 | 234.88 | -838.10 | 0.00000D+00 | 7.97730D-21 | 2.75517D-02 |
| Q( 8) | 2 - 1 | 661.05 | -411.93 | 0.00000D+00 | 1.49612D-24 | -1.16557D-01 |
| Q( 8) | 2 - 2 | 1072.98 | 0.00 | 0.00000D+00 | 1.00000D+00 | -1.08221D+00 |
| Q( 9) | 2 - 0 | 239.18 | -837.99 | 0.00000D+00 | 7.77338D-21 | 2.75559D-02 |
| Q( 9) | 2 - 1 | 665.30 | -411.87 | 0.00000D+00 | 1.76491D-24 | -1.16520D-01 |
| Q( 9) | 2 - 2 | 1077.17 | 0.00 | 0.00000D+00 | 1.00000D+00 | -1.08228D+00 |
| Q( 10) | 2 - 0 | 243.96 | -837.87 | 0.00000D+00 | 7.54712D-21 | 2.75605D-02 |
| Q( 10) | 2 - 1 | 670.02 | -411.81 | 0.00000D+00 | 2.00765D-24 | -1.16479D-01 |
| Q( 10) | 2 - 2 | 1081.83 | -0.00 | 0.00000D+00 | 1.00000D+00 | -1.08236D+00 |

| | | | | | | |
|---|---|---|---|---|---|---|
| Q( 11) | 2 - 0 | 249.22 | -837.74 | 0.00000D+00 | 7.30323D-21 | 2.75656D-02 |
| Q( 11) | 2 - 1 | 675.22 | -411.74 | 0.00000D+00 | 2.56019D-24 | -1.16434D-01 |
| Q( 11) | 2 - 2 | 1086.96 | -0.00 | 0.00000D+00 | 1.00000D+00 | -1.08244D+00 |
| Q( 12) | 2 - 0 | 254.95 | -837.60 | 0.00000D+00 | 7.04413D-21 | 2.75712D-02 |
| Q( 12) | 2 - 1 | 680.88 | -411.67 | 0.00000D+00 | 3.16533D-24 | -1.16385D-01 |
| Q( 12) | 2 - 2 | 1092.55 | -0.00 | 0.00000D+00 | 1.00000D+00 | -1.08253D+00 |
| Q( 13) | 2 - 0 | 261.16 | -837.44 | 0.00000D+00 | 6.76762D-21 | 2.75772D-02 |
| Q( 13) | 2 - 1 | 687.02 | -411.58 | 0.00000D+00 | 4.21663D-24 | -1.16331D-01 |
| Q( 13) | 2 - 2 | 1098.60 | -0.00 | 0.00000D+00 | 1.00000D+00 | -1.08263D+00 |
| Q( 14) | 2 - 0 | 267.85 | -837.27 | 0.00000D+00 | 9.84177D-21 | 2.75837D-02 |
| Q( 14) | 2 - 1 | 693.62 | -411.50 | 0.00000D+00 | 5.42880D-24 | -1.16274D-01 |
| Q( 14) | 2 - 2 | 1105.12 | -0.00 | 0.00000D+00 | 1.00000D+00 | -1.08273D+00 |
| Q( 15) | 2 - 0 | 275.02 | -837.09 | 0.00000D+00 | 9.45224D-21 | 2.75907D-02 |
| Q( 15) | 2 - 1 | 700.70 | -411.40 | 0.00000D+00 | 7.15909D-24 | -1.16212D-01 |
| Q( 15) | 2 - 2 | 1112.11 | -0.00 | 0.00000D+00 | 1.00000D+00 | -1.08284D+00 |
| Q( 16) | 2 - 0 | 282.66 | -836.89 | 0.00000D+00 | 9.04787D-21 | 2.75981D-02 |
| Q( 16) | 2 - 1 | 708.26 | -411.30 | 0.00000D+00 | 9.62874D-24 | -1.16146D-01 |
| Q( 16) | 2 - 2 | 1119.56 | -0.00 | 0.00000D+00 | 1.00000D+00 | -1.08296D+00 |
| Q( 17) | 2 - 0 | 290.78 | -836.69 | 0.00000D+00 | 8.62913D-21 | 2.76060D-02 |
| Q( 17) | 2 - 1 | 716.28 | -411.19 | 0.00000D+00 | 1.27997D-23 | -1.16076D-01 |
| Q( 17) | 2 - 2 | 1127.47 | -0.00 | 0.00000D+00 | 1.00000D+00 | -1.08309D+00 |
| Q( 18) | 2 - 0 | 299.38 | -836.47 | 0.00000D+00 | 8.19523D-21 | 2.76143D-02 |
| Q( 18) | 2 - 1 | 724.77 | -411.08 | 0.00000D+00 | 1.71313D-23 | -1.16002D-01 |
| Q( 18) | 2 - 2 | 1135.85 | -0.00 | 0.00000D+00 | 1.00000D+00 | -1.08323D+00 |
| Q( 19) | 2 - 0 | 308.46 | -836.24 | 0.00000D+00 | 7.75016D-21 | 2.76232D-02 |
| Q( 19) | 2 - 1 | 733.73 | -410.96 | 0.00000D+00 | 2.36640D-23 | -1.15923D-01 |
| Q( 19) | 2 - 2 | 1144.70 | -0.00 | 0.00000D+00 | 1.00000D+00 | -1.08337D+00 |
| Q( 20) | 2 - 0 | 318.01 | -836.00 | 0.00000D+00 | 7.26620D-21 | 2.76325D-02 |
| Q( 20) | 2 - 1 | 743.17 | -410.84 | 0.00000D+00 | 4.33047D-23 | -1.15841D-01 |

| | | | | | | | |
|---|---|---|---|---|---|---|---|
| Q( 20) | 2 - 2 | 1154.01 | -0.00 | 0.00000D+00 | 1.00000D+00 | -1.08352D+00 |
| Q( 0) | 3 - 0 | 217.67 | -1235.87 | 0.00000D+00 | 1.46417D-19 | 3.52712D-03 |
| Q( 0) | 3 - 1 | 644.05 | -809.49 | 0.00000D+00 | 2.02013D-26 | -4.83750D-02 |
| Q( 0) | 3 - 2 | 1056.21 | -397.33 | 0.00000D+00 | 5.89629D-24 | 1.25870D-01 |
| Q( 0) | 3 - 3 | 1453.54 | 0.00 | 0.00000D+00 | 1.00000D+00 | 1.07218D+00 |
| Q( 1) | 3 - 0 | 218.15 | -1235.85 | 0.00000D+00 | 5.77246D-20 | 3.52733D-03 |
| Q( 1) | 3 - 1 | 644.53 | -809.48 | 0.00000D+00 | 3.56646D-19 | -4.83758D-02 |
| Q( 1) | 3 - 2 | 1056.67 | -397.33 | 0.00000D+00 | 5.35275D-18 | 1.25864D-01 |
| Q( 1) | 3 - 3 | 1454.00 | -0.00 | 0.00000D+00 | 1.00000D+00 | 1.07218D+00 |
| Q( 2) | 3 - 0 | 219.10 | -1235.82 | 0.00000D+00 | 1.08228D-19 | 3.52776D-03 |
| Q( 2) | 3 - 1 | 645.47 | -809.45 | 0.00000D+00 | 8.91066D-18 | -4.83773D-02 |
| Q( 2) | 3 - 2 | 1057.61 | -397.31 | 0.00000D+00 | 1.33574D-16 | 1.25853D-01 |
| Q( 2) | 3 - 3 | 1454.92 | -0.00 | 0.00000D+00 | 1.00000D+00 | 1.07220D+00 |
| Q( 3) | 3 - 0 | 220.54 | -1235.76 | 0.00000D+00 | 1.46164D-19 | 3.52841D-03 |
| Q( 3) | 3 - 1 | 646.89 | -809.41 | 0.00000D+00 | 6.12058D-26 | -4.83795D-02 |
| Q( 3) | 3 - 2 | 1059.00 | -397.30 | 0.00000D+00 | 8.54063D-25 | 1.25835D-01 |
| Q( 3) | 3 - 3 | 1456.30 | 0.00 | 0.00000D+00 | 1.00000D+00 | 1.07221D+00 |
| Q( 4) | 3 - 0 | 222.45 | -1235.69 | 0.00000D+00 | 1.45960D-19 | 3.52927D-03 |
| Q( 4) | 3 - 1 | 648.78 | -809.36 | 0.00000D+00 | 6.25794D-26 | -4.83826D-02 |
| Q( 4) | 3 - 2 | 1060.87 | -397.27 | 0.00000D+00 | 8.92187D-25 | 1.25812D-01 |
| Q( 4) | 3 - 3 | 1458.14 | 0.00 | 0.00000D+00 | 1.00000D+00 | 1.07224D+00 |
| Q( 5) | 3 - 0 | 224.84 | -1235.59 | 0.00000D+00 | 1.45698D-19 | 3.53035D-03 |
| Q( 5) | 3 - 1 | 651.14 | -809.30 | 0.00000D+00 | 5.07548D-26 | -4.83863D-02 |
| Q( 5) | 3 - 2 | 1063.20 | -397.24 | 0.00000D+00 | 8.80036D-25 | 1.25783D-01 |
| Q( 5) | 3 - 3 | 1460.43 | 0.00 | 0.00000D+00 | 1.00000D+00 | 1.07226D+00 |
| Q( 6) | 3 - 0 | 227.71 | -1235.48 | 0.00000D+00 | 1.45380D-19 | 3.53164D-03 |
| Q( 6) | 3 - 1 | 653.97 | -809.22 | 0.00000D+00 | 5.82933D-26 | -4.83909D-02 |
| Q( 6) | 3 - 2 | 1065.99 | -397.20 | 0.00000D+00 | 9.56705D-25 | 1.25749D-01 |
| Q( 6) | 3 - 3 | 1463.19 | 0.00 | 0.00000D+00 | 1.00000D+00 | 1.07230D+00 |

| | | | | | | | |
|---|---|---|---|---|---|---|---|
| Q( 7) | 3 - 0 | 231.05 | -1235.35 | 0.00000D+00 | 1.45017D-19 | 3.53315D-03 |
| Q( 7) | 3 - 1 | 657.27 | -809.13 | 0.00000D+00 | 4.29145D-26 | -4.83962D-02 |
| Q( 7) | 3 - 2 | 1069.25 | -397.15 | 0.00000D+00 | 1.07440D-24 | 1.25708D-01 |
| Q( 7) | 3 - 3 | 1466.41 | 0.00 | 0.00000D+00 | 1.00000D+00 | 1.07234D+00 |
| Q( 8) | 3 - 0 | 234.88 | -1235.21 | 0.00000D+00 | 1.44597D-19 | 3.53487D-03 |
| Q( 8) | 3 - 1 | 661.05 | -809.03 | 0.00000D+00 | 3.71550D-26 | -4.84022D-02 |
| Q( 8) | 3 - 2 | 1072.98 | -397.10 | 0.00000D+00 | 1.14468D-24 | 1.25662D-01 |
| Q( 8) | 3 - 3 | 1470.09 | 0.00 | 0.00000D+00 | 1.00000D+00 | 1.07238D+00 |
| Q( 9) | 3 - 0 | 239.18 | -1235.04 | 0.00000D+00 | 1.44141D-19 | 3.53681D-03 |
| Q( 9) | 3 - 1 | 665.30 | -808.92 | 0.00000D+00 | 2.77025D-26 | -4.84090D-02 |
| Q( 9) | 3 - 2 | 1077.17 | -397.05 | 0.00000D+00 | 1.46404D-24 | 1.25610D-01 |
| Q( 9) | 3 - 3 | 1474.22 | 0.00 | 0.00000D+00 | 1.00000D+00 | 1.07243D+00 |
| Q( 10) | 3 - 0 | 243.96 | -1234.86 | 0.00000D+00 | 1.43613D-19 | 3.53897D-03 |
| Q( 10) | 3 - 1 | 670.02 | -808.79 | 0.00000D+00 | 1.55495D-26 | -4.84166D-02 |
| Q( 10) | 3 - 2 | 1081.83 | -396.98 | 0.00000D+00 | 1.79415D-24 | 1.25552D-01 |
| Q( 10) | 3 - 3 | 1478.82 | 0.00 | 0.00000D+00 | 1.00000D+00 | 1.07249D+00 |
| Q( 11) | 3 - 0 | 249.22 | -1234.65 | 0.00000D+00 | 1.43035D-19 | 3.54134D-03 |
| Q( 11) | 3 - 1 | 675.22 | -808.65 | 0.00000D+00 | 7.05609D-27 | -4.84249D-02 |
| Q( 11) | 3 - 2 | 1086.96 | -396.91 | 0.00000D+00 | 2.25886D-24 | 1.25488D-01 |
| Q( 11) | 3 - 3 | 1483.87 | 0.00 | 0.00000D+00 | 1.00000D+00 | 1.07255D+00 |
| Q( 12) | 3 - 0 | 254.95 | -1234.43 | 0.00000D+00 | 1.42430D-19 | 3.54393D-03 |
| Q( 12) | 3 - 1 | 680.88 | -808.50 | 0.00000D+00 | 1.77914D-28 | -4.84340D-02 |
| Q( 12) | 3 - 2 | 1092.55 | -396.84 | 0.00000D+00 | 3.05523D-24 | 1.25419D-01 |
| Q( 12) | 3 - 3 | 1489.38 | 0.00 | 0.00000D+00 | 1.00000D+00 | 1.07262D+00 |
| Q( 13) | 3 - 0 | 261.16 | -1234.19 | 0.00000D+00 | 1.41764D-19 | 3.54674D-03 |
| Q( 13) | 3 - 1 | 687.02 | -808.34 | 0.00000D+00 | 1.90044D-27 | -4.84438D-02 |
| Q( 13) | 3 - 2 | 1098.60 | -396.75 | 0.00000D+00 | 3.94513D-24 | 1.25343D-01 |
| Q( 13) | 3 - 3 | 1495.35 | 0.00 | 0.00000D+00 | 1.00000D+00 | 1.07269D+00 |
| Q( 14) | 3 - 0 | 267.85 | -1233.93 | 0.00000D+00 | 1.43334D-19 | 3.54977D-03 |

| | | | | | | | |
|---|---|---|---|---|---|---|---|
| Q( 14) | 3 - 1 | 693.62 | -808.16 | 0.00000D+00 | 9.59413D-26 | -4.84544D-02 |
| Q( 14) | 3 - 2 | 1105.12 | -396.66 | 0.00000D+00 | 9.22362D-24 | 1.25262D-01 |
| Q( 14) | 3 - 3 | 1501.78 | -0.00 | 0.00000D+00 | 1.00000D+00 | 1.07277D+00 |
| Q( 15) | 3 - 0 | 275.02 | -1233.66 | 0.00000D+00 | 1.42581D-19 | 3.55302D-03 |
| Q( 15) | 3 - 1 | 700.70 | -807.97 | 0.00000D+00 | 1.82156D-25 | -4.84658D-02 |
| Q( 15) | 3 - 2 | 1112.11 | -396.57 | 0.00000D+00 | 1.23481D-23 | 1.25175D-01 |
| Q( 15) | 3 - 3 | 1508.67 | -0.00 | 0.00000D+00 | 1.00000D+00 | 1.07285D+00 |
| Q( 16) | 3 - 0 | 282.66 | -1233.36 | 0.00000D+00 | 1.41798D-19 | 3.55649D-03 |
| Q( 16) | 3 - 1 | 708.26 | -807.77 | 0.00000D+00 | 3.35992D-25 | -4.84779D-02 |
| Q( 16) | 3 - 2 | 1119.56 | -396.47 | 0.00000D+00 | 1.66396D-23 | 1.25082D-01 |
| Q( 16) | 3 - 3 | 1516.02 | -0.00 | 0.00000D+00 | 1.00000D+00 | 1.07294D+00 |
| Q( 17) | 3 - 0 | 290.78 | -1233.04 | 0.00000D+00 | 1.40971D-19 | 3.56018D-03 |
| Q( 17) | 3 - 1 | 716.28 | -807.55 | 0.00000D+00 | 5.90228D-25 | -4.84908D-02 |
| Q( 17) | 3 - 2 | 1127.47 | -396.36 | 0.00000D+00 | 2.31180D-23 | 1.24983D-01 |
| Q( 17) | 3 - 3 | 1523.83 | -0.00 | 0.00000D+00 | 1.00000D+00 | 1.07303D+00 |
| Q( 18) | 3 - 0 | 299.38 | -1232.71 | 0.00000D+00 | 1.40083D-19 | 3.56409D-03 |
| Q( 18) | 3 - 1 | 724.77 | -807.32 | 0.00000D+00 | 1.00015D-24 | -4.85044D-02 |
| Q( 18) | 3 - 2 | 1135.85 | -396.24 | 0.00000D+00 | 3.16767D-23 | 1.24878D-01 |
| Q( 18) | 3 - 3 | 1532.09 | -0.00 | 0.00000D+00 | 1.00000D+00 | 1.07313D+00 |
| Q( 19) | 3 - 0 | 308.46 | -1232.36 | 0.00000D+00 | 1.39172D-19 | 3.56823D-03 |
| Q( 19) | 3 - 1 | 733.73 | -807.08 | 0.00000D+00 | 1.52924D-24 | -4.85188D-02 |
| Q( 19) | 3 - 2 | 1144.70 | -396.12 | 0.00000D+00 | 4.32014D-23 | 1.24767D-01 |
| Q( 19) | 3 - 3 | 1540.82 | -0.00 | 0.00000D+00 | 1.00000D+00 | 1.07324D+00 |
| Q( 20) | 3 - 0 | 318.01 | -1231.99 | 0.00000D+00 | 1.38216D-19 | 3.57259D-03 |
| Q( 20) | 3 - 1 | 743.17 | -806.83 | 0.00000D+00 | 2.32585D-24 | -4.85339D-02 |
| Q( 20) | 3 - 2 | 1154.01 | -395.99 | 0.00000D+00 | 5.95558D-23 | 1.24651D-01 |
| Q( 20) | 3 - 3 | 1550.00 | -0.00 | 0.00000D+00 | 1.00000D+00 | 1.07335D+00 |
| Q( 0) | 4 - 0 | 217.67 | -1619.92 | 0.00000D+00 | 4.15786D-22 | 2.35846D-04 |
| Q( 0) | 4 - 1 | 644.05 | -1193.54 | 0.00000D+00 | 2.23568D-25 | -7.78783D-03 |

| | | | | | | | |
|---|---|---|---|---|---|---|---|
| Q( 0) | 4 - 2 | 1056.21 | -781.38 | 0.00000D+00 | 3.18247D-24 | 6.89399D-02 |
| Q( 0) | 4 - 3 | 1453.54 | -384.05 | 0.00000D+00 | 1.11553D-22 | -1.23695D-01 |
| Q( 0) | 4 - 4 | 1837.59 | 0.00 | 0.00000D+00 | 1.00000D+00 | -1.05459D+00 |
| Q( 1) | 4 - 0 | 218.15 | -1619.89 | 0.00000D+00 | 6.87013D-21 | 2.35885D-04 |
| Q( 1) | 4 - 1 | 644.53 | -1193.52 | 0.00000D+00 | 6.43683D-20 | -7.78825D-03 |
| Q( 1) | 4 - 2 | 1056.67 | -781.37 | 0.00000D+00 | 6.47524D-19 | 6.89409D-02 |
| Q( 1) | 4 - 3 | 1454.00 | -384.04 | 0.00000D+00 | 7.52083D-18 | -1.23688D-01 |
| Q( 1) | 4 - 4 | 1838.04 | -0.00 | 0.00000D+00 | 1.00000D+00 | -1.05459D+00 |
| Q( 2) | 4 - 0 | 219.10 | -1619.85 | 0.00000D+00 | 1.10861D-19 | 2.35964D-04 |
| Q( 2) | 4 - 1 | 645.47 | -1193.48 | 0.00000D+00 | 1.60396D-18 | -7.78909D-03 |
| Q( 2) | 4 - 2 | 1057.61 | -781.34 | 0.00000D+00 | 1.61272D-17 | 6.89429D-02 |
| Q( 2) | 4 - 3 | 1454.92 | -384.03 | 0.00000D+00 | 1.86843D-16 | -1.23672D-01 |
| Q( 2) | 4 - 4 | 1838.95 | -0.00 | 0.00000D+00 | 1.00000D+00 | -1.05460D+00 |
| Q( 3) | 4 - 0 | 220.54 | -1619.77 | 0.00000D+00 | 3.92143D-22 | 2.36083D-04 |
| Q( 3) | 4 - 1 | 646.89 | -1193.42 | 0.00000D+00 | 3.12486D-26 | -7.79034D-03 |
| Q( 3) | 4 - 2 | 1059.00 | -781.31 | 0.00000D+00 | 7.69856D-26 | 6.89459D-02 |
| Q( 3) | 4 - 3 | 1456.30 | -384.01 | 0.00000D+00 | 1.26292D-23 | -1.23649D-01 |
| Q( 3) | 4 - 4 | 1840.31 | 0.00 | 0.00000D+00 | 1.00000D+00 | -1.05461D+00 |
| Q( 4) | 4 - 0 | 222.45 | -1619.67 | 0.00000D+00 | 3.80793D-22 | 2.36241D-04 |
| Q( 4) | 4 - 1 | 648.78 | -1193.35 | 0.00000D+00 | 3.06152D-26 | -7.79201D-03 |
| Q( 4) | 4 - 2 | 1060.87 | -781.25 | 0.00000D+00 | 8.24108D-26 | 6.89498D-02 |
| Q( 4) | 4 - 3 | 1458.14 | -383.98 | 0.00000D+00 | 1.24692D-23 | -1.23617D-01 |
| Q( 4) | 4 - 4 | 1842.12 | 0.00 | 0.00000D+00 | 1.00000D+00 | -1.05462D+00 |
| Q( 5) | 4 - 0 | 224.84 | -1619.55 | 0.00000D+00 | 3.67125D-22 | 2.36439D-04 |
| Q( 5) | 4 - 1 | 651.14 | -1193.25 | 0.00000D+00 | 2.71454D-26 | -7.79410D-03 |
| Q( 5) | 4 - 2 | 1063.20 | -781.19 | 0.00000D+00 | 6.39686D-26 | 6.89548D-02 |
| Q( 5) | 4 - 3 | 1460.43 | -383.95 | 0.00000D+00 | 1.29395D-23 | -1.23578D-01 |
| Q( 5) | 4 - 4 | 1844.39 | 0.00 | 0.00000D+00 | 1.00000D+00 | -1.05464D+00 |
| Q( 6) | 4 - 0 | 227.71 | -1619.40 | 0.00000D+00 | 3.51094D-22 | 2.36677D-04 |

| | | | | | | |
|---|---|---|---|---|---|---|
| Q( 6) | 4 - 1 | 653.97 | -1193.14 | 0.00000D+00 | 2.72201D-26 | -7.79661D-03 |
| Q( 6) | 4 - 2 | 1065.99 | -781.11 | 0.00000D+00 | 5.90331D-26 | 6.89608D-02 |
| Q( 6) | 4 - 3 | 1463.19 | -383.91 | 0.00000D+00 | 1.33035D-23 | -1.23532D-01 |
| Q( 6) | 4 - 4 | 1847.11 | 0.00 | 0.00000D+00 | 1.00000D+00 | -1.05466D+00 |
| Q( 7) | 4 - 0 | 231.05 | -1619.22 | 0.00000D+00 | 3.32855D-22 | 2.36955D-04 |
| Q( 7) | 4 - 1 | 657.27 | -1193.00 | 0.00000D+00 | 2.35404D-26 | -7.79954D-03 |
| Q( 7) | 4 - 2 | 1069.25 | -781.03 | 0.00000D+00 | 4.22021D-26 | 6.89677D-02 |
| Q( 7) | 4 - 3 | 1466.41 | -383.87 | 0.00000D+00 | 1.36400D-23 | -1.23477D-01 |
| Q( 7) | 4 - 4 | 1850.28 | 0.00 | 0.00000D+00 | 1.00000D+00 | -1.05468D+00 |
| Q( 8) | 4 - 0 | 234.88 | -1619.03 | 0.00000D+00 | 3.12531D-22 | 2.37274D-04 |
| Q( 8) | 4 - 1 | 661.05 | -1192.85 | 0.00000D+00 | 2.07181D-26 | -7.80288D-03 |
| Q( 8) | 4 - 2 | 1072.98 | -780.92 | 0.00000D+00 | 3.28096D-26 | 6.89756D-02 |
| Q( 8) | 4 - 3 | 1470.09 | -383.82 | 0.00000D+00 | 1.49853D-23 | -1.23414D-01 |
| Q( 8) | 4 - 4 | 1853.90 | 0.00 | 0.00000D+00 | 1.00000D+00 | -1.05471D+00 |
| Q( 9) | 4 - 0 | 239.18 | -1618.80 | 0.00000D+00 | 2.90862D-22 | 2.37632D-04 |
| Q( 9) | 4 - 1 | 665.30 | -1192.68 | 0.00000D+00 | 1.72834D-26 | -7.80665D-03 |
| Q( 9) | 4 - 2 | 1077.17 | -780.81 | 0.00000D+00 | 2.11853D-26 | 6.89846D-02 |
| Q( 9) | 4 - 3 | 1474.22 | -383.76 | 0.00000D+00 | 1.60518D-23 | -1.23344D-01 |
| Q( 9) | 4 - 4 | 1857.98 | 0.00 | 0.00000D+00 | 1.00000D+00 | -1.05474D+00 |
| Q( 10) | 4 - 0 | 243.96 | -1618.55 | 0.00000D+00 | 2.67485D-22 | 2.38032D-04 |
| Q( 10) | 4 - 1 | 670.02 | -1192.49 | 0.00000D+00 | 1.21947D-26 | -7.81083D-03 |
| Q( 10) | 4 - 2 | 1081.83 | -780.68 | 0.00000D+00 | 8.04317D-27 | 6.89945D-02 |
| Q( 10) | 4 - 3 | 1478.82 | -383.70 | 0.00000D+00 | 1.72798D-23 | -1.23266D-01 |
| Q( 10) | 4 - 4 | 1862.51 | 0.00 | 0.00000D+00 | 1.00000D+00 | -1.05477D+00 |
| Q( 11) | 4 - 0 | 249.22 | -1618.28 | 0.00000D+00 | 2.43176D-22 | 2.38472D-04 |
| Q( 11) | 4 - 1 | 675.22 | -1192.28 | 0.00000D+00 | 8.68619D-27 | -7.81543D-03 |
| Q( 11) | 4 - 2 | 1086.96 | -780.54 | 0.00000D+00 | 4.75409D-30 | 6.90054D-02 |
| Q( 11) | 4 - 3 | 1483.87 | -383.63 | 0.00000D+00 | 1.92597D-23 | -1.23180D-01 |
| Q( 11) | 4 - 4 | 1867.50 | 0.00 | 0.00000D+00 | 1.00000D+00 | -1.05480D+00 |

| | | | | | | | |
|---|---|---|---|---|---|---|---|
| Q( 12) | 4 - 0 | 254.95 | -1617.98 | 0.00000D+00 | 2.17965D-22 | 2.38953D-04 |
| Q( 12) | 4 - 1 | 680.88 | -1192.05 | 0.00000D+00 | 3.15979D-27 | -7.82046D-03 |
| Q( 12) | 4 - 2 | 1092.55 | -780.39 | 0.00000D+00 | 5.51176D-27 | 6.90173D-02 |
| Q( 12) | 4 - 3 | 1489.38 | -383.55 | 0.00000D+00 | 2.22667D-23 | -1.23086D-01 |
| Q( 12) | 4 - 4 | 1872.93 | 0.00 | 0.00000D+00 | 1.00000D+00 | -1.05484D+00 |
| Q( 13) | 4 - 0 | 261.16 | -1617.66 | 0.00000D+00 | 1.92503D-22 | 2.39476D-04 |
| Q( 13) | 4 - 1 | 687.02 | -1191.81 | 0.00000D+00 | 9.43597D-28 | -7.82590D-03 |
| Q( 13) | 4 - 2 | 1098.60 | -780.22 | 0.00000D+00 | 3.59298D-26 | 6.90302D-02 |
| Q( 13) | 4 - 3 | 1495.35 | -383.47 | 0.00000D+00 | 2.58892D-23 | -1.22984D-01 |
| Q( 13) | 4 - 4 | 1878.82 | 0.00 | 0.00000D+00 | 1.00000D+00 | -1.05489D+00 |
| Q( 14) | 4 - 0 | 267.85 | -1617.31 | 0.00000D+00 | 5.50425D-22 | 2.40040D-04 |
| Q( 14) | 4 - 1 | 693.62 | -1191.54 | 0.00000D+00 | 5.29053D-28 | -7.83176D-03 |
| Q( 14) | 4 - 2 | 1105.12 | -780.04 | 0.00000D+00 | 1.12370D-25 | 6.90442D-02 |
| Q( 14) | 4 - 3 | 1501.78 | -383.38 | 0.00000D+00 | 3.11169D-23 | -1.22874D-01 |
| Q( 14) | 4 - 4 | 1885.16 | 0.00 | 0.00000D+00 | 1.00000D+00 | -1.05493D+00 |
| Q( 15) | 4 - 0 | 275.02 | -1616.94 | 0.00000D+00 | 5.02090D-22 | 2.40647D-04 |
| Q( 15) | 4 - 1 | 700.70 | -1191.25 | 0.00000D+00 | 5.57038D-27 | -7.83804D-03 |
| Q( 15) | 4 - 2 | 1112.11 | -779.85 | 0.00000D+00 | 2.51086D-25 | 6.90590D-02 |
| Q( 15) | 4 - 3 | 1508.67 | -383.28 | 0.00000D+00 | 3.77430D-23 | -1.22756D-01 |
| Q( 15) | 4 - 4 | 1891.96 | 0.00 | 0.00000D+00 | 1.00000D+00 | -1.05498D+00 |
| Q( 16) | 4 - 0 | 282.66 | -1616.54 | 0.00000D+00 | 4.54354D-22 | 2.41296D-04 |
| Q( 16) | 4 - 1 | 708.26 | -1190.95 | 0.00000D+00 | 6.40311D-26 | -7.84474D-03 |
| Q( 16) | 4 - 2 | 1119.56 | -779.65 | 0.00000D+00 | 1.14345D-24 | 6.90749D-02 |
| Q( 16) | 4 - 3 | 1516.02 | -383.18 | 0.00000D+00 | 6.32578D-23 | -1.22630D-01 |
| Q( 16) | 4 - 4 | 1899.20 | 0.00 | 0.00000D+00 | 1.00000D+00 | -1.05503D+00 |
| Q( 17) | 4 - 0 | 290.78 | -1616.12 | 0.00000D+00 | 4.05753D-22 | 2.41988D-04 |
| Q( 17) | 4 - 1 | 716.28 | -1190.62 | 0.00000D+00 | 1.19234D-25 | -7.85187D-03 |
| Q( 17) | 4 - 2 | 1127.47 | -779.43 | 0.00000D+00 | 1.84712D-24 | 6.90918D-02 |
| Q( 17) | 4 - 3 | 1523.83 | -383.07 | 0.00000D+00 | 8.05245D-23 | -1.22497D-01 |

| | | | | | | |
|---|---|---|---|---|---|---|
| Q( 17) | 4 - 4 | 1906.90 | 0.00 | 0.00000D+00 | 1.00000D+00 | -1.05509D+00 |
| Q( 18) | 4 - 0 | 299.38 | -1615.67 | 0.00000D+00 | 3.57754D-22 | 2.42724D-04 |
| Q( 18) | 4 - 1 | 724.77 | -1190.28 | 0.00000D+00 | 2.06571D-25 | -7.85941D-03 |
| Q( 18) | 4 - 2 | 1135.85 | -779.20 | 0.00000D+00 | 2.91417D-24 | 6.91097D-02 |
| Q( 18) | 4 - 3 | 1532.09 | -382.96 | 0.00000D+00 | 1.02531D-22 | -1.22355D-01 |
| Q( 18) | 4 - 4 | 1915.05 | 0.00 | 0.00000D+00 | 1.00000D+00 | -1.05514D+00 |
| Q( 19) | 4 - 0 | 308.46 | -1615.19 | 0.00000D+00 | 3.10557D-22 | 2.43503D-04 |
| Q( 19) | 4 - 1 | 733.73 | -1189.92 | 0.00000D+00 | 3.26925D-25 | -7.86738D-03 |
| Q( 19) | 4 - 2 | 1144.70 | -778.95 | 0.00000D+00 | 4.37869D-24 | 6.91286D-02 |
| Q( 19) | 4 - 3 | 1540.82 | -382.83 | 0.00000D+00 | 1.30684D-22 | -1.22205D-01 |
| Q( 19) | 4 - 4 | 1923.65 | -0.00 | 0.00000D+00 | 1.00000D+00 | -1.05521D+00 |
| Q( 20) | 4 - 0 | 318.01 | -1614.70 | 0.00000D+00 | 2.65005D-22 | 2.44327D-04 |
| Q( 20) | 4 - 1 | 743.17 | -1189.53 | 0.00000D+00 | 5.06292D-25 | -7.87577D-03 |
| Q( 20) | 4 - 2 | 1154.01 | -778.70 | 0.00000D+00 | 6.48981D-24 | 6.91485D-02 |
| Q( 20) | 4 - 3 | 1550.00 | -382.71 | 0.00000D+00 | 1.68859D-22 | -1.22047D-01 |
| Q( 20) | 4 - 4 | 1932.70 | -0.00 | 0.00000D+00 | 1.00000D+00 | -1.05527D+00 |
| Q( 0) | 5 - 0 | 217.67 | -1989.15 | 0.00000D+00 | 4.17838D-20 | -2.89561D-05 |
| Q( 0) | 5 - 1 | 644.05 | -1562.77 | 0.00000D+00 | 2.68222D-26 | -8.75300D-04 |
| Q( 0) | 5 - 2 | 1056.21 | -1150.62 | 0.00000D+00 | 3.74376D-27 | 1.27735D-02 |
| Q( 0) | 5 - 3 | 1453.54 | -753.28 | 0.00000D+00 | 1.35289D-24 | -8.95869D-02 |
| Q( 0) | 5 - 4 | 1837.59 | -369.23 | 0.00000D+00 | 2.38547D-22 | 1.10530D-01 |
| Q( 0) | 5 - 5 | 2206.82 | 0.00 | 0.00000D+00 | 1.00000D+00 | 1.02931D+00 |
| Q( 1) | 5 - 0 | 218.15 | -1989.12 | 0.00000D+00 | 5.69743D-20 | -2.89676D-05 |
| Q( 1) | 5 - 1 | 644.53 | -1562.74 | 0.00000D+00 | 1.93932D-20 | -8.75464D-04 |
| Q( 1) | 5 - 2 | 1056.67 | -1150.60 | 0.00000D+00 | 1.76464D-19 | 1.27741D-02 |
| Q( 1) | 5 - 3 | 1454.00 | -753.27 | 0.00000D+00 | 1.33224D-18 | -8.95882D-02 |
| Q( 1) | 5 - 4 | 1838.04 | -369.23 | 0.00000D+00 | 1.34367D-17 | 1.10519D-01 |
| Q( 1) | 5 - 5 | 2207.27 | -0.00 | 0.00000D+00 | 1.00000D+00 | 1.02931D+00 |
| Q( 2) | 5 - 0 | 219.10 | -1989.06 | 0.00000D+00 | 1.41314D-19 | -2.89907D-05 |

| | | | | | | | |
|---|---|---|---|---|---|---|---|
| Q( 2) | 5 - 1 | 645.47 | -1562.69 | 0.00000D+00 | 4.83809D-19 | -8.75793D-04 |
| Q( 2) | 5 - 2 | 1057.61 | -1150.55 | 0.00000D+00 | 4.41177D-18 | 1.27753D-02 |
| Q( 2) | 5 - 3 | 1454.92 | -753.24 | 0.00000D+00 | 3.33567D-17 | -8.95907D-02 |
| Q( 2) | 5 - 4 | 1838.95 | -369.21 | 0.00000D+00 | 3.33660D-16 | 1.10498D-01 |
| Q( 2) | 5 - 5 | 2208.16 | -0.00 | 0.00000D+00 | 1.00000D+00 | 1.02931D+00 |
| Q( 3) | 5 - 0 | 220.54 | -1988.96 | 0.00000D+00 | 4.16532D-20 | -2.90253D-05 |
| Q( 3) | 5 - 1 | 646.89 | -1562.61 | 0.00000D+00 | 2.23994D-26 | -8.76287D-04 |
| Q( 3) | 5 - 2 | 1059.00 | -1150.49 | 0.00000D+00 | 7.89045D-27 | 1.27771D-02 |
| Q( 3) | 5 - 3 | 1456.30 | -753.20 | 0.00000D+00 | 1.50476D-24 | -8.95945D-02 |
| Q( 3) | 5 - 4 | 1840.31 | -369.19 | 0.00000D+00 | 2.30847D-22 | 1.10466D-01 |
| Q( 3) | 5 - 5 | 2209.50 | 0.00 | 0.00000D+00 | 1.00000D+00 | 1.02931D+00 |
| Q( 4) | 5 - 0 | 222.45 | -1988.83 | 0.00000D+00 | 4.15691D-20 | -2.90715D-05 |
| Q( 4) | 5 - 1 | 648.78 | -1562.50 | 0.00000D+00 | 2.40366D-26 | -8.76945D-04 |
| Q( 4) | 5 - 2 | 1060.87 | -1150.41 | 0.00000D+00 | 8.46255D-27 | 1.27795D-02 |
| Q( 4) | 5 - 3 | 1458.14 | -753.14 | 0.00000D+00 | 1.49066D-24 | -8.95996D-02 |
| Q( 4) | 5 - 4 | 1842.12 | -369.16 | 0.00000D+00 | 2.30973D-22 | 1.10423D-01 |
| Q( 4) | 5 - 5 | 2211.28 | 0.00 | 0.00000D+00 | 1.00000D+00 | 1.02931D+00 |
| Q( 5) | 5 - 0 | 224.84 | -1988.67 | 0.00000D+00 | 4.14642D-20 | -2.91293D-05 |
| Q( 5) | 5 - 1 | 651.14 | -1562.37 | 0.00000D+00 | 2.41318D-26 | -8.77768D-04 |
| Q( 5) | 5 - 2 | 1063.20 | -1150.31 | 0.00000D+00 | 4.69830D-27 | 1.27826D-02 |
| Q( 5) | 5 - 3 | 1460.43 | -753.07 | 0.00000D+00 | 1.40527D-24 | -8.96060D-02 |
| Q( 5) | 5 - 4 | 1844.39 | -369.12 | 0.00000D+00 | 2.32670D-22 | 1.10370D-01 |
| Q( 5) | 5 - 5 | 2213.51 | 0.00 | 0.00000D+00 | 1.00000D+00 | 1.02931D+00 |
| Q( 6) | 5 - 0 | 227.71 | -1988.47 | 0.00000D+00 | 4.13363D-20 | -2.91987D-05 |
| Q( 6) | 5 - 1 | 653.97 | -1562.21 | 0.00000D+00 | 2.64917D-26 | -8.78756D-04 |
| Q( 6) | 5 - 2 | 1065.99 | -1150.19 | 0.00000D+00 | 3.56230D-27 | 1.27863D-02 |
| Q( 6) | 5 - 3 | 1463.19 | -752.99 | 0.00000D+00 | 1.29767D-24 | -8.96136D-02 |
| Q( 6) | 5 - 4 | 1847.11 | -369.07 | 0.00000D+00 | 2.35996D-22 | 1.10306D-01 |
| Q( 6) | 5 - 5 | 2216.18 | -0.00 | 0.00000D+00 | 1.00000D+00 | 1.02932D+00 |

| | | | | | | |
|---|---|---|---|---|---|---|
| Q( 7) | 5 - 0 | 231.05 | -1988.24 | 0.00000D+00 | 4.11915D-20 | -2.92798D-05 |
| Q( 7) | 5 - 1 | 657.27 | -1562.02 | 0.00000D+00 | 2.81986D-26 | -8.79910D-04 |
| Q( 7) | 5 - 2 | 1069.25 | -1150.04 | 0.00000D+00 | 1.43133D-27 | 1.27905D-02 |
| Q( 7) | 5 - 3 | 1466.41 | -752.89 | 0.00000D+00 | 1.15334D-24 | -8.96225D-02 |
| Q( 7) | 5 - 4 | 1850.28 | -369.02 | 0.00000D+00 | 2.41076D-22 | 1.10231D-01 |
| Q( 7) | 5 - 5 | 2219.30 | -0.00 | 0.00000D+00 | 1.00000D+00 | 1.02932D+00 |
| Q( 8) | 5 - 0 | 234.88 | -1987.98 | 0.00000D+00 | 4.10246D-20 | -2.93726D-05 |
| Q( 8) | 5 - 1 | 661.05 | -1561.81 | 0.00000D+00 | 3.15022D-26 | -8.81230D-04 |
| Q( 8) | 5 - 2 | 1072.98 | -1149.88 | 0.00000D+00 | 1.08976D-28 | 1.27954D-02 |
| Q( 8) | 5 - 3 | 1470.09 | -752.78 | 0.00000D+00 | 1.12259D-24 | -8.96327D-02 |
| Q( 8) | 5 - 4 | 1853.90 | -368.96 | 0.00000D+00 | 2.46286D-22 | 1.10146D-01 |
| Q( 8) | 5 - 5 | 2222.86 | -0.00 | 0.00000D+00 | 1.00000D+00 | 1.02932D+00 |
| Q( 9) | 5 - 0 | 239.18 | -1987.69 | 0.00000D+00 | 4.08409D-20 | -2.94771D-05 |
| Q( 9) | 5 - 1 | 665.30 | -1561.57 | 0.00000D+00 | 3.59319D-26 | -8.82717D-04 |
| Q( 9) | 5 - 2 | 1077.17 | -1149.70 | 0.00000D+00 | 5.26611D-28 | 1.28009D-02 |
| Q( 9) | 5 - 3 | 1474.22 | -752.65 | 0.00000D+00 | 8.93475D-25 | -8.96441D-02 |
| Q( 9) | 5 - 4 | 1857.98 | -368.89 | 0.00000D+00 | 2.56182D-22 | 1.10049D-01 |
| Q( 9) | 5 - 5 | 2226.87 | -0.00 | 0.00000D+00 | 1.00000D+00 | 1.02932D+00 |
| Q( 10) | 5 - 0 | 243.96 | -1987.36 | 0.00000D+00 | 4.06311D-20 | -2.95934D-05 |
| Q( 10) | 5 - 1 | 670.02 | -1561.30 | 0.00000D+00 | 4.09330D-26 | -8.84371D-04 |
| Q( 10) | 5 - 2 | 1081.83 | -1149.49 | 0.00000D+00 | 4.54539D-27 | 1.28070D-02 |
| Q( 10) | 5 - 3 | 1478.82 | -752.51 | 0.00000D+00 | 6.70901D-25 | -8.96568D-02 |
| Q( 10) | 5 - 4 | 1862.51 | -368.81 | 0.00000D+00 | 2.68009D-22 | 1.09942D-01 |
| Q( 10) | 5 - 5 | 2231.32 | -0.00 | 0.00000D+00 | 1.00000D+00 | 1.02933D+00 |
| Q( 11) | 5 - 0 | 249.22 | -1987.01 | 0.00000D+00 | 4.04034D-20 | -2.97216D-05 |
| Q( 11) | 5 - 1 | 675.22 | -1561.01 | 0.00000D+00 | 4.77484D-26 | -8.86193D-04 |
| Q( 11) | 5 - 2 | 1086.96 | -1149.27 | 0.00000D+00 | 1.53599D-26 | 1.28137D-02 |
| Q( 11) | 5 - 3 | 1483.87 | -752.35 | 0.00000D+00 | 4.24509D-25 | -8.96708D-02 |
| Q( 11) | 5 - 4 | 1867.50 | -368.73 | 0.00000D+00 | 2.86532D-22 | 1.09825D-01 |

| | | | | | | |
|---|---|---|---|---|---|---|
| Q( 11) | 5 - 5 | 2236.22 | -0.00 | 0.00000D+00 | 1.00000D+00 | 1.02933D+00 |
| Q( 12) | 5 - 0 | 254.95 | -1986.62 | 0.00000D+00 | 4.01610D-20 | -2.98616D-05 |
| Q( 12) | 5 - 1 | 680.88 | -1560.69 | 0.00000D+00 | 5.64619D-26 | -8.88182D-04 |
| Q( 12) | 5 - 2 | 1092.55 | -1149.02 | 0.00000D+00 | 4.00227D-26 | 1.28211D-02 |
| Q( 12) | 5 - 3 | 1489.38 | -752.18 | 0.00000D+00 | 2.03872D-25 | -8.96861D-02 |
| Q( 12) | 5 - 4 | 1872.93 | -368.63 | 0.00000D+00 | 3.06848D-22 | 1.09696D-01 |
| Q( 12) | 5 - 5 | 2241.57 | -0.00 | 0.00000D+00 | 1.00000D+00 | 1.02933D+00 |
| Q( 13) | 5 - 0 | 261.16 | -1986.19 | 0.00000D+00 | 3.98988D-20 | -3.00137D-05 |
| Q( 13) | 5 - 1 | 687.02 | -1560.34 | 0.00000D+00 | 7.40603D-26 | -8.90341D-04 |
| Q( 13) | 5 - 2 | 1098.60 | -1148.75 | 0.00000D+00 | 8.35399D-26 | 1.28290D-02 |
| Q( 13) | 5 - 3 | 1495.35 | -752.00 | 0.00000D+00 | 3.69662D-26 | -8.97026D-02 |
| Q( 13) | 5 - 4 | 1878.82 | -368.53 | 0.00000D+00 | 3.32579D-22 | 1.09557D-01 |
| Q( 13) | 5 - 5 | 2247.35 | -0.00 | 0.00000D+00 | 1.00000D+00 | 1.02934D+00 |
| Q( 14) | 5 - 0 | 267.85 | -1985.73 | 0.00000D+00 | 4.11920D-20 | -3.01778D-05 |
| Q( 14) | 5 - 1 | 693.62 | -1559.96 | 0.00000D+00 | 9.95841D-26 | -8.92670D-04 |
| Q( 14) | 5 - 2 | 1105.12 | -1148.47 | 0.00000D+00 | 1.57939D-25 | 1.28376D-02 |
| Q( 14) | 5 - 3 | 1501.78 | -751.80 | 0.00000D+00 | 1.37000D-26 | -8.97204D-02 |
| Q( 14) | 5 - 4 | 1885.16 | -368.42 | 0.00000D+00 | 3.65517D-22 | 1.09406D-01 |
| Q( 14) | 5 - 5 | 2253.59 | -0.00 | 0.00000D+00 | 1.00000D+00 | 1.02934D+00 |
| Q( 15) | 5 - 0 | 275.02 | -1985.24 | 0.00000D+00 | 4.08956D-20 | -3.03540D-05 |
| Q( 15) | 5 - 1 | 700.70 | -1559.56 | 0.00000D+00 | 1.29007D-25 | -8.95170D-04 |
| Q( 15) | 5 - 2 | 1112.11 | -1148.16 | 0.00000D+00 | 2.82791D-25 | 1.28468D-02 |
| Q( 15) | 5 - 3 | 1508.67 | -751.59 | 0.00000D+00 | 2.33955D-25 | -8.97395D-02 |
| Q( 15) | 5 - 4 | 1891.96 | -368.31 | 0.00000D+00 | 4.08879D-22 | 1.09245D-01 |
| Q( 15) | 5 - 5 | 2260.26 | -0.00 | 0.00000D+00 | 1.00000D+00 | 1.02934D+00 |
| Q( 16) | 5 - 0 | 282.66 | -1984.72 | 0.00000D+00 | 4.05861D-20 | -3.05424D-05 |
| Q( 16) | 5 - 1 | 708.26 | -1559.13 | 0.00000D+00 | 1.70643D-25 | -8.97841D-04 |
| Q( 16) | 5 - 2 | 1119.56 | -1147.83 | 0.00000D+00 | 4.84777D-25 | 1.28567D-02 |
| Q( 16) | 5 - 3 | 1516.02 | -751.36 | 0.00000D+00 | 8.78499D-25 | -8.97599D-02 |

| | | | | | | |
|---|---|---|---|---|---|---|
| Q( 16) | 5 - 4 | 1899.20 | -368.18 | 0.00000D+00 | 4.64122D-22 | 1.09073D-01 |
| Q( 16) | 5 - 5 | 2267.39 | -0.00 | 0.00000D+00 | 1.00000D+00 | 1.02935D+00 |
| Q( 17) | 5 - 0 | 290.78 | -1984.17 | 0.00000D+00 | 4.02612D-20 | -3.07430D-05 |
| Q( 17) | 5 - 1 | 716.28 | -1558.67 | 0.00000D+00 | 2.19896D-25 | -9.00685D-04 |
| Q( 17) | 5 - 2 | 1127.47 | -1147.48 | 0.00000D+00 | 7.80661D-25 | 1.28671D-02 |
| Q( 17) | 5 - 3 | 1523.83 | -751.12 | 0.00000D+00 | 2.15633D-24 | -8.97816D-02 |
| Q( 17) | 5 - 4 | 1906.90 | -368.05 | 0.00000D+00 | 5.33344D-22 | 1.08890D-01 |
| Q( 17) | 5 - 5 | 2274.95 | -0.00 | 0.00000D+00 | 1.00000D+00 | 1.02935D+00 |
| Q( 18) | 5 - 0 | 299.38 | -1983.58 | 0.00000D+00 | 3.99162D-20 | -3.09560D-05 |
| Q( 18) | 5 - 1 | 724.77 | -1558.19 | 0.00000D+00 | 2.89878D-25 | -9.03703D-04 |
| Q( 18) | 5 - 2 | 1135.85 | -1147.11 | 0.00000D+00 | 1.21729D-24 | 1.28782D-02 |
| Q( 18) | 5 - 3 | 1532.09 | -750.87 | 0.00000D+00 | 4.23197D-24 | -8.98045D-02 |
| Q( 18) | 5 - 4 | 1915.05 | -367.91 | 0.00000D+00 | 6.24957D-22 | 1.08695D-01 |
| Q( 18) | 5 - 5 | 2282.96 | -0.00 | 0.00000D+00 | 1.00000D+00 | 1.02935D+00 |
| Q( 19) | 5 - 0 | 308.46 | -1982.96 | 0.00000D+00 | 3.95614D-20 | -3.11815D-05 |
| Q( 19) | 5 - 1 | 733.73 | -1557.68 | 0.00000D+00 | 3.95030D-25 | -9.06895D-04 |
| Q( 19) | 5 - 2 | 1144.70 | -1146.72 | 0.00000D+00 | 1.87015D-24 | 1.28899D-02 |
| Q( 19) | 5 - 3 | 1540.82 | -750.60 | 0.00000D+00 | 7.78906D-24 | -8.98287D-02 |
| Q( 19) | 5 - 4 | 1923.65 | -367.76 | 0.00000D+00 | 7.51221D-22 | 1.08490D-01 |
| Q( 19) | 5 - 5 | 2291.41 | -0.00 | 0.00000D+00 | 1.00000D+00 | 1.02935D+00 |
| Q( 20) | 5 - 0 | 318.01 | -1982.30 | 0.00000D+00 | 3.91912D-20 | -3.14195D-05 |
| Q( 20) | 5 - 1 | 743.17 | -1557.14 | 0.00000D+00 | 5.32986D-25 | -9.10263D-04 |
| Q( 20) | 5 - 2 | 1154.01 | -1146.30 | 0.00000D+00 | 2.82034D-24 | 1.29023D-02 |
| Q( 20) | 5 - 3 | 1550.00 | -750.31 | 0.00000D+00 | 1.32927D-23 | -8.98542D-02 |
| Q( 20) | 5 - 4 | 1932.70 | -367.60 | 0.00000D+00 | 9.01714D-22 | 1.08273D-01 |
| Q( 20) | 5 - 5 | 2300.31 | -0.00 | 0.00000D+00 | 1.00000D+00 | 1.02936D+00 |
