# Supplementary material for: Ab initio spectroscopic studies of AlF and AlCl molecules
Source: arXiv:2303.08681 source file (2023-03-15)
Supplement: Supplementary file 3 [file AlCl_singlet_sigma_-_S16.pdf]

# AlCl $X^1\Sigma$: Rotational parameters

Note that (v',J') & (v",J") strictly label the upper and lower levels, resp., and E(lower)=E"

but E(2)-E(1) is: (energy of State-2 level) - (energy of State-1 level)

In the following table, E is expressed in $cm^{-1}$, A in $s^{-1}$ and transition dipole moment in debye.

| dJ(J") | Band v' v" | E(lower) | E(2)-E(1) | A(Einstein) | F-C Factor | <v'j'\|M\|v"j"> |
|---|---|---|---|---|---|---|
| ------ | ------- | -------- | -------- | ----------- | ----------- | ----------- |
| R( 0) | 0 - 0 | 240.35 | -0.48 | 3.05340D-08 | 1.00000D+00 | -1.62109D+00 |
| R( 1) | 0 - 0 | 240.84 | -0.96 | 2.93140D-07 | 1.00000D+00 | -1.62113D+00 |
| R( 2) | 0 - 0 | 241.80 | -1.44 | 1.06006D-06 | 1.00000D+00 | -1.62121D+00 |
| R( 3) | 0 - 0 | 243.24 | -1.92 | 2.60602D-06 | 1.00000D+00 | -1.62131D+00 |
| R( 4) | 0 - 0 | 245.16 | -2.40 | 5.20612D-06 | 1.00000D+00 | -1.62144D+00 |
| R( 5) | 0 - 0 | 247.57 | -2.88 | 9.13577D-06 | 1.00000D+00 | -1.62160D+00 |
| R( 6) | 0 - 0 | 250.45 | -3.37 | 1.46707D-05 | 1.00000D+00 | -1.62179D+00 |
| R( 7) | 0 - 0 | 253.82 | -3.85 | 2.20871D-05 | 1.00000D+00 | -1.62201D+00 |
| R( 8) | 0 - 0 | 257.66 | -4.33 | 3.16616D-05 | 1.00000D+00 | -1.62225D+00 |
| R( 9) | 0 - 0 | 261.99 | -4.81 | 4.36712D-05 | 1.00000D+00 | -1.62253D+00 |
| R( 10) | 0 - 0 | 266.80 | -5.29 | 5.83937D-05 | 1.00000D+00 | -1.62284D+00 |
| R( 11) | 0 - 0 | 272.08 | -5.77 | 7.61073D-05 | 1.00000D+00 | -1.62317D+00 |
| R( 12) | 0 - 0 | 277.85 | -6.25 | 9.70913D-05 | 1.00000D+00 | -1.62353D+00 |
| R( 13) | 0 - 0 | 284.10 | -6.73 | 1.21625D-04 | 1.00000D+00 | -1.62393D+00 |
| R( 14) | 0 - 0 | 290.83 | -7.21 | 1.49990D-04 | 1.00000D+00 | -1.62435D+00 |
| R( 15) | 0 - 0 | 298.04 | -7.69 | 1.82468D-04 | 9.99999D-01 | -1.62480D+00 |
| R( 16) | 0 - 0 | 305.73 | -8.17 | 2.19340D-04 | 9.99999D-01 | -1.62528D+00 |
| R( 17) | 0 - 0 | 313.89 | -8.65 | 2.60891D-04 | 9.99999D-01 | -1.62579D+00 |
| R( 18) | 0 - 0 | 322.54 | -9.13 | 3.07405D-04 | 9.99999D-01 | -1.62633D+00 |

| | | | | | | | |
|---|---|---|---|---|---|---|---|
| R( 19) | 0 - 0 | 331.67 | -9.61 | 3.59168D-04 | 9.99999D-01 | -1.62690D+00 |
| P( 1) | 1 - 0 | 240.84 | -477.18 | 3.56474D+00 | 2.01409D-09 | 3.23441D-01 |
| R( 0) | 1 - 0 | 240.35 | -478.13 | 1.19432D+00 | 2.01512D-09 | 3.23292D-01 |
| P( 2) | 1 - 0 | 241.80 | -476.69 | 2.37039D+00 | 8.05726D-09 | 3.23517D-01 |
| R( 0) | 1 - 1 | 718.01 | -0.48 | 3.26613D-08 | 1.00000D+00 | 1.69228D+00 |
| R( 1) | 1 - 0 | 240.84 | -478.61 | 1.43682D+00 | 8.06006D-09 | 3.23220D-01 |
| P( 3) | 1 - 0 | 243.24 | -476.21 | 2.12785D+00 | 1.81290D-08 | 3.23595D-01 |
| R( 1) | 1 - 1 | 718.49 | -0.96 | 3.13562D-07 | 1.00000D+00 | 1.69233D+00 |
| R( 2) | 1 - 0 | 241.80 | -479.08 | 1.54333D+00 | 1.81315D-08 | 3.23149D-01 |
| P( 4) | 1 - 0 | 245.16 | -475.72 | 2.02127D+00 | 3.22349D-08 | 3.23674D-01 |
| R( 2) | 1 - 1 | 719.45 | -1.43 | 1.13390D-06 | 1.00000D+00 | 1.69240D+00 |
| R( 3) | 1 - 0 | 243.24 | -479.55 | 1.60451D+00 | 3.22344D-08 | 3.23080D-01 |
| P( 5) | 1 - 0 | 247.57 | -475.22 | 1.96000D+00 | 5.03687D-08 | 3.23755D-01 |
| R( 3) | 1 - 1 | 720.88 | -1.91 | 2.78753D-06 | 1.00000D+00 | 1.69250D+00 |
| R( 4) | 1 - 0 | 245.16 | -480.02 | 1.64507D+00 | 5.03675D-08 | 3.23012D-01 |
| P( 6) | 1 - 0 | 250.45 | -474.73 | 1.91932D+00 | 7.25338D-08 | 3.23837D-01 |
| R( 4) | 1 - 1 | 722.79 | -2.39 | 5.56871D-06 | 1.00000D+00 | 1.69264D+00 |
| R( 5) | 1 - 0 | 247.57 | -480.48 | 1.67453D+00 | 7.25316D-08 | 3.22946D-01 |
| P( 7) | 1 - 0 | 253.82 | -474.23 | 1.88973D+00 | 9.87312D-08 | 3.23921D-01 |
| R( 5) | 1 - 1 | 725.18 | -2.87 | 9.77199D-06 | 1.00000D+00 | 1.69280D+00 |
| R( 6) | 1 - 0 | 250.45 | -480.94 | 1.69731D+00 | 9.87275D-08 | 3.22880D-01 |
| P( 8) | 1 - 0 | 257.66 | -473.73 | 1.86678D+00 | 1.28962D-07 | 3.24006D-01 |
| R( 6) | 1 - 1 | 728.05 | -3.34 | 1.56923D-05 | 1.00000D+00 | 1.69299D+00 |
| R( 7) | 1 - 0 | 253.82 | -481.40 | 1.71578D+00 | 1.28956D-07 | 3.22817D-01 |
| P( 9) | 1 - 0 | 261.99 | -473.22 | 1.84812D+00 | 1.63227D-07 | 3.24092D-01 |
| R( 7) | 1 - 1 | 731.39 | -3.82 | 2.36249D-05 | 1.00000D+00 | 1.69321D+00 |
| R( 8) | 1 - 0 | 257.66 | -481.85 | 1.73129D+00 | 1.63219D-07 | 3.22754D-01 |
| P( 10) | 1 - 0 | 266.80 | -472.72 | 1.83241D+00 | 2.01528D-07 | 3.24180D-01 |
| R( 8) | 1 - 1 | 735.21 | -4.30 | 3.38656D-05 | 1.00000D+00 | 1.69345D+00 |

| | | | | | | | |
|---|---|---|---|---|---|---|---|
| R( 9) | 1 - 0 | 261.99 | -482.30 | 1.74468D+00 | 2.01517D-07 | 3.22693D-01 |
| P( 11) | 1 - 0 | 272.08 | -472.21 | 1.81878D+00 | 2.43867D-07 | 3.24269D-01 |
| R( 9) | 1 - 1 | 739.51 | -4.78 | 4.67107D-05 | 9.99999D-01 | 1.69373D+00 |
| R( 10) | 1 - 0 | 266.80 | -482.75 | 1.75650D+00 | 2.43851D-07 | 3.22634D-01 |
| P( 12) | 1 - 0 | 277.85 | -471.69 | 1.80671D+00 | 2.90245D-07 | 3.24360D-01 |
| R( 10) | 1 - 1 | 744.29 | -5.25 | 6.24570D-05 | 9.99999D-01 | 1.69404D+00 |
| R( 11) | 1 - 0 | 272.08 | -483.19 | 1.76712D+00 | 2.90224D-07 | 3.22575D-01 |
| P( 13) | 1 - 0 | 284.10 | -471.18 | 1.79580D+00 | 3.40664D-07 | 3.24453D-01 |
| R( 11) | 1 - 1 | 749.54 | -5.73 | 8.14022D-05 | 9.99999D-01 | 1.69438D+00 |
| R( 12) | 1 - 0 | 277.85 | -483.63 | 1.77682D+00 | 3.40638D-07 | 3.22518D-01 |
| P( 14) | 1 - 0 | 290.83 | -470.66 | 1.78581D+00 | 3.95126D-07 | 3.24546D-01 |
| R( 12) | 1 - 1 | 755.28 | -6.21 | 1.03844D-04 | 9.99999D-01 | 1.69474D+00 |
| R( 13) | 1 - 0 | 284.10 | -484.07 | 1.78576D+00 | 3.95093D-07 | 3.22463D-01 |
| P( 15) | 1 - 0 | 298.04 | -470.14 | 1.77654D+00 | 4.53633D-07 | 3.24642D-01 |
| R( 13) | 1 - 1 | 761.49 | -6.69 | 1.30083D-04 | 9.99999D-01 | 1.69514D+00 |
| R( 14) | 1 - 0 | 290.83 | -484.51 | 1.79411D+00 | 4.53593D-07 | 3.22408D-01 |
| P( 16) | 1 - 0 | 305.73 | -469.61 | 1.76784D+00 | 5.16189D-07 | 3.24738D-01 |
| R( 14) | 1 - 1 | 768.17 | -7.16 | 1.60417D-04 | 9.99999D-01 | 1.69556D+00 |
| R( 15) | 1 - 0 | 298.04 | -484.94 | 1.80196D+00 | 5.16139D-07 | 3.22356D-01 |
| P( 17) | 1 - 0 | 313.89 | -469.08 | 1.75962D+00 | 5.82794D-07 | 3.24837D-01 |
| R( 15) | 1 - 1 | 775.34 | -7.64 | 1.95148D-04 | 9.99998D-01 | 1.69602D+00 |
| R( 16) | 1 - 0 | 305.73 | -485.37 | 1.80940D+00 | 5.82735D-07 | 3.22304D-01 |
| P( 18) | 1 - 0 | 322.54 | -468.55 | 1.75178D+00 | 6.53452D-07 | 3.24936D-01 |
| R( 16) | 1 - 1 | 782.98 | -8.12 | 2.34578D-04 | 9.99998D-01 | 1.69650D+00 |
| R( 17) | 1 - 0 | 313.89 | -485.80 | 1.81649D+00 | 6.53382D-07 | 3.22254D-01 |
| P( 19) | 1 - 0 | 331.67 | -468.02 | 1.74427D+00 | 7.28166D-07 | 3.25037D-01 |
| R( 17) | 1 - 1 | 791.10 | -8.60 | 2.79010D-04 | 9.99998D-01 | 1.69702D+00 |
| R( 18) | 1 - 0 | 322.54 | -486.22 | 1.82329D+00 | 7.28083D-07 | 3.22205D-01 |
| P( 20) | 1 - 0 | 341.28 | -467.48 | 1.73704D+00 | 8.06939D-07 | 3.25140D-01 |

| | | | | | | | |
|---|---|---|---|---|---|---|---|
| R( 18) | 1 - 1 | 799.69 | -9.07 | 3.28747D-04 | 9.99998D-01 | 1.69756D+00 |
| R( 19) | 1 - 0 | 331.67 | -486.64 | 1.82983D+00 | 8.06842D-07 | 3.22157D-01 |
| P( 21) | 1 - 0 | 351.37 | -466.94 | 1.73003D+00 | 8.89774D-07 | 3.25244D-01 |
| R( 19) | 1 - 1 | 808.76 | -9.55 | 3.84095D-04 | 9.99998D-01 | 1.69813D+00 |
| P( 1) | 2 - 0 | 240.84 | -951.11 | 4.18033D-02 | 4.59627D-12 | 1.24467D-02 |
| P( 1) | 2 - 1 | 718.49 | -473.46 | 6.98710D+00 | 4.01979D-09 | -4.58164D-01 |
| R( 0) | 2 - 0 | 240.35 | -952.07 | 1.40525D-02 | 4.60896D-12 | 1.24805D-02 |
| P( 2) | 2 - 0 | 241.80 | -950.63 | 2.77512D-02 | 1.83589D-11 | 1.24300D-02 |
| R( 0) | 2 - 1 | 718.01 | -474.41 | 2.34086D+00 | 4.02390D-09 | -4.57944D-01 |
| P( 2) | 2 - 1 | 719.45 | -472.98 | 4.64617D+00 | 1.60833D-08 | -4.58277D-01 |
| R( 0) | 2 - 2 | 1191.95 | -0.47 | 3.51274D-08 | 1.00000D+00 | -1.77596D+00 |
| R( 1) | 2 - 0 | 240.84 | -952.54 | 1.69341D-02 | 1.84663D-11 | 1.24976D-02 |
| P( 3) | 2 - 0 | 243.24 | -950.13 | 2.48704D-02 | 4.12443D-11 | 1.24133D-02 |
| R( 1) | 2 - 1 | 718.49 | -474.88 | 2.81609D+00 | 1.60926D-08 | -4.57838D-01 |
| P( 3) | 2 - 1 | 720.88 | -472.49 | 4.17080D+00 | 3.61902D-08 | -4.58393D-01 |
| R( 1) | 2 - 2 | 1192.42 | -0.95 | 3.37237D-07 | 1.00000D+00 | -1.77600D+00 |
| R( 2) | 2 - 0 | 241.80 | -953.00 | 1.82201D-02 | 4.15846D-11 | 1.25148D-02 |
| P( 4) | 2 - 0 | 245.16 | -949.63 | 2.35857D-02 | 7.32529D-11 | 1.23968D-02 |
| R( 2) | 2 - 1 | 719.45 | -475.35 | 3.02477D+00 | 3.62030D-08 | -4.57734D-01 |
| P( 4) | 2 - 1 | 722.79 | -472.01 | 3.96191D+00 | 6.43478D-08 | -4.58511D-01 |
| R( 2) | 2 - 2 | 1193.37 | -1.42 | 1.21952D-06 | 1.00000D+00 | -1.77607D+00 |
| R( 3) | 2 - 0 | 243.24 | -953.45 | 1.89743D-02 | 7.40286D-11 | 1.25321D-02 |
| P( 5) | 2 - 0 | 247.57 | -949.12 | 2.28332D-02 | 1.14311D-10 | 1.23804D-02 |
| R( 3) | 2 - 1 | 720.88 | -475.81 | 3.14457D+00 | 6.43605D-08 | -4.57633D-01 |
| P( 5) | 2 - 1 | 725.18 | -471.51 | 3.84182D+00 | 1.00552D-07 | -4.58632D-01 |
| R( 3) | 2 - 2 | 1194.79 | -1.90 | 2.99799D-06 | 1.00000D+00 | -1.77618D+00 |
| R( 4) | 2 - 0 | 245.16 | -953.90 | 1.94869D-02 | 1.15828D-10 | 1.25496D-02 |
| P( 6) | 2 - 0 | 250.45 | -948.61 | 2.23227D-02 | 1.64399D-10 | 1.23641D-02 |
| R( 4) | 2 - 1 | 722.79 | -476.27 | 3.22396D+00 | 1.00565D-07 | -4.57534D-01 |

| | | | | | | | |
|---|---|---|---|---|---|---|---|
| P( 6) | 2 - 1 | 728.05 | -471.02 | 3.76208D+00 | 1.44807D-07 | -4.58755D-01 |
| R( 4) | 2 - 2 | 1196.69 | -2.37 | 5.98910D-06 | 1.00000D+00 | -1.77631D+00 |
| R( 5) | 2 - 0 | 247.57 | -954.34 | 1.98696D-02 | 1.67021D-10 | 1.25671D-02 |
| P( 7) | 2 - 0 | 253.82 | -948.09 | 2.19426D-02 | 2.23484D-10 | 1.23479D-02 |
| R( 5) | 2 - 1 | 725.18 | -476.73 | 3.28156D+00 | 1.44820D-07 | -4.57437D-01 |
| P( 7) | 2 - 1 | 731.39 | -470.52 | 3.70405D+00 | 1.97118D-07 | -4.58880D-01 |
| R( 5) | 2 - 2 | 1199.06 | -2.84 | 1.05096D-05 | 1.00000D+00 | -1.77647D+00 |
| R( 6) | 2 - 0 | 250.45 | -954.77 | 2.01743D-02 | 2.27649D-10 | 1.25848D-02 |
| P( 8) | 2 - 0 | 257.66 | -947.56 | 2.16409D-02 | 2.91533D-10 | 1.23318D-02 |
| R( 6) | 2 - 1 | 728.05 | -477.18 | 3.32608D+00 | 1.97128D-07 | -4.57342D-01 |
| P( 8) | 2 - 1 | 735.21 | -470.01 | 3.65903D+00 | 2.57487D-07 | -4.59008D-01 |
| R( 6) | 2 - 2 | 1201.91 | -3.32 | 1.68766D-05 | 1.00000D+00 | -1.77666D+00 |
| R( 7) | 2 - 0 | 253.82 | -955.20 | 2.04287D-02 | 2.97752D-10 | 1.26025D-02 |
| P( 9) | 2 - 0 | 261.99 | -947.03 | 2.13900D-02 | 3.68515D-10 | 1.23158D-02 |
| R( 7) | 2 - 1 | 731.39 | -477.63 | 3.36212D+00 | 2.57492D-07 | -4.57250D-01 |
| P( 9) | 2 - 1 | 739.51 | -469.50 | 3.62243D+00 | 3.25919D-07 | -4.59138D-01 |
| R( 7) | 2 - 2 | 1205.22 | -3.79 | 2.54076D-05 | 9.99999D-01 | -1.77688D+00 |
| R( 8) | 2 - 0 | 257.66 | -955.62 | 2.06488D-02 | 3.77371D-10 | 1.26204D-02 |
| P( 10) | 2 - 0 | 266.80 | -946.49 | 2.11738D-02 | 4.54397D-10 | 1.23000D-02 |
| R( 8) | 2 - 1 | 735.21 | -478.07 | 3.39235D+00 | 3.25917D-07 | -4.57160D-01 |
| P( 10) | 2 - 1 | 744.29 | -468.99 | 3.59156D+00 | 4.02419D-07 | -4.59271D-01 |
| R( 8) | 2 - 2 | 1209.02 | -4.27 | 3.64206D-05 | 9.99999D-01 | -1.77713D+00 |
| R( 9) | 2 - 0 | 261.99 | -956.03 | 2.08444D-02 | 4.66548D-10 | 1.26385D-02 |
| P( 11) | 2 - 0 | 272.08 | -945.94 | 2.09827D-02 | 5.49150D-10 | 1.22843D-02 |
| R( 9) | 2 - 1 | 739.51 | -478.51 | 3.41841D+00 | 4.02408D-07 | -4.57073D-01 |
| P( 11) | 2 - 1 | 749.54 | -468.48 | 3.56479D+00 | 4.86993D-07 | -4.59406D-01 |
| R( 9) | 2 - 2 | 1213.28 | -4.74 | 5.02341D-05 | 9.99999D-01 | -1.77741D+00 |
| R( 10) | 2 - 0 | 266.80 | -956.44 | 2.10219D-02 | 5.65326D-10 | 1.26566D-02 |
| P( 12) | 2 - 0 | 277.85 | -945.38 | 2.08100D-02 | 6.52743D-10 | 1.22686D-02 |

| | | | | | | | |
|---|---|---|---|---|---|---|---|
| R( 10) | 2 - 1 | 744.29 | -478.95 | 3.44139D+00 | 4.86969D-07 | -4.56988D-01 |
| P( 12) | 2 - 1 | 755.28 | -467.96 | 3.54104D+00 | 5.79647D-07 | -4.59544D-01 |
| R( 10) | 2 - 2 | 1218.02 | -5.21 | 6.71672D-05 | 9.99999D-01 | -1.77772D+00 |
| R( 11) | 2 - 0 | 272.08 | -956.84 | 2.11858D-02 | 6.73749D-10 | 1.26749D-02 |
| P( 13) | 2 - 0 | 284.10 | -944.82 | 2.06514D-02 | 7.65147D-10 | 1.22531D-02 |
| R( 11) | 2 - 1 | 749.54 | -479.38 | 3.46201D+00 | 5.79606D-07 | -4.56905D-01 |
| P( 13) | 2 - 1 | 761.49 | -467.44 | 3.51957D+00 | 6.80388D-07 | -4.59684D-01 |
| R( 11) | 2 - 2 | 1223.23 | -5.69 | 8.75397D-05 | 9.99999D-01 | -1.77806D+00 |
| R( 12) | 2 - 0 | 277.85 | -957.23 | 2.13392D-02 | 7.91861D-10 | 1.26932D-02 |
| P( 14) | 2 - 0 | 290.83 | -944.25 | 2.05039D-02 | 8.86333D-10 | 1.22378D-02 |
| R( 12) | 2 - 1 | 755.28 | -479.81 | 3.48078D+00 | 6.80326D-07 | -4.56824D-01 |
| P( 14) | 2 - 1 | 768.17 | -466.91 | 3.49987D+00 | 7.89222D-07 | -4.59826D-01 |
| R( 12) | 2 - 2 | 1228.92 | -6.16 | 1.11672D-04 | 9.99998D-01 | -1.77842D+00 |
| R( 13) | 2 - 0 | 284.10 | -957.62 | 2.14842D-02 | 9.19706D-10 | 1.27118D-02 |
| P( 15) | 2 - 0 | 298.04 | -943.68 | 2.03652D-02 | 1.01627D-09 | 1.22225D-02 |
| R( 13) | 2 - 1 | 761.49 | -480.23 | 3.49809D+00 | 7.89136D-07 | -4.56746D-01 |
| P( 15) | 2 - 1 | 775.34 | -466.38 | 3.48157D+00 | 9.06158D-07 | -4.59971D-01 |
| R( 13) | 2 - 2 | 1235.08 | -6.63 | 1.39885D-04 | 9.99998D-01 | -1.77882D+00 |
| R( 14) | 2 - 0 | 290.83 | -958.00 | 2.16226D-02 | 1.05733D-09 | 1.27304D-02 |
| P( 16) | 2 - 0 | 305.73 | -943.10 | 2.02337D-02 | 1.15494D-09 | 1.22074D-02 |
| R( 14) | 2 - 1 | 768.17 | -480.65 | 3.51420D+00 | 9.06044D-07 | -4.56670D-01 |
| P( 16) | 2 - 1 | 782.98 | -465.85 | 3.46440D+00 | 1.03120D-06 | -4.60119D-01 |
| R( 14) | 2 - 2 | 1241.72 | -7.11 | 1.72502D-04 | 9.99998D-01 | -1.77925D+00 |
| R( 15) | 2 - 0 | 298.04 | -958.37 | 2.17556D-02 | 1.20478D-09 | 1.27492D-02 |
| P( 17) | 2 - 0 | 313.89 | -942.51 | 2.01081D-02 | 1.30231D-09 | 1.21923D-02 |
| R( 15) | 2 - 1 | 775.34 | -481.07 | 3.52933D+00 | 1.03106D-06 | -4.56596D-01 |
| P( 17) | 2 - 1 | 791.10 | -465.31 | 3.44813D+00 | 1.16437D-06 | -4.60269D-01 |
| R( 15) | 2 - 2 | 1248.82 | -7.58 | 2.09845D-04 | 9.99997D-01 | -1.77970D+00 |
| R( 16) | 2 - 0 | 305.73 | -958.73 | 2.18842D-02 | 1.36211D-09 | 1.27681D-02 |

| | | | | | | | |
|---|---|---|---|---|---|---|---|
| P( 18) | 2 - 0 | 322.54 | -941.92 | 1.99875D-02 | 1.45835D-09 | 1.21775D-02 |
| R( 16) | 2 - 1 | 782.98 | -481.48 | 3.54364D+00 | 1.16418D-06 | -4.56524D-01 |
| P( 18) | 2 - 1 | 799.69 | -464.77 | 3.43262D+00 | 1.30566D-06 | -4.60421D-01 |
| R( 16) | 2 - 2 | 1256.41 | -8.05 | 2.52239D-04 | 9.99997D-01 | -1.78019D+00 |
| R( 17) | 2 - 0 | 313.89 | -959.09 | 2.20092D-02 | 1.52935D-09 | 1.27872D-02 |
| P( 19) | 2 - 0 | 331.67 | -941.32 | 1.98710D-02 | 1.62304D-09 | 1.21627D-02 |
| R( 17) | 2 - 1 | 791.10 | -481.89 | 3.55725D+00 | 1.30544D-06 | -4.56455D-01 |
| P( 19) | 2 - 1 | 808.76 | -464.22 | 3.41774D+00 | 1.45510D-06 | -4.60576D-01 |
| R( 17) | 2 - 2 | 1264.46 | -8.53 | 3.00008D-04 | 9.99997D-01 | -1.78070D+00 |
| R( 18) | 2 - 0 | 322.54 | -959.44 | 2.21311D-02 | 1.70657D-09 | 1.28064D-02 |
| P( 20) | 2 - 0 | 341.28 | -940.71 | 1.97582D-02 | 1.79635D-09 | 1.21481D-02 |
| R( 18) | 2 - 1 | 799.69 | -482.30 | 3.57027D+00 | 1.45482D-06 | -4.56388D-01 |
| P( 20) | 2 - 1 | 818.31 | -463.68 | 3.40338D+00 | 1.61268D-06 | -4.60734D-01 |
| R( 18) | 2 - 2 | 1272.99 | -9.00 | 3.53479D-04 | 9.99996D-01 | -1.78125D+00 |
| R( 19) | 2 - 0 | 331.67 | -959.79 | 2.22505D-02 | 1.89381D-09 | 1.28257D-02 |
| P( 21) | 2 - 0 | 351.37 | -940.09 | 1.96486D-02 | 1.97827D-09 | 1.21336D-02 |
| R( 19) | 2 - 1 | 808.76 | -482.70 | 3.58277D+00 | 1.61235D-06 | -4.56323D-01 |
| P( 21) | 2 - 1 | 828.34 | -463.12 | 3.38946D+00 | 1.77843D-06 | -4.60894D-01 |
| R( 19) | 2 - 2 | 1281.99 | -9.47 | 4.12980D-04 | 9.99996D-01 | -1.78182D+00 |
| P( 1) | 3 - 0 | 240.84 | -1421.03 | 3.88543D-04 | 3.73641D-14 | 6.57076D-04 |
| P( 1) | 3 - 1 | 718.49 | -943.37 | 1.65355D-01 | 1.54720D-11 | -2.50602D-02 |
| P( 1) | 3 - 2 | 1192.42 | -469.44 | 1.02436D+01 | 6.00674D-09 | 5.61901D-01 |
| R( 0) | 3 - 0 | 240.35 | -1421.98 | 1.31313D-04 | 3.74512D-14 | 6.60960D-04 |
| P( 2) | 3 - 0 | 241.80 | -1420.53 | 2.57110D-04 | 1.49061D-13 | 6.54979D-04 |
| R( 0) | 3 - 1 | 718.01 | -944.32 | 5.55377D-02 | 1.54330D-11 | -2.51174D-02 |
| P( 2) | 3 - 1 | 719.45 | -942.89 | 1.09818D-01 | 6.17281D-11 | -2.50318D-02 |
| R( 0) | 3 - 2 | 1191.95 | -470.38 | 3.43172D+00 | 6.00688D-09 | 5.61619D-01 |
| P( 2) | 3 - 2 | 1193.37 | -468.96 | 6.81173D+00 | 2.40274D-08 | 5.62047D-01 |
| R( 0) | 3 - 3 | 1661.86 | -0.47 | 3.77615D-08 | 1.00000D+00 | 1.86554D+00 |

| | | | | | | | |
|---|---|---|---|---|---|---|---|
| R( 1) | 3 - 0 | 240.84 | -1422.43 | 1.58582D-04 | 1.50290D-13 | 6.62747D-04 |
| P( 3) | 3 - 0 | 243.24 | -1420.03 | 2.29603D-04 | 3.34429D-13 | 6.52777D-04 |
| R( 1) | 3 - 1 | 718.49 | -944.78 | 6.68968D-02 | 6.19043D-11 | -2.51463D-02 |
| P( 3) | 3 - 1 | 720.88 | -942.39 | 9.84583D-02 | 1.38635D-10 | -2.50036D-02 |
| R( 1) | 3 - 2 | 1192.42 | -470.85 | 4.12831D+00 | 2.40289D-08 | 5.61483D-01 |
| P( 3) | 3 - 2 | 1194.79 | -468.48 | 6.11490D+00 | 5.40621D-08 | 5.62195D-01 |
| R( 1) | 3 - 3 | 1662.33 | -0.94 | 3.62524D-07 | 1.00000D+00 | 1.86558D+00 |
| R( 2) | 3 - 0 | 241.80 | -1422.88 | 1.70935D-04 | 3.38157D-13 | 6.64430D-04 |
| P( 4) | 3 - 0 | 245.16 | -1419.52 | 2.16892D-04 | 5.94075D-13 | 6.50472D-04 |
| R( 2) | 3 - 1 | 719.45 | -945.24 | 7.19447D-02 | 1.39466D-10 | -2.51754D-02 |
| P( 4) | 3 - 1 | 722.79 | -941.89 | 9.34104D-02 | 2.46181D-10 | -2.49755D-02 |
| R( 2) | 3 - 2 | 1193.37 | -471.31 | 4.43411D+00 | 5.40620D-08 | 5.61350D-01 |
| P( 4) | 3 - 2 | 1196.69 | -467.99 | 5.80873D+00 | 9.61214D-08 | 5.62347D-01 |
| R( 2) | 3 - 3 | 1663.27 | -1.41 | 1.31096D-06 | 1.00000D+00 | 1.86565D+00 |
| R( 3) | 3 - 0 | 243.24 | -1423.32 | 1.78275D-04 | 6.02183D-13 | 6.66010D-04 |
| P( 5) | 3 - 0 | 247.57 | -1418.99 | 2.09077D-04 | 9.26388D-13 | 6.48063D-04 |
| R( 3) | 3 - 1 | 720.88 | -945.68 | 7.48887D-02 | 2.48311D-10 | -2.52047D-02 |
| P( 5) | 3 - 1 | 725.18 | -941.38 | 9.04662D-02 | 3.84152D-10 | -2.49477D-02 |
| R( 3) | 3 - 2 | 1194.79 | -471.77 | 4.60961D+00 | 9.61140D-08 | 5.61220D-01 |
| P( 5) | 3 - 2 | 1199.06 | -467.50 | 5.63274D+00 | 1.50201D-07 | 5.62502D-01 |
| R( 3) | 3 - 3 | 1664.68 | -1.88 | 3.22277D-06 | 1.00000D+00 | 1.86576D+00 |
| R( 4) | 3 - 0 | 245.16 | -1423.75 | 1.83301D-04 | 9.42429D-13 | 6.67487D-04 |
| P( 6) | 3 - 0 | 250.45 | -1418.46 | 2.03456D-04 | 1.33130D-12 | 6.45550D-04 |
| R( 4) | 3 - 1 | 722.79 | -946.12 | 7.68765D-02 | 3.88538D-10 | -2.52341D-02 |
| P( 6) | 3 - 1 | 728.05 | -940.86 | 8.84783D-02 | 5.52483D-10 | -2.49200D-02 |
| R( 4) | 3 - 2 | 1196.69 | -472.22 | 4.72584D+00 | 1.50186D-07 | 5.61093D-01 |
| P( 6) | 3 - 2 | 1201.91 | -467.00 | 5.51590D+00 | 2.16309D-07 | 5.62660D-01 |
| R( 4) | 3 - 3 | 1666.56 | -2.35 | 6.43810D-06 | 1.00000D+00 | 1.86589D+00 |
| R( 5) | 3 - 0 | 247.57 | -1424.16 | 1.87051D-04 | 1.35921D-12 | 6.68861D-04 |

| | | | | | | |
|---|---|---|---|---|---|---|
| P( 7) | 3 - 0 | 253.82 | -1417.91 | 1.98993D-04 | 1.80831D-12 | 6.42933D-04 |
| R( 5) | 3 - 1 | 725.18 | -946.55 | 7.83493D-02 | 5.60274D-10 | -2.52637D-02 |
| P( 7) | 3 - 1 | 731.39 | -940.34 | 8.70053D-02 | 7.51072D-10 | -2.48924D-02 |
| R( 5) | 3 - 2 | 1199.06 | -472.67 | 4.81013D+00 | 2.16283D-07 | 5.60969D-01 |
| P( 7) | 3 - 2 | 1205.22 | -466.51 | 5.43087D+00 | 2.94450D-07 | 5.62822D-01 |
| R( 5) | 3 - 3 | 1668.91 | -2.82 | 1.12974D-05 | 9.99999D-01 | 1.86605D+00 |
| R( 6) | 3 - 0 | 250.45 | -1424.57 | 1.90011D-04 | 1.85282D-12 | 6.70133D-04 |
| P( 8) | 3 - 0 | 257.66 | -1417.36 | 1.95203D-04 | 2.35693D-12 | 6.40213D-04 |
| R( 6) | 3 - 1 | 728.05 | -946.97 | 7.95132D-02 | 7.63648D-10 | -2.52935D-02 |
| P( 8) | 3 - 1 | 735.21 | -939.81 | 8.58413D-02 | 9.79821D-10 | -2.48651D-02 |
| R( 6) | 3 - 2 | 1201.91 | -473.11 | 4.87523D+00 | 2.94410D-07 | 5.60848D-01 |
| P( 8) | 3 - 2 | 1209.02 | -466.00 | 5.36491D+00 | 3.84633D-07 | 5.62986D-01 |
| R( 6) | 3 - 3 | 1671.73 | -3.29 | 1.81415D-05 | 9.99999D-01 | 1.86624D+00 |
| R( 7) | 3 - 0 | 253.82 | -1424.96 | 1.92437D-04 | 2.42353D-12 | 6.71302D-04 |
| P( 9) | 3 - 0 | 261.99 | -1416.79 | 1.91832D-04 | 2.97661D-12 | 6.37390D-04 |
| R( 7) | 3 - 1 | 731.39 | -947.39 | 8.04771D-02 | 9.98792D-10 | -2.53234D-02 |
| P( 9) | 3 - 1 | 739.51 | -939.27 | 8.48772D-02 | 1.23863D-09 | -2.48379D-02 |
| R( 7) | 3 - 2 | 1205.22 | -473.55 | 4.92789D+00 | 3.84573D-07 | 5.60730D-01 |
| P( 9) | 3 - 2 | 1213.28 | -465.50 | 5.31127D+00 | 4.86866D-07 | 5.63154D-01 |
| R( 7) | 3 - 3 | 1675.02 | -3.76 | 2.73117D-05 | 9.99999D-01 | 1.86646D+00 |
| R( 8) | 3 - 0 | 257.66 | -1425.34 | 1.94476D-04 | 3.07161D-12 | 6.72368D-04 |
| P( 10) | 3 - 0 | 266.80 | -1416.21 | 1.88731D-04 | 3.66682D-12 | 6.34462D-04 |
| R( 8) | 3 - 1 | 735.21 | -947.79 | 8.13042D-02 | 1.26584D-09 | -2.53536D-02 |
| P( 10) | 3 - 1 | 744.29 | -938.72 | 8.40500D-02 | 1.52741D-09 | -2.48109D-02 |
| R( 8) | 3 - 2 | 1209.02 | -473.99 | 4.97202D+00 | 4.86780D-07 | 5.60616D-01 |
| P( 10) | 3 - 2 | 1218.02 | -464.99 | 5.26605D+00 | 6.01157D-07 | 5.63324D-01 |
| R( 8) | 3 - 3 | 1678.78 | -4.23 | 3.91495D-05 | 9.99999D-01 | 1.86672D+00 |
| R( 9) | 3 - 0 | 261.99 | -1425.72 | 1.96220D-04 | 3.79730D-12 | 6.73333D-04 |
| P( 11) | 3 - 0 | 272.08 | -1415.62 | 1.85811D-04 | 4.42701D-12 | 6.31432D-04 |

| | | | | | | | |
|---|---|---|---|---|---|---|---|
| R( 9) | 3 - 1 | 739.51 | -948.19 | 8.20336D-02 | 1.56493D-09 | -2.53839D-02 |
| P( 11) | 3 - 1 | 749.54 | -938.16 | 8.33206D-02 | 1.84607D-09 | -2.47840D-02 |
| R( 9) | 3 - 2 | 1213.28 | -474.42 | 5.01003D+00 | 6.01039D-07 | 5.60504D-01 |
| P( 11) | 3 - 2 | 1223.23 | -464.47 | 5.22681D+00 | 7.27517D-07 | 5.63498D-01 |
| R( 9) | 3 - 3 | 1683.01 | -4.70 | 5.39973D-05 | 9.99999D-01 | 1.86700D+00 |
| R( 10) | 3 - 0 | 266.80 | -1426.08 | 1.97729D-04 | 4.60083D-12 | 6.74197D-04 |
| P( 12) | 3 - 0 | 277.85 | -1415.02 | 1.83011D-04 | 5.25659D-12 | 6.28298D-04 |
| R( 10) | 3 - 1 | 744.29 | -948.58 | 8.26907D-02 | 1.89620D-09 | -2.54145D-02 |
| P( 12) | 3 - 1 | 755.28 | -937.60 | 8.26635D-02 | 2.19452D-09 | -2.47574D-02 |
| R( 10) | 3 - 2 | 1218.02 | -474.85 | 5.04350D+00 | 7.27359D-07 | 5.60395D-01 |
| P( 12) | 3 - 2 | 1228.92 | -463.95 | 5.19199D+00 | 8.65957D-07 | 5.63676D-01 |
| R( 10) | 3 - 3 | 1687.71 | -5.17 | 7.21978D-05 | 9.99998D-01 | 1.86731D+00 |
| R( 11) | 3 - 0 | 272.08 | -1426.43 | 1.99044D-04 | 5.48240D-12 | 6.74959D-04 |
| P( 13) | 3 - 0 | 284.10 | -1414.41 | 1.80293D-04 | 6.15497D-12 | 6.25062D-04 |
| R( 11) | 3 - 1 | 749.54 | -948.97 | 8.32929D-02 | 2.25979D-09 | -2.54452D-02 |
| P( 13) | 3 - 1 | 761.49 | -937.03 | 8.20613D-02 | 2.57267D-09 | -2.47309D-02 |
| R( 11) | 3 - 2 | 1223.23 | -475.28 | 5.07351D+00 | 8.65752D-07 | 5.60289D-01 |
| P( 13) | 3 - 2 | 1235.08 | -463.43 | 5.16051D+00 | 1.01649D-06 | 5.63856D-01 |
| R( 11) | 3 - 3 | 1692.87 | -5.64 | 9.40946D-05 | 9.99998D-01 | 1.86764D+00 |
| R( 12) | 3 - 0 | 277.85 | -1426.77 | 2.00193D-04 | 6.44220D-12 | 6.75621D-04 |
| P( 14) | 3 - 0 | 290.83 | -1413.79 | 1.77630D-04 | 7.12155D-12 | 6.21723D-04 |
| R( 12) | 3 - 1 | 755.28 | -949.34 | 8.38524D-02 | 2.65586D-09 | -2.54761D-02 |
| P( 14) | 3 - 1 | 768.17 | -936.45 | 8.15019D-02 | 2.98043D-09 | -2.47045D-02 |
| R( 12) | 3 - 2 | 1228.92 | -475.70 | 5.10081D+00 | 1.01623D-06 | 5.60187D-01 |
| P( 14) | 3 - 2 | 1241.72 | -462.90 | 5.13161D+00 | 1.17913D-06 | 5.64040D-01 |
| R( 12) | 3 - 3 | 1698.51 | -6.11 | 1.20032D-04 | 9.99998D-01 | 1.86801D+00 |
| R( 13) | 3 - 0 | 284.10 | -1427.10 | 2.01196D-04 | 7.48041D-12 | 6.76183D-04 |
| P( 15) | 3 - 0 | 298.04 | -1413.16 | 1.75001D-04 | 8.15570D-12 | 6.18281D-04 |
| R( 13) | 3 - 1 | 761.49 | -949.71 | 8.43780D-02 | 3.08454D-09 | -2.55072D-02 |

| | | | | | | |
|---|---|---|---|---|---|---|
| P( 15) | 3 - 1 | 775.34 | -935.86 | 8.09766D-02 | 3.41773D-09 | -2.46784D-02 |
| R( 13) | 3 - 2 | 1235.08 | -476.11 | 5.12594D+00 | 1.17880D-06 | 5.60087D-01 |
| P( 15) | 3 - 2 | 1248.82 | -462.37 | 5.10476D+00 | 1.35388D-06 | 5.64227D-01 |
| R( 13) | 3 - 3 | 1704.62 | -6.58 | 1.50354D-04 | 9.99997D-01 | 1.86841D+00 |
| R( 14) | 3 - 0 | 290.83 | -1427.41 | 2.02070D-04 | 8.59719D-12 | 6.76644D-04 |
| P( 16) | 3 - 0 | 305.73 | -1412.52 | 1.72393D-04 | 9.25679D-12 | 6.14738D-04 |
| R( 14) | 3 - 1 | 768.17 | -950.07 | 8.48763D-02 | 3.54600D-09 | -2.55385D-02 |
| P( 16) | 3 - 1 | 782.98 | -935.26 | 8.04787D-02 | 3.88448D-09 | -2.46524D-02 |
| R( 14) | 3 - 2 | 1241.72 | -476.53 | 5.14932D+00 | 1.35348D-06 | 5.59990D-01 |
| P( 16) | 3 - 2 | 1256.41 | -461.84 | 5.07955D+00 | 1.54078D-06 | 5.64417D-01 |
| R( 14) | 3 - 3 | 1711.20 | -7.05 | 1.85408D-04 | 9.99997D-01 | 1.86884D+00 |
| R( 15) | 3 - 0 | 298.04 | -1427.72 | 2.02826D-04 | 9.79268D-12 | 6.77007D-04 |
| P( 17) | 3 - 0 | 313.89 | -1411.86 | 1.69796D-04 | 1.04242D-11 | 6.11093D-04 |
| R( 15) | 3 - 1 | 775.34 | -950.42 | 8.53523D-02 | 4.04038D-09 | -2.55700D-02 |
| P( 17) | 3 - 1 | 791.10 | -934.66 | 8.00033D-02 | 4.38062D-09 | -2.46266D-02 |
| R( 15) | 3 - 2 | 1248.82 | -476.93 | 5.17124D+00 | 1.54029D-06 | 5.59896D-01 |
| P( 17) | 3 - 2 | 1264.46 | -461.30 | 5.05567D+00 | 1.73982D-06 | 5.64611D-01 |
| R( 15) | 3 - 3 | 1718.24 | -7.52 | 2.25541D-04 | 9.99996D-01 | 1.86930D+00 |
| R( 16) | 3 - 0 | 305.73 | -1428.02 | 2.03473D-04 | 1.10670D-11 | 6.77270D-04 |
| P( 18) | 3 - 0 | 322.54 | -1411.20 | 1.67203D-04 | 1.16571D-11 | 6.07346D-04 |
| R( 16) | 3 - 1 | 782.98 | -950.76 | 8.58098D-02 | 4.56785D-09 | -2.56017D-02 |
| P( 18) | 3 - 1 | 799.69 | -934.05 | 7.95466D-02 | 4.90609D-09 | -2.46010D-02 |
| R( 16) | 3 - 2 | 1256.41 | -477.34 | 5.19195D+00 | 1.73924D-06 | 5.59805D-01 |
| P( 18) | 3 - 2 | 1272.99 | -460.75 | 5.03287D+00 | 1.95104D-06 | 5.64808D-01 |
| R( 16) | 3 - 3 | 1725.76 | -7.98 | 2.71099D-04 | 9.99996D-01 | 1.86978D+00 |
| R( 17) | 3 - 0 | 313.89 | -1428.30 | 2.04018D-04 | 1.24203D-11 | 6.77435D-04 |
| P( 19) | 3 - 0 | 331.67 | -1410.52 | 1.64607D-04 | 1.29551D-11 | 6.03498D-04 |
| R( 17) | 3 - 1 | 791.10 | -951.10 | 8.62517D-02 | 5.12856D-09 | -2.56336D-02 |
| P( 19) | 3 - 1 | 808.76 | -933.43 | 7.91056D-02 | 5.46075D-09 | -2.45755D-02 |

| | | | | | | | |
|---|---|---|---|---|---|---|---|
| R( 17) | 3 - 2 | 1264.46 | -477.74 | 5.21163D+00 | 1.95034D-06 | 5.59717D-01 |
| P( 19) | 3 - 2 | 1281.99 | -460.21 | 5.01099D+00 | 2.17444D-06 | 5.65008D-01 |
| R( 17) | 3 - 3 | 1733.74 | -8.45 | 3.22431D-04 | 9.99995D-01 | 1.87030D+00 |
| R( 18) | 3 - 0 | 322.54 | -1428.57 | 2.04467D-04 | 1.38526D-11 | 6.77503D-04 |
| P( 20) | 3 - 0 | 341.28 | -1409.84 | 1.62004D-04 | 1.43172D-11 | 5.99550D-04 |
| R( 18) | 3 - 1 | 799.69 | -951.43 | 8.66806D-02 | 5.72264D-09 | -2.56657D-02 |
| P( 20) | 3 - 1 | 818.31 | -932.81 | 7.86779D-02 | 6.04458D-09 | -2.45503D-02 |
| R( 18) | 3 - 2 | 1272.99 | -478.13 | 5.23042D+00 | 2.17362D-06 | 5.59632D-01 |
| P( 20) | 3 - 2 | 1291.46 | -459.66 | 4.98987D+00 | 2.41005D-06 | 5.65211D-01 |
| R( 18) | 3 - 3 | 1742.20 | -8.92 | 3.79889D-04 | 9.99995D-01 | 1.87085D+00 |
| R( 19) | 3 - 0 | 331.67 | -1428.84 | 2.04824D-04 | 1.53641D-11 | 6.77473D-04 |
| P( 21) | 3 - 0 | 351.37 | -1409.14 | 1.59392D-04 | 1.57429D-11 | 5.95501D-04 |
| R( 19) | 3 - 1 | 808.76 | -951.75 | 8.70982D-02 | 6.35033D-09 | -2.56980D-02 |
| P( 21) | 3 - 1 | 828.34 | -932.17 | 7.82617D-02 | 6.65751D-09 | -2.45252D-02 |
| R( 19) | 3 - 2 | 1281.99 | -478.52 | 5.24845D+00 | 2.40910D-06 | 5.59550D-01 |
| P( 21) | 3 - 2 | 1301.41 | -459.10 | 4.96939D+00 | 2.65789D-06 | 5.65418D-01 |
| R( 19) | 3 - 3 | 1751.12 | -9.39 | 4.43823D-04 | 9.99994D-01 | 1.87142D+00 |
| P( 1) | 4 - 0 | 240.84 | -1887.02 | 2.77710D-04 | 1.29396D-15 | 3.63020D-04 |
| P( 1) | 4 - 1 | 718.49 | -1409.36 | 3.37018D-03 | 1.88988D-13 | -1.95925D-03 |
| P( 1) | 4 - 2 | 1192.42 | -935.43 | 3.81026D-01 | 3.27616D-11 | 3.85265D-02 |
| P( 1) | 4 - 3 | 1662.33 | -465.52 | 1.33628D+01 | 7.97563D-09 | -6.49884D-01 |
| R( 0) | 4 - 0 | 240.35 | -1887.97 | 9.29279D-05 | 1.30463D-15 | 3.63447D-04 |
| P( 2) | 4 - 0 | 241.80 | -1886.52 | 1.84715D-04 | 5.16981D-15 | 3.62746D-04 |
| R( 0) | 4 - 1 | 718.01 | -1410.31 | 1.13517D-03 | 1.86834D-13 | -1.96752D-03 |
| P( 2) | 4 - 1 | 719.45 | -1408.88 | 2.23455D-03 | 7.51648D-13 | -1.95493D-03 |
| R( 0) | 4 - 2 | 1191.95 | -936.37 | 1.27918D-01 | 3.28426D-11 | 3.86059D-02 |
| P( 2) | 4 - 2 | 1193.37 | -934.95 | 2.53107D-01 | 1.30883D-10 | 3.84871D-02 |
| R( 0) | 4 - 3 | 1661.86 | -466.46 | 4.47651D+00 | 7.97570D-09 | -6.49544D-01 |
| P( 2) | 4 - 3 | 1663.27 | -465.05 | 8.88616D+00 | 3.19031D-08 | -6.50059D-01 |

| | | | | | | |
|---|---|---|---|---|---|---|
| R( 0) | 4 - 4 | 2127.85 | -0.47 | 4.02504D-08 | 1.00000D+00 | -1.94875D+00 |
| R( 1) | 4 - 0 | 240.84 | -1888.42 | 1.11687D-04 | 5.23049D-15 | 3.63600D-04 |
| P( 3) | 4 - 0 | 243.24 | -1886.01 | 1.65820D-04 | 1.15982D-14 | 3.62431D-04 |
| R( 1) | 4 - 1 | 718.49 | -1410.76 | 1.36900D-03 | 7.51975D-13 | -1.97146D-03 |
| P( 3) | 4 - 1 | 720.88 | -1408.37 | 1.99980D-03 | 1.68523D-12 | -1.95047D-03 |
| R( 1) | 4 - 2 | 1192.42 | -936.83 | 1.54046D-01 | 1.31556D-10 | 3.86460D-02 |
| P( 3) | 4 - 2 | 1194.79 | -934.46 | 2.26975D-01 | 2.94098D-10 | 3.84479D-02 |
| R( 1) | 4 - 3 | 1662.33 | -466.92 | 5.38507D+00 | 3.19043D-08 | -6.49379D-01 |
| P( 3) | 4 - 3 | 1664.68 | -464.57 | 7.97732D+00 | 7.17826D-08 | -6.50237D-01 |
| R( 1) | 4 - 4 | 2128.32 | -0.93 | 3.86418D-07 | 1.00000D+00 | -1.94879D+00 |
| R( 2) | 4 - 0 | 241.80 | -1888.85 | 1.19822D-04 | 1.17353D-14 | 3.63712D-04 |
| P( 4) | 4 - 0 | 245.16 | -1885.49 | 1.57483D-04 | 2.06373D-14 | 3.62075D-04 |
| R( 2) | 4 - 1 | 719.45 | -1411.21 | 1.47385D-03 | 1.69458D-12 | -1.97528D-03 |
| P( 4) | 4 - 1 | 722.79 | -1407.86 | 1.89357D-03 | 2.99158D-12 | -1.94589D-03 |
| R( 2) | 4 - 2 | 1193.37 | -937.28 | 1.65632D-01 | 2.96267D-10 | 3.86862D-02 |
| P( 4) | 4 - 2 | 1196.69 | -933.96 | 2.15385D-01 | 5.22352D-10 | 3.84090D-02 |
| R( 2) | 4 - 3 | 1663.27 | -467.38 | 5.78387D+00 | 7.17805D-08 | -6.49217D-01 |
| P( 4) | 4 - 3 | 1666.56 | -464.09 | 7.57811D+00 | 1.27627D-07 | -6.50418D-01 |
| R( 2) | 4 - 4 | 2129.25 | -1.40 | 1.39736D-06 | 1.00000D+00 | -1.94886D+00 |
| R( 3) | 4 - 0 | 243.24 | -1889.28 | 1.24392D-04 | 2.08796D-14 | 3.63784D-04 |
| P( 5) | 4 - 0 | 247.57 | -1884.95 | 1.52643D-04 | 3.21916D-14 | 3.61679D-04 |
| R( 3) | 4 - 1 | 720.88 | -1411.64 | 1.53556D-03 | 3.01919D-12 | -1.97896D-03 |
| P( 5) | 4 - 1 | 725.18 | -1407.34 | 1.83002D-03 | 4.66457D-12 | -1.94118D-03 |
| R( 3) | 4 - 2 | 1194.79 | -937.72 | 1.72370D-01 | 5.27347D-10 | 3.87266D-02 |
| P( 5) | 4 - 2 | 1199.06 | -933.46 | 2.08641D-01 | 8.15244D-10 | 3.83702D-02 |
| R( 3) | 4 - 3 | 1664.68 | -467.84 | 6.01269D+00 | 1.27613D-07 | -6.49058D-01 |
| P( 5) | 4 - 3 | 1668.91 | -463.61 | 7.34873D+00 | 1.99430D-07 | -6.50603D-01 |
| R( 3) | 4 - 4 | 2130.65 | -1.87 | 3.43516D-06 | 1.00000D+00 | -1.94897D+00 |
| R( 4) | 4 - 0 | 245.16 | -1889.69 | 1.27324D-04 | 3.26498D-14 | 3.63815D-04 |

| | | | | | | | |
|---|---|---|---|---|---|---|---|
| P( 6) | 4 - 0 | 250.45 | -1884.40 | 1.49374D-04 | 4.62718D-14 | 3.61243D-04 |
| R( 4) | 4 - 1 | 722.79 | -1412.06 | 1.57752D-03 | 4.72656D-12 | -1.98252D-03 |
| P( 6) | 4 - 1 | 728.05 | -1406.80 | 1.78576D-03 | 6.70365D-12 | -1.93634D-03 |
| R( 4) | 4 - 2 | 1196.69 | -938.16 | 1.76904D-01 | 8.25006D-10 | 3.87673D-02 |
| P( 6) | 4 - 2 | 1201.91 | -932.94 | 2.04099D-01 | 1.17263D-09 | 3.83316D-02 |
| R( 4) | 4 - 3 | 1666.56 | -468.29 | 6.16422D+00 | 1.99404D-07 | -6.48903D-01 |
| P( 6) | 4 - 3 | 1671.73 | -463.12 | 7.19651D+00 | 2.87202D-07 | -6.50792D-01 |
| R( 4) | 4 - 4 | 2132.52 | -2.33 | 6.86235D-06 | 1.00000D+00 | -1.94910D+00 |
| R( 5) | 4 - 0 | 247.57 | -1890.08 | 1.29356D-04 | 4.70492D-14 | 3.63805D-04 |
| P( 7) | 4 - 0 | 253.82 | -1883.83 | 1.46937D-04 | 6.28592D-14 | 3.60765D-04 |
| R( 5) | 4 - 1 | 725.18 | -1412.47 | 1.60873D-03 | 6.81833D-12 | -1.98595D-03 |
| P( 7) | 4 - 1 | 731.39 | -1406.26 | 1.75178D-03 | 9.10680D-12 | -1.93137D-03 |
| R( 5) | 4 - 2 | 1199.06 | -938.58 | 1.80251D-01 | 1.18950D-09 | 3.88082D-02 |
| P( 7) | 4 - 2 | 1205.22 | -932.42 | 2.00743D-01 | 1.59429D-09 | 3.82933D-02 |
| R( 5) | 4 - 3 | 1668.91 | -468.74 | 6.27409D+00 | 2.87156D-07 | -6.48751D-01 |
| P( 7) | 4 - 3 | 1675.02 | -462.63 | 7.08581D+00 | 3.90949D-07 | -6.50983D-01 |
| R( 5) | 4 - 4 | 2134.85 | -2.80 | 1.20418D-05 | 9.99999D-01 | -1.94926D+00 |
| R( 6) | 4 - 0 | 250.45 | -1890.46 | 1.30836D-04 | 6.40797D-14 | 3.63755D-04 |
| P( 8) | 4 - 0 | 257.66 | -1883.25 | 1.44986D-04 | 8.19335D-14 | 3.60248D-04 |
| R( 6) | 4 - 1 | 728.05 | -1412.86 | 1.63340D-03 | 9.29614D-12 | -1.98926D-03 |
| P( 8) | 4 - 1 | 735.21 | -1405.70 | 1.72389D-03 | 1.18719D-11 | -1.92627D-03 |
| R( 6) | 4 - 2 | 1201.91 | -939.00 | 1.82885D-01 | 1.62109D-09 | 3.88493D-02 |
| P( 8) | 4 - 2 | 1209.02 | -931.89 | 1.98098D-01 | 2.08003D-09 | 3.82551D-02 |
| R( 6) | 4 - 3 | 1671.73 | -469.18 | 6.35893D+00 | 3.90876D-07 | -6.48602D-01 |
| P( 8) | 4 - 3 | 1678.78 | -462.13 | 6.99999D+00 | 5.10679D-07 | -6.51178D-01 |
| R( 6) | 4 - 4 | 2137.65 | -3.26 | 1.93367D-05 | 9.99999D-01 | -1.94945D+00 |
| R( 7) | 4 - 0 | 253.82 | -1890.82 | 1.31945D-04 | 8.37416D-14 | 3.63663D-04 |
| P( 9) | 4 - 0 | 261.99 | -1882.65 | 1.43338D-04 | 1.03471D-13 | 3.59689D-04 |
| R( 7) | 4 - 1 | 731.39 | -1413.25 | 1.65375D-03 | 1.21616D-11 | -1.99244D-03 |

| | | | | | | | |
|---|---|---|---|---|---|---|---|
| P( 9) | 4 - 1 | 739.51 | -1405.13 | 1.69987D-03 | 1.49969D-11 | -1.92104D-03 |
| R( 7) | 4 - 2 | 1205.22 | -939.42 | 1.85058D-01 | 2.12005D-09 | 3.88906D-02 |
| P( 9) | 4 - 2 | 1213.28 | -931.36 | 1.95913D-01 | 2.62966D-09 | 3.82171D-02 |
| R( 7) | 4 - 3 | 1675.02 | -469.62 | 6.42756D+00 | 5.10571D-07 | -6.48456D-01 |
| P( 9) | 4 - 3 | 1683.01 | -461.63 | 6.93026D+00 | 6.46401D-07 | -6.51376D-01 |
| R( 7) | 4 - 4 | 2140.91 | -3.73 | 2.91107D-05 | 9.99999D-01 | -1.94967D+00 |
| R( 8) | 4 - 0 | 257.66 | -1891.17 | 1.32791D-04 | 1.06034D-13 | 3.63531D-04 |
| P( 10) | 4 - 0 | 266.80 | -1882.04 | 1.41887D-04 | 1.27453D-13 | 3.59090D-04 |
| R( 8) | 4 - 1 | 735.21 | -1413.62 | 1.67106D-03 | 1.54162D-11 | -1.99549D-03 |
| P( 10) | 4 - 1 | 744.29 | -1404.55 | 1.67843D-03 | 1.84797D-11 | -1.91568D-03 |
| R( 8) | 4 - 2 | 1209.02 | -939.82 | 1.86914D-01 | 2.68665D-09 | 3.89322D-02 |
| P( 10) | 4 - 2 | 1218.02 | -930.81 | 1.94042D-01 | 3.24297D-09 | 3.81794D-02 |
| R( 8) | 4 - 3 | 1678.78 | -470.06 | 6.48507D+00 | 6.46248D-07 | -6.48314D-01 |
| P( 10) | 4 - 3 | 1687.71 | -461.13 | 6.87150D+00 | 7.98126D-07 | -6.51578D-01 |
| R( 8) | 4 - 4 | 2144.64 | -4.20 | 4.17278D-05 | 9.99999D-01 | -1.94992D+00 |
| R( 9) | 4 - 0 | 261.99 | -1891.51 | 1.33437D-04 | 1.30955D-13 | 3.63358D-04 |
| P( 11) | 4 - 0 | 272.08 | -1881.41 | 1.40568D-04 | 1.53851D-13 | 3.58451D-04 |
| R( 9) | 4 - 1 | 739.51 | -1413.99 | 1.68612D-03 | 1.90615D-11 | -1.99842D-03 |
| P( 11) | 4 - 1 | 749.54 | -1403.95 | 1.65878D-03 | 2.23179D-11 | -1.91020D-03 |
| R( 9) | 4 - 2 | 1213.28 | -940.22 | 1.88544D-01 | 3.32117D-09 | 3.89739D-02 |
| P( 11) | 4 - 2 | 1223.23 | -930.26 | 1.92396D-01 | 3.91979D-09 | 3.81418D-02 |
| R( 9) | 4 - 3 | 1683.01 | -470.49 | 6.53461D+00 | 7.97915D-07 | -6.48174D-01 |
| P( 11) | 4 - 3 | 1692.87 | -460.62 | 6.82058D+00 | 9.65866D-07 | -6.51783D-01 |
| R( 9) | 4 - 4 | 2148.84 | -4.66 | 5.75527D-05 | 9.99998D-01 | -1.95020D+00 |
| R( 10) | 4 - 0 | 266.80 | -1891.83 | 1.33927D-04 | 1.58497D-13 | 3.63144D-04 |
| P( 12) | 4 - 0 | 277.85 | -1880.77 | 1.39339D-04 | 1.82642D-13 | 3.57770D-04 |
| R( 10) | 4 - 1 | 744.29 | -1414.34 | 1.69947D-03 | 2.30990D-11 | -2.00122D-03 |
| P( 12) | 4 - 1 | 755.28 | -1403.35 | 1.64041D-03 | 2.65095D-11 | -1.90458D-03 |
| R( 10) | 4 - 2 | 1218.02 | -940.60 | 1.90007D-01 | 4.02389D-09 | 3.90159D-02 |

| | | | | | | | |
|---|---|---|---|---|---|---|---|
| P( 12) | 4 - 2 | 1228.92 | -929.70 | 1.90915D-01 | 4.65991D-09 | 3.81044D-02 |
| R( 10) | 4 - 3 | 1687.71 | -470.92 | 6.57825D+00 | 9.65584D-07 | -6.48038D-01 |
| P( 12) | 4 - 3 | 1698.51 | -460.11 | 6.77542D+00 | 1.14963D-06 | -6.51992D-01 |
| R( 10) | 4 - 4 | 2153.50 | -5.13 | 7.69505D-05 | 9.99998D-01 | -1.95051D+00 |
| R( 11) | 4 - 0 | 272.08 | -1892.14 | 1.34291D-04 | 1.88656D-13 | 3.62888D-04 |
| P( 13) | 4 - 0 | 284.10 | -1880.12 | 1.38171D-04 | 2.13796D-13 | 3.57049D-04 |
| R( 11) | 4 - 1 | 749.54 | -1414.68 | 1.71144D-03 | 2.75301D-11 | -2.00389D-03 |
| P( 13) | 4 - 1 | 761.49 | -1402.73 | 1.62295D-03 | 3.10521D-11 | -1.89884D-03 |
| R( 11) | 4 - 2 | 1223.23 | -940.98 | 1.91343D-01 | 4.79510D-09 | 3.90580D-02 |
| P( 13) | 4 - 2 | 1235.08 | -929.14 | 1.89560D-01 | 5.46318D-09 | 3.80672D-02 |
| R( 11) | 4 - 3 | 1692.87 | -471.35 | 6.61737D+00 | 1.14927D-06 | -6.47905D-01 |
| P( 13) | 4 - 3 | 1704.62 | -459.60 | 6.73463D+00 | 1.34944D-06 | -6.52203D-01 |
| R( 11) | 4 - 4 | 2158.63 | -5.59 | 1.00287D-04 | 9.99997D-01 | -1.95085D+00 |
| R( 12) | 4 - 0 | 277.85 | -1892.43 | 1.34547D-04 | 2.21425D-13 | 3.62592D-04 |
| P( 14) | 4 - 0 | 290.83 | -1879.45 | 1.37043D-04 | 2.47285D-13 | 3.56286D-04 |
| R( 12) | 4 - 1 | 755.28 | -1415.00 | 1.72229D-03 | 3.23562D-11 | -2.00644D-03 |
| P( 14) | 4 - 1 | 768.17 | -1402.11 | 1.60618D-03 | 3.59434D-11 | -1.89296D-03 |
| R( 12) | 4 - 2 | 1228.92 | -941.36 | 1.92579D-01 | 5.63510D-09 | 3.91004D-02 |
| P( 14) | 4 - 2 | 1241.72 | -928.56 | 1.88303D-01 | 6.32939D-09 | 3.80302D-02 |
| R( 12) | 4 - 3 | 1698.51 | -471.77 | 6.65297D+00 | 1.34897D-06 | -6.47775D-01 |
| P( 14) | 4 - 3 | 1711.20 | -459.08 | 6.69723D+00 | 1.56530D-06 | -6.52419D-01 |
| R( 12) | 4 - 4 | 2164.22 | -6.06 | 1.27929D-04 | 9.99997D-01 | -1.95121D+00 |
| R( 13) | 4 - 0 | 284.10 | -1892.71 | 1.34712D-04 | 2.56793D-13 | 3.62254D-04 |
| P( 15) | 4 - 0 | 298.04 | -1878.77 | 1.35942D-04 | 2.83078D-13 | 3.55483D-04 |
| R( 13) | 4 - 1 | 761.49 | -1415.32 | 1.73219D-03 | 3.75788D-11 | -2.00886D-03 |
| P( 15) | 4 - 1 | 775.34 | -1401.47 | 1.58990D-03 | 4.11812D-11 | -1.88696D-03 |
| R( 13) | 4 - 2 | 1235.08 | -941.72 | 1.93736D-01 | 6.54418D-09 | 3.91430D-02 |
| P( 15) | 4 - 2 | 1248.82 | -927.98 | 1.87123D-01 | 7.25840D-09 | 3.79934D-02 |
| R( 13) | 4 - 3 | 1704.62 | -472.19 | 6.68576D+00 | 1.56472D-06 | -6.47649D-01 |

| | | | | | | | |
|---|---|---|---|---|---|---|---|
| P( 15) | 4 - 3 | 1718.24 | -458.56 | 6.66250D+00 | 1.79723D-06 | -6.52638D-01 |
| R( 13) | 4 - 4 | 2170.28 | -6.53 | 1.60244D-04 | 9.99996D-01 | -1.95161D+00 |
| R( 14) | 4 - 0 | 290.83 | -1892.97 | 1.34796D-04 | 2.94751D-13 | 3.61874D-04 |
| P( 16) | 4 - 0 | 305.73 | -1878.07 | 1.34856D-04 | 3.21143D-13 | 3.54639D-04 |
| R( 14) | 4 - 1 | 768.17 | -1415.62 | 1.74128D-03 | 4.31990D-11 | -2.01116D-03 |
| P( 16) | 4 - 1 | 782.98 | -1400.82 | 1.57399D-03 | 4.67630D-11 | -1.88083D-03 |
| R( 14) | 4 - 2 | 1241.72 | -942.08 | 1.94829D-01 | 7.52266D-09 | 3.91859D-02 |
| P( 16) | 4 - 2 | 1256.41 | -927.39 | 1.86006D-01 | 8.25003D-09 | 3.79567D-02 |
| R( 14) | 4 - 3 | 1711.20 | -472.60 | 6.71627D+00 | 1.79651D-06 | -6.47525D-01 |
| P( 16) | 4 - 3 | 1725.76 | -458.04 | 6.62992D+00 | 2.04525D-06 | -6.52860D-01 |
| R( 14) | 4 - 4 | 2176.80 | -6.99 | 1.97600D-04 | 9.99996D-01 | -1.95204D+00 |
| R( 15) | 4 - 0 | 298.04 | -1893.22 | 1.34807D-04 | 3.35285D-13 | 3.61453D-04 |
| P( 17) | 4 - 0 | 313.89 | -1877.36 | 1.33777D-04 | 3.61448D-13 | 3.53754D-04 |
| R( 15) | 4 - 1 | 775.34 | -1415.92 | 1.74966D-03 | 4.92183D-11 | -2.01334D-03 |
| P( 17) | 4 - 1 | 791.10 | -1400.16 | 1.55836D-03 | 5.26864D-11 | -1.87457D-03 |
| R( 15) | 4 - 2 | 1248.82 | -942.43 | 1.95869D-01 | 8.57084D-09 | 3.92289D-02 |
| P( 17) | 4 - 2 | 1264.46 | -926.79 | 1.84939D-01 | 9.30410D-09 | 3.79202D-02 |
| R( 15) | 4 - 3 | 1718.24 | -473.01 | 6.74489D+00 | 2.04438D-06 | -6.47405D-01 |
| P( 17) | 4 - 3 | 1733.74 | -457.51 | 6.59908D+00 | 2.30937D-06 | -6.53085D-01 |
| R( 15) | 4 - 4 | 2183.80 | -7.46 | 2.40366D-04 | 9.99995D-01 | -1.95249D+00 |
| R( 16) | 4 - 0 | 305.73 | -1893.45 | 1.34753D-04 | 3.78383D-13 | 3.60991D-04 |
| P( 18) | 4 - 0 | 322.54 | -1876.63 | 1.32699D-04 | 4.03957D-13 | 3.52827D-04 |
| R( 16) | 4 - 1 | 782.98 | -1416.20 | 1.75741D-03 | 5.56380D-11 | -2.01539D-03 |
| P( 18) | 4 - 1 | 799.69 | -1399.48 | 1.54293D-03 | 5.89473D-11 | -1.86817D-03 |
| R( 16) | 4 - 2 | 1256.41 | -942.77 | 1.96865D-01 | 9.68903D-09 | 3.92721D-02 |
| P( 18) | 4 - 2 | 1272.99 | -926.19 | 1.83914D-01 | 1.04205D-08 | 3.78839D-02 |
| R( 16) | 4 - 3 | 1725.76 | -473.42 | 6.77195D+00 | 2.30833D-06 | -6.47288D-01 |
| P( 18) | 4 - 3 | 1742.20 | -456.98 | 6.56967D+00 | 2.58963D-06 | -6.53315D-01 |
| R( 16) | 4 - 4 | 2191.25 | -7.92 | 2.88912D-04 | 9.99995D-01 | -1.95298D+00 |

| | | | | | | | |
|---|---|---|---|---|---|---|---|
| R( 17) | 4 - 0 | 313.89 | -1893.67 | 1.34637D-04 | 4.24028D-13 | 3.60487D-04 |
| P( 19) | 4 - 0 | 331.67 | -1875.89 | 1.31618D-04 | 4.48634D-13 | 3.51859D-04 |
| R( 17) | 4 - 1 | 791.10 | -1416.47 | 1.76458D-03 | 6.24591D-11 | -2.01732D-03 |
| P( 19) | 4 - 1 | 808.76 | -1398.80 | 1.52763D-03 | 6.55465D-11 | -1.86165D-03 |
| R( 17) | 4 - 2 | 1264.46 | -943.10 | 1.97825D-01 | 1.08776D-08 | 3.93156D-02 |
| P( 19) | 4 - 2 | 1281.99 | -925.58 | 1.82924D-01 | 1.15990D-08 | 3.78478D-02 |
| R( 17) | 4 - 3 | 1733.74 | -473.82 | 6.79766D+00 | 2.58839D-06 | -6.47173D-01 |
| P( 19) | 4 - 3 | 1751.12 | -456.45 | 6.54146D+00 | 2.88602D-06 | -6.53547D-01 |
| R( 17) | 4 - 4 | 2199.18 | -8.39 | 3.43610D-04 | 9.99994D-01 | -1.95349D+00 |
| R( 18) | 4 - 0 | 322.54 | -1893.87 | 1.34464D-04 | 4.72203D-13 | 3.59941D-04 |
| P( 20) | 4 - 0 | 341.28 | -1875.14 | 1.30529D-04 | 4.95442D-13 | 3.50849D-04 |
| R( 18) | 4 - 1 | 799.69 | -1416.73 | 1.77122D-03 | 6.96849D-11 | -2.01912D-03 |
| P( 20) | 4 - 1 | 818.31 | -1398.10 | 1.51244D-03 | 7.24799D-11 | -1.85501D-03 |
| R( 18) | 4 - 2 | 1272.99 | -943.43 | 1.98752D-01 | 1.21368D-08 | 3.93592D-02 |
| P( 20) | 4 - 2 | 1291.46 | -924.96 | 1.81964D-01 | 1.28395D-08 | 3.78118D-02 |
| R( 18) | 4 - 3 | 1742.20 | -474.22 | 6.82224D+00 | 2.88457D-06 | -6.47062D-01 |
| P( 20) | 4 - 3 | 1760.51 | -455.91 | 6.51426D+00 | 3.19859D-06 | -6.53783D-01 |
| R( 18) | 4 - 4 | 2207.56 | -8.85 | 4.04832D-04 | 9.99993D-01 | -1.95404D+00 |
| R( 19) | 4 - 0 | 331.67 | -1894.06 | 1.34237D-04 | 5.22891D-13 | 3.59352D-04 |
| P( 21) | 4 - 0 | 351.37 | -1874.37 | 1.29431D-04 | 5.44342D-13 | 3.49798D-04 |
| R( 19) | 4 - 1 | 808.76 | -1416.97 | 1.77738D-03 | 7.73128D-11 | -2.02081D-03 |
| P( 21) | 4 - 1 | 828.34 | -1397.40 | 1.49730D-03 | 7.97448D-11 | -1.84823D-03 |
| R( 19) | 4 - 2 | 1281.99 | -943.75 | 1.99653D-01 | 1.34670D-08 | 3.94031D-02 |
| P( 21) | 4 - 2 | 1301.41 | -924.33 | 1.81028D-01 | 1.41418D-08 | 3.77760D-02 |
| R( 19) | 4 - 3 | 1751.12 | -474.62 | 6.84583D+00 | 3.19689D-06 | -6.46954D-01 |
| P( 21) | 4 - 3 | 1770.37 | -455.37 | 6.48790D+00 | 3.52734D-06 | -6.54023D-01 |
| R( 19) | 4 - 4 | 2216.42 | -9.32 | 4.72951D-04 | 9.99993D-01 | -1.95461D+00 |
| P( 1) | 5 - 0 | 240.84 | -2349.95 | 1.37574D-04 | 1.07804D-16 | 1.83856D-04 |
| P( 1) | 5 - 1 | 718.49 | -1872.30 | 1.01728D-03 | 6.06239D-15 | -7.03002D-04 |

| | | | | | | | |
|---|---|---|---|---|---|---|---|
| P( 1) | 5 - 2 | 1192.42 | -1398.36 | 1.17257D-02 | 5.09186D-13 | 3.69777D-03 |
| P( 1) | 5 - 3 | 1662.33 | -928.46 | 6.15871D-01 | 5.35471D-11 | -4.95339D-02 |
| P( 1) | 5 - 4 | 2128.32 | -462.47 | 1.64274D+01 | 9.91422D-09 | 7.27721D-01 |
| R( 0) | 5 - 0 | 240.35 | -2350.89 | 4.59683D-05 | 1.10294D-16 | 1.83967D-04 |
| P( 2) | 5 - 0 | 241.80 | -2349.45 | 9.15991D-05 | 4.32414D-16 | 1.83798D-04 |
| R( 0) | 5 - 1 | 718.01 | -1873.24 | 3.40691D-04 | 7.05400D-15 | -7.04127D-04 |
| P( 2) | 5 - 1 | 719.45 | -1871.80 | 6.76404D-04 | 2.51359D-14 | -7.02356D-04 |
| R( 0) | 5 - 2 | 1191.95 | -1399.30 | 3.94458D-03 | 5.10977D-13 | 3.71103D-03 |
| P( 2) | 5 - 2 | 1193.37 | -1397.88 | 7.78120D-03 | 2.03317D-12 | 3.69118D-03 |
| R( 0) | 5 - 3 | 1661.86 | -929.39 | 2.06755D-01 | 5.36794D-11 | -4.96354D-02 |
| P( 2) | 5 - 3 | 1663.27 | -927.98 | 4.09113D-01 | 2.13922D-10 | -4.94834D-02 |
| R( 0) | 5 - 4 | 2127.85 | -463.39 | 5.50292D+00 | 9.91416D-09 | 7.27326D-01 |
| P( 2) | 5 - 4 | 2129.25 | -462.00 | 1.09244D+01 | 3.96575D-08 | 7.27923D-01 |
| R( 0) | 5 - 5 | 2590.79 | -0.46 | 4.25767D-08 | 1.00000D+00 | 2.02503D+00 |
| R( 1) | 5 - 0 | 240.84 | -2351.34 | 5.52243D-05 | 4.40773D-16 | 1.84018D-04 |
| P( 3) | 5 - 0 | 243.24 | -2348.94 | 8.23303D-05 | 9.71220D-16 | 1.83737D-04 |
| R( 1) | 5 - 1 | 718.49 | -1873.69 | 4.09678D-04 | 2.73022D-14 | -7.04604D-04 |
| P( 3) | 5 - 1 | 720.88 | -1871.30 | 6.07052D-04 | 5.71049D-14 | -7.01653D-04 |
| R( 1) | 5 - 2 | 1192.42 | -1399.75 | 4.75513D-03 | 2.04837D-12 | 3.71770D-03 |
| P( 3) | 5 - 2 | 1194.79 | -1397.38 | 6.97076D-03 | 4.56544D-12 | 3.68461D-03 |
| R( 1) | 5 - 3 | 1662.33 | -929.84 | 2.48982D-01 | 2.15013D-10 | -4.96864D-02 |
| P( 3) | 5 - 3 | 1664.68 | -927.49 | 3.66879D-01 | 4.80697D-10 | -4.94330D-02 |
| R( 1) | 5 - 4 | 2128.32 | -463.85 | 6.61968D+00 | 3.96581D-08 | 7.27134D-01 |
| P( 3) | 5 - 4 | 2130.65 | -461.52 | 9.80733D+00 | 8.92302D-08 | 7.28129D-01 |
| R( 1) | 5 - 5 | 2591.25 | -0.93 | 4.08750D-07 | 1.00000D+00 | 2.02507D+00 |
| R( 2) | 5 - 0 | 241.80 | -2351.77 | 5.92329D-05 | 9.86180D-16 | 1.84068D-04 |
| P( 4) | 5 - 0 | 245.16 | -2348.40 | 7.83024D-05 | 1.73176D-15 | 1.83674D-04 |
| R( 2) | 5 - 1 | 719.45 | -1874.12 | 4.39771D-04 | 6.06048D-14 | -7.05025D-04 |
| P( 4) | 5 - 1 | 722.79 | -1870.77 | 5.76411D-04 | 1.02182D-13 | -7.00893D-04 |

| | | | | | | | |
|---|---|---|---|---|---|---|---|
| R( 2) | 5 - 2 | 1193.37 | -1400.19 | 5.11799D-03 | 4.61159D-12 | 3.72440D-03 |
| P( 4) | 5 - 2 | 1196.69 | -1396.87 | 6.60808D-03 | 8.10927D-12 | 3.67807D-03 |
| R( 2) | 5 - 3 | 1663.27 | -930.29 | 2.67704D-01 | 4.84232D-10 | -4.97375D-02 |
| P( 4) | 5 - 3 | 1666.56 | -927.00 | 3.48146D-01 | 8.53733D-10 | -4.93829D-02 |
| R( 2) | 5 - 4 | 2129.25 | -464.31 | 7.10978D+00 | 8.92254D-08 | 7.26945D-01 |
| P( 4) | 5 - 4 | 2132.52 | -461.05 | 9.31681D+00 | 1.58646D-07 | 7.28338D-01 |
| R( 2) | 5 - 5 | 2592.18 | -1.39 | 1.47811D-06 | 1.00000D+00 | 2.02514D+00 |
| R( 3) | 5 - 0 | 243.24 | -2352.18 | 6.14901D-05 | 1.75323D-15 | 1.84114D-04 |
| P( 5) | 5 - 0 | 247.57 | -2347.85 | 7.60195D-05 | 2.70410D-15 | 1.83608D-04 |
| R( 3) | 5 - 1 | 720.88 | -1874.54 | 4.56836D-04 | 1.07221D-13 | -7.05390D-04 |
| P( 5) | 5 - 1 | 725.18 | -1870.24 | 5.58614D-04 | 1.59996D-13 | -7.00077D-04 |
| R( 3) | 5 - 2 | 1194.79 | -1400.62 | 5.33163D-03 | 8.21151D-12 | 3.73112D-03 |
| P( 5) | 5 - 2 | 1199.06 | -1396.36 | 6.39466D-03 | 1.26514D-11 | 3.67155D-03 |
| R( 3) | 5 - 3 | 1664.68 | -930.74 | 2.78589D-01 | 8.61907D-10 | -4.97889D-02 |
| P( 5) | 5 - 3 | 1668.91 | -926.51 | 3.37247D-01 | 1.33241D-09 | -4.93328D-02 |
| R( 3) | 5 - 4 | 2130.65 | -464.76 | 7.39096D+00 | 1.58626D-07 | 7.26759D-01 |
| P( 5) | 5 - 4 | 2134.85 | -460.57 | 9.03507D+00 | 2.47899D-07 | 7.28550D-01 |
| R( 3) | 5 - 5 | 2593.56 | -1.85 | 3.63365D-06 | 1.00000D+00 | 2.02524D+00 |
| R( 4) | 5 - 0 | 245.16 | -2352.57 | 6.29495D-05 | 2.74019D-15 | 1.84159D-04 |
| P( 6) | 5 - 0 | 250.45 | -2347.28 | 7.45280D-05 | 3.89055D-15 | 1.83540D-04 |
| R( 4) | 5 - 1 | 722.79 | -1874.94 | 4.67929D-04 | 1.67121D-13 | -7.05697D-04 |
| P( 6) | 5 - 1 | 728.05 | -1869.69 | 5.46606D-04 | 2.30580D-13 | -6.99203D-04 |
| R( 4) | 5 - 2 | 1196.69 | -1401.04 | 5.47746D-03 | 1.28511D-11 | 3.73787D-03 |
| P( 6) | 5 - 2 | 1201.91 | -1395.83 | 6.24911D-03 | 1.81904D-11 | 3.66506D-03 |
| R( 4) | 5 - 3 | 1666.56 | -931.17 | 2.85911D-01 | 1.34838D-09 | -4.98404D-02 |
| P( 6) | 5 - 3 | 1671.73 | -926.00 | 3.29907D-01 | 1.91646D-09 | -4.92830D-02 |
| R( 4) | 5 - 4 | 2132.52 | -465.22 | 7.57712D+00 | 2.47859D-07 | 7.26576D-01 |
| P( 6) | 5 - 4 | 2137.65 | -460.09 | 8.84821D+00 | 3.56998D-07 | 7.28766D-01 |
| R( 4) | 5 - 5 | 2595.42 | -2.32 | 7.25883D-06 | 9.99999D-01 | 2.02537D+00 |

| | | | | | | |
|---|---|---|---|---|---|---|
| R( 5) | 5 - 0 | 247.57 | -2352.94 | 6.39777D-05 | 3.94745D-15 | 1.84201D-04 |
| P( 7) | 5 - 0 | 253.82 | -2346.69 | 7.34611D-05 | 5.29021D-15 | 1.83470D-04 |
| R( 5) | 5 - 1 | 725.18 | -1875.33 | 4.75763D-04 | 2.40342D-13 | -7.05948D-04 |
| P( 7) | 5 - 1 | 731.39 | -1869.12 | 5.37674D-04 | 3.13860D-13 | -6.98273D-04 |
| R( 5) | 5 - 2 | 1199.06 | -1401.45 | 5.58679D-03 | 1.85356D-11 | 3.74464D-03 |
| P( 7) | 5 - 2 | 1205.22 | -1395.29 | 6.14011D-03 | 2.47218D-11 | 3.65859D-03 |
| R( 5) | 5 - 3 | 1668.91 | -931.60 | 2.91314D-01 | 1.94407D-09 | -4.98920D-02 |
| P( 7) | 5 - 3 | 1675.02 | -925.49 | 3.24483D-01 | 2.60553D-09 | -4.92332D-02 |
| R( 5) | 5 - 4 | 2134.85 | -465.66 | 7.71208D+00 | 3.56929D-07 | 7.26397D-01 |
| P( 7) | 5 - 4 | 2140.91 | -459.60 | 8.71240D+00 | 4.85951D-07 | 7.28986D-01 |
| R( 5) | 5 - 5 | 2597.73 | -2.78 | 1.27374D-05 | 9.99999D-01 | 2.02553D+00 |
| R( 6) | 5 - 0 | 250.45 | -2353.30 | 6.47458D-05 | 5.37531D-15 | 1.84240D-04 |
| P( 8) | 5 - 0 | 257.66 | -2346.09 | 7.26478D-05 | 6.90211D-15 | 1.83398D-04 |
| R( 6) | 5 - 1 | 728.05 | -1875.71 | 4.81601D-04 | 3.26921D-13 | -7.06142D-04 |
| P( 8) | 5 - 1 | 735.21 | -1868.54 | 5.30553D-04 | 4.09758D-13 | -6.97285D-04 |
| R( 6) | 5 - 2 | 1201.91 | -1401.85 | 5.67423D-03 | 2.52701D-11 | 3.75144D-03 |
| P( 8) | 5 - 2 | 1209.02 | -1394.74 | 6.05306D-03 | 3.22413D-11 | 3.65215D-03 |
| R( 6) | 5 - 3 | 1671.73 | -932.02 | 2.95565D-01 | 2.64937D-09 | -4.99438D-02 |
| P( 8) | 5 - 3 | 1678.78 | -924.97 | 3.20207D-01 | 3.39928D-09 | -4.91837D-02 |
| R( 6) | 5 - 4 | 2137.65 | -466.11 | 7.81631D+00 | 4.85840D-07 | 7.26221D-01 |
| P( 8) | 5 - 4 | 2144.64 | -459.11 | 8.60719D+00 | 6.34766D-07 | 7.29208D-01 |
| R( 6) | 5 - 5 | 2600.51 | -3.24 | 2.04536D-05 | 9.99999D-01 | 2.02572D+00 |
| R( 7) | 5 - 0 | 253.82 | -2353.64 | 6.53443D-05 | 7.02404D-15 | 1.84277D-04 |
| P( 9) | 5 - 0 | 261.99 | -2345.47 | 7.19973D-05 | 8.72533D-15 | 1.83323D-04 |
| R( 7) | 5 - 1 | 731.39 | -1876.07 | 4.86115D-04 | 4.26888D-13 | -7.06278D-04 |
| P( 9) | 5 - 1 | 739.51 | -1867.94 | 5.24572D-04 | 5.18191D-13 | -6.96240D-04 |
| R( 7) | 5 - 2 | 1205.22 | -1402.23 | 5.74751D-03 | 3.30598D-11 | 3.75827D-03 |
| P( 9) | 5 - 2 | 1213.28 | -1394.17 | 5.98022D-03 | 4.07446D-11 | 3.64573D-03 |
| R( 7) | 5 - 3 | 1675.02 | -932.44 | 2.99068D-01 | 3.46473D-09 | -4.99958D-02 |

| | | | | | | | |
|---|---|---|---|---|---|---|---|
| P( 9) | 5 - 3 | 1683.01 | -924.45 | 3.16675D-01 | 4.29735D-09 | -4.91342D-02 |
| R( 7) | 5 - 4 | 2140.91 | -466.55 | 7.90060D+00 | 6.34600D-07 | 7.26049D-01 |
| P( 9) | 5 - 4 | 2148.84 | -458.62 | 8.52177D+00 | 8.03451D-07 | 7.29434D-01 |
| R( 7) | 5 - 5 | 2603.75 | -3.70 | 3.07918D-05 | 9.99999D-01 | 2.02594D+00 |
| R( 8) | 5 - 0 | 257.66 | -2353.96 | 6.58256D-05 | 8.89383D-15 | 1.84312D-04 |
| P( 10) | 5 - 0 | 266.80 | -2344.83 | 7.14574D-05 | 1.07586D-14 | 1.83245D-04 |
| R( 8) | 5 - 1 | 735.21 | -1876.41 | 4.89692D-04 | 5.40271D-13 | -7.06357D-04 |
| P( 10) | 5 - 1 | 744.29 | -1867.33 | 5.19344D-04 | 6.39075D-13 | -6.95136D-04 |
| R( 8) | 5 - 2 | 1209.02 | -1402.61 | 5.81111D-03 | 4.19102D-11 | 3.76512D-03 |
| P( 10) | 5 - 2 | 1218.02 | -1393.60 | 5.91711D-03 | 5.02274D-11 | 3.63934D-03 |
| R( 8) | 5 - 3 | 1678.78 | -932.85 | 3.02060D-01 | 4.39055D-09 | -5.00480D-02 |
| P( 10) | 5 - 3 | 1687.71 | -923.92 | 3.13651D-01 | 5.29941D-09 | -4.90850D-02 |
| R( 8) | 5 - 4 | 2144.64 | -466.98 | 7.97125D+00 | 8.03216D-07 | 7.25879D-01 |
| P( 10) | 5 - 4 | 2153.50 | -458.13 | 8.44986D+00 | 9.92018D-07 | 7.29664D-01 |
| R( 8) | 5 - 5 | 2607.46 | -4.17 | 4.41370D-05 | 9.99998D-01 | 2.02618D+00 |
| R( 9) | 5 - 0 | 261.99 | -2354.26 | 6.62222D-05 | 1.09847D-14 | 1.84343D-04 |
| P( 11) | 5 - 0 | 272.08 | -2344.17 | 7.09953D-05 | 1.30009D-14 | 1.83165D-04 |
| R( 9) | 5 - 1 | 739.51 | -1876.74 | 4.92572D-04 | 6.67093D-13 | -7.06377D-04 |
| P( 11) | 5 - 1 | 749.54 | -1866.71 | 5.14627D-04 | 7.72318D-13 | -6.93974D-04 |
| R( 9) | 5 - 2 | 1213.28 | -1402.97 | 5.86780D-03 | 5.18266D-11 | 3.77201D-03 |
| P( 11) | 5 - 2 | 1223.23 | -1393.02 | 5.86097D-03 | 6.06856D-11 | 3.63296D-03 |
| R( 9) | 5 - 3 | 1683.01 | -933.25 | 3.04687D-01 | 5.42728D-09 | -5.01003D-02 |
| P( 11) | 5 - 3 | 1692.87 | -923.38 | 3.10988D-01 | 6.40512D-09 | -4.90358D-02 |
| R( 9) | 5 - 4 | 2148.84 | -467.42 | 8.03211D+00 | 9.91695D-07 | 7.25713D-01 |
| P( 11) | 5 - 4 | 2158.63 | -457.63 | 8.38759D+00 | 1.20048D-06 | 7.29897D-01 |
| R( 9) | 5 - 5 | 2611.62 | -4.63 | 6.08748D-05 | 9.99998D-01 | 2.02646D+00 |
| R( 10) | 5 - 0 | 266.80 | -2354.55 | 6.65552D-05 | 1.32969D-14 | 1.84372D-04 |
| P( 12) | 5 - 0 | 277.85 | -2343.50 | 7.05901D-05 | 1.54509D-14 | 1.83083D-04 |
| R( 10) | 5 - 1 | 744.29 | -1877.06 | 4.94909D-04 | 8.07376D-13 | -7.06338D-04 |

| | | | | | | | |
|---|---|---|---|---|---|---|---|
| P( 12) | 5 - 1 | 755.28 | -1866.07 | 5.10266D-04 | 9.17828D-13 | -6.92753D-04 |
| R( 10) | 5 - 2 | 1218.02 | -1403.33 | 5.91938D-03 | 6.28145D-11 | 3.77891D-03 |
| P( 12) | 5 - 2 | 1228.92 | -1392.43 | 5.80997D-03 | 7.21151D-11 | 3.62661D-03 |
| R( 10) | 5 - 3 | 1687.71 | -933.64 | 3.07042D-01 | 6.57535D-09 | -5.01528D-02 |
| P( 12) | 5 - 3 | 1698.51 | -922.84 | 3.08593D-01 | 7.61417D-09 | -4.89868D-02 |
| R( 10) | 5 - 4 | 2153.50 | -467.85 | 8.08573D+00 | 1.20005D-06 | 7.25550D-01 |
| P( 12) | 5 - 4 | 2164.22 | -457.13 | 8.33242D+00 | 1.42884D-06 | 7.30133D-01 |
| R( 10) | 5 - 5 | 2616.25 | -5.09 | 8.13912D-05 | 9.99997D-01 | 2.02676D+00 |
| R( 11) | 5 - 0 | 272.08 | -2354.82 | 6.68390D-05 | 1.58305D-14 | 1.84398D-04 |
| P( 13) | 5 - 0 | 284.10 | -2342.80 | 7.02271D-05 | 1.81076D-14 | 1.82998D-04 |
| R( 11) | 5 - 1 | 749.54 | -1877.36 | 4.96810D-04 | 9.61134D-13 | -7.06241D-04 |
| P( 13) | 5 - 1 | 761.49 | -1865.42 | 5.06155D-04 | 1.07551D-12 | -6.91473D-04 |
| R( 11) | 5 - 2 | 1223.23 | -1403.67 | 5.96709D-03 | 7.48796D-11 | 3.78585D-03 |
| P( 13) | 5 - 2 | 1235.08 | -1391.82 | 5.76289D-03 | 8.45118D-11 | 3.62029D-03 |
| R( 11) | 5 - 3 | 1692.87 | -934.03 | 3.09190D-01 | 7.83521D-09 | -5.02054D-02 |
| P( 13) | 5 - 3 | 1704.62 | -922.28 | 3.06401D-01 | 8.92622D-09 | -4.89379D-02 |
| R( 11) | 5 - 4 | 2158.63 | -468.28 | 8.13383D+00 | 1.42828D-06 | 7.25390D-01 |
| P( 13) | 5 - 4 | 2170.28 | -456.62 | 8.28264D+00 | 1.67712D-06 | 7.30373D-01 |
| R( 11) | 5 - 5 | 2621.35 | -5.56 | 1.06073D-04 | 9.99997D-01 | 2.02709D+00 |
| R( 12) | 5 - 0 | 277.85 | -2355.07 | 6.70835D-05 | 1.85852D-14 | 1.84421D-04 |
| P( 14) | 5 - 0 | 290.83 | -2342.09 | 6.98963D-05 | 2.09694D-14 | 1.82910D-04 |
| R( 12) | 5 - 1 | 755.28 | -1877.64 | 4.98350D-04 | 1.12838D-12 | -7.06084D-04 |
| P( 14) | 5 - 1 | 768.17 | -1864.75 | 5.02217D-04 | 1.24526D-12 | -6.90132D-04 |
| R( 12) | 5 - 2 | 1228.92 | -1404.00 | 6.01179D-03 | 8.80272D-11 | 3.79281D-03 |
| P( 14) | 5 - 2 | 1241.72 | -1391.20 | 5.71887D-03 | 9.78716D-11 | 3.61398D-03 |
| R( 12) | 5 - 3 | 1698.51 | -934.41 | 3.11177D-01 | 9.20731D-09 | -5.02582D-02 |
| P( 14) | 5 - 3 | 1711.20 | -921.73 | 3.04366D-01 | 1.03410D-08 | -4.88892D-02 |
| R( 12) | 5 - 4 | 2164.22 | -468.70 | 8.17761D+00 | 1.67641D-06 | 7.25234D-01 |
| P( 14) | 5 - 4 | 2176.80 | -456.12 | 8.23704D+00 | 1.94534D-06 | 7.30616D-01 |

| | | | | | | | |
|---|---|---|---|---|---|---|---|
| R( 12) | 5 - 5 | 2626.90 | -6.02 | 1.35307D-04 | 9.99996D-01 | 2.02746D+00 |
| R( 13) | 5 - 0 | 284.10 | -2355.30 | 6.72960D-05 | 2.15610D-14 | 1.84441D-04 |
| P( 15) | 5 - 0 | 298.04 | -2341.36 | 6.95904D-05 | 2.40351D-14 | 1.82820D-04 |
| R( 13) | 5 - 1 | 761.49 | -1877.92 | 4.99581D-04 | 1.30912D-12 | -7.05867D-04 |
| P( 15) | 5 - 1 | 775.34 | -1864.06 | 4.98400D-04 | 1.42697D-12 | -6.88731D-04 |
| R( 13) | 5 - 2 | 1235.08 | -1404.32 | 6.05410D-03 | 1.02263D-10 | 3.79979D-03 |
| P( 15) | 5 - 2 | 1248.82 | -1390.58 | 5.67728D-03 | 1.12191D-10 | 3.60769D-03 |
| R( 13) | 5 - 3 | 1704.62 | -934.78 | 3.13036D-01 | 1.06921D-08 | -5.03112D-02 |
| P( 15) | 5 - 3 | 1718.24 | -921.16 | 3.02456D-01 | 1.18581D-08 | -4.88406D-02 |
| R( 13) | 5 - 4 | 2170.28 | -469.12 | 8.21794D+00 | 1.94445D-06 | 7.25080D-01 |
| P( 15) | 5 - 4 | 2183.80 | -455.61 | 8.19473D+00 | 2.23350D-06 | 7.30863D-01 |
| R( 13) | 5 - 5 | 2632.92 | -6.48 | 1.69483D-04 | 9.99996D-01 | 2.02785D+00 |
| R( 14) | 5 - 0 | 290.83 | -2355.52 | 6.74820D-05 | 2.47578D-14 | 1.84458D-04 |
| P( 16) | 5 - 0 | 305.73 | -2340.62 | 6.93037D-05 | 2.73032D-14 | 1.82727D-04 |
| R( 14) | 5 - 1 | 768.17 | -1878.17 | 5.00543D-04 | 1.50335D-12 | -7.05589D-04 |
| P( 16) | 5 - 1 | 782.98 | -1863.37 | 4.94663D-04 | 1.62053D-12 | -6.87269D-04 |
| R( 14) | 5 - 2 | 1241.72 | -1404.63 | 6.09449D-03 | 1.17594D-10 | 3.80680D-03 |
| P( 16) | 5 - 2 | 1256.41 | -1389.94 | 5.63765D-03 | 1.27465D-10 | 3.60143D-03 |
| R( 14) | 5 - 3 | 1711.20 | -935.15 | 3.14790D-01 | 1.22900D-08 | -5.03643D-02 |
| P( 16) | 5 - 3 | 1725.76 | -920.59 | 3.00646D-01 | 1.34772D-08 | -4.87921D-02 |
| R( 14) | 5 - 4 | 2176.80 | -469.54 | 8.25549D+00 | 2.23241D-06 | 7.24930D-01 |
| P( 16) | 5 - 4 | 2191.25 | -455.09 | 8.15508D+00 | 2.54163D-06 | 7.31114D-01 |
| R( 14) | 5 - 5 | 2639.40 | -6.94 | 2.08988D-04 | 9.99995D-01 | 2.02827D+00 |
| R( 15) | 5 - 0 | 298.04 | -2355.71 | 6.76454D-05 | 2.81751D-14 | 1.84472D-04 |
| P( 17) | 5 - 0 | 313.89 | -2339.86 | 6.90321D-05 | 3.07722D-14 | 1.82630D-04 |
| R( 15) | 5 - 1 | 775.34 | -1878.41 | 5.01266D-04 | 1.71109D-12 | -7.05249D-04 |
| P( 17) | 5 - 1 | 791.10 | -1862.65 | 4.90975D-04 | 1.82584D-12 | -6.85745D-04 |
| R( 15) | 5 - 2 | 1248.82 | -1404.93 | 6.13331D-03 | 1.34024D-10 | 3.81384D-03 |
| P( 17) | 5 - 2 | 1264.46 | -1389.29 | 5.59963D-03 | 1.43691D-10 | 3.59518D-03 |

|  |  |  |  |  |  |  |
|---|---|---|---|---|---|---|
| R( 15) | 5 - 3 | 1718.24 | -935.51 | 3.16459D-01 | 1.40016D-08 | -5.04176D-02 |
| P( 17) | 5 - 3 | 1733.74 | -920.01 | 2.98917D-01 | 1.51981D-08 | -4.87437D-02 |
| R( 15) | 5 - 4 | 2183.80 | -469.96 | 8.29074D+00 | 2.54031D-06 | 7.24783D-01 |
| P( 17) | 5 - 4 | 2199.18 | -454.58 | 8.11759D+00 | 2.86974D-06 | 7.31368D-01 |
| R( 15) | 5 - 5 | 2646.35 | -7.41 | 2.54214D-04 | 9.99994D-01 | 2.02871D+00 |
| R( 16) | 5 - 0 | 305.73 | -2355.89 | 6.77894D-05 | 3.18127D-14 | 1.84483D-04 |
| P( 18) | 5 - 0 | 322.54 | -2339.08 | 6.87725D-05 | 3.44405D-14 | 1.82531D-04 |
| R( 16) | 5 - 1 | 782.98 | -1878.64 | 5.01771D-04 | 1.93231D-12 | -7.04848D-04 |
| P( 18) | 5 - 1 | 799.69 | -1861.93 | 4.87313D-04 | 2.04258D-12 | -6.84158D-04 |
| R( 16) | 5 - 2 | 1256.41 | -1405.21 | 6.17082D-03 | 1.51560D-10 | 3.82090D-03 |
| P( 18) | 5 - 2 | 1272.99 | -1388.63 | 5.56295D-03 | 1.60864D-10 | 3.58896D-03 |
| R( 16) | 5 - 3 | 1725.76 | -935.86 | 3.18056D-01 | 1.58273D-08 | -5.04710D-02 |
| P( 18) | 5 - 3 | 1742.20 | -919.42 | 2.97256D-01 | 1.70205D-08 | -4.86954D-02 |
| R( 16) | 5 - 4 | 2191.25 | -470.37 | 8.32407D+00 | 2.86815D-06 | 7.24639D-01 |
| P( 18) | 5 - 4 | 2207.56 | -454.06 | 8.08187D+00 | 3.21786D-06 | 7.31625D-01 |
| R( 16) | 5 - 5 | 2653.75 | -7.87 | 3.05550D-04 | 9.99994D-01 | 2.02919D+00 |
| R( 17) | 5 - 0 | 313.89 | -2356.06 | 6.79164D-05 | 3.56702D-14 | 1.84490D-04 |
| P( 19) | 5 - 0 | 331.67 | -2338.28 | 6.85223D-05 | 3.83065D-14 | 1.82429D-04 |
| R( 17) | 5 - 1 | 791.10 | -1878.85 | 5.02078D-04 | 2.16702D-12 | -7.04384D-04 |
| P( 19) | 5 - 1 | 808.76 | -1861.19 | 4.83659D-04 | 2.27099D-12 | -6.82508D-04 |
| R( 17) | 5 - 2 | 1264.46 | -1405.49 | 6.20724D-03 | 1.70208D-10 | 3.82799D-03 |
| P( 19) | 5 - 2 | 1281.99 | -1387.96 | 5.52739D-03 | 1.78982D-10 | 3.58275D-03 |
| R( 17) | 5 - 3 | 1733.74 | -936.21 | 3.19592D-01 | 1.77675D-08 | -5.05246D-02 |
| P( 19) | 5 - 3 | 1751.12 | -918.83 | 2.95651D-01 | 1.89440D-08 | -4.86473D-02 |
| R( 17) | 5 - 4 | 2199.18 | -470.77 | 8.35578D+00 | 3.21597D-06 | 7.24498D-01 |
| P( 19) | 5 - 4 | 2216.42 | -453.53 | 8.04764D+00 | 3.58599D-06 | 7.31886D-01 |
| R( 17) | 5 - 5 | 2661.62 | -8.33 | 3.63389D-04 | 9.99993D-01 | 2.02970D+00 |
| R( 18) | 5 - 0 | 322.54 | -2356.20 | 6.80282D-05 | 3.97470D-14 | 1.84493D-04 |
| P( 20) | 5 - 0 | 341.28 | -2337.46 | 6.82794D-05 | 4.23684D-14 | 1.82324D-04 |

| | | | | | | | |
|---|---|---|---|---|---|---|---|
| R( 18) | 5 - 1 | 799.69 | -1879.05 | 5.02198D-04 | 2.41539D-12 | -7.03856D-04 |
| P( 20) | 5 - 1 | 818.31 | -1860.43 | 4.79997D-04 | 2.51078D-12 | -6.80793D-04 |
| R( 18) | 5 - 2 | 1272.99 | -1405.76 | 6.24274D-03 | 1.89974D-10 | 3.83510D-03 |
| P( 20) | 5 - 2 | 1291.46 | -1387.28 | 5.49279D-03 | 1.98039D-10 | 3.57656D-03 |
| R( 18) | 5 - 3 | 1742.20 | -936.55 | 3.21077D-01 | 1.98228D-08 | -5.05783D-02 |
| P( 20) | 5 - 3 | 1760.51 | -918.23 | 2.94093D-01 | 2.09684D-08 | -4.85992D-02 |
| R( 18) | 5 - 4 | 2207.56 | -471.18 | 8.38610D+00 | 3.58377D-06 | 7.24361D-01 |
| P( 20) | 5 - 4 | 2225.74 | -453.01 | 8.01465D+00 | 3.97417D-06 | 7.32150D-01 |
| R( 18) | 5 - 5 | 2669.95 | -8.79 | 4.28124D-04 | 9.99992D-01 | 2.03023D+00 |
| R( 19) | 5 - 0 | 331.67 | -2356.33 | 6.81264D-05 | 4.40425D-14 | 1.84493D-04 |
| P( 21) | 5 - 0 | 351.37 | -2336.63 | 6.80422D-05 | 4.66244D-14 | 1.82216D-04 |
| R( 19) | 5 - 1 | 808.76 | -1879.23 | 5.02144D-04 | 2.67702D-12 | -7.03265D-04 |
| P( 21) | 5 - 1 | 828.34 | -1859.66 | 4.76317D-04 | 2.76181D-12 | -6.79014D-04 |
| R( 19) | 5 - 2 | 1281.99 | -1406.01 | 6.27745D-03 | 2.10864D-10 | 3.84224D-03 |
| P( 21) | 5 - 2 | 1301.41 | -1386.59 | 5.45901D-03 | 2.18033D-10 | 3.57039D-03 |
| R( 19) | 5 - 3 | 1751.12 | -936.88 | 3.22518D-01 | 2.19937D-08 | -5.06322D-02 |
| P( 21) | 5 - 3 | 1770.37 | -917.63 | 2.92576D-01 | 2.30933D-08 | -4.85512D-02 |
| R( 19) | 5 - 4 | 2216.42 | -471.58 | 8.41523D+00 | 3.97159D-06 | 7.24226D-01 |
| P( 21) | 5 - 4 | 2235.52 | -452.48 | 7.98272D+00 | 4.38242D-06 | 7.32418D-01 |
| R( 19) | 5 - 5 | 2678.74 | -9.25 | 5.00149D-04 | 9.99991D-01 | 2.03080D+00 |
| Q( 0) | 0 - 0 | 240.35 | 0.00 | 0.00000D+00 | 1.00000D+00 | -1.62108D+00 |
| Q( 1) | 0 - 0 | 240.84 | -0.00 | 0.00000D+00 | 1.00000D+00 | -1.62110D+00 |
| Q( 2) | 0 - 0 | 241.80 | -0.00 | 0.00000D+00 | 1.00000D+00 | -1.62116D+00 |
| Q( 3) | 0 - 0 | 243.24 | 0.00 | 0.00000D+00 | 1.00000D+00 | -1.62125D+00 |
| Q( 4) | 0 - 0 | 245.16 | 0.00 | 0.00000D+00 | 1.00000D+00 | -1.62137D+00 |
| Q( 5) | 0 - 0 | 247.57 | 0.00 | 0.00000D+00 | 1.00000D+00 | -1.62151D+00 |
| Q( 6) | 0 - 0 | 250.45 | 0.00 | 0.00000D+00 | 1.00000D+00 | -1.62169D+00 |
| Q( 7) | 0 - 0 | 253.82 | 0.00 | 0.00000D+00 | 1.00000D+00 | -1.62189D+00 |
| Q( 8) | 0 - 0 | 257.66 | 0.00 | 0.00000D+00 | 1.00000D+00 | -1.62212D+00 |

| | | | | | | |
|---|---|---|---|---|---|---|
| Q( 9) | 0 - 0 | 261.99 | 0.00 | 0.00000D+00 | 1.00000D+00 | -1.62238D+00 |
| Q( 10) | 0 - 0 | 266.80 | 0.00 | 0.00000D+00 | 1.00000D+00 | -1.62268D+00 |
| Q( 11) | 0 - 0 | 272.08 | 0.00 | 0.00000D+00 | 1.00000D+00 | -1.62300D+00 |
| Q( 12) | 0 - 0 | 277.85 | 0.00 | 0.00000D+00 | 1.00000D+00 | -1.62334D+00 |
| Q( 13) | 0 - 0 | 284.10 | 0.00 | 0.00000D+00 | 1.00000D+00 | -1.62372D+00 |
| Q( 14) | 0 - 0 | 290.83 | 0.00 | 0.00000D+00 | 1.00000D+00 | -1.62413D+00 |
| Q( 15) | 0 - 0 | 298.04 | 0.00 | 0.00000D+00 | 1.00000D+00 | -1.62457D+00 |
| Q( 16) | 0 - 0 | 305.73 | 0.00 | 0.00000D+00 | 1.00000D+00 | -1.62503D+00 |
| Q( 17) | 0 - 0 | 313.89 | 0.00 | 0.00000D+00 | 1.00000D+00 | -1.62553D+00 |
| Q( 18) | 0 - 0 | 322.54 | 0.00 | 0.00000D+00 | 1.00000D+00 | -1.62605D+00 |
| Q( 19) | 0 - 0 | 331.67 | 0.00 | 0.00000D+00 | 1.00000D+00 | -1.62660D+00 |
| Q( 20) | 0 - 0 | 341.28 | 0.00 | 0.00000D+00 | 1.00000D+00 | -1.62719D+00 |
| Q( 0) | 1 - 0 | 240.35 | -477.66 | 0.00000D+00 | 2.82549D-17 | 3.23366D-01 |
| Q( 0) | 1 - 1 | 718.01 | 0.00 | 0.00000D+00 | 1.00000D+00 | 1.69227D+00 |
| Q( 1) | 1 - 0 | 240.84 | -477.65 | 0.00000D+00 | 3.88720D-17 | 3.23367D-01 |
| Q( 1) | 1 - 1 | 718.49 | -0.00 | 0.00000D+00 | 1.00000D+00 | 1.69230D+00 |
| Q( 2) | 1 - 0 | 241.80 | -477.65 | 0.00000D+00 | 9.82651D-17 | 3.23370D-01 |
| Q( 2) | 1 - 1 | 719.45 | -0.00 | 0.00000D+00 | 1.00000D+00 | 1.69236D+00 |
| Q( 3) | 1 - 0 | 243.24 | -477.64 | 0.00000D+00 | 1.65364D-19 | 3.23374D-01 |
| Q( 3) | 1 - 1 | 720.88 | 0.00 | 0.00000D+00 | 1.00000D+00 | 1.69245D+00 |
| Q( 4) | 1 - 0 | 245.16 | -477.63 | 0.00000D+00 | 1.65110D-19 | 3.23380D-01 |
| Q( 4) | 1 - 1 | 722.79 | 0.00 | 0.00000D+00 | 1.00000D+00 | 1.69256D+00 |
| Q( 5) | 1 - 0 | 247.57 | -477.61 | 0.00000D+00 | 1.64753D-19 | 3.23387D-01 |
| Q( 5) | 1 - 1 | 725.18 | 0.00 | 0.00000D+00 | 1.00000D+00 | 1.69271D+00 |
| Q( 6) | 1 - 0 | 250.45 | -477.59 | 0.00000D+00 | 1.64377D-19 | 3.23396D-01 |
| Q( 6) | 1 - 1 | 728.05 | 0.00 | 0.00000D+00 | 1.00000D+00 | 1.69288D+00 |
| Q( 7) | 1 - 0 | 253.82 | -477.57 | 0.00000D+00 | 1.63960D-19 | 3.23406D-01 |
| Q( 7) | 1 - 1 | 731.39 | 0.00 | 0.00000D+00 | 1.00000D+00 | 1.69309D+00 |
| Q( 8) | 1 - 0 | 257.66 | -477.55 | 0.00000D+00 | 1.63474D-19 | 3.23417D-01 |

| | | | | | | | |
|---|---|---|---|---|---|---|---|
| Q( 8) | 1 - 1 | 735.21 | 0.00 | 0.00000D+00 | 1.00000D+00 | 1.69332D+00 |
| Q( 9) | 1 - 0 | 261.99 | -477.52 | 0.00000D+00 | 1.68296D-19 | 3.23430D-01 |
| Q( 9) | 1 - 1 | 739.51 | 0.00 | 0.00000D+00 | 1.00000D+00 | 1.69359D+00 |
| Q( 10) | 1 - 0 | 266.80 | -477.49 | 0.00000D+00 | 1.67697D-19 | 3.23444D-01 |
| Q( 10) | 1 - 1 | 744.29 | 0.00 | 0.00000D+00 | 1.00000D+00 | 1.69388D+00 |
| Q( 11) | 1 - 0 | 272.08 | -477.46 | 0.00000D+00 | 1.67022D-19 | 3.23459D-01 |
| Q( 11) | 1 - 1 | 749.54 | 0.00 | 0.00000D+00 | 1.00000D+00 | 1.69420D+00 |
| Q( 12) | 1 - 0 | 277.85 | -477.42 | 0.00000D+00 | 1.66284D-19 | 3.23476D-01 |
| Q( 12) | 1 - 1 | 755.28 | 0.00 | 0.00000D+00 | 1.00000D+00 | 1.69455D+00 |
| Q( 13) | 1 - 0 | 284.10 | -477.39 | 0.00000D+00 | 1.65525D-19 | 3.23495D-01 |
| Q( 13) | 1 - 1 | 761.49 | 0.00 | 0.00000D+00 | 1.00000D+00 | 1.69493D+00 |
| Q( 14) | 1 - 0 | 290.83 | -477.34 | 0.00000D+00 | 1.64734D-19 | 3.23514D-01 |
| Q( 14) | 1 - 1 | 768.17 | 0.00 | 0.00000D+00 | 1.00000D+00 | 1.69535D+00 |
| Q( 15) | 1 - 0 | 298.04 | -477.30 | 0.00000D+00 | 1.63864D-19 | 3.23536D-01 |
| Q( 15) | 1 - 1 | 775.34 | 0.00 | 0.00000D+00 | 1.00000D+00 | 1.69578D+00 |
| Q( 16) | 1 - 0 | 305.73 | -477.25 | 0.00000D+00 | 1.62966D-19 | 3.23558D-01 |
| Q( 16) | 1 - 1 | 782.98 | 0.00 | 0.00000D+00 | 1.00000D+00 | 1.69625D+00 |
| Q( 17) | 1 - 0 | 313.89 | -477.20 | 0.00000D+00 | 1.62057D-19 | 3.23582D-01 |
| Q( 17) | 1 - 1 | 791.10 | 0.00 | 0.00000D+00 | 1.00000D+00 | 1.69675D+00 |
| Q( 18) | 1 - 0 | 322.54 | -477.15 | 0.00000D+00 | 1.61109D-19 | 3.23608D-01 |
| Q( 18) | 1 - 1 | 799.69 | 0.00 | 0.00000D+00 | 1.00000D+00 | 1.69728D+00 |
| Q( 19) | 1 - 0 | 331.67 | -477.09 | 0.00000D+00 | 1.60118D-19 | 3.23635D-01 |
| Q( 19) | 1 - 1 | 808.76 | 0.00 | 0.00000D+00 | 1.00000D+00 | 1.69784D+00 |
| Q( 20) | 1 - 0 | 341.28 | -477.03 | 0.00000D+00 | 1.59116D-19 | 3.23663D-01 |
| Q( 20) | 1 - 1 | 818.31 | 0.00 | 0.00000D+00 | 1.00000D+00 | 1.69843D+00 |
| Q( 0) | 2 - 0 | 240.35 | -951.60 | 0.00000D+00 | 1.77851D-21 | 1.24636D-02 |
| Q( 0) | 2 - 1 | 718.01 | -473.94 | 0.00000D+00 | 2.50733D-16 | -4.58053D-01 |
| Q( 0) | 2 - 2 | 1191.95 | 0.00 | 0.00000D+00 | 1.00000D+00 | -1.77594D+00 |
| Q( 1) | 2 - 0 | 240.84 | -951.59 | 0.00000D+00 | 2.87646D-20 | 1.24637D-02 |

| | | | | | | |
|---|---|---|---|---|---|---|
| Q( 1) | 2 - 1 | 718.49 | -473.94 | 0.00000D+00 | 2.87652D-16 | -4.58055D-01 |
| Q( 1) | 2 - 2 | 1192.42 | -0.00 | 0.00000D+00 | 1.00000D+00 | -1.77597D+00 |
| Q( 2) | 2 - 0 | 241.80 | -951.58 | 0.00000D+00 | 1.03328D-18 | 1.24639D-02 |
| Q( 2) | 2 - 1 | 719.45 | -473.93 | 0.00000D+00 | 4.60931D-16 | -4.58060D-01 |
| Q( 2) | 2 - 2 | 1193.37 | -0.00 | 0.00000D+00 | 1.00000D+00 | -1.77603D+00 |
| Q( 3) | 2 - 0 | 243.24 | -951.56 | 0.00000D+00 | 2.92660D-21 | 1.24643D-02 |
| Q( 3) | 2 - 1 | 720.88 | -473.92 | 0.00000D+00 | 2.48090D-16 | -4.58067D-01 |
| Q( 3) | 2 - 2 | 1194.79 | 0.00 | 0.00000D+00 | 1.00000D+00 | -1.77612D+00 |
| Q( 4) | 2 - 0 | 245.16 | -951.53 | 0.00000D+00 | 2.91249D-21 | 1.24647D-02 |
| Q( 4) | 2 - 1 | 722.79 | -473.90 | 0.00000D+00 | 2.47691D-16 | -4.58077D-01 |
| Q( 4) | 2 - 2 | 1196.69 | 0.00 | 0.00000D+00 | 1.00000D+00 | -1.77623D+00 |
| Q( 5) | 2 - 0 | 247.57 | -951.49 | 0.00000D+00 | 2.89344D-21 | 1.24653D-02 |
| Q( 5) | 2 - 1 | 725.18 | -473.88 | 0.00000D+00 | 2.47195D-16 | -4.58089D-01 |
| Q( 5) | 2 - 2 | 1199.06 | 0.00 | 0.00000D+00 | 1.00000D+00 | -1.77638D+00 |
| Q( 6) | 2 - 0 | 250.45 | -951.45 | 0.00000D+00 | 2.87151D-21 | 1.24660D-02 |
| Q( 6) | 2 - 1 | 728.05 | -473.86 | 0.00000D+00 | 2.46601D-16 | -4.58103D-01 |
| Q( 6) | 2 - 2 | 1201.91 | 0.00 | 0.00000D+00 | 1.00000D+00 | -1.77656D+00 |
| Q( 7) | 2 - 0 | 253.82 | -951.41 | 0.00000D+00 | 2.84699D-21 | 1.24669D-02 |
| Q( 7) | 2 - 1 | 731.39 | -473.83 | 0.00000D+00 | 2.45913D-16 | -4.58120D-01 |
| Q( 7) | 2 - 2 | 1205.22 | 0.00 | 0.00000D+00 | 1.00000D+00 | -1.77676D+00 |
| Q( 8) | 2 - 0 | 257.66 | -951.35 | 0.00000D+00 | 2.81821D-21 | 1.24678D-02 |
| Q( 8) | 2 - 1 | 735.21 | -473.80 | 0.00000D+00 | 2.45132D-16 | -4.58139D-01 |
| Q( 8) | 2 - 2 | 1209.02 | 0.00 | 0.00000D+00 | 1.00000D+00 | -1.77700D+00 |
| Q( 9) | 2 - 0 | 261.99 | -951.29 | 0.00000D+00 | 3.43358D-21 | 1.24689D-02 |
| Q( 9) | 2 - 1 | 739.51 | -473.77 | 0.00000D+00 | 2.44256D-16 | -4.58160D-01 |
| Q( 9) | 2 - 2 | 1213.28 | 0.00 | 0.00000D+00 | 1.00000D+00 | -1.77726D+00 |
| Q( 10) | 2 - 0 | 266.80 | -951.23 | 0.00000D+00 | 3.39498D-21 | 1.24701D-02 |
| Q( 10) | 2 - 1 | 744.29 | -473.73 | 0.00000D+00 | 2.43292D-16 | -4.58184D-01 |
| Q( 10) | 2 - 2 | 1218.02 | 0.00 | 0.00000D+00 | 1.00000D+00 | -1.77756D+00 |

| | | | | | | | |
|---|---|---|---|---|---|---|---|
| Q( 11) | 2 - 0 | 272.08 | -951.15 | 0.00000D+00 | 3.34961D-21 | 1.24714D-02 |
| Q( 11) | 2 - 1 | 749.54 | -473.69 | 0.00000D+00 | 2.42240D-16 | -4.58210D-01 |
| Q( 11) | 2 - 2 | 1223.23 | 0.00 | 0.00000D+00 | 1.00000D+00 | -1.77788D+00 |
| Q( 12) | 2 - 0 | 277.85 | -951.07 | 0.00000D+00 | 3.30233D-21 | 1.24728D-02 |
| Q( 12) | 2 - 1 | 755.28 | -473.65 | 0.00000D+00 | 2.41103D-16 | -4.58239D-01 |
| Q( 12) | 2 - 2 | 1228.92 | 0.00 | 0.00000D+00 | 1.00000D+00 | -1.77823D+00 |
| Q( 13) | 2 - 0 | 284.10 | -950.98 | 0.00000D+00 | 3.25037D-21 | 1.24744D-02 |
| Q( 13) | 2 - 1 | 761.49 | -473.60 | 0.00000D+00 | 2.39883D-16 | -4.58269D-01 |
| Q( 13) | 2 - 2 | 1235.08 | 0.00 | 0.00000D+00 | 1.00000D+00 | -1.77862D+00 |
| Q( 14) | 2 - 0 | 290.83 | -950.89 | 0.00000D+00 | 3.19471D-21 | 1.24761D-02 |
| Q( 14) | 2 - 1 | 768.17 | -473.54 | 0.00000D+00 | 2.38584D-16 | -4.58303D-01 |
| Q( 14) | 2 - 2 | 1241.72 | 0.00 | 0.00000D+00 | 1.00000D+00 | -1.77903D+00 |
| Q( 15) | 2 - 0 | 298.04 | -950.79 | 0.00000D+00 | 3.13793D-21 | 1.24779D-02 |
| Q( 15) | 2 - 1 | 775.34 | -473.49 | 0.00000D+00 | 2.37208D-16 | -4.58338D-01 |
| Q( 15) | 2 - 2 | 1248.82 | 0.00 | 0.00000D+00 | 1.00000D+00 | -1.77947D+00 |
| Q( 16) | 2 - 0 | 305.73 | -950.68 | 0.00000D+00 | 3.07539D-21 | 1.24799D-02 |
| Q( 16) | 2 - 1 | 782.98 | -473.43 | 0.00000D+00 | 2.35758D-16 | -4.58376D-01 |
| Q( 16) | 2 - 2 | 1256.41 | 0.00 | 0.00000D+00 | 1.00000D+00 | -1.77994D+00 |
| Q( 17) | 2 - 0 | 313.89 | -950.57 | 0.00000D+00 | 3.01104D-21 | 1.24820D-02 |
| Q( 17) | 2 - 1 | 791.10 | -473.36 | 0.00000D+00 | 2.34238D-16 | -4.58417D-01 |
| Q( 17) | 2 - 2 | 1264.46 | 0.00 | 0.00000D+00 | 1.00000D+00 | -1.78044D+00 |
| Q( 18) | 2 - 0 | 322.54 | -950.44 | 0.00000D+00 | 2.94423D-21 | 1.24842D-02 |
| Q( 18) | 2 - 1 | 799.69 | -473.30 | 0.00000D+00 | 2.39038D-16 | -4.58460D-01 |
| Q( 18) | 2 - 2 | 1272.99 | 0.00 | 0.00000D+00 | 1.00000D+00 | -1.78097D+00 |
| Q( 19) | 2 - 0 | 331.67 | -950.32 | 0.00000D+00 | 2.87441D-21 | 1.24866D-02 |
| Q( 19) | 2 - 1 | 808.76 | -473.22 | 0.00000D+00 | 2.37350D-16 | -4.58505D-01 |
| Q( 19) | 2 - 2 | 1281.99 | 0.00 | 0.00000D+00 | 1.00000D+00 | -1.78153D+00 |
| Q( 20) | 2 - 0 | 341.28 | -950.18 | 0.00000D+00 | 2.80003D-21 | 1.24891D-02 |
| Q( 20) | 2 - 1 | 818.31 | -473.15 | 0.00000D+00 | 2.35601D-16 | -4.58552D-01 |

| | | | | | | |
|---|---|---|---|---|---|---|
| Q( 20) | 2 - 2 | 1291.46 | 0.00 | 0.00000D+00 | 1.00000D+00 | -1.78212D+00 |
| Q( 0) | 3 - 0 | 240.35 | -1421.51 | 0.00000D+00 | 8.41790D-21 | 6.59070D-04 |
| Q( 0) | 3 - 1 | 718.01 | -943.85 | 0.00000D+00 | 2.57016D-17 | -2.50887D-02 |
| Q( 0) | 3 - 2 | 1191.95 | -469.91 | 0.00000D+00 | 4.72589D-20 | 5.61759D-01 |
| Q( 0) | 3 - 3 | 1661.86 | 0.00 | 0.00000D+00 | 1.00000D+00 | 1.86552D+00 |
| Q( 1) | 3 - 0 | 240.84 | -1421.50 | 0.00000D+00 | 5.08525D-22 | 6.58965D-04 |
| Q( 1) | 3 - 1 | 718.49 | -943.84 | 0.00000D+00 | 2.26328D-17 | -2.50889D-02 |
| Q( 1) | 3 - 2 | 1192.42 | -469.91 | 0.00000D+00 | 2.16728D-18 | 5.61762D-01 |
| Q( 1) | 3 - 3 | 1662.33 | -0.00 | 0.00000D+00 | 1.00000D+00 | 1.86555D+00 |
| Q( 2) | 3 - 0 | 241.80 | -1421.47 | 0.00000D+00 | 6.46134D-20 | 6.58756D-04 |
| Q( 2) | 3 - 1 | 719.45 | -943.83 | 0.00000D+00 | 1.23356D-17 | -2.50893D-02 |
| Q( 2) | 3 - 2 | 1193.37 | -469.90 | 0.00000D+00 | 4.21300D-17 | 5.61768D-01 |
| Q( 2) | 3 - 3 | 1663.27 | -0.00 | 0.00000D+00 | 1.00000D+00 | 1.86561D+00 |
| Q( 3) | 3 - 0 | 243.24 | -1421.44 | 0.00000D+00 | 8.92403D-21 | 6.58442D-04 |
| Q( 3) | 3 - 1 | 720.88 | -943.80 | 0.00000D+00 | 2.57164D-17 | -2.50898D-02 |
| Q( 3) | 3 - 2 | 1194.79 | -469.89 | 0.00000D+00 | 2.78336D-20 | 5.61777D-01 |
| Q( 3) | 3 - 3 | 1664.68 | 0.00 | 0.00000D+00 | 1.00000D+00 | 1.86570D+00 |
| Q( 4) | 3 - 0 | 245.16 | -1421.40 | 0.00000D+00 | 8.91692D-21 | 6.58024D-04 |
| Q( 4) | 3 - 1 | 722.79 | -943.77 | 0.00000D+00 | 2.56423D-17 | -2.50905D-02 |
| Q( 4) | 3 - 2 | 1196.69 | -469.87 | 0.00000D+00 | 2.77796D-20 | 5.61790D-01 |
| Q( 4) | 3 - 3 | 1666.56 | 0.00 | 0.00000D+00 | 1.00000D+00 | 1.86582D+00 |
| Q( 5) | 3 - 0 | 247.57 | -1421.34 | 0.00000D+00 | 8.90629D-21 | 6.57501D-04 |
| Q( 5) | 3 - 1 | 725.18 | -943.73 | 0.00000D+00 | 2.55499D-17 | -2.50914D-02 |
| Q( 5) | 3 - 2 | 1199.06 | -469.85 | 0.00000D+00 | 2.77234D-20 | 5.61805D-01 |
| Q( 5) | 3 - 3 | 1668.91 | 0.00 | 0.00000D+00 | 1.00000D+00 | 1.86596D+00 |
| Q( 6) | 3 - 0 | 250.45 | -1421.28 | 0.00000D+00 | 8.89436D-21 | 6.56874D-04 |
| Q( 6) | 3 - 1 | 728.05 | -943.68 | 0.00000D+00 | 2.54395D-17 | -2.50925D-02 |
| Q( 6) | 3 - 2 | 1201.91 | -469.82 | 0.00000D+00 | 2.76681D-20 | 5.61824D-01 |
| Q( 6) | 3 - 3 | 1671.73 | 0.00 | 0.00000D+00 | 1.00000D+00 | 1.86614D+00 |

| | | | | | | | |
|---|---|---|---|---|---|---|---|
| Q( 7) | 3 - 0 | 253.82 | -1421.20 | 0.00000D+00 | 8.88131D-21 | 6.56143D-04 |
| Q( 7) | 3 - 1 | 731.39 | -943.63 | 0.00000D+00 | 2.53116D-17 | -2.50938D-02 |
| Q( 7) | 3 - 2 | 1205.22 | -469.80 | 0.00000D+00 | 2.75960D-20 | 5.61846D-01 |
| Q( 7) | 3 - 3 | 1675.02 | 0.00 | 0.00000D+00 | 1.00000D+00 | 1.86635D+00 |
| Q( 8) | 3 - 0 | 257.66 | -1421.12 | 0.00000D+00 | 8.86690D-21 | 6.55308D-04 |
| Q( 8) | 3 - 1 | 735.21 | -943.57 | 0.00000D+00 | 2.51662D-17 | -2.50953D-02 |
| Q( 8) | 3 - 2 | 1209.02 | -469.76 | 0.00000D+00 | 2.75121D-20 | 5.61871D-01 |
| Q( 8) | 3 - 3 | 1678.78 | 0.00 | 0.00000D+00 | 1.00000D+00 | 1.86658D+00 |
| Q( 9) | 3 - 0 | 261.99 | -1421.02 | 0.00000D+00 | 8.77905D-21 | 6.54369D-04 |
| Q( 9) | 3 - 1 | 739.51 | -943.49 | 0.00000D+00 | 2.50037D-17 | -2.50969D-02 |
| Q( 9) | 3 - 2 | 1213.28 | -469.73 | 0.00000D+00 | 2.74356D-20 | 5.61899D-01 |
| Q( 9) | 3 - 3 | 1683.01 | 0.00 | 0.00000D+00 | 1.00000D+00 | 1.86685D+00 |
| Q( 10) | 3 - 0 | 266.80 | -1420.91 | 0.00000D+00 | 8.76274D-21 | 6.53327D-04 |
| Q( 10) | 3 - 1 | 744.29 | -943.42 | 0.00000D+00 | 2.48246D-17 | -2.50988D-02 |
| Q( 10) | 3 - 2 | 1218.02 | -469.68 | 0.00000D+00 | 2.73321D-20 | 5.61930D-01 |
| Q( 10) | 3 - 3 | 1687.71 | 0.00 | 0.00000D+00 | 1.00000D+00 | 1.86714D+00 |
| Q( 11) | 3 - 0 | 272.08 | -1420.79 | 0.00000D+00 | 8.74254D-21 | 6.52182D-04 |
| Q( 11) | 3 - 1 | 749.54 | -943.33 | 0.00000D+00 | 2.46293D-17 | -2.51008D-02 |
| Q( 11) | 3 - 2 | 1223.23 | -469.64 | 0.00000D+00 | 2.79145D-20 | 5.61964D-01 |
| Q( 11) | 3 - 3 | 1692.87 | 0.00 | 0.00000D+00 | 1.00000D+00 | 1.86747D+00 |
| Q( 12) | 3 - 0 | 277.85 | -1420.66 | 0.00000D+00 | 8.72221D-21 | 6.50933D-04 |
| Q( 12) | 3 - 1 | 755.28 | -943.24 | 0.00000D+00 | 2.44184D-17 | -2.51030D-02 |
| Q( 12) | 3 - 2 | 1228.92 | -469.59 | 0.00000D+00 | 2.78145D-20 | 5.62001D-01 |
| Q( 12) | 3 - 3 | 1698.51 | 0.00 | 0.00000D+00 | 1.00000D+00 | 1.86782D+00 |
| Q( 13) | 3 - 0 | 284.10 | -1420.52 | 0.00000D+00 | 8.69927D-21 | 6.49582D-04 |
| Q( 13) | 3 - 1 | 761.49 | -943.13 | 0.00000D+00 | 2.41920D-17 | -2.51054D-02 |
| Q( 13) | 3 - 2 | 1235.08 | -469.54 | 0.00000D+00 | 2.76900D-20 | 5.62042D-01 |
| Q( 13) | 3 - 3 | 1704.62 | 0.00 | 0.00000D+00 | 1.00000D+00 | 1.86821D+00 |
| Q( 14) | 3 - 0 | 290.83 | -1420.37 | 0.00000D+00 | 8.67453D-21 | 6.48129D-04 |

| | | | | | | |
|---|---|---|---|---|---|---|
| Q( 14) | 3 - 1 | 768.17 | -943.02 | 0.00000D+00 | 2.39510D-17 | -2.51080D-02 |
| Q( 14) | 3 - 2 | 1241.72 | -469.48 | 0.00000D+00 | 2.75805D-20 | 5.62085D-01 |
| Q( 14) | 3 - 3 | 1711.20 | 0.00 | 0.00000D+00 | 1.00000D+00 | 1.86862D+00 |
| Q( 15) | 3 - 0 | 298.04 | -1420.20 | 0.00000D+00 | 8.64817D-21 | 6.46573D-04 |
| Q( 15) | 3 - 1 | 775.34 | -942.90 | 0.00000D+00 | 2.36959D-17 | -2.51108D-02 |
| Q( 15) | 3 - 2 | 1248.82 | -469.42 | 0.00000D+00 | 2.74533D-20 | 5.62132D-01 |
| Q( 15) | 3 - 3 | 1718.24 | 0.00 | 0.00000D+00 | 1.00000D+00 | 1.86906D+00 |
| Q( 16) | 3 - 0 | 305.73 | -1420.03 | 0.00000D+00 | 8.61939D-21 | 6.44917D-04 |
| Q( 16) | 3 - 1 | 782.98 | -942.78 | 0.00000D+00 | 2.34272D-17 | -2.51138D-02 |
| Q( 16) | 3 - 2 | 1256.41 | -469.35 | 0.00000D+00 | 2.73302D-20 | 5.62182D-01 |
| Q( 16) | 3 - 3 | 1725.76 | 0.00 | 0.00000D+00 | 1.00000D+00 | 1.86954D+00 |
| Q( 17) | 3 - 0 | 313.89 | -1419.85 | 0.00000D+00 | 8.59092D-21 | 6.43159D-04 |
| Q( 17) | 3 - 1 | 791.10 | -942.65 | 0.00000D+00 | 2.31456D-17 | -2.51170D-02 |
| Q( 17) | 3 - 2 | 1264.46 | -469.28 | 0.00000D+00 | 2.72098D-20 | 5.62235D-01 |
| Q( 17) | 3 - 3 | 1733.74 | 0.00 | 0.00000D+00 | 1.00000D+00 | 1.87004D+00 |
| Q( 18) | 3 - 0 | 322.54 | -1419.65 | 0.00000D+00 | 8.55442D-21 | 6.41300D-04 |
| Q( 18) | 3 - 1 | 799.69 | -942.50 | 0.00000D+00 | 2.51250D-17 | -2.51204D-02 |
| Q( 18) | 3 - 2 | 1272.99 | -469.21 | 0.00000D+00 | 2.73382D-20 | 5.62291D-01 |
| Q( 18) | 3 - 3 | 1742.20 | 0.00 | 0.00000D+00 | 1.00000D+00 | 1.87057D+00 |
| Q( 19) | 3 - 0 | 331.67 | -1419.45 | 0.00000D+00 | 8.51935D-21 | 6.39341D-04 |
| Q( 19) | 3 - 1 | 808.76 | -942.35 | 0.00000D+00 | 2.47960D-17 | -2.51240D-02 |
| Q( 19) | 3 - 2 | 1281.99 | -469.13 | 0.00000D+00 | 2.72387D-20 | 5.62350D-01 |
| Q( 19) | 3 - 3 | 1751.12 | 0.00 | 0.00000D+00 | 1.00000D+00 | 1.87113D+00 |
| Q( 20) | 3 - 0 | 341.28 | -1419.23 | 0.00000D+00 | 8.48303D-21 | 6.37283D-04 |
| Q( 20) | 3 - 1 | 818.31 | -942.20 | 0.00000D+00 | 2.44552D-17 | -2.51278D-02 |
| Q( 20) | 3 - 2 | 1291.46 | -469.05 | 0.00000D+00 | 2.71595D-20 | 5.62412D-01 |
| Q( 20) | 3 - 3 | 1760.51 | 0.00 | 0.00000D+00 | 1.00000D+00 | 1.87172D+00 |
| Q( 0) | 4 - 0 | 240.35 | -1887.50 | 0.00000D+00 | 1.37720D-21 | 3.63254D-04 |
| Q( 0) | 4 - 1 | 718.01 | -1409.84 | 0.00000D+00 | 2.72253D-18 | -1.96345D-03 |

| | | | | | | | |
|---|---|---|---|---|---|---|---|
| Q( 0) | 4 - 2 | 1191.95 | -935.90 | 0.00000D+00 | 4.13751D-21 | 3.85661D-02 |
| Q( 0) | 4 - 3 | 1661.86 | -465.99 | 0.00000D+00 | 1.39051D-20 | -6.49712D-01 |
| Q( 0) | 4 - 4 | 2127.85 | 0.00 | 0.00000D+00 | 1.00000D+00 | -1.94873D+00 |
| Q( 1) | 4 - 0 | 240.84 | -1887.48 | 0.00000D+00 | 3.95522D-21 | 3.63213D-04 |
| Q( 1) | 4 - 1 | 718.49 | -1409.83 | 0.00000D+00 | 2.36631D-18 | -1.96332D-03 |
| Q( 1) | 4 - 2 | 1192.42 | -935.90 | 0.00000D+00 | 9.55687D-20 | 3.85663D-02 |
| Q( 1) | 4 - 3 | 1662.33 | -465.99 | 0.00000D+00 | 2.06207D-18 | -6.49715D-01 |
| Q( 1) | 4 - 4 | 2128.32 | -0.00 | 0.00000D+00 | 1.00000D+00 | -1.94876D+00 |
| Q( 2) | 4 - 0 | 241.80 | -1887.46 | 0.00000D+00 | 2.75586D-20 | 3.63132D-04 |
| Q( 2) | 4 - 1 | 719.45 | -1409.81 | 0.00000D+00 | 1.18991D-18 | -1.96306D-03 |
| Q( 2) | 4 - 2 | 1193.37 | -935.88 | 0.00000D+00 | 3.24954D-18 | 3.85668D-02 |
| Q( 2) | 4 - 3 | 1663.27 | -465.98 | 0.00000D+00 | 4.49946D-17 | -6.49722D-01 |
| Q( 2) | 4 - 4 | 2129.25 | -0.00 | 0.00000D+00 | 1.00000D+00 | -1.94882D+00 |
| Q( 3) | 4 - 0 | 243.24 | -1887.41 | 0.00000D+00 | 1.36571D-21 | 3.63009D-04 |
| Q( 3) | 4 - 1 | 720.88 | -1409.77 | 0.00000D+00 | 2.72945D-18 | -1.96267D-03 |
| Q( 3) | 4 - 2 | 1194.79 | -935.86 | 0.00000D+00 | 4.20027D-21 | 3.85675D-02 |
| Q( 3) | 4 - 3 | 1664.68 | -465.97 | 0.00000D+00 | 1.33639D-20 | -6.49732D-01 |
| Q( 3) | 4 - 4 | 2130.65 | 0.00 | 0.00000D+00 | 1.00000D+00 | -1.94891D+00 |
| Q( 4) | 4 - 0 | 245.16 | -1887.35 | 0.00000D+00 | 1.36018D-21 | 3.62846D-04 |
| Q( 4) | 4 - 1 | 722.79 | -1409.73 | 0.00000D+00 | 2.73364D-18 | -1.96215D-03 |
| Q( 4) | 4 - 2 | 1196.69 | -935.83 | 0.00000D+00 | 4.18811D-21 | 3.85684D-02 |
| Q( 4) | 4 - 3 | 1666.56 | -465.96 | 0.00000D+00 | 1.33451D-20 | -6.49745D-01 |
| Q( 4) | 4 - 4 | 2132.52 | 0.00 | 0.00000D+00 | 1.00000D+00 | -1.94902D+00 |
| Q( 5) | 4 - 0 | 247.57 | -1887.28 | 0.00000D+00 | 1.35283D-21 | 3.62642D-04 |
| Q( 5) | 4 - 1 | 725.18 | -1409.67 | 0.00000D+00 | 2.73886D-18 | -1.96150D-03 |
| Q( 5) | 4 - 2 | 1199.06 | -935.79 | 0.00000D+00 | 4.17225D-21 | 3.85695D-02 |
| Q( 5) | 4 - 3 | 1668.91 | -465.94 | 0.00000D+00 | 1.33182D-20 | -6.49761D-01 |
| Q( 5) | 4 - 4 | 2134.85 | 0.00 | 0.00000D+00 | 1.00000D+00 | -1.94917D+00 |
| Q( 6) | 4 - 0 | 250.45 | -1887.19 | 0.00000D+00 | 1.34473D-21 | 3.62397D-04 |

| | | | | | | | |
|---|---|---|---|---|---|---|---|
| Q( 6) | 4 - 1 | 728.05 | -1409.60 | 0.00000D+00 | 2.74512D-18 | -1.96072D-03 |
| Q( 6) | 4 - 2 | 1201.91 | -935.74 | 0.00000D+00 | 4.15651D-21 | 3.85708D-02 |
| Q( 6) | 4 - 3 | 1671.73 | -465.92 | 0.00000D+00 | 1.32921D-20 | -6.49781D-01 |
| Q( 6) | 4 - 4 | 2137.65 | 0.00 | 0.00000D+00 | 1.00000D+00 | -1.94935D+00 |
| Q( 7) | 4 - 0 | 253.82 | -1887.09 | 0.00000D+00 | 1.33491D-21 | 3.62111D-04 |
| Q( 7) | 4 - 1 | 731.39 | -1409.52 | 0.00000D+00 | 2.75245D-18 | -1.95981D-03 |
| Q( 7) | 4 - 2 | 1205.22 | -935.69 | 0.00000D+00 | 4.13647D-21 | 3.85724D-02 |
| Q( 7) | 4 - 3 | 1675.02 | -465.89 | 0.00000D+00 | 1.32548D-20 | -6.49804D-01 |
| Q( 7) | 4 - 4 | 2140.91 | 0.00 | 0.00000D+00 | 1.00000D+00 | -1.94955D+00 |
| Q( 8) | 4 - 0 | 257.66 | -1886.98 | 0.00000D+00 | 1.32374D-21 | 3.61784D-04 |
| Q( 8) | 4 - 1 | 735.21 | -1409.43 | 0.00000D+00 | 2.76078D-18 | -1.95877D-03 |
| Q( 8) | 4 - 2 | 1209.02 | -935.62 | 0.00000D+00 | 4.11287D-21 | 3.85742D-02 |
| Q( 8) | 4 - 3 | 1678.78 | -465.86 | 0.00000D+00 | 1.32222D-20 | -6.49830D-01 |
| Q( 8) | 4 - 4 | 2144.64 | 0.00 | 0.00000D+00 | 1.00000D+00 | -1.94979D+00 |
| Q( 9) | 4 - 0 | 261.99 | -1886.85 | 0.00000D+00 | 1.55441D-21 | 3.61417D-04 |
| Q( 9) | 4 - 1 | 739.51 | -1409.32 | 0.00000D+00 | 2.77016D-18 | -1.95761D-03 |
| Q( 9) | 4 - 2 | 1213.28 | -935.55 | 0.00000D+00 | 4.08671D-21 | 3.85762D-02 |
| Q( 9) | 4 - 3 | 1683.01 | -465.83 | 0.00000D+00 | 1.31852D-20 | -6.49860D-01 |
| Q( 9) | 4 - 4 | 2148.84 | 0.00 | 0.00000D+00 | 1.00000D+00 | -1.95006D+00 |
| Q( 10) | 4 - 0 | 266.80 | -1886.70 | 0.00000D+00 | 1.53972D-21 | 3.61008D-04 |
| Q( 10) | 4 - 1 | 744.29 | -1409.21 | 0.00000D+00 | 2.78053D-18 | -1.95631D-03 |
| Q( 10) | 4 - 2 | 1218.02 | -935.48 | 0.00000D+00 | 4.05678D-21 | 3.85784D-02 |
| Q( 10) | 4 - 3 | 1687.71 | -465.79 | 0.00000D+00 | 1.31434D-20 | -6.49893D-01 |
| Q( 10) | 4 - 4 | 2153.50 | 0.00 | 0.00000D+00 | 1.00000D+00 | -1.95035D+00 |
| Q( 11) | 4 - 0 | 272.08 | -1886.54 | 0.00000D+00 | 1.52328D-21 | 3.60558D-04 |
| Q( 11) | 4 - 1 | 749.54 | -1409.08 | 0.00000D+00 | 2.79194D-18 | -1.95488D-03 |
| Q( 11) | 4 - 2 | 1223.23 | -935.39 | 0.00000D+00 | 4.34370D-21 | 3.85809D-02 |
| Q( 11) | 4 - 3 | 1692.87 | -465.75 | 0.00000D+00 | 1.30981D-20 | -6.49929D-01 |
| Q( 11) | 4 - 4 | 2158.63 | 0.00 | 0.00000D+00 | 1.00000D+00 | -1.95067D+00 |

| | | | | | | | |
|---|---|---|---|---|---|---|---|
| Q( 12) | 4 - 0 | 277.85 | -1886.37 | 0.00000D+00 | 1.50537D-21 | 3.60066D-04 |
| Q( 12) | 4 - 1 | 755.28 | -1408.94 | 0.00000D+00 | 2.80438D-18 | -1.95332D-03 |
| Q( 12) | 4 - 2 | 1228.92 | -935.30 | 0.00000D+00 | 4.30870D-21 | 3.85835D-02 |
| Q( 12) | 4 - 3 | 1698.51 | -465.71 | 0.00000D+00 | 1.30528D-20 | -6.49968D-01 |
| Q( 12) | 4 - 4 | 2164.22 | 0.00 | 0.00000D+00 | 1.00000D+00 | -1.95103D+00 |
| Q( 13) | 4 - 0 | 284.10 | -1886.18 | 0.00000D+00 | 1.48689D-21 | 3.59534D-04 |
| Q( 13) | 4 - 1 | 761.49 | -1408.79 | 0.00000D+00 | 2.81780D-18 | -1.95164D-03 |
| Q( 13) | 4 - 2 | 1235.08 | -935.20 | 0.00000D+00 | 4.26702D-21 | 3.85864D-02 |
| Q( 13) | 4 - 3 | 1704.62 | -465.66 | 0.00000D+00 | 1.33121D-20 | -6.50011D-01 |
| Q( 13) | 4 - 4 | 2170.28 | 0.00 | 0.00000D+00 | 1.00000D+00 | -1.95141D+00 |
| Q( 14) | 4 - 0 | 290.83 | -1885.98 | 0.00000D+00 | 1.46629D-21 | 3.58960D-04 |
| Q( 14) | 4 - 1 | 768.17 | -1408.63 | 0.00000D+00 | 2.83222D-18 | -1.94982D-03 |
| Q( 14) | 4 - 2 | 1241.72 | -935.09 | 0.00000D+00 | 4.22645D-21 | 3.85895D-02 |
| Q( 14) | 4 - 3 | 1711.20 | -465.61 | 0.00000D+00 | 1.32625D-20 | -6.50057D-01 |
| Q( 14) | 4 - 4 | 2176.80 | 0.00 | 0.00000D+00 | 1.00000D+00 | -1.95182D+00 |
| Q( 15) | 4 - 0 | 298.04 | -1885.76 | 0.00000D+00 | 1.44517D-21 | 3.58344D-04 |
| Q( 15) | 4 - 1 | 775.34 | -1408.46 | 0.00000D+00 | 2.84767D-18 | -1.94788D-03 |
| Q( 15) | 4 - 2 | 1248.82 | -934.97 | 0.00000D+00 | 4.18030D-21 | 3.85928D-02 |
| Q( 15) | 4 - 3 | 1718.24 | -465.55 | 0.00000D+00 | 1.32141D-20 | -6.50106D-01 |
| Q( 15) | 4 - 4 | 2183.80 | 0.00 | 0.00000D+00 | 1.00000D+00 | -1.95226D+00 |
| Q( 16) | 4 - 0 | 305.73 | -1885.53 | 0.00000D+00 | 1.42240D-21 | 3.57687D-04 |
| Q( 16) | 4 - 1 | 782.98 | -1408.27 | 0.00000D+00 | 2.86408D-18 | -1.94581D-03 |
| Q( 16) | 4 - 2 | 1256.41 | -934.85 | 0.00000D+00 | 4.13054D-21 | 3.85962D-02 |
| Q( 16) | 4 - 3 | 1725.76 | -465.50 | 0.00000D+00 | 1.31691D-20 | -6.50159D-01 |
| Q( 16) | 4 - 4 | 2191.25 | 0.00 | 0.00000D+00 | 1.00000D+00 | -1.95273D+00 |
| Q( 17) | 4 - 0 | 313.89 | -1885.28 | 0.00000D+00 | 1.39903D-21 | 3.56989D-04 |
| Q( 17) | 4 - 1 | 791.10 | -1408.08 | 0.00000D+00 | 2.88149D-18 | -1.94361D-03 |
| Q( 17) | 4 - 2 | 1264.46 | -934.72 | 0.00000D+00 | 4.07958D-21 | 3.85999D-02 |
| Q( 17) | 4 - 3 | 1733.74 | -465.43 | 0.00000D+00 | 1.31278D-20 | -6.50215D-01 |

| | | | | | | |
|---|---|---|---|---|---|---|
| Q( 17) | 4 - 4 | 2199.18 | 0.00 | 0.00000D+00 | 1.00000D+00 | -1.95323D+00 |
| Q( 18) | 4 - 0 | 322.54 | -1885.02 | 0.00000D+00 | 1.37605D-21 | 3.56248D-04 |
| Q( 18) | 4 - 1 | 799.69 | -1407.87 | 0.00000D+00 | 2.53731D-18 | -1.94128D-03 |
| Q( 18) | 4 - 2 | 1272.99 | -934.58 | 0.00000D+00 | 3.99443D-21 | 3.86038D-02 |
| Q( 18) | 4 - 3 | 1742.20 | -465.37 | 0.00000D+00 | 1.32882D-20 | -6.50274D-01 |
| Q( 18) | 4 - 4 | 2207.56 | -0.00 | 0.00000D+00 | 1.00000D+00 | -1.95376D+00 |
| Q( 19) | 4 - 0 | 331.67 | -1884.75 | 0.00000D+00 | 1.35074D-21 | 3.55466D-04 |
| Q( 19) | 4 - 1 | 808.76 | -1407.65 | 0.00000D+00 | 2.55785D-18 | -1.93882D-03 |
| Q( 19) | 4 - 2 | 1281.99 | -934.43 | 0.00000D+00 | 3.93120D-21 | 3.86079D-02 |
| Q( 19) | 4 - 3 | 1751.12 | -465.30 | 0.00000D+00 | 1.32661D-20 | -6.50337D-01 |
| Q( 19) | 4 - 4 | 2216.42 | -0.00 | 0.00000D+00 | 1.00000D+00 | -1.95432D+00 |
| Q( 20) | 4 - 0 | 341.28 | -1884.46 | 0.00000D+00 | 1.32469D-21 | 3.54641D-04 |
| Q( 20) | 4 - 1 | 818.31 | -1407.42 | 0.00000D+00 | 2.57943D-18 | -1.93624D-03 |
| Q( 20) | 4 - 2 | 1291.46 | -934.27 | 0.00000D+00 | 3.86928D-21 | 3.86122D-02 |
| Q( 20) | 4 - 3 | 1760.51 | -465.23 | 0.00000D+00 | 1.32553D-20 | -6.50402D-01 |
| Q( 20) | 4 - 4 | 2225.74 | -0.00 | 0.00000D+00 | 1.00000D+00 | -1.95491D+00 |
| Q( 0) | 5 - 0 | 240.35 | -2350.43 | 0.00000D+00 | 2.45411D-21 | 1.83913D-04 |
| Q( 0) | 5 - 1 | 718.01 | -1872.77 | 0.00000D+00 | 8.90564D-18 | -7.03593D-04 |
| Q( 0) | 5 - 2 | 1191.95 | -1398.84 | 0.00000D+00 | 1.24016D-23 | 3.70439D-03 |
| Q( 0) | 5 - 3 | 1661.86 | -928.93 | 0.00000D+00 | 2.53274D-21 | -4.95846D-02 |
| Q( 0) | 5 - 4 | 2127.85 | -462.93 | 0.00000D+00 | 2.26086D-23 | 7.27522D-01 |
| Q( 0) | 5 - 5 | 2590.79 | 0.00 | 0.00000D+00 | 1.00000D+00 | 2.02501D+00 |
| Q( 1) | 5 - 0 | 240.84 | -2350.41 | 0.00000D+00 | 3.57339D-21 | 1.83910D-04 |
| Q( 1) | 5 - 1 | 718.49 | -1872.76 | 0.00000D+00 | 9.16943D-18 | -7.03536D-04 |
| Q( 1) | 5 - 2 | 1192.42 | -1398.82 | 0.00000D+00 | 1.92389D-20 | 3.70441D-03 |
| Q( 1) | 5 - 3 | 1662.33 | -928.92 | 0.00000D+00 | 1.28157D-19 | -4.95847D-02 |
| Q( 1) | 5 - 4 | 2128.32 | -462.93 | 0.00000D+00 | 1.80159D-18 | 7.27525D-01 |
| Q( 1) | 5 - 5 | 2591.25 | -0.00 | 0.00000D+00 | 1.00000D+00 | 2.02504D+00 |
| Q( 2) | 5 - 0 | 241.80 | -2350.38 | 0.00000D+00 | 1.01417D-20 | 1.83906D-04 |

| | | | | | | | |
|---|---|---|---|---|---|---|---|
| Q( 2) | 5 - 1 | 719.45 | -1872.73 | 0.00000D+00 | 1.02723D-17 | -7.03422D-04 |
| Q( 2) | 5 - 2 | 1193.37 | -1398.80 | 0.00000D+00 | 5.00556D-19 | 3.70446D-03 |
| Q( 2) | 5 - 3 | 1663.27 | -928.90 | 0.00000D+00 | 3.96350D-18 | -4.95851D-02 |
| Q( 2) | 5 - 4 | 2129.25 | -462.92 | 0.00000D+00 | 4.47766D-17 | 7.27532D-01 |
| Q( 2) | 5 - 5 | 2592.18 | -0.00 | 0.00000D+00 | 1.00000D+00 | 2.02510D+00 |
| Q( 3) | 5 - 0 | 243.24 | -2350.32 | 0.00000D+00 | 2.45190D-21 | 1.83899D-04 |
| Q( 3) | 5 - 1 | 720.88 | -1872.69 | 0.00000D+00 | 8.87960D-18 | -7.03251D-04 |
| Q( 3) | 5 - 2 | 1194.79 | -1398.77 | 0.00000D+00 | 1.27480D-23 | 3.70452D-03 |
| Q( 3) | 5 - 3 | 1664.68 | -928.88 | 0.00000D+00 | 2.52457D-21 | -4.95856D-02 |
| Q( 3) | 5 - 4 | 2130.65 | -462.91 | 0.00000D+00 | 2.20749D-23 | 7.27542D-01 |
| Q( 3) | 5 - 5 | 2593.56 | 0.00 | 0.00000D+00 | 1.00000D+00 | 2.02519D+00 |
| Q( 4) | 5 - 0 | 245.16 | -2350.25 | 0.00000D+00 | 2.45061D-21 | 1.83889D-04 |
| Q( 4) | 5 - 1 | 722.79 | -1872.63 | 0.00000D+00 | 8.86230D-18 | -7.03023D-04 |
| Q( 4) | 5 - 2 | 1196.69 | -1398.73 | 0.00000D+00 | 1.29493D-23 | 3.70462D-03 |
| Q( 4) | 5 - 3 | 1666.56 | -928.86 | 0.00000D+00 | 2.51763D-21 | -4.95864D-02 |
| Q( 4) | 5 - 4 | 2132.52 | -462.90 | 0.00000D+00 | 2.23463D-23 | 7.27555D-01 |
| Q( 4) | 5 - 5 | 2595.42 | 0.00 | 0.00000D+00 | 1.00000D+00 | 2.02530D+00 |
| Q( 5) | 5 - 0 | 247.57 | -2350.17 | 0.00000D+00 | 2.44855D-21 | 1.83877D-04 |
| Q( 5) | 5 - 1 | 725.18 | -1872.55 | 0.00000D+00 | 8.84076D-18 | -7.02738D-04 |
| Q( 5) | 5 - 2 | 1199.06 | -1398.67 | 0.00000D+00 | 1.32278D-23 | 3.70473D-03 |
| Q( 5) | 5 - 3 | 1668.91 | -928.82 | 0.00000D+00 | 2.50886D-21 | -4.95873D-02 |
| Q( 5) | 5 - 4 | 2134.85 | -462.88 | 0.00000D+00 | 2.24595D-23 | 7.27572D-01 |
| Q( 5) | 5 - 5 | 2597.73 | 0.00 | 0.00000D+00 | 1.00000D+00 | 2.02545D+00 |
| Q( 6) | 5 - 0 | 250.45 | -2350.06 | 0.00000D+00 | 2.44645D-21 | 1.83863D-04 |
| Q( 6) | 5 - 1 | 728.05 | -1872.46 | 0.00000D+00 | 8.81501D-18 | -7.02395D-04 |
| Q( 6) | 5 - 2 | 1201.91 | -1398.61 | 0.00000D+00 | 1.35101D-23 | 3.70487D-03 |
| Q( 6) | 5 - 3 | 1671.73 | -928.78 | 0.00000D+00 | 2.49945D-21 | -4.95884D-02 |
| Q( 6) | 5 - 4 | 2137.65 | -462.86 | 0.00000D+00 | 2.23916D-23 | 7.27592D-01 |
| Q( 6) | 5 - 5 | 2600.51 | -0.00 | 0.00000D+00 | 1.00000D+00 | 2.02562D+00 |

| | | | | | | | |
|---|---|---|---|---|---|---|---|
| Q( 7) | 5 - 0 | 253.82 | -2349.94 | 0.00000D+00 | 2.44404D-21 | 1.83846D-04 |
| Q( 7) | 5 - 1 | 731.39 | -1872.36 | 0.00000D+00 | 8.78510D-18 | -7.01994D-04 |
| Q( 7) | 5 - 2 | 1205.22 | -1398.53 | 0.00000D+00 | 1.39010D-23 | 3.70503D-03 |
| Q( 7) | 5 - 3 | 1675.02 | -928.73 | 0.00000D+00 | 2.48654D-21 | -4.95896D-02 |
| Q( 7) | 5 - 4 | 2140.91 | -462.84 | 0.00000D+00 | 2.25738D-23 | 7.27615D-01 |
| Q( 7) | 5 - 5 | 2603.75 | -0.00 | 0.00000D+00 | 1.00000D+00 | 2.02582D+00 |
| Q( 8) | 5 - 0 | 257.66 | -2349.79 | 0.00000D+00 | 2.44125D-21 | 1.83827D-04 |
| Q( 8) | 5 - 1 | 735.21 | -1872.24 | 0.00000D+00 | 8.75112D-18 | -7.01535D-04 |
| Q( 8) | 5 - 2 | 1209.02 | -1398.44 | 0.00000D+00 | 1.42941D-23 | 3.70521D-03 |
| Q( 8) | 5 - 3 | 1678.78 | -928.68 | 0.00000D+00 | 2.47325D-21 | -4.95910D-02 |
| Q( 8) | 5 - 4 | 2144.64 | -462.82 | 0.00000D+00 | 2.29613D-23 | 7.27642D-01 |
| Q( 8) | 5 - 5 | 2607.46 | -0.00 | 0.00000D+00 | 1.00000D+00 | 2.02605D+00 |
| Q( 9) | 5 - 0 | 261.99 | -2349.63 | 0.00000D+00 | 2.38279D-21 | 1.83805D-04 |
| Q( 9) | 5 - 1 | 739.51 | -1872.11 | 0.00000D+00 | 8.71306D-18 | -7.01018D-04 |
| Q( 9) | 5 - 2 | 1213.28 | -1398.34 | 0.00000D+00 | 1.47747D-23 | 3.70542D-03 |
| Q( 9) | 5 - 3 | 1683.01 | -928.62 | 0.00000D+00 | 2.45931D-21 | -4.95926D-02 |
| Q( 9) | 5 - 4 | 2148.84 | -462.79 | 0.00000D+00 | 2.26655D-23 | 7.27672D-01 |
| Q( 9) | 5 - 5 | 2611.62 | -0.00 | 0.00000D+00 | 1.00000D+00 | 2.02632D+00 |
| Q( 10) | 5 - 0 | 266.80 | -2349.46 | 0.00000D+00 | 2.38036D-21 | 1.83780D-04 |
| Q( 10) | 5 - 1 | 744.29 | -1871.96 | 0.00000D+00 | 8.67104D-18 | -7.00441D-04 |
| Q( 10) | 5 - 2 | 1218.02 | -1398.23 | 0.00000D+00 | 1.52865D-23 | 3.70564D-03 |
| Q( 10) | 5 - 3 | 1687.71 | -928.55 | 0.00000D+00 | 2.44247D-21 | -4.95944D-02 |
| Q( 10) | 5 - 4 | 2153.50 | -462.76 | 0.00000D+00 | 2.34741D-23 | 7.27705D-01 |
| Q( 10) | 5 - 5 | 2616.25 | -0.00 | 0.00000D+00 | 1.00000D+00 | 2.02660D+00 |
| Q( 11) | 5 - 0 | 272.08 | -2349.26 | 0.00000D+00 | 2.37717D-21 | 1.83753D-04 |
| Q( 11) | 5 - 1 | 749.54 | -1871.80 | 0.00000D+00 | 8.62515D-18 | -6.99806D-04 |
| Q( 11) | 5 - 2 | 1223.23 | -1398.11 | 0.00000D+00 | 5.59686D-24 | 3.70589D-03 |
| Q( 11) | 5 - 3 | 1692.87 | -928.47 | 0.00000D+00 | 2.42264D-21 | -4.95964D-02 |
| Q( 11) | 5 - 4 | 2158.63 | -462.72 | 0.00000D+00 | 2.37001D-23 | 7.27742D-01 |

| | | | | | | |
|---|---|---|---|---|---|---|
| Q( 11) | 5 - 5 | 2621.35 | -0.00 | 0.00000D+00 | 1.00000D+00 | 2.02692D+00 |
| Q( 12) | 5 - 0 | 277.85 | -2349.05 | 0.00000D+00 | 2.37339D-21 | 1.83723D-04 |
| Q( 12) | 5 - 1 | 755.28 | -1871.63 | 0.00000D+00 | 8.57549D-18 | -6.99111D-04 |
| Q( 12) | 5 - 2 | 1228.92 | -1397.98 | 0.00000D+00 | 6.01227D-24 | 3.70616D-03 |
| Q( 12) | 5 - 3 | 1698.51 | -928.39 | 0.00000D+00 | 2.40312D-21 | -4.95985D-02 |
| Q( 12) | 5 - 4 | 2164.22 | -462.68 | 0.00000D+00 | 2.41319D-23 | 7.27782D-01 |
| Q( 12) | 5 - 5 | 2626.90 | -0.00 | 0.00000D+00 | 1.00000D+00 | 2.02727D+00 |
| Q( 13) | 5 - 0 | 284.10 | -2348.82 | 0.00000D+00 | 2.36994D-21 | 1.83690D-04 |
| Q( 13) | 5 - 1 | 761.49 | -1871.43 | 0.00000D+00 | 8.52211D-18 | -6.98355D-04 |
| Q( 13) | 5 - 2 | 1235.08 | -1397.84 | 0.00000D+00 | 6.44565D-24 | 3.70645D-03 |
| Q( 13) | 5 - 3 | 1704.62 | -928.30 | 0.00000D+00 | 2.54640D-21 | -4.96007D-02 |
| Q( 13) | 5 - 4 | 2170.28 | -462.64 | 0.00000D+00 | 2.51271D-23 | 7.27825D-01 |
| Q( 13) | 5 - 5 | 2632.92 | -0.00 | 0.00000D+00 | 1.00000D+00 | 2.02765D+00 |
| Q( 14) | 5 - 0 | 290.83 | -2348.57 | 0.00000D+00 | 2.36624D-21 | 1.83654D-04 |
| Q( 14) | 5 - 1 | 768.17 | -1871.23 | 0.00000D+00 | 8.46532D-18 | -6.97538D-04 |
| Q( 14) | 5 - 2 | 1241.72 | -1397.69 | 0.00000D+00 | 6.61667D-24 | 3.70677D-03 |
| Q( 14) | 5 - 3 | 1711.20 | -928.21 | 0.00000D+00 | 2.50171D-21 | -4.96032D-02 |
| Q( 14) | 5 - 4 | 2176.80 | -462.60 | 0.00000D+00 | 3.32097D-23 | 7.27872D-01 |
| Q( 14) | 5 - 5 | 2639.40 | -0.00 | 0.00000D+00 | 1.00000D+00 | 2.02805D+00 |
| Q( 15) | 5 - 0 | 298.04 | -2348.31 | 0.00000D+00 | 2.36219D-21 | 1.83615D-04 |
| Q( 15) | 5 - 1 | 775.34 | -1871.01 | 0.00000D+00 | 8.40492D-18 | -6.96660D-04 |
| Q( 15) | 5 - 2 | 1248.82 | -1397.52 | 0.00000D+00 | 7.10847D-24 | 3.70710D-03 |
| Q( 15) | 5 - 3 | 1718.24 | -928.10 | 0.00000D+00 | 2.47349D-21 | -4.96058D-02 |
| Q( 15) | 5 - 4 | 2183.80 | -462.55 | 0.00000D+00 | 3.52703D-23 | 7.27922D-01 |
| Q( 15) | 5 - 5 | 2646.35 | -0.00 | 0.00000D+00 | 1.00000D+00 | 2.02849D+00 |
| Q( 16) | 5 - 0 | 305.73 | -2348.03 | 0.00000D+00 | 2.35753D-21 | 1.83573D-04 |
| Q( 16) | 5 - 1 | 782.98 | -1870.77 | 0.00000D+00 | 8.34117D-18 | -6.95720D-04 |
| Q( 16) | 5 - 2 | 1256.41 | -1397.35 | 0.00000D+00 | 7.60067D-24 | 3.70745D-03 |
| Q( 16) | 5 - 3 | 1725.76 | -927.99 | 0.00000D+00 | 2.44188D-21 | -4.96085D-02 |

| | | | | | | |
|---|---|---|---|---|---|---|
| Q( 16) | 5 - 4 | 2191.25 | -462.50 | 0.00000D+00 | 3.80228D-23 | 7.27976D-01 |
| Q( 16) | 5 - 5 | 2653.75 | -0.00 | 0.00000D+00 | 1.00000D+00 | 2.02895D+00 |
| Q( 17) | 5 - 0 | 313.89 | -2347.73 | 0.00000D+00 | 2.35275D-21 | 1.83528D-04 |
| Q( 17) | 5 - 1 | 791.10 | -1870.52 | 0.00000D+00 | 8.27422D-18 | -6.94717D-04 |
| Q( 17) | 5 - 2 | 1264.46 | -1397.16 | 0.00000D+00 | 8.17596D-24 | 3.70782D-03 |
| Q( 17) | 5 - 3 | 1733.74 | -927.88 | 0.00000D+00 | 2.40877D-21 | -4.96114D-02 |
| Q( 17) | 5 - 4 | 2199.18 | -462.44 | 0.00000D+00 | 4.09648D-23 | 7.28032D-01 |
| Q( 17) | 5 - 5 | 2661.62 | -0.00 | 0.00000D+00 | 1.00000D+00 | 2.02944D+00 |
| Q( 18) | 5 - 0 | 322.54 | -2347.41 | 0.00000D+00 | 2.34854D-21 | 1.83480D-04 |
| Q( 18) | 5 - 1 | 799.69 | -1870.26 | 0.00000D+00 | 8.58994D-18 | -6.93650D-04 |
| Q( 18) | 5 - 2 | 1272.99 | -1396.96 | 0.00000D+00 | 8.77222D-24 | 3.70822D-03 |
| Q( 18) | 5 - 3 | 1742.20 | -927.75 | 0.00000D+00 | 2.37238D-21 | -4.96144D-02 |
| Q( 18) | 5 - 4 | 2207.56 | -462.39 | 0.00000D+00 | 4.45649D-23 | 7.28092D-01 |
| Q( 18) | 5 - 5 | 2669.95 | -0.00 | 0.00000D+00 | 1.00000D+00 | 2.02996D+00 |
| Q( 19) | 5 - 0 | 331.67 | -2347.07 | 0.00000D+00 | 2.34311D-21 | 1.83428D-04 |
| Q( 19) | 5 - 1 | 808.76 | -1869.98 | 0.00000D+00 | 8.51572D-18 | -6.92519D-04 |
| Q( 19) | 5 - 2 | 1281.99 | -1396.76 | 0.00000D+00 | 9.40226D-24 | 3.70863D-03 |
| Q( 19) | 5 - 3 | 1751.12 | -927.62 | 0.00000D+00 | 2.33683D-21 | -4.96176D-02 |
| Q( 19) | 5 - 4 | 2216.42 | -462.33 | 0.00000D+00 | 4.85793D-23 | 7.28156D-01 |
| Q( 19) | 5 - 5 | 2678.74 | -0.00 | 0.00000D+00 | 1.00000D+00 | 2.03051D+00 |
| Q( 20) | 5 - 0 | 341.28 | -2346.72 | 0.00000D+00 | 2.33749D-21 | 1.83373D-04 |
| Q( 20) | 5 - 1 | 818.31 | -1869.69 | 0.00000D+00 | 8.43862D-18 | -6.91323D-04 |
| Q( 20) | 5 - 2 | 1291.46 | -1396.54 | 0.00000D+00 | 1.01057D-23 | 3.70906D-03 |
| Q( 20) | 5 - 3 | 1760.51 | -927.49 | 0.00000D+00 | 2.29778D-21 | -4.96209D-02 |
| Q( 20) | 5 - 4 | 2225.74 | -462.26 | 0.00000D+00 | 5.32504D-23 | 7.28222D-01 |
| Q( 20) | 5 - 5 | 2688.00 | -0.00 | 0.00000D+00 | 1.00000D+00 | 2.03109D+00 |
