# Supplementary material for: Ab initio spectroscopic studies of AlF and AlCl molecules
Source: arXiv:2303.08681 source file (2023-03-15)
Supplement: Supplementary file 4 [file AlCl_triplet_pi_-_S17.pdf]

# AlCl $a^3\Pi$: Rotational parameters

Note that (v',J') & (v",J") strictly label the upper and lower levels, resp., and E(lower)=E"

but E(2)-E(1) is: (energy of State-2 level) - (energy of State-1 level)

In the following table, E is expressed in $cm^{-1}$, A in $s^{-1}$ and transition dipole moment in debye.

| dJ(J") | Band v' v" | E(lower) | E(2)-E(1) | A(Einstein) | F-C Factor | <v'j'\|M\|v"j"> |
|---|---|---|---|---|---|---|
| ------ | ------- | -------- | -------- | ----------- | ----------- | ----------- |
| R( 0) | 0 - 0 | 260.52 | -0.49 | 3.61841D-08 | 1.00000D+00 | -1.69084D+00 |
| R( 1) | 0 - 0 | 261.02 | -0.99 | 3.47376D-07 | 1.00000D+00 | -1.69087D+00 |
| R( 2) | 0 - 0 | 262.01 | -1.48 | 1.25615D-06 | 1.00000D+00 | -1.69091D+00 |
| R( 3) | 0 - 0 | 263.49 | -1.98 | 3.08794D-06 | 1.00000D+00 | -1.69098D+00 |
| R( 4) | 0 - 0 | 265.47 | -2.47 | 6.16850D-06 | 1.00000D+00 | -1.69106D+00 |
| R( 5) | 0 - 0 | 267.94 | -2.97 | 1.08238D-05 | 1.00000D+00 | -1.69116D+00 |
| R( 6) | 0 - 0 | 270.91 | -3.46 | 1.73800D-05 | 1.00000D+00 | -1.69128D+00 |
| R( 7) | 0 - 0 | 274.37 | -3.96 | 2.61634D-05 | 1.00000D+00 | -1.69142D+00 |
| R( 8) | 0 - 0 | 278.33 | -4.45 | 3.75007D-05 | 1.00000D+00 | -1.69157D+00 |
| R( 9) | 0 - 0 | 282.78 | -4.95 | 5.17187D-05 | 1.00000D+00 | -1.69174D+00 |
| R( 10) | 0 - 0 | 287.73 | -5.44 | 6.91447D-05 | 1.00000D+00 | -1.69194D+00 |
| R( 11) | 0 - 0 | 293.17 | -5.93 | 9.01061D-05 | 1.00000D+00 | -1.69215D+00 |
| R( 12) | 0 - 0 | 299.10 | -6.43 | 1.14931D-04 | 1.00000D+00 | -1.69238D+00 |
| R( 13) | 0 - 0 | 305.53 | -6.92 | 1.43948D-04 | 1.00000D+00 | -1.69262D+00 |
| R( 14) | 0 - 0 | 312.46 | -7.42 | 1.77485D-04 | 1.00000D+00 | -1.69289D+00 |
| R( 15) | 0 - 0 | 319.87 | -7.91 | 2.15872D-04 | 1.00000D+00 | -1.69317D+00 |
| R( 16) | 0 - 0 | 327.79 | -8.41 | 2.59438D-04 | 1.00000D+00 | -1.69347D+00 |
| R( 17) | 0 - 0 | 336.19 | -8.90 | 3.08515D-04 | 9.99999D-01 | -1.69379D+00 |
| R( 18) | 0 - 0 | 345.09 | -9.39 | 3.63432D-04 | 9.99999D-01 | -1.69413D+00 |

| | | | | | | | |
|---|---|---|---|---|---|---|---|
| R( 19) | 0 - 0 | 354.48 | -9.89 | 4.24522D-04 | 9.99999D-01 | -1.69449D+00 |
| P( 1) | 1 - 0 | 261.02 | -517.13 | 2.08640D+00 | 1.72385D-09 | 2.19327D-01 |
| R( 0) | 1 - 0 | 260.52 | -518.12 | 6.98546D-01 | 1.72438D-09 | 2.19185D-01 |
| P( 2) | 1 - 0 | 262.01 | -516.64 | 1.38783D+00 | 6.89583D-09 | 2.19399D-01 |
| R( 0) | 1 - 1 | 778.15 | -0.49 | 3.73057D-08 | 1.00000D+00 | 1.73306D+00 |
| R( 1) | 1 - 0 | 261.02 | -518.61 | 8.40086D-01 | 6.89749D-09 | 2.19114D-01 |
| P( 3) | 1 - 0 | 263.49 | -516.14 | 1.24623D+00 | 1.55156D-08 | 2.19471D-01 |
| R( 1) | 1 - 1 | 778.64 | -0.98 | 3.58143D-07 | 1.00000D+00 | 1.73309D+00 |
| R( 2) | 1 - 0 | 262.01 | -519.09 | 9.02043D-01 | 1.55170D-08 | 2.19044D-01 |
| P( 4) | 1 - 0 | 265.47 | -515.63 | 1.18420D+00 | 2.75870D-08 | 2.19543D-01 |
| R( 2) | 1 - 1 | 779.63 | -1.47 | 1.29508D-06 | 1.00000D+00 | 1.73314D+00 |
| R( 3) | 1 - 0 | 263.49 | -519.58 | 9.37463D-01 | 2.75864D-08 | 2.18974D-01 |
| P( 5) | 1 - 0 | 267.94 | -515.12 | 1.14867D+00 | 4.31062D-08 | 2.19616D-01 |
| R( 3) | 1 - 1 | 781.10 | -1.97 | 3.18363D-06 | 1.00000D+00 | 1.73320D+00 |
| R( 4) | 1 - 0 | 265.47 | -520.06 | 9.60812D-01 | 4.31050D-08 | 2.18904D-01 |
| P( 6) | 1 - 0 | 270.91 | -514.61 | 1.12519D+00 | 6.20755D-08 | 2.19689D-01 |
| R( 4) | 1 - 1 | 783.07 | -2.46 | 6.35965D-06 | 1.00000D+00 | 1.73328D+00 |
| R( 5) | 1 - 0 | 267.94 | -520.53 | 9.77656D-01 | 6.20734D-08 | 2.18835D-01 |
| P( 7) | 1 - 0 | 274.37 | -514.10 | 1.10818D+00 | 8.44958D-08 | 2.19763D-01 |
| R( 5) | 1 - 1 | 785.53 | -2.95 | 1.11592D-05 | 1.00000D+00 | 1.73338D+00 |
| R( 6) | 1 - 0 | 270.91 | -521.01 | 9.90591D-01 | 8.44925D-08 | 2.18766D-01 |
| P( 8) | 1 - 0 | 278.33 | -513.59 | 1.09506D+00 | 1.10368D-07 | 2.19837D-01 |
| R( 6) | 1 - 1 | 788.47 | -3.44 | 1.79184D-05 | 1.00000D+00 | 1.73350D+00 |
| R( 7) | 1 - 0 | 274.37 | -521.48 | 1.00099D+00 | 1.10363D-07 | 2.18697D-01 |
| P( 9) | 1 - 0 | 282.78 | -513.07 | 1.08445D+00 | 1.39693D-07 | 2.19911D-01 |
| R( 7) | 1 - 1 | 791.92 | -3.93 | 2.69739D-05 | 1.00000D+00 | 1.73364D+00 |
| R( 8) | 1 - 0 | 278.33 | -521.94 | 1.00965D+00 | 1.39686D-07 | 2.18629D-01 |
| P( 10) | 1 - 0 | 287.73 | -512.54 | 1.07555D+00 | 1.72473D-07 | 2.19985D-01 |
| R( 8) | 1 - 1 | 795.85 | -4.42 | 3.86622D-05 | 1.00000D+00 | 1.73379D+00 |

| | | | | | | | |
|---|---|---|---|---|---|---|---|
| R( 9) | 1 - 0 | 282.78 | -522.41 | 1.01707D+00 | 1.72463D-07 | 2.18561D-01 |
| P( 11) | 1 - 0 | 293.17 | -512.02 | 1.06787D+00 | 2.08708D-07 | 2.20060D-01 |
| R( 9) | 1 - 1 | 800.27 | -4.92 | 5.33203D-05 | 9.99999D-01 | 1.73397D+00 |
| R( 10) | 1 - 0 | 287.73 | -522.87 | 1.02356D+00 | 2.08695D-07 | 2.18493D-01 |
| P( 12) | 1 - 0 | 299.10 | -511.49 | 1.06108D+00 | 2.48400D-07 | 2.20136D-01 |
| R( 10) | 1 - 1 | 805.19 | -5.41 | 7.12856D-05 | 9.99999D-01 | 1.73416D+00 |
| R( 11) | 1 - 0 | 293.17 | -523.32 | 1.02934D+00 | 2.48383D-07 | 2.18426D-01 |
| P( 13) | 1 - 0 | 305.53 | -510.96 | 1.05498D+00 | 2.91552D-07 | 2.20211D-01 |
| R( 11) | 1 - 1 | 810.59 | -5.90 | 9.28954D-05 | 9.99999D-01 | 1.73437D+00 |
| R( 12) | 1 - 0 | 299.10 | -523.78 | 1.03458D+00 | 2.91530D-07 | 2.18359D-01 |
| P( 14) | 1 - 0 | 312.46 | -510.42 | 1.04940D+00 | 3.38164D-07 | 2.20288D-01 |
| R( 12) | 1 - 1 | 816.49 | -6.39 | 1.18488D-04 | 9.99999D-01 | 1.73460D+00 |
| R( 13) | 1 - 0 | 305.53 | -524.23 | 1.03937D+00 | 3.38137D-07 | 2.18292D-01 |
| P( 15) | 1 - 0 | 319.87 | -509.89 | 1.04424D+00 | 3.88239D-07 | 2.20364D-01 |
| R( 13) | 1 - 1 | 822.88 | -6.88 | 1.48402D-04 | 9.99999D-01 | 1.73485D+00 |
| R( 14) | 1 - 0 | 312.46 | -524.68 | 1.04380D+00 | 3.88206D-07 | 2.18226D-01 |
| P( 16) | 1 - 0 | 327.79 | -509.35 | 1.03941D+00 | 4.41779D-07 | 2.20441D-01 |
| R( 14) | 1 - 1 | 829.76 | -7.37 | 1.82975D-04 | 9.99999D-01 | 1.73511D+00 |
| R( 15) | 1 - 0 | 319.87 | -525.12 | 1.04793D+00 | 4.41739D-07 | 2.18159D-01 |
| P( 17) | 1 - 0 | 336.19 | -508.80 | 1.03485D+00 | 4.98786D-07 | 2.20518D-01 |
| R( 15) | 1 - 1 | 837.13 | -7.86 | 2.22547D-04 | 9.99999D-01 | 1.73539D+00 |
| R( 16) | 1 - 0 | 327.79 | -525.56 | 1.05182D+00 | 4.98738D-07 | 2.18093D-01 |
| P( 18) | 1 - 0 | 345.09 | -508.26 | 1.03051D+00 | 5.59263D-07 | 2.20596D-01 |
| R( 16) | 1 - 1 | 844.99 | -8.35 | 2.67459D-04 | 9.99998D-01 | 1.73570D+00 |
| R( 17) | 1 - 0 | 336.19 | -526.00 | 1.05549D+00 | 5.59206D-07 | 2.18028D-01 |
| P( 19) | 1 - 0 | 354.48 | -507.71 | 1.02635D+00 | 6.23212D-07 | 2.20674D-01 |
| R( 17) | 1 - 1 | 853.35 | -8.84 | 3.18050D-04 | 9.99998D-01 | 1.73602D+00 |
| R( 18) | 1 - 0 | 345.09 | -526.44 | 1.05899D+00 | 6.23145D-07 | 2.17963D-01 |
| P( 20) | 1 - 0 | 364.37 | -507.16 | 1.02235D+00 | 6.90635D-07 | 2.20753D-01 |

| | | | | | | | |
|---|---|---|---|---|---|---|---|
| R( 18) | 1 - 1 | 862.19 | -9.33 | 3.74660D-04 | 9.99998D-01 | 1.73636D+00 |
| R( 19) | 1 - 0 | 354.48 | -526.87 | 1.06232D+00 | 6.90558D-07 | 2.17898D-01 |
| P( 21) | 1 - 0 | 374.75 | -506.60 | 1.01848D+00 | 7.61537D-07 | 2.20831D-01 |
| R( 19) | 1 - 1 | 871.53 | -9.83 | 4.37633D-04 | 9.99998D-01 | 1.73671D+00 |
| P( 1) | 2 - 0 | 261.02 | -1030.44 | 6.14280D-02 | 3.91370D-12 | 1.33798D-02 |
| P( 1) | 2 - 1 | 778.64 | -512.81 | 4.03872D+00 | 3.45671D-09 | -3.09019D-01 |
| R( 0) | 2 - 0 | 260.52 | -1031.42 | 2.05926D-02 | 3.93309D-12 | 1.33987D-02 |
| P( 2) | 2 - 0 | 262.01 | -1029.94 | 4.08356D-02 | 1.56434D-11 | 1.33705D-02 |
| R( 0) | 2 - 1 | 778.15 | -513.79 | 1.35216D+00 | 3.46037D-09 | -3.08812D-01 |
| P( 2) | 2 - 1 | 779.63 | -512.32 | 2.68650D+00 | 1.38304D-08 | -3.09123D-01 |
| R( 0) | 2 - 2 | 1291.45 | -0.49 | 3.84102D-08 | 1.00000D+00 | -1.77546D+00 |
| R( 1) | 2 - 0 | 261.02 | -1031.90 | 2.47812D-02 | 1.57309D-11 | 1.34083D-02 |
| P( 3) | 2 - 0 | 263.49 | -1029.43 | 3.66475D-02 | 3.51788D-11 | 1.33614D-02 |
| R( 1) | 2 - 1 | 778.64 | -514.28 | 1.62611D+00 | 1.38361D-08 | -3.08709D-01 |
| P( 3) | 2 - 1 | 781.10 | -511.82 | 2.41244D+00 | 3.11245D-08 | -3.09228D-01 |
| R( 1) | 2 - 2 | 1291.94 | -0.98 | 3.68735D-07 | 1.00000D+00 | -1.77549D+00 |
| R( 2) | 2 - 0 | 262.01 | -1032.38 | 2.66265D-02 | 3.54583D-11 | 1.34180D-02 |
| P( 4) | 2 - 0 | 265.47 | -1028.92 | 3.48030D-02 | 6.24395D-11 | 1.33523D-02 |
| R( 2) | 2 - 1 | 779.63 | -514.76 | 1.74601D+00 | 3.11331D-08 | -3.08607D-01 |
| P( 4) | 2 - 1 | 783.07 | -511.32 | 2.29238D+00 | 5.53316D-08 | -3.09333D-01 |
| R( 2) | 2 - 2 | 1292.92 | -1.47 | 1.33343D-06 | 1.00000D+00 | -1.77553D+00 |
| R( 3) | 2 - 0 | 263.49 | -1032.85 | 2.76909D-02 | 6.30815D-11 | 1.34278D-02 |
| P( 5) | 2 - 0 | 267.94 | -1028.40 | 3.37398D-02 | 9.74866D-11 | 1.33434D-02 |
| R( 3) | 2 - 1 | 781.10 | -515.24 | 1.81454D+00 | 5.53418D-08 | -3.08505D-01 |
| P( 5) | 2 - 1 | 785.53 | -510.81 | 2.22364D+00 | 8.64667D-08 | -3.09438D-01 |
| R( 3) | 2 - 2 | 1294.38 | -1.95 | 3.27786D-06 | 1.00000D+00 | -1.77560D+00 |
| R( 4) | 2 - 0 | 265.47 | -1033.31 | 2.84002D-02 | 9.86898D-11 | 1.34377D-02 |
| P( 6) | 2 - 0 | 270.91 | -1027.87 | 3.30317D-02 | 1.40216D-10 | 1.33345D-02 |
| R( 4) | 2 - 1 | 783.07 | -515.71 | 1.85971D+00 | 8.64726D-08 | -3.08404D-01 |

| | | | | | | |
|---|---|---|---|---|---|---|
| P( 6) | 2 - 1 | 788.47 | -510.31 | 2.17820D+00 | 1.24519D-07 | -3.09544D-01 |
| R( 4) | 2 - 2 | 1296.34 | -2.44 | 6.54787D-06 | 1.00000D+00 | -1.77568D+00 |
| R( 5) | 2 - 0 | 267.94 | -1033.77 | 2.89185D-02 | 1.42295D-10 | 1.34477D-02 |
| P( 7) | 2 - 0 | 274.37 | -1027.34 | 3.25150D-02 | 1.90626D-10 | 1.33258D-02 |
| R( 5) | 2 - 1 | 785.53 | -516.19 | 1.89228D+00 | 1.24523D-07 | -3.08303D-01 |
| P( 7) | 2 - 1 | 791.92 | -509.80 | 2.14531D+00 | 1.69495D-07 | -3.09651D-01 |
| R( 5) | 2 - 2 | 1298.78 | -2.93 | 1.14894D-05 | 1.00000D+00 | -1.77578D+00 |
| R( 6) | 2 - 0 | 270.91 | -1034.22 | 2.93223D-02 | 1.93928D-10 | 1.34578D-02 |
| P( 8) | 2 - 0 | 278.33 | -1026.80 | 3.21132D-02 | 2.48693D-10 | 1.33172D-02 |
| R( 6) | 2 - 1 | 788.47 | -516.66 | 1.91728D+00 | 1.69496D-07 | -3.08203D-01 |
| P( 8) | 2 - 1 | 795.85 | -509.28 | 2.11993D+00 | 2.21395D-07 | -3.09758D-01 |
| R( 6) | 2 - 2 | 1301.71 | -3.42 | 1.84487D-05 | 1.00000D+00 | -1.77590D+00 |
| R( 7) | 2 - 0 | 274.37 | -1034.66 | 2.96519D-02 | 2.53622D-10 | 1.34681D-02 |
| P( 9) | 2 - 0 | 282.78 | -1026.26 | 3.17857D-02 | 3.14390D-10 | 1.33087D-02 |
| R( 7) | 2 - 1 | 791.92 | -517.12 | 1.93737D+00 | 2.21392D-07 | -3.08102D-01 |
| P( 9) | 2 - 1 | 800.27 | -508.77 | 2.09940D+00 | 2.80224D-07 | -3.09866D-01 |
| R( 7) | 2 - 2 | 1305.13 | -3.91 | 2.77720D-05 | 9.99999D-01 | -1.77604D+00 |
| R( 8) | 2 - 0 | 278.33 | -1035.10 | 2.99309D-02 | 3.21410D-10 | 1.34784D-02 |
| P( 10) | 2 - 0 | 287.73 | -1025.71 | 3.15091D-02 | 3.87693D-10 | 1.33002D-02 |
| R( 8) | 2 - 1 | 795.85 | -517.59 | 1.95410D+00 | 2.80214D-07 | -3.08003D-01 |
| P( 10) | 2 - 1 | 805.19 | -508.25 | 2.08219D+00 | 3.45982D-07 | -3.09974D-01 |
| R( 8) | 2 - 2 | 1309.04 | -4.40 | 3.98059D-05 | 9.99999D-01 | -1.77619D+00 |
| R( 9) | 2 - 0 | 282.78 | -1035.54 | 3.01737D-02 | 3.97324D-10 | 1.34889D-02 |
| P( 11) | 2 - 0 | 293.17 | -1025.15 | 3.12690D-02 | 4.68578D-10 | 1.32919D-02 |
| R( 9) | 2 - 1 | 800.27 | -518.05 | 1.96841D+00 | 3.45964D-07 | -3.07904D-01 |
| P( 11) | 2 - 1 | 810.59 | -507.72 | 2.06734D+00 | 4.18674D-07 | -3.10082D-01 |
| R( 9) | 2 - 2 | 1313.43 | -4.88 | 5.48974D-05 | 9.99999D-01 | -1.77637D+00 |
| R( 10) | 2 - 0 | 287.73 | -1035.96 | 3.03898D-02 | 4.81398D-10 | 1.34994D-02 |
| P( 12) | 2 - 0 | 299.10 | -1024.59 | 3.10558D-02 | 5.57021D-10 | 1.32837D-02 |

| | | | | | | |
|---|---|---|---|---|---|---|
| R( 10) | 2 - 1 | 805.19 | -518.50 | 1.98093D+00 | 4.18646D-07 | -3.07805D-01 |
| P( 12) | 2 - 1 | 816.49 | -507.20 | 2.05422D+00 | 4.98303D-07 | -3.10191D-01 |
| R( 10) | 2 - 2 | 1318.32 | -5.37 | 7.33936D-05 | 9.99999D-01 | -1.77656D+00 |
| R( 11) | 2 - 0 | 293.17 | -1036.38 | 3.05857D-02 | 5.73666D-10 | 1.35101D-02 |
| P( 13) | 2 - 0 | 305.53 | -1024.02 | 3.08631D-02 | 6.52998D-10 | 1.32757D-02 |
| R( 11) | 2 - 1 | 810.59 | -518.96 | 1.99209D+00 | 4.98261D-07 | -3.07706D-01 |
| P( 13) | 2 - 1 | 822.88 | -506.67 | 2.04242D+00 | 5.84872D-07 | -3.10301D-01 |
| R( 11) | 2 - 2 | 1323.69 | -5.86 | 9.56419D-05 | 9.99999D-01 | -1.77677D+00 |
| R( 12) | 2 - 0 | 299.10 | -1036.79 | 3.07659D-02 | 6.74165D-10 | 1.35209D-02 |
| P( 14) | 2 - 0 | 312.46 | -1023.44 | 3.06864D-02 | 7.56487D-10 | 1.32677D-02 |
| R( 12) | 2 - 1 | 816.49 | -519.41 | 2.00217D+00 | 5.84813D-07 | -3.07609D-01 |
| P( 14) | 2 - 1 | 829.76 | -506.14 | 2.03163D+00 | 6.78385D-07 | -3.10411D-01 |
| R( 12) | 2 - 2 | 1329.55 | -6.35 | 1.21990D-04 | 9.99999D-01 | -1.77700D+00 |
| R( 13) | 2 - 0 | 305.53 | -1037.20 | 3.09336D-02 | 7.82928D-10 | 1.35318D-02 |
| P( 15) | 2 - 0 | 319.87 | -1022.86 | 3.05224D-02 | 8.67465D-10 | 1.32598D-02 |
| R( 13) | 2 - 1 | 822.88 | -519.85 | 2.01139D+00 | 6.78307D-07 | -3.07511D-01 |
| P( 15) | 2 - 1 | 837.13 | -505.60 | 2.02165D+00 | 7.78846D-07 | -3.10522D-01 |
| R( 13) | 2 - 2 | 1335.90 | -6.84 | 1.52787D-04 | 9.99998D-01 | -1.77725D+00 |
| R( 14) | 2 - 0 | 312.46 | -1037.60 | 3.10913D-02 | 8.99992D-10 | 1.35427D-02 |
| P( 16) | 2 - 0 | 327.79 | -1022.27 | 3.03688D-02 | 9.85910D-10 | 1.32520D-02 |
| R( 14) | 2 - 1 | 829.76 | -520.30 | 2.01992D+00 | 7.78746D-07 | -3.07414D-01 |
| P( 16) | 2 - 1 | 844.99 | -505.06 | 2.01231D+00 | 8.86260D-07 | -3.10633D-01 |
| R( 14) | 2 - 2 | 1342.73 | -7.32 | 1.88381D-04 | 9.99998D-01 | -1.77751D+00 |
| R( 15) | 2 - 0 | 319.87 | -1038.00 | 3.12408D-02 | 1.02539D-09 | 1.35539D-02 |
| P( 17) | 2 - 0 | 336.19 | -1021.68 | 3.02235D-02 | 1.11180D-09 | 1.32444D-02 |
| R( 15) | 2 - 1 | 837.13 | -520.74 | 2.02788D+00 | 8.86134D-07 | -3.07317D-01 |
| P( 17) | 2 - 1 | 853.35 | -504.52 | 2.00349D+00 | 1.00063D-06 | -3.10744D-01 |
| R( 15) | 2 - 2 | 1350.06 | -7.81 | 2.29120D-04 | 9.99998D-01 | -1.77779D+00 |
| R( 16) | 2 - 0 | 327.79 | -1038.39 | 3.13836D-02 | 1.15917D-09 | 1.35651D-02 |

| | | | | | | | |
|---|---|---|---|---|---|---|---|
| P( 18) | 2 - 0 | 345.09 | -1021.08 | 3.00853D-02 | 1.24512D-09 | 1.32368D-02 |
| R( 16) | 2 - 1 | 844.99 | -521.18 | 2.03535D+00 | 1.00048D-06 | -3.07221D-01 |
| P( 18) | 2 - 1 | 862.19 | -503.98 | 1.99510D+00 | 1.12197D-06 | -3.10857D-01 |
| R( 16) | 2 - 2 | 1357.87 | -8.30 | 2.75356D-04 | 9.99997D-01 | -1.77810D+00 |
| R( 17) | 2 - 0 | 336.19 | -1038.77 | 3.15207D-02 | 1.30136D-09 | 1.35764D-02 |
| P( 19) | 2 - 0 | 354.48 | -1020.47 | 2.99530D-02 | 1.38584D-09 | 1.32294D-02 |
| R( 17) | 2 - 1 | 853.35 | -521.61 | 2.04241D+00 | 1.12178D-06 | -3.07125D-01 |
| P( 19) | 2 - 1 | 871.53 | -503.43 | 1.98707D+00 | 1.25027D-06 | -3.10969D-01 |
| R( 17) | 2 - 2 | 1366.17 | -8.79 | 3.27437D-04 | 9.99997D-01 | -1.77842D+00 |
| R( 18) | 2 - 0 | 345.09 | -1039.14 | 3.16531D-02 | 1.45199D-09 | 1.35878D-02 |
| P( 20) | 2 - 0 | 364.37 | -1019.86 | 2.98257D-02 | 1.53394D-09 | 1.32221D-02 |
| R( 18) | 2 - 1 | 862.19 | -522.04 | 2.04912D+00 | 1.25004D-06 | -3.07029D-01 |
| P( 20) | 2 - 1 | 881.35 | -502.88 | 1.97933D+00 | 1.38555D-06 | -3.11083D-01 |
| R( 18) | 2 - 2 | 1374.96 | -9.28 | 3.85715D-04 | 9.99997D-01 | -1.77876D+00 |
| R( 19) | 2 - 0 | 354.48 | -1039.51 | 3.17815D-02 | 1.61112D-09 | 1.35994D-02 |
| P( 21) | 2 - 0 | 374.75 | -1019.24 | 2.97027D-02 | 1.68941D-09 | 1.32148D-02 |
| R( 19) | 2 - 1 | 871.53 | -522.47 | 2.05552D+00 | 1.38528D-06 | -3.06934D-01 |
| P( 21) | 2 - 1 | 891.67 | -502.33 | 1.97185D+00 | 1.52781D-06 | -3.11197D-01 |
| R( 19) | 2 - 2 | 1384.23 | -9.76 | 4.50541D-04 | 9.99997D-01 | -1.77911D+00 |
| P( 1) | 3 - 0 | 261.02 | -1539.25 | 7.58787D-04 | 2.82261D-14 | 8.14510D-04 |
| P( 1) | 3 - 1 | 778.64 | -1021.62 | 1.84985D-01 | 1.18853D-11 | -2.35198D-02 |
| P( 1) | 3 - 2 | 1291.94 | -508.32 | 5.85328D+00 | 5.20442D-09 | 3.76957D-01 |
| R( 0) | 3 - 0 | 260.52 | -1540.23 | 2.55193D-04 | 2.83983D-14 | 8.17367D-04 |
| P( 2) | 3 - 0 | 262.01 | -1538.74 | 5.03597D-04 | 1.12733D-13 | 8.13088D-04 |
| R( 0) | 3 - 1 | 778.15 | -1022.60 | 6.20083D-02 | 1.18794D-11 | -2.35520D-02 |
| P( 2) | 3 - 1 | 779.63 | -1021.12 | 1.22978D-01 | 4.74436D-11 | -2.35040D-02 |
| R( 0) | 3 - 2 | 1291.45 | -509.29 | 1.95962D+00 | 5.20956D-09 | 3.76697D-01 |
| P( 2) | 3 - 2 | 1292.92 | -507.83 | 3.89358D+00 | 2.08229D-08 | 3.77088D-01 |
| R( 0) | 3 - 3 | 1800.26 | -0.49 | 3.94955D-08 | 1.00000D+00 | 1.81808D+00 |

| | | | | | | |
|---|---|---|---|---|---|---|
| R( 1) | 3 - 0 | 261.02 | -1540.70 | 3.07591D-04 | 1.13846D-13 | 8.18800D-04 |
| P( 3) | 3 - 0 | 263.49 | -1538.23 | 4.51204D-04 | 2.53067D-13 | 8.11668D-04 |
| R( 1) | 3 - 1 | 778.64 | -1023.08 | 7.46185D-02 | 4.76239D-11 | -2.35684D-02 |
| P( 3) | 3 - 1 | 781.10 | -1020.62 | 1.10369D-01 | 1.06574D-10 | -2.34883D-02 |
| R( 1) | 3 - 2 | 1291.94 | -509.78 | 2.35661D+00 | 2.08342D-08 | 3.76567D-01 |
| P( 3) | 3 - 2 | 1294.38 | -507.33 | 3.49643D+00 | 4.68549D-08 | 3.77219D-01 |
| R( 1) | 3 - 3 | 1800.75 | -0.97 | 3.79165D-07 | 1.00000D+00 | 1.81811D+00 |
| R( 2) | 3 - 0 | 262.01 | -1541.17 | 3.31020D-04 | 2.56025D-13 | 8.20237D-04 |
| P( 4) | 3 - 0 | 265.47 | -1537.71 | 4.27784D-04 | 4.49819D-13 | 8.10252D-04 |
| R( 2) | 3 - 1 | 779.63 | -1023.55 | 8.01721D-02 | 1.07266D-10 | -2.35850D-02 |
| P( 4) | 3 - 1 | 783.07 | -1020.11 | 1.04818D-01 | 1.89274D-10 | -2.34729D-02 |
| R( 2) | 3 - 2 | 1292.92 | -510.26 | 2.53033D+00 | 4.68693D-08 | 3.76438D-01 |
| P( 4) | 3 - 2 | 1296.34 | -506.84 | 3.32246D+00 | 8.33090D-08 | 3.77351D-01 |
| R( 2) | 3 - 3 | 1801.72 | -1.46 | 1.37110D-06 | 1.00000D+00 | 1.81816D+00 |
| R( 3) | 3 - 0 | 263.49 | -1541.63 | 3.44794D-04 | 4.55941D-13 | 8.21678D-04 |
| P( 5) | 3 - 0 | 267.94 | -1537.17 | 4.14022D-04 | 7.01683D-13 | 8.08840D-04 |
| R( 3) | 3 - 1 | 781.10 | -1024.01 | 8.33738D-02 | 1.90963D-10 | -2.36018D-02 |
| P( 5) | 3 - 1 | 785.53 | -1019.59 | 1.01620D-01 | 2.95367D-10 | -2.34577D-02 |
| R( 3) | 3 - 2 | 1294.38 | -510.73 | 2.62960D+00 | 8.33217D-08 | 3.76310D-01 |
| P( 5) | 3 - 2 | 1298.78 | -506.34 | 3.22286D+00 | 1.30179D-07 | 3.77484D-01 |
| R( 3) | 3 - 3 | 1803.17 | -1.94 | 3.37049D-06 | 1.00000D+00 | 1.81822D+00 |
| R( 4) | 3 - 0 | 265.47 | -1542.07 | 3.54180D-04 | 7.13642D-13 | 8.23123D-04 |
| P( 6) | 3 - 0 | 270.91 | -1536.63 | 4.04651D-04 | 1.00877D-12 | 8.07431D-04 |
| R( 4) | 3 - 1 | 783.07 | -1024.47 | 8.55067D-02 | 2.98784D-10 | -2.36188D-02 |
| P( 6) | 3 - 1 | 788.47 | -1019.07 | 9.94911D-02 | 4.24807D-10 | -2.34427D-02 |
| R( 4) | 3 - 2 | 1296.34 | -511.20 | 2.69500D+00 | 1.30191D-07 | 3.76182D-01 |
| P( 6) | 3 - 2 | 1301.71 | -505.83 | 3.15704D+00 | 1.87470D-07 | 3.77617D-01 |
| R( 4) | 3 - 3 | 1805.12 | -2.43 | 6.73288D-06 | 1.00000D+00 | 1.81830D+00 |
| R( 5) | 3 - 0 | 267.94 | -1542.51 | 3.61203D-04 | 1.02943D-12 | 8.24571D-04 |

| | | | | | | |
|---|---|---|---|---|---|---|
| P( 7) | 3 - 0 | 274.37 | -1536.08 | 3.97646D-04 | 1.37080D-12 | 8.06025D-04 |
| R( 5) | 3 - 1 | 785.53 | -1024.93 | 8.70642D-02 | 4.30823D-10 | -2.36360D-02 |
| P( 7) | 3 - 1 | 791.92 | -1018.54 | 9.79386D-02 | 5.77517D-10 | -2.34279D-02 |
| R( 5) | 3 - 2 | 1298.78 | -511.67 | 2.74215D+00 | 1.87478D-07 | 3.76055D-01 |
| P( 7) | 3 - 2 | 1305.13 | -505.32 | 3.10940D+00 | 2.55185D-07 | 3.77751D-01 |
| R( 5) | 3 - 3 | 1807.54 | -2.91 | 1.18140D-05 | 1.00000D+00 | 1.81840D+00 |
| R( 6) | 3 - 0 | 270.91 | -1542.94 | 3.66809D-04 | 1.40363D-12 | 8.26023D-04 |
| P( 8) | 3 - 0 | 278.33 | -1535.52 | 3.92060D-04 | 1.78753D-12 | 8.04623D-04 |
| R( 6) | 3 - 1 | 788.47 | -1025.38 | 8.82768D-02 | 5.87177D-10 | -2.36534D-02 |
| P( 8) | 3 - 1 | 795.85 | -1018.00 | 9.67320D-02 | 7.53418D-10 | -2.34132D-02 |
| R( 6) | 3 - 2 | 1301.71 | -512.14 | 2.77833D+00 | 2.55186D-07 | 3.75928D-01 |
| P( 8) | 3 - 2 | 1309.04 | -504.81 | 3.07264D+00 | 3.33327D-07 | 3.77885D-01 |
| R( 6) | 3 - 3 | 1810.45 | -3.40 | 1.89698D-05 | 9.99999D-01 | 1.81852D+00 |
| R( 7) | 3 - 0 | 274.37 | -1543.36 | 3.71500D-04 | 1.83654D-12 | 8.27479D-04 |
| P( 9) | 3 - 0 | 282.78 | -1534.95 | 3.87393D-04 | 2.25870D-12 | 8.03224D-04 |
| R( 7) | 3 - 1 | 791.92 | -1025.82 | 8.92662D-02 | 7.67943D-10 | -2.36710D-02 |
| P( 9) | 3 - 1 | 800.27 | -1017.46 | 9.57494D-02 | 9.52437D-10 | -2.33988D-02 |
| R( 7) | 3 - 2 | 1305.13 | -512.60 | 2.80739D+00 | 3.33318D-07 | 3.75802D-01 |
| P( 9) | 3 - 2 | 1313.43 | -504.30 | 3.04292D+00 | 4.21901D-07 | 3.78020D-01 |
| R( 7) | 3 - 3 | 1813.85 | -3.88 | 2.85563D-05 | 9.99999D-01 | 1.81866D+00 |
| R( 8) | 3 - 0 | 278.33 | -1543.77 | 3.75563D-04 | 2.32848D-12 | 8.28939D-04 |
| P( 10) | 3 - 0 | 287.73 | -1534.37 | 3.83356D-04 | 2.78404D-12 | 8.01828D-04 |
| R( 8) | 3 - 1 | 795.85 | -1026.25 | 9.01031D-02 | 9.73221D-10 | -2.36888D-02 |
| P( 10) | 3 - 1 | 805.19 | -1016.91 | 9.49201D-02 | 1.17450D-09 | -2.33846D-02 |
| R( 8) | 3 - 2 | 1309.04 | -513.06 | 2.83157D+00 | 4.21877D-07 | 3.75676D-01 |
| P( 10) | 3 - 2 | 1318.32 | -503.78 | 3.01800D+00 | 5.20910D-07 | 3.78156D-01 |
| R( 8) | 3 - 3 | 1817.73 | -4.37 | 4.09300D-05 | 9.99999D-01 | 1.81882D+00 |
| R( 9) | 3 - 0 | 282.78 | -1544.17 | 3.79180D-04 | 2.87978D-12 | 8.30402D-04 |
| P( 11) | 3 - 0 | 293.17 | -1533.78 | 3.79770D-04 | 3.36332D-12 | 8.00435D-04 |

| | | | | | | |
|---|---|---|---|---|---|---|
| R( 9) | 3 - 1 | 800.27 | -1026.68 | 9.08311D-02 | 1.20311D-09 | -2.37068D-02 |
| P( 11) | 3 - 1 | 810.59 | -1016.36 | 9.42005D-02 | 1.41953D-09 | -2.33705D-02 |
| R( 9) | 3 - 2 | 1313.43 | -513.52 | 2.85225D+00 | 5.20867D-07 | 3.75551D-01 |
| P( 11) | 3 - 2 | 1323.69 | -503.26 | 2.99649D+00 | 6.30360D-07 | 3.78292D-01 |
| R( 9) | 3 - 3 | 1822.10 | -4.85 | 5.64474D-05 | 9.99999D-01 | 1.81899D+00 |
| R( 10) | 3 - 0 | 287.73 | -1544.56 | 3.82466D-04 | 3.49077D-12 | 8.31870D-04 |
| P( 12) | 3 - 0 | 299.10 | -1533.19 | 3.76516D-04 | 3.99628D-12 | 7.99046D-04 |
| R( 10) | 3 - 1 | 805.19 | -1027.10 | 9.14789D-02 | 1.45772D-09 | -2.37250D-02 |
| P( 12) | 3 - 1 | 816.49 | -1015.80 | 9.35621D-02 | 1.68747D-09 | -2.33567D-02 |
| R( 10) | 3 - 2 | 1318.32 | -513.97 | 2.87034D+00 | 6.30291D-07 | 3.75426D-01 |
| P( 12) | 3 - 2 | 1329.55 | -502.74 | 2.97750D+00 | 7.50255D-07 | 3.78428D-01 |
| R( 10) | 3 - 3 | 1826.95 | -5.34 | 7.54653D-05 | 9.99999D-01 | 1.81919D+00 |
| R( 11) | 3 - 0 | 293.17 | -1544.94 | 3.85502D-04 | 4.16177D-12 | 8.33342D-04 |
| P( 13) | 3 - 0 | 305.53 | -1532.58 | 3.73516D-04 | 4.68268D-12 | 7.97660D-04 |
| R( 11) | 3 - 1 | 810.59 | -1027.52 | 9.20656D-02 | 1.73715D-09 | -2.37434D-02 |
| P( 13) | 3 - 1 | 822.88 | -1015.23 | 9.29856D-02 | 1.97823D-09 | -2.33431D-02 |
| R( 11) | 3 - 2 | 1323.69 | -514.42 | 2.88643D+00 | 7.50156D-07 | 3.75301D-01 |
| P( 13) | 3 - 2 | 1335.90 | -502.21 | 2.96041D+00 | 8.80602D-07 | 3.78566D-01 |
| R( 11) | 3 - 3 | 1832.29 | -5.82 | 9.83411D-05 | 9.99998D-01 | 1.81940D+00 |
| R( 12) | 3 - 0 | 299.10 | -1545.31 | 3.88343D-04 | 4.89312D-12 | 8.34817D-04 |
| P( 14) | 3 - 0 | 312.46 | -1531.96 | 3.70714D-04 | 5.42228D-12 | 7.96277D-04 |
| R( 12) | 3 - 1 | 816.49 | -1027.93 | 9.26050D-02 | 2.04150D-09 | -2.37620D-02 |
| P( 14) | 3 - 1 | 829.76 | -1014.66 | 9.24572D-02 | 2.29176D-09 | -2.33296D-02 |
| R( 12) | 3 - 2 | 1329.55 | -514.87 | 2.90098D+00 | 8.80465D-07 | 3.75177D-01 |
| P( 14) | 3 - 2 | 1342.73 | -501.68 | 2.94480D+00 | 1.02141D-06 | 3.78703D-01 |
| R( 12) | 3 - 3 | 1838.11 | -6.31 | 1.25432D-04 | 9.99998D-01 | 1.81963D+00 |
| R( 13) | 3 - 0 | 305.53 | -1545.68 | 3.91030D-04 | 5.68517D-12 | 8.36297D-04 |
| P( 15) | 3 - 0 | 319.87 | -1531.34 | 3.68069D-04 | 6.21485D-12 | 7.94897D-04 |
| R( 13) | 3 - 1 | 822.88 | -1028.33 | 9.31070D-02 | 2.37089D-09 | -2.37808D-02 |

| | | | | | | | |
|---|---|---|---|---|---|---|---|
| P( 15) | 3 - 1 | 837.13 | -1014.08 | 9.19671D-02 | 2.62798D-09 | -2.33164D-02 |
| R( 13) | 3 - 2 | 1335.90 | -515.31 | 2.91427D+00 | 1.02123D-06 | 3.75054D-01 |
| P( 15) | 3 - 2 | 1350.06 | -501.15 | 2.93034D+00 | 1.17268D-06 | 3.78842D-01 |
| R( 13) | 3 - 3 | 1844.42 | -6.79 | 1.57097D-04 | 9.99998D-01 | 1.81988D+00 |
| R( 14) | 3 - 0 | 312.46 | -1546.03 | 3.93593D-04 | 6.53826D-12 | 8.37781D-04 |
| P( 16) | 3 - 0 | 327.79 | -1530.70 | 3.65551D-04 | 7.06015D-12 | 7.93520D-04 |
| R( 14) | 3 - 1 | 829.76 | -1028.73 | 9.35788D-02 | 2.72542D-09 | -2.37998D-02 |
| P( 16) | 3 - 1 | 844.99 | -1013.49 | 9.15080D-02 | 2.98684D-09 | -2.33034D-02 |
| R( 14) | 3 - 2 | 1342.73 | -515.75 | 2.92656D+00 | 1.17244D-06 | 3.74931D-01 |
| P( 16) | 3 - 2 | 1357.87 | -500.62 | 2.91682D+00 | 1.33442D-06 | 3.78981D-01 |
| R( 14) | 3 - 3 | 1851.21 | -7.28 | 1.93693D-04 | 9.99997D-01 | 1.82014D+00 |
| R( 15) | 3 - 0 | 319.87 | -1546.37 | 3.96054D-04 | 7.45274D-12 | 8.39269D-04 |
| P( 17) | 3 - 0 | 336.19 | -1530.06 | 3.63137D-04 | 7.95796D-12 | 7.92146D-04 |
| R( 15) | 3 - 1 | 837.13 | -1029.12 | 9.40261D-02 | 3.10521D-09 | -2.38190D-02 |
| P( 17) | 3 - 1 | 853.35 | -1012.90 | 9.10743D-02 | 3.36827D-09 | -2.32905D-02 |
| R( 15) | 3 - 2 | 1350.06 | -516.19 | 2.93801D+00 | 1.33412D-06 | 3.74808D-01 |
| P( 17) | 3 - 2 | 1366.17 | -500.08 | 2.90405D+00 | 1.50664D-06 | 3.79121D-01 |
| R( 15) | 3 - 3 | 1858.49 | -7.76 | 2.35580D-04 | 9.99997D-01 | 1.82043D+00 |
| R( 16) | 3 - 0 | 327.79 | -1546.71 | 3.98432D-04 | 8.42896D-12 | 8.40762D-04 |
| P( 18) | 3 - 0 | 345.09 | -1529.40 | 3.60811D-04 | 8.90805D-12 | 7.90776D-04 |
| R( 16) | 3 - 1 | 844.99 | -1029.50 | 9.44531D-02 | 3.51037D-09 | -2.38384D-02 |
| P( 18) | 3 - 1 | 862.19 | -1012.30 | 9.06619D-02 | 3.77220D-09 | -2.32779D-02 |
| R( 16) | 3 - 2 | 1357.87 | -516.62 | 2.94876D+00 | 1.50627D-06 | 3.74686D-01 |
| P( 18) | 3 - 2 | 1374.96 | -499.54 | 2.89189D+00 | 1.68934D-06 | 3.79261D-01 |
| R( 16) | 3 - 3 | 1866.25 | -8.25 | 2.83117D-04 | 9.99996D-01 | 1.82073D+00 |
| R( 17) | 3 - 0 | 336.19 | -1547.03 | 4.00740D-04 | 9.46729D-12 | 8.42259D-04 |
| P( 19) | 3 - 0 | 354.48 | -1528.74 | 3.58557D-04 | 9.91019D-12 | 7.89408D-04 |
| R( 17) | 3 - 1 | 853.35 | -1029.88 | 9.48631D-02 | 3.94102D-09 | -2.38580D-02 |
| P( 19) | 3 - 1 | 871.53 | -1011.70 | 9.02672D-02 | 4.19860D-09 | -2.32654D-02 |

| | | | | | | | |
|---|---|---|---|---|---|---|---|
| R( 17) | 3 - 2 | 1366.17 | -517.05 | 2.95891D+00 | 1.68890D-06 | 3.74565D-01 |
| P( 19) | 3 - 2 | 1384.23 | -498.99 | 2.88025D+00 | 1.88255D-06 | 3.79402D-01 |
| R( 17) | 3 - 3 | 1874.49 | -8.73 | 3.36663D-04 | 9.99996D-01 | 1.82106D+00 |
| R( 18) | 3 - 0 | 345.09 | -1547.35 | 4.02989D-04 | 1.05681D-11 | 8.43760D-04 |
| P( 20) | 3 - 0 | 364.37 | -1528.07 | 3.56366D-04 | 1.09642D-11 | 7.88043D-04 |
| R( 18) | 3 - 1 | 862.19 | -1030.25 | 9.52588D-02 | 4.39726D-09 | -2.38778D-02 |
| P( 20) | 3 - 1 | 881.35 | -1011.09 | 8.98876D-02 | 4.64738D-09 | -2.32532D-02 |
| R( 18) | 3 - 2 | 1374.96 | -517.48 | 2.96856D+00 | 1.88202D-06 | 3.74443D-01 |
| P( 20) | 3 - 2 | 1394.00 | -498.44 | 2.86904D+00 | 2.08626D-06 | 3.79544D-01 |
| R( 18) | 3 - 3 | 1883.22 | -9.21 | 3.96579D-04 | 9.99996D-01 | 1.82140D+00 |
| R( 19) | 3 - 0 | 354.48 | -1547.65 | 4.05187D-04 | 1.17317D-11 | 8.45265D-04 |
| P( 21) | 3 - 0 | 374.75 | -1527.39 | 3.54228D-04 | 1.20698D-11 | 7.86682D-04 |
| R( 19) | 3 - 1 | 871.53 | -1030.61 | 9.56424D-02 | 4.87921D-09 | -2.38978D-02 |
| P( 21) | 3 - 1 | 891.67 | -1010.47 | 8.95211D-02 | 5.11848D-09 | -2.32412D-02 |
| R( 19) | 3 - 2 | 1384.23 | -517.90 | 2.97775D+00 | 2.08563D-06 | 3.74323D-01 |
| P( 21) | 3 - 2 | 1404.25 | -497.89 | 2.85819D+00 | 2.30048D-06 | 3.79686D-01 |
| R( 19) | 3 - 3 | 1892.44 | -9.70 | 4.63227D-04 | 9.99995D-01 | 1.82176D+00 |
| P( 1) | 4 - 0 | 261.02 | -2043.27 | 2.25886D-05 | 3.96086D-16 | 9.18872D-05 |
| P( 1) | 4 - 1 | 778.64 | -1525.65 | 3.03799D-03 | 1.15027D-13 | -1.65163D-03 |
| P( 1) | 4 - 2 | 1291.94 | -1012.35 | 3.72118D-01 | 2.40851D-11 | 3.38178D-02 |
| P( 1) | 4 - 3 | 1800.75 | -503.54 | 7.52370D+00 | 6.97930D-09 | -4.33475D-01 |
| R( 0) | 4 - 0 | 260.52 | -2044.25 | 7.59726D-06 | 4.00852D-16 | 9.22333D-05 |
| P( 2) | 4 - 0 | 262.01 | -2042.76 | 1.49914D-05 | 1.58210D-15 | 9.17146D-05 |
| R( 0) | 4 - 1 | 778.15 | -1526.62 | 1.02168D-03 | 1.14568D-13 | -1.65738D-03 |
| P( 2) | 4 - 1 | 779.63 | -1525.14 | 2.01632D-03 | 4.58305D-13 | -1.64876D-03 |
| R( 0) | 4 - 2 | 1291.45 | -1013.32 | 1.24727D-01 | 2.40285D-11 | 3.38628D-02 |
| P( 2) | 4 - 2 | 1292.92 | -1011.85 | 2.47393D-01 | 9.61004D-11 | 3.37958D-02 |
| R( 0) | 4 - 3 | 1800.26 | -504.51 | 2.51879D+00 | 6.98117D-09 | -4.33166D-01 |
| P( 2) | 4 - 3 | 1801.72 | -503.05 | 5.00480D+00 | 2.79193D-08 | -4.33630D-01 |

| | | | | | | |
|---|---|---|---|---|---|---|
| R( 0) | 4 - 4 | 2304.29 | -0.48 | 4.05457D-08 | 1.00000D+00 | -1.86025D+00 |
| R( 1) | 4 - 0 | 261.02 | -2044.72 | 9.15735D-06 | 1.60913D-15 | 9.24068D-05 |
| P( 3) | 4 - 0 | 263.49 | -2042.24 | 1.34314D-05 | 3.54606D-15 | 9.15423D-05 |
| R( 1) | 4 - 1 | 778.64 | -1527.09 | 1.23143D-03 | 4.60347D-13 | -1.66026D-03 |
| P( 3) | 4 - 1 | 781.10 | -1524.63 | 1.80659D-03 | 1.02813D-12 | -1.64590D-03 |
| R( 1) | 4 - 2 | 1291.94 | -1013.79 | 1.50087D-01 | 9.63698D-11 | 3.38857D-02 |
| P( 3) | 4 - 2 | 1294.38 | -1011.35 | 2.22037D-01 | 2.15847D-10 | 3.37741D-02 |
| R( 1) | 4 - 3 | 1800.75 | -504.99 | 3.02901D+00 | 2.79240D-08 | -4.33012D-01 |
| P( 3) | 4 - 3 | 1803.17 | -502.56 | 4.49436D+00 | 6.28196D-08 | -4.33786D-01 |
| R( 1) | 4 - 4 | 2304.77 | -0.96 | 3.89247D-07 | 1.00000D+00 | -1.86027D+00 |
| R( 2) | 4 - 0 | 262.01 | -2045.17 | 9.85501D-06 | 3.60283D-15 | 9.25807D-05 |
| P( 4) | 4 - 0 | 265.47 | -2041.71 | 1.27338D-05 | 6.32124D-15 | 9.13703D-05 |
| R( 2) | 4 - 1 | 779.63 | -1527.55 | 1.32520D-03 | 1.03653D-12 | -1.66316D-03 |
| P( 4) | 4 - 1 | 783.07 | -1524.11 | 1.71285D-03 | 1.82622D-12 | -1.64305D-03 |
| R( 2) | 4 - 2 | 1292.92 | -1014.26 | 1.61252D-01 | 2.17105D-10 | 3.39089D-02 |
| P( 4) | 4 - 2 | 1296.34 | -1010.84 | 2.10879D-01 | 3.83301D-10 | 3.37527D-02 |
| R( 2) | 4 - 3 | 1801.72 | -505.46 | 3.25225D+00 | 6.28229D-08 | -4.32859D-01 |
| P( 4) | 4 - 3 | 1805.12 | -502.07 | 4.27079D+00 | 1.11691D-07 | -4.33942D-01 |
| R( 2) | 4 - 4 | 2305.73 | -1.45 | 1.40755D-06 | 1.00000D+00 | -1.86032D+00 |
| R( 3) | 4 - 0 | 263.49 | -2045.62 | 1.02652D-05 | 6.41727D-15 | 9.27548D-05 |
| P( 5) | 4 - 0 | 267.94 | -2041.17 | 1.23237D-05 | 9.85876D-15 | 9.11986D-05 |
| R( 3) | 4 - 1 | 781.10 | -1528.01 | 1.38031D-03 | 1.84663D-12 | -1.66606D-03 |
| P( 5) | 4 - 1 | 785.53 | -1523.58 | 1.65779D-03 | 2.84811D-12 | -1.64021D-03 |
| R( 3) | 4 - 2 | 1294.38 | -1014.73 | 1.67686D-01 | 3.86534D-10 | 3.39325D-02 |
| P( 5) | 4 - 2 | 1298.78 | -1010.33 | 2.04453D-01 | 5.98131D-10 | 3.37317D-02 |
| R( 3) | 4 - 3 | 1803.17 | -505.93 | 3.37979D+00 | 1.11686D-07 | -4.32706D-01 |
| P( 5) | 4 - 3 | 1807.54 | -501.57 | 4.14281D+00 | 1.74526D-07 | -4.34099D-01 |
| R( 3) | 4 - 4 | 2307.18 | -1.93 | 3.46010D-06 | 1.00000D+00 | -1.86038D+00 |
| R( 4) | 4 - 0 | 265.47 | -2046.05 | 1.05447D-05 | 1.00463D-14 | 9.29293D-05 |

| | | | | | | | |
|---|---|---|---|---|---|---|---|
| P( 6) | 4 - 0 | 270.91 | -2040.61 | 1.20443D-05 | 1.41706D-14 | 9.10272D-05 |
| R( 4) | 4 - 1 | 783.07 | -1528.45 | 1.41785D-03 | 2.89105D-12 | -1.66897D-03 |
| P( 6) | 4 - 1 | 788.47 | -1523.05 | 1.62030D-03 | 4.09396D-12 | -1.63738D-03 |
| R( 4) | 4 - 2 | 1296.34 | -1015.18 | 1.71970D-01 | 6.04803D-10 | 3.39564D-02 |
| P( 6) | 4 - 2 | 1301.71 | -1009.81 | 2.00179D-01 | 8.60237D-10 | 3.37109D-02 |
| R( 4) | 4 - 3 | 1805.12 | -506.40 | 3.46380D+00 | 1.74512D-07 | -4.32554D-01 |
| P( 6) | 4 - 3 | 1810.45 | -501.07 | 4.05825D+00 | 2.51332D-07 | -4.34257D-01 |
| R( 4) | 4 - 4 | 2309.11 | -2.41 | 6.91186D-06 | 1.00000D+00 | -1.86047D+00 |
| R( 5) | 4 - 0 | 267.94 | -2046.47 | 1.07539D-05 | 1.44945D-14 | 9.31041D-05 |
| P( 7) | 4 - 0 | 274.37 | -2040.04 | 1.18353D-05 | 1.92526D-14 | 9.08561D-05 |
| R( 5) | 4 - 1 | 785.53 | -1528.89 | 1.44593D-03 | 4.17103D-12 | -1.67188D-03 |
| P( 7) | 4 - 1 | 791.92 | -1522.50 | 1.59229D-03 | 5.56269D-12 | -1.63455D-03 |
| R( 5) | 4 - 2 | 1298.78 | -1015.63 | 1.75098D-01 | 8.72104D-10 | 3.39806D-02 |
| P( 7) | 4 - 2 | 1305.13 | -1009.28 | 1.97065D-01 | 1.16946D-09 | 3.36905D-02 |
| R( 5) | 4 - 3 | 1807.54 | -506.87 | 3.52434D+00 | 2.51305D-07 | -4.32403D-01 |
| P( 7) | 4 - 3 | 1813.85 | -500.56 | 3.99705D+00 | 3.42112D-07 | -4.34415D-01 |
| R( 5) | 4 - 4 | 2311.52 | -2.89 | 1.21280D-05 | 9.99999D-01 | -1.86057D+00 |
| R( 6) | 4 - 0 | 270.91 | -2046.88 | 1.09208D-05 | 1.97670D-14 | 9.32793D-05 |
| P( 8) | 4 - 0 | 278.33 | -2039.46 | 1.16686D-05 | 2.51006D-14 | 9.06852D-05 |
| R( 6) | 4 - 1 | 788.47 | -1529.31 | 1.46834D-03 | 5.68784D-12 | -1.67481D-03 |
| P( 8) | 4 - 1 | 795.85 | -1521.94 | 1.56996D-03 | 7.25325D-12 | -1.63173D-03 |
| R( 6) | 4 - 2 | 1301.71 | -1016.08 | 1.77531D-01 | 1.18863D-09 | 3.40051D-02 |
| P( 8) | 4 - 2 | 1309.04 | -1008.75 | 1.94646D-01 | 1.52566D-09 | 3.36703D-02 |
| R( 6) | 4 - 3 | 1810.45 | -507.33 | 3.57077D+00 | 3.42066D-07 | -4.32251D-01 |
| P( 8) | 4 - 3 | 1817.73 | -500.05 | 3.94985D+00 | 4.46871D-07 | -4.34574D-01 |
| R( 6) | 4 - 4 | 2314.41 | -3.37 | 1.94739D-05 | 9.99999D-01 | -1.86069D+00 |
| R( 7) | 4 - 0 | 274.37 | -2047.27 | 1.10604D-05 | 2.58684D-14 | 9.34548D-05 |
| P( 9) | 4 - 0 | 282.78 | -2038.86 | 1.15292D-05 | 3.17105D-14 | 9.05147D-05 |
| R( 7) | 4 - 1 | 791.92 | -1529.73 | 1.48709D-03 | 7.44275D-12 | -1.67774D-03 |

| | | | | | | |
|---|---|---|---|---|---|---|
| P( 9) | 4 - 1 | 800.27 | -1521.37 | 1.55131D-03 | 9.16463D-12 | -1.62891D-03 |
| R( 7) | 4 - 2 | 1305.13 | -1016.51 | 1.79516D-01 | 1.55459D-09 | 3.40299D-02 |
| P( 9) | 4 - 2 | 1313.43 | -1008.21 | 1.92678D-01 | 1.92867D-09 | 3.36505D-02 |
| R( 7) | 4 - 3 | 1813.85 | -507.79 | 3.60807D+00 | 4.46799D-07 | -4.32101D-01 |
| P( 9) | 4 - 3 | 1822.10 | -499.54 | 3.91168D+00 | 5.65615D-07 | -4.34733D-01 |
| R( 7) | 4 - 4 | 2317.79 | -3.86 | 2.93152D-05 | 9.99999D-01 | -1.86083D+00 |
| R( 8) | 4 - 0 | 278.33 | -2047.65 | 1.11814D-05 | 3.28038D-14 | 9.36306D-05 |
| P( 10) | 4 - 0 | 287.73 | -2038.25 | 1.14084D-05 | 3.90783D-14 | 9.03444D-05 |
| R( 8) | 4 - 1 | 795.85 | -1530.13 | 1.50332D-03 | 9.43709D-12 | -1.68068D-03 |
| P( 10) | 4 - 1 | 805.19 | -1520.80 | 1.53517D-03 | 1.12958D-11 | -1.62610D-03 |
| R( 8) | 4 - 2 | 1309.04 | -1016.94 | 1.81194D-01 | 1.97017D-09 | 3.40550D-02 |
| P( 10) | 4 - 2 | 1318.32 | -1007.67 | 1.91019D-01 | 2.37836D-09 | 3.36310D-02 |
| R( 8) | 4 - 3 | 1817.73 | -508.25 | 3.63908D+00 | 5.65509D-07 | -4.31951D-01 |
| P( 10) | 4 - 3 | 1826.95 | -499.03 | 3.87967D+00 | 6.98349D-07 | -4.34893D-01 |
| R( 8) | 4 - 4 | 2321.64 | -4.34 | 4.20175D-05 | 9.99999D-01 | -1.86099D+00 |
| R( 9) | 4 - 0 | 282.78 | -2048.02 | 1.12890D-05 | 4.05782D-14 | 9.38068D-05 |
| P( 11) | 4 - 0 | 293.17 | -2037.63 | 1.13011D-05 | 4.72000D-14 | 9.01744D-05 |
| R( 9) | 4 - 1 | 800.27 | -1530.53 | 1.51776D-03 | 1.16721D-11 | -1.68363D-03 |
| P( 11) | 4 - 1 | 810.59 | -1520.21 | 1.52084D-03 | 1.36458D-11 | -1.62330D-03 |
| R( 9) | 4 - 2 | 1313.43 | -1017.37 | 1.82654D-01 | 2.43559D-09 | 3.40804D-02 |
| P( 11) | 4 - 2 | 1323.69 | -1007.11 | 1.89580D-01 | 2.87458D-09 | 3.36118D-02 |
| R( 9) | 4 - 3 | 1822.10 | -508.70 | 3.66559D+00 | 6.98201D-07 | -4.31801D-01 |
| P( 11) | 4 - 3 | 1832.29 | -498.51 | 3.85206D+00 | 8.45079D-07 | -4.35053D-01 |
| R( 9) | 4 - 4 | 2325.98 | -4.82 | 5.79469D-05 | 9.99998D-01 | -1.86116D+00 |
| R( 10) | 4 - 0 | 287.73 | -2048.38 | 1.13867D-05 | 4.91966D-14 | 9.39834D-05 |
| P( 12) | 4 - 0 | 299.10 | -2037.00 | 1.12037D-05 | 5.60718D-14 | 9.00047D-05 |
| R( 10) | 4 - 1 | 805.19 | -1530.92 | 1.53088D-03 | 1.41493D-11 | -1.68659D-03 |
| P( 12) | 4 - 1 | 816.49 | -1519.61 | 1.50785D-03 | 1.62135D-11 | -1.62051D-03 |
| R( 10) | 4 - 2 | 1318.32 | -1017.79 | 1.83952D-01 | 2.95105D-09 | 3.41061D-02 |

| | | | | | | |
|---|---|---|---|---|---|---|
| P( 12) | 4 - 2 | 1329.55 | -1006.56 | 1.88306D-01 | 3.41719D-09 | 3.35929D-02 |
| R( 10) | 4 - 3 | 1826.95 | -509.15 | 3.68876D+00 | 8.44880D-07 | -4.31652D-01 |
| P( 12) | 4 - 3 | 1838.11 | -497.99 | 3.82768D+00 | 1.00581D-06 | -4.35214D-01 |
| R( 10) | 4 - 4 | 2330.80 | -5.30 | 7.74696D-05 | 9.99998D-01 | -1.86136D+00 |
| R( 11) | 4 - 0 | 293.17 | -2048.72 | 1.14770D-05 | 5.86643D-14 | 9.41604D-05 |
| P( 13) | 4 - 0 | 305.53 | -2036.36 | 1.11138D-05 | 6.56897D-14 | 8.98352D-05 |
| R( 11) | 4 - 1 | 810.59 | -1531.30 | 1.54299D-03 | 1.68699D-11 | -1.68955D-03 |
| P( 13) | 4 - 1 | 822.88 | -1519.01 | 1.49587D-03 | 1.89982D-11 | -1.61772D-03 |
| R( 11) | 4 - 2 | 1323.69 | -1018.20 | 1.85128D-01 | 3.51677D-09 | 3.41322D-02 |
| P( 13) | 4 - 2 | 1335.90 | -1005.99 | 1.87155D-01 | 4.00605D-09 | 3.35743D-02 |
| R( 11) | 4 - 3 | 1832.29 | -509.60 | 3.70938D+00 | 1.00555D-06 | -4.31503D-01 |
| P( 13) | 4 - 3 | 1844.42 | -497.47 | 3.80574D+00 | 1.18056D-06 | -4.35376D-01 |
| R( 11) | 4 - 4 | 2336.11 | -5.78 | 1.00952D-04 | 9.99998D-01 | -1.86157D+00 |
| R( 12) | 4 - 0 | 299.10 | -2049.05 | 1.15614D-05 | 6.89863D-14 | 9.43377D-05 |
| P( 14) | 4 - 0 | 312.46 | -2035.70 | 1.10297D-05 | 7.60499D-14 | 8.96661D-05 |
| R( 12) | 4 - 1 | 816.49 | -1531.66 | 1.55433D-03 | 1.98352D-11 | -1.69253D-03 |
| P( 14) | 4 - 1 | 829.76 | -1518.39 | 1.48467D-03 | 2.19987D-11 | -1.61494D-03 |
| R( 12) | 4 - 2 | 1329.55 | -1018.61 | 1.86209D-01 | 4.13297D-09 | 3.41586D-02 |
| P( 14) | 4 - 2 | 1342.73 | -1005.42 | 1.86102D-01 | 4.64103D-09 | 3.35560D-02 |
| R( 12) | 4 - 3 | 1838.11 | -510.04 | 3.72799D+00 | 1.18023D-06 | -4.31355D-01 |
| P( 14) | 4 - 3 | 1851.21 | -496.95 | 3.78570D+00 | 1.36933D-06 | -4.35538D-01 |
| R( 12) | 4 - 4 | 2341.89 | -6.27 | 1.28762D-04 | 9.99997D-01 | -1.86180D+00 |
| R( 13) | 4 - 0 | 305.53 | -2049.37 | 1.16412D-05 | 8.01681D-14 | 9.45154D-05 |
| P( 15) | 4 - 0 | 319.87 | -2035.03 | 1.09503D-05 | 8.71487D-14 | 8.94972D-05 |
| R( 13) | 4 - 1 | 822.88 | -1532.02 | 1.56505D-03 | 2.30468D-11 | -1.69551D-03 |
| P( 15) | 4 - 1 | 837.13 | -1517.77 | 1.47411D-03 | 2.52142D-11 | -1.61216D-03 |
| R( 13) | 4 - 2 | 1335.90 | -1019.01 | 1.87214D-01 | 4.79987D-09 | 3.41852D-02 |
| P( 15) | 4 - 2 | 1350.06 | -1004.84 | 1.85126D-01 | 5.32201D-09 | 3.35380D-02 |
| R( 13) | 4 - 3 | 1844.42 | -510.48 | 3.74501D+00 | 1.36891D-06 | -4.31207D-01 |

| | | | | | | | |
|---|---|---|---|---|---|---|---|
| P( 15) | 4 - 3 | 1858.49 | -496.42 | 3.76715D+00 | 1.57212D-06 | -4.35701D-01 |
| R( 13) | 4 - 4 | 2348.16 | -6.75 | 1.61266D-04 | 9.99997D-01 | -1.86205D+00 |
| R( 14) | 4 - 0 | 312.46 | -2049.68 | 1.17173D-05 | 9.22149D-14 | 9.46935D-05 |
| P( 16) | 4 - 0 | 327.79 | -2034.35 | 1.08747D-05 | 9.89824D-14 | 8.93285D-05 |
| R( 14) | 4 - 1 | 829.76 | -1532.37 | 1.57527D-03 | 2.65061D-11 | -1.69850D-03 |
| P( 16) | 4 - 1 | 844.99 | -1517.14 | 1.46406D-03 | 2.86438D-11 | -1.60939D-03 |
| R( 14) | 4 - 2 | 1342.73 | -1019.40 | 1.88159D-01 | 5.51769D-09 | 3.42122D-02 |
| P( 16) | 4 - 2 | 1357.87 | -1004.26 | 1.84212D-01 | 6.04885D-09 | 3.35204D-02 |
| R( 14) | 4 - 3 | 1851.21 | -510.92 | 3.76072D+00 | 1.57160D-06 | -4.31060D-01 |
| P( 16) | 4 - 3 | 1866.25 | -495.88 | 3.74978D+00 | 1.78896D-06 | -4.35865D-01 |
| R( 14) | 4 - 4 | 2354.90 | -7.23 | 1.98833D-04 | 9.99996D-01 | -1.86232D+00 |
| R( 15) | 4 - 0 | 319.87 | -2049.97 | 1.17904D-05 | 1.05132D-13 | 9.48721D-05 |
| P( 17) | 4 - 0 | 336.19 | -2033.65 | 1.08021D-05 | 1.11547D-13 | 8.91602D-05 |
| R( 15) | 4 - 1 | 837.13 | -1532.71 | 1.58508D-03 | 3.02144D-11 | -1.70150D-03 |
| P( 17) | 4 - 1 | 853.35 | -1516.50 | 1.45442D-03 | 3.22865D-11 | -1.60662D-03 |
| R( 15) | 4 - 2 | 1350.06 | -1019.78 | 1.89055D-01 | 6.28667D-09 | 3.42395D-02 |
| P( 17) | 4 - 2 | 1366.17 | -1003.67 | 1.83350D-01 | 6.82143D-09 | 3.35030D-02 |
| R( 15) | 4 - 3 | 1858.49 | -511.36 | 3.77535D+00 | 1.78832D-06 | -4.30913D-01 |
| P( 17) | 4 - 3 | 1874.49 | -495.35 | 3.73339D+00 | 2.01984D-06 | -4.36029D-01 |
| R( 15) | 4 - 4 | 2362.13 | -7.71 | 2.41829D-04 | 9.99996D-01 | -1.86261D+00 |
| R( 16) | 4 - 0 | 327.79 | -2050.25 | 1.18609D-05 | 1.18925D-13 | 9.50510D-05 |
| P( 18) | 4 - 0 | 345.09 | -2032.94 | 1.07321D-05 | 1.24840D-13 | 8.89921D-05 |
| R( 16) | 4 - 1 | 844.99 | -1533.04 | 1.59456D-03 | 3.41733D-11 | -1.70450D-03 |
| P( 18) | 4 - 1 | 862.19 | -1515.84 | 1.44513D-03 | 3.61415D-11 | -1.60387D-03 |
| R( 16) | 4 - 2 | 1357.87 | -1020.16 | 1.89911D-01 | 7.10703D-09 | 3.42672D-02 |
| P( 18) | 4 - 2 | 1374.96 | -1003.08 | 1.82531D-01 | 7.63968D-09 | 3.34860D-02 |
| R( 16) | 4 - 3 | 1866.25 | -511.79 | 3.78908D+00 | 2.01908D-06 | -4.30766D-01 |
| P( 18) | 4 - 3 | 1883.22 | -494.81 | 3.71779D+00 | 2.26479D-06 | -4.36194D-01 |
| R( 16) | 4 - 4 | 2369.84 | -8.19 | 2.90624D-04 | 9.99995D-01 | -1.86291D+00 |

| | | | | | | |
|---|---|---|---|---|---|---|
| R( 17) | 4 - 0 | 336.19 | -2050.52 | 1.19293D-05 | 1.33600D-13 | 9.52304D-05 |
| P( 19) | 4 - 0 | 354.48 | -2032.22 | 1.06643D-05 | 1.38856D-13 | 8.88244D-05 |
| R( 17) | 4 - 1 | 853.35 | -1533.36 | 1.60375D-03 | 3.83842D-11 | -1.70752D-03 |
| P( 19) | 4 - 1 | 871.53 | -1515.18 | 1.43613D-03 | 4.02070D-11 | -1.60111D-03 |
| R( 17) | 4 - 2 | 1366.17 | -1020.54 | 1.90732D-01 | 7.97902D-09 | 3.42951D-02 |
| P( 19) | 4 - 2 | 1384.23 | -1002.48 | 1.81747D-01 | 8.50340D-09 | 3.34693D-02 |
| R( 17) | 4 - 3 | 1874.49 | -512.21 | 3.80205D+00 | 2.26387D-06 | -4.30620D-01 |
| P( 19) | 4 - 3 | 1892.44 | -494.27 | 3.70285D+00 | 2.52380D-06 | -4.36360D-01 |
| R( 17) | 4 - 4 | 2378.03 | -8.67 | 3.45588D-04 | 9.99995D-01 | -1.86324D+00 |
| R( 18) | 4 - 0 | 345.09 | -2050.77 | 1.19959D-05 | 1.49162D-13 | 9.54102D-05 |
| P( 20) | 4 - 0 | 364.37 | -2031.49 | 1.05983D-05 | 1.53593D-13 | 8.86569D-05 |
| R( 18) | 4 - 1 | 862.19 | -1533.67 | 1.61271D-03 | 4.28486D-11 | -1.71054D-03 |
| P( 20) | 4 - 1 | 881.35 | -1514.51 | 1.42738D-03 | 4.44840D-11 | -1.59837D-03 |
| R( 18) | 4 - 2 | 1374.96 | -1020.90 | 1.91525D-01 | 8.90283D-09 | 3.43233D-02 |
| P( 20) | 4 - 2 | 1394.00 | -1001.87 | 1.80995D-01 | 9.41251D-09 | 3.34529D-02 |
| R( 18) | 4 - 3 | 1883.22 | -512.64 | 3.81435D+00 | 2.52273D-06 | -4.30475D-01 |
| P( 20) | 4 - 3 | 1902.14 | -493.73 | 3.68845D+00 | 2.79691D-06 | -4.36526D-01 |
| R( 18) | 4 - 4 | 2386.71 | -9.15 | 4.07089D-04 | 9.99994D-01 | -1.86358D+00 |
| R( 19) | 4 - 0 | 354.48 | -2051.01 | 1.20610D-05 | 1.65617D-13 | 9.55905D-05 |
| P( 21) | 4 - 0 | 374.75 | -2030.75 | 1.05339D-05 | 1.69047D-13 | 8.84896D-05 |
| R( 19) | 4 - 1 | 871.53 | -1533.97 | 1.62147D-03 | 4.75691D-11 | -1.71358D-03 |
| P( 21) | 4 - 1 | 891.67 | -1513.83 | 1.41884D-03 | 4.89706D-11 | -1.59562D-03 |
| R( 19) | 4 - 2 | 1384.23 | -1021.27 | 1.92294D-01 | 9.87879D-09 | 3.43519D-02 |
| P( 21) | 4 - 2 | 1404.25 | -1001.25 | 1.80268D-01 | 1.03669D-08 | 3.34368D-02 |
| R( 19) | 4 - 3 | 1892.44 | -513.06 | 3.82608D+00 | 2.79565D-06 | -4.30329D-01 |
| P( 21) | 4 - 3 | 1912.32 | -493.18 | 3.67452D+00 | 3.08410D-06 | -4.36693D-01 |
| R( 19) | 4 - 4 | 2395.86 | -9.64 | 4.75498D-04 | 9.99994D-01 | -1.86394D+00 |
| P( 1) | 5 - 0 | 261.02 | -2542.44 | 8.55561D-07 | 8.61330D-18 | 1.28839D-05 |
| P( 1) | 5 - 1 | 778.64 | -2024.81 | 1.20308D-04 | 1.84380D-15 | -2.14965D-04 |

| | | | | | | | |
|---|---|---|---|---|---|---|---|
| P( 1) | 5 - 2 | 1291.94 | -1511.51 | 7.37073D-03 | 2.87868D-13 | 2.60877D-03 |
| P( 1) | 5 - 3 | 1800.75 | -1002.71 | 6.18410D-01 | 4.03960D-11 | -4.42258D-02 |
| P( 1) | 5 - 4 | 2304.77 | -498.69 | 9.05877D+00 | 8.78239D-09 | 4.82607D-01 |
| R( 0) | 5 - 0 | 260.52 | -2543.41 | 2.87787D-07 | 8.95942D-18 | 1.29351D-05 |
| P( 2) | 5 - 0 | 262.01 | -2541.93 | 5.67707D-07 | 3.45496D-17 | 1.28576D-05 |
| R( 0) | 5 - 1 | 778.15 | -2025.78 | 4.04519D-05 | 2.18638D-15 | -2.15744D-04 |
| P( 2) | 5 - 1 | 779.63 | -2024.31 | 7.98595D-05 | 7.67526D-15 | -2.14582D-04 |
| R( 0) | 5 - 2 | 1291.45 | -1512.48 | 2.47895D-03 | 2.89764D-13 | 2.61793D-03 |
| P( 2) | 5 - 2 | 1292.92 | -1511.02 | 4.89190D-03 | 1.15008D-12 | 2.60423D-03 |
| R( 0) | 5 - 3 | 1800.26 | -1003.67 | 2.07268D-01 | 4.04805D-11 | -4.42831D-02 |
| P( 2) | 5 - 3 | 1801.72 | -1002.22 | 4.11146D-01 | 1.61363D-10 | -4.41978D-02 |
| R( 0) | 5 - 4 | 2304.29 | -499.65 | 3.03262D+00 | 8.78497D-09 | 4.82252D-01 |
| P( 2) | 5 - 4 | 2305.73 | -498.20 | 6.02602D+00 | 3.51326D-08 | 4.82785D-01 |
| R( 0) | 5 - 5 | 2803.46 | -0.48 | 4.15334D-08 | 1.00000D+00 | 1.90056D+00 |
| R( 1) | 5 - 0 | 261.02 | -2543.88 | 3.46863D-07 | 3.59383D-17 | 1.29600D-05 |
| P( 3) | 5 - 0 | 263.49 | -2541.40 | 5.08495D-07 | 7.72745D-17 | 1.28309D-05 |
| R( 1) | 5 - 1 | 778.64 | -2026.25 | 4.87539D-05 | 8.43903D-15 | -2.16139D-04 |
| P( 3) | 5 - 1 | 781.10 | -2023.79 | 7.15645D-05 | 1.74465D-14 | -2.14202D-04 |
| R( 1) | 5 - 2 | 1291.94 | -1512.95 | 2.98803D-03 | 1.16104D-12 | 2.62255D-03 |
| P( 3) | 5 - 2 | 1294.38 | -1510.51 | 4.38306D-03 | 2.58261D-12 | 2.59972D-03 |
| R( 1) | 5 - 3 | 1800.75 | -1004.14 | 2.49403D-01 | 1.62167D-10 | -4.43124D-02 |
| P( 3) | 5 - 3 | 1803.17 | -1001.72 | 3.69019D-01 | 3.62574D-10 | -4.41702D-02 |
| R( 1) | 5 - 4 | 2304.77 | -500.12 | 3.64688D+00 | 3.51385D-08 | 4.82076D-01 |
| P( 3) | 5 - 4 | 2307.18 | -497.71 | 5.41149D+00 | 7.90502D-08 | 4.82964D-01 |
| R( 1) | 5 - 5 | 2803.93 | -0.96 | 3.98729D-07 | 1.00000D+00 | 1.90058D+00 |
| R( 2) | 5 - 0 | 262.01 | -2544.32 | 3.73240D-07 | 7.93275D-17 | 1.29844D-05 |
| P( 4) | 5 - 0 | 265.47 | -2540.86 | 4.81921D-07 | 1.39084D-16 | 1.28037D-05 |
| R( 2) | 5 - 1 | 779.63 | -2026.70 | 5.24647D-05 | 1.86669D-14 | -2.16539D-04 |
| P( 4) | 5 - 1 | 783.07 | -2023.26 | 6.78644D-05 | 3.12973D-14 | -2.13826D-04 |

| | | | | | | | |
|---|---|---|---|---|---|---|---|
| R( 2) | 5 - 2 | 1292.92 | -1513.41 | 3.21576D-03 | 2.61223D-12 | 2.62720D-03 |
| P( 4) | 5 - 2 | 1296.34 | -1509.99 | 4.15569D-03 | 4.58920D-12 | 2.59524D-03 |
| R( 2) | 5 - 3 | 1801.72 | -1004.61 | 2.67949D-01 | 3.65200D-10 | -4.43421D-02 |
| P( 4) | 5 - 3 | 1805.12 | -1001.21 | 3.50485D-01 | 6.43980D-10 | -4.41430D-02 |
| R( 2) | 5 - 4 | 2305.73 | -500.60 | 3.91561D+00 | 7.90528D-08 | 4.81899D-01 |
| P( 4) | 5 - 4 | 2309.11 | -497.22 | 5.14237D+00 | 1.40549D-07 | 4.83143D-01 |
| R( 2) | 5 - 5 | 2804.89 | -1.44 | 1.44183D-06 | 1.00000D+00 | 1.90063D+00 |
| R( 3) | 5 - 0 | 263.49 | -2544.76 | 3.88691D-07 | 1.41307D-16 | 1.30084D-05 |
| P( 5) | 5 - 0 | 267.94 | -2540.30 | 4.66203D-07 | 2.16908D-16 | 1.27760D-05 |
| R( 3) | 5 - 1 | 781.10 | -2027.15 | 5.46462D-05 | 3.30363D-14 | -2.16941D-04 |
| P( 5) | 5 - 1 | 785.53 | -2022.72 | 6.56970D-05 | 4.90069D-14 | -2.13454D-04 |
| R( 3) | 5 - 2 | 1294.38 | -1513.86 | 3.34973D-03 | 4.65198D-12 | 2.63188D-03 |
| P( 5) | 5 - 2 | 1298.78 | -1509.47 | 4.02219D-03 | 7.15905D-12 | 2.59078D-03 |
| R( 3) | 5 - 3 | 1803.17 | -1005.07 | 2.78634D-01 | 6.50087D-10 | -4.43722D-02 |
| P( 5) | 5 - 3 | 1807.54 | -1000.70 | 3.39816D-01 | 1.00502D-09 | -4.41163D-02 |
| R( 3) | 5 - 4 | 2307.18 | -501.07 | 4.06911D+00 | 1.40539D-07 | 4.81723D-01 |
| P( 5) | 5 - 4 | 2311.52 | -496.73 | 4.98834D+00 | 2.19619D-07 | 4.83323D-01 |
| R( 3) | 5 - 5 | 2806.33 | -1.92 | 3.54437D-06 | 1.00000D+00 | 1.90070D+00 |
| R( 4) | 5 - 0 | 265.47 | -2545.17 | 3.99157D-07 | 2.21236D-16 | 1.30319D-05 |
| P( 6) | 5 - 0 | 270.91 | -2539.73 | 4.55401D-07 | 3.11759D-16 | 1.27478D-05 |
| R( 4) | 5 - 1 | 783.07 | -2027.57 | 5.61335D-05 | 5.15199D-14 | -2.17348D-04 |
| P( 6) | 5 - 1 | 788.47 | -2022.17 | 6.42271D-05 | 7.06290D-14 | -2.13085D-04 |
| R( 4) | 5 - 2 | 1296.34 | -1514.30 | 3.44114D-03 | 7.28141D-12 | 2.63658D-03 |
| P( 6) | 5 - 2 | 1301.71 | -1508.93 | 3.93138D-03 | 1.02925D-11 | 2.58636D-03 |
| R( 4) | 5 - 3 | 1805.12 | -1005.53 | 2.85746D-01 | 1.01707D-09 | -4.44028D-02 |
| P( 6) | 5 - 3 | 1810.45 | -1000.19 | 3.32724D-01 | 1.44554D-09 | -4.40899D-02 |
| R( 4) | 5 - 4 | 2309.11 | -501.53 | 4.17020D+00 | 2.19594D-07 | 4.81548D-01 |
| P( 6) | 5 - 4 | 2314.41 | -496.23 | 4.88659D+00 | 3.16268D-07 | 4.83503D-01 |
| R( 4) | 5 - 5 | 2808.25 | -2.40 | 7.08019D-06 | 1.00000D+00 | 1.90078D+00 |

| | | | | | | | |
|---|---|---|---|---|---|---|---|
| R( 5) | 5 - 0 | 267.94 | -2545.57 | 4.06923D-07 | 3.19225D-16 | 1.30549D-05 |
| P( 7) | 5 - 0 | 274.37 | -2539.14 | 4.47233D-07 | 4.23544D-16 | 1.27191D-05 |
| R( 5) | 5 - 1 | 785.53 | -2027.99 | 5.72480D-05 | 7.41425D-14 | -2.17759D-04 |
| P( 7) | 5 - 1 | 791.92 | -2021.60 | 6.31337D-05 | 9.61438D-14 | -2.12720D-04 |
| R( 5) | 5 - 2 | 1298.78 | -1514.74 | 3.50964D-03 | 1.05037D-11 | 2.64132D-03 |
| P( 7) | 5 - 2 | 1305.13 | -1508.39 | 3.86359D-03 | 1.39870D-11 | 2.58195D-03 |
| R( 5) | 5 - 3 | 1807.54 | -1005.97 | 2.90936D-01 | 1.46647D-09 | -4.44338D-02 |
| P( 7) | 5 - 3 | 1813.85 | -999.67 | 3.27559D-01 | 1.96526D-09 | -4.40640D-02 |
| R( 5) | 5 - 4 | 2311.52 | -502.00 | 4.24303D+00 | 3.16222D-07 | 4.81373D-01 |
| P( 7) | 5 - 4 | 2317.79 | -495.73 | 4.81297D+00 | 4.30502D-07 | 4.83683D-01 |
| R( 5) | 5 - 5 | 2810.64 | -2.87 | 1.24234D-05 | 9.99999D-01 | 1.90088D+00 |
| R( 6) | 5 - 0 | 270.91 | -2545.96 | 4.13054D-07 | 4.35388D-16 | 1.30774D-05 |
| P( 8) | 5 - 0 | 278.33 | -2538.54 | 4.40631D-07 | 5.52171D-16 | 1.26900D-05 |
| R( 6) | 5 - 1 | 788.47 | -2028.40 | 5.81393D-05 | 1.00929D-13 | -2.18173D-04 |
| P( 8) | 5 - 1 | 795.85 | -2021.02 | 6.22668D-05 | 1.25531D-13 | -2.12359D-04 |
| R( 6) | 5 - 2 | 1301.71 | -1515.16 | 3.56442D-03 | 1.43222D-11 | 2.64608D-03 |
| P( 8) | 5 - 2 | 1309.04 | -1507.83 | 3.80964D-03 | 1.82399D-11 | 2.57758D-03 |
| R( 6) | 5 - 3 | 1810.45 | -1006.42 | 2.94973D-01 | 1.99862D-09 | -4.44652D-02 |
| P( 8) | 5 - 3 | 1817.73 | -999.14 | 3.23551D-01 | 2.56395D-09 | -4.40385D-02 |
| R( 6) | 5 - 4 | 2314.41 | -502.46 | 4.29888D+00 | 4.30425D-07 | 4.81198D-01 |
| P( 8) | 5 - 4 | 2321.64 | -495.23 | 4.75619D+00 | 5.62326D-07 | 4.83864D-01 |
| R( 6) | 5 - 5 | 2813.52 | -3.35 | 1.99481D-05 | 9.99999D-01 | 1.90100D+00 |
| R( 7) | 5 - 0 | 274.37 | -2546.33 | 4.18114D-07 | 5.69840D-16 | 1.30995D-05 |
| P( 9) | 5 - 0 | 282.78 | -2537.92 | 4.35032D-07 | 6.97548D-16 | 1.26603D-05 |
| R( 7) | 5 - 1 | 791.92 | -2028.79 | 5.88870D-05 | 1.31906D-13 | -2.18592D-04 |
| P( 9) | 5 - 1 | 800.27 | -2020.43 | 6.15470D-05 | 1.58773D-13 | -2.12002D-04 |
| R( 7) | 5 - 2 | 1305.13 | -1515.57 | 3.61036D-03 | 1.87401D-11 | 2.65087D-03 |
| P( 9) | 5 - 2 | 1313.43 | -1507.27 | 3.76466D-03 | 2.30487D-11 | 2.57323D-03 |
| R( 7) | 5 - 3 | 1813.85 | -1006.85 | 2.98264D-01 | 2.61384D-09 | -4.44970D-02 |

| | | | | | | |
|---|---|---|---|---|---|---|
| P( 9) | 5 - 3 | 1822.10 | -998.60 | 3.20291D-01 | 3.24134D-09 | -4.40134D-02 |
| R( 7) | 5 - 4 | 2317.79 | -502.92 | 4.34372D+00 | 5.62207D-07 | 4.81024D-01 |
| P( 9) | 5 - 4 | 2325.98 | -494.72 | 4.71029D+00 | 7.11745D-07 | 4.84046D-01 |
| R( 7) | 5 - 5 | 2816.87 | -3.83 | 3.00288D-05 | 9.99999D-01 | 1.90114D+00 |
| R( 8) | 5 - 0 | 278.33 | -2546.68 | 4.22429D-07 | 7.22697D-16 | 1.31211D-05 |
| P( 10) | 5 - 0 | 287.73 | -2537.29 | 4.30109D-07 | 8.59585D-16 | 1.26302D-05 |
| R( 8) | 5 - 1 | 795.85 | -2029.17 | 5.95369D-05 | 1.67099D-13 | -2.19014D-04 |
| P( 10) | 5 - 1 | 805.19 | -2019.83 | 6.09283D-05 | 1.95849D-13 | -2.11648D-04 |
| R( 8) | 5 - 2 | 1309.04 | -1515.98 | 3.65025D-03 | 2.37608D-11 | 2.65569D-03 |
| P( 10) | 5 - 2 | 1318.32 | -1506.70 | 3.72583D-03 | 2.84111D-11 | 2.56891D-03 |
| R( 8) | 5 - 3 | 1817.73 | -1007.28 | 3.01047D-01 | 3.31249D-09 | -4.45292D-02 |
| P( 10) | 5 - 3 | 1826.95 | -998.06 | 3.17545D-01 | 3.99718D-09 | -4.39888D-02 |
| R( 8) | 5 - 4 | 2321.64 | -503.37 | 4.38100D+00 | 7.11573D-07 | 4.80850D-01 |
| P( 10) | 5 - 4 | 2330.80 | -494.21 | 4.67182D+00 | 8.78767D-07 | 4.84228D-01 |
| R( 8) | 5 - 5 | 2820.70 | -4.31 | 4.30402D-05 | 9.99998D-01 | 1.90130D+00 |
| R( 9) | 5 - 0 | 282.78 | -2547.02 | 4.26202D-07 | 8.94078D-16 | 1.31422D-05 |
| P( 11) | 5 - 0 | 293.17 | -2536.64 | 4.25660D-07 | 1.03820D-15 | 1.25996D-05 |
| R( 9) | 5 - 1 | 800.27 | -2029.53 | 6.01175D-05 | 2.06536D-13 | -2.19440D-04 |
| P( 11) | 5 - 1 | 810.59 | -2019.21 | 6.03823D-05 | 2.36742D-13 | -2.11298D-04 |
| R( 9) | 5 - 2 | 1313.43 | -1516.37 | 3.68585D-03 | 2.93879D-11 | 2.66053D-03 |
| P( 11) | 5 - 2 | 1323.69 | -1506.12 | 3.69141D-03 | 3.43246D-11 | 2.56461D-03 |
| R( 9) | 5 - 3 | 1822.10 | -1007.70 | 3.03466D-01 | 4.09490D-09 | -4.45619D-02 |
| P( 11) | 5 - 3 | 1832.29 | -997.52 | 3.15166D-01 | 4.83125D-09 | -4.39645D-02 |
| R( 9) | 5 - 4 | 2325.98 | -503.82 | 4.41286D+00 | 8.78528D-07 | 4.80677D-01 |
| P( 11) | 5 - 4 | 2336.11 | -493.70 | 4.63863D+00 | 1.06340D-06 | 4.84411D-01 |
| R( 9) | 5 - 5 | 2825.01 | -4.79 | 5.93570D-05 | 9.99998D-01 | 1.90148D+00 |
| R( 10) | 5 - 0 | 287.73 | -2547.35 | 4.29563D-07 | 1.08410D-15 | 1.31628D-05 |
| P( 12) | 5 - 0 | 299.10 | -2535.97 | 4.21552D-07 | 1.23329D-15 | 1.25684D-05 |
| R( 10) | 5 - 1 | 805.19 | -2029.89 | 6.06473D-05 | 2.50242D-13 | -2.19869D-04 |

| | | | | | | |
|---|---|---|---|---|---|---|
| P( 12) | 5 - 1 | 816.49 | -2018.58 | 5.98905D-05 | 2.81434D-13 | -2.10951D-04 |
| R( 10) | 5 - 2 | 1318.32 | -1516.76 | 3.71829D-03 | 3.56247D-11 | 2.66541D-03 |
| P( 12) | 5 - 2 | 1329.55 | -1505.52 | 3.66028D-03 | 4.07870D-11 | 2.56034D-03 |
| R( 10) | 5 - 3 | 1826.95 | -1008.12 | 3.05617D-01 | 4.96143D-09 | -4.45950D-02 |
| P( 12) | 5 - 3 | 1838.11 | -996.96 | 3.13060D-01 | 5.74331D-09 | -4.39407D-02 |
| R( 10) | 5 - 4 | 2330.80 | -504.27 | 4.44070D+00 | 1.06308D-06 | 4.80504D-01 |
| P( 12) | 5 - 4 | 2341.89 | -493.18 | 4.60934D+00 | 1.26565D-06 | 4.84594D-01 |
| R( 10) | 5 - 5 | 2829.80 | -5.27 | 7.93545D-05 | 9.99998D-01 | 1.90167D+00 |
| R( 11) | 5 - 0 | 293.17 | -2547.65 | 4.32602D-07 | 1.29289D-15 | 1.31829D-05 |
| P( 13) | 5 - 0 | 305.53 | -2535.29 | 4.17697D-07 | 1.44479D-15 | 1.25368D-05 |
| R( 11) | 5 - 1 | 810.59 | -2030.23 | 6.11389D-05 | 2.98247D-13 | -2.20303D-04 |
| P( 13) | 5 - 1 | 822.88 | -2017.94 | 5.94400D-05 | 3.29906D-13 | -2.10608D-04 |
| R( 11) | 5 - 2 | 1323.69 | -1517.13 | 3.74834D-03 | 4.24749D-11 | 2.67031D-03 |
| P( 13) | 5 - 2 | 1335.90 | -1504.92 | 3.63164D-03 | 4.77958D-11 | 2.55609D-03 |
| R( 11) | 5 - 3 | 1832.29 | -1008.53 | 3.07565D-01 | 5.91244D-09 | -4.46284D-02 |
| P( 13) | 5 - 3 | 1844.42 | -996.40 | 3.11160D-01 | 6.73312D-09 | -4.39173D-02 |
| R( 11) | 5 - 4 | 2336.11 | -504.72 | 4.46547D+00 | 1.26523D-06 | 4.80331D-01 |
| P( 13) | 5 - 4 | 2348.16 | -492.67 | 4.58299D+00 | 1.48553D-06 | 4.84777D-01 |
| R( 11) | 5 - 5 | 2835.07 | -5.75 | 1.03408D-04 | 9.99997D-01 | 1.90189D+00 |
| R( 12) | 5 - 0 | 299.10 | -2547.95 | 4.35380D-07 | 1.52057D-15 | 1.32026D-05 |
| P( 14) | 5 - 0 | 312.46 | -2534.59 | 4.14031D-07 | 1.67261D-15 | 1.25046D-05 |
| R( 12) | 5 - 1 | 816.49 | -2030.56 | 6.16012D-05 | 3.50579D-13 | -2.20740D-04 |
| P( 14) | 5 - 1 | 829.76 | -2017.29 | 5.90222D-05 | 3.82143D-13 | -2.10268D-04 |
| R( 12) | 5 - 2 | 1329.55 | -1517.50 | 3.77655D-03 | 4.99422D-11 | 2.67525D-03 |
| P( 14) | 5 - 2 | 1342.73 | -1504.31 | 3.60496D-03 | 5.53490D-11 | 2.55187D-03 |
| R( 12) | 5 - 3 | 1838.11 | -1008.94 | 3.09356D-01 | 6.94829D-09 | -4.46624D-02 |
| P( 14) | 5 - 3 | 1851.21 | -995.84 | 3.09422D-01 | 7.80047D-09 | -4.38944D-02 |
| R( 12) | 5 - 4 | 2341.89 | -505.16 | 4.48782D+00 | 1.48499D-06 | 4.80159D-01 |
| P( 14) | 5 - 4 | 2354.90 | -492.15 | 4.55892D+00 | 1.72304D-06 | 4.84962D-01 |

| | | | | | | | |
|---|---|---|---|---|---|---|---|
| R( 12) | 5 - 5 | 2840.82 | -6.23 | 1.31894D-04 | 9.99997D-01 | 1.90212D+00 |
| R( 13) | 5 - 0 | 305.53 | -2548.22 | 4.37945D-07 | 1.76727D-15 | 1.32217D-05 |
| P( 15) | 5 - 0 | 319.87 | -2533.88 | 4.10508D-07 | 1.91667D-15 | 1.24719D-05 |
| R( 13) | 5 - 1 | 822.88 | -2030.87 | 6.20405D-05 | 4.07265D-13 | -2.21181D-04 |
| P( 15) | 5 - 1 | 837.13 | -2016.62 | 5.86304D-05 | 4.38127D-13 | -2.09931D-04 |
| R( 13) | 5 - 2 | 1335.90 | -1517.86 | 3.80331D-03 | 5.80302D-11 | 2.68021D-03 |
| P( 15) | 5 - 2 | 1350.06 | -1503.70 | 3.57985D-03 | 6.34443D-11 | 2.54768D-03 |
| R( 13) | 5 - 3 | 1844.42 | -1009.34 | 3.11021D-01 | 8.06936D-09 | -4.46967D-02 |
| P( 15) | 5 - 3 | 1858.49 | -995.27 | 3.07812D-01 | 8.94514D-09 | -4.38718D-02 |
| R( 13) | 5 - 4 | 2348.16 | -505.60 | 4.50824D+00 | 1.72237D-06 | 4.79987D-01 |
| P( 15) | 5 - 4 | 2362.13 | -491.62 | 4.53664D+00 | 1.97820D-06 | 4.85146D-01 |
| R( 13) | 5 - 5 | 2847.05 | -6.71 | 1.65187D-04 | 9.99996D-01 | 1.90237D+00 |
| R( 14) | 5 - 0 | 312.46 | -2548.48 | 4.40327D-07 | 2.03311D-15 | 1.32404D-05 |
| P( 16) | 5 - 0 | 327.79 | -2533.15 | 4.07095D-07 | 2.17687D-15 | 1.24387D-05 |
| R( 14) | 5 - 1 | 829.76 | -2031.18 | 6.24617D-05 | 4.68336D-13 | -2.21625D-04 |
| P( 16) | 5 - 1 | 844.99 | -2015.94 | 5.82599D-05 | 4.97842D-13 | -2.09598D-04 |
| R( 14) | 5 - 2 | 1342.73 | -1518.20 | 3.82891D-03 | 6.67427D-11 | 2.68520D-03 |
| P( 16) | 5 - 2 | 1357.87 | -1503.07 | 3.55601D-03 | 7.20796D-11 | 2.54351D-03 |
| R( 14) | 5 - 3 | 1851.21 | -1009.73 | 3.12587D-01 | 9.27601D-09 | -4.47315D-02 |
| P( 16) | 5 - 3 | 1866.25 | -994.69 | 3.06307D-01 | 1.01669D-08 | -4.38497D-02 |
| R( 14) | 5 - 4 | 2354.90 | -506.03 | 4.52710D+00 | 1.97737D-06 | 4.79815D-01 |
| P( 16) | 5 - 4 | 2369.84 | -491.10 | 4.51580D+00 | 2.25102D-06 | 4.85332D-01 |
| R( 14) | 5 - 5 | 2853.75 | -7.18 | 2.03665D-04 | 9.99996D-01 | 1.90264D+00 |
| R( 15) | 5 - 0 | 319.87 | -2548.73 | 4.42554D-07 | 2.31822D-15 | 1.32585D-05 |
| P( 17) | 5 - 0 | 336.19 | -2532.41 | 4.03765D-07 | 2.45315D-15 | 1.24049D-05 |
| R( 15) | 5 - 1 | 837.13 | -2031.47 | 6.28683D-05 | 5.33821D-13 | -2.22073D-04 |
| P( 17) | 5 - 1 | 853.35 | -2015.25 | 5.79071D-05 | 5.61271D-13 | -2.09268D-04 |
| R( 15) | 5 - 2 | 1350.06 | -1518.54 | 3.85357D-03 | 7.60835D-11 | 2.69022D-03 |
| P( 17) | 5 - 2 | 1366.17 | -1502.43 | 3.53322D-03 | 8.12529D-11 | 2.53937D-03 |

| | | | | | | | |
|---|---|---|---|---|---|---|---|
| R( 15) | 5 - 3 | 1858.49 | -1010.11 | 3.14071D-01 | 1.05686D-08 | -4.47666D-02 |
| P( 17) | 5 - 3 | 1874.49 | -994.11 | 3.04887D-01 | 1.14656D-08 | -4.38280D-02 |
| R( 15) | 5 - 4 | 2362.13 | -506.47 | 4.54466D+00 | 2.25001D-06 | 4.79644D-01 |
| P( 17) | 5 - 4 | 2378.03 | -490.57 | 4.49612D+00 | 2.54151D-06 | 4.85518D-01 |
| R( 15) | 5 - 5 | 2860.94 | -7.66 | 2.47705D-04 | 9.99995D-01 | 1.90293D+00 |
| R( 16) | 5 - 0 | 327.79 | -2548.96 | 4.44643D-07 | 2.62273D-15 | 1.32761D-05 |
| P( 18) | 5 - 0 | 345.09 | -2531.65 | 4.00499D-07 | 2.74543D-15 | 1.23706D-05 |
| R( 16) | 5 - 1 | 844.99 | -2031.75 | 6.32631D-05 | 6.03751D-13 | -2.22525D-04 |
| P( 18) | 5 - 1 | 862.19 | -2014.55 | 5.75691D-05 | 6.28399D-13 | -2.08941D-04 |
| R( 16) | 5 - 2 | 1357.87 | -1518.87 | 3.87747D-03 | 8.60565D-11 | 2.69527D-03 |
| P( 18) | 5 - 2 | 1374.96 | -1501.78 | 3.51131D-03 | 9.09589D-11 | 2.53525D-03 |
| R( 16) | 5 - 3 | 1866.25 | -1010.49 | 3.15488D-01 | 1.19476D-08 | -4.48022D-02 |
| P( 18) | 5 - 3 | 1883.22 | -993.52 | 3.03538D-01 | 1.28410D-08 | -4.38067D-02 |
| R( 16) | 5 - 4 | 2369.84 | -506.90 | 4.56114D+00 | 2.54029D-06 | 4.79473D-01 |
| P( 18) | 5 - 4 | 2386.71 | -490.03 | 4.47740D+00 | 2.84968D-06 | 4.85704D-01 |
| R( 16) | 5 - 5 | 2868.60 | -8.14 | 2.97683D-04 | 9.99994D-01 | 1.90323D+00 |
| R( 17) | 5 - 0 | 336.19 | -2549.17 | 4.46609D-07 | 2.94677D-15 | 1.32932D-05 |
| P( 19) | 5 - 0 | 354.48 | -2530.88 | 3.97282D-07 | 3.05362D-15 | 1.23358D-05 |
| R( 17) | 5 - 1 | 853.35 | -2032.01 | 6.36482D-05 | 6.78156D-13 | -2.22980D-04 |
| P( 19) | 5 - 1 | 871.53 | -2013.83 | 5.72436D-05 | 6.99156D-13 | -2.08618D-04 |
| R( 17) | 5 - 2 | 1366.17 | -1519.19 | 3.90074D-03 | 9.66658D-11 | 2.70034D-03 |
| P( 19) | 5 - 2 | 1384.23 | -1501.13 | 3.49014D-03 | 1.01202D-10 | 2.53115D-03 |
| R( 17) | 5 - 3 | 1874.49 | -1010.87 | 3.16848D-01 | 1.34134D-08 | -4.48382D-02 |
| P( 19) | 5 - 3 | 1892.44 | -992.92 | 3.02249D-01 | 1.42928D-08 | -4.37858D-02 |
| R( 17) | 5 - 4 | 2378.03 | -507.33 | 4.57668D+00 | 2.84823D-06 | 4.79302D-01 |
| P( 19) | 5 - 4 | 2395.86 | -489.50 | 4.45947D+00 | 3.17555D-06 | 4.85891D-01 |
| R( 17) | 5 - 5 | 2876.74 | -8.62 | 3.53979D-04 | 9.99994D-01 | 1.90356D+00 |
| R( 18) | 5 - 0 | 345.09 | -2549.37 | 4.48465D-07 | 3.29049D-15 | 1.33098D-05 |
| P( 20) | 5 - 0 | 364.37 | -2530.09 | 3.94100D-07 | 3.37765D-15 | 1.23003D-05 |

| | | | | | | |
|---|---|---|---|---|---|---|
| R( 18) | 5 - 1 | 862.19 | -2032.27 | 6.40254D-05 | 7.57068D-13 | -2.23439D-04 |
| P( 20) | 5 - 1 | 881.35 | -2013.11 | 5.69290D-05 | 7.73634D-13 | -2.08297D-04 |
| R( 18) | 5 - 2 | 1374.96 | -1519.50 | 3.92348D-03 | 1.07919D-10 | 2.70545D-03 |
| P( 20) | 5 - 2 | 1394.00 | -1500.46 | 3.46962D-03 | 1.11977D-10 | 2.52708D-03 |
| R( 18) | 5 - 3 | 1883.22 | -1011.23 | 3.18162D-01 | 1.49663D-08 | -4.48747D-02 |
| P( 20) | 5 - 3 | 1902.14 | -992.32 | 3.01011D-01 | 1.58210D-08 | -4.37653D-02 |
| R( 18) | 5 - 4 | 2386.71 | -507.75 | 4.59144D+00 | 3.17384D-06 | 4.79132D-01 |
| P( 20) | 5 - 4 | 2405.50 | -488.96 | 4.44220D+00 | 3.51912D-06 | 4.86079D-01 |
| R( 18) | 5 - 5 | 2885.36 | -9.10 | 4.16969D-04 | 9.99993D-01 | 1.90390D+00 |
| R( 19) | 5 - 0 | 354.48 | -2549.55 | 4.50220D-07 | 3.65400D-15 | 1.33258D-05 |
| P( 21) | 5 - 0 | 374.75 | -2529.28 | 3.90945D-07 | 3.71744D-15 | 1.22643D-05 |
| R( 19) | 5 - 1 | 871.53 | -2032.51 | 6.43959D-05 | 8.40580D-13 | -2.23901D-04 |
| P( 21) | 5 - 1 | 891.67 | -2012.37 | 5.66238D-05 | 8.51766D-13 | -2.07979D-04 |
| R( 19) | 5 - 2 | 1384.23 | -1519.80 | 3.94578D-03 | 1.19813D-10 | 2.71058D-03 |
| P( 21) | 5 - 2 | 1404.25 | -1499.79 | 3.44964D-03 | 1.23282D-10 | 2.52304D-03 |
| R( 19) | 5 - 3 | 1892.44 | -1011.59 | 3.19435D-01 | 1.66068D-08 | -4.49115D-02 |
| P( 21) | 5 - 3 | 1912.32 | -991.71 | 2.99817D-01 | 1.74253D-08 | -4.37453D-02 |
| R( 19) | 5 - 4 | 2395.86 | -508.17 | 4.60550D+00 | 3.51713D-06 | 4.78962D-01 |
| P( 21) | 5 - 4 | 2415.61 | -488.42 | 4.42549D+00 | 3.88042D-06 | 4.86267D-01 |
| R( 19) | 5 - 5 | 2894.46 | -9.58 | 4.87034D-04 | 9.99992D-01 | 1.90426D+00 |
| Q( 0) | 0 - 0 | 260.52 | 0.00 | 0.00000D+00 | 1.00000D+00 | -1.69083D+00 |
| Q( 1) | 0 - 0 | 261.02 | -0.00 | 0.00000D+00 | 1.00000D+00 | -1.69085D+00 |
| Q( 2) | 0 - 0 | 262.01 | -0.00 | 0.00000D+00 | 1.00000D+00 | -1.69089D+00 |
| Q( 3) | 0 - 0 | 263.49 | 0.00 | 0.00000D+00 | 1.00000D+00 | -1.69094D+00 |
| Q( 4) | 0 - 0 | 265.47 | 0.00 | 0.00000D+00 | 1.00000D+00 | -1.69101D+00 |
| Q( 5) | 0 - 0 | 267.94 | 0.00 | 0.00000D+00 | 1.00000D+00 | -1.69111D+00 |
| Q( 6) | 0 - 0 | 270.91 | 0.00 | 0.00000D+00 | 1.00000D+00 | -1.69122D+00 |
| Q( 7) | 0 - 0 | 274.37 | 0.00 | 0.00000D+00 | 1.00000D+00 | -1.69134D+00 |
| Q( 8) | 0 - 0 | 278.33 | 0.00 | 0.00000D+00 | 1.00000D+00 | -1.69149D+00 |

| | | | | | | |
|---|---|---|---|---|---|---|
| Q( 9) | 0 - 0 | 282.78 | 0.00 | 0.00000D+00 | 1.00000D+00 | -1.69165D+00 |
| Q( 10) | 0 - 0 | 287.73 | 0.00 | 0.00000D+00 | 1.00000D+00 | -1.69184D+00 |
| Q( 11) | 0 - 0 | 293.17 | 0.00 | 0.00000D+00 | 1.00000D+00 | -1.69204D+00 |
| Q( 12) | 0 - 0 | 299.10 | 0.00 | 0.00000D+00 | 1.00000D+00 | -1.69226D+00 |
| Q( 13) | 0 - 0 | 305.53 | 0.00 | 0.00000D+00 | 1.00000D+00 | -1.69249D+00 |
| Q( 14) | 0 - 0 | 312.46 | 0.00 | 0.00000D+00 | 1.00000D+00 | -1.69275D+00 |
| Q( 15) | 0 - 0 | 319.87 | 0.00 | 0.00000D+00 | 1.00000D+00 | -1.69302D+00 |
| Q( 16) | 0 - 0 | 327.79 | 0.00 | 0.00000D+00 | 1.00000D+00 | -1.69332D+00 |
| Q( 17) | 0 - 0 | 336.19 | 0.00 | 0.00000D+00 | 1.00000D+00 | -1.69363D+00 |
| Q( 18) | 0 - 0 | 345.09 | 0.00 | 0.00000D+00 | 1.00000D+00 | -1.69396D+00 |
| Q( 19) | 0 - 0 | 354.48 | 0.00 | 0.00000D+00 | 1.00000D+00 | -1.69430D+00 |
| Q( 20) | 0 - 0 | 364.37 | 0.00 | 0.00000D+00 | 1.00000D+00 | -1.69467D+00 |
| Q( 0) | 1 - 0 | 260.52 | -517.63 | 0.00000D+00 | 8.18520D-18 | 2.19256D-01 |
| Q( 0) | 1 - 1 | 778.15 | 0.00 | 0.00000D+00 | 1.00000D+00 | 1.73305D+00 |
| Q( 1) | 1 - 0 | 261.02 | -517.63 | 0.00000D+00 | 1.33508D-17 | 2.19256D-01 |
| Q( 1) | 1 - 1 | 778.64 | -0.00 | 0.00000D+00 | 1.00000D+00 | 1.73307D+00 |
| Q( 2) | 1 - 0 | 262.01 | -517.62 | 0.00000D+00 | 4.65936D-17 | 2.19257D-01 |
| Q( 2) | 1 - 1 | 779.63 | -0.00 | 0.00000D+00 | 1.00000D+00 | 1.73311D+00 |
| Q( 3) | 1 - 0 | 263.49 | -517.61 | 0.00000D+00 | 1.40274D-23 | 2.19258D-01 |
| Q( 3) | 1 - 1 | 781.10 | 0.00 | 0.00000D+00 | 1.00000D+00 | 1.73316D+00 |
| Q( 4) | 1 - 0 | 265.47 | -517.60 | 0.00000D+00 | 1.40068D-23 | 2.19259D-01 |
| Q( 4) | 1 - 1 | 783.07 | 0.00 | 0.00000D+00 | 1.00000D+00 | 1.73324D+00 |
| Q( 5) | 1 - 0 | 267.94 | -517.58 | 0.00000D+00 | 1.40297D-23 | 2.19261D-01 |
| Q( 5) | 1 - 1 | 785.53 | 0.00 | 0.00000D+00 | 1.00000D+00 | 1.73333D+00 |
| Q( 6) | 1 - 0 | 270.91 | -517.56 | 0.00000D+00 | 1.40592D-23 | 2.19263D-01 |
| Q( 6) | 1 - 1 | 788.47 | 0.00 | 0.00000D+00 | 1.00000D+00 | 1.73344D+00 |
| Q( 7) | 1 - 0 | 274.37 | -517.54 | 0.00000D+00 | 1.41106D-23 | 2.19266D-01 |
| Q( 7) | 1 - 1 | 791.92 | 0.00 | 0.00000D+00 | 1.00000D+00 | 1.73357D+00 |
| Q( 8) | 1 - 0 | 278.33 | -517.52 | 0.00000D+00 | 1.42393D-23 | 2.19268D-01 |

| | | | | | | | |
|---|---|---|---|---|---|---|---|
| Q( 8) | 1 - 1 | 795.85 | 0.00 | 0.00000D+00 | 1.00000D+00 | 1.73371D+00 |
| Q( 9) | 1 - 0 | 282.78 | -517.49 | 0.00000D+00 | 1.41416D-23 | 2.19271D-01 |
| Q( 9) | 1 - 1 | 800.27 | 0.00 | 0.00000D+00 | 1.00000D+00 | 1.73388D+00 |
| Q( 10) | 1 - 0 | 287.73 | -517.46 | 0.00000D+00 | 1.43110D-23 | 2.19275D-01 |
| Q( 10) | 1 - 1 | 805.19 | 0.00 | 0.00000D+00 | 1.00000D+00 | 1.73406D+00 |
| Q( 11) | 1 - 0 | 293.17 | -517.43 | 0.00000D+00 | 1.45963D-23 | 2.19279D-01 |
| Q( 11) | 1 - 1 | 810.59 | 0.00 | 0.00000D+00 | 1.00000D+00 | 1.73426D+00 |
| Q( 12) | 1 - 0 | 299.10 | -517.39 | 0.00000D+00 | 1.47774D-23 | 2.19283D-01 |
| Q( 12) | 1 - 1 | 816.49 | 0.00 | 0.00000D+00 | 1.00000D+00 | 1.73448D+00 |
| Q( 13) | 1 - 0 | 305.53 | -517.35 | 0.00000D+00 | 1.54532D-23 | 2.19287D-01 |
| Q( 13) | 1 - 1 | 822.88 | 0.00 | 0.00000D+00 | 1.00000D+00 | 1.73472D+00 |
| Q( 14) | 1 - 0 | 312.46 | -517.30 | 0.00000D+00 | 1.57771D-23 | 2.19292D-01 |
| Q( 14) | 1 - 1 | 829.76 | 0.00 | 0.00000D+00 | 1.00000D+00 | 1.73498D+00 |
| Q( 15) | 1 - 0 | 319.87 | -517.26 | 0.00000D+00 | 1.64493D-23 | 2.19297D-01 |
| Q( 15) | 1 - 1 | 837.13 | 0.00 | 0.00000D+00 | 1.00000D+00 | 1.73525D+00 |
| Q( 16) | 1 - 0 | 327.79 | -517.21 | 0.00000D+00 | 1.69312D-23 | 2.19303D-01 |
| Q( 16) | 1 - 1 | 844.99 | 0.00 | 0.00000D+00 | 1.00000D+00 | 1.73554D+00 |
| Q( 17) | 1 - 0 | 336.19 | -517.16 | 0.00000D+00 | 1.77668D-23 | 2.19309D-01 |
| Q( 17) | 1 - 1 | 853.35 | 0.00 | 0.00000D+00 | 1.00000D+00 | 1.73585D+00 |
| Q( 18) | 1 - 0 | 345.09 | -517.10 | 0.00000D+00 | 2.12966D-23 | 2.19315D-01 |
| Q( 18) | 1 - 1 | 862.19 | 0.00 | 0.00000D+00 | 1.00000D+00 | 1.73618D+00 |
| Q( 19) | 1 - 0 | 354.48 | -517.04 | 0.00000D+00 | 2.26940D-23 | 2.19322D-01 |
| Q( 19) | 1 - 1 | 871.53 | 0.00 | 0.00000D+00 | 1.00000D+00 | 1.73653D+00 |
| Q( 20) | 1 - 0 | 364.37 | -516.98 | 0.00000D+00 | 2.41259D-23 | 2.19329D-01 |
| Q( 20) | 1 - 1 | 881.35 | 0.00 | 0.00000D+00 | 1.00000D+00 | 1.73690D+00 |
| Q( 0) | 2 - 0 | 260.52 | -1030.93 | 0.00000D+00 | 1.30225D-18 | 1.33892D-02 |
| Q( 0) | 2 - 1 | 778.15 | -513.30 | 0.00000D+00 | 2.33259D-16 | -3.08915D-01 |
| Q( 0) | 2 - 2 | 1291.45 | 0.00 | 0.00000D+00 | 1.00000D+00 | -1.77545D+00 |
| Q( 1) | 2 - 0 | 261.02 | -1030.93 | 0.00000D+00 | 1.75187D-18 | 1.33893D-02 |

| | | | | | | |
|---|---|---|---|---|---|---|
| Q( 1) | 2 - 1 | 778.64 | -513.30 | 0.00000D+00 | 2.63952D-16 | -3.08916D-01 |
| Q( 1) | 2 - 2 | 1291.94 | -0.00 | 0.00000D+00 | 1.00000D+00 | -1.77547D+00 |
| Q( 2) | 2 - 0 | 262.01 | -1030.91 | 0.00000D+00 | 2.54396D-25 | 1.33895D-02 |
| Q( 2) | 2 - 1 | 779.63 | -513.29 | 0.00000D+00 | 8.39762D-17 | -3.08917D-01 |
| Q( 2) | 2 - 2 | 1292.92 | 0.00 | 0.00000D+00 | 1.00000D+00 | -1.77550D+00 |
| Q( 3) | 2 - 0 | 263.49 | -1030.89 | 0.00000D+00 | 2.69915D-18 | 1.33899D-02 |
| Q( 3) | 2 - 1 | 781.10 | -513.28 | 0.00000D+00 | 3.22069D-16 | -3.08918D-01 |
| Q( 3) | 2 - 2 | 1294.38 | -0.00 | 0.00000D+00 | 1.00000D+00 | -1.77556D+00 |
| Q( 4) | 2 - 0 | 265.47 | -1030.87 | 0.00000D+00 | 2.43417D-25 | 1.33903D-02 |
| Q( 4) | 2 - 1 | 783.07 | -513.27 | 0.00000D+00 | 8.37565D-17 | -3.08920D-01 |
| Q( 4) | 2 - 2 | 1296.34 | 0.00 | 0.00000D+00 | 1.00000D+00 | -1.77563D+00 |
| Q( 5) | 2 - 0 | 267.94 | -1030.84 | 0.00000D+00 | 2.42658D-25 | 1.33909D-02 |
| Q( 5) | 2 - 1 | 785.53 | -513.26 | 0.00000D+00 | 8.36006D-17 | -3.08922D-01 |
| Q( 5) | 2 - 2 | 1298.78 | 0.00 | 0.00000D+00 | 1.00000D+00 | -1.77572D+00 |
| Q( 6) | 2 - 0 | 270.91 | -1030.80 | 0.00000D+00 | 2.39895D-25 | 1.33915D-02 |
| Q( 6) | 2 - 1 | 788.47 | -513.24 | 0.00000D+00 | 8.34141D-17 | -3.08925D-01 |
| Q( 6) | 2 - 2 | 1301.71 | 0.00 | 0.00000D+00 | 1.00000D+00 | -1.77583D+00 |
| Q( 7) | 2 - 0 | 274.37 | -1030.76 | 0.00000D+00 | 2.43292D-25 | 1.33923D-02 |
| Q( 7) | 2 - 1 | 791.92 | -513.21 | 0.00000D+00 | 8.31980D-17 | -3.08928D-01 |
| Q( 7) | 2 - 2 | 1305.13 | 0.00 | 0.00000D+00 | 1.00000D+00 | -1.77596D+00 |
| Q( 8) | 2 - 0 | 278.33 | -1030.71 | 0.00000D+00 | 2.36171D-25 | 1.33932D-02 |
| Q( 8) | 2 - 1 | 795.85 | -513.19 | 0.00000D+00 | 8.29512D-17 | -3.08932D-01 |
| Q( 8) | 2 - 2 | 1309.04 | 0.00 | 0.00000D+00 | 1.00000D+00 | -1.77611D+00 |
| Q( 9) | 2 - 0 | 282.78 | -1030.65 | 0.00000D+00 | 2.21229D-25 | 1.33942D-02 |
| Q( 9) | 2 - 1 | 800.27 | -513.16 | 0.00000D+00 | 8.26766D-17 | -3.08936D-01 |
| Q( 9) | 2 - 2 | 1313.43 | 0.00 | 0.00000D+00 | 1.00000D+00 | -1.77627D+00 |
| Q( 10) | 2 - 0 | 287.73 | -1030.59 | 0.00000D+00 | 2.14565D-25 | 1.33953D-02 |
| Q( 10) | 2 - 1 | 805.19 | -513.13 | 0.00000D+00 | 8.23730D-17 | -3.08941D-01 |
| Q( 10) | 2 - 2 | 1318.32 | 0.00 | 0.00000D+00 | 1.00000D+00 | -1.77646D+00 |

| | | | | | | |
|---|---|---|---|---|---|---|
| Q( 11) | 2 - 0 | 293.17 | -1030.52 | 0.00000D+00 | 2.10076D-25 | 1.33966D-02 |
| Q( 11) | 2 - 1 | 810.59 | -513.10 | 0.00000D+00 | 8.20420D-17 | -3.08946D-01 |
| Q( 11) | 2 - 2 | 1323.69 | 0.00 | 0.00000D+00 | 1.00000D+00 | -1.77666D+00 |
| Q( 12) | 2 - 0 | 299.10 | -1030.45 | 0.00000D+00 | 1.95698D-25 | 1.33979D-02 |
| Q( 12) | 2 - 1 | 816.49 | -513.06 | 0.00000D+00 | 8.16840D-17 | -3.08952D-01 |
| Q( 12) | 2 - 2 | 1329.55 | 0.00 | 0.00000D+00 | 1.00000D+00 | -1.77688D+00 |
| Q( 13) | 2 - 0 | 305.53 | -1030.37 | 0.00000D+00 | 2.33929D-25 | 1.33994D-02 |
| Q( 13) | 2 - 1 | 822.88 | -513.02 | 0.00000D+00 | 8.12996D-17 | -3.08958D-01 |
| Q( 13) | 2 - 2 | 1335.90 | 0.00 | 0.00000D+00 | 1.00000D+00 | -1.77712D+00 |
| Q( 14) | 2 - 0 | 312.46 | -1030.28 | 0.00000D+00 | 2.12195D-25 | 1.34009D-02 |
| Q( 14) | 2 - 1 | 829.76 | -512.97 | 0.00000D+00 | 8.08896D-17 | -3.08964D-01 |
| Q( 14) | 2 - 2 | 1342.73 | 0.00 | 0.00000D+00 | 1.00000D+00 | -1.77738D+00 |
| Q( 15) | 2 - 0 | 319.87 | -1030.18 | 0.00000D+00 | 1.99817D-25 | 1.34026D-02 |
| Q( 15) | 2 - 1 | 837.13 | -512.93 | 0.00000D+00 | 8.04562D-17 | -3.08971D-01 |
| Q( 15) | 2 - 2 | 1350.06 | 0.00 | 0.00000D+00 | 1.00000D+00 | -1.77765D+00 |
| Q( 16) | 2 - 0 | 327.79 | -1030.09 | 0.00000D+00 | 1.78520D-25 | 1.34044D-02 |
| Q( 16) | 2 - 1 | 844.99 | -512.88 | 0.00000D+00 | 7.99985D-17 | -3.08979D-01 |
| Q( 16) | 2 - 2 | 1357.87 | 0.00 | 0.00000D+00 | 1.00000D+00 | -1.77794D+00 |
| Q( 17) | 2 - 0 | 336.19 | -1029.98 | 0.00000D+00 | 9.78461D-26 | 1.34063D-02 |
| Q( 17) | 2 - 1 | 853.35 | -512.82 | 0.00000D+00 | 7.95268D-17 | -3.08987D-01 |
| Q( 17) | 2 - 2 | 1366.17 | 0.00 | 0.00000D+00 | 1.00000D+00 | -1.77826D+00 |
| Q( 18) | 2 - 0 | 345.09 | -1029.87 | 0.00000D+00 | 7.72137D-26 | 1.34083D-02 |
| Q( 18) | 2 - 1 | 862.19 | -512.77 | 0.00000D+00 | 7.90262D-17 | -3.08995D-01 |
| Q( 18) | 2 - 2 | 1374.96 | 0.00 | 0.00000D+00 | 1.00000D+00 | -1.77859D+00 |
| Q( 19) | 2 - 0 | 354.48 | -1029.75 | 0.00000D+00 | 5.17365D-26 | 1.34104D-02 |
| Q( 19) | 2 - 1 | 871.53 | -512.71 | 0.00000D+00 | 8.07232D-17 | -3.09004D-01 |
| Q( 19) | 2 - 2 | 1384.23 | 0.00 | 0.00000D+00 | 1.00000D+00 | -1.77893D+00 |
| Q( 20) | 2 - 0 | 364.37 | -1029.63 | 0.00000D+00 | 3.31778D-26 | 1.34127D-02 |
| Q( 20) | 2 - 1 | 881.35 | -512.65 | 0.00000D+00 | 8.01709D-17 | -3.09013D-01 |

| | | | | | | | |
|---|---|---|---|---|---|---|---|
| Q( 20) | 2 - 2 | 1394.00 | 0.00 | 0.00000D+00 | 1.00000D+00 | -1.77930D+00 |
| Q( 0) | 3 - 0 | 260.52 | -1539.74 | 0.00000D+00 | 7.20096D-21 | 8.15937D-04 |
| Q( 0) | 3 - 1 | 778.15 | -1022.11 | 0.00000D+00 | 7.10977D-18 | -2.35358D-02 |
| Q( 0) | 3 - 2 | 1291.45 | -508.81 | 0.00000D+00 | 3.09309D-16 | 3.76826D-01 |
| Q( 0) | 3 - 3 | 1800.26 | 0.00 | 0.00000D+00 | 1.00000D+00 | 1.81807D+00 |
| Q( 1) | 3 - 0 | 261.02 | -1539.73 | 0.00000D+00 | 2.03046D-20 | 8.15940D-04 |
| Q( 1) | 3 - 1 | 778.64 | -1022.11 | 0.00000D+00 | 5.77405D-18 | -2.35360D-02 |
| Q( 1) | 3 - 2 | 1291.94 | -508.81 | 0.00000D+00 | 3.48736D-16 | 3.76827D-01 |
| Q( 1) | 3 - 3 | 1800.75 | -0.00 | 0.00000D+00 | 1.00000D+00 | 1.81809D+00 |
| Q( 2) | 3 - 0 | 262.01 | -1539.71 | 0.00000D+00 | 1.39149D-19 | 8.15946D-04 |
| Q( 2) | 3 - 1 | 779.63 | -1022.09 | 0.00000D+00 | 1.82506D-18 | -2.35364D-02 |
| Q( 2) | 3 - 2 | 1292.92 | -508.80 | 0.00000D+00 | 5.30372D-16 | 3.76828D-01 |
| Q( 2) | 3 - 3 | 1801.72 | -0.00 | 0.00000D+00 | 1.00000D+00 | 1.81813D+00 |
| Q( 3) | 3 - 0 | 263.49 | -1539.68 | 0.00000D+00 | 7.31108D-25 | 8.15956D-04 |
| Q( 3) | 3 - 1 | 781.10 | -1022.07 | 0.00000D+00 | 9.30737D-18 | -2.35370D-02 |
| Q( 3) | 3 - 2 | 1294.38 | -508.79 | 0.00000D+00 | 2.54317D-16 | 3.76830D-01 |
| Q( 3) | 3 - 3 | 1803.17 | 0.00 | 0.00000D+00 | 1.00000D+00 | 1.81818D+00 |
| Q( 4) | 3 - 0 | 265.47 | -1539.65 | 0.00000D+00 | 7.27999D-25 | 8.15968D-04 |
| Q( 4) | 3 - 1 | 783.07 | -1022.05 | 0.00000D+00 | 9.28295D-18 | -2.35378D-02 |
| Q( 4) | 3 - 2 | 1296.34 | -508.78 | 0.00000D+00 | 2.53927D-16 | 3.76832D-01 |
| Q( 4) | 3 - 3 | 1805.12 | 0.00 | 0.00000D+00 | 1.00000D+00 | 1.81826D+00 |
| Q( 5) | 3 - 0 | 267.94 | -1539.60 | 0.00000D+00 | 7.32892D-25 | 8.15984D-04 |
| Q( 5) | 3 - 1 | 785.53 | -1022.02 | 0.00000D+00 | 9.25268D-18 | -2.35389D-02 |
| Q( 5) | 3 - 2 | 1298.78 | -508.76 | 0.00000D+00 | 2.53439D-16 | 3.76834D-01 |
| Q( 5) | 3 - 3 | 1807.54 | 0.00 | 0.00000D+00 | 1.00000D+00 | 1.81835D+00 |
| Q( 6) | 3 - 0 | 270.91 | -1539.54 | 0.00000D+00 | 7.29154D-25 | 8.16003D-04 |
| Q( 6) | 3 - 1 | 788.47 | -1021.98 | 0.00000D+00 | 9.21648D-18 | -2.35401D-02 |
| Q( 6) | 3 - 2 | 1301.71 | -508.74 | 0.00000D+00 | 2.52857D-16 | 3.76838D-01 |
| Q( 6) | 3 - 3 | 1810.45 | 0.00 | 0.00000D+00 | 1.00000D+00 | 1.81846D+00 |

| | | | | | | |
|---|---|---|---|---|---|---|
| Q( 7) | 3 - 0 | 274.37 | -1539.48 | 0.00000D+00 | 7.22969D-25 | 8.16025D-04 |
| Q( 7) | 3 - 1 | 791.92 | -1021.93 | 0.00000D+00 | 9.17449D-18 | -2.35415D-02 |
| Q( 7) | 3 - 2 | 1305.13 | -508.72 | 0.00000D+00 | 2.52182D-16 | 3.76841D-01 |
| Q( 7) | 3 - 3 | 1813.85 | 0.00 | 0.00000D+00 | 1.00000D+00 | 1.81859D+00 |
| Q( 8) | 3 - 0 | 278.33 | -1539.40 | 0.00000D+00 | 7.20749D-25 | 8.16050D-04 |
| Q( 8) | 3 - 1 | 795.85 | -1021.88 | 0.00000D+00 | 9.12657D-18 | -2.35432D-02 |
| Q( 8) | 3 - 2 | 1309.04 | -508.69 | 0.00000D+00 | 2.51415D-16 | 3.76846D-01 |
| Q( 8) | 3 - 3 | 1817.73 | 0.00 | 0.00000D+00 | 1.00000D+00 | 1.81874D+00 |
| Q( 9) | 3 - 0 | 282.78 | -1539.32 | 0.00000D+00 | 7.14594D-25 | 8.16079D-04 |
| Q( 9) | 3 - 1 | 800.27 | -1021.83 | 0.00000D+00 | 9.07321D-18 | -2.35450D-02 |
| Q( 9) | 3 - 2 | 1313.43 | -508.67 | 0.00000D+00 | 2.50558D-16 | 3.76851D-01 |
| Q( 9) | 3 - 3 | 1822.10 | 0.00 | 0.00000D+00 | 1.00000D+00 | 1.81890D+00 |
| Q( 10) | 3 - 0 | 287.73 | -1539.22 | 0.00000D+00 | 7.10992D-25 | 8.16110D-04 |
| Q( 10) | 3 - 1 | 805.19 | -1021.76 | 0.00000D+00 | 9.01430D-18 | -2.35471D-02 |
| Q( 10) | 3 - 2 | 1318.32 | -508.63 | 0.00000D+00 | 2.49612D-16 | 3.76856D-01 |
| Q( 10) | 3 - 3 | 1826.95 | 0.00 | 0.00000D+00 | 1.00000D+00 | 1.81909D+00 |
| Q( 11) | 3 - 0 | 293.17 | -1539.12 | 0.00000D+00 | 7.16296D-25 | 8.16145D-04 |
| Q( 11) | 3 - 1 | 810.59 | -1021.70 | 0.00000D+00 | 8.95005D-18 | -2.35494D-02 |
| Q( 11) | 3 - 2 | 1323.69 | -508.60 | 0.00000D+00 | 2.48579D-16 | 3.76862D-01 |
| Q( 11) | 3 - 3 | 1832.29 | 0.00 | 0.00000D+00 | 1.00000D+00 | 1.81929D+00 |
| Q( 12) | 3 - 0 | 299.10 | -1539.01 | 0.00000D+00 | 6.97322D-25 | 8.16183D-04 |
| Q( 12) | 3 - 1 | 816.49 | -1021.62 | 0.00000D+00 | 8.88055D-18 | -2.35518D-02 |
| Q( 12) | 3 - 2 | 1329.55 | -508.56 | 0.00000D+00 | 2.47464D-16 | 3.76868D-01 |
| Q( 12) | 3 - 3 | 1838.11 | 0.00 | 0.00000D+00 | 1.00000D+00 | 1.81951D+00 |
| Q( 13) | 3 - 0 | 305.53 | -1538.89 | 0.00000D+00 | 6.87657D-25 | 8.16224D-04 |
| Q( 13) | 3 - 1 | 822.88 | -1021.54 | 0.00000D+00 | 8.80603D-18 | -2.35545D-02 |
| Q( 13) | 3 - 2 | 1335.90 | -508.52 | 0.00000D+00 | 2.46268D-16 | 3.76875D-01 |
| Q( 13) | 3 - 3 | 1844.42 | 0.00 | 0.00000D+00 | 1.00000D+00 | 1.81975D+00 |
| Q( 14) | 3 - 0 | 312.46 | -1538.75 | 0.00000D+00 | 6.35310D-25 | 8.16268D-04 |

| | | | | | | | |
|---|---|---|---|---|---|---|---|
| Q( 14) | 3 - 1 | 829.76 | -1021.45 | 0.00000D+00 | 8.72587D-18 | -2.35574D-02 |
| Q( 14) | 3 - 2 | 1342.73 | -508.48 | 0.00000D+00 | 2.45007D-16 | 3.76883D-01 |
| Q( 14) | 3 - 3 | 1851.21 | 0.00 | 0.00000D+00 | 1.00000D+00 | 1.82001D+00 |
| Q( 15) | 3 - 0 | 319.87 | -1538.61 | 0.00000D+00 | 6.30302D-25 | 8.16316D-04 |
| Q( 15) | 3 - 1 | 837.13 | -1021.35 | 0.00000D+00 | 8.64162D-18 | -2.35605D-02 |
| Q( 15) | 3 - 2 | 1350.06 | -508.43 | 0.00000D+00 | 2.43657D-16 | 3.76891D-01 |
| Q( 15) | 3 - 3 | 1858.49 | 0.00 | 0.00000D+00 | 1.00000D+00 | 1.82029D+00 |
| Q( 16) | 3 - 0 | 327.79 | -1538.46 | 0.00000D+00 | 6.16947D-25 | 8.16367D-04 |
| Q( 16) | 3 - 1 | 844.99 | -1021.25 | 0.00000D+00 | 8.55274D-18 | -2.35638D-02 |
| Q( 16) | 3 - 2 | 1357.87 | -508.38 | 0.00000D+00 | 2.42237D-16 | 3.76899D-01 |
| Q( 16) | 3 - 3 | 1866.25 | 0.00 | 0.00000D+00 | 1.00000D+00 | 1.82058D+00 |
| Q( 17) | 3 - 0 | 336.19 | -1538.30 | 0.00000D+00 | 6.02062D-25 | 8.16421D-04 |
| Q( 17) | 3 - 1 | 853.35 | -1021.15 | 0.00000D+00 | 8.45953D-18 | -2.35673D-02 |
| Q( 17) | 3 - 2 | 1366.17 | -508.32 | 0.00000D+00 | 2.40747D-16 | 3.76908D-01 |
| Q( 17) | 3 - 3 | 1874.49 | 0.00 | 0.00000D+00 | 1.00000D+00 | 1.82089D+00 |
| Q( 18) | 3 - 0 | 345.09 | -1538.13 | 0.00000D+00 | 5.83232D-25 | 8.16478D-04 |
| Q( 18) | 3 - 1 | 862.19 | -1021.03 | 0.00000D+00 | 8.36215D-18 | -2.35711D-02 |
| Q( 18) | 3 - 2 | 1374.96 | -508.27 | 0.00000D+00 | 2.45361D-16 | 3.76918D-01 |
| Q( 18) | 3 - 3 | 1883.22 | 0.00 | 0.00000D+00 | 1.00000D+00 | 1.82123D+00 |
| Q( 19) | 3 - 0 | 354.48 | -1537.95 | 0.00000D+00 | 5.63001D-25 | 8.16539D-04 |
| Q( 19) | 3 - 1 | 871.53 | -1020.91 | 0.00000D+00 | 9.08394D-18 | -2.35750D-02 |
| Q( 19) | 3 - 2 | 1384.23 | -508.21 | 0.00000D+00 | 2.43709D-16 | 3.76928D-01 |
| Q( 19) | 3 - 3 | 1892.44 | 0.00 | 0.00000D+00 | 1.00000D+00 | 1.82158D+00 |
| Q( 20) | 3 - 0 | 364.37 | -1537.77 | 0.00000D+00 | 5.33229D-25 | 8.16603D-04 |
| Q( 20) | 3 - 1 | 881.35 | -1020.79 | 0.00000D+00 | 8.97080D-18 | -2.35791D-02 |
| Q( 20) | 3 - 2 | 1394.00 | -508.14 | 0.00000D+00 | 2.41996D-16 | 3.76939D-01 |
| Q( 20) | 3 - 3 | 1902.14 | 0.00 | 0.00000D+00 | 1.00000D+00 | 1.82195D+00 |
| Q( 0) | 4 - 0 | 260.52 | -2043.77 | 0.00000D+00 | 9.17408D-22 | 9.20601D-05 |
| Q( 0) | 4 - 1 | 778.15 | -1526.14 | 0.00000D+00 | 4.50711D-19 | -1.65450D-03 |

| | | | | | | | |
|---|---|---|---|---|---|---|---|
| Q( 0) | 4 - 2 | 1291.45 | -1012.83 | 0.00000D+00 | 3.63341D-17 | 3.38401D-02 |
| Q( 0) | 4 - 3 | 1800.26 | -504.03 | 0.00000D+00 | 2.99034D-17 | -4.33320D-01 |
| Q( 0) | 4 - 4 | 2304.29 | 0.00 | 0.00000D+00 | 1.00000D+00 | -1.86024D+00 |
| Q( 1) | 4 - 0 | 261.02 | -2043.75 | 0.00000D+00 | 2.65514D-21 | 9.20602D-05 |
| Q( 1) | 4 - 1 | 778.64 | -1526.13 | 0.00000D+00 | 3.33498D-19 | -1.65450D-03 |
| Q( 1) | 4 - 2 | 1291.94 | -1012.83 | 0.00000D+00 | 3.25118D-17 | 3.38405D-02 |
| Q( 1) | 4 - 3 | 1800.75 | -504.02 | 0.00000D+00 | 4.42014D-17 | -4.33320D-01 |
| Q( 1) | 4 - 4 | 2304.77 | -0.00 | 0.00000D+00 | 1.00000D+00 | -1.86026D+00 |
| Q( 2) | 4 - 0 | 262.01 | -2043.73 | 0.00000D+00 | 1.86258D-20 | 9.20605D-05 |
| Q( 2) | 4 - 1 | 779.63 | -1526.11 | 0.00000D+00 | 4.06623D-20 | -1.65452D-03 |
| Q( 2) | 4 - 2 | 1292.92 | -1012.82 | 0.00000D+00 | 1.93814D-17 | 3.38411D-02 |
| Q( 2) | 4 - 3 | 1801.72 | -504.02 | 0.00000D+00 | 1.29276D-16 | -4.33322D-01 |
| Q( 2) | 4 - 4 | 2305.73 | -0.00 | 0.00000D+00 | 1.00000D+00 | -1.86029D+00 |
| Q( 3) | 4 - 0 | 263.49 | -2043.69 | 0.00000D+00 | 1.39150D-25 | 9.20611D-05 |
| Q( 3) | 4 - 1 | 781.10 | -1526.08 | 0.00000D+00 | 6.48198D-19 | -1.65454D-03 |
| Q( 3) | 4 - 2 | 1294.38 | -1012.80 | 0.00000D+00 | 4.18886D-17 | 3.38421D-02 |
| Q( 3) | 4 - 3 | 1803.17 | -504.01 | 0.00000D+00 | 1.44485D-17 | -4.33323D-01 |
| Q( 3) | 4 - 4 | 2307.18 | 0.00 | 0.00000D+00 | 1.00000D+00 | -1.86035D+00 |
| Q( 4) | 4 - 0 | 265.47 | -2043.64 | 0.00000D+00 | 1.37472D-25 | 9.20618D-05 |
| Q( 4) | 4 - 1 | 783.07 | -1526.04 | 0.00000D+00 | 6.49557D-19 | -1.65456D-03 |
| Q( 4) | 4 - 2 | 1296.34 | -1012.77 | 0.00000D+00 | 4.17872D-17 | 3.38434D-02 |
| Q( 4) | 4 - 3 | 1805.12 | -503.99 | 0.00000D+00 | 1.44258D-17 | -4.33325D-01 |
| Q( 4) | 4 - 4 | 2309.11 | 0.00 | 0.00000D+00 | 1.00000D+00 | -1.86042D+00 |
| Q( 5) | 4 - 0 | 267.94 | -2043.58 | 0.00000D+00 | 1.38895D-25 | 9.20626D-05 |
| Q( 5) | 4 - 1 | 785.53 | -1525.99 | 0.00000D+00 | 6.51257D-19 | -1.65460D-03 |
| Q( 5) | 4 - 2 | 1298.78 | -1012.74 | 0.00000D+00 | 4.16608D-17 | 3.38450D-02 |
| Q( 5) | 4 - 3 | 1807.54 | -503.98 | 0.00000D+00 | 1.43975D-17 | -4.33328D-01 |
| Q( 5) | 4 - 4 | 2311.52 | 0.00 | 0.00000D+00 | 1.00000D+00 | -1.86051D+00 |
| Q( 6) | 4 - 0 | 270.91 | -2043.50 | 0.00000D+00 | 1.37514D-25 | 9.20637D-05 |

| | | | | | | | |
|---|---|---|---|---|---|---|---|
| Q( 6) | 4 - 1 | 788.47 | -1525.94 | 0.00000D+00 | 6.53288D-19 | -1.65464D-03 |
| Q( 6) | 4 - 2 | 1301.71 | -1012.70 | 0.00000D+00 | 4.15097D-17 | 3.38469D-02 |
| Q( 6) | 4 - 3 | 1810.45 | -503.96 | 0.00000D+00 | 1.43638D-17 | -4.33331D-01 |
| Q( 6) | 4 - 4 | 2314.41 | 0.00 | 0.00000D+00 | 1.00000D+00 | -1.86063D+00 |
| Q( 7) | 4 - 0 | 274.37 | -2043.41 | 0.00000D+00 | 1.37160D-25 | 9.20649D-05 |
| Q( 7) | 4 - 1 | 791.92 | -1525.87 | 0.00000D+00 | 6.55672D-19 | -1.65468D-03 |
| Q( 7) | 4 - 2 | 1305.13 | -1012.66 | 0.00000D+00 | 4.13346D-17 | 3.38492D-02 |
| Q( 7) | 4 - 3 | 1813.85 | -503.94 | 0.00000D+00 | 1.43248D-17 | -4.33335D-01 |
| Q( 7) | 4 - 4 | 2317.79 | 0.00 | 0.00000D+00 | 1.00000D+00 | -1.86076D+00 |
| Q( 8) | 4 - 0 | 278.33 | -2043.31 | 0.00000D+00 | 1.38374D-25 | 9.20663D-05 |
| Q( 8) | 4 - 1 | 795.85 | -1525.80 | 0.00000D+00 | 6.58373D-19 | -1.65473D-03 |
| Q( 8) | 4 - 2 | 1309.04 | -1012.61 | 0.00000D+00 | 4.11353D-17 | 3.38517D-02 |
| Q( 8) | 4 - 3 | 1817.73 | -503.91 | 0.00000D+00 | 1.42803D-17 | -4.33339D-01 |
| Q( 8) | 4 - 4 | 2321.64 | 0.00 | 0.00000D+00 | 1.00000D+00 | -1.86090D+00 |
| Q( 9) | 4 - 0 | 282.78 | -2043.20 | 0.00000D+00 | 1.35816D-25 | 9.20678D-05 |
| Q( 9) | 4 - 1 | 800.27 | -1525.71 | 0.00000D+00 | 6.61426D-19 | -1.65479D-03 |
| Q( 9) | 4 - 2 | 1313.43 | -1012.55 | 0.00000D+00 | 4.09128D-17 | 3.38546D-02 |
| Q( 9) | 4 - 3 | 1822.10 | -503.88 | 0.00000D+00 | 1.42306D-17 | -4.33344D-01 |
| Q( 9) | 4 - 4 | 2325.98 | 0.00 | 0.00000D+00 | 1.00000D+00 | -1.86107D+00 |
| Q( 10) | 4 - 0 | 287.73 | -2043.08 | 0.00000D+00 | 1.36413D-25 | 9.20695D-05 |
| Q( 10) | 4 - 1 | 805.19 | -1525.62 | 0.00000D+00 | 6.64807D-19 | -1.65486D-03 |
| Q( 10) | 4 - 2 | 1318.32 | -1012.49 | 0.00000D+00 | 4.06675D-17 | 3.38579D-02 |
| Q( 10) | 4 - 3 | 1826.95 | -503.85 | 0.00000D+00 | 1.41760D-17 | -4.33350D-01 |
| Q( 10) | 4 - 4 | 2330.80 | 0.00 | 0.00000D+00 | 1.00000D+00 | -1.86126D+00 |
| Q( 11) | 4 - 0 | 293.17 | -2042.94 | 0.00000D+00 | 1.36507D-25 | 9.20715D-05 |
| Q( 11) | 4 - 1 | 810.59 | -1525.51 | 0.00000D+00 | 6.68525D-19 | -1.65493D-03 |
| Q( 11) | 4 - 2 | 1323.69 | -1012.42 | 0.00000D+00 | 4.03996D-17 | 3.38614D-02 |
| Q( 11) | 4 - 3 | 1832.29 | -503.82 | 0.00000D+00 | 1.41163D-17 | -4.33356D-01 |
| Q( 11) | 4 - 4 | 2336.11 | 0.00 | 0.00000D+00 | 1.00000D+00 | -1.86146D+00 |

| | | | | | | | |
|---|---|---|---|---|---|---|---|
| Q( 12) | 4 - 0 | 299.10 | -2042.79 | 0.00000D+00 | 1.36380D-25 | 9.20736D-05 |
| Q( 12) | 4 - 1 | 816.49 | -1525.40 | 0.00000D+00 | 6.72578D-19 | -1.65501D-03 |
| Q( 12) | 4 - 2 | 1329.55 | -1012.34 | 0.00000D+00 | 4.01102D-17 | 3.38653D-02 |
| Q( 12) | 4 - 3 | 1838.11 | -503.78 | 0.00000D+00 | 1.40518D-17 | -4.33362D-01 |
| Q( 12) | 4 - 4 | 2341.89 | 0.00 | 0.00000D+00 | 1.00000D+00 | -1.86168D+00 |
| Q( 13) | 4 - 0 | 305.53 | -2042.62 | 0.00000D+00 | 1.58726D-25 | 9.20759D-05 |
| Q( 13) | 4 - 1 | 822.88 | -1525.27 | 0.00000D+00 | 6.76965D-19 | -1.65510D-03 |
| Q( 13) | 4 - 2 | 1335.90 | -1012.26 | 0.00000D+00 | 3.97996D-17 | 3.38695D-02 |
| Q( 13) | 4 - 3 | 1844.42 | -503.74 | 0.00000D+00 | 1.39826D-17 | -4.33369D-01 |
| Q( 13) | 4 - 4 | 2348.16 | 0.00 | 0.00000D+00 | 1.00000D+00 | -1.86192D+00 |
| Q( 14) | 4 - 0 | 312.46 | -2042.45 | 0.00000D+00 | 1.56601D-25 | 9.20784D-05 |
| Q( 14) | 4 - 1 | 829.76 | -1525.14 | 0.00000D+00 | 6.81675D-19 | -1.65519D-03 |
| Q( 14) | 4 - 2 | 1342.73 | -1012.17 | 0.00000D+00 | 3.94689D-17 | 3.38740D-02 |
| Q( 14) | 4 - 3 | 1851.21 | -503.69 | 0.00000D+00 | 1.39092D-17 | -4.33377D-01 |
| Q( 14) | 4 - 4 | 2354.90 | 0.00 | 0.00000D+00 | 1.00000D+00 | -1.86218D+00 |
| Q( 15) | 4 - 0 | 319.87 | -2042.26 | 0.00000D+00 | 1.57768D-25 | 9.20811D-05 |
| Q( 15) | 4 - 1 | 837.13 | -1525.00 | 0.00000D+00 | 6.86718D-19 | -1.65529D-03 |
| Q( 15) | 4 - 2 | 1350.06 | -1012.07 | 0.00000D+00 | 3.91181D-17 | 3.38788D-02 |
| Q( 15) | 4 - 3 | 1858.49 | -503.65 | 0.00000D+00 | 1.41679D-17 | -4.33385D-01 |
| Q( 15) | 4 - 4 | 2362.13 | 0.00 | 0.00000D+00 | 1.00000D+00 | -1.86246D+00 |
| Q( 16) | 4 - 0 | 327.79 | -2042.06 | 0.00000D+00 | 1.57502D-25 | 9.20840D-05 |
| Q( 16) | 4 - 1 | 844.99 | -1524.85 | 0.00000D+00 | 6.92108D-19 | -1.65539D-03 |
| Q( 16) | 4 - 2 | 1357.87 | -1011.97 | 0.00000D+00 | 3.87488D-17 | 3.38840D-02 |
| Q( 16) | 4 - 3 | 1866.25 | -503.60 | 0.00000D+00 | 1.40843D-17 | -4.33393D-01 |
| Q( 16) | 4 - 4 | 2369.84 | 0.00 | 0.00000D+00 | 1.00000D+00 | -1.86276D+00 |
| Q( 17) | 4 - 0 | 336.19 | -2041.84 | 0.00000D+00 | 1.60212D-25 | 9.20871D-05 |
| Q( 17) | 4 - 1 | 853.35 | -1524.69 | 0.00000D+00 | 6.97811D-19 | -1.65550D-03 |
| Q( 17) | 4 - 2 | 1366.17 | -1011.86 | 0.00000D+00 | 3.83613D-17 | 3.38895D-02 |
| Q( 17) | 4 - 3 | 1874.49 | -503.54 | 0.00000D+00 | 1.39969D-17 | -4.33403D-01 |

| | | | | | | |
|---|---|---|---|---|---|---|
| Q( 17) | 4 - 4 | 2378.03 | 0.00 | 0.00000D+00 | 1.00000D+00 | -1.86307D+00 |
| Q( 18) | 4 - 0 | 345.09 | -2041.62 | 0.00000D+00 | 1.62079D-25 | 9.20904D-05 |
| Q( 18) | 4 - 1 | 862.19 | -1524.52 | 0.00000D+00 | 7.03849D-19 | -1.65562D-03 |
| Q( 18) | 4 - 2 | 1374.96 | -1011.75 | 0.00000D+00 | 4.09730D-17 | 3.38953D-02 |
| Q( 18) | 4 - 3 | 1883.22 | -503.48 | 0.00000D+00 | 1.39057D-17 | -4.33412D-01 |
| Q( 18) | 4 - 4 | 2386.71 | 0.00 | 0.00000D+00 | 1.00000D+00 | -1.86341D+00 |
| Q( 19) | 4 - 0 | 354.48 | -2041.38 | 0.00000D+00 | 1.59867D-25 | 9.20940D-05 |
| Q( 19) | 4 - 1 | 871.53 | -1524.34 | 0.00000D+00 | 5.94809D-19 | -1.65575D-03 |
| Q( 19) | 4 - 2 | 1384.23 | -1011.63 | 0.00000D+00 | 4.05256D-17 | 3.39014D-02 |
| Q( 19) | 4 - 3 | 1892.44 | -503.42 | 0.00000D+00 | 1.38110D-17 | -4.33423D-01 |
| Q( 19) | 4 - 4 | 2395.86 | 0.00 | 0.00000D+00 | 1.00000D+00 | -1.86376D+00 |
| Q( 20) | 4 - 0 | 364.37 | -2041.13 | 0.00000D+00 | 1.62362D-25 | 9.20977D-05 |
| Q( 20) | 4 - 1 | 881.35 | -1524.15 | 0.00000D+00 | 6.01646D-19 | -1.65588D-03 |
| Q( 20) | 4 - 2 | 1394.00 | -1011.50 | 0.00000D+00 | 4.00620D-17 | 3.39079D-02 |
| Q( 20) | 4 - 3 | 1902.14 | -503.36 | 0.00000D+00 | 1.37130D-17 | -4.33433D-01 |
| Q( 20) | 4 - 4 | 2405.50 | 0.00 | 0.00000D+00 | 1.00000D+00 | -1.86413D+00 |
| Q( 0) | 5 - 0 | 260.52 | -2542.93 | 0.00000D+00 | 4.91615D-22 | 1.29098D-05 |
| Q( 0) | 5 - 1 | 778.15 | -2025.30 | 0.00000D+00 | 3.41922D-18 | -2.15353D-04 |
| Q( 0) | 5 - 2 | 1291.45 | -1512.00 | 0.00000D+00 | 1.34568D-19 | 2.61334D-03 |
| Q( 0) | 5 - 3 | 1800.26 | -1003.19 | 0.00000D+00 | 5.16604D-19 | -4.42543D-02 |
| Q( 0) | 5 - 4 | 2304.29 | -499.17 | 0.00000D+00 | 4.78406D-17 | 4.82430D-01 |
| Q( 0) | 5 - 5 | 2803.46 | 0.00 | 0.00000D+00 | 1.00000D+00 | 1.90055D+00 |
| Q( 1) | 5 - 0 | 261.02 | -2542.92 | 0.00000D+00 | 9.24163D-22 | 1.29093D-05 |
| Q( 1) | 5 - 1 | 778.64 | -2025.29 | 0.00000D+00 | 3.55550D-18 | -2.15356D-04 |
| Q( 1) | 5 - 2 | 1291.94 | -1511.99 | 0.00000D+00 | 2.38742D-19 | 2.61336D-03 |
| Q( 1) | 5 - 3 | 1800.75 | -1003.19 | 0.00000D+00 | 1.23295D-19 | -4.42547D-02 |
| Q( 1) | 5 - 4 | 2304.77 | -499.16 | 0.00000D+00 | 6.65502D-17 | 4.82430D-01 |
| Q( 1) | 5 - 5 | 2803.93 | -0.00 | 0.00000D+00 | 1.00000D+00 | 1.90057D+00 |
| Q( 2) | 5 - 0 | 262.01 | -2542.89 | 0.00000D+00 | 4.00736D-21 | 1.29083D-05 |

| | | | | | | | |
|---|---|---|---|---|---|---|---|
| Q( 2) | 5 - 1 | 779.63 | -2025.27 | 0.00000D+00 | 4.13020D-18 | -2.15363D-04 |
| Q( 2) | 5 - 2 | 1292.92 | -1511.97 | 0.00000D+00 | 9.55026D-19 | 2.61342D-03 |
| Q( 2) | 5 - 3 | 1801.72 | -1003.17 | 0.00000D+00 | 1.25098D-18 | -4.42556D-02 |
| Q( 2) | 5 - 4 | 2305.73 | -499.16 | 0.00000D+00 | 1.72247D-16 | 4.82431D-01 |
| Q( 2) | 5 - 5 | 2804.89 | -0.00 | 0.00000D+00 | 1.00000D+00 | 1.90060D+00 |
| Q( 3) | 5 - 0 | 263.49 | -2542.84 | 0.00000D+00 | 1.86181D-25 | 1.29068D-05 |
| Q( 3) | 5 - 1 | 781.10 | -2025.23 | 0.00000D+00 | 3.06079D-18 | -2.15374D-04 |
| Q( 3) | 5 - 2 | 1294.38 | -1511.95 | 0.00000D+00 | 1.48252D-21 | 2.61350D-03 |
| Q( 3) | 5 - 3 | 1803.17 | -1003.16 | 0.00000D+00 | 2.84216D-18 | -4.42569D-02 |
| Q( 3) | 5 - 4 | 2307.18 | -499.15 | 0.00000D+00 | 1.31832D-17 | 4.82432D-01 |
| Q( 3) | 5 - 5 | 2806.33 | 0.00 | 0.00000D+00 | 1.00000D+00 | 1.90066D+00 |
| Q( 4) | 5 - 0 | 265.47 | -2542.78 | 0.00000D+00 | 1.84659D-25 | 1.29048D-05 |
| Q( 4) | 5 - 1 | 783.07 | -2025.18 | 0.00000D+00 | 3.05564D-18 | -2.15388D-04 |
| Q( 4) | 5 - 2 | 1296.34 | -1511.91 | 0.00000D+00 | 1.26016D-21 | 2.61360D-03 |
| Q( 4) | 5 - 3 | 1805.12 | -1003.13 | 0.00000D+00 | 2.83547D-18 | -4.42586D-02 |
| Q( 4) | 5 - 4 | 2309.11 | -499.14 | 0.00000D+00 | 1.31621D-17 | 4.82434D-01 |
| Q( 4) | 5 - 5 | 2808.25 | 0.00 | 0.00000D+00 | 1.00000D+00 | 1.90073D+00 |
| Q( 5) | 5 - 0 | 267.94 | -2542.70 | 0.00000D+00 | 1.86380D-25 | 1.29023D-05 |
| Q( 5) | 5 - 1 | 785.53 | -2025.12 | 0.00000D+00 | 3.04926D-18 | -2.15406D-04 |
| Q( 5) | 5 - 2 | 1298.78 | -1511.86 | 0.00000D+00 | 1.00827D-21 | 2.61374D-03 |
| Q( 5) | 5 - 3 | 1807.54 | -1003.10 | 0.00000D+00 | 2.82707D-18 | -4.42608D-02 |
| Q( 5) | 5 - 4 | 2311.52 | -499.12 | 0.00000D+00 | 1.31361D-17 | 4.82436D-01 |
| Q( 5) | 5 - 5 | 2810.64 | 0.00 | 0.00000D+00 | 1.00000D+00 | 1.90083D+00 |
| Q( 6) | 5 - 0 | 270.91 | -2542.61 | 0.00000D+00 | 1.86040D-25 | 1.28994D-05 |
| Q( 6) | 5 - 1 | 788.47 | -2025.04 | 0.00000D+00 | 3.04164D-18 | -2.15427D-04 |
| Q( 6) | 5 - 2 | 1301.71 | -1511.81 | 0.00000D+00 | 7.43316D-22 | 2.61389D-03 |
| Q( 6) | 5 - 3 | 1810.45 | -1003.06 | 0.00000D+00 | 2.81697D-18 | -4.42634D-02 |
| Q( 6) | 5 - 4 | 2314.41 | -499.10 | 0.00000D+00 | 1.31050D-17 | 4.82439D-01 |
| Q( 6) | 5 - 5 | 2813.52 | 0.00 | 0.00000D+00 | 1.00000D+00 | 1.90094D+00 |

| | | | | | | | |
|---|---|---|---|---|---|---|---|
| Q( 7) | 5 - 0 | 274.37 | -2542.50 | 0.00000D+00 | 1.83927D-25 | 1.28959D-05 |
| Q( 7) | 5 - 1 | 791.92 | -2024.95 | 0.00000D+00 | 3.03277D-18 | -2.15451D-04 |
| Q( 7) | 5 - 2 | 1305.13 | -1511.74 | 0.00000D+00 | 4.85917D-22 | 2.61408D-03 |
| Q( 7) | 5 - 3 | 1813.85 | -1003.02 | 0.00000D+00 | 2.80537D-18 | -4.42665D-02 |
| Q( 7) | 5 - 4 | 2317.79 | -499.08 | 0.00000D+00 | 1.30688D-17 | 4.82442D-01 |
| Q( 7) | 5 - 5 | 2816.87 | 0.00 | 0.00000D+00 | 1.00000D+00 | 1.90107D+00 |
| Q( 8) | 5 - 0 | 278.33 | -2542.37 | 0.00000D+00 | 1.86387D-25 | 1.28919D-05 |
| Q( 8) | 5 - 1 | 795.85 | -2024.85 | 0.00000D+00 | 3.02265D-18 | -2.15479D-04 |
| Q( 8) | 5 - 2 | 1309.04 | -1511.67 | 0.00000D+00 | 2.58834D-22 | 2.61429D-03 |
| Q( 8) | 5 - 3 | 1817.73 | -1002.97 | 0.00000D+00 | 2.79209D-18 | -4.42700D-02 |
| Q( 8) | 5 - 4 | 2321.64 | -499.06 | 0.00000D+00 | 1.30277D-17 | 4.82446D-01 |
| Q( 8) | 5 - 5 | 2820.70 | 0.00 | 0.00000D+00 | 1.00000D+00 | 1.90122D+00 |
| Q( 9) | 5 - 0 | 282.78 | -2542.23 | 0.00000D+00 | 1.85555D-25 | 1.28874D-05 |
| Q( 9) | 5 - 1 | 800.27 | -2024.74 | 0.00000D+00 | 3.01137D-18 | -2.15511D-04 |
| Q( 9) | 5 - 2 | 1313.43 | -1511.58 | 0.00000D+00 | 8.88240D-23 | 2.61453D-03 |
| Q( 9) | 5 - 3 | 1822.10 | -1002.91 | 0.00000D+00 | 2.77729D-18 | -4.42739D-02 |
| Q( 9) | 5 - 4 | 2325.98 | -499.03 | 0.00000D+00 | 1.29819D-17 | 4.82450D-01 |
| Q( 9) | 5 - 5 | 2825.01 | 0.00 | 0.00000D+00 | 1.00000D+00 | 1.90139D+00 |
| Q( 10) | 5 - 0 | 287.73 | -2542.08 | 0.00000D+00 | 1.85448D-25 | 1.28823D-05 |
| Q( 10) | 5 - 1 | 805.19 | -2024.62 | 0.00000D+00 | 2.99886D-18 | -2.15546D-04 |
| Q( 10) | 5 - 2 | 1318.32 | -1511.49 | 0.00000D+00 | 4.18018D-24 | 2.61479D-03 |
| Q( 10) | 5 - 3 | 1826.95 | -1002.85 | 0.00000D+00 | 2.76098D-18 | -4.42783D-02 |
| Q( 10) | 5 - 4 | 2330.80 | -499.00 | 0.00000D+00 | 1.29314D-17 | 4.82455D-01 |
| Q( 10) | 5 - 5 | 2829.80 | 0.00 | 0.00000D+00 | 1.00000D+00 | 1.90157D+00 |
| Q( 11) | 5 - 0 | 293.17 | -2541.91 | 0.00000D+00 | 1.87979D-25 | 1.28768D-05 |
| Q( 11) | 5 - 1 | 810.59 | -2024.48 | 0.00000D+00 | 2.98523D-18 | -2.15584D-04 |
| Q( 11) | 5 - 2 | 1323.69 | -1511.38 | 0.00000D+00 | 3.64432D-23 | 2.61508D-03 |
| Q( 11) | 5 - 3 | 1832.29 | -1002.78 | 0.00000D+00 | 2.74315D-18 | -4.42831D-02 |
| Q( 11) | 5 - 4 | 2336.11 | -498.97 | 0.00000D+00 | 1.28765D-17 | 4.82460D-01 |

| | | | | | | | |
|---|---|---|---|---|---|---|---|
| Q( 11) | 5 - 5 | 2835.07 | 0.00 | 0.00000D+00 | 1.00000D+00 | 1.90178D+00 |
| Q( 12) | 5 - 0 | 299.10 | -2541.72 | 0.00000D+00 | 1.86855D-25 | 1.28707D-05 |
| Q( 12) | 5 - 1 | 816.49 | -2024.33 | 0.00000D+00 | 2.97047D-18 | -2.15625D-04 |
| Q( 12) | 5 - 2 | 1329.55 | -1511.27 | 0.00000D+00 | 2.19195D-22 | 2.61540D-03 |
| Q( 12) | 5 - 3 | 1838.11 | -1002.71 | 0.00000D+00 | 2.72389D-18 | -4.42883D-02 |
| Q( 12) | 5 - 4 | 2341.89 | -498.93 | 0.00000D+00 | 1.28168D-17 | 4.82465D-01 |
| Q( 12) | 5 - 5 | 2840.82 | 0.00 | 0.00000D+00 | 1.00000D+00 | 1.90200D+00 |
| Q( 13) | 5 - 0 | 305.53 | -2541.52 | 0.00000D+00 | 1.81059D-25 | 1.28641D-05 |
| Q( 13) | 5 - 1 | 822.88 | -2024.17 | 0.00000D+00 | 2.95461D-18 | -2.15670D-04 |
| Q( 13) | 5 - 2 | 1335.90 | -1511.15 | 0.00000D+00 | 5.88649D-22 | 2.61574D-03 |
| Q( 13) | 5 - 3 | 1844.42 | -1002.63 | 0.00000D+00 | 2.70321D-18 | -4.42940D-02 |
| Q( 13) | 5 - 4 | 2348.16 | -498.89 | 0.00000D+00 | 1.27532D-17 | 4.82471D-01 |
| Q( 13) | 5 - 5 | 2847.05 | 0.00 | 0.00000D+00 | 1.00000D+00 | 1.90224D+00 |
| Q( 14) | 5 - 0 | 312.46 | -2541.30 | 0.00000D+00 | 1.79333D-25 | 1.28570D-05 |
| Q( 14) | 5 - 1 | 829.76 | -2023.99 | 0.00000D+00 | 2.93763D-18 | -2.15718D-04 |
| Q( 14) | 5 - 2 | 1342.73 | -1511.02 | 0.00000D+00 | 1.18249D-21 | 2.61611D-03 |
| Q( 14) | 5 - 3 | 1851.21 | -1002.54 | 0.00000D+00 | 2.68121D-18 | -4.43001D-02 |
| Q( 14) | 5 - 4 | 2354.90 | -498.85 | 0.00000D+00 | 1.26855D-17 | 4.82477D-01 |
| Q( 14) | 5 - 5 | 2853.75 | 0.00 | 0.00000D+00 | 1.00000D+00 | 1.90250D+00 |
| Q( 15) | 5 - 0 | 319.87 | -2541.06 | 0.00000D+00 | 1.82870D-25 | 1.28493D-05 |
| Q( 15) | 5 - 1 | 837.13 | -2023.81 | 0.00000D+00 | 2.91963D-18 | -2.15769D-04 |
| Q( 15) | 5 - 2 | 1350.06 | -1510.88 | 0.00000D+00 | 2.04011D-21 | 2.61650D-03 |
| Q( 15) | 5 - 3 | 1858.49 | -1002.45 | 0.00000D+00 | 2.84464D-18 | -4.43066D-02 |
| Q( 15) | 5 - 4 | 2362.13 | -498.81 | 0.00000D+00 | 1.26139D-17 | 4.82484D-01 |
| Q( 15) | 5 - 5 | 2860.94 | 0.00 | 0.00000D+00 | 1.00000D+00 | 1.90278D+00 |
| Q( 16) | 5 - 0 | 327.79 | -2540.82 | 0.00000D+00 | 1.83752D-25 | 1.28411D-05 |
| Q( 16) | 5 - 1 | 844.99 | -2023.61 | 0.00000D+00 | 2.90062D-18 | -2.15823D-04 |
| Q( 16) | 5 - 2 | 1357.87 | -1510.73 | 0.00000D+00 | 3.20332D-21 | 2.61692D-03 |
| Q( 16) | 5 - 3 | 1866.25 | -1002.35 | 0.00000D+00 | 2.81868D-18 | -4.43136D-02 |

| | | | | | | |
|---|---|---|---|---|---|---|
| Q( 16) | 5 - 4 | 2369.84 | -498.76 | 0.00000D+00 | 1.28293D-17 | 4.82492D-01 |
| Q( 16) | 5 - 5 | 2868.60 | 0.00 | 0.00000D+00 | 1.00000D+00 | 1.90308D+00 |
| Q( 17) | 5 - 0 | 336.19 | -2540.55 | 0.00000D+00 | 1.85558D-25 | 1.28323D-05 |
| Q( 17) | 5 - 1 | 853.35 | -2023.39 | 0.00000D+00 | 2.88063D-18 | -2.15880D-04 |
| Q( 17) | 5 - 2 | 1366.17 | -1510.57 | 0.00000D+00 | 4.71456D-21 | 2.61737D-03 |
| Q( 17) | 5 - 3 | 1874.49 | -1002.25 | 0.00000D+00 | 2.79145D-18 | -4.43210D-02 |
| Q( 17) | 5 - 4 | 2378.03 | -498.71 | 0.00000D+00 | 1.27491D-17 | 4.82499D-01 |
| Q( 17) | 5 - 5 | 2876.74 | 0.00 | 0.00000D+00 | 1.00000D+00 | 1.90340D+00 |
| Q( 18) | 5 - 0 | 345.09 | -2540.27 | 0.00000D+00 | 1.85568D-25 | 1.28229D-05 |
| Q( 18) | 5 - 1 | 862.19 | -2023.17 | 0.00000D+00 | 2.85968D-18 | -2.15941D-04 |
| Q( 18) | 5 - 2 | 1374.96 | -1510.40 | 0.00000D+00 | 7.05642D-21 | 2.61784D-03 |
| Q( 18) | 5 - 3 | 1883.22 | -1002.14 | 0.00000D+00 | 2.76301D-18 | -4.43288D-02 |
| Q( 18) | 5 - 4 | 2386.71 | -498.65 | 0.00000D+00 | 1.26651D-17 | 4.82507D-01 |
| Q( 18) | 5 - 5 | 2885.36 | 0.00 | 0.00000D+00 | 1.00000D+00 | 1.90373D+00 |
| Q( 19) | 5 - 0 | 354.48 | -2539.97 | 0.00000D+00 | 1.86625D-25 | 1.28130D-05 |
| Q( 19) | 5 - 1 | 871.53 | -2022.93 | 0.00000D+00 | 2.95181D-18 | -2.16004D-04 |
| Q( 19) | 5 - 2 | 1384.23 | -1510.22 | 0.00000D+00 | 4.87843D-21 | 2.61833D-03 |
| Q( 19) | 5 - 3 | 1892.44 | -1002.02 | 0.00000D+00 | 2.73341D-18 | -4.43371D-02 |
| Q( 19) | 5 - 4 | 2395.86 | -498.59 | 0.00000D+00 | 1.25780D-17 | 4.82516D-01 |
| Q( 19) | 5 - 5 | 2894.46 | 0.00 | 0.00000D+00 | 1.00000D+00 | 1.90409D+00 |
| Q( 20) | 5 - 0 | 364.37 | -2539.66 | 0.00000D+00 | 1.88045D-25 | 1.28024D-05 |
| Q( 20) | 5 - 1 | 881.35 | -2022.68 | 0.00000D+00 | 2.92895D-18 | -2.16070D-04 |
| Q( 20) | 5 - 2 | 1394.00 | -1510.04 | 0.00000D+00 | 3.03222D-21 | 2.61885D-03 |
| Q( 20) | 5 - 3 | 1902.14 | -1001.90 | 0.00000D+00 | 2.70274D-18 | -4.43458D-02 |
| Q( 20) | 5 - 4 | 2405.50 | -498.53 | 0.00000D+00 | 1.24884D-17 | 4.82525D-01 |
| Q( 20) | 5 - 5 | 2904.03 | 0.00 | 0.00000D+00 | 1.00000D+00 | 1.90446D+00 |
