# Supplementary material for: Ab initio spectroscopic studies of AlF and AlCl molecules
Source: arXiv:2303.08681 source file (2023-03-15)
Supplement: Supplementary file 5 [file AlF_X1Sigma_S1.pdf]

AlF $X^1\Sigma$ --> centrifugal distortion constants (in $cm^{-1}$).

| v | Dv | Hv | Lv | Mv | Nv | Ov |
|---|---|---|---|---|---|---|
| 0 | -1.1783408D-06 | -1.4149025D-12 | 2.2078918D-16 | -1.2650691D-21 | -2.3592917D-25 | 2.4050205D-30 |
| 1 | -8.0275481D-07 | -9.6121708D-12 | -3.4258020D-16 | 1.1054928D-20 | 5.0869044D-25 | -4.4438134D-30 |
| 2 | -8.2103797D-07 | 1.0382513D-11 | -2.3473144D-16 | -1.6939438D-20 | 8.2437295D-26 | 4.9411979D-30 |
| 3 | -1.0775273D-06 | 3.2673512D-12 | 6.4560139D-16 | -7.7286443D-21 | -1.1694132D-24 | 2.7984798D-29 |
| 4 | -9.2078527D-07 | -1.0474645D-11 | -2.8931559D-16 | 4.5198930D-20 | 8.0316530D-25 | -9.4092717D-29 |
| 5 | -8.9641958D-07 | 1.0347906D-11 | -6.5710800D-16 | -4.2669359D-20 | 1.8431901D-24 | 8.0517502D-29 |
| 6 | -1.1209601D-06 | 4.6148772D-12 | 1.0887027D-15 | -2.7881491D-20 | -3.8169187D-24 | 1.1390778D-28 |
| 7 | -1.0037565D-06 | -1.4538333D-11 | -1.7609313D-16 | 9.6764601D-20 | 8.3708285D-25 | -3.4412288D-28 |
| 8 | -9.3763892D-07 | 6.9949733D-12 | -1.1558938D-15 | -6.1578375D-20 | 5.7258364D-24 | 2.2944820D-28 |
| 9 | -1.1280028D-06 | 7.1262959D-12 | 1.3139726D-15 | -7.4962973D-20 | -7.0147928D-24 | 3.5374218D-28 |
| 10 | -1.0627451D-06 | -1.6645050D-11 | 4.3993649D-16 | 1.5400254D-19 | -2.9820424D-24 | -7.7267944D-28 |
| 11 | -9.2355695D-07 | 8.0207960D-13 | -1.8665535D-15 | -1.9748444D-20 | 1.3169356D-23 | 1.7088413D-28 |
| 12 | -1.0554851D-06 | 1.5049623D-11 | 6.7954907D-16 | -1.7737190D-19 | -4.9545382D-24 | 9.2997732D-28 |
| 13 | -1.0964316D-06 | -9.9809344D-12 | 1.7626417D-15 | 1.2208109D-19 | -1.5462227D-23 | -7.1656182D-28 |
| 14 | -9.3314381D-07 | -1.1659969D-11 | -1.6607485D-15 | 1.5456766D-19 | 1.5970564D-23 | -9.8850218D-28 |
| 15 | -9.4435924D-07 | 1.4438592D-11 | -1.1986155D-15 | -2.1255346D-19 | 1.1014261D-23 | 1.4265339D-27 |
| 16 | -1.0714584D-06 | 6.6585064D-12 | 2.2424589D-15 | -1.0784636D-19 | -2.2722193D-23 | 8.9481377D-28 |
| 17 | -9.9942382D-07 | -1.7130544D-11 | 6.9431905D-16 | 2.8523702D-19 | -7.9550555D-24 | -2.3675014D-27 |
| 18 | -8.7404064D-07 | -3.2631257D-12 | -2.5956998D-15 | 5.1308789D-20 | 3.0332008D-23 | -2.7104486D-28 |
| 19 | -9.4155096D-07 | 1.7914474D-11 | -3.3424291D-16 | -3.2018635D-19 | 3.6812275D-24 | 2.6309594D-27 |
| 20 | -1.0302273D-06 | 1.9643916D-12 | 2.7668672D-15 | -3.6103637D-20 | -3.5203599D-23 | 4.8321846D-28 |
| 21 | -9.4166820D-07 | -1.7747297D-11 | 2.4774009D-16 | 3.6486105D-19 | -3.2032011D-24 | -3.6681849D-27 |
| 22 | -8.4079649D-07 | -1.5956472D-12 | -2.8992869D-15 | 3.1251897D-20 | 4.0656844D-23 | -1.0868483D-28 |
| 23 | -9.0210198D-07 | 1.8018578D-11 | -4.0646576D-16 | -3.8255674D-19 | 5.4152983D-24 | 3.7881865D-27 |
| 24 | -9.8276430D-07 | 3.9912931D-12 | 2.9480491D-15 | -8.5295966D-20 | -4.4203590D-23 | 1.0974038D-27 |
| 25 | -9.1801517D-07 | -1.6881945D-11 | 8.7436155D-16 | 4.0918372D-19 | -1.4130110D-23 | -4.7647404D-27 |
| 26 | -8.1529477D-07 | -6.4844274D-12 | -2.9065313D-15 | 1.6196922D-19 | 4.7836821D-23 | -1.7031231D-27 |
| 27 | -8.4000455D-07 | 1.5952133D-11 | -1.5673956D-15 | -3.8823662D-19 | 2.5129496D-23 | 4.5188282D-27 |
| 28 | -9.2821718D-07 | 1.1601153D-11 | 2.5106162D-15 | -2.8927795D-19 | -4.2298575D-23 | 3.6226922D-27 |
| 29 | -9.1685954D-07 | -1.1508218D-11 | 2.4521315D-15 | 3.1869726D-19 | -4.4673882D-23 | -4.0346394D-27 |
| 30 | -8.1687562D-07 | -1.4933187D-11 | -1.7219514D-15 | 4.2223405D-19 | 3.2658679D-23 | -5.6225849D-27 |
| 31 | -7.7897868D-07 | 6.2253054D-12 | -3.1503122D-15 | -1.6899584D-19 | 5.8335015D-23 | 2.4782120D-27 |
| 32 | -8.4596877D-07 | 1.8035118D-11 | 3.4655485D-16 | -5.0467661D-19 | -6.6769785D-24 | 6.7081128D-27 |
| 33 | -9.0003741D-07 | 2.9696667D-12 | 3.3598721D-15 | -7.6989212D-20 | -6.6411945D-23 | 1.3408182D-27 |
| 34 | -8.5210094D-07 | -1.5717914D-11 | 1.3365489D-15 | 4.9744527D-19 | -2.7882906D-23 | -7.4359572D-27 |
| 35 | -7.6784786D-07 | -1.0468878D-11 | -2.7056826D-15 | 3.3773935D-19 | 5.7663461D-23 | -4.9441644D-27 |
| 36 | -7.5947120D-07 | 1.0195316D-11 | -2.8391759D-15 | -3.1591070D-19 | 5.9209808D-23 | 4.9110990D-27 |
| 37 | -8.2527811D-07 | 1.6885422D-11 | 9.8705644D-16 | -5.3477388D-19 | -2.1017490D-23 | 8.0981789D-27 |
| 38 | -8.6455013D-07 | 1.0475329D-12 | 3.5003781D-15 | -2.4424154D-20 | -7.8146437D-23 | 6.9005514D-28 |
| 39 | -8.1932803D-07 | -1.5514742D-11 | 1.2909751D-15 | 5.4813858D-19 | -3.0271580D-23 | -9.1582547D-27 |
| 40 | -7.4620875D-07 | -1.0912237D-11 | -2.6684686D-15 | 3.9229486D-19 | 6.3332510D-23 | -6.4719619D-27 |
| 41 | -7.3354639D-07 | 8.0433087D-12 | -3.1584301D-15 | -2.7705154D-19 | 7.3709178D-23 | 4.8631026D-27 |
| 42 | -7.8757236D-07 | 1.7036178D-11 | 2.9896019D-16 | -6.0094081D-19 | -7.0950351D-24 | 1.0067520D-26 |
| 43 | -8.3406474D-07 | 5.5499683D-12 | 3.4036591D-15 | -1.9636951D-19 | -8.3241037D-23 | 3.7401276D-27 |
| 44 | -8.1352773D-07 | -1.2114003D-11 | 2.4202471D-15 | 4.6858191D-19 | -6.2210440D-23 | -8.4481727D-27 |
| 45 | -7.4892581D-07 | -1.4936969D-11 | -1.4753876D-15 | 5.8547779D-19 | 3.8726708D-23 | -1.0927907D-26 |
| 46 | -7.1268015D-07 | -2.1838218D-13 | -3.6390728D-15 | 1.0966276D-20 | 9.4684960D-23 | 1.3553335D-28 |
| 47 | -7.4005261D-07 | 1.4624468D-11 | -1.6828798D-15 | -5.7177135D-19 | 4.3229884D-23 | 1.0615517D-26 |
| 48 | -7.9449139D-07 | 1.3381989D-11 | 2.0923207D-15 | -5.3212783D-19 | -5.5334460D-23 | 1.0133429D-26 |
| 49 | -8.1421783D-07 | -1.9969020D-12 | 3.6184208D-15 | 8.4099153D-20 | -9.9651962D-23 | -1.3076590D-27 |
| 50 | -7.7845039D-07 | -1.4929466D-11 | 1.2956557D-15 | 6.3062968D-19 | -3.6996416D-23 | -1.2832240D-26 |
| 51 | -7.2509321D-07 | -1.2146232D-11 | -2.3880017D-15 | 5.1579722D-19 | 6.9010429D-23 | -1.0494476D-26 |
| 52 | -7.0737902D-07 | 2.8142923D-12 | -3.6053798D-15 | -1.3017945D-19 | 1.0315550D-22 | 3.0124050D-27 |
| 53 | -7.3961008D-07 | 1.4561875D-11 | -1.2534151D-15 | -6.4177438D-19 | 3.5490340D-23 | 1.3127055D-26 |
| 54 | -7.8758894D-07 | 1.1960084D-11 | 2.2738079D-15 | -5.3918095D-19 | -6.6531190D-23 | 1.1363249D-26 |
| 55 | -8.0567452D-07 | -1.9958372D-12 | 3.6428122D-15 | 7.6618141D-20 | -1.1033667D-22 | -1.2978561D-27 |

| | | | | | | |
|---|---|---|---|---|---|---|
| 56 | -7.7936697D-07 | -1.4084995D-11 | 1.6185915D-15 | 6.3593666D-19 | -5.0558433D-23 | -1.4146127D-26 |
| 57 | -7.3532018D-07 | -1.3479753D-11 | -1.8759469D-15 | 6.1317423D-19 | 5.9668072D-23 | -1.3776014D-26 |
| 58 | -7.1375069D-07 | -1.2953480D-12 | -3.6594587D-15 | 3.9700083D-20 | 1.1574831D-22 | -5.0669366D-28 |
| 59 | -7.3205766D-07 | 1.1448970D-11 | -2.2622282D-15 | -5.6208497D-19 | 7.1321182D-23 | 1.2744768D-26 |
| 60 | -7.7262830D-07 | 1.4138449D-11 | 1.0114492D-15 | -6.9333951D-19 | -3.1838022D-23 | 1.5739168D-26 |
| 61 | -8.0108752D-07 | 5.0511377D-12 | 3.4419773D-15 | -2.5873392D-19 | -1.1231538D-22 | 6.3783362D-27 |
| 62 | -7.9526939D-07 | -8.0884251D-12 | 3.1066184D-15 | 3.9553357D-19 | -1.0485667D-22 | -9.2696701D-27 |
| 63 | -7.6098829D-07 | -1.4772551D-11 | 3.2709291D-16 | 7.4377532D-19 | -1.0977026D-23 | -1.8359442D-26 |
| 64 | -7.2475632D-07 | -1.0125230D-11 | -2.6749308D-15 | 5.1030038D-19 | 9.3367720D-23 | -1.2447720D-26 |
| 65 | -7.1234139D-07 | 1.7535241D-12 | -3.6325748D-15 | -1.0487988D-19 | 1.2570478D-22 | 2.9989276D-27 |
| 66 | -7.3040058D-07 | 1.1877904D-11 | -1.9404538D-15 | -6.3413950D-19 | 6.6876260D-23 | 1.5748776D-26 |
| 67 | -7.6328824D-07 | 1.3347651D-11 | 1.0919656D-15 | -7.1736695D-19 | -3.8063201D-23 | 1.7912728D-26 |
| 68 | -7.8632941D-07 | 5.5531242D-12 | 3.3384816D-15 | -3.0944718D-19 | -1.1937907D-22 | 8.2582111D-27 |
| 69 | -7.8384858D-07 | -5.9298648D-12 | 3.3319297D-15 | 3.1571135D-19 | -1.2265149D-22 | -7.9624511D-27 |
| 70 | -7.5765105D-07 | -1.3330298D-11 | 1.1263169D-15 | 7.3585276D-19 | -4.2197009D-23 | -1.9795435D-26 |
| 71 | -7.2434888D-07 | -1.2134872D-11 | -1.7902407D-15 | 6.7558929D-19 | 6.8448290D-23 | -1.8268566D-26 |
| 72 | -7.0397134D-07 | -3.5056241D-12 | -3.5207800D-15 | 1.8750291D-19 | 1.3411109D-22 | -4.6596683D-27 |
| 73 | -7.0641724D-07 | 6.9495453D-12 | -3.0819443D-15 | -4.0808982D-19 | 1.1668174D-22 | 1.1386966D-26 |
| 74 | -7.2748641D-07 | 1.2921258D-11 | -8.3676383D-16 | -7.5213376D-19 | 3.1519512D-23 | 2.0446790D-26 |
| 75 | -7.5254970D-07 | 1.1340423D-11 | 1.8483244D-15 | -6.6637229D-19 | -7.1465066D-23 | 1.8452224D-26 |
| 76 | -7.6591093D-07 | 3.4230138D-12 | 3.4576662D-15 | -2.0571664D-19 | -1.3643780D-22 | 6.1849838D-27 |
| 77 | -7.5967456D-07 | -6.1462170D-12 | 3.1612417D-15 | 3.6990643D-19 | -1.2775152D-22 | -1.0371874D-26 |
| 78 | -7.3663446D-07 | -1.2207886D-11 | 1.1614768D-15 | 7.4816693D-19 | -4.7621338D-23 | -2.2014292D-26 |
| 79 | -7.0830405D-07 | -1.1729101D-11 | -1.4068710D-15 | 7.2689838D-19 | 5.8877730D-23 | -2.1551157D-26 |
| 80 | -6.8749840D-07 | -5.2975206D-12 | -3.2161891D-15 | 3.3174477D-19 | 1.3432246D-22 | -9.4927637D-27 |
| 81 | -6.8238940D-07 | 3.6064743D-12 | -3.3848245D-15 | -2.2149062D-19 | 1.4074725D-22 | 7.0048729D-27 |
| 82 | -6.9249465D-07 | 1.0586217D-11 | -1.9371872D-15 | -6.5777432D-19 | 8.0512212D-23 | 1.9669915D-26 |
| 83 | -7.1045726D-07 | 1.2542160D-11 | 3.9054772D-16 | -7.8347269D-19 | -1.6445466D-23 | 2.3444423D-26 |
| 84 | -7.2565944D-07 | 8.8645844D-12 | 2.4924614D-15 | -5.5284739D-19 | -1.0596715D-22 | 1.7027069D-26 |
| 85 | -7.2971372D-07 | 1.5126136D-12 | 3.4655125D-15 | -7.8164067D-20 | -1.5040708D-22 | 2.8709882D-27 |
| 86 | -7.1942304D-07 | -6.1657208D-12 | 2.9145931D-15 | 4.3290475D-19 | -1.2892975D-22 | -1.3426891D-26 |
| 87 | -6.9791558D-07 | -1.0839184D-11 | 1.1379799D-15 | 7.5458217D-19 | -5.0822494D-23 | -2.4253443D-26 |
| 88 | -6.7247280D-07 | -1.0747178D-11 | -1.0760403D-15 | 7.5877107D-19 | 4.9443841D-23 | -2.4605632D-26 |
| 89 | -6.5121852D-07 | -6.1140493D-12 | -2.8065852D-15 | 4.5113998D-19 | 1.2836801D-22 | -1.4343173D-26 |
| 90 | -6.3983696D-07 | 9.7913866D-13 | -3.3866879D-15 | -2.6389909D-20 | 1.5428305D-22 | 1.3193350D-27 |
| 91 | -6.3949181D-07 | 7.7427385D-12 | -2.6696673D-15 | -4.8394407D-19 | 1.2153895D-22 | 1.5962847D-26 |
| 92 | -6.4716555D-07 | 1.1726696D-11 | -9.7492402D-16 | -7.5485013D-19 | 4.4666567D-23 | 2.4557888D-26 |
| 93 | -6.5694384D-07 | 1.1664940D-11 | 1.0317275D-15 | -7.5016523D-19 | -4.6852809D-23 | 2.4606683D-26 |
| 94 | -6.6262612D-07 | 7.8480184D-12 | 2.6431334D-15 | -4.8504936D-19 | -1.2239220D-22 | 1.6439589D-26 |
| 95 | -6.5975100D-07 | 1.7614736D-12 | 3.3260840D-15 | -5.2414590D-20 | -1.5693168D-22 | 2.2504551D-27 |
| 96 | -6.4687122D-07 | -4.3976347D-12 | 2.8740192D-15 | 3.9582462D-19 | -1.3772432D-22 | -1.3263364D-26 |
| 97 | -6.2590097D-07 | -8.5727002D-12 | 1.4882240D-15 | 7.0872522D-19 | -7.2070173D-23 | -2.4615811D-26 |
| 98 | -6.0100778D-07 | -9.5107814D-12 | -3.5363608D-16 | 7.8823425D-19 | 1.7963832D-23 | -2.7759999D-26 |
| 99 | -5.7726344D-07 | -7.0405711D-12 | -2.0467068D-15 | 6.1256190D-19 | 1.0155859D-22 | -2.1460262D-26 |
| 100 | -5.5908126D-07 | -2.1284476D-12 | -3.0660739D-15 | 2.5028677D-19 | 1.5121380D-22 | -8.4427328D-27 |
| 101 | -5.4896499D-07 | 3.5883605D-12 | -3.1477119D-15 | -1.7827858D-19 | 1.5438789D-22 | 6.6555305D-27 |
| 102 | -5.4714459D-07 | 8.3941167D-12 | -2.3055867D-15 | -5.4615978D-19 | 1.1251011D-22 | 1.9431702D-26 |
| 103 | -5.5147220D-07 | 1.0972709D-11 | -8.1488624D-16 | -7.4958447D-19 | 3.9394200D-23 | 2.6455244D-26 |
| 104 | -5.5792750D-07 | 1.0777438D-11 | 8.6999720D-16 | -7.4200400D-19 | -4.3237516D-23 | 2.6341879D-26 |
| 105 | -5.6212319D-07 | 7.9867532D-12 | 2.2748659D-15 | -5.3540193D-19 | -1.1391454D-22 | 1.9425310D-26 |
| 106 | -5.6105042D-07 | 3.3289090D-12 | 3.0325244D-15 | -1.8478362D-19 | -1.5437095D-22 | 7.1292397D-27 |
| 107 | -5.5385670D-07 | -1.9207125D-12 | 2.9792730D-15 | 2.1461993D-19 | -1.5369155D-22 | -7.4728382D-27 |
| 108 | -5.4111574D-07 | -6.2587649D-12 | 2.1675892D-15 | 5.5162970D-19 | -1.1285410D-22 | -2.0296540D-26 |
| 109 | -5.2429629D-07 | -8.6353591D-12 | 8.0786574D-16 | 7.4220638D-19 | -4.2471799D-23 | -2.7891879D-26 |
| 110 | -5.0625782D-07 | -8.6568279D-12 | -7.3765727D-16 | 7.4611193D-19 | 3.9009757D-23 | -2.8207720D-26 |
| 111 | -4.9026015D-07 | -6.3485640D-12 | -2.0521942D-15 | 5.6381671D-19 | 1.0898829D-22 | -2.1133055D-26 |
| 112 | -4.7829436D-07 | -2.3329707D-12 | -2.8498957D-15 | 2.4665736D-19 | 1.5090803D-22 | -8.9414737D-27 |
| 113 | -4.7155234D-07 | 2.2526422D-12 | -2.9696950D-15 | -1.1721540D-19 | 1.5676767D-22 | 4.8224499D-27 |
| 114 | -4.7019957D-07 | 6.4112784D-12 | -2.3915542D-15 | -4.4831014D-19 | 1.2616359D-22 | 1.7158764D-26 |

| | | | | | | |
|---|---|---|---|---|---|---|
| 115 | -4.7272067D-07 | 9.2347235D-12 | -1.3011265D-15 | -6.7427726D-19 | 6.8478549D-23 | 2.5509464D-26 |
| 116 | -4.7726692D-07 | 1.0071237D-11 | 5.5172328D-17 | -7.4360875D-19 | -3.2469085D-24 | 2.8122586D-26 |
| 117 | -4.8158703D-07 | 8.9258319D-12 | 1.3723343D-15 | -6.5632916D-19 | -7.3511104D-23 | 2.5079657D-26 |
| 118 | -4.8359765D-07 | 6.0282813D-12 | 2.3577030D-15 | -4.3009451D-19 | -1.2760235D-22 | 1.6835980D-26 |
| 119 | -4.8237381D-07 | 2.0249385D-12 | 2.8406311D-15 | -1.1605645D-19 | -1.5612631D-22 | 4.9010136D-27 |
| 120 | -4.7768007D-07 | -2.2766824D-12 | 2.7020460D-15 | 2.1793408D-19 | -1.5107905D-22 | -8.2677285D-27 |
| 121 | -4.7083558D-07 | -6.1077973D-12 | 2.0190663D-15 | 5.0662668D-19 | -1.1529457D-22 | -1.9963206D-26 |
| 122 | -4.6356551D-07 | -8.6738808D-12 | 9.4640428D-16 | 6.8730721D-19 | -5.6079808D-23 | -2.7426805D-26 |
| 123 | -4.5752163D-07 | -9.5406489D-12 | -2.7960618D-16 | 7.3374985D-19 | 1.3653101D-23 | -2.9495415D-26 |
| 124 | -4.5361459D-07 | -8.4980329D-12 | -1.4317097D-15 | 6.2984915D-19 | 7.9742256D-23 | -2.5328279D-26 |
| 125 | -4.5252341D-07 | -6.0463609D-12 | -2.3238633D-15 | 4.0932125D-19 | 1.2984515D-22 | -1.6336037D-26 |
| 126 | -4.5569257D-07 | -2.8978468D-12 | -2.7808164D-15 | 1.1864746D-19 | 1.5419410D-22 | -4.4168992D-27 |
| 127 | -4.6439575D-07 | 2.6329146D-13 | -2.7168555D-15 | -1.7942634D-19 | 1.5025120D-22 | 7.6019534D-27 |
| 128 | -4.7841882D-07 | 3.0781952D-12 | -2.1648042D-15 | -4.4726200D-19 | 1.1926980D-22 | 1.8208185D-26 |
| 129 | -4.9632305D-07 | 4.8806621D-12 | -1.3061883D-15 | -6.3263996D-19 | 7.0228597D-23 | 2.5471694D-26 |
| 130 | -5.1771562D-07 | 5.1848526D-12 | -2.5807904D-16 | -7.0423257D-19 | 9.9578696D-24 | 2.8476245D-26 |
| 131 | -5.4204264D-07 | 4.0542209D-12 | 8.1572970D-16 | -6.5897282D-19 | -5.1589686D-23 | 2.6777147D-26 |
| 132 | -5.6800066D-07 | 1.7203984D-12 | 1.6844482D-15 | -5.2032415D-19 | -1.0329524D-22 | 2.1429395D-26 |
| 133 | -5.9564914D-07 | -1.8098718D-12 | 2.2368423D-15 | -2.9258190D-19 | -1.3824983D-22 | 1.2345467D-26 |
| 134 | -6.2586497D-07 | -5.8758990D-12 | 2.4386354D-15 | -3.4409856D-20 | -1.5390100D-22 | 1.7273065D-27 |
| 135 | -6.5931530D-07 | -1.0156417D-11 | 2.2042339D-15 | 2.2462707D-19 | -1.4481422D-22 | -9.4057977D-27 |
| 136 | -6.9832297D-07 | -1.4330603D-11 | 1.6517690D-15 | 4.5332195D-19 | -1.1517048D-22 | -1.9379867D-26 |
| 137 | -7.4455517D-07 | -1.7712846D-11 | 8.9925430D-16 | 6.0547172D-19 | -7.1011167D-23 | -2.6081676D-26 |
| 138 | -7.9821764D-07 | -2.0000966D-11 | 5.9027721D-17 | 6.8547475D-19 | -1.6699722D-23 | -2.9791868D-26 |
| 139 | -8.5779634D-07 | -2.0628985D-11 | -7.2602717D-16 | 6.5061536D-19 | 3.2388069D-23 | -2.8974823D-26 |
| 140 | -9.2115292D-07 | -2.0574590D-11 | -1.6506884D-15 | 5.2369960D-19 | 8.0747371D-23 | -2.4761395D-26 |
| 141 | -9.9417209D-07 | -2.1808763D-11 | -2.5886847D-15 | 3.5257648D-19 | 1.2009876D-22 | -1.7322330D-26 |
| 142 | -1.0889423D-06 | -2.5108777D-11 | -3.1770214D-15 | 2.0152058D-19 | 1.4435056D-22 | -1.0171918D-26 |
| 143 | -1.2124283D-06 | -2.8971014D-11 | -3.3938817D-15 | -4.6301226D-20 | 1.3386214D-22 | -1.5964223D-27 |
| 144 | -1.3696972D-06 | -3.6486407D-11 | -4.3393024D-15 | -3.4273823D-19 | 1.3721701D-22 | 8.7089498D-27 |
| 145 | -1.5908142D-06 | -5.2814901D-11 | -5.5452960D-15 | -5.6439672D-19 | 9.8809528D-23 | 9.4749387D-27 |
| 146 | -1.9207817D-06 | -8.3105200D-11 | -8.9239931D-15 | -1.3009966D-18 | -1.1803157D-23 | 8.9209528D-27 |
| 147 | -2.4781413D-06 | -1.5941029D-10 | -2.1417457D-14 | -3.5685862D-18 | -4.5606886D-22 | -8.8346975D-26 |
| 148 | -3.6936551D-06 | -4.2427939D-10 | -9.1843755D-14 | -2.4850240D-17 | -7.1500455D-21 | -2.2404806D-24 |
| 149 | -8.7768479D-06 | -2.8881891D-09 | -1.4482391D-12 | -8.0626736D-16 | -4.6705012D-19 | -2.7840323D-22 |
