# Supplementary material for: Ab initio spectroscopic studies of AlF and AlCl molecules
Source: arXiv:2303.08681 source file (2023-03-15)
Supplement: Supplementary file 6 [file AlF_singlet_pi_-_S9.pdf]

# AlF $A^1\Pi$: Rotational parameters

Note that (v',J') & (v",J") strictly label the upper and lower levels, resp., and E(lower)=E"

but E(2)-E(1) is: (energy of State-2 level) - (energy of State-1 level)

In the following table, E is expressed in $cm^{-1}$, A in $s^{-1}$ and transition dipole moment in debye.

| dJ(J") | Band v' v" | E(lower) | E(2)-E(1) | A(Einstein) | F-C Factor | <v'j'\|M\|v"j"> |
|---|---|---|---|---|---|---|
| R( 0) | 0 - 0 | 399.14 | -1.09 | 3.32905D-07 | 1.00000D+00 | -1.56719D+00 |
| R( 1) | 0 - 0 | 400.23 | -2.18 | 3.19589D-06 | 1.00000D+00 | -1.56722D+00 |
| R( 2) | 0 - 0 | 402.41 | -3.27 | 1.15568D-05 | 1.00000D+00 | -1.56728D+00 |
| R( 3) | 0 - 0 | 405.68 | -4.36 | 2.84092D-05 | 1.00000D+00 | -1.56737D+00 |
| R( 4) | 0 - 0 | 410.04 | -5.45 | 5.67497D-05 | 1.00000D+00 | -1.56747D+00 |
| R( 5) | 0 - 0 | 415.49 | -6.54 | 9.95764D-05 | 1.00000D+00 | -1.56760D+00 |
| R( 6) | 0 - 0 | 422.03 | -7.63 | 1.59889D-04 | 1.00000D+00 | -1.56776D+00 |
| R( 7) | 0 - 0 | 429.67 | -8.72 | 2.40687D-04 | 1.00000D+00 | -1.56794D+00 |
| R( 8) | 0 - 0 | 438.39 | -9.81 | 3.44974D-04 | 1.00000D+00 | -1.56814D+00 |
| R( 9) | 0 - 0 | 448.20 | -10.90 | 4.75754D-04 | 9.99999D-01 | -1.56836D+00 |
| R( 10) | 0 - 0 | 459.10 | -11.99 | 6.36033D-04 | 9.99999D-01 | -1.56861D+00 |
| R( 11) | 0 - 0 | 471.09 | -13.08 | 8.28819D-04 | 9.99999D-01 | -1.56888D+00 |
| R( 12) | 0 - 0 | 484.17 | -14.17 | 1.05712D-03 | 9.99999D-01 | -1.56918D+00 |
| R( 13) | 0 - 0 | 498.33 | -15.25 | 1.32396D-03 | 9.99999D-01 | -1.56950D+00 |
| R( 14) | 0 - 0 | 513.59 | -16.34 | 1.63235D-03 | 9.99999D-01 | -1.56984D+00 |
| R( 15) | 0 - 0 | 529.93 | -17.43 | 1.98530D-03 | 9.99999D-01 | -1.57021D+00 |
| R( 16) | 0 - 0 | 547.36 | -18.52 | 2.38585D-03 | 9.99999D-01 | -1.57060D+00 |
| R( 17) | 0 - 0 | 565.88 | -19.60 | 2.83702D-03 | 9.99998D-01 | -1.57102D+00 |
| R( 18) | 0 - 0 | 585.48 | -20.69 | 3.34183D-03 | 9.99998D-01 | -1.57146D+00 |

| | | | | | | | |
|---|---|---|---|---|---|---|---|
| R( 19) | 0 - 0 | 606.17 | -21.78 | 3.90333D-03 | 9.99998D-01 | -1.57192D+00 |
| P( 1) | 1 - 0 | 400.23 | -790.08 | 4.18821D+00 | 5.14014D-09 | 1.64553D-01 |
| R( 0) | 1 - 0 | 399.14 | -792.25 | 1.40371D+00 | 5.14044D-09 | 1.64325D-01 |
| P( 2) | 1 - 0 | 402.41 | -788.98 | 2.78435D+00 | 2.05605D-08 | 1.64668D-01 |
| R( 0) | 1 - 1 | 1190.31 | -1.08 | 3.39230D-07 | 1.00000D+00 | 1.60410D+00 |
| R( 1) | 1 - 0 | 400.23 | -793.32 | 1.68896D+00 | 2.05607D-08 | 1.64212D-01 |
| P( 3) | 1 - 0 | 405.68 | -787.87 | 2.49883D+00 | 4.62647D-08 | 1.64782D-01 |
| R( 1) | 1 - 1 | 1191.39 | -2.16 | 3.25661D-06 | 1.00000D+00 | 1.60413D+00 |
| R( 2) | 1 - 0 | 402.41 | -794.38 | 1.81436D+00 | 4.62631D-08 | 1.64099D-01 |
| P( 4) | 1 - 0 | 410.04 | -786.75 | 2.37301D+00 | 8.22533D-08 | 1.64897D-01 |
| R( 2) | 1 - 1 | 1193.55 | -3.24 | 1.17763D-05 | 1.00000D+00 | 1.60419D+00 |
| R( 3) | 1 - 0 | 405.68 | -795.43 | 1.88644D+00 | 8.22495D-08 | 1.63986D-01 |
| P( 5) | 1 - 0 | 415.49 | -785.62 | 2.30038D+00 | 1.28531D-07 | 1.65013D-01 |
| R( 3) | 1 - 1 | 1196.79 | -4.32 | 2.89488D-05 | 1.00000D+00 | 1.60427D+00 |
| R( 4) | 1 - 0 | 410.04 | -796.47 | 1.93423D+00 | 1.28523D-07 | 1.63874D-01 |
| P( 6) | 1 - 0 | 422.03 | -784.48 | 2.25189D+00 | 1.85101D-07 | 1.65129D-01 |
| R( 4) | 1 - 1 | 1201.11 | -5.40 | 5.78272D-05 | 1.00000D+00 | 1.60438D+00 |
| R( 5) | 1 - 0 | 415.49 | -797.50 | 1.96892D+00 | 1.85088D-07 | 1.63761D-01 |
| P( 7) | 1 - 0 | 429.67 | -783.33 | 2.21637D+00 | 2.51970D-07 | 1.65245D-01 |
| R( 5) | 1 - 1 | 1206.51 | -6.48 | 1.01466D-04 | 9.99999D-01 | 1.60451D+00 |
| R( 6) | 1 - 0 | 422.03 | -798.52 | 1.99571D+00 | 2.51949D-07 | 1.63649D-01 |
| P( 8) | 1 - 0 | 438.39 | -782.17 | 2.18861D+00 | 3.29144D-07 | 1.65361D-01 |
| R( 6) | 1 - 1 | 1212.99 | -7.56 | 1.62922D-04 | 9.99999D-01 | 1.60466D+00 |
| R( 7) | 1 - 0 | 429.67 | -799.53 | 2.01736D+00 | 3.29113D-07 | 1.63538D-01 |
| P( 9) | 1 - 0 | 448.20 | -781.00 | 2.16584D+00 | 4.16630D-07 | 1.65478D-01 |
| R( 7) | 1 - 1 | 1220.55 | -8.64 | 2.45251D-04 | 9.99999D-01 | 1.60483D+00 |
| R( 8) | 1 - 0 | 438.39 | -800.53 | 2.03548D+00 | 4.16586D-07 | 1.63426D-01 |
| P( 10) | 1 - 0 | 459.10 | -779.82 | 2.14647D+00 | 5.14437D-07 | 1.65595D-01 |
| R( 8) | 1 - 1 | 1229.20 | -9.72 | 3.51512D-04 | 9.99999D-01 | 1.60503D+00 |

| | | | | | | | |
|---|---|---|---|---|---|---|---|
| R( 9) | 1 - 0 | 448.20 | -801.52 | 2.05105D+00 | 5.14376D-07 | 1.63315D-01 |
| P( 11) | 1 - 0 | 471.09 | -778.63 | 2.12952D+00 | 6.22574D-07 | 1.65713D-01 |
| R( 9) | 1 - 1 | 1238.92 | -10.80 | 4.84766D-04 | 9.99998D-01 | 1.60525D+00 |
| R( 10) | 1 - 0 | 459.10 | -802.50 | 2.06472D+00 | 6.22493D-07 | 1.63204D-01 |
| P( 12) | 1 - 0 | 484.17 | -777.43 | 2.11432D+00 | 7.41051D-07 | 1.65831D-01 |
| R( 10) | 1 - 1 | 1249.72 | -11.88 | 6.48073D-04 | 9.99998D-01 | 1.60550D+00 |
| R( 11) | 1 - 0 | 471.09 | -803.47 | 2.07691D+00 | 7.40946D-07 | 1.63093D-01 |
| P( 13) | 1 - 0 | 498.33 | -776.22 | 2.10046D+00 | 8.69879D-07 | 1.65950D-01 |
| R( 11) | 1 - 1 | 1261.60 | -12.96 | 8.44497D-04 | 9.99998D-01 | 1.60577D+00 |
| R( 12) | 1 - 0 | 484.17 | -804.42 | 2.08795D+00 | 8.69746D-07 | 1.62983D-01 |
| P( 14) | 1 - 0 | 513.59 | -775.00 | 2.08761D+00 | 1.00907D-06 | 1.66068D-01 |
| R( 12) | 1 - 1 | 1274.55 | -14.04 | 1.07710D-03 | 9.99997D-01 | 1.60606D+00 |
| R( 13) | 1 - 0 | 498.33 | -805.37 | 2.09806D+00 | 1.00891D-06 | 1.62873D-01 |
| P( 15) | 1 - 0 | 529.93 | -773.77 | 2.07556D+00 | 1.15864D-06 | 1.66188D-01 |
| R( 13) | 1 - 1 | 1288.59 | -15.11 | 1.34896D-03 | 9.99997D-01 | 1.60637D+00 |
| R( 14) | 1 - 0 | 513.59 | -806.31 | 2.10739D+00 | 1.15844D-06 | 1.62762D-01 |
| P( 16) | 1 - 0 | 547.36 | -772.54 | 2.06415D+00 | 1.31860D-06 | 1.66307D-01 |
| R( 14) | 1 - 1 | 1303.70 | -16.19 | 1.66315D-03 | 9.99997D-01 | 1.60671D+00 |
| R( 15) | 1 - 0 | 529.93 | -807.24 | 2.11608D+00 | 1.31835D-06 | 1.62653D-01 |
| P( 17) | 1 - 0 | 565.88 | -771.29 | 2.05324D+00 | 1.48897D-06 | 1.66428D-01 |
| R( 15) | 1 - 1 | 1319.90 | -17.27 | 2.02272D-03 | 9.99996D-01 | 1.60707D+00 |
| R( 16) | 1 - 0 | 547.36 | -808.15 | 2.12422D+00 | 1.48867D-06 | 1.62543D-01 |
| P( 18) | 1 - 0 | 585.48 | -770.03 | 2.04274D+00 | 1.66975D-06 | 1.66548D-01 |
| R( 16) | 1 - 1 | 1337.17 | -18.35 | 2.43078D-03 | 9.99996D-01 | 1.60746D+00 |
| R( 17) | 1 - 0 | 565.88 | -809.06 | 2.13188D+00 | 1.66940D-06 | 1.62433D-01 |
| P( 19) | 1 - 0 | 606.17 | -768.77 | 2.03257D+00 | 1.86098D-06 | 1.66669D-01 |
| R( 17) | 1 - 1 | 1355.51 | -19.42 | 2.89038D-03 | 9.99995D-01 | 1.60786D+00 |
| R( 18) | 1 - 0 | 585.48 | -809.96 | 2.13913D+00 | 1.86056D-06 | 1.62324D-01 |
| P( 20) | 1 - 0 | 627.95 | -767.49 | 2.02268D+00 | 2.06266D-06 | 1.66790D-01 |

| | | | | | | | |
|---|---|---|---|---|---|---|---|
| R( 18) | 1 - 1 | 1374.94 | -20.50 | 3.40461D-03 | 9.99994D-01 | 1.60830D+00 |
| R( 19) | 1 - 0 | 606.17 | -810.84 | 2.14602D+00 | 2.06218D-06 | 1.62214D-01 |
| P( 21) | 1 - 0 | 650.81 | -766.20 | 2.01302D+00 | 2.27482D-06 | 1.66912D-01 |
| R( 19) | 1 - 1 | 1395.44 | -21.58 | 3.97657D-03 | 9.99994D-01 | 1.60875D+00 |
| P( 1) | 2 - 0 | 400.23 | -1572.99 | 2.19818D-01 | 1.70112D-11 | 1.34196D-02 |
| P( 1) | 2 - 1 | 1191.39 | -781.83 | 7.92135D+00 | 1.02706D-08 | -2.29893D-01 |
| R( 0) | 2 - 0 | 399.14 | -1575.16 | 7.37938D-02 | 1.70755D-11 | 1.34395D-02 |
| P( 2) | 2 - 0 | 402.41 | -1571.88 | 1.46027D-01 | 6.79181D-11 | 1.34101D-02 |
| R( 0) | 2 - 1 | 1190.31 | -783.98 | 2.65467D+00 | 1.02710D-08 | -2.29563D-01 |
| P( 2) | 2 - 1 | 1193.55 | -780.74 | 5.26642D+00 | 4.10828D-08 | -2.30059D-01 |
| R( 0) | 2 - 2 | 1973.22 | -1.07 | 3.45177D-07 | 1.00000D+00 | -1.64075D+00 |
| R( 1) | 2 - 0 | 400.23 | -1576.21 | 8.88670D-02 | 6.84038D-11 | 1.34499D-02 |
| P( 3) | 2 - 0 | 405.68 | -1570.75 | 1.30960D-01 | 1.52576D-10 | 1.34008D-02 |
| R( 1) | 2 - 1 | 1191.39 | -785.05 | 3.19397D+00 | 4.10821D-08 | -2.29399D-01 |
| P( 3) | 2 - 1 | 1196.79 | -779.64 | 4.72659D+00 | 9.24437D-08 | -2.30225D-01 |
| R( 1) | 2 - 2 | 1974.29 | -2.14 | 3.31369D-06 | 1.00000D+00 | -1.64078D+00 |
| R( 2) | 2 - 0 | 402.41 | -1577.24 | 9.55528D-02 | 1.54184D-10 | 1.34606D-02 |
| P( 4) | 2 - 0 | 410.04 | -1569.60 | 1.24283D-01 | 2.70787D-10 | 1.33918D-02 |
| R( 2) | 2 - 1 | 1193.55 | -786.10 | 3.43095D+00 | 9.24372D-08 | -2.29235D-01 |
| P( 4) | 2 - 1 | 1201.11 | -778.53 | 4.48880D+00 | 1.64355D-07 | -2.30392D-01 |
| R( 2) | 2 - 2 | 1976.43 | -3.21 | 1.19827D-05 | 1.00000D+00 | -1.64084D+00 |
| R( 3) | 2 - 0 | 405.68 | -1578.25 | 9.94438D-02 | 2.74598D-10 | 1.34715D-02 |
| P( 5) | 2 - 0 | 415.49 | -1568.43 | 1.20404D-01 | 4.22395D-10 | 1.33831D-02 |
| R( 3) | 2 - 1 | 1196.79 | -787.14 | 3.56708D+00 | 1.64340D-07 | -2.29072D-01 |
| P( 5) | 2 - 1 | 1206.51 | -777.41 | 4.35161D+00 | 2.56826D-07 | -2.30559D-01 |
| R( 3) | 2 - 2 | 1979.64 | -4.28 | 2.94560D-05 | 1.00000D+00 | -1.64092D+00 |
| R( 4) | 2 - 0 | 410.04 | -1579.24 | 1.02065D-01 | 4.29839D-10 | 1.34827D-02 |
| P( 6) | 2 - 0 | 422.03 | -1567.24 | 1.17797D-01 | 6.07238D-10 | 1.33747D-02 |
| R( 4) | 2 - 1 | 1201.11 | -788.17 | 3.65728D+00 | 2.56796D-07 | -2.28909D-01 |

| | | | | | | | |
|---|---|---|---|---|---|---|---|
| P( 6) | 2 - 1 | 1212.99 | -776.28 | 4.26008D+00 | 3.69865D-07 | -2.30727D-01 |
| R( 4) | 2 - 2 | 1983.93 | -5.35 | 5.88403D-05 | 9.99999D-01 | -1.64103D+00 |
| R( 5) | 2 - 0 | 415.49 | -1580.21 | 1.04004D-01 | 6.20103D-10 | 1.34942D-02 |
| P( 7) | 2 - 0 | 429.67 | -1566.03 | 1.15877D-01 | 8.25156D-10 | 1.33665D-02 |
| R( 5) | 2 - 1 | 1206.51 | -789.19 | 3.72269D+00 | 3.69813D-07 | -2.28746D-01 |
| P( 7) | 2 - 1 | 1220.55 | -775.14 | 4.19307D+00 | 5.03484D-07 | -2.30895D-01 |
| R( 5) | 2 - 2 | 1989.28 | -6.42 | 1.03243D-04 | 9.99999D-01 | -1.64116D+00 |
| R( 6) | 2 - 0 | 422.03 | -1581.16 | 1.05533D-01 | 8.45588D-10 | 1.35060D-02 |
| P( 8) | 2 - 0 | 438.39 | -1564.80 | 1.14368D-01 | 1.07599D-09 | 1.33586D-02 |
| R( 6) | 2 - 1 | 1212.99 | -790.20 | 3.77316D+00 | 5.03400D-07 | -2.28584D-01 |
| P( 8) | 2 - 1 | 1229.20 | -773.99 | 4.14073D+00 | 6.57695D-07 | -2.31064D-01 |
| R( 6) | 2 - 2 | 1995.70 | -7.49 | 1.65774D-04 | 9.99999D-01 | -1.64131D+00 |
| R( 7) | 2 - 0 | 429.67 | -1582.09 | 1.06798D-01 | 1.10650D-09 | 1.35181D-02 |
| P( 9) | 2 - 0 | 448.20 | -1563.55 | 1.13127D-01 | 1.35960D-09 | 1.33510D-02 |
| R( 7) | 2 - 1 | 1220.55 | -791.20 | 3.81392D+00 | 6.57571D-07 | -2.28422D-01 |
| P( 9) | 2 - 1 | 1238.92 | -772.84 | 4.09784D+00 | 8.32514D-07 | -2.31233D-01 |
| R( 7) | 2 - 2 | 2003.19 | -8.56 | 2.49543D-04 | 9.99998D-01 | -1.64149D+00 |
| R( 8) | 2 - 0 | 438.39 | -1583.00 | 1.07883D-01 | 1.40305D-09 | 1.35304D-02 |
| P( 10) | 2 - 0 | 459.10 | -1562.28 | 1.12068D-01 | 1.67583D-09 | 1.33437D-02 |
| R( 8) | 2 - 1 | 1229.20 | -792.19 | 3.84799D+00 | 8.32338D-07 | -2.28260D-01 |
| P( 10) | 2 - 1 | 1249.72 | -771.67 | 4.06137D+00 | 1.02796D-06 | -2.31402D-01 |
| R( 8) | 2 - 2 | 2011.75 | -9.63 | 3.57662D-04 | 9.99998D-01 | -1.64168D+00 |
| R( 9) | 2 - 0 | 448.20 | -1583.88 | 1.08839D-01 | 1.73544D-09 | 1.35430D-02 |
| P( 11) | 2 - 0 | 471.09 | -1561.00 | 1.11142D-01 | 2.02453D-09 | 1.33367D-02 |
| R( 9) | 2 - 1 | 1238.92 | -793.17 | 3.87723D+00 | 1.02772D-06 | -2.28099D-01 |
| P( 11) | 2 - 1 | 1261.60 | -770.49 | 4.02946D+00 | 1.24405D-06 | -2.31573D-01 |
| R( 9) | 2 - 2 | 2021.38 | -10.70 | 4.93242D-04 | 9.99997D-01 | -1.64191D+00 |
| R( 10) | 2 - 0 | 459.10 | -1584.75 | 1.09701D-01 | 2.10389D-09 | 1.35559D-02 |
| P( 12) | 2 - 0 | 484.17 | -1559.69 | 1.10312D-01 | 2.40557D-09 | 1.33299D-02 |

| | | | | | | | |
|---|---|---|---|---|---|---|---|
| R( 10) | 2 - 1 | 1249.72 | -794.14 | 3.90287D+00 | 1.24372D-06 | -2.27938D-01 |
| P( 12) | 2 - 1 | 1274.55 | -769.30 | 4.00089D+00 | 1.48080D-06 | -2.31744D-01 |
| R( 10) | 2 - 2 | 2032.08 | -11.77 | 6.59398D-04 | 9.99997D-01 | -1.64215D+00 |
| R( 11) | 2 - 0 | 471.09 | -1585.60 | 1.10491D-01 | 2.50862D-09 | 1.35691D-02 |
| P( 13) | 2 - 0 | 498.33 | -1558.36 | 1.09557D-01 | 2.81880D-09 | 1.33234D-02 |
| R( 11) | 2 - 1 | 1261.60 | -795.09 | 3.92574D+00 | 1.48038D-06 | -2.27777D-01 |
| P( 13) | 2 - 1 | 1288.59 | -768.10 | 3.97483D+00 | 1.73824D-06 | -2.31915D-01 |
| R( 11) | 2 - 2 | 2043.85 | -12.84 | 8.59246D-04 | 9.99996D-01 | -1.64242D+00 |
| R( 12) | 2 - 0 | 484.17 | -1586.43 | 1.11226D-01 | 2.94986D-09 | 1.35825D-02 |
| P( 14) | 2 - 0 | 513.59 | -1557.01 | 1.08860D-01 | 3.26409D-09 | 1.33172D-02 |
| R( 12) | 2 - 1 | 1274.55 | -796.04 | 3.94641D+00 | 1.73770D-06 | -2.27617D-01 |
| P( 14) | 2 - 1 | 1303.70 | -766.89 | 3.95069D+00 | 2.01639D-06 | -2.32087D-01 |
| R( 12) | 2 - 2 | 2056.69 | -13.91 | 1.09590D-03 | 9.99996D-01 | -1.64271D+00 |
| R( 13) | 2 - 0 | 498.33 | -1587.24 | 1.11917D-01 | 3.42784D-09 | 1.35962D-02 |
| P( 15) | 2 - 0 | 529.93 | -1555.64 | 1.08209D-01 | 3.74131D-09 | 1.33113D-02 |
| R( 13) | 2 - 1 | 1288.59 | -796.98 | 3.96531D+00 | 2.01572D-06 | -2.27457D-01 |
| P( 15) | 2 - 1 | 1319.90 | -765.68 | 3.92805D+00 | 2.31528D-06 | -2.32260D-01 |
| R( 13) | 2 - 2 | 2070.60 | -14.97 | 1.37249D-03 | 9.99995D-01 | -1.64303D+00 |
| R( 14) | 2 - 0 | 513.59 | -1588.03 | 1.12574D-01 | 3.94279D-09 | 1.36102D-02 |
| P( 16) | 2 - 0 | 547.36 | -1554.25 | 1.07596D-01 | 4.25033D-09 | 1.33056D-02 |
| R( 14) | 2 - 1 | 1303.70 | -797.91 | 3.98275D+00 | 2.31446D-06 | -2.27297D-01 |
| P( 16) | 2 - 1 | 1337.17 | -764.45 | 3.90661D+00 | 2.63493D-06 | -2.32433D-01 |
| R( 14) | 2 - 2 | 2085.57 | -16.04 | 1.69213D-03 | 9.99994D-01 | -1.64337D+00 |
| R( 15) | 2 - 0 | 529.93 | -1588.80 | 1.13202D-01 | 4.49494D-09 | 1.36245D-02 |
| P( 17) | 2 - 0 | 565.88 | -1552.85 | 1.07014D-01 | 4.79102D-09 | 1.33002D-02 |
| R( 15) | 2 - 1 | 1319.90 | -798.83 | 3.99897D+00 | 2.63394D-06 | -2.27138D-01 |
| P( 17) | 2 - 1 | 1355.51 | -763.21 | 3.88613D+00 | 2.97539D-06 | -2.32607D-01 |
| R( 15) | 2 - 2 | 2101.61 | -17.11 | 2.05795D-03 | 9.99993D-01 | -1.64373D+00 |
| R( 16) | 2 - 0 | 547.36 | -1589.54 | 1.13806D-01 | 5.08453D-09 | 1.36390D-02 |

| | | | | | | | |
|---|---|---|---|---|---|---|---|
| P( 18) | 2 - 0 | 585.48 | -1551.42 | 1.06458D-01 | 5.36327D-09 | 1.32951D-02 |
| R( 16) | 2 - 1 | 1337.17 | -799.74 | 4.01415D+00 | 2.97419D-06 | -2.26979D-01 |
| P( 18) | 2 - 1 | 1374.94 | -761.97 | 3.86641D+00 | 3.33667D-06 | -2.32781D-01 |
| R( 16) | 2 - 2 | 2118.72 | -18.18 | 2.47307D-03 | 9.99992D-01 | -1.64412D+00 |
| R( 17) | 2 - 0 | 565.88 | -1590.27 | 1.14392D-01 | 5.71183D-09 | 1.36539D-02 |
| P( 19) | 2 - 0 | 606.17 | -1549.97 | 1.05924D-01 | 5.96694D-09 | 1.32903D-02 |
| R( 17) | 2 - 1 | 1355.51 | -800.63 | 4.02843D+00 | 3.33525D-06 | -2.26820D-01 |
| P( 19) | 2 - 1 | 1395.44 | -760.71 | 3.84733D+00 | 3.71882D-06 | -2.32956D-01 |
| R( 17) | 2 - 2 | 2136.90 | -19.24 | 2.94062D-03 | 9.99992D-01 | -1.64453D+00 |
| R( 18) | 2 - 0 | 585.48 | -1590.98 | 1.14961D-01 | 6.37706D-09 | 1.36689D-02 |
| P( 20) | 2 - 0 | 627.95 | -1548.51 | 1.05409D-01 | 6.60193D-09 | 1.32857D-02 |
| R( 18) | 2 - 1 | 1374.94 | -801.52 | 4.04192D+00 | 3.71715D-06 | -2.26661D-01 |
| P( 20) | 2 - 1 | 1417.01 | -759.44 | 3.82877D+00 | 4.12187D-06 | -2.33132D-01 |
| R( 18) | 2 - 2 | 2156.15 | -20.31 | 3.46374D-03 | 9.99991D-01 | -1.64496D+00 |
| R( 19) | 2 - 0 | 606.17 | -1591.66 | 1.15517D-01 | 7.08050D-09 | 1.36843D-02 |
| P( 21) | 2 - 0 | 650.81 | -1547.02 | 1.04910D-01 | 7.26813D-09 | 1.32814D-02 |
| R( 19) | 2 - 1 | 1395.44 | -802.40 | 4.05472D+00 | 4.11992D-06 | -2.26503D-01 |
| P( 21) | 2 - 1 | 1439.66 | -758.17 | 3.81063D+00 | 4.54586D-06 | -2.33308D-01 |
| R( 19) | 2 - 2 | 2176.46 | -21.38 | 4.04556D-03 | 9.99990D-01 | -1.64542D+00 |
| P( 1) | 3 - 0 | 400.23 | -2345.37 | 1.99495D-03 | 1.86171D-13 | 7.02181D-04 |
| P( 1) | 3 - 1 | 1191.39 | -1554.21 | 6.23586D-01 | 5.10363D-11 | -2.30136D-02 |
| P( 1) | 3 - 2 | 1974.29 | -771.30 | 1.11894D+01 | 1.55149D-08 | 2.78847D-01 |
| R( 0) | 3 - 0 | 399.14 | -2347.52 | 6.75026D-04 | 1.87193D-13 | 7.06491D-04 |
| P( 2) | 3 - 0 | 402.41 | -2344.25 | 1.32059D-03 | 7.42599D-13 | 7.00202D-04 |
| R( 0) | 3 - 1 | 1190.31 | -1556.35 | 2.09329D-01 | 5.12266D-11 | -2.30470D-02 |
| P( 2) | 3 - 1 | 1193.55 | -1553.11 | 4.14266D-01 | 2.03773D-10 | -2.29976D-02 |
| R( 0) | 3 - 2 | 1973.22 | -773.43 | 3.74960D+00 | 1.55152D-08 | 2.78431D-01 |
| P( 2) | 3 - 2 | 1976.43 | -770.22 | 7.43941D+00 | 6.20606D-08 | 2.79056D-01 |
| R( 0) | 3 - 3 | 2745.59 | -1.06 | 3.50694D-07 | 1.00000D+00 | 1.67836D+00 |

| | | | | | | |
|---|---|---|---|---|---|---|
| R( 1) | 3 - 0 | 400.23 | -2348.55 | 8.16457D-04 | 7.49918D-13 | 7.08822D-04 |
| P( 3) | 3 - 0 | 405.68 | -2343.09 | 1.18047D-03 | 1.66773D-12 | 6.98340D-04 |
| R( 1) | 3 - 1 | 1191.39 | -1557.39 | 2.52081D-01 | 2.05223D-10 | -2.30645D-02 |
| P( 3) | 3 - 1 | 1196.79 | -1551.98 | 3.71532D-01 | 4.57769D-10 | -2.29821D-02 |
| R( 1) | 3 - 2 | 1974.29 | -774.48 | 4.51114D+00 | 6.20579D-08 | 2.78224D-01 |
| P( 3) | 3 - 2 | 1979.64 | -769.13 | 6.67705D+00 | 1.39649D-07 | 2.79265D-01 |
| R( 1) | 3 - 3 | 2746.65 | -2.12 | 3.36665D-06 | 1.00000D+00 | 1.67840D+00 |
| R( 2) | 3 - 0 | 402.41 | -2349.55 | 8.81953D-04 | 1.69140D-12 | 7.11269D-04 |
| P( 4) | 3 - 0 | 410.04 | -2341.91 | 1.11696D-03 | 2.95809D-12 | 6.96594D-04 |
| R( 2) | 3 - 1 | 1193.55 | -1558.41 | 2.71039D-01 | 4.62583D-10 | -2.30825D-02 |
| P( 4) | 3 - 1 | 1201.11 | -1550.84 | 3.52600D-01 | 8.12459D-10 | -2.29672D-02 |
| R( 2) | 3 - 2 | 1976.43 | -775.52 | 4.84564D+00 | 1.39634D-07 | 2.78018D-01 |
| P( 4) | 3 - 2 | 1983.93 | -768.03 | 6.34132D+00 | 2.48284D-07 | 2.79474D-01 |
| R( 2) | 3 - 3 | 2748.77 | -3.18 | 1.21742D-05 | 1.00000D+00 | 1.67846D+00 |
| R( 3) | 3 - 0 | 405.68 | -2350.51 | 9.22367D-04 | 3.01428D-12 | 7.13835D-04 |
| P( 5) | 3 - 0 | 415.49 | -2340.70 | 1.07918D-03 | 4.61156D-12 | 6.94965D-04 |
| R( 3) | 3 - 1 | 1196.79 | -1559.40 | 2.82069D-01 | 8.23871D-10 | -2.31010D-02 |
| P( 5) | 3 - 1 | 1206.51 | -1549.68 | 3.41604D-01 | 1.26738D-09 | -2.29527D-02 |
| R( 3) | 3 - 2 | 1979.64 | -776.55 | 5.03765D+00 | 2.48249D-07 | 2.77812D-01 |
| P( 5) | 3 - 2 | 1989.28 | -766.92 | 6.14767D+00 | 3.87981D-07 | 2.79685D-01 |
| R( 3) | 3 - 3 | 2751.95 | -4.24 | 2.99266D-05 | 9.99999D-01 | 1.67854D+00 |
| R( 4) | 3 - 0 | 410.04 | -2351.45 | 9.51574D-04 | 4.72140D-12 | 7.16518D-04 |
| P( 6) | 3 - 0 | 422.03 | -2339.46 | 1.05327D-03 | 6.62579D-12 | 6.93452D-04 |
| R( 4) | 3 - 1 | 1201.11 | -1560.38 | 2.89498D-01 | 1.28968D-09 | -2.31199D-02 |
| P( 6) | 3 - 1 | 1212.99 | -1548.50 | 3.34219D-01 | 1.82208D-09 | -2.29387D-02 |
| R( 4) | 3 - 2 | 1983.93 | -777.57 | 5.16477D+00 | 3.87912D-07 | 2.77606D-01 |
| P( 6) | 3 - 2 | 1995.70 | -765.79 | 6.01850D+00 | 5.58756D-07 | 2.79896D-01 |
| R( 4) | 3 - 3 | 2756.19 | -5.30 | 5.97800D-05 | 9.99999D-01 | 1.67864D+00 |
| R( 5) | 3 - 0 | 415.49 | -2352.36 | 9.74910D-04 | 6.81567D-12 | 7.19320D-04 |

| | | | | | | | |
|---|---|---|---|---|---|---|---|
| P( 7) | 3 - 0 | 429.67 | -2338.19 | 1.03390D-03 | 8.99845D-12 | 6.92056D-04 |
| R( 5) | 3 - 1 | 1206.51 | -1561.34 | 2.94989D-01 | 1.86061D-09 | -2.31394D-02 |
| P( 7) | 3 - 1 | 1220.55 | -1547.30 | 3.28780D-01 | 2.47610D-09 | -2.29252D-02 |
| R( 5) | 3 - 2 | 1989.28 | -778.57 | 5.25685D+00 | 5.58636D-07 | 2.77401D-01 |
| P( 7) | 3 - 2 | 2003.19 | -764.66 | 5.92395D+00 | 7.60629D-07 | 2.80107D-01 |
| R( 5) | 3 - 3 | 2761.49 | -6.36 | 1.04892D-04 | 9.99999D-01 | 1.67877D+00 |
| R( 6) | 3 - 0 | 422.03 | -2353.24 | 9.94872D-04 | 9.30010D-12 | 7.22239D-04 |
| P( 8) | 3 - 0 | 438.39 | -2336.88 | 1.01856D-03 | 1.17273D-11 | 6.90777D-04 |
| R( 6) | 3 - 1 | 1212.99 | -1562.28 | 2.99320D-01 | 2.53729D-09 | -2.31594D-02 |
| P( 8) | 3 - 1 | 1229.20 | -1546.07 | 3.24510D-01 | 3.22900D-09 | -2.29123D-02 |
| R( 6) | 3 - 2 | 1995.70 | -779.57 | 5.32783D+00 | 7.60438D-07 | 2.77196D-01 |
| P( 8) | 3 - 2 | 2011.75 | -763.52 | 5.85011D+00 | 9.93622D-07 | 2.80319D-01 |
| R( 6) | 3 - 3 | 2767.85 | -7.42 | 1.68420D-04 | 9.99998D-01 | 1.67892D+00 |
| R( 7) | 3 - 0 | 429.67 | -2354.08 | 1.01278D-03 | 1.21777D-11 | 7.25277D-04 |
| P( 9) | 3 - 0 | 448.20 | -2335.55 | 1.00595D-03 | 1.48101D-11 | 6.89614D-04 |
| R( 7) | 3 - 1 | 1220.55 | -1563.19 | 3.02902D-01 | 3.32036D-09 | -2.31799D-02 |
| P( 9) | 3 - 1 | 1238.92 | -1544.83 | 3.20998D-01 | 4.08037D-09 | -2.28998D-02 |
| R( 7) | 3 - 2 | 2003.19 | -780.56 | 5.38506D+00 | 9.93337D-07 | 2.76992D-01 |
| P( 9) | 3 - 2 | 2021.38 | -762.36 | 5.78959D+00 | 1.25776D-06 | 2.80532D-01 |
| R( 7) | 3 - 3 | 2775.27 | -8.48 | 2.53524D-04 | 9.99998D-01 | 1.67910D+00 |
| R( 8) | 3 - 0 | 438.39 | -2354.90 | 1.02941D-03 | 1.54516D-11 | 7.28433D-04 |
| P( 10) | 3 - 0 | 459.10 | -2334.19 | 9.95286D-04 | 1.82447D-11 | 6.88567D-04 |
| R( 8) | 3 - 1 | 1229.20 | -1564.09 | 3.05972D-01 | 4.21048D-09 | -2.32008D-02 |
| P( 10) | 3 - 1 | 1249.72 | -1543.57 | 3.18006D-01 | 5.02980D-09 | -2.28879D-02 |
| R( 8) | 3 - 2 | 2011.75 | -781.53 | 5.43282D+00 | 1.25736D-06 | 2.76788D-01 |
| P( 10) | 3 - 2 | 2032.08 | -761.20 | 5.73814D+00 | 1.55308D-06 | 2.80745D-01 |
| R( 8) | 3 - 3 | 2783.75 | -9.54 | 3.63363D-04 | 9.99997D-01 | 1.67930D+00 |
| R( 9) | 3 - 0 | 448.20 | -2355.68 | 1.04522D-03 | 1.91251D-11 | 7.31709D-04 |
| P( 11) | 3 - 0 | 471.09 | -2332.79 | 9.86103D-04 | 2.20290D-11 | 6.87637D-04 |

| | | | | | | | |
|---|---|---|---|---|---|---|---|
| R( 9) | 3 - 1 | 1238.92 | -1564.96 | 3.08679D-01 | 5.20833D-09 | -2.32223D-02 |
| P( 11) | 3 - 1 | 1261.60 | -1542.28 | 3.15387D-01 | 6.07689D-09 | -2.28764D-02 |
| R( 9) | 3 - 2 | 2021.38 | -782.50 | 5.47375D+00 | 1.55252D-06 | 2.76584D-01 |
| P( 11) | 3 - 2 | 2043.85 | -760.03 | 5.69310D+00 | 1.87960D-06 | 2.80959D-01 |
| R( 9) | 3 - 3 | 2793.28 | -10.60 | 5.01099D-04 | 9.99996D-01 | 1.67952D+00 |
| R( 10) | 3 - 0 | 459.10 | -2356.44 | 1.06055D-03 | 2.32012D-11 | 7.35103D-04 |
| P( 12) | 3 - 0 | 484.17 | -2331.37 | 9.78089D-04 | 2.61610D-11 | 6.86823D-04 |
| R( 10) | 3 - 1 | 1249.72 | -1565.82 | 3.11117D-01 | 6.31460D-09 | -2.32443D-02 |
| P( 12) | 3 - 1 | 1274.55 | -1540.98 | 3.13045D-01 | 7.22129D-09 | -2.28655D-02 |
| R( 10) | 3 - 2 | 2032.08 | -783.45 | 5.50958D+00 | 1.87886D-06 | 2.76381D-01 |
| P( 12) | 3 - 2 | 2056.69 | -758.84 | 5.65277D+00 | 2.23737D-06 | 2.81174D-01 |
| R( 10) | 3 - 3 | 2803.88 | -11.65 | 6.69895D-04 | 9.99996D-01 | 1.67977D+00 |
| R( 11) | 3 - 0 | 471.09 | -2357.16 | 1.07560D-03 | 2.76834D-11 | 7.38618D-04 |
| P( 13) | 3 - 0 | 498.33 | -2329.91 | 9.71031D-04 | 3.06386D-11 | 6.86126D-04 |
| R( 11) | 3 - 1 | 1261.60 | -1566.65 | 3.13353D-01 | 7.52999D-09 | -2.32668D-02 |
| P( 13) | 3 - 1 | 1288.59 | -1539.66 | 3.10914D-01 | 8.46262D-09 | -2.28550D-02 |
| R( 11) | 3 - 2 | 2043.85 | -784.39 | 5.54146D+00 | 2.23641D-06 | 2.76178D-01 |
| P( 13) | 3 - 2 | 2070.60 | -757.65 | 5.61596D+00 | 2.62642D-06 | 2.81389D-01 |
| R( 11) | 3 - 3 | 2815.53 | -12.71 | 8.72914D-04 | 9.99995D-01 | 1.68004D+00 |
| R( 12) | 3 - 0 | 484.17 | -2357.85 | 1.09052D-03 | 3.25751D-11 | 7.42251D-04 |
| P( 14) | 3 - 0 | 513.59 | -2328.43 | 9.64779D-04 | 3.54600D-11 | 6.85545D-04 |
| R( 12) | 3 - 1 | 1274.55 | -1567.46 | 3.15432D-01 | 8.85525D-09 | -2.32898D-02 |
| P( 14) | 3 - 1 | 1303.70 | -1538.31 | 3.08949D-01 | 9.80053D-09 | -2.28451D-02 |
| R( 12) | 3 - 2 | 2056.69 | -785.33 | 5.57023D+00 | 2.62519D-06 | 2.75975D-01 |
| P( 14) | 3 - 2 | 2085.57 | -756.44 | 5.58186D+00 | 3.04679D-06 | 2.81605D-01 |
| R( 12) | 3 - 3 | 2828.25 | -13.77 | 1.11332D-03 | 9.99994D-01 | 1.68033D+00 |
| R( 13) | 3 - 0 | 498.33 | -2358.51 | 1.10543D-03 | 3.78796D-11 | 7.46005D-04 |
| P( 15) | 3 - 0 | 529.93 | -2326.92 | 9.59225D-04 | 4.06232D-11 | 6.85081D-04 |
| R( 13) | 3 - 1 | 1288.59 | -1568.26 | 3.17388D-01 | 1.02911D-08 | -2.33133D-02 |

| | | | | | | | |
|---|---|---|---|---|---|---|---|
| P( 15) | 3 - 1 | 1319.90 | -1536.95 | 3.07115D-01 | 1.12347D-08 | -2.28357D-02 |
| R( 13) | 3 - 2 | 2070.60 | -786.25 | 5.59647D+00 | 3.04527D-06 | 2.75773D-01 |
| P( 15) | 3 - 2 | 2101.61 | -755.23 | 5.54986D+00 | 3.49854D-06 | 2.81821D-01 |
| R( 13) | 3 - 3 | 2842.02 | -14.83 | 1.39429D-03 | 9.99993D-01 | 1.68064D+00 |
| R( 14) | 3 - 0 | 513.59 | -2359.14 | 1.12041D-03 | 4.36006D-11 | 7.49879D-04 |
| P( 16) | 3 - 0 | 547.36 | -2325.37 | 9.54288D-04 | 4.61264D-11 | 6.84733D-04 |
| R( 14) | 3 - 1 | 1303.70 | -1569.03 | 3.19245D-01 | 1.18383D-08 | -2.33373D-02 |
| P( 16) | 3 - 1 | 1337.17 | -1535.56 | 3.05389D-01 | 1.27648D-08 | -2.28268D-02 |
| R( 14) | 3 - 2 | 2085.57 | -787.16 | 5.62064D+00 | 3.49666D-06 | 2.75571D-01 |
| P( 16) | 3 - 2 | 2118.72 | -754.01 | 5.51953D+00 | 3.98171D-06 | 2.82039D-01 |
| R( 14) | 3 - 3 | 2856.84 | -15.89 | 1.71898D-03 | 9.99992D-01 | 1.68098D+00 |
| R( 15) | 3 - 0 | 529.93 | -2359.74 | 1.13553D-03 | 4.97416D-11 | 7.53874D-04 |
| P( 17) | 3 - 0 | 565.88 | -2323.80 | 9.49905D-04 | 5.19677D-11 | 6.84501D-04 |
| R( 15) | 3 - 1 | 1319.90 | -1569.78 | 3.21023D-01 | 1.34977D-08 | -2.33618D-02 |
| P( 17) | 3 - 1 | 1355.51 | -1534.16 | 3.03752D-01 | 1.43906D-08 | -2.28184D-02 |
| R( 15) | 3 - 2 | 2101.61 | -788.06 | 5.64306D+00 | 3.97943D-06 | 2.75369D-01 |
| P( 17) | 3 - 2 | 2136.90 | -752.77 | 5.49054D+00 | 4.49635D-06 | 2.82257D-01 |
| R( 15) | 3 - 3 | 2872.73 | -16.94 | 2.09056D-03 | 9.99991D-01 | 1.68135D+00 |
| R( 16) | 3 - 0 | 547.36 | -2360.31 | 1.15085D-03 | 5.63063D-11 | 7.57990D-04 |
| P( 18) | 3 - 0 | 585.48 | -2322.19 | 9.46028D-04 | 5.81455D-11 | 6.84387D-04 |
| R( 16) | 3 - 1 | 1337.17 | -1570.51 | 3.22735D-01 | 1.52701D-08 | -2.33869D-02 |
| P( 18) | 3 - 1 | 1374.94 | -1532.74 | 3.02189D-01 | 1.61117D-08 | -2.28105D-02 |
| R( 16) | 3 - 2 | 2118.72 | -788.95 | 5.66400D+00 | 4.49361D-06 | 2.75168D-01 |
| P( 18) | 3 - 2 | 2156.15 | -751.53 | 5.46263D+00 | 5.04252D-06 | 2.82476D-01 |
| R( 16) | 3 - 3 | 2889.67 | -18.00 | 2.51221D-03 | 9.99989D-01 | 1.68173D+00 |
| R( 17) | 3 - 0 | 565.88 | -2360.85 | 1.16640D-03 | 6.32984D-11 | 7.62227D-04 |
| P( 19) | 3 - 0 | 606.17 | -2320.56 | 9.42619D-04 | 6.46579D-11 | 6.84389D-04 |
| R( 17) | 3 - 1 | 1355.51 | -1571.21 | 3.24393D-01 | 1.71563D-08 | -2.34124D-02 |
| P( 19) | 3 - 1 | 1395.44 | -1531.29 | 3.00689D-01 | 1.79279D-08 | -2.28031D-02 |

| | | | | | | | |
|---|---|---|---|---|---|---|---|
| R( 17) | 3 - 2 | 2136.90 | -789.83 | 5.68364D+00 | 5.03927D-06 | 2.74967D-01 |
| P( 19) | 3 - 2 | 2176.46 | -750.27 | 5.43559D+00 | 5.62028D-06 | 2.82695D-01 |
| R( 17) | 3 - 3 | 2907.67 | -19.06 | 2.98711D-03 | 9.99988D-01 | 1.68214D+00 |
| R( 18) | 3 - 0 | 585.48 | -2361.36 | 1.18222D-03 | 7.07217D-11 | 7.66586D-04 |
| P( 20) | 3 - 0 | 627.95 | -2318.89 | 9.39648D-04 | 7.15034D-11 | 6.84507D-04 |
| R( 18) | 3 - 1 | 1374.94 | -1571.90 | 3.26006D-01 | 1.91570D-08 | -2.34385D-02 |
| P( 20) | 3 - 1 | 1417.01 | -1529.83 | 2.99243D-01 | 1.98389D-08 | -2.27963D-02 |
| R( 18) | 3 - 2 | 2156.15 | -790.69 | 5.70216D+00 | 5.61645D-06 | 2.74765D-01 |
| P( 20) | 3 - 2 | 2197.83 | -749.01 | 5.40926D+00 | 6.22969D-06 | 2.82915D-01 |
| R( 18) | 3 - 3 | 2926.73 | -20.11 | 3.51843D-03 | 9.99987D-01 | 1.68257D+00 |
| R( 19) | 3 - 0 | 606.17 | -2361.83 | 1.19834D-03 | 7.85801D-11 | 7.71067D-04 |
| P( 21) | 3 - 0 | 650.81 | -2317.20 | 9.37090D-04 | 7.86803D-11 | 6.84743D-04 |
| R( 19) | 3 - 1 | 1395.44 | -1572.57 | 3.27582D-01 | 2.12733D-08 | -2.34650D-02 |
| P( 21) | 3 - 1 | 1439.66 | -1528.34 | 2.97843D-01 | 2.18445D-08 | -2.27900D-02 |
| R( 19) | 3 - 2 | 2176.46 | -791.55 | 5.71967D+00 | 6.22522D-06 | 2.74565D-01 |
| P( 21) | 3 - 2 | 2220.27 | -747.73 | 5.38353D+00 | 6.87082D-06 | 2.83136D-01 |
| R( 19) | 3 - 3 | 2946.84 | -21.17 | 4.10936D-03 | 9.99985D-01 | 1.68303D+00 |
| P( 1) | 4 - 0 | 400.23 | -3106.17 | 7.37198D-04 | 3.79188D-15 | -2.80061D-04 |
| P( 1) | 4 - 1 | 1191.39 | -2315.01 | 1.00820D-02 | 7.23979D-13 | -1.60969D-03 |
| P( 1) | 4 - 2 | 1974.29 | -1532.11 | 1.24195D+00 | 1.04897D-10 | 3.31831D-02 |
| P( 1) | 4 - 3 | 2746.65 | -759.75 | 1.39435D+01 | 2.08923D-08 | -3.18407D-01 |
| R( 0) | 4 - 0 | 399.14 | -3108.31 | 2.45212D-04 | 3.82269D-15 | -2.79475D-04 |
| P( 2) | 4 - 0 | 402.41 | -3105.04 | 4.91902D-04 | 1.51108D-14 | -2.80338D-04 |
| R( 0) | 4 - 1 | 1190.31 | -2317.14 | 3.40611D-03 | 7.28009D-13 | -1.61830D-03 |
| P( 2) | 4 - 1 | 1193.55 | -2313.90 | 6.67724D-03 | 2.88797D-12 | -1.60556D-03 |
| R( 0) | 4 - 2 | 1973.22 | -1534.23 | 4.16847D-01 | 1.05281D-10 | 3.32287D-02 |
| P( 2) | 4 - 2 | 1976.43 | -1531.02 | 8.25124D-01 | 4.18836D-10 | 3.31615D-02 |
| R( 0) | 4 - 3 | 2745.59 | -761.86 | 4.67212D+00 | 2.08923D-08 | -3.17913D-01 |
| P( 2) | 4 - 3 | 2748.77 | -758.68 | 9.27085D+00 | 8.35712D-08 | -3.18654D-01 |

| | | | | | | |
|---|---|---|---|---|---|---|
| R( 0) | 4 - 4 | 3506.40 | -1.05 | 3.55341D-07 | 1.00000D+00 | -1.71545D+00 |
| R( 1) | 4 - 0 | 400.23 | -3109.32 | 2.93890D-04 | 1.52938D-14 | -2.79167D-04 |
| P( 3) | 4 - 0 | 405.68 | -3103.87 | 4.43053D-04 | 3.39563D-14 | -2.80605D-04 |
| R( 1) | 4 - 1 | 1191.39 | -2318.16 | 4.11543D-03 | 2.91693D-12 | -1.62279D-03 |
| P( 3) | 4 - 1 | 1196.79 | -2312.76 | 5.97063D-03 | 6.48516D-12 | -1.60154D-03 |
| R( 1) | 4 - 2 | 1974.29 | -1535.26 | 5.01949D-01 | 4.21781D-10 | 3.32528D-02 |
| P( 3) | 4 - 2 | 1979.64 | -1529.90 | 7.40069D-01 | 9.40916D-10 | 3.31408D-02 |
| R( 1) | 4 - 3 | 2746.65 | -762.89 | 5.62077D+00 | 8.35653D-08 | -3.17666D-01 |
| P( 3) | 4 - 3 | 2751.95 | -757.59 | 8.32107D+00 | 1.88053D-07 | -3.18902D-01 |
| R( 1) | 4 - 4 | 3507.45 | -2.10 | 3.41125D-06 | 1.00000D+00 | -1.71549D+00 |
| R( 2) | 4 - 0 | 402.41 | -3110.29 | 3.14456D-04 | 3.45067D-14 | -2.78847D-04 |
| P( 4) | 4 - 0 | 410.04 | -3102.65 | 4.22232D-04 | 6.02184D-14 | -2.80862D-04 |
| R( 2) | 4 - 1 | 1193.55 | -2319.15 | 4.44008D-03 | 6.57923D-12 | -1.62738D-03 |
| P( 4) | 4 - 1 | 1201.11 | -2311.58 | 5.65003D-03 | 1.15024D-11 | -1.59764D-03 |
| R( 2) | 4 - 2 | 1976.43 | -1536.26 | 5.39669D-01 | 9.50709D-10 | 3.32777D-02 |
| P( 4) | 4 - 2 | 1983.93 | -1528.77 | 7.02418D-01 | 1.67001D-09 | 3.31209D-02 |
| R( 2) | 4 - 3 | 2748.77 | -763.92 | 6.03724D+00 | 1.88026D-07 | -3.17419D-01 |
| P( 4) | 4 - 3 | 2756.19 | -756.50 | 7.90289D+00 | 3.34346D-07 | -3.19151D-01 |
| R( 2) | 4 - 4 | 3509.55 | -3.15 | 1.23354D-05 | 1.00000D+00 | -1.71555D+00 |
| R( 3) | 4 - 0 | 405.68 | -3111.21 | 3.25622D-04 | 6.15197D-14 | -2.78518D-04 |
| P( 5) | 4 - 0 | 415.49 | -3101.40 | 4.10725D-04 | 9.38647D-14 | -2.81108D-04 |
| R( 3) | 4 - 1 | 1196.79 | -2320.10 | 4.63698D-03 | 1.17254D-11 | -1.63210D-03 |
| P( 5) | 4 - 1 | 1206.51 | -2310.38 | 5.45853D-03 | 1.79312D-11 | -1.59385D-03 |
| R( 3) | 4 - 2 | 1979.64 | -1537.25 | 5.61603D-01 | 1.69323D-09 | 3.33034D-02 |
| P( 5) | 4 - 2 | 1989.28 | -1527.61 | 6.80578D-01 | 2.60520D-09 | 3.31019D-02 |
| R( 3) | 4 - 3 | 2751.95 | -764.94 | 6.27613D+00 | 3.34282D-07 | -3.17173D-01 |
| P( 5) | 4 - 3 | 2761.49 | -755.40 | 7.66174D+00 | 5.22472D-07 | -3.19399D-01 |
| R( 3) | 4 - 4 | 3512.70 | -4.20 | 3.03228D-05 | 9.99999D-01 | -1.71563D+00 |
| R( 4) | 4 - 0 | 410.04 | -3112.10 | 3.32492D-04 | 9.64037D-14 | -2.78177D-04 |

| | | | | | | |
|---|---|---|---|---|---|---|
| P( 6) | 4 - 0 | 422.03 | -3100.10 | 4.03427D-04 | 1.34847D-13 | -2.81344D-04 |
| R( 4) | 4 - 1 | 1201.11 | -2321.03 | 4.77620D-03 | 1.83668D-11 | -1.63693D-03 |
| P( 6) | 4 - 1 | 1212.99 | -2309.14 | 5.32606D-03 | 2.57621D-11 | -1.59018D-03 |
| R( 4) | 4 - 2 | 1983.93 | -1538.21 | 5.76367D-01 | 2.65055D-09 | 3.33300D-02 |
| P( 6) | 4 - 2 | 1995.70 | -1526.44 | 6.65929D-01 | 3.74556D-09 | 3.30837D-02 |
| R( 4) | 4 - 3 | 2756.19 | -765.94 | 6.43413D+00 | 5.22345D-07 | -3.16927D-01 |
| P( 6) | 4 - 3 | 2767.85 | -754.29 | 7.50090D+00 | 7.52454D-07 | -3.19648D-01 |
| R( 4) | 4 - 4 | 3516.89 | -5.25 | 6.05711D-05 | 9.99999D-01 | -1.71573D+00 |
| R( 5) | 4 - 0 | 415.49 | -3112.94 | 3.37026D-04 | 1.39232D-13 | -2.77825D-04 |
| P( 7) | 4 - 0 | 429.67 | -3098.77 | 3.98375D-04 | 1.83119D-13 | -2.81569D-04 |
| R( 5) | 4 - 1 | 1206.51 | -2321.92 | 4.88469D-03 | 2.65151D-11 | -1.64188D-03 |
| P( 7) | 4 - 1 | 1220.55 | -2307.88 | 5.22566D-03 | 3.49860D-11 | -1.58662D-03 |
| R( 5) | 4 - 2 | 1989.28 | -1539.15 | 5.87277D-01 | 3.82394D-09 | 3.33574D-02 |
| P( 7) | 4 - 2 | 2003.19 | -1525.24 | 6.55159D-01 | 5.09019D-09 | 3.30664D-02 |
| R( 5) | 4 - 3 | 2761.49 | -766.94 | 6.54844D+00 | 7.52235D-07 | -3.16681D-01 |
| P( 7) | 4 - 3 | 2775.27 | -753.16 | 7.38318D+00 | 1.02432D-06 | -3.19897D-01 |
| R( 5) | 4 - 4 | 3522.14 | -6.29 | 1.06279D-04 | 9.99998D-01 | -1.71586D+00 |
| R( 6) | 4 - 0 | 422.03 | -3113.74 | 3.40142D-04 | 1.90082D-13 | -2.77461D-04 |
| P( 8) | 4 - 0 | 438.39 | -3097.39 | 3.94652D-04 | 2.38638D-13 | -2.81782D-04 |
| R( 6) | 4 - 1 | 1212.99 | -2322.78 | 4.97504D-03 | 3.61819D-11 | -1.64695D-03 |
| P( 8) | 4 - 1 | 1229.20 | -2306.58 | 5.14475D-03 | 4.55939D-11 | -1.58318D-03 |
| R( 6) | 4 - 2 | 1995.70 | -1540.08 | 5.95878D-01 | 5.21469D-09 | 3.33857D-02 |
| P( 8) | 4 - 2 | 2011.75 | -1524.02 | 6.46720D-01 | 6.63826D-09 | 3.30499D-02 |
| R( 6) | 4 - 3 | 2767.85 | -767.92 | 6.63641D+00 | 1.02397D-06 | -3.16435D-01 |
| P( 8) | 4 - 3 | 2783.75 | -752.03 | 7.29124D+00 | 1.33810D-06 | -3.20147D-01 |
| R( 6) | 4 - 4 | 3528.43 | -7.34 | 1.70646D-04 | 9.99998D-01 | -1.71601D+00 |
| R( 7) | 4 - 0 | 429.67 | -3114.50 | 3.42322D-04 | 2.49033D-13 | -2.77085D-04 |
| P( 9) | 4 - 0 | 448.20 | -3095.97 | 3.91772D-04 | 3.01363D-13 | -2.81984D-04 |
| R( 7) | 4 - 1 | 1220.55 | -2323.61 | 5.05391D-03 | 4.73795D-11 | -1.65214D-03 |

| | | | | | | |
|---|---|---|---|---|---|---|
| P( 9) | 4 - 1 | 1238.92 | -2305.25 | 5.07666D-03 | 5.75771D-11 | -1.57984D-03 |
| R( 7) | 4 - 2 | 2003.19 | -1540.98 | 6.02990D-01 | 6.82413D-09 | 3.34148D-02 |
| P( 9) | 4 - 2 | 2021.38 | -1522.78 | 6.39794D-01 | 8.38893D-09 | 3.30343D-02 |
| R( 7) | 4 - 3 | 2775.27 | -768.90 | 6.70724D+00 | 1.33758D-06 | -3.16190D-01 |
| P( 9) | 4 - 3 | 2793.28 | -750.88 | 7.21588D+00 | 1.69384D-06 | -3.20397D-01 |
| R( 7) | 4 - 4 | 3535.77 | -8.39 | 2.56872D-04 | 9.99997D-01 | -1.71619D+00 |
| R( 8) | 4 - 0 | 438.39 | -3115.22 | 3.43847D-04 | 3.16168D-13 | -2.76697D-04 |
| P( 10) | 4 - 0 | 459.10 | -3094.51 | 3.89454D-04 | 3.71257D-13 | -2.82174D-04 |
| R( 8) | 4 - 1 | 1229.20 | -2324.41 | 5.12515D-03 | 6.01202D-11 | -1.65744D-03 |
| P( 10) | 4 - 1 | 1249.72 | -2303.89 | 5.01753D-03 | 7.09270D-11 | -1.57662D-03 |
| R( 8) | 4 - 2 | 2011.75 | -1541.86 | 6.09087D-01 | 8.65366D-09 | 3.34448D-02 |
| P( 10) | 4 - 2 | 2032.08 | -1521.52 | 6.33907D-01 | 1.03414D-08 | 3.30195D-02 |
| R( 8) | 4 - 3 | 2783.75 | -769.86 | 6.76623D+00 | 1.69310D-06 | -3.15944D-01 |
| P( 10) | 4 - 3 | 2803.88 | -749.73 | 7.15178D+00 | 2.09158D-06 | -3.20647D-01 |
| R( 8) | 4 - 4 | 3544.17 | -9.44 | 3.68158D-04 | 9.99996D-01 | -1.71639D+00 |
| R( 9) | 4 - 0 | 448.20 | -3115.90 | 3.44889D-04 | 3.91572D-13 | -2.76295D-04 |
| P( 11) | 4 - 0 | 471.09 | -3093.01 | 3.87523D-04 | 4.48284D-13 | -2.82351D-04 |
| R( 9) | 4 - 1 | 1238.92 | -2325.18 | 5.19117D-03 | 7.44167D-11 | -1.66286D-03 |
| P( 11) | 4 - 1 | 1261.60 | -2302.50 | 4.96497D-03 | 8.56355D-11 | -1.57352D-03 |
| R( 9) | 4 - 2 | 2021.38 | -1542.71 | 6.14462D-01 | 1.07047D-08 | 3.34756D-02 |
| P( 11) | 4 - 2 | 2043.85 | -1520.24 | 6.28764D-01 | 1.24950D-08 | 3.30055D-02 |
| R( 9) | 4 - 3 | 2793.28 | -770.81 | 6.81667D+00 | 2.09057D-06 | -3.15699D-01 |
| P( 11) | 4 - 3 | 2815.53 | -748.56 | 7.09565D+00 | 2.53136D-06 | -3.20898D-01 |
| R( 9) | 4 - 4 | 3553.61 | -10.49 | 5.07705D-04 | 9.99995D-01 | -1.71661D+00 |
| R( 10) | 4 - 0 | 459.10 | -3116.53 | 3.45560D-04 | 4.75336D-13 | -2.75880D-04 |
| P( 12) | 4 - 0 | 484.17 | -3091.47 | 3.85863D-04 | 5.32412D-13 | -2.82516D-04 |
| R( 10) | 4 - 1 | 1249.72 | -2325.91 | 5.25352D-03 | 9.02819D-11 | -1.66840D-03 |
| P( 12) | 4 - 1 | 1274.55 | -2301.08 | 4.91740D-03 | 1.01694D-10 | -1.57052D-03 |
| R( 10) | 4 - 2 | 2032.08 | -1543.55 | 6.19306D-01 | 1.29786D-08 | 3.35073D-02 |

| | | | | | | | | |
|---|---|---|---|---|---|---|---|---|
| P( 12) | 4 - 2 | 2056.69 | -1518.94 | 6.24176D-01 | 1.48489D-08 | 3.29924D-02 | | |
| R( 10) | 4 - 3 | 2803.88 | -771.75 | 6.86072D+00 | 2.53001D-06 | -3.15454D-01 | | |
| P( 12) | 4 - 3 | 2828.25 | -747.38 | 7.04535D+00 | 3.01324D-06 | -3.21150D-01 | | |
| R( 10) | 4 - 4 | 3564.09 | -11.54 | 6.78716D-04 | 9.99994D-01 | -1.71686D+00 | | |
| R( 11) | 4 - 0 | 471.09 | -3117.13 | 3.45936D-04 | 5.67550D-13 | -2.75451D-04 | | |
| P( 13) | 4 - 0 | 498.33 | -3089.88 | 3.84397D-04 | 6.23610D-13 | -2.82667D-04 | | |
| R( 11) | 4 - 1 | 1261.60 | -2326.62 | 5.31327D-03 | 1.07729D-10 | -1.67406D-03 | | |
| P( 13) | 4 - 1 | 1288.59 | -2299.62 | 4.87377D-03 | 1.19096D-10 | -1.56763D-03 | | |
| R( 11) | 4 - 2 | 2043.85 | -1544.36 | 6.23751D-01 | 1.54770D-08 | 3.35398D-02 | | |
| P( 13) | 4 - 2 | 2070.60 | -1517.62 | 6.20011D-01 | 1.74025D-08 | 3.29802D-02 | | |
| R( 11) | 4 - 3 | 2815.53 | -772.68 | 6.89983D+00 | 3.01148D-06 | -3.15208D-01 | | |
| P( 13) | 4 - 3 | 2842.02 | -746.20 | 6.99942D+00 | 3.53727D-06 | -3.21401D-01 | | |
| R( 11) | 4 - 4 | 3575.63 | -12.58 | 8.84395D-04 | 9.99993D-01 | -1.71713D+00 | | |
| R( 12) | 4 - 0 | 484.17 | -3117.68 | 3.46069D-04 | 6.68311D-13 | -2.75007D-04 | | |
| P( 14) | 4 - 0 | 513.59 | -3088.26 | 3.83069D-04 | 7.21852D-13 | -2.82804D-04 | | |
| R( 12) | 4 - 1 | 1274.55 | -2327.29 | 5.37116D-03 | 1.26772D-10 | -1.67984D-03 | | |
| P( 14) | 4 - 1 | 1303.70 | -2298.14 | 4.83332D-03 | 1.37832D-10 | -1.56486D-03 | | |
| R( 12) | 4 - 2 | 2056.69 | -1545.15 | 6.27887D-01 | 1.82014D-08 | 3.35731D-02 | | |
| P( 14) | 4 - 2 | 2085.57 | -1516.27 | 6.16178D-01 | 2.01551D-08 | 3.29689D-02 | | |
| R( 12) | 4 - 3 | 2828.25 | -773.60 | 6.93503D+00 | 3.53504D-06 | -3.14963D-01 | | |
| P( 14) | 4 - 3 | 2856.84 | -745.00 | 6.95684D+00 | 4.10351D-06 | -3.21654D-01 | | |
| R( 12) | 4 - 4 | 3588.21 | -13.63 | 1.12795D-03 | 9.99992D-01 | -1.71742D+00 | | |
| R( 13) | 4 - 0 | 498.33 | -3118.19 | 3.45998D-04 | 7.77717D-13 | -2.74547D-04 | | |
| P( 15) | 4 - 0 | 529.93 | -3086.59 | 3.81838D-04 | 8.27112D-13 | -2.82926D-04 | | |
| R( 13) | 4 - 1 | 1288.59 | -2327.93 | 5.42774D-03 | 1.47424D-10 | -1.68573D-03 | | |
| P( 15) | 4 - 1 | 1319.90 | -2296.63 | 4.79549D-03 | 1.57896D-10 | -1.56219D-03 | | |
| R( 13) | 4 - 2 | 2070.60 | -1545.93 | 6.31780D-01 | 2.11534D-08 | 3.36073D-02 | | |
| P( 15) | 4 - 2 | 2101.61 | -1514.91 | 6.12611D-01 | 2.31062D-08 | 3.29583D-02 | | |
| R( 13) | 4 - 3 | 2842.02 | -774.51 | 6.96705D+00 | 4.10073D-06 | -3.14718D-01 | | |

| | | | | | | | |
|---|---|---|---|---|---|---|---|
| P( 15) | 4 - 3 | 2872.73 | -743.79 | 6.91686D+00 | 4.71204D-06 | -3.21906D-01 |
| R( 13) | 4 - 4 | 3601.84 | -14.68 | 1.41257D-03 | 9.99991D-01 | -1.71774D+00 |
| R( 14) | 4 - 0 | 513.59 | -3118.66 | 3.45749D-04 | 8.95871D-13 | -2.74070D-04 |
| P( 16) | 4 - 0 | 547.36 | -3084.89 | 3.80672D-04 | 9.39369D-13 | -2.83033D-04 |
| R( 14) | 4 - 1 | 1303.70 | -2328.54 | 5.48341D-03 | 1.69699D-10 | -1.69174D-03 |
| P( 16) | 4 - 1 | 1337.17 | -2295.08 | 4.75989D-03 | 1.79280D-10 | -1.55963D-03 |
| R( 14) | 4 - 2 | 2085.57 | -1546.67 | 6.35481D-01 | 2.43346D-08 | 3.36424D-02 |
| P( 16) | 4 - 2 | 2118.72 | -1513.52 | 6.09261D-01 | 2.62551D-08 | 3.29487D-02 |
| R( 14) | 4 - 3 | 2856.84 | -775.40 | 6.99645D+00 | 4.70861D-06 | -3.14473D-01 |
| P( 16) | 4 - 3 | 2889.67 | -742.57 | 6.87893D+00 | 5.36292D-06 | -3.22159D-01 |
| R( 14) | 4 - 4 | 3616.52 | -15.72 | 1.74149D-03 | 9.99989D-01 | -1.71808D+00 |
| R( 15) | 4 - 0 | 529.93 | -3119.09 | 3.45342D-04 | 1.02288D-12 | -2.73577D-04 |
| P( 17) | 4 - 0 | 565.88 | -3083.14 | 3.79549D-04 | 1.05860D-12 | -2.83123D-04 |
| R( 15) | 4 - 1 | 1319.90 | -2329.12 | 5.53848D-03 | 1.93612D-10 | -1.69786D-03 |
| P( 17) | 4 - 1 | 1355.51 | -2293.50 | 4.72619D-03 | 2.01978D-10 | -1.55718D-03 |
| R( 15) | 4 - 2 | 2101.61 | -1547.40 | 6.39027D-01 | 2.77466D-08 | 3.36783D-02 |
| P( 17) | 4 - 2 | 2136.90 | -1512.12 | 6.06090D-01 | 2.96012D-08 | 3.29399D-02 |
| R( 15) | 4 - 3 | 2872.73 | -776.29 | 7.02364D+00 | 5.35875D-06 | -3.14227D-01 |
| P( 17) | 4 - 3 | 2907.67 | -741.34 | 6.84263D+00 | 6.05622D-06 | -3.22413D-01 |
| R( 15) | 4 - 4 | 3632.25 | -16.77 | 2.11790D-03 | 9.99988D-01 | -1.71844D+00 |
| R( 16) | 4 - 0 | 547.36 | -3119.47 | 3.44793D-04 | 1.15885D-12 | -2.73065D-04 |
| P( 18) | 4 - 0 | 585.48 | -3081.35 | 3.78448D-04 | 1.18479D-12 | -2.83196D-04 |
| R( 16) | 4 - 1 | 1337.17 | -2329.67 | 5.59319D-03 | 2.19178D-10 | -1.70411D-03 |
| P( 18) | 4 - 1 | 1374.94 | -2291.90 | 4.69416D-03 | 2.25982D-10 | -1.55483D-03 |
| R( 16) | 4 - 2 | 2118.72 | -1548.11 | 6.42446D-01 | 3.13912D-08 | 3.37151D-02 |
| P( 18) | 4 - 2 | 2156.15 | -1510.69 | 6.03070D-01 | 3.31442D-08 | 3.29320D-02 |
| R( 16) | 4 - 3 | 2889.67 | -777.16 | 7.04894D+00 | 6.05122D-06 | -3.13982D-01 |
| P( 18) | 4 - 3 | 2926.73 | -740.11 | 6.80765D+00 | 6.79203D-06 | -3.22667D-01 |
| R( 16) | 4 - 4 | 3649.02 | -17.82 | 2.54501D-03 | 9.99986D-01 | -1.71882D+00 |

| | | | | | | |
|---|---|---|---|---|---|---|
| R( 17) | 4 - 0 | 565.88 | -3119.82 | 3.44114D-04 | 1.30390D-12 | -2.72534D-04 |
| P( 19) | 4 - 0 | 606.17 | -3079.52 | 3.77355D-04 | 1.31793D-12 | -2.83252D-04 |
| R( 17) | 4 - 1 | 1355.51 | -2330.18 | 5.64772D-03 | 2.46412D-10 | -1.71047D-03 |
| P( 19) | 4 - 1 | 1395.44 | -2290.26 | 4.66359D-03 | 2.51286D-10 | -1.55259D-03 |
| R( 17) | 4 - 2 | 2136.90 | -1548.79 | 6.45761D-01 | 3.52702D-08 | 3.37528D-02 |
| P( 19) | 4 - 2 | 2176.46 | -1509.24 | 6.00178D-01 | 3.68835D-08 | 3.29250D-02 |
| R( 17) | 4 - 3 | 2907.67 | -778.02 | 7.07260D+00 | 6.78609D-06 | -3.13736D-01 |
| P( 19) | 4 - 3 | 2946.84 | -738.86 | 6.77374D+00 | 7.57044D-06 | -3.22922D-01 |
| R( 17) | 4 - 4 | 3666.83 | -18.86 | 3.02603D-03 | 9.99984D-01 | -1.71923D+00 |
| R( 18) | 4 - 0 | 585.48 | -3120.12 | 3.43311D-04 | 1.45813D-12 | -2.71983D-04 |
| P( 20) | 4 - 0 | 627.95 | -3077.65 | 3.76257D-04 | 1.45800D-12 | -2.83288D-04 |
| R( 18) | 4 - 1 | 1374.94 | -2330.66 | 5.70223D-03 | 2.75329D-10 | -1.71695D-03 |
| P( 20) | 4 - 1 | 1417.01 | -2288.59 | 4.63435D-03 | 2.77884D-10 | -1.55045D-03 |
| R( 18) | 4 - 2 | 2156.15 | -1549.46 | 6.48989D-01 | 3.93853D-08 | 3.37913D-02 |
| P( 20) | 4 - 2 | 2197.83 | -1507.77 | 5.97395D-01 | 4.08186D-08 | 3.29189D-02 |
| R( 18) | 4 - 3 | 2926.73 | -778.87 | 7.09483D+00 | 7.56344D-06 | -3.13491D-01 |
| P( 20) | 4 - 3 | 2968.01 | -737.60 | 6.74069D+00 | 8.39152D-06 | -3.23177D-01 |
| R( 18) | 4 - 4 | 3685.69 | -19.91 | 3.56418D-03 | 9.99983D-01 | -1.71967D+00 |
| R( 19) | 4 - 0 | 606.17 | -3120.38 | 3.42392D-04 | 1.62168D-12 | -2.71410D-04 |
| P( 21) | 4 - 0 | 650.81 | -3075.74 | 3.75142D-04 | 1.60499D-12 | -2.83305D-04 |
| R( 19) | 4 - 1 | 1395.44 | -2331.12 | 5.75682D-03 | 3.05945D-10 | -1.72354D-03 |
| P( 21) | 4 - 1 | 1439.66 | -2286.89 | 4.60629D-03 | 3.05769D-10 | -1.54842D-03 |
| R( 19) | 4 - 2 | 2176.46 | -1550.10 | 6.52146D-01 | 4.37385D-08 | 3.38307D-02 |
| P( 21) | 4 - 2 | 2220.27 | -1506.28 | 5.94709D-01 | 4.49492D-08 | 3.29136D-02 |
| R( 19) | 4 - 3 | 2946.84 | -779.71 | 7.11577D+00 | 8.38336D-06 | -3.13245D-01 |
| P( 21) | 4 - 3 | 2990.23 | -736.33 | 6.70835D+00 | 9.25539D-06 | -3.23433D-01 |
| R( 19) | 4 - 4 | 3705.60 | -20.95 | 4.16268D-03 | 9.99981D-01 | -1.72012D+00 |
| P( 1) | 5 - 0 | 400.23 | -3853.74 | 1.95018D-04 | 9.11503D-17 | -1.04235D-04 |
| P( 1) | 5 - 1 | 1191.39 | -3062.58 | 3.60084D-04 | 1.93144D-14 | 1.99926D-04 |

| | | | | | | | |
|---|---|---|---|---|---|---|---|
| P( 1) | 5 - 2 | 1974.29 | -2279.68 | 2.27838D-02 | 1.86258D-12 | 2.47629D-03 |
| P( 1) | 5 - 3 | 2746.65 | -1507.32 | 2.11763D+00 | 1.80129D-10 | -4.44035D-02 |
| P( 1) | 5 - 4 | 3507.45 | -746.52 | 1.60612D+01 | 2.65274D-08 | 3.50853D-01 |
| R( 0) | 5 - 0 | 399.14 | -3855.87 | 6.51258D-05 | 9.26535D-17 | -1.04244D-04 |
| P( 2) | 5 - 0 | 402.41 | -3852.60 | 1.30075D-04 | 3.62503D-16 | -1.04306D-04 |
| R( 0) | 5 - 1 | 1190.31 | -3064.70 | 1.18643D-04 | 1.94556D-14 | 1.98563D-04 |
| P( 2) | 5 - 1 | 1193.55 | -3061.46 | 2.41144D-04 | 7.69821D-14 | 2.00489D-04 |
| R( 0) | 5 - 2 | 1973.22 | -2281.79 | 7.70064D-03 | 1.87274D-12 | 2.49006D-03 |
| P( 2) | 5 - 2 | 1976.43 | -2278.58 | 1.50842D-02 | 7.43042D-12 | 2.46951D-03 |
| R( 0) | 5 - 3 | 2745.59 | -1509.41 | 7.10641D-01 | 1.80781D-10 | -4.44603D-02 |
| P( 2) | 5 - 3 | 2748.77 | -1506.23 | 1.40706D+00 | 7.19252D-10 | -4.43774D-02 |
| R( 0) | 5 - 4 | 3506.40 | -748.61 | 5.38122D+00 | 2.65270D-08 | 3.50282D-01 |
| P( 2) | 5 - 4 | 3509.55 | -745.46 | 1.06792D+01 | 1.06113D-07 | 3.51138D-01 |
| R( 0) | 5 - 5 | 4253.97 | -1.04 | 3.58642D-07 | 1.00000D+00 | 1.75117D+00 |
| R( 1) | 5 - 0 | 400.23 | -3856.86 | 7.83332D-05 | 3.69073D-16 | -1.04326D-04 |
| P( 3) | 5 - 0 | 405.68 | -3851.40 | 1.17235D-04 | 8.16078D-16 | -1.04429D-04 |
| R( 1) | 5 - 1 | 1191.39 | -3065.70 | 1.41363D-04 | 7.78782D-14 | 1.97762D-04 |
| P( 3) | 5 - 1 | 1196.79 | -3060.29 | 2.17828D-04 | 1.72938D-13 | 2.00972D-04 |
| R( 1) | 5 - 2 | 1974.29 | -2282.79 | 9.30506D-03 | 7.50459D-12 | 2.49706D-03 |
| P( 3) | 5 - 2 | 1979.64 | -2277.44 | 1.34820D-02 | 1.66850D-11 | 2.46281D-03 |
| R( 1) | 5 - 3 | 2746.65 | -1510.43 | 8.55668D-01 | 7.24264D-10 | -4.44908D-02 |
| P( 3) | 5 - 3 | 2751.95 | -1505.13 | 1.26216D+00 | 1.61583D-09 | -4.43527D-02 |
| R( 1) | 5 - 4 | 3507.45 | -749.63 | 6.47350D+00 | 1.06103D-07 | 3.49996D-01 |
| P( 3) | 5 - 4 | 3512.70 | -744.39 | 9.58543D+00 | 2.38780D-07 | 3.51422D-01 |
| R( 1) | 5 - 5 | 4255.01 | -2.08 | 3.44293D-06 | 1.00000D+00 | 1.75120D+00 |
| R( 2) | 5 - 0 | 402.41 | -3857.79 | 8.42030D-05 | 8.33028D-16 | -1.04458D-04 |
| P( 4) | 5 - 0 | 410.04 | -3850.16 | 1.11916D-04 | 1.44658D-15 | -1.04603D-04 |
| R( 2) | 5 - 1 | 1193.55 | -3066.65 | 1.50255D-04 | 1.75703D-13 | 1.96882D-04 |
| P( 4) | 5 - 1 | 1201.11 | -3059.09 | 2.08043D-04 | 3.06670D-13 | 2.01376D-04 |

| | | | | | | | |
|---|---|---|---|---|---|---|---|
| R( 2) | 5 - 2 | 1976.43 | -2283.77 | 1.00391D-02 | 1.69274D-11 | 2.50413D-03 |
| P( 4) | 5 - 2 | 1983.93 | -2276.27 | 1.27513D-02 | 2.95945D-11 | 2.45617D-03 |
| R( 2) | 5 - 3 | 2748.77 | -1511.42 | 9.19922D-01 | 1.63252D-09 | -4.45229D-02 |
| P( 4) | 5 - 3 | 2756.19 | -1504.01 | 1.19811D+00 | 2.86798D-09 | -4.43295D-02 |
| R( 2) | 5 - 4 | 3509.55 | -750.65 | 6.95273D+00 | 2.38735D-07 | 3.49710D-01 |
| P( 4) | 5 - 4 | 3516.89 | -743.31 | 9.10393D+00 | 4.24539D-07 | 3.51707D-01 |
| R( 2) | 5 - 5 | 4257.08 | -3.11 | 1.24499D-05 | 9.99999D-01 | 1.75126D+00 |
| R( 3) | 5 - 0 | 405.68 | -3858.67 | 8.76889D-05 | 1.48588D-15 | -1.04642D-04 |
| P( 5) | 5 - 0 | 415.49 | -3848.86 | 1.09166D-04 | 2.25373D-15 | -1.04829D-04 |
| R( 3) | 5 - 1 | 1196.79 | -3067.56 | 1.54441D-04 | 3.13223D-13 | 1.95921D-04 |
| P( 5) | 5 - 1 | 1206.51 | -3057.84 | 2.02668D-04 | 4.77978D-13 | 2.01700D-04 |
| R( 3) | 5 - 2 | 1979.64 | -2284.71 | 1.04833D-02 | 3.01690D-11 | 2.51127D-03 |
| P( 5) | 5 - 2 | 1989.28 | -2275.07 | 1.23114D-02 | 4.61372D-11 | 2.44960D-03 |
| R( 3) | 5 - 3 | 2751.95 | -1512.40 | 9.57275D-01 | 2.90755D-09 | -4.45564D-02 |
| P( 5) | 5 - 3 | 2761.49 | -1502.86 | 1.16103D+00 | 4.47419D-09 | -4.43078D-02 |
| R( 3) | 5 - 4 | 3512.70 | -751.66 | 7.22736D+00 | 4.24434D-07 | 3.49423D-01 |
| P( 5) | 5 - 4 | 3522.14 | -742.21 | 8.82627D+00 | 6.63421D-07 | 3.51990D-01 |
| R( 3) | 5 - 5 | 4260.20 | -4.15 | 3.06041D-05 | 9.99999D-01 | 1.75134D+00 |
| R( 4) | 5 - 0 | 410.04 | -3859.50 | 9.01426D-05 | 2.32971D-15 | -1.04877D-04 |
| P( 6) | 5 - 0 | 422.03 | -3847.51 | 1.07634D-04 | 3.23607D-15 | -1.05105D-04 |
| R( 4) | 5 - 1 | 1201.11 | -3068.43 | 1.56410D-04 | 4.90779D-13 | 1.94881D-04 |
| P( 6) | 5 - 1 | 1212.99 | -3056.55 | 1.99214D-04 | 6.86595D-13 | 2.01945D-04 |
| R( 4) | 5 - 2 | 1983.93 | -2285.62 | 1.07962D-02 | 4.72596D-11 | 2.51849D-03 |
| P( 6) | 5 - 2 | 1995.70 | -2273.84 | 1.20040D-02 | 6.62902D-11 | 2.44311D-03 |
| R( 4) | 5 - 3 | 2756.19 | -1513.35 | 9.82419D-01 | 4.55149D-09 | -4.45914D-02 |
| P( 6) | 5 - 3 | 2767.85 | -1501.69 | 1.13622D+00 | 6.43293D-09 | -4.42875D-02 |
| R( 4) | 5 - 4 | 3516.89 | -752.65 | 7.40877D+00 | 6.63216D-07 | 3.49136D-01 |
| P( 6) | 5 - 4 | 3528.43 | -741.11 | 8.64107D+00 | 9.55458D-07 | 3.52274D-01 |
| R( 4) | 5 - 5 | 4264.35 | -5.19 | 6.11325D-05 | 9.99999D-01 | 1.75145D+00 |

| | | | | | | | |
|---|---|---|---|---|---|---|---|
| R( 5) | 5 - 0 | 415.49 | -3860.28 | 9.20844D-05 | 3.36665D-15 | -1.05162D-04 |
| P( 7) | 5 - 0 | 429.67 | -3846.10 | 1.06801D-04 | 4.39224D-15 | -1.05433D-04 |
| R( 5) | 5 - 1 | 1206.51 | -3069.26 | 1.57121D-04 | 7.08719D-13 | 1.93759D-04 |
| P( 7) | 5 - 1 | 1220.55 | -3055.21 | 1.96724D-04 | 9.32264D-13 | 2.02110D-04 |
| R( 5) | 5 - 2 | 1989.28 | -2286.49 | 1.10385D-02 | 6.82301D-11 | 2.52578D-03 |
| P( 7) | 5 - 2 | 2003.19 | -2272.58 | 1.17682D-02 | 9.00311D-11 | 2.43668D-03 |
| R( 5) | 5 - 3 | 2761.49 | -1514.28 | 1.00101D+00 | 6.56653D-09 | -4.46278D-02 |
| P( 7) | 5 - 3 | 2775.27 | -1500.50 | 1.11804D+00 | 8.74275D-09 | -4.42688D-02 |
| R( 5) | 5 - 4 | 3522.14 | -753.63 | 7.53980D+00 | 9.55104D-07 | 3.48849D-01 |
| P( 7) | 5 - 4 | 3535.77 | -739.99 | 8.50550D+00 | 1.30069D-06 | 3.52557D-01 |
| R( 5) | 5 - 5 | 4269.54 | -6.23 | 1.07263D-04 | 9.99998D-01 | 1.75158D+00 |
| R( 6) | 5 - 0 | 422.03 | -3861.00 | 9.37577D-05 | 4.59896D-15 | -1.05499D-04 |
| P( 8) | 5 - 0 | 438.39 | -3844.65 | 1.06425D-04 | 5.72093D-15 | -1.05812D-04 |
| R( 6) | 5 - 1 | 1212.99 | -3070.04 | 1.57021D-04 | 9.67404D-13 | 1.92557D-04 |
| P( 8) | 5 - 1 | 1229.20 | -3053.84 | 1.94751D-04 | 1.21474D-12 | 2.02195D-04 |
| R( 6) | 5 - 2 | 1995.70 | -2287.33 | 1.12388D-02 | 9.31124D-11 | 2.53315D-03 |
| P( 8) | 5 - 2 | 2011.75 | -2271.28 | 1.15755D-02 | 1.17338D-10 | 2.43031D-03 |
| R( 6) | 5 - 3 | 2767.85 | -1515.18 | 1.01567D+00 | 8.95495D-09 | -4.46658D-02 |
| P( 8) | 5 - 3 | 2783.75 | -1499.29 | 1.10385D+00 | 1.14023D-08 | -4.42515D-02 |
| R( 6) | 5 - 4 | 3528.43 | -754.60 | 7.64044D+00 | 1.30013D-06 | 3.48561D-01 |
| P( 8) | 5 - 4 | 3544.17 | -738.87 | 8.39956D+00 | 1.69916D-06 | 3.52841D-01 |
| R( 6) | 5 - 5 | 4275.77 | -7.27 | 1.72224D-04 | 9.99997D-01 | 1.75173D+00 |
| R( 7) | 5 - 0 | 429.67 | -3861.67 | 9.52917D-05 | 6.02895D-15 | -1.05887D-04 |
| P( 9) | 5 - 0 | 448.20 | -3843.14 | 1.06378D-04 | 7.22094D-15 | -1.06243D-04 |
| R( 7) | 5 - 1 | 1220.55 | -3070.78 | 1.56350D-04 | 1.26720D-12 | 1.91273D-04 |
| P( 9) | 5 - 1 | 1238.92 | -3052.42 | 1.93058D-04 | 1.53377D-12 | 2.02199D-04 |
| R( 7) | 5 - 2 | 2003.19 | -2288.15 | 1.14120D-02 | 1.21939D-10 | 2.54059D-03 |
| P( 9) | 5 - 2 | 2021.38 | -2269.95 | 1.14108D-02 | 1.48192D-10 | 2.42401D-03 |
| R( 7) | 5 - 3 | 2775.27 | -1516.07 | 1.02781D+00 | 1.17191D-08 | -4.47052D-02 |

| | | | | | | |
|---|---|---|---|---|---|---|
| P( 9) | 5 - 3 | 2793.28 | -1498.05 | 1.09225D+00 | 1.44102D-08 | -4.42357D-02 |
| R( 7) | 5 - 4 | 3535.77 | -755.56 | 7.72127D+00 | 1.69832D-06 | 3.48272D-01 |
| P( 9) | 5 - 4 | 3553.61 | -737.73 | 8.31267D+00 | 2.15092D-06 | 3.53124D-01 |
| R( 7) | 5 - 5 | 4283.03 | -8.30 | 2.59244D-04 | 9.99996D-01 | 1.75190D+00 |
| R( 8) | 5 - 0 | 438.39 | -3862.29 | 9.67621D-05 | 7.65906D-15 | -1.06326D-04 |
| P( 10) | 5 - 0 | 459.10 | -3841.58 | 1.06588D-04 | 8.89111D-15 | -1.06725D-04 |
| R( 8) | 5 - 1 | 1229.20 | -3071.48 | 1.55244D-04 | 1.60850D-12 | 1.89907D-04 |
| P( 10) | 5 - 1 | 1249.72 | -3050.96 | 1.91508D-04 | 1.88913D-12 | 2.02123D-04 |
| R( 8) | 5 - 2 | 2011.75 | -2288.92 | 1.15669D-02 | 1.54745D-10 | 2.54810D-03 |
| P( 10) | 5 - 2 | 2032.08 | -2268.59 | 1.12655D-02 | 1.82571D-10 | 2.41777D-03 |
| R( 8) | 5 - 3 | 2783.75 | -1516.93 | 1.03824D+00 | 1.48615D-08 | -4.47461D-02 |
| P( 10) | 5 - 3 | 2803.88 | -1496.80 | 1.08244D+00 | 1.77653D-08 | -4.42214D-02 |
| R( 8) | 5 - 4 | 3544.17 | -756.51 | 7.78841D+00 | 2.14973D-06 | 3.47983D-01 |
| P( 10) | 5 - 4 | 3564.09 | -736.58 | 8.23870D+00 | 2.65604D-06 | 3.53406D-01 |
| R( 8) | 5 - 5 | 4291.34 | -9.34 | 3.71552D-04 | 9.99995D-01 | 1.75210D+00 |
| R( 9) | 5 - 0 | 448.20 | -3862.85 | 9.82161D-05 | 9.49179D-15 | -1.06816D-04 |
| P( 11) | 5 - 0 | 471.09 | -3839.97 | 1.07009D-04 | 1.07304D-14 | -1.07258D-04 |
| R( 9) | 5 - 1 | 1238.92 | -3072.14 | 1.53792D-04 | 1.99168D-12 | 1.88458D-04 |
| P( 11) | 5 - 1 | 1261.60 | -3049.46 | 1.90017D-04 | 2.28059D-12 | 2.01964D-04 |
| R( 9) | 5 - 2 | 2021.38 | -2289.67 | 1.17089D-02 | 1.91564D-10 | 2.55568D-03 |
| P( 11) | 5 - 2 | 2043.85 | -2267.20 | 1.11341D-02 | 2.20457D-10 | 2.41160D-03 |
| R( 9) | 5 - 3 | 2793.28 | -1517.77 | 1.04745D+00 | 1.83845D-08 | -4.47884D-02 |
| P( 11) | 5 - 3 | 2815.53 | -1495.52 | 1.07390D+00 | 2.14664D-08 | -4.42086D-02 |
| R( 9) | 5 - 4 | 3553.61 | -757.45 | 7.84566D+00 | 2.65439D-06 | 3.47693D-01 |
| P( 11) | 5 - 4 | 3575.63 | -735.42 | 8.17388D+00 | 3.21456D-06 | 3.53689D-01 |
| R( 9) | 5 - 5 | 4300.68 | -10.38 | 5.12377D-04 | 9.99994D-01 | 1.75232D+00 |
| R( 10) | 5 - 0 | 459.10 | -3863.37 | 9.96850D-05 | 1.15298D-14 | -1.07357D-04 |
| P( 12) | 5 - 0 | 484.17 | -3838.30 | 1.07611D-04 | 1.27378D-14 | -1.07843D-04 |
| R( 10) | 5 - 1 | 1249.72 | -3072.75 | 1.52050D-04 | 2.41714D-12 | 1.86926D-04 |

| | | | | | | |
|---|---|---|---|---|---|---|
| P( 12) | 5 - 1 | 1274.55 | -3047.91 | 1.88530D-04 | 2.70793D-12 | 2.01725D-04 |
| R( 10) | 5 - 2 | 2032.08 | -2290.38 | 1.18414D-02 | 2.32432D-10 | 2.56334D-03 |
| P( 12) | 5 - 2 | 2056.69 | -2265.78 | 1.10131D-02 | 2.61831D-10 | 2.40548D-03 |
| R( 10) | 5 - 3 | 2803.88 | -1518.59 | 1.05577D+00 | 2.22908D-08 | -4.48323D-02 |
| P( 12) | 5 - 3 | 2828.25 | -1494.22 | 1.06633D+00 | 2.55123D-08 | -4.41973D-02 |
| R( 10) | 5 - 4 | 3564.09 | -758.37 | 7.89548D+00 | 3.21238D-06 | 3.47402D-01 |
| P( 12) | 5 - 4 | 3588.21 | -734.25 | 8.11571D+00 | 3.82657D-06 | 3.53971D-01 |
| R( 10) | 5 - 5 | 4311.05 | -11.41 | 6.84949D-04 | 9.99993D-01 | 1.75256D+00 |
| R( 11) | 5 - 0 | 471.09 | -3863.83 | 1.01191D-04 | 1.37757D-14 | -1.07950D-04 |
| P( 13) | 5 - 0 | 498.33 | -3836.58 | 1.08377D-04 | 1.49124D-14 | -1.08480D-04 |
| R( 11) | 5 - 1 | 1261.60 | -3073.32 | 1.50059D-04 | 2.88531D-12 | 1.85309D-04 |
| P( 13) | 5 - 1 | 1288.59 | -3046.33 | 1.87009D-04 | 3.17095D-12 | 2.01402D-04 |
| R( 11) | 5 - 2 | 2043.85 | -2291.06 | 1.19669D-02 | 2.77386D-10 | 2.57106D-03 |
| P( 13) | 5 - 2 | 2070.60 | -2264.32 | 1.09001D-02 | 3.06676D-10 | 2.39942D-03 |
| R( 11) | 5 - 3 | 2815.53 | -1519.38 | 1.06342D+00 | 2.65832D-08 | -4.48777D-02 |
| P( 13) | 5 - 3 | 2842.02 | -1492.90 | 1.05949D+00 | 2.99022D-08 | -4.41876D-02 |
| R( 11) | 5 - 4 | 3575.63 | -759.29 | 7.93955D+00 | 3.82373D-06 | 3.47111D-01 |
| P( 13) | 5 - 4 | 3601.84 | -733.07 | 8.06254D+00 | 4.49215D-06 | 3.54253D-01 |
| R( 11) | 5 - 5 | 4322.47 | -12.45 | 8.92499D-04 | 9.99991D-01 | 1.75283D+00 |
| R( 12) | 5 - 0 | 484.17 | -3864.24 | 1.02750D-04 | 1.62325D-14 | -1.08593D-04 |
| P( 14) | 5 - 0 | 513.59 | -3834.81 | 1.09293D-04 | 1.72535D-14 | -1.09168D-04 |
| R( 12) | 5 - 1 | 1274.55 | -3073.85 | 1.47846D-04 | 3.39659D-12 | 1.83608D-04 |
| P( 14) | 5 - 1 | 1303.70 | -3044.70 | 1.85428D-04 | 3.66945D-12 | 2.00996D-04 |
| R( 12) | 5 - 2 | 2056.69 | -2291.71 | 1.20870D-02 | 3.26463D-10 | 2.57886D-03 |
| P( 14) | 5 - 2 | 2085.57 | -2262.83 | 1.07933D-02 | 3.54976D-10 | 2.39341D-03 |
| R( 12) | 5 - 3 | 2828.25 | -1520.16 | 1.07056D+00 | 3.12643D-08 | -4.49245D-02 |
| P( 14) | 5 - 3 | 2856.84 | -1491.56 | 1.05323D+00 | 3.46350D-08 | -4.41793D-02 |
| R( 12) | 5 - 4 | 3588.21 | -760.19 | 7.97906D+00 | 4.48853D-06 | 3.46820D-01 |
| P( 14) | 5 - 4 | 3616.52 | -731.88 | 8.01316D+00 | 5.21136D-06 | 3.54535D-01 |

| | | | | | | |
|---|---|---|---|---|---|---|
| R( 12) | 5 - 5 | 4334.92 | -13.49 | 1.13826D-03 | 9.99990D-01 | 1.75312D+00 |
| R( 13) | 5 - 0 | 498.33 | -3864.59 | 1.04373D-04 | 1.89030D-14 | -1.09288D-04 |
| P( 15) | 5 - 0 | 529.93 | -3832.99 | 1.10349D-04 | 1.97602D-14 | -1.09908D-04 |
| R( 13) | 5 - 1 | 1288.59 | -3074.33 | 1.45435D-04 | 3.95142D-12 | 1.81820D-04 |
| P( 15) | 5 - 1 | 1319.90 | -3043.03 | 1.83768D-04 | 4.20322D-12 | 2.00506D-04 |
| R( 13) | 5 - 2 | 2070.60 | -2292.33 | 1.22029D-02 | 3.79704D-10 | 2.58672D-03 |
| P( 15) | 5 - 2 | 2101.61 | -2261.31 | 1.06916D-02 | 4.06714D-10 | 2.38745D-03 |
| R( 13) | 5 - 3 | 2842.02 | -1520.91 | 1.07731D+00 | 3.63370D-08 | -4.49729D-02 |
| P( 15) | 5 - 3 | 2872.73 | -1490.19 | 1.04744D+00 | 3.97099D-08 | -4.41726D-02 |
| R( 13) | 5 - 4 | 3601.84 | -761.08 | 8.01485D+00 | 5.20685D-06 | 3.46527D-01 |
| P( 15) | 5 - 4 | 3632.25 | -730.68 | 7.96674D+00 | 5.98432D-06 | 3.54817D-01 |
| R( 13) | 5 - 5 | 4348.40 | -14.52 | 1.42545D-03 | 9.99988D-01 | 1.75343D+00 |
| R( 14) | 5 - 0 | 513.59 | -3864.89 | 1.06072D-04 | 2.17904D-14 | -1.10034D-04 |
| P( 16) | 5 - 0 | 547.36 | -3831.12 | 1.11541D-04 | 2.24319D-14 | -1.10700D-04 |
| R( 14) | 5 - 1 | 1303.70 | -3074.78 | 1.42842D-04 | 4.55025D-12 | 1.79946D-04 |
| P( 16) | 5 - 1 | 1337.17 | -3041.31 | 1.82016D-04 | 4.77209D-12 | 1.99932D-04 |
| R( 14) | 5 - 2 | 2085.57 | -2292.91 | 1.23155D-02 | 4.37147D-10 | 2.59465D-03 |
| P( 16) | 5 - 2 | 2118.72 | -2259.76 | 1.05940D-02 | 4.61875D-10 | 2.38154D-03 |
| R( 14) | 5 - 3 | 2856.84 | -1521.64 | 1.08375D+00 | 4.18044D-08 | -4.50227D-02 |
| P( 16) | 5 - 3 | 2889.67 | -1488.81 | 1.04203D+00 | 4.51260D-08 | -4.41674D-02 |
| R( 14) | 5 - 4 | 3616.52 | -761.96 | 8.04756D+00 | 5.97876D-06 | 3.46234D-01 |
| P( 16) | 5 - 4 | 3649.02 | -729.46 | 7.92264D+00 | 6.81110D-06 | 3.55099D-01 |
| R( 14) | 5 - 5 | 4362.92 | -15.56 | 1.75732D-03 | 9.99987D-01 | 1.75377D+00 |
| R( 15) | 5 - 0 | 529.93 | -3865.14 | 1.07852D-04 | 2.48977D-14 | -1.10831D-04 |
| P( 17) | 5 - 0 | 565.88 | -3829.20 | 1.12863D-04 | 2.52682D-14 | -1.11544D-04 |
| R( 15) | 5 - 1 | 1319.90 | -3075.18 | 1.40081D-04 | 5.19353D-12 | 1.77984D-04 |
| P( 17) | 5 - 1 | 1355.51 | -3039.56 | 1.80161D-04 | 5.37587D-12 | 1.99272D-04 |
| R( 15) | 5 - 2 | 2101.61 | -2293.46 | 1.24255D-02 | 4.98833D-10 | 2.60265D-03 |
| P( 17) | 5 - 2 | 2136.90 | -2258.17 | 1.04999D-02 | 5.20444D-10 | 2.37568D-03 |

| | | | | | | | |
|---|---|---|---|---|---|---|---|
| R( 15) | 5 - 3 | 2872.73 | -1522.34 | 1.08993D+00 | 4.76693D-08 | -4.50741D-02 |
| P( 17) | 5 - 3 | 2907.67 | -1487.40 | 1.03694D+00 | 5.08826D-08 | -4.41637D-02 |
| R( 15) | 5 - 4 | 3632.25 | -762.83 | 8.07767D+00 | 6.80436D-06 | 3.45940D-01 |
| P( 17) | 5 - 4 | 3666.83 | -728.24 | 7.88037D+00 | 7.69183D-06 | 3.55381D-01 |
| R( 15) | 5 - 5 | 4378.48 | -16.59 | 2.13709D-03 | 9.99985D-01 | 1.75413D+00 |
| R( 16) | 5 - 0 | 547.36 | -3865.34 | 1.09722D-04 | 2.82284D-14 | -1.11680D-04 |
| P( 18) | 5 - 0 | 585.48 | -3827.22 | 1.14312D-04 | 2.82686D-14 | -1.12439D-04 |
| R( 16) | 5 - 1 | 1337.17 | -3075.53 | 1.37164D-04 | 5.88173D-12 | 1.75933D-04 |
| P( 18) | 5 - 1 | 1374.94 | -3037.76 | 1.78196D-04 | 6.01439D-12 | 1.98525D-04 |
| R( 16) | 5 - 2 | 2118.72 | -2293.97 | 1.25333D-02 | 5.64805D-10 | 2.61071D-03 |
| P( 18) | 5 - 2 | 2156.15 | -2256.55 | 1.04085D-02 | 5.82408D-10 | 2.36986D-03 |
| R( 16) | 5 - 3 | 2889.67 | -1523.03 | 1.09592D+00 | 5.39350D-08 | -4.51270D-02 |
| P( 18) | 5 - 3 | 2926.73 | -1485.97 | 1.03211D+00 | 5.69790D-08 | -4.41616D-02 |
| R( 16) | 5 - 4 | 3649.02 | -763.68 | 8.10555D+00 | 7.68373D-06 | 3.45646D-01 |
| P( 18) | 5 - 4 | 3685.69 | -727.00 | 7.83957D+00 | 8.62660D-06 | 3.55662D-01 |
| R( 16) | 5 - 5 | 4395.07 | -17.63 | 2.56800D-03 | 9.99983D-01 | 1.75451D+00 |
| R( 17) | 5 - 0 | 565.88 | -3865.48 | 1.11687D-04 | 3.17859D-14 | -1.12579D-04 |
| P( 19) | 5 - 0 | 606.17 | -3825.19 | 1.15888D-04 | 3.14326D-14 | -1.13387D-04 |
| R( 17) | 5 - 1 | 1355.51 | -3075.85 | 1.34100D-04 | 6.61532D-12 | 1.73792D-04 |
| P( 19) | 5 - 1 | 1395.44 | -3035.92 | 1.76116D-04 | 6.68749D-12 | 1.97691D-04 |
| R( 17) | 5 - 2 | 2136.90 | -2294.46 | 1.26395D-02 | 6.35106D-10 | 2.61883D-03 |
| P( 19) | 5 - 2 | 2176.46 | -2254.90 | 1.03196D-02 | 6.47753D-10 | 2.36409D-03 |
| R( 17) | 5 - 3 | 2907.67 | -1523.69 | 1.10174D+00 | 6.06047D-08 | -4.51814D-02 |
| P( 19) | 5 - 3 | 2946.84 | -1484.52 | 1.02752D+00 | 6.34147D-08 | -4.41611D-02 |
| R( 17) | 5 - 4 | 3666.83 | -764.53 | 8.13147D+00 | 8.61697D-06 | 3.45350D-01 |
| P( 19) | 5 - 4 | 3705.60 | -725.76 | 7.79996D+00 | 9.61553D-06 | 3.55943D-01 |
| R( 17) | 5 - 5 | 4412.70 | -18.66 | 3.05327D-03 | 9.99981D-01 | 1.75492D+00 |
| R( 18) | 5 - 0 | 585.48 | -3865.57 | 1.13751D-04 | 3.55737D-14 | -1.13530D-04 |
| P( 20) | 5 - 0 | 627.95 | -3823.11 | 1.17589D-04 | 3.47601D-14 | -1.14387D-04 |

| | | | | | | |
|---|---|---|---|---|---|---|
| R( 18) | 5 - 1 | 1374.94 | -3076.12 | 1.30898D-04 | 7.39480D-12 | 1.71560D-04 |
| P( 20) | 5 - 1 | 1417.01 | -3034.04 | 1.73916D-04 | 7.39501D-12 | 1.96768D-04 |
| R( 18) | 5 - 2 | 2156.15 | -2294.91 | 1.27442D-02 | 7.09781D-10 | 2.62702D-03 |
| P( 20) | 5 - 2 | 2197.83 | -2253.22 | 1.02328D-02 | 7.16468D-10 | 2.35835D-03 |
| R( 18) | 5 - 3 | 2926.73 | -1524.33 | 1.10744D+00 | 6.76817D-08 | -4.52374D-02 |
| P( 20) | 5 - 3 | 2968.01 | -1483.05 | 1.02313D+00 | 7.01892D-08 | -4.41621D-02 |
| R( 18) | 5 - 4 | 3685.69 | -765.36 | 8.15568D+00 | 9.60420D-06 | 3.45054D-01 |
| P( 20) | 5 - 4 | 3726.55 | -724.50 | 7.76129D+00 | 1.06587D-05 | 3.56225D-01 |
| R( 18) | 5 - 5 | 4431.36 | -19.69 | 3.59615D-03 | 9.99978D-01 | 1.75534D+00 |
| R( 19) | 5 - 0 | 606.17 | -3865.61 | 1.15921D-04 | 3.95958D-14 | -1.14533D-04 |
| P( 21) | 5 - 0 | 650.81 | -3820.97 | 1.19415D-04 | 3.82509D-14 | -1.15438D-04 |
| R( 19) | 5 - 1 | 1395.44 | -3076.35 | 1.27567D-04 | 8.22066D-12 | 1.69236D-04 |
| P( 21) | 5 - 1 | 1439.66 | -3032.12 | 1.71594D-04 | 8.13679D-12 | 1.95755D-04 |
| R( 19) | 5 - 2 | 2176.46 | -2295.33 | 1.28478D-02 | 7.88874D-10 | 2.63526D-03 |
| P( 21) | 5 - 2 | 2220.27 | -2251.51 | 1.01477D-02 | 7.88540D-10 | 2.35264D-03 |
| R( 19) | 5 - 3 | 2946.84 | -1524.94 | 1.11303D+00 | 7.51694D-08 | -4.52949D-02 |
| P( 21) | 5 - 3 | 2990.23 | -1481.55 | 1.01892D+00 | 7.73019D-08 | -4.41647D-02 |
| R( 19) | 5 - 4 | 3705.60 | -766.18 | 8.17834D+00 | 1.06455D-05 | 3.44756D-01 |
| P( 21) | 5 - 4 | 3748.55 | -723.23 | 7.72340D+00 | 1.17564D-05 | 3.56506D-01 |
| R( 19) | 5 - 5 | 4451.05 | -20.73 | 4.19987D-03 | 9.99976D-01 | 1.75580D+00 |
| Q( 0) | 0 - 0 | 399.14 | 0.00 | 0.00000D+00 | 1.00000D+00 | -1.56718D+00 |
| Q( 1) | 0 - 0 | 400.23 | -0.00 | 0.00000D+00 | 1.00000D+00 | -1.56720D+00 |
| Q( 2) | 0 - 0 | 402.41 | 0.00 | 0.00000D+00 | 1.00000D+00 | -1.56725D+00 |
| Q( 3) | 0 - 0 | 405.68 | 0.00 | 0.00000D+00 | 1.00000D+00 | -1.56732D+00 |
| Q( 4) | 0 - 0 | 410.04 | 0.00 | 0.00000D+00 | 1.00000D+00 | -1.56741D+00 |
| Q( 5) | 0 - 0 | 415.49 | 0.00 | 0.00000D+00 | 1.00000D+00 | -1.56753D+00 |
| Q( 6) | 0 - 0 | 422.03 | 0.00 | 0.00000D+00 | 1.00000D+00 | -1.56768D+00 |
| Q( 7) | 0 - 0 | 429.67 | 0.00 | 0.00000D+00 | 1.00000D+00 | -1.56784D+00 |
| Q( 8) | 0 - 0 | 438.39 | 0.00 | 0.00000D+00 | 1.00000D+00 | -1.56803D+00 |

| | | | | | | | |
|---|---|---|---|---|---|---|---|
| Q( 9) | 0 - 0 | 448.20 | 0.00 | 0.00000D+00 | 1.00000D+00 | -1.56824D+00 |
| Q( 10) | 0 - 0 | 459.10 | 0.00 | 0.00000D+00 | 1.00000D+00 | -1.56848D+00 |
| Q( 11) | 0 - 0 | 471.09 | 0.00 | 0.00000D+00 | 1.00000D+00 | -1.56874D+00 |
| Q( 12) | 0 - 0 | 484.17 | 0.00 | 0.00000D+00 | 1.00000D+00 | -1.56903D+00 |
| Q( 13) | 0 - 0 | 498.33 | 0.00 | 0.00000D+00 | 1.00000D+00 | -1.56933D+00 |
| Q( 14) | 0 - 0 | 513.59 | 0.00 | 0.00000D+00 | 1.00000D+00 | -1.56967D+00 |
| Q( 15) | 0 - 0 | 529.93 | 0.00 | 0.00000D+00 | 1.00000D+00 | -1.57002D+00 |
| Q( 16) | 0 - 0 | 547.36 | 0.00 | 0.00000D+00 | 1.00000D+00 | -1.57040D+00 |
| Q( 17) | 0 - 0 | 565.88 | 0.00 | 0.00000D+00 | 1.00000D+00 | -1.57080D+00 |
| Q( 18) | 0 - 0 | 585.48 | 0.00 | 0.00000D+00 | 1.00000D+00 | -1.57123D+00 |
| Q( 19) | 0 - 0 | 606.17 | 0.00 | 0.00000D+00 | 1.00000D+00 | -1.57168D+00 |
| Q( 20) | 0 - 0 | 627.95 | 0.00 | 0.00000D+00 | 1.00000D+00 | -1.57216D+00 |
| Q( 0) | 1 - 0 | 399.14 | -791.17 | 0.00000D+00 | 3.63545D-21 | 1.64439D-01 |
| Q( 0) | 1 - 1 | 1190.31 | 0.00 | 0.00000D+00 | 1.00000D+00 | 1.60409D+00 |
| Q( 1) | 1 - 0 | 400.23 | -791.16 | 0.00000D+00 | 6.10830D-18 | 1.64440D-01 |
| Q( 1) | 1 - 1 | 1191.39 | -0.00 | 0.00000D+00 | 1.00000D+00 | 1.60411D+00 |
| Q( 2) | 1 - 0 | 402.41 | -791.14 | 0.00000D+00 | 3.37994D-21 | 1.64440D-01 |
| Q( 2) | 1 - 1 | 1193.55 | 0.00 | 0.00000D+00 | 1.00000D+00 | 1.60416D+00 |
| Q( 3) | 1 - 0 | 405.68 | -791.11 | 0.00000D+00 | 3.37716D-21 | 1.64441D-01 |
| Q( 3) | 1 - 1 | 1196.79 | 0.00 | 0.00000D+00 | 1.00000D+00 | 1.60423D+00 |
| Q( 4) | 1 - 0 | 410.04 | -791.07 | 0.00000D+00 | 3.36710D-21 | 1.64442D-01 |
| Q( 4) | 1 - 1 | 1201.11 | 0.00 | 0.00000D+00 | 1.00000D+00 | 1.60432D+00 |
| Q( 5) | 1 - 0 | 415.49 | -791.02 | 0.00000D+00 | 3.36023D-21 | 1.64444D-01 |
| Q( 5) | 1 - 1 | 1206.51 | 0.00 | 0.00000D+00 | 1.00000D+00 | 1.60444D+00 |
| Q( 6) | 1 - 0 | 422.03 | -790.96 | 0.00000D+00 | 3.35292D-21 | 1.64446D-01 |
| Q( 6) | 1 - 1 | 1212.99 | 0.00 | 0.00000D+00 | 1.00000D+00 | 1.60458D+00 |
| Q( 7) | 1 - 0 | 429.67 | -790.89 | 0.00000D+00 | 3.34769D-21 | 1.64448D-01 |
| Q( 7) | 1 - 1 | 1220.55 | 0.00 | 0.00000D+00 | 1.00000D+00 | 1.60474D+00 |
| Q( 8) | 1 - 0 | 438.39 | -790.81 | 0.00000D+00 | 3.34426D-21 | 1.64451D-01 |

| | | | | | | |
|---|---|---|---|---|---|---|
| Q( 8) | 1 - 1 | 1229.20 | 0.00 | 0.00000D+00 | 1.00000D+00 | 1.60493D+00 |
| Q( 9) | 1 - 0 | 448.20 | -790.72 | 0.00000D+00 | 3.33911D-21 | 1.64454D-01 |
| Q( 9) | 1 - 1 | 1238.92 | 0.00 | 0.00000D+00 | 1.00000D+00 | 1.60514D+00 |
| Q( 10) | 1 - 0 | 459.10 | -790.62 | 0.00000D+00 | 3.34018D-21 | 1.64457D-01 |
| Q( 10) | 1 - 1 | 1249.72 | 0.00 | 0.00000D+00 | 1.00000D+00 | 1.60537D+00 |
| Q( 11) | 1 - 0 | 471.09 | -790.51 | 0.00000D+00 | 3.34810D-21 | 1.64460D-01 |
| Q( 11) | 1 - 1 | 1261.60 | 0.00 | 0.00000D+00 | 1.00000D+00 | 1.60563D+00 |
| Q( 12) | 1 - 0 | 484.17 | -790.39 | 0.00000D+00 | 3.35719D-21 | 1.64464D-01 |
| Q( 12) | 1 - 1 | 1274.55 | 0.00 | 0.00000D+00 | 1.00000D+00 | 1.60591D+00 |
| Q( 13) | 1 - 0 | 498.33 | -790.26 | 0.00000D+00 | 3.37591D-21 | 1.64468D-01 |
| Q( 13) | 1 - 1 | 1288.59 | 0.00 | 0.00000D+00 | 1.00000D+00 | 1.60621D+00 |
| Q( 14) | 1 - 0 | 513.59 | -790.12 | 0.00000D+00 | 3.48158D-21 | 1.64473D-01 |
| Q( 14) | 1 - 1 | 1303.70 | -0.00 | 0.00000D+00 | 1.00000D+00 | 1.60654D+00 |
| Q( 15) | 1 - 0 | 529.93 | -789.97 | 0.00000D+00 | 3.53296D-21 | 1.64477D-01 |
| Q( 15) | 1 - 1 | 1319.90 | -0.00 | 0.00000D+00 | 1.00000D+00 | 1.60689D+00 |
| Q( 16) | 1 - 0 | 547.36 | -789.81 | 0.00000D+00 | 3.59255D-21 | 1.64482D-01 |
| Q( 16) | 1 - 1 | 1337.17 | -0.00 | 0.00000D+00 | 1.00000D+00 | 1.60726D+00 |
| Q( 17) | 1 - 0 | 565.88 | -789.64 | 0.00000D+00 | 3.80225D-21 | 1.64488D-01 |
| Q( 17) | 1 - 1 | 1355.51 | -0.00 | 0.00000D+00 | 1.00000D+00 | 1.60766D+00 |
| Q( 18) | 1 - 0 | 585.48 | -789.46 | 0.00000D+00 | 3.90500D-21 | 1.64493D-01 |
| Q( 18) | 1 - 1 | 1374.94 | -0.00 | 0.00000D+00 | 1.00000D+00 | 1.60808D+00 |
| Q( 19) | 1 - 0 | 606.17 | -789.27 | 0.00000D+00 | 4.03284D-21 | 1.64499D-01 |
| Q( 19) | 1 - 1 | 1395.44 | -0.00 | 0.00000D+00 | 1.00000D+00 | 1.60852D+00 |
| Q( 20) | 1 - 0 | 627.95 | -789.06 | 0.00000D+00 | 4.18521D-21 | 1.64506D-01 |
| Q( 20) | 1 - 1 | 1417.01 | -0.00 | 0.00000D+00 | 1.00000D+00 | 1.60899D+00 |
| Q( 0) | 2 - 0 | 399.14 | -1574.08 | 0.00000D+00 | 4.40584D-23 | 1.34294D-02 |
| Q( 0) | 2 - 1 | 1190.31 | -782.91 | 0.00000D+00 | 6.43798D-23 | -2.29728D-01 |
| Q( 0) | 2 - 2 | 1973.22 | 0.00 | 0.00000D+00 | 1.00000D+00 | -1.64074D+00 |
| Q( 1) | 2 - 0 | 400.23 | -1574.06 | 0.00000D+00 | 3.31592D-19 | 1.34297D-02 |

| | | | | | | | |
|---|---|---|---|---|---|---|---|
| Q( 1) | 2 - 1 | 1191.39 | -782.90 | 0.00000D+00 | 9.04106D-18 | -2.29729D-01 |
| Q( 1) | 2 - 2 | 1974.29 | -0.00 | 0.00000D+00 | 1.00000D+00 | -1.64076D+00 |
| Q( 2) | 2 - 0 | 402.41 | -1574.02 | 0.00000D+00 | 4.76457D-23 | 1.34303D-02 |
| Q( 2) | 2 - 1 | 1193.55 | -782.88 | 0.00000D+00 | 4.30729D-23 | -2.29730D-01 |
| Q( 2) | 2 - 2 | 1976.43 | 0.00 | 0.00000D+00 | 1.00000D+00 | -1.64081D+00 |
| Q( 3) | 2 - 0 | 405.68 | -1573.96 | 0.00000D+00 | 4.72515D-23 | 1.34312D-02 |
| Q( 3) | 2 - 1 | 1196.79 | -782.85 | 0.00000D+00 | 4.34020D-23 | -2.29731D-01 |
| Q( 3) | 2 - 2 | 1979.64 | 0.00 | 0.00000D+00 | 1.00000D+00 | -1.64088D+00 |
| Q( 4) | 2 - 0 | 410.04 | -1573.88 | 0.00000D+00 | 4.66485D-23 | 1.34323D-02 |
| Q( 4) | 2 - 1 | 1201.11 | -782.81 | 0.00000D+00 | 4.39694D-23 | -2.29733D-01 |
| Q( 4) | 2 - 2 | 1983.93 | 0.00 | 0.00000D+00 | 1.00000D+00 | -1.64097D+00 |
| Q( 5) | 2 - 0 | 415.49 | -1573.78 | 0.00000D+00 | 4.60590D-23 | 1.34338D-02 |
| Q( 5) | 2 - 1 | 1206.51 | -782.77 | 0.00000D+00 | 4.48588D-23 | -2.29735D-01 |
| Q( 5) | 2 - 2 | 1989.28 | 0.00 | 0.00000D+00 | 1.00000D+00 | -1.64109D+00 |
| Q( 6) | 2 - 0 | 422.03 | -1573.66 | 0.00000D+00 | 4.51611D-23 | 1.34355D-02 |
| Q( 6) | 2 - 1 | 1212.99 | -782.71 | 0.00000D+00 | 4.73415D-23 | -2.29738D-01 |
| Q( 6) | 2 - 2 | 1995.70 | 0.00 | 0.00000D+00 | 1.00000D+00 | -1.64123D+00 |
| Q( 7) | 2 - 0 | 429.67 | -1573.52 | 0.00000D+00 | 4.42745D-23 | 1.34376D-02 |
| Q( 7) | 2 - 1 | 1220.55 | -782.64 | 0.00000D+00 | 4.85264D-23 | -2.29741D-01 |
| Q( 7) | 2 - 2 | 2003.19 | 0.00 | 0.00000D+00 | 1.00000D+00 | -1.64139D+00 |
| Q( 8) | 2 - 0 | 438.39 | -1573.36 | 0.00000D+00 | 4.29231D-23 | 1.34399D-02 |
| Q( 8) | 2 - 1 | 1229.20 | -782.56 | 0.00000D+00 | 5.05503D-23 | -2.29744D-01 |
| Q( 8) | 2 - 2 | 2011.75 | 0.00 | 0.00000D+00 | 1.00000D+00 | -1.64158D+00 |
| Q( 9) | 2 - 0 | 448.20 | -1573.18 | 0.00000D+00 | 4.16072D-23 | 1.34425D-02 |
| Q( 9) | 2 - 1 | 1238.92 | -782.47 | 0.00000D+00 | 5.37880D-23 | -2.29748D-01 |
| Q( 9) | 2 - 2 | 2021.38 | 0.00 | 0.00000D+00 | 1.00000D+00 | -1.64179D+00 |
| Q( 10) | 2 - 0 | 459.10 | -1572.98 | 0.00000D+00 | 4.00375D-23 | 1.34454D-02 |
| Q( 10) | 2 - 1 | 1249.72 | -782.37 | 0.00000D+00 | 5.73729D-23 | -2.29753D-01 |
| Q( 10) | 2 - 2 | 2032.08 | 0.00 | 0.00000D+00 | 1.00000D+00 | -1.64203D+00 |

| | | | | | | |
|---|---|---|---|---|---|---|
| Q( 11) | 2 - 0 | 471.09 | -1572.76 | 0.00000D+00 | 3.82451D-23 | 1.34486D-02 |
| Q( 11) | 2 - 1 | 1261.60 | -782.26 | 0.00000D+00 | 6.27875D-23 | -2.29758D-01 |
| Q( 11) | 2 - 2 | 2043.85 | 0.00 | 0.00000D+00 | 1.00000D+00 | -1.64228D+00 |
| Q( 12) | 2 - 0 | 484.17 | -1572.52 | 0.00000D+00 | 3.60857D-23 | 1.34521D-02 |
| Q( 12) | 2 - 1 | 1274.55 | -782.14 | 0.00000D+00 | 6.93823D-23 | -2.29763D-01 |
| Q( 12) | 2 - 2 | 2056.69 | -0.00 | 0.00000D+00 | 1.00000D+00 | -1.64257D+00 |
| Q( 13) | 2 - 0 | 498.33 | -1572.26 | 0.00000D+00 | 3.37125D-23 | 1.34559D-02 |
| Q( 13) | 2 - 1 | 1288.59 | -782.01 | 0.00000D+00 | 7.81360D-23 | -2.29769D-01 |
| Q( 13) | 2 - 2 | 2070.60 | -0.00 | 0.00000D+00 | 1.00000D+00 | -1.64287D+00 |
| Q( 14) | 2 - 0 | 513.59 | -1571.98 | 0.00000D+00 | 3.11904D-23 | 1.34599D-02 |
| Q( 14) | 2 - 1 | 1303.70 | -781.87 | 0.00000D+00 | 9.06541D-23 | -2.29775D-01 |
| Q( 14) | 2 - 2 | 2085.57 | -0.00 | 0.00000D+00 | 1.00000D+00 | -1.64320D+00 |
| Q( 15) | 2 - 0 | 529.93 | -1571.68 | 0.00000D+00 | 2.83662D-23 | 1.34643D-02 |
| Q( 15) | 2 - 1 | 1319.90 | -781.72 | 0.00000D+00 | 1.05860D-22 | -2.29782D-01 |
| Q( 15) | 2 - 2 | 2101.61 | -0.00 | 0.00000D+00 | 1.00000D+00 | -1.64355D+00 |
| Q( 16) | 2 - 0 | 547.36 | -1571.36 | 0.00000D+00 | 2.52664D-23 | 1.34689D-02 |
| Q( 16) | 2 - 1 | 1337.17 | -781.56 | 0.00000D+00 | 1.26045D-22 | -2.29789D-01 |
| Q( 16) | 2 - 2 | 2118.72 | -0.00 | 0.00000D+00 | 1.00000D+00 | -1.64393D+00 |
| Q( 17) | 2 - 0 | 565.88 | -1571.02 | 0.00000D+00 | 3.09112D-23 | 1.34738D-02 |
| Q( 17) | 2 - 1 | 1355.51 | -781.39 | 0.00000D+00 | 1.53290D-22 | -2.29797D-01 |
| Q( 17) | 2 - 2 | 2136.90 | -0.00 | 0.00000D+00 | 1.00000D+00 | -1.64433D+00 |
| Q( 18) | 2 - 0 | 585.48 | -1570.66 | 0.00000D+00 | 2.32786D-23 | 1.34790D-02 |
| Q( 18) | 2 - 1 | 1374.94 | -781.21 | 0.00000D+00 | 2.40781D-22 | -2.29805D-01 |
| Q( 18) | 2 - 2 | 2156.15 | -0.00 | 0.00000D+00 | 1.00000D+00 | -1.64475D+00 |
| Q( 19) | 2 - 0 | 606.17 | -1570.29 | 0.00000D+00 | 1.88960D-23 | 1.34845D-02 |
| Q( 19) | 2 - 1 | 1395.44 | -781.02 | 0.00000D+00 | 2.97523D-22 | -2.29813D-01 |
| Q( 19) | 2 - 2 | 2176.46 | -0.00 | 0.00000D+00 | 1.00000D+00 | -1.64519D+00 |
| Q( 20) | 2 - 0 | 627.95 | -1569.89 | 0.00000D+00 | 1.46157D-23 | 1.34902D-02 |
| Q( 20) | 2 - 1 | 1417.01 | -780.82 | 0.00000D+00 | 3.71240D-22 | -2.29822D-01 |

| | | | | | | | |
|---|---|---|---|---|---|---|---|
| Q( 20) | 2 - 2 | 2197.83 | -0.00 | 0.00000D+00 | 1.00000D+00 | -1.64566D+00 |
| Q( 0) | 3 - 0 | 399.14 | -2346.46 | 0.00000D+00 | 1.88978D-22 | 7.04278D-04 |
| Q( 0) | 3 - 1 | 1190.31 | -1555.29 | 0.00000D+00 | 2.53174D-24 | -2.30300D-02 |
| Q( 0) | 3 - 2 | 1973.22 | -772.37 | 0.00000D+00 | 2.87692D-23 | 2.78639D-01 |
| Q( 0) | 3 - 3 | 2745.59 | 0.00 | 0.00000D+00 | 1.00000D+00 | 1.67835D+00 |
| Q( 1) | 3 - 0 | 400.23 | -2346.43 | 0.00000D+00 | 3.20465D-20 | 7.04394D-04 |
| Q( 1) | 3 - 1 | 1191.39 | -1555.27 | 0.00000D+00 | 7.03731D-19 | -2.30306D-02 |
| Q( 1) | 3 - 2 | 1974.29 | -772.36 | 0.00000D+00 | 1.14598D-17 | 2.78639D-01 |
| Q( 1) | 3 - 3 | 2746.65 | -0.00 | 0.00000D+00 | 1.00000D+00 | 1.67838D+00 |
| Q( 2) | 3 - 0 | 402.41 | -2346.37 | 0.00000D+00 | 1.91309D-22 | 7.04628D-04 |
| Q( 2) | 3 - 1 | 1193.55 | -1555.23 | 0.00000D+00 | 3.91027D-24 | -2.30316D-02 |
| Q( 2) | 3 - 2 | 1976.43 | -772.34 | 0.00000D+00 | 1.44931D-23 | 2.78641D-01 |
| Q( 2) | 3 - 3 | 2748.77 | 0.00 | 0.00000D+00 | 1.00000D+00 | 1.67842D+00 |
| Q( 3) | 3 - 0 | 405.68 | -2346.27 | 0.00000D+00 | 1.91155D-22 | 7.04978D-04 |
| Q( 3) | 3 - 1 | 1196.79 | -1555.16 | 0.00000D+00 | 3.87543D-24 | -2.30332D-02 |
| Q( 3) | 3 - 2 | 1979.64 | -772.31 | 0.00000D+00 | 1.46240D-23 | 2.78642D-01 |
| Q( 3) | 3 - 3 | 2751.95 | 0.00 | 0.00000D+00 | 1.00000D+00 | 1.67849D+00 |
| Q( 4) | 3 - 0 | 410.04 | -2346.15 | 0.00000D+00 | 1.90495D-22 | 7.05445D-04 |
| Q( 4) | 3 - 1 | 1201.11 | -1555.08 | 0.00000D+00 | 3.81380D-24 | -2.30353D-02 |
| Q( 4) | 3 - 2 | 1983.93 | -772.27 | 0.00000D+00 | 1.47900D-23 | 2.78644D-01 |
| Q( 4) | 3 - 3 | 2756.19 | 0.00 | 0.00000D+00 | 1.00000D+00 | 1.67859D+00 |
| Q( 5) | 3 - 0 | 415.49 | -2346.00 | 0.00000D+00 | 1.90078D-22 | 7.06029D-04 |
| Q( 5) | 3 - 1 | 1206.51 | -1554.98 | 0.00000D+00 | 3.75101D-24 | -2.30379D-02 |
| Q( 5) | 3 - 2 | 1989.28 | -772.22 | 0.00000D+00 | 1.53322D-23 | 2.78647D-01 |
| Q( 5) | 3 - 3 | 2761.49 | 0.00 | 0.00000D+00 | 1.00000D+00 | 1.67870D+00 |
| Q( 6) | 3 - 0 | 422.03 | -2345.82 | 0.00000D+00 | 1.89549D-22 | 7.06730D-04 |
| Q( 6) | 3 - 1 | 1212.99 | -1554.86 | 0.00000D+00 | 4.02220D-24 | -2.30410D-02 |
| Q( 6) | 3 - 2 | 1995.70 | -772.15 | 0.00000D+00 | 1.58935D-23 | 2.78650D-01 |
| Q( 6) | 3 - 3 | 2767.85 | 0.00 | 0.00000D+00 | 1.00000D+00 | 1.67884D+00 |

| | | | | | | |
|---|---|---|---|---|---|---|
| Q( 7) | 3 - 0 | 429.67 | -2345.60 | 0.00000D+00 | 1.88896D-22 | 7.07548D-04 |
| Q( 7) | 3 - 1 | 1220.55 | -1554.71 | 0.00000D+00 | 3.87955D-24 | -2.30447D-02 |
| Q( 7) | 3 - 2 | 2003.19 | -772.08 | 0.00000D+00 | 1.69748D-23 | 2.78653D-01 |
| Q( 7) | 3 - 3 | 2775.27 | 0.00 | 0.00000D+00 | 1.00000D+00 | 1.67901D+00 |
| Q( 8) | 3 - 0 | 438.39 | -2345.36 | 0.00000D+00 | 1.88116D-22 | 7.08483D-04 |
| Q( 8) | 3 - 1 | 1229.20 | -1554.55 | 0.00000D+00 | 3.65994D-24 | -2.30488D-02 |
| Q( 8) | 3 - 2 | 2011.75 | -772.00 | 0.00000D+00 | 1.83426D-23 | 2.78657D-01 |
| Q( 8) | 3 - 3 | 2783.75 | 0.00 | 0.00000D+00 | 1.00000D+00 | 1.67920D+00 |
| Q( 9) | 3 - 0 | 448.20 | -2345.09 | 0.00000D+00 | 1.87046D-22 | 7.09535D-04 |
| Q( 9) | 3 - 1 | 1238.92 | -1554.37 | 0.00000D+00 | 3.44120D-24 | -2.30535D-02 |
| Q( 9) | 3 - 2 | 2021.38 | -771.90 | 0.00000D+00 | 2.00172D-23 | 2.78662D-01 |
| Q( 9) | 3 - 3 | 2793.28 | 0.00 | 0.00000D+00 | 1.00000D+00 | 1.67941D+00 |
| Q( 10) | 3 - 0 | 459.10 | -2344.78 | 0.00000D+00 | 1.86049D-22 | 7.10704D-04 |
| Q( 10) | 3 - 1 | 1249.72 | -1554.16 | 0.00000D+00 | 3.13544D-24 | -2.30588D-02 |
| Q( 10) | 3 - 2 | 2032.08 | -771.80 | 0.00000D+00 | 2.29397D-23 | 2.78667D-01 |
| Q( 10) | 3 - 3 | 2803.88 | 0.00 | 0.00000D+00 | 1.00000D+00 | 1.67964D+00 |
| Q( 11) | 3 - 0 | 471.09 | -2344.45 | 0.00000D+00 | 1.84755D-22 | 7.11991D-04 |
| Q( 11) | 3 - 1 | 1261.60 | -1553.94 | 0.00000D+00 | 2.75602D-24 | -2.30645D-02 |
| Q( 11) | 3 - 2 | 2043.85 | -771.68 | 0.00000D+00 | 2.62793D-23 | 2.78673D-01 |
| Q( 11) | 3 - 3 | 2815.53 | 0.00 | 0.00000D+00 | 1.00000D+00 | 1.67990D+00 |
| Q( 12) | 3 - 0 | 484.17 | -2344.08 | 0.00000D+00 | 1.83133D-22 | 7.13396D-04 |
| Q( 12) | 3 - 1 | 1274.55 | -1553.69 | 0.00000D+00 | 2.31824D-24 | -2.30708D-02 |
| Q( 12) | 3 - 2 | 2056.69 | -771.56 | 0.00000D+00 | 3.12605D-23 | 2.78679D-01 |
| Q( 12) | 3 - 3 | 2828.25 | -0.00 | 0.00000D+00 | 1.00000D+00 | 1.68018D+00 |
| Q( 13) | 3 - 0 | 498.33 | -2343.68 | 0.00000D+00 | 1.81362D-22 | 7.14919D-04 |
| Q( 13) | 3 - 1 | 1288.59 | -1553.43 | 0.00000D+00 | 1.84650D-24 | -2.30776D-02 |
| Q( 13) | 3 - 2 | 2070.60 | -771.42 | 0.00000D+00 | 3.82904D-23 | 2.78685D-01 |
| Q( 13) | 3 - 3 | 2842.02 | -0.00 | 0.00000D+00 | 1.00000D+00 | 1.68049D+00 |
| Q( 14) | 3 - 0 | 513.59 | -2343.26 | 0.00000D+00 | 1.76961D-22 | 7.16559D-04 |

| | | | | | | | |
|---|---|---|---|---|---|---|---|
| Q( 14) | 3 - 1 | 1303.70 | -1553.14 | 0.00000D+00 | 6.29694D-25 | -2.30849D-02 |
| Q( 14) | 3 - 2 | 2085.57 | -771.27 | 0.00000D+00 | 7.14205D-23 | 2.78693D-01 |
| Q( 14) | 3 - 3 | 2856.84 | -0.00 | 0.00000D+00 | 1.00000D+00 | 1.68081D+00 |
| Q( 15) | 3 - 0 | 529.93 | -2342.80 | 0.00000D+00 | 1.74420D-22 | 7.18318D-04 |
| Q( 15) | 3 - 1 | 1319.90 | -1552.83 | 0.00000D+00 | 2.41745D-25 | -2.30928D-02 |
| Q( 15) | 3 - 2 | 2101.61 | -771.12 | 0.00000D+00 | 9.15081D-23 | 2.78700D-01 |
| Q( 15) | 3 - 3 | 2872.73 | -0.00 | 0.00000D+00 | 1.00000D+00 | 1.68117D+00 |
| Q( 16) | 3 - 0 | 547.36 | -2342.31 | 0.00000D+00 | 1.71269D-22 | 7.20195D-04 |
| Q( 16) | 3 - 1 | 1337.17 | -1552.51 | 0.00000D+00 | 2.23262D-26 | -2.31012D-02 |
| Q( 16) | 3 - 2 | 2118.72 | -770.95 | 0.00000D+00 | 1.17341D-22 | 2.78708D-01 |
| Q( 16) | 3 - 3 | 2889.67 | -0.00 | 0.00000D+00 | 1.00000D+00 | 1.68154D+00 |
| Q( 17) | 3 - 0 | 565.88 | -2341.80 | 0.00000D+00 | 1.67999D-22 | 7.22190D-04 |
| Q( 17) | 3 - 1 | 1355.51 | -1552.16 | 0.00000D+00 | 6.06297D-26 | -2.31102D-02 |
| Q( 17) | 3 - 2 | 2136.90 | -770.77 | 0.00000D+00 | 1.52135D-22 | 2.78717D-01 |
| Q( 17) | 3 - 3 | 2907.67 | -0.00 | 0.00000D+00 | 1.00000D+00 | 1.68194D+00 |
| Q( 18) | 3 - 0 | 585.48 | -2341.25 | 0.00000D+00 | 1.64435D-22 | 7.24304D-04 |
| Q( 18) | 3 - 1 | 1374.94 | -1551.79 | 0.00000D+00 | 3.56098D-25 | -2.31196D-02 |
| Q( 18) | 3 - 2 | 2156.15 | -770.58 | 0.00000D+00 | 1.97708D-22 | 2.78726D-01 |
| Q( 18) | 3 - 3 | 2926.73 | -0.00 | 0.00000D+00 | 1.00000D+00 | 1.68236D+00 |
| Q( 19) | 3 - 0 | 606.17 | -2340.67 | 0.00000D+00 | 1.60409D-22 | 7.26537D-04 |
| Q( 19) | 3 - 1 | 1395.44 | -1551.40 | 0.00000D+00 | 1.24166D-24 | -2.31296D-02 |
| Q( 19) | 3 - 2 | 2176.46 | -770.38 | 0.00000D+00 | 2.58921D-22 | 2.78735D-01 |
| Q( 19) | 3 - 3 | 2946.84 | -0.00 | 0.00000D+00 | 1.00000D+00 | 1.68281D+00 |
| Q( 20) | 3 - 0 | 627.95 | -2340.06 | 0.00000D+00 | 1.56078D-22 | 7.28890D-04 |
| Q( 20) | 3 - 1 | 1417.01 | -1550.99 | 0.00000D+00 | 2.98646D-24 | -2.31402D-02 |
| Q( 20) | 3 - 2 | 2197.83 | -770.17 | 0.00000D+00 | 3.39692D-22 | 2.78745D-01 |
| Q( 20) | 3 - 3 | 2968.01 | -0.00 | 0.00000D+00 | 1.00000D+00 | 1.68328D+00 |
| Q( 0) | 4 - 0 | 399.14 | -3107.26 | 0.00000D+00 | 2.06665D-23 | -2.79773D-04 |
| Q( 0) | 4 - 1 | 1190.31 | -2316.09 | 0.00000D+00 | 3.90024D-25 | -1.61394D-03 |

| | | | | | | | |
|---|---|---|---|---|---|---|---|
| Q( 0) | 4 - 2 | 1973.22 | -1533.18 | 0.00000D+00 | 7.20561D-25 | 3.32055D-02 |
| Q( 0) | 4 - 3 | 2745.59 | -760.81 | 0.00000D+00 | 3.35602D-23 | -3.18160D-01 |
| Q( 0) | 4 - 4 | 3506.40 | 0.00 | 0.00000D+00 | 1.00000D+00 | -1.71544D+00 |
| Q( 1) | 4 - 0 | 400.23 | -3107.22 | 0.00000D+00 | 6.53222D-21 | -2.79763D-04 |
| Q( 1) | 4 - 1 | 1191.39 | -2316.06 | 0.00000D+00 | 1.02928D-19 | -1.61405D-03 |
| Q( 1) | 4 - 2 | 1974.29 | -1533.16 | 0.00000D+00 | 1.12934D-18 | 3.32063D-02 |
| Q( 1) | 4 - 3 | 2746.65 | -760.80 | 0.00000D+00 | 1.40923D-17 | -3.18160D-01 |
| Q( 1) | 4 - 4 | 3507.45 | -0.00 | 0.00000D+00 | 1.00000D+00 | -1.71546D+00 |
| Q( 2) | 4 - 0 | 402.41 | -3107.14 | 0.00000D+00 | 2.01784D-23 | -2.79743D-04 |
| Q( 2) | 4 - 1 | 1193.55 | -2316.00 | 0.00000D+00 | 6.45627D-25 | -1.61429D-03 |
| Q( 2) | 4 - 2 | 1976.43 | -1533.12 | 0.00000D+00 | 2.05899D-24 | 3.32081D-02 |
| Q( 2) | 4 - 3 | 2748.77 | -760.77 | 0.00000D+00 | 1.37780D-23 | -3.18160D-01 |
| Q( 2) | 4 - 4 | 3509.55 | 0.00 | 0.00000D+00 | 1.00000D+00 | -1.71551D+00 |
| Q( 3) | 4 - 0 | 405.68 | -3107.02 | 0.00000D+00 | 2.00723D-23 | -2.79713D-04 |
| Q( 3) | 4 - 1 | 1196.79 | -2315.91 | 0.00000D+00 | 6.49984D-25 | -1.61463D-03 |
| Q( 3) | 4 - 2 | 1979.64 | -1533.05 | 0.00000D+00 | 2.00864D-24 | 3.32107D-02 |
| Q( 3) | 4 - 3 | 2751.95 | -760.74 | 0.00000D+00 | 1.41000D-23 | -3.18161D-01 |
| Q( 3) | 4 - 4 | 3512.70 | 0.00 | 0.00000D+00 | 1.00000D+00 | -1.71558D+00 |
| Q( 4) | 4 - 0 | 410.04 | -3106.85 | 0.00000D+00 | 1.99190D-23 | -2.79672D-04 |
| Q( 4) | 4 - 1 | 1201.11 | -2315.78 | 0.00000D+00 | 6.32292D-25 | -1.61510D-03 |
| Q( 4) | 4 - 2 | 1983.93 | -1532.97 | 0.00000D+00 | 1.91156D-24 | 3.32142D-02 |
| Q( 4) | 4 - 3 | 2756.19 | -760.70 | 0.00000D+00 | 1.45907D-23 | -3.18162D-01 |
| Q( 4) | 4 - 4 | 3516.89 | 0.00 | 0.00000D+00 | 1.00000D+00 | -1.71568D+00 |
| Q( 5) | 4 - 0 | 415.49 | -3106.65 | 0.00000D+00 | 1.97759D-23 | -2.79621D-04 |
| Q( 5) | 4 - 1 | 1206.51 | -2315.63 | 0.00000D+00 | 6.24633D-25 | -1.61567D-03 |
| Q( 5) | 4 - 2 | 1989.28 | -1532.86 | 0.00000D+00 | 1.83301D-24 | 3.32185D-02 |
| Q( 5) | 4 - 3 | 2761.49 | -760.65 | 0.00000D+00 | 1.55246D-23 | -3.18164D-01 |
| Q( 5) | 4 - 4 | 3522.14 | 0.00 | 0.00000D+00 | 1.00000D+00 | -1.71579D+00 |
| Q( 6) | 4 - 0 | 422.03 | -3106.40 | 0.00000D+00 | 1.95805D-23 | -2.79559D-04 |

| | | | | | | | |
|---|---|---|---|---|---|---|---|
| Q( 6) | 4 - 1 | 1212.99 | -2315.44 | 0.00000D+00 | 5.30106D-25 | -1.61637D-03 |
| Q( 6) | 4 - 2 | 1995.70 | -1532.73 | 0.00000D+00 | 1.67103D-24 | 3.32238D-02 |
| Q( 6) | 4 - 3 | 2767.85 | -760.58 | 0.00000D+00 | 1.68762D-23 | -3.18165D-01 |
| Q( 6) | 4 - 4 | 3528.43 | 0.00 | 0.00000D+00 | 1.00000D+00 | -1.71593D+00 |
| Q( 7) | 4 - 0 | 429.67 | -3106.11 | 0.00000D+00 | 1.93641D-23 | -2.79486D-04 |
| Q( 7) | 4 - 1 | 1220.55 | -2315.22 | 0.00000D+00 | 5.05131D-25 | -1.61718D-03 |
| Q( 7) | 4 - 2 | 2003.19 | -1532.58 | 0.00000D+00 | 1.54742D-24 | 3.32299D-02 |
| Q( 7) | 4 - 3 | 2775.27 | -760.51 | 0.00000D+00 | 1.86084D-23 | -3.18167D-01 |
| Q( 7) | 4 - 4 | 3535.77 | 0.00 | 0.00000D+00 | 1.00000D+00 | -1.71610D+00 |
| Q( 8) | 4 - 0 | 438.39 | -3105.78 | 0.00000D+00 | 1.91012D-23 | -2.79401D-04 |
| Q( 8) | 4 - 1 | 1229.20 | -2314.97 | 0.00000D+00 | 4.68936D-25 | -1.61810D-03 |
| Q( 8) | 4 - 2 | 2011.75 | -1532.42 | 0.00000D+00 | 1.33341D-24 | 3.32369D-02 |
| Q( 8) | 4 - 3 | 2783.75 | -760.42 | 0.00000D+00 | 2.07666D-23 | -3.18169D-01 |
| Q( 8) | 4 - 4 | 3544.17 | 0.00 | 0.00000D+00 | 1.00000D+00 | -1.71629D+00 |
| Q( 9) | 4 - 0 | 448.20 | -3105.41 | 0.00000D+00 | 1.88209D-23 | -2.79304D-04 |
| Q( 9) | 4 - 1 | 1238.92 | -2314.69 | 0.00000D+00 | 4.36961D-25 | -1.61914D-03 |
| Q( 9) | 4 - 2 | 2021.38 | -1532.22 | 0.00000D+00 | 1.08315D-24 | 3.32447D-02 |
| Q( 9) | 4 - 3 | 2793.28 | -760.32 | 0.00000D+00 | 2.39300D-23 | -3.18172D-01 |
| Q( 9) | 4 - 4 | 3553.61 | 0.00 | 0.00000D+00 | 1.00000D+00 | -1.71650D+00 |
| Q( 10) | 4 - 0 | 459.10 | -3105.00 | 0.00000D+00 | 1.85424D-23 | -2.79195D-04 |
| Q( 10) | 4 - 1 | 1249.72 | -2314.38 | 0.00000D+00 | 3.87807D-25 | -1.62029D-03 |
| Q( 10) | 4 - 2 | 2032.08 | -1532.01 | 0.00000D+00 | 8.57730D-25 | 3.32535D-02 |
| Q( 10) | 4 - 3 | 2803.88 | -760.22 | 0.00000D+00 | 2.83318D-23 | -3.18174D-01 |
| Q( 10) | 4 - 4 | 3564.09 | 0.00 | 0.00000D+00 | 1.00000D+00 | -1.71673D+00 |
| Q( 11) | 4 - 0 | 471.09 | -3104.54 | 0.00000D+00 | 1.82731D-23 | -2.79073D-04 |
| Q( 11) | 4 - 1 | 1261.60 | -2314.04 | 0.00000D+00 | 3.39158D-25 | -1.62156D-03 |
| Q( 11) | 4 - 2 | 2043.85 | -1531.78 | 0.00000D+00 | 5.74894D-25 | 3.32631D-02 |
| Q( 11) | 4 - 3 | 2815.53 | -760.10 | 0.00000D+00 | 3.39013D-23 | -3.18177D-01 |
| Q( 11) | 4 - 4 | 3575.63 | -0.00 | 0.00000D+00 | 1.00000D+00 | -1.71699D+00 |

| | | | | | | |
|---|---|---|---|---|---|---|
| Q( 12) | 4 - 0 | 484.17 | -3104.05 | 0.00000D+00 | 1.79246D-23 | -2.78937D-04 |
| Q( 12) | 4 - 1 | 1274.55 | -2313.66 | 0.00000D+00 | 2.77197D-25 | -1.62294D-03 |
| Q( 12) | 4 - 2 | 2056.69 | -1531.52 | 0.00000D+00 | 3.13256D-25 | 3.32736D-02 |
| Q( 12) | 4 - 3 | 2828.25 | -759.97 | 0.00000D+00 | 4.18077D-23 | -3.18181D-01 |
| Q( 12) | 4 - 4 | 3588.21 | -0.00 | 0.00000D+00 | 1.00000D+00 | -1.71727D+00 |
| Q( 13) | 4 - 0 | 498.33 | -3103.51 | 0.00000D+00 | 1.76286D-23 | -2.78788D-04 |
| Q( 13) | 4 - 1 | 1288.59 | -2313.26 | 0.00000D+00 | 2.13663D-25 | -1.62443D-03 |
| Q( 13) | 4 - 2 | 2070.60 | -1531.25 | 0.00000D+00 | 1.07667D-25 | 3.32850D-02 |
| Q( 13) | 4 - 3 | 2842.02 | -759.83 | 0.00000D+00 | 5.35948D-23 | -3.18184D-01 |
| Q( 13) | 4 - 4 | 3601.84 | -0.00 | 0.00000D+00 | 1.00000D+00 | -1.71758D+00 |
| Q( 14) | 4 - 0 | 513.59 | -3102.94 | 0.00000D+00 | 1.72897D-23 | -2.78623D-04 |
| Q( 14) | 4 - 1 | 1303.70 | -2312.82 | 0.00000D+00 | 1.51780D-25 | -1.62604D-03 |
| Q( 14) | 4 - 2 | 2085.57 | -1530.95 | 0.00000D+00 | 1.22430D-26 | 3.32973D-02 |
| Q( 14) | 4 - 3 | 2856.84 | -759.68 | 0.00000D+00 | 6.78914D-23 | -3.18188D-01 |
| Q( 14) | 4 - 4 | 3616.52 | -0.00 | 0.00000D+00 | 1.00000D+00 | -1.71791D+00 |
| Q( 15) | 4 - 0 | 529.93 | -3102.32 | 0.00000D+00 | 1.69789D-23 | -2.78442D-04 |
| Q( 15) | 4 - 1 | 1319.90 | -2312.35 | 0.00000D+00 | 8.31278D-26 | -1.62776D-03 |
| Q( 15) | 4 - 2 | 2101.61 | -1530.63 | 0.00000D+00 | 5.10160D-26 | 3.33105D-02 |
| Q( 15) | 4 - 3 | 2872.73 | -759.52 | 0.00000D+00 | 8.81028D-23 | -3.18191D-01 |
| Q( 15) | 4 - 4 | 3632.25 | -0.00 | 0.00000D+00 | 1.00000D+00 | -1.71826D+00 |
| Q( 16) | 4 - 0 | 547.36 | -3101.66 | 0.00000D+00 | 1.66985D-23 | -2.78245D-04 |
| Q( 16) | 4 - 1 | 1337.17 | -2311.85 | 0.00000D+00 | 3.15235D-26 | -1.62959D-03 |
| Q( 16) | 4 - 2 | 2118.72 | -1530.29 | 0.00000D+00 | 3.90043D-25 | 3.33245D-02 |
| Q( 16) | 4 - 3 | 2889.67 | -759.34 | 0.00000D+00 | 1.14754D-22 | -3.18196D-01 |
| Q( 16) | 4 - 4 | 3649.02 | -0.00 | 0.00000D+00 | 1.00000D+00 | -1.71864D+00 |
| Q( 17) | 4 - 0 | 565.88 | -3100.96 | 0.00000D+00 | 2.06462D-23 | -2.78031D-04 |
| Q( 17) | 4 - 1 | 1355.51 | -2311.32 | 0.00000D+00 | 1.84388D-27 | -1.63153D-03 |
| Q( 17) | 4 - 2 | 2136.90 | -1529.93 | 0.00000D+00 | 1.18236D-24 | 3.33395D-02 |
| Q( 17) | 4 - 3 | 2907.67 | -759.16 | 0.00000D+00 | 1.52080D-22 | -3.18200D-01 |

| | | | | | | | |
|---|---|---|---|---|---|---|---|
| Q( 17) | 4 - 4 | 3666.83 | -0.00 | 0.00000D+00 | 1.00000D+00 | -1.71904D+00 |
| Q( 18) | 4 - 0 | 585.48 | -3100.21 | 0.00000D+00 | 2.03178D-23 | -2.77798D-04 |
| Q( 18) | 4 - 1 | 1374.94 | -2310.76 | 0.00000D+00 | 2.61090D-26 | -1.63358D-03 |
| Q( 18) | 4 - 2 | 2156.15 | -1529.55 | 0.00000D+00 | 2.69406D-24 | 3.33554D-02 |
| Q( 18) | 4 - 3 | 2926.73 | -758.97 | 0.00000D+00 | 2.01526D-22 | -3.18204D-01 |
| Q( 18) | 4 - 4 | 3685.69 | -0.00 | 0.00000D+00 | 1.00000D+00 | -1.71946D+00 |
| Q( 19) | 4 - 0 | 606.17 | -3099.43 | 0.00000D+00 | 2.06922D-23 | -2.77546D-04 |
| Q( 19) | 4 - 1 | 1395.44 | -2310.17 | 0.00000D+00 | 4.23664D-25 | -1.63574D-03 |
| Q( 19) | 4 - 2 | 2176.46 | -1529.15 | 0.00000D+00 | 1.05873D-23 | 3.33722D-02 |
| Q( 19) | 4 - 3 | 2946.84 | -758.76 | 0.00000D+00 | 3.92186D-22 | -3.18209D-01 |
| Q( 19) | 4 - 4 | 3705.60 | -0.00 | 0.00000D+00 | 1.00000D+00 | -1.71991D+00 |
| Q( 20) | 4 - 0 | 627.95 | -3098.61 | 0.00000D+00 | 2.04847D-23 | -2.77274D-04 |
| Q( 20) | 4 - 1 | 1417.01 | -2309.54 | 0.00000D+00 | 7.98776D-25 | -1.63802D-03 |
| Q( 20) | 4 - 2 | 2197.83 | -1528.72 | 0.00000D+00 | 1.67238D-23 | 3.33898D-02 |
| Q( 20) | 4 - 3 | 2968.01 | -758.55 | 0.00000D+00 | 5.13452D-22 | -3.18214D-01 |
| Q( 20) | 4 - 4 | 3726.55 | -0.00 | 0.00000D+00 | 1.00000D+00 | -1.72038D+00 |
| Q( 0) | 5 - 0 | 399.14 | -3854.83 | 0.00000D+00 | 5.57210D-23 | -1.04214D-04 |
| Q( 0) | 5 - 1 | 1190.31 | -3063.66 | 0.00000D+00 | 1.57311D-24 | 1.99284D-04 |
| Q( 0) | 5 - 2 | 1973.22 | -2280.75 | 0.00000D+00 | 1.84782D-27 | 2.48314D-03 |
| Q( 0) | 5 - 3 | 2745.59 | -1508.38 | 0.00000D+00 | 1.04167D-24 | -4.44312D-02 |
| Q( 0) | 5 - 4 | 3506.40 | -747.57 | 0.00000D+00 | 3.87406D-23 | 3.50568D-01 |
| Q( 0) | 5 - 5 | 4253.97 | 0.00 | 0.00000D+00 | 1.00000D+00 | 1.75116D+00 |
| Q( 1) | 5 - 0 | 400.23 | -3854.78 | 0.00000D+00 | 1.58309D-21 | -1.04265D-04 |
| Q( 1) | 5 - 1 | 1191.39 | -3063.62 | 0.00000D+00 | 1.91165D-20 | 1.99205D-04 |
| Q( 1) | 5 - 2 | 1974.29 | -2280.72 | 0.00000D+00 | 1.89109D-19 | 2.48321D-03 |
| Q( 1) | 5 - 3 | 2746.65 | -1508.35 | 0.00000D+00 | 1.55914D-18 | -4.44327D-02 |
| Q( 1) | 5 - 4 | 3507.45 | -747.56 | 0.00000D+00 | 1.67100D-17 | 3.50568D-01 |
| Q( 1) | 5 - 5 | 4255.01 | -0.00 | 0.00000D+00 | 1.00000D+00 | 1.75118D+00 |
| Q( 2) | 5 - 0 | 402.41 | -3854.68 | 0.00000D+00 | 5.54698D-23 | -1.04367D-04 |

| | | | | | | | |
|---|---|---|---|---|---|---|---|
| Q( 2) | 5 - 1 | 1193.55 | -3063.54 | 0.00000D+00 | 1.43653D-24 | 1.99048D-04 |
| Q( 2) | 5 - 2 | 1976.43 | -2280.65 | 0.00000D+00 | 1.86933D-26 | 2.48336D-03 |
| Q( 2) | 5 - 3 | 2748.77 | -1508.31 | 0.00000D+00 | 2.31565D-24 | -4.44357D-02 |
| Q( 2) | 5 - 4 | 3509.55 | -747.54 | 0.00000D+00 | 2.11684D-23 | 3.50567D-01 |
| Q( 2) | 5 - 5 | 4257.08 | 0.00 | 0.00000D+00 | 1.00000D+00 | 1.75123D+00 |
| Q( 3) | 5 - 0 | 405.68 | -3854.52 | 0.00000D+00 | 5.54713D-23 | -1.04521D-04 |
| Q( 3) | 5 - 1 | 1196.79 | -3063.41 | 0.00000D+00 | 1.42819D-24 | 1.98812D-04 |
| Q( 3) | 5 - 2 | 1979.64 | -2280.55 | 0.00000D+00 | 1.95868D-26 | 2.48357D-03 |
| Q( 3) | 5 - 3 | 2751.95 | -1508.24 | 0.00000D+00 | 2.31062D-24 | -4.44402D-02 |
| Q( 3) | 5 - 4 | 3512.70 | -747.50 | 0.00000D+00 | 2.11776D-23 | 3.50566D-01 |
| Q( 3) | 5 - 5 | 4260.20 | 0.00 | 0.00000D+00 | 1.00000D+00 | 1.75130D+00 |
| Q( 4) | 5 - 0 | 410.04 | -3854.31 | 0.00000D+00 | 5.53218D-23 | -1.04726D-04 |
| Q( 4) | 5 - 1 | 1201.11 | -3063.24 | 0.00000D+00 | 1.43132D-24 | 1.98496D-04 |
| Q( 4) | 5 - 2 | 1983.93 | -2280.43 | 0.00000D+00 | 1.86047D-26 | 2.48386D-03 |
| Q( 4) | 5 - 3 | 2756.19 | -1508.16 | 0.00000D+00 | 2.29728D-24 | -4.44463D-02 |
| Q( 4) | 5 - 4 | 3516.89 | -747.46 | 0.00000D+00 | 2.13205D-23 | 3.50564D-01 |
| Q( 4) | 5 - 5 | 4264.35 | 0.00 | 0.00000D+00 | 1.00000D+00 | 1.75139D+00 |
| Q( 5) | 5 - 0 | 415.49 | -3854.05 | 0.00000D+00 | 5.52361D-23 | -1.04982D-04 |
| Q( 5) | 5 - 1 | 1206.51 | -3063.03 | 0.00000D+00 | 1.43869D-24 | 1.98101D-04 |
| Q( 5) | 5 - 2 | 1989.28 | -2280.26 | 0.00000D+00 | 1.69143D-26 | 2.48422D-03 |
| Q( 5) | 5 - 3 | 2761.49 | -1508.05 | 0.00000D+00 | 2.20815D-24 | -4.44539D-02 |
| Q( 5) | 5 - 4 | 3522.14 | -747.40 | 0.00000D+00 | 2.16226D-23 | 3.50562D-01 |
| Q( 5) | 5 - 5 | 4269.54 | 0.00 | 0.00000D+00 | 1.00000D+00 | 1.75151D+00 |
| Q( 6) | 5 - 0 | 422.03 | -3853.73 | 0.00000D+00 | 5.51326D-23 | -1.05289D-04 |
| Q( 6) | 5 - 1 | 1212.99 | -3062.77 | 0.00000D+00 | 1.51619D-24 | 1.97627D-04 |
| Q( 6) | 5 - 2 | 1995.70 | -2280.07 | 0.00000D+00 | 1.51662D-26 | 2.48465D-03 |
| Q( 6) | 5 - 3 | 2767.85 | -1507.92 | 0.00000D+00 | 2.15521D-24 | -4.44630D-02 |
| Q( 6) | 5 - 4 | 3528.43 | -747.34 | 0.00000D+00 | 2.23162D-23 | 3.50560D-01 |
| Q( 6) | 5 - 5 | 4275.77 | 0.00 | 0.00000D+00 | 1.00000D+00 | 1.75165D+00 |

| | | | | | | | |
|---|---|---|---|---|---|---|---|
| Q( 7) | 5 - 0 | 429.67 | -3853.37 | 0.00000D+00 | 5.50737D-23 | -1.05647D-04 |
| Q( 7) | 5 - 1 | 1220.55 | -3062.48 | 0.00000D+00 | 1.51794D-24 | 1.97073D-04 |
| Q( 7) | 5 - 2 | 2003.19 | -2279.84 | 0.00000D+00 | 1.26868D-26 | 2.48514D-03 |
| Q( 7) | 5 - 3 | 2775.27 | -1507.76 | 0.00000D+00 | 2.02701D-24 | -4.44736D-02 |
| Q( 7) | 5 - 4 | 3535.77 | -747.26 | 0.00000D+00 | 2.35912D-23 | 3.50558D-01 |
| Q( 7) | 5 - 5 | 4283.03 | 0.00 | 0.00000D+00 | 1.00000D+00 | 1.75181D+00 |
| Q( 8) | 5 - 0 | 438.39 | -3852.95 | 0.00000D+00 | 5.49159D-23 | -1.06057D-04 |
| Q( 8) | 5 - 1 | 1229.20 | -3062.14 | 0.00000D+00 | 1.51785D-24 | 1.96438D-04 |
| Q( 8) | 5 - 2 | 2011.75 | -2279.58 | 0.00000D+00 | 9.00314D-27 | 2.48571D-03 |
| Q( 8) | 5 - 3 | 2783.75 | -1507.59 | 0.00000D+00 | 1.85119D-24 | -4.44857D-02 |
| Q( 8) | 5 - 4 | 3544.17 | -747.17 | 0.00000D+00 | 2.49357D-23 | 3.50555D-01 |
| Q( 8) | 5 - 5 | 4291.34 | 0.00 | 0.00000D+00 | 1.00000D+00 | 1.75200D+00 |
| Q( 9) | 5 - 0 | 448.20 | -3852.48 | 0.00000D+00 | 5.48947D-23 | -1.06518D-04 |
| Q( 9) | 5 - 1 | 1238.92 | -3061.76 | 0.00000D+00 | 1.61939D-24 | 1.95723D-04 |
| Q( 9) | 5 - 2 | 2021.38 | -2279.29 | 0.00000D+00 | 1.53638D-27 | 2.48634D-03 |
| Q( 9) | 5 - 3 | 2793.28 | -1507.39 | 0.00000D+00 | 9.24583D-25 | -4.44994D-02 |
| Q( 9) | 5 - 4 | 3553.61 | -747.07 | 0.00000D+00 | 3.92342D-23 | 3.50551D-01 |
| Q( 9) | 5 - 5 | 4300.68 | -0.00 | 0.00000D+00 | 1.00000D+00 | 1.75221D+00 |
| Q( 10) | 5 - 0 | 459.10 | -3851.95 | 0.00000D+00 | 5.47960D-23 | -1.07031D-04 |
| Q( 10) | 5 - 1 | 1249.72 | -3061.34 | 0.00000D+00 | 1.65905D-24 | 1.94926D-04 |
| Q( 10) | 5 - 2 | 2032.08 | -2278.97 | 0.00000D+00 | 9.39274D-27 | 2.48704D-03 |
| Q( 10) | 5 - 3 | 2803.88 | -1507.17 | 0.00000D+00 | 5.96175D-25 | -4.45146D-02 |
| Q( 10) | 5 - 4 | 3564.09 | -746.96 | 0.00000D+00 | 4.76257D-23 | 3.50548D-01 |
| Q( 10) | 5 - 5 | 4311.05 | -0.00 | 0.00000D+00 | 1.00000D+00 | 1.75244D+00 |
| Q( 11) | 5 - 0 | 471.09 | -3851.38 | 0.00000D+00 | 5.46872D-23 | -1.07594D-04 |
| Q( 11) | 5 - 1 | 1261.60 | -3060.87 | 0.00000D+00 | 1.70678D-24 | 1.94046D-04 |
| Q( 11) | 5 - 2 | 2043.85 | -2278.61 | 0.00000D+00 | 2.95642D-26 | 2.48781D-03 |
| Q( 11) | 5 - 3 | 2815.53 | -1506.93 | 0.00000D+00 | 2.95849D-25 | -4.45314D-02 |
| Q( 11) | 5 - 4 | 3575.63 | -746.84 | 0.00000D+00 | 5.68551D-23 | 3.50544D-01 |

| | | | | | | |
|---|---|---|---|---|---|---|
| Q( 11) | 5 - 5 | 4322.47 | -0.00 | 0.00000D+00 | 1.00000D+00 | 1.75270D+00 |
| Q( 12) | 5 - 0 | 484.17 | -3850.75 | 0.00000D+00 | 5.45415D-23 | -1.08210D-04 |
| Q( 12) | 5 - 1 | 1274.55 | -3060.36 | 0.00000D+00 | 1.76232D-24 | 1.93085D-04 |
| Q( 12) | 5 - 2 | 2056.69 | -2278.23 | 0.00000D+00 | 6.66784D-26 | 2.48864D-03 |
| Q( 12) | 5 - 3 | 2828.25 | -1506.67 | 0.00000D+00 | 7.84801D-26 | -4.45497D-02 |
| Q( 12) | 5 - 4 | 3588.21 | -746.70 | 0.00000D+00 | 6.99370D-23 | 3.50539D-01 |
| Q( 12) | 5 - 5 | 4334.92 | -0.00 | 0.00000D+00 | 1.00000D+00 | 1.75297D+00 |
| Q( 13) | 5 - 0 | 498.33 | -3850.07 | 0.00000D+00 | 5.44607D-23 | -1.08876D-04 |
| Q( 13) | 5 - 1 | 1288.59 | -3059.81 | 0.00000D+00 | 1.82504D-24 | 1.92039D-04 |
| Q( 13) | 5 - 2 | 2070.60 | -2277.80 | 0.00000D+00 | 1.27069D-25 | 2.48952D-03 |
| Q( 13) | 5 - 3 | 2842.02 | -1506.39 | 0.00000D+00 | 1.39297D-27 | -4.45695D-02 |
| Q( 13) | 5 - 4 | 3601.84 | -746.56 | 0.00000D+00 | 8.73732D-23 | 3.50534D-01 |
| Q( 13) | 5 - 5 | 4348.40 | -0.00 | 0.00000D+00 | 1.00000D+00 | 1.75328D+00 |
| Q( 14) | 5 - 0 | 513.59 | -3849.34 | 0.00000D+00 | 5.43308D-23 | -1.09595D-04 |
| Q( 14) | 5 - 1 | 1303.70 | -3059.22 | 0.00000D+00 | 1.93029D-24 | 1.90910D-04 |
| Q( 14) | 5 - 2 | 2085.57 | -2277.35 | 0.00000D+00 | 2.74285D-25 | 2.49047D-03 |
| Q( 14) | 5 - 3 | 2856.84 | -1506.08 | 0.00000D+00 | 1.19999D-25 | -4.45909D-02 |
| Q( 14) | 5 - 4 | 3616.52 | -746.40 | 0.00000D+00 | 1.10634D-22 | 3.50529D-01 |
| Q( 14) | 5 - 5 | 4362.92 | -0.00 | 0.00000D+00 | 1.00000D+00 | 1.75360D+00 |
| Q( 15) | 5 - 0 | 529.93 | -3848.55 | 0.00000D+00 | 5.42606D-23 | -1.10365D-04 |
| Q( 15) | 5 - 1 | 1319.90 | -3058.58 | 0.00000D+00 | 2.04038D-24 | 1.89695D-04 |
| Q( 15) | 5 - 2 | 2101.61 | -2276.87 | 0.00000D+00 | 4.47019D-25 | 2.49148D-03 |
| Q( 15) | 5 - 3 | 2872.73 | -1505.75 | 0.00000D+00 | 6.33960D-25 | -4.46138D-02 |
| Q( 15) | 5 - 4 | 3632.25 | -746.23 | 0.00000D+00 | 1.42015D-22 | 3.50523D-01 |
| Q( 15) | 5 - 5 | 4378.48 | -0.00 | 0.00000D+00 | 1.00000D+00 | 1.75395D+00 |
| Q( 16) | 5 - 0 | 547.36 | -3847.71 | 0.00000D+00 | 5.41807D-23 | -1.11186D-04 |
| Q( 16) | 5 - 1 | 1337.17 | -3057.91 | 0.00000D+00 | 2.17576D-24 | 1.88394D-04 |
| Q( 16) | 5 - 2 | 2118.72 | -2276.35 | 0.00000D+00 | 7.10625D-25 | 2.49254D-03 |
| Q( 16) | 5 - 3 | 2889.67 | -1505.40 | 0.00000D+00 | 1.73243D-24 | -4.46384D-02 |

| | | | | | | | |
|---|---|---|---|---|---|---|---|
| Q( 16) | 5 - 4 | 3649.02 | -746.06 | 0.00000D+00 | 1.83877D-22 | 3.50517D-01 |
| Q( 16) | 5 - 5 | 4395.07 | -0.00 | 0.00000D+00 | 1.00000D+00 | 1.75433D+00 |
| Q( 17) | 5 - 0 | 565.88 | -3846.82 | 0.00000D+00 | 5.38571D-23 | -1.12059D-04 |
| Q( 17) | 5 - 1 | 1355.51 | -3057.19 | 0.00000D+00 | 2.36353D-24 | 1.87006D-04 |
| Q( 17) | 5 - 2 | 2136.90 | -2275.80 | 0.00000D+00 | 1.09928D-24 | 2.49366D-03 |
| Q( 17) | 5 - 3 | 2907.67 | -1505.03 | 0.00000D+00 | 3.71716D-24 | -4.46645D-02 |
| Q( 17) | 5 - 4 | 3666.83 | -745.87 | 0.00000D+00 | 2.40799D-22 | 3.50510D-01 |
| Q( 17) | 5 - 5 | 4412.70 | -0.00 | 0.00000D+00 | 1.00000D+00 | 1.75472D+00 |
| Q( 18) | 5 - 0 | 585.48 | -3845.88 | 0.00000D+00 | 5.38387D-23 | -1.12984D-04 |
| Q( 18) | 5 - 1 | 1374.94 | -3056.42 | 0.00000D+00 | 2.68746D-24 | 1.85530D-04 |
| Q( 18) | 5 - 2 | 2156.15 | -2275.21 | 0.00000D+00 | 1.64707D-24 | 2.49482D-03 |
| Q( 18) | 5 - 3 | 2926.73 | -1504.63 | 0.00000D+00 | 6.98329D-24 | -4.46921D-02 |
| Q( 18) | 5 - 4 | 3685.69 | -745.66 | 0.00000D+00 | 3.17782D-22 | 3.50503D-01 |
| Q( 18) | 5 - 5 | 4431.36 | -0.00 | 0.00000D+00 | 1.00000D+00 | 1.75514D+00 |
| Q( 19) | 5 - 0 | 606.17 | -3844.88 | 0.00000D+00 | 5.38703D-23 | -1.13961D-04 |
| Q( 19) | 5 - 1 | 1395.44 | -3055.62 | 0.00000D+00 | 2.95621D-24 | 1.83965D-04 |
| Q( 19) | 5 - 2 | 2176.46 | -2274.60 | 0.00000D+00 | 2.44892D-24 | 2.49604D-03 |
| Q( 19) | 5 - 3 | 2946.84 | -1504.21 | 0.00000D+00 | 1.20107D-23 | -4.47214D-02 |
| Q( 19) | 5 - 4 | 3705.60 | -745.45 | 0.00000D+00 | 4.18277D-22 | 3.50495D-01 |
| Q( 19) | 5 - 5 | 4451.05 | -0.00 | 0.00000D+00 | 1.00000D+00 | 1.75558D+00 |
| Q( 20) | 5 - 0 | 627.95 | -3843.83 | 0.00000D+00 | 5.39487D-23 | -1.14989D-04 |
| Q( 20) | 5 - 1 | 1417.01 | -3054.77 | 0.00000D+00 | 3.27739D-24 | 1.82309D-04 |
| Q( 20) | 5 - 2 | 2197.83 | -2273.95 | 0.00000D+00 | 3.54422D-24 | 2.49730D-03 |
| Q( 20) | 5 - 3 | 2968.01 | -1503.78 | 0.00000D+00 | 1.95869D-23 | -4.47523D-02 |
| Q( 20) | 5 - 4 | 3726.55 | -745.23 | 0.00000D+00 | 5.52088D-22 | 3.50487D-01 |
| Q( 20) | 5 - 5 | 4471.78 | -0.00 | 0.00000D+00 | 1.00000D+00 | 1.75605D+00 |
