# Supplementary material for: Ab initio spectroscopic studies of AlF and AlCl molecules
Source: arXiv:2303.08681 source file (2023-03-15)
Supplement: Supplementary file 7 [file AlF_singlet_sigma_-_S7.pdf]

# AlF $X^1\Sigma$: Rotational parameters

Note that (v',J') & (v",J") strictly label the upper and lower levels, resp., and E(lower)=E"

but E(2)-E(1) is: (energy of State-2 level) - (energy of State-1 level)

In the following table, E is expressed in $cm^{-1}$, A in $s^{-1}$ and transition dipole moment in debye.

| dJ(J") | Band v' v" | E(lower) | E(2)-E(1) | A(Einstein) | F-C Factor | <v'j'\|M\|v"j"> |
|---|---|---|---|---|---|---|
| ------ | ------- | -------- | -------- | ----------- | ----------- | ----------- |
| R( 0) | 0 - 0 | 360.13 | -1.09 | 2.76264D-07 | 1.00000D+00 | -1.42101D+00 |
| R( 1) | 0 - 0 | 361.22 | -2.19 | 2.65216D-06 | 1.00000D+00 | -1.42105D+00 |
| R( 2) | 0 - 0 | 363.41 | -3.28 | 9.59075D-06 | 1.00000D+00 | -1.42112D+00 |
| R( 3) | 0 - 0 | 366.69 | -4.38 | 2.35768D-05 | 1.00000D+00 | -1.42122D+00 |
| R( 4) | 0 - 0 | 371.06 | -5.47 | 4.70981D-05 | 1.00000D+00 | -1.42135D+00 |
| R( 5) | 0 - 0 | 376.53 | -6.56 | 8.26443D-05 | 1.00000D+00 | -1.42151D+00 |
| R( 6) | 0 - 0 | 383.09 | -7.66 | 1.32707D-04 | 1.00000D+00 | -1.42170D+00 |
| R( 7) | 0 - 0 | 390.75 | -8.75 | 1.99780D-04 | 1.00000D+00 | -1.42192D+00 |
| R( 8) | 0 - 0 | 399.50 | -9.84 | 2.86360D-04 | 9.99999D-01 | -1.42216D+00 |
| R( 9) | 0 - 0 | 409.34 | -10.93 | 3.94945D-04 | 9.99999D-01 | -1.42244D+00 |
| R( 10) | 0 - 0 | 420.27 | -12.03 | 5.28039D-04 | 9.99999D-01 | -1.42274D+00 |
| R( 11) | 0 - 0 | 432.30 | -13.12 | 6.88149D-04 | 9.99999D-01 | -1.42307D+00 |
| R( 12) | 0 - 0 | 445.42 | -14.21 | 8.77784D-04 | 9.99999D-01 | -1.42343D+00 |
| R( 13) | 0 - 0 | 459.63 | -15.30 | 1.09946D-03 | 9.99999D-01 | -1.42383D+00 |
| R( 14) | 0 - 0 | 474.93 | -16.39 | 1.35570D-03 | 9.99999D-01 | -1.42425D+00 |
| R( 15) | 0 - 0 | 491.32 | -17.48 | 1.64902D-03 | 9.99998D-01 | -1.42470D+00 |
| R( 16) | 0 - 0 | 508.80 | -18.57 | 1.98196D-03 | 9.99998D-01 | -1.42518D+00 |
| R( 17) | 0 - 0 | 527.37 | -19.66 | 2.35706D-03 | 9.99998D-01 | -1.42569D+00 |
| R( 18) | 0 - 0 | 547.03 | -20.75 | 2.77685D-03 | 9.99998D-01 | -1.42623D+00 |

| | | | | | | | |
|---|---|---|---|---|---|---|---|
| R( 19) | 0 - 0 | 567.78 | -21.84 | 3.24390D-03 | 9.99997D-01 | -1.42680D+00 |
| P( 1) | 1 - 0 | 361.22 | -738.66 | 4.27133D+00 | 6.33211D-09 | -1.83830D-01 |
| R( 0) | 1 - 0 | 360.13 | -740.83 | 1.43280D+00 | 6.33177D-09 | -1.83600D-01 |
| P( 2) | 1 - 0 | 363.41 | -737.55 | 2.83906D+00 | 2.53299D-08 | -1.83968D-01 |
| R( 0) | 1 - 1 | 1099.88 | -1.08 | 3.22649D-07 | 1.00000D+00 | -1.55793D+00 |
| R( 1) | 1 - 0 | 361.22 | -741.91 | 1.72511D+00 | 2.53288D-08 | -1.83508D-01 |
| P( 3) | 1 - 0 | 366.69 | -736.44 | 2.54783D+00 | 5.69946D-08 | -1.84122D-01 |
| R( 1) | 1 - 1 | 1100.96 | -2.17 | 3.09747D-06 | 1.00000D+00 | -1.55797D+00 |
| R( 2) | 1 - 0 | 363.41 | -742.97 | 1.85473D+00 | 5.69928D-08 | -1.83431D-01 |
| P( 4) | 1 - 0 | 371.06 | -735.31 | 2.41983D+00 | 1.01332D-07 | -1.84291D-01 |
| R( 2) | 1 - 1 | 1103.13 | -3.25 | 1.12011D-05 | 1.00000D+00 | -1.55803D+00 |
| R( 3) | 1 - 0 | 366.69 | -744.02 | 1.93031D+00 | 1.01328D-07 | -1.83369D-01 |
| P( 5) | 1 - 0 | 376.53 | -734.18 | 2.34642D+00 | 1.58348D-07 | -1.84475D-01 |
| R( 3) | 1 - 1 | 1106.38 | -4.33 | 2.75356D-05 | 1.00000D+00 | -1.55812D+00 |
| R( 4) | 1 - 0 | 371.06 | -745.06 | 1.98148D+00 | 1.58340D-07 | -1.83323D-01 |
| P( 6) | 1 - 0 | 383.09 | -733.03 | 2.29795D+00 | 2.28051D-07 | -1.84674D-01 |
| R( 4) | 1 - 1 | 1110.71 | -5.42 | 5.50064D-05 | 1.00000D+00 | -1.55824D+00 |
| R( 5) | 1 - 0 | 376.53 | -746.09 | 2.01964D+00 | 2.28036D-07 | -1.83292D-01 |
| P( 7) | 1 - 0 | 390.75 | -731.88 | 2.26304D+00 | 3.10449D-07 | -1.84889D-01 |
| R( 5) | 1 - 1 | 1116.13 | -6.50 | 9.65214D-05 | 9.99999D-01 | -1.55838D+00 |
| R( 6) | 1 - 0 | 383.09 | -747.11 | 2.05012D+00 | 3.10426D-07 | -1.83276D-01 |
| P( 8) | 1 - 0 | 399.50 | -730.71 | 2.23635D+00 | 4.05554D-07 | -1.85119D-01 |
| R( 6) | 1 - 1 | 1122.63 | -7.58 | 1.54991D-04 | 9.99999D-01 | -1.55854D+00 |
| R( 7) | 1 - 0 | 390.75 | -748.12 | 2.07573D+00 | 4.05519D-07 | -1.83275D-01 |
| P( 9) | 1 - 0 | 409.34 | -729.53 | 2.21508D+00 | 5.13377D-07 | -1.85365D-01 |
| R( 7) | 1 - 1 | 1130.21 | -8.67 | 2.33327D-04 | 9.99999D-01 | -1.55874D+00 |
| R( 8) | 1 - 0 | 399.50 | -749.12 | 2.09811D+00 | 5.13328D-07 | -1.83290D-01 |
| P( 10) | 1 - 0 | 420.27 | -728.35 | 2.19759D+00 | 6.33934D-07 | -1.85626D-01 |
| R( 8) | 1 - 1 | 1138.87 | -9.75 | 3.34446D-04 | 9.99999D-01 | -1.55895D+00 |

| | | | | | | |
|---|---|---|---|---|---|---|
| R( 9) | 1 - 0 | 409.34 | -750.11 | 2.11827D+00 | 6.33867D-07 | -1.83320D-01 |
| P( 11) | 1 - 0 | 432.30 | -727.15 | 2.18286D+00 | 7.67239D-07 | -1.85903D-01 |
| R( 9) | 1 - 1 | 1148.62 | -10.83 | 4.61266D-04 | 9.99998D-01 | -1.55920D+00 |
| R( 10) | 1 - 0 | 420.27 | -751.09 | 2.13688D+00 | 7.67150D-07 | -1.83365D-01 |
| P( 12) | 1 - 0 | 445.42 | -725.95 | 2.17025D+00 | 9.13310D-07 | -1.86195D-01 |
| R( 10) | 1 - 1 | 1159.45 | -11.91 | 6.16712D-04 | 9.99998D-01 | -1.55947D+00 |
| R( 11) | 1 - 0 | 432.30 | -752.06 | 2.15438D+00 | 9.13193D-07 | -1.83425D-01 |
| P( 13) | 1 - 0 | 459.63 | -724.73 | 2.15929D+00 | 1.07216D-06 | -1.86502D-01 |
| R( 11) | 1 - 1 | 1171.37 | -13.00 | 8.03709D-04 | 9.99998D-01 | -1.55976D+00 |
| R( 12) | 1 - 0 | 445.42 | -753.02 | 2.17110D+00 | 1.07202D-06 | -1.83501D-01 |
| P( 14) | 1 - 0 | 474.93 | -723.51 | 2.14968D+00 | 1.24382D-06 | -1.86825D-01 |
| R( 12) | 1 - 1 | 1184.36 | -14.08 | 1.02519D-03 | 9.99997D-01 | -1.56008D+00 |
| R( 13) | 1 - 0 | 459.63 | -753.97 | 2.18727D+00 | 1.24363D-06 | -1.83592D-01 |
| P( 15) | 1 - 0 | 491.32 | -722.28 | 2.14118D+00 | 1.42830D-06 | -1.87164D-01 |
| R( 13) | 1 - 1 | 1198.44 | -15.16 | 1.28409D-03 | 9.99997D-01 | -1.56043D+00 |
| R( 14) | 1 - 0 | 474.93 | -754.91 | 2.20306D+00 | 1.42807D-06 | -1.83698D-01 |
| P( 16) | 1 - 0 | 508.80 | -721.04 | 2.13362D+00 | 1.62562D-06 | -1.87518D-01 |
| R( 14) | 1 - 1 | 1213.60 | -16.24 | 1.58336D-03 | 9.99996D-01 | -1.56080D+00 |
| R( 15) | 1 - 0 | 491.32 | -755.84 | 2.21861D+00 | 1.62534D-06 | -1.83820D-01 |
| P( 17) | 1 - 0 | 527.37 | -719.79 | 2.12688D+00 | 1.83581D-06 | -1.87888D-01 |
| R( 15) | 1 - 1 | 1229.84 | -17.32 | 1.92593D-03 | 9.99996D-01 | -1.56119D+00 |
| R( 16) | 1 - 0 | 508.80 | -756.76 | 2.23401D+00 | 1.83548D-06 | -1.83956D-01 |
| P( 18) | 1 - 0 | 547.03 | -718.53 | 2.12085D+00 | 2.05889D-06 | -1.88273D-01 |
| R( 16) | 1 - 1 | 1247.16 | -18.40 | 2.31477D-03 | 9.99995D-01 | -1.56161D+00 |
| R( 17) | 1 - 0 | 527.37 | -757.67 | 2.24936D+00 | 2.05849D-06 | -1.84108D-01 |
| P( 19) | 1 - 0 | 567.78 | -717.26 | 2.11546D+00 | 2.29487D-06 | -1.88674D-01 |
| R( 17) | 1 - 1 | 1265.56 | -19.48 | 2.75284D-03 | 9.99995D-01 | -1.56206D+00 |
| R( 18) | 1 - 0 | 547.03 | -758.57 | 2.26472D+00 | 2.29441D-06 | -1.84276D-01 |
| P( 20) | 1 - 0 | 589.62 | -715.98 | 2.11063D+00 | 2.54380D-06 | -1.89091D-01 |

| | | | | | | |
|---|---|---|---|---|---|---|
| R( 18) | 1 - 1 | 1285.04 | -20.56 | 3.24310D-03 | 9.99994D-01 | -1.56253D+00 |
| R( 19) | 1 - 0 | 567.78 | -759.46 | 2.28015D+00 | 2.54326D-06 | -1.84458D-01 |
| P( 21) | 1 - 0 | 612.55 | -714.70 | 2.10633D+00 | 2.80569D-06 | -1.89523D-01 |
| R( 19) | 1 - 1 | 1305.60 | -21.64 | 3.78852D-03 | 9.99993D-01 | -1.56303D+00 |
| P( 1) | 2 - 0 | 361.22 | -1528.59 | 3.46932D+00 | 1.76636D-11 | -5.56526D-02 |
| P( 1) | 2 - 1 | 1100.96 | -788.85 | 1.18495D+01 | 9.84579D-09 | -2.77433D-01 |
| R( 0) | 2 - 0 | 360.13 | -1530.75 | 1.16014D+00 | 1.77311D-11 | -5.56238D-02 |
| P( 2) | 2 - 0 | 363.41 | -1527.46 | 2.30924D+00 | 7.05039D-11 | -5.56702D-02 |
| R( 0) | 2 - 1 | 1099.88 | -791.00 | 3.97331D+00 | 9.84525D-09 | -2.77124D-01 |
| P( 2) | 2 - 1 | 1103.13 | -787.75 | 7.87552D+00 | 3.93880D-08 | -2.77591D-01 |
| R( 0) | 2 - 2 | 1889.81 | -1.06 | 3.39058D-07 | 1.00000D+00 | -1.64306D+00 |
| R( 1) | 2 - 0 | 361.22 | -1531.78 | 1.39443D+00 | 7.10321D-11 | -5.56127D-02 |
| P( 3) | 2 - 0 | 366.69 | -1526.31 | 2.07509D+00 | 1.58290D-10 | -5.56901D-02 |
| R( 1) | 2 - 1 | 1100.96 | -792.04 | 4.78167D+00 | 3.93853D-08 | -2.76974D-01 |
| P( 3) | 2 - 1 | 1106.38 | -786.62 | 7.06588D+00 | 8.86362D-08 | -2.77752D-01 |
| R( 1) | 2 - 2 | 1890.87 | -2.13 | 3.25501D-06 | 1.00000D+00 | -1.64310D+00 |
| R( 2) | 2 - 0 | 363.41 | -1532.78 | 1.49649D+00 | 1.60059D-10 | -5.56039D-02 |
| P( 4) | 2 - 0 | 371.06 | -1525.12 | 1.97324D+00 | 2.80734D-10 | -5.57122D-02 |
| R( 2) | 2 - 1 | 1103.13 | -793.06 | 5.13761D+00 | 8.86292D-08 | -2.76827D-01 |
| P( 4) | 2 - 1 | 1110.71 | -785.48 | 6.70800D+00 | 1.57611D-07 | -2.77916D-01 |
| R( 2) | 2 - 2 | 1893.00 | -3.19 | 1.17709D-05 | 1.00000D+00 | -1.64317D+00 |
| R( 3) | 2 - 0 | 366.69 | -1533.75 | 1.55449D+00 | 2.84927D-10 | -5.55971D-02 |
| P( 5) | 2 - 0 | 376.53 | -1523.91 | 1.91550D+00 | 4.37538D-10 | -5.57364D-02 |
| R( 3) | 2 - 1 | 1106.38 | -794.06 | 5.34252D+00 | 1.57594D-07 | -2.76682D-01 |
| P( 5) | 2 - 1 | 1116.13 | -784.31 | 6.50051D+00 | 2.46338D-07 | -2.78083D-01 |
| R( 3) | 2 - 2 | 1896.19 | -4.25 | 2.89364D-05 | 1.00000D+00 | -1.64328D+00 |
| R( 4) | 2 - 0 | 371.06 | -1534.69 | 1.59248D+00 | 4.45726D-10 | -5.55925D-02 |
| P( 6) | 2 - 0 | 383.09 | -1522.66 | 1.87784D+00 | 6.28364D-10 | -5.57628D-02 |
| R( 4) | 2 - 1 | 1110.71 | -795.04 | 5.47861D+00 | 2.46305D-07 | -2.76540D-01 |

| | | | | | | | |
|---|---|---|---|---|---|---|---|
| P( 6) | 2 - 1 | 1122.63 | -783.13 | 6.36120D+00 | 3.54850D-07 | -2.78253D-01 |
| R( 4) | 2 - 2 | 1900.44 | -5.31 | 5.78054D-05 | 9.99999D-01 | -1.64341D+00 |
| R( 5) | 2 - 0 | 376.53 | -1535.60 | 1.61970D+00 | 6.42511D-10 | -5.55899D-02 |
| P( 7) | 2 - 0 | 390.75 | -1521.38 | 1.85099D+00 | 8.52847D-10 | -5.57913D-02 |
| R( 5) | 2 - 1 | 1116.13 | -796.01 | 5.57748D+00 | 3.54794D-07 | -2.76401D-01 |
| P( 7) | 2 - 1 | 1130.21 | -781.92 | 6.25847D+00 | 4.83188D-07 | -2.78426D-01 |
| R( 5) | 2 - 2 | 1905.75 | -6.38 | 1.01434D-04 | 9.99999D-01 | -1.64357D+00 |
| R( 6) | 2 - 0 | 383.09 | -1536.48 | 1.64048D+00 | 8.75308D-10 | -5.55893D-02 |
| P( 8) | 2 - 0 | 399.50 | -1520.07 | 1.83064D+00 | 1.11059D-09 | -5.58218D-02 |
| R( 6) | 2 - 1 | 1122.63 | -796.95 | 5.65388D+00 | 4.83098D-07 | -2.76265D-01 |
| P( 8) | 2 - 1 | 1138.87 | -780.70 | 6.17757D+00 | 6.31400D-07 | -2.78602D-01 |
| R( 6) | 2 - 2 | 1912.13 | -7.44 | 1.62881D-04 | 9.99999D-01 | -1.64376D+00 |
| R( 7) | 2 - 0 | 390.75 | -1537.32 | 1.65709D+00 | 1.14411D-09 | -5.55907D-02 |
| P( 9) | 2 - 0 | 409.34 | -1518.74 | 1.81449D+00 | 1.40117D-09 | -5.58543D-02 |
| R( 7) | 2 - 1 | 1130.21 | -797.87 | 5.71562D+00 | 6.31265D-07 | -2.76131D-01 |
| P( 9) | 2 - 1 | 1148.62 | -779.45 | 6.11069D+00 | 7.99540D-07 | -2.78781D-01 |
| R( 7) | 2 - 2 | 1919.57 | -8.50 | 2.45209D-04 | 9.99998D-01 | -1.64398D+00 |
| R( 8) | 2 - 0 | 399.50 | -1538.14 | 1.67084D+00 | 1.44889D-09 | -5.55940D-02 |
| P( 10) | 2 - 0 | 420.27 | -1517.37 | 1.80123D+00 | 1.72414D-09 | -5.58887D-02 |
| R( 8) | 2 - 1 | 1138.87 | -798.77 | 5.76723D+00 | 7.99348D-07 | -2.76000D-01 |
| P( 10) | 2 - 1 | 1159.45 | -778.19 | 6.05331D+00 | 9.87671D-07 | -2.78962D-01 |
| R( 8) | 2 - 2 | 1928.07 | -9.57 | 3.51484D-04 | 9.99998D-01 | -1.64423D+00 |
| R( 9) | 2 - 0 | 409.34 | -1538.93 | 1.68257D+00 | 1.78957D-09 | -5.55991D-02 |
| P( 11) | 2 - 0 | 432.30 | -1515.97 | 1.79002D+00 | 2.07900D-09 | -5.59249D-02 |
| R( 9) | 2 - 1 | 1148.62 | -799.65 | 5.81150D+00 | 9.87407D-07 | -2.75871D-01 |
| P( 11) | 2 - 1 | 1171.37 | -776.90 | 6.00263D+00 | 1.19586D-06 | -2.79148D-01 |
| R( 9) | 2 - 2 | 1937.64 | -10.63 | 4.84775D-04 | 9.99998D-01 | -1.64451D+00 |
| R( 10) | 2 - 0 | 420.27 | -1539.68 | 1.69279D+00 | 2.16607D-09 | -5.56058D-02 |
| P( 12) | 2 - 0 | 445.42 | -1514.54 | 1.78033D+00 | 2.46526D-09 | -5.59629D-02 |

| | | | | | | | |
|---|---|---|---|---|---|---|---|
| R( 10) | 2 - 1 | 1159.45 | -800.50 | 5.85025D+00 | 1.19551D-06 | -2.75745D-01 |
| P( 12) | 2 - 1 | 1184.36 | -775.60 | 5.95683D+00 | 1.42419D-06 | -2.79336D-01 |
| R( 10) | 2 - 2 | 1948.27 | -11.69 | 6.48158D-04 | 9.99997D-01 | -1.64481D+00 |
| R( 11) | 2 - 0 | 432.30 | -1540.41 | 1.70186D+00 | 2.57825D-09 | -5.56142D-02 |
| P( 13) | 2 - 0 | 459.63 | -1513.08 | 1.77178D+00 | 2.88236D-09 | -5.60026D-02 |
| R( 11) | 2 - 1 | 1171.37 | -801.34 | 5.88473D+00 | 1.42374D-06 | -2.75622D-01 |
| P( 13) | 2 - 1 | 1198.44 | -774.27 | 5.91468D+00 | 1.67275D-06 | -2.79527D-01 |
| R( 11) | 2 - 2 | 1959.96 | -12.75 | 8.44711D-04 | 9.99997D-01 | -1.64515D+00 |
| R( 12) | 2 - 0 | 445.42 | -1541.10 | 1.71003D+00 | 3.02597D-09 | -5.56241D-02 |
| P( 14) | 2 - 0 | 474.93 | -1511.59 | 1.76412D+00 | 3.32975D-09 | -5.60439D-02 |
| R( 12) | 2 - 1 | 1184.36 | -802.16 | 5.91581D+00 | 1.67216D-06 | -2.75502D-01 |
| P( 14) | 2 - 1 | 1213.60 | -772.92 | 5.87531D+00 | 1.94161D-06 | -2.79722D-01 |
| R( 12) | 2 - 2 | 1972.71 | -13.81 | 1.07752D-03 | 9.99996D-01 | -1.64551D+00 |
| R( 13) | 2 - 0 | 459.63 | -1541.77 | 1.71748D+00 | 3.50904D-09 | -5.56354D-02 |
| P( 15) | 2 - 0 | 491.32 | -1510.08 | 1.75716D+00 | 3.80683D-09 | -5.60866D-02 |
| R( 13) | 2 - 1 | 1198.44 | -802.96 | 5.94412D+00 | 1.94089D-06 | -2.75384D-01 |
| P( 15) | 2 - 1 | 1229.84 | -771.56 | 5.83808D+00 | 2.23090D-06 | -2.79920D-01 |
| R( 13) | 2 - 2 | 1986.52 | -14.87 | 1.34968D-03 | 9.99995D-01 | -1.64591D+00 |
| R( 14) | 2 - 0 | 474.93 | -1542.40 | 1.72435D+00 | 4.02726D-09 | -5.56480D-02 |
| P( 16) | 2 - 0 | 508.80 | -1508.53 | 1.75074D+00 | 4.31300D-09 | -5.61306D-02 |
| R( 14) | 2 - 1 | 1213.60 | -803.73 | 5.97013D+00 | 2.23000D-06 | -2.75269D-01 |
| P( 16) | 2 - 1 | 1247.16 | -770.17 | 5.80253D+00 | 2.54070D-06 | -2.80121D-01 |
| R( 14) | 2 - 2 | 2001.39 | -15.94 | 1.66428D-03 | 9.99995D-01 | -1.64633D+00 |
| R( 15) | 2 - 0 | 491.32 | -1543.01 | 1.73071D+00 | 4.58038D-09 | -5.56617D-02 |
| P( 17) | 2 - 0 | 527.37 | -1506.95 | 1.74476D+00 | 4.84759D-09 | -5.61759D-02 |
| R( 15) | 2 - 1 | 1229.84 | -804.49 | 5.99420D+00 | 2.53962D-06 | -2.75157D-01 |
| P( 17) | 2 - 1 | 1265.56 | -768.77 | 5.76831D+00 | 2.87115D-06 | -2.80326D-01 |
| R( 15) | 2 - 2 | 2017.33 | -17.00 | 2.02444D-03 | 9.99994D-01 | -1.64679D+00 |
| R( 16) | 2 - 0 | 508.80 | -1543.58 | 1.73666D+00 | 5.16816D-09 | -5.56763D-02 |

| | | | | | | | |
|---|---|---|---|---|---|---|---|
| P( 18) | 2 - 0 | 547.03 | -1505.35 | 1.73914D+00 | 5.40997D-09 | -5.62222D-02 |
| R( 16) | 2 - 1 | 1247.16 | -805.22 | 6.01659D+00 | 2.86985D-06 | -2.75048D-01 |
| P( 18) | 2 - 1 | 1285.04 | -767.34 | 5.73515D+00 | 3.22236D-06 | -2.80535D-01 |
| R( 16) | 2 - 2 | 2034.33 | -18.06 | 2.43327D-03 | 9.99993D-01 | -1.64727D+00 |
| R( 17) | 2 - 0 | 527.37 | -1544.13 | 1.74223D+00 | 5.79029D-09 | -5.56919D-02 |
| P( 19) | 2 - 0 | 567.78 | -1503.71 | 1.73379D+00 | 5.99942D-09 | -5.62695D-02 |
| R( 17) | 2 - 1 | 1265.56 | -805.94 | 6.03753D+00 | 3.22081D-06 | -2.74941D-01 |
| P( 19) | 2 - 1 | 1305.60 | -765.89 | 5.70284D+00 | 3.59446D-06 | -2.80747D-01 |
| R( 17) | 2 - 2 | 2052.38 | -19.12 | 2.89388D-03 | 9.99992D-01 | -1.64778D+00 |
| R( 18) | 2 - 0 | 547.03 | -1544.64 | 1.74747D+00 | 6.44648D-09 | -5.57081D-02 |
| P( 20) | 2 - 0 | 589.62 | -1502.05 | 1.72866D+00 | 6.61525D-09 | -5.63175D-02 |
| R( 18) | 2 - 1 | 1285.04 | -806.63 | 6.05719D+00 | 3.59264D-06 | -2.74837D-01 |
| P( 20) | 2 - 1 | 1327.25 | -764.43 | 5.67122D+00 | 3.98759D-06 | -2.80963D-01 |
| R( 18) | 2 - 2 | 2071.50 | -20.18 | 3.40941D-03 | 9.99991D-01 | -1.64832D+00 |
| R( 19) | 2 - 0 | 567.78 | -1545.13 | 1.75242D+00 | 7.13637D-09 | -5.57249D-02 |
| P( 21) | 2 - 0 | 612.55 | -1500.36 | 1.72370D+00 | 7.25673D-09 | -5.63662D-02 |
| R( 19) | 2 - 1 | 1305.60 | -807.31 | 6.07569D+00 | 3.98547D-06 | -2.74737D-01 |
| P( 21) | 2 - 1 | 1349.97 | -762.94 | 5.64014D+00 | 4.40191D-06 | -2.81182D-01 |
| R( 19) | 2 - 2 | 2091.67 | -21.24 | 3.98300D-03 | 9.99990D-01 | -1.64889D+00 |
| P( 1) | 3 - 0 | 361.22 | -2326.90 | 5.60858D-01 | 7.79179D-13 | 1.19141D-02 |
| P( 1) | 3 - 1 | 1100.96 | -1587.16 | 9.74998D-02 | 7.03531D-11 | -8.81803D-03 |
| P( 1) | 3 - 2 | 1890.87 | -797.24 | 2.04928D+01 | 1.36649D-08 | -3.59098D-01 |
| R( 0) | 3 - 0 | 360.13 | -2329.04 | 1.87831D-01 | 7.81046D-13 | 1.19255D-02 |
| P( 2) | 3 - 0 | 363.41 | -2325.76 | 3.73972D-01 | 3.11152D-12 | 1.19238D-02 |
| R( 0) | 3 - 1 | 1099.88 | -1589.29 | 3.23202D-02 | 7.05478D-11 | -8.77587D-03 |
| P( 2) | 3 - 1 | 1103.13 | -1586.04 | 6.52547D-02 | 2.81013D-10 | -8.84460D-03 |
| R( 0) | 3 - 2 | 1889.81 | -799.36 | 6.87077D+00 | 1.36637D-08 | -3.58714D-01 |
| P( 2) | 3 - 2 | 1893.00 | -796.17 | 1.36219D+01 | 5.46627D-08 | -3.59297D-01 |
| R( 0) | 3 - 3 | 2688.12 | -1.05 | 3.57965D-07 | 1.00000D+00 | -1.70991D+00 |

| | | | | | | | |
|---|---|---|---|---|---|---|---|
| R( 1) | 3 - 0 | 361.22 | -2330.06 | 2.26496D-01 | 3.12704D-12 | 1.19467D-02 |
| P( 3) | 3 - 0 | 366.69 | -2324.59 | 3.37200D-01 | 6.98617D-12 | 1.19439D-02 |
| R( 1) | 3 - 1 | 1100.96 | -1590.32 | 3.87213D-02 | 2.82542D-10 | -8.76028D-03 |
| P( 3) | 3 - 1 | 1106.38 | -1584.90 | 5.90039D-02 | 6.31433D-10 | -8.87484D-03 |
| R( 1) | 3 - 2 | 1890.87 | -800.41 | 8.26878D+00 | 5.46572D-08 | -3.58529D-01 |
| P( 3) | 3 - 2 | 1896.19 | -795.09 | 1.22237D+01 | 1.22995D-07 | -3.59500D-01 |
| R( 1) | 3 - 3 | 2689.17 | -2.11 | 3.43653D-06 | 1.00000D+00 | -1.70997D+00 |
| R( 2) | 3 - 0 | 363.41 | -2331.03 | 2.44263D-01 | 7.03918D-12 | 1.19783D-02 |
| P( 4) | 3 - 0 | 371.06 | -2323.38 | 3.22276D-01 | 1.23906D-11 | 1.19744D-02 |
| R( 2) | 3 - 1 | 1103.13 | -1591.31 | 4.14518D-02 | 6.36555D-10 | -8.74834D-03 |
| P( 4) | 3 - 1 | 1110.71 | -1583.73 | 5.64992D-02 | 1.12098D-09 | -8.90876D-03 |
| R( 2) | 3 - 2 | 1893.00 | -801.44 | 8.88492D+00 | 1.22980D-07 | -3.58349D-01 |
| P( 4) | 3 - 2 | 1900.44 | -794.00 | 1.16073D+01 | 2.18671D-07 | -3.59709D-01 |
| R( 2) | 3 - 3 | 2691.28 | -3.16 | 1.24274D-05 | 1.00000D+00 | -1.71006D+00 |
| R( 3) | 3 - 0 | 366.69 | -2331.97 | 2.55390D-01 | 1.25161D-11 | 1.20201D-02 |
| P( 5) | 3 - 0 | 376.53 | -2322.12 | 3.14950D-01 | 1.93084D-11 | 1.20151D-02 |
| R( 3) | 3 - 1 | 1106.38 | -1592.28 | 4.29839D-02 | 1.13312D-09 | -8.74005D-03 |
| P( 5) | 3 - 1 | 1116.13 | -1582.53 | 5.52690D-02 | 1.74905D-09 | -8.94640D-03 |
| R( 3) | 3 - 2 | 1896.19 | -802.47 | 9.24040D+00 | 2.18636D-07 | -3.58173D-01 |
| P( 5) | 3 - 2 | 1905.75 | -792.90 | 1.12514D+01 | 3.41699D-07 | -3.59923D-01 |
| R( 3) | 3 - 3 | 2694.44 | -4.22 | 3.05509D-05 | 9.99999D-01 | -1.71020D+00 |
| R( 4) | 3 - 0 | 371.06 | -2332.86 | 2.63770D-01 | 1.95535D-11 | 1.20723D-02 |
| P( 6) | 3 - 0 | 383.09 | -2320.83 | 3.11335D-01 | 2.77208D-11 | 1.20661D-02 |
| R( 4) | 3 - 1 | 1110.71 | -1593.22 | 4.39920D-02 | 1.77278D-09 | -8.73544D-03 |
| P( 6) | 3 - 1 | 1122.63 | -1581.30 | 5.46394D-02 | 2.51504D-09 | -8.98776D-03 |
| R( 4) | 3 - 2 | 1900.44 | -803.49 | 9.47737D+00 | 3.41631D-07 | -3.58003D-01 |
| P( 6) | 3 - 2 | 1912.13 | -791.79 | 1.10139D+01 | 4.92090D-07 | -3.60141D-01 |
| R( 4) | 3 - 3 | 2698.66 | -5.27 | 6.10319D-05 | 9.99999D-01 | -1.71038D+00 |
| R( 5) | 3 - 0 | 376.53 | -2333.72 | 2.70903D-01 | 2.81438D-11 | 1.21347D-02 |

| | | | | | | | |
|---|---|---|---|---|---|---|---|
| P( 7) | 3 - 0 | 390.75 | -2319.50 | 3.09941D-01 | 3.76060D-11 | 1.21275D-02 |
| R( 5) | 3 - 1 | 1116.13 | -1594.12 | 4.47356D-02 | 2.55605D-09 | -8.73452D-03 |
| P( 7) | 3 - 1 | 1130.21 | -1580.04 | 5.43518D-02 | 3.41830D-09 | -9.03288D-03 |
| R( 5) | 3 - 2 | 1905.75 | -804.50 | 9.65050D+00 | 4.91973D-07 | -3.57837D-01 |
| P( 7) | 3 - 2 | 1919.57 | -790.68 | 1.08402D+01 | 6.69857D-07 | -3.60364D-01 |
| R( 5) | 3 - 3 | 2703.93 | -6.32 | 1.07098D-04 | 9.99999D-01 | -1.71060D+00 |
| R( 6) | 3 - 0 | 383.09 | -2334.53 | 2.77496D-01 | 3.82769D-11 | 1.22074D-02 |
| P( 8) | 3 - 0 | 399.50 | -2318.13 | 3.10073D-01 | 4.89393D-11 | 1.21990D-02 |
| R( 6) | 3 - 1 | 1122.63 | -1595.00 | 4.53361D-02 | 3.48345D-09 | -8.73729D-03 |
| P( 8) | 3 - 1 | 1138.87 | -1578.75 | 5.42856D-02 | 4.45819D-09 | -9.08178D-03 |
| R( 6) | 3 - 2 | 1912.13 | -805.49 | 9.78531D+00 | 6.69671D-07 | -3.57675D-01 |
| P( 8) | 3 - 2 | 1928.07 | -789.55 | 1.07047D+01 | 8.75016D-07 | -3.60592D-01 |
| R( 6) | 3 - 3 | 2710.25 | -7.38 | 1.71982D-04 | 9.99998D-01 | -1.71086D+00 |
| R( 7) | 3 - 0 | 390.75 | -2335.31 | 2.83926D-01 | 4.99394D-11 | 1.22904D-02 |
| P( 9) | 3 - 0 | 409.34 | -2316.72 | 3.11366D-01 | 6.16933D-11 | 1.22808D-02 |
| R( 7) | 3 - 1 | 1130.21 | -1595.85 | 4.58581D-02 | 4.55546D-09 | -8.74378D-03 |
| P( 9) | 3 - 1 | 1148.62 | -1577.43 | 5.43775D-02 | 5.63404D-09 | -9.13450D-03 |
| R( 7) | 3 - 2 | 1919.57 | -806.48 | 9.89530D+00 | 8.74737D-07 | -3.57519D-01 |
| P( 9) | 3 - 2 | 1937.64 | -788.42 | 1.05939D+01 | 1.10758D-06 | -3.60825D-01 |
| R( 7) | 3 - 3 | 2717.63 | -8.43 | 2.58919D-04 | 9.99998D-01 | -1.71115D+00 |
| R( 8) | 3 - 0 | 399.50 | -2336.04 | 2.90418D-01 | 6.31151D-11 | 1.23835D-02 |
| P( 10) | 3 - 0 | 420.27 | -2315.27 | 3.13611D-01 | 7.58378D-11 | 1.23728D-02 |
| R( 8) | 3 - 1 | 1138.87 | -1596.67 | 4.63392D-02 | 5.77258D-09 | -8.75402D-03 |
| P( 10) | 3 - 1 | 1159.45 | -1576.09 | 5.45912D-02 | 6.94518D-09 | -9.19108D-03 |
| R( 8) | 3 - 2 | 1928.07 | -807.46 | 9.98829D+00 | 1.10719D-06 | -3.57367D-01 |
| P( 10) | 3 - 2 | 1948.27 | -787.27 | 1.05000D+01 | 1.36758D-06 | -3.61063D-01 |
| R( 8) | 3 - 3 | 2726.06 | -9.48 | 3.71150D-04 | 9.99997D-01 | -1.71149D+00 |
| R( 9) | 3 - 0 | 409.34 | -2336.74 | 2.97113D-01 | 7.77846D-11 | 1.24869D-02 |
| P( 11) | 3 - 0 | 432.30 | -2313.78 | 3.16682D-01 | 9.13396D-11 | 1.24750D-02 |

| | | | | | | | |
|---|---|---|---|---|---|---|---|
| R( 9) | 3 - 1 | 1148.62 | -1597.45 | 4.68028D-02 | 7.13528D-09 | -8.76803D-03 |
| P( 11) | 3 - 1 | 1171.37 | -1574.71 | 5.49045D-02 | 8.39090D-09 | -9.25156D-03 |
| R( 9) | 3 - 2 | 1937.64 | -808.44 | 1.00691D+01 | 1.36703D-06 | -3.57220D-01 |
| P( 11) | 3 - 2 | 1959.96 | -786.12 | 1.04182D+01 | 1.65503D-06 | -3.61306D-01 |
| R( 9) | 3 - 3 | 2735.54 | -10.54 | 5.11921D-04 | 9.99997D-01 | -1.71186D+00 |
| R( 10) | 3 - 0 | 420.27 | -2337.39 | 3.04110D-01 | 9.39259D-11 | 1.26004D-02 |
| P( 12) | 3 - 0 | 445.42 | -2312.25 | 3.20500D-01 | 1.08163D-10 | 1.25874D-02 |
| R( 10) | 3 - 1 | 1159.45 | -1598.21 | 4.72649D-02 | 8.64402D-09 | -8.78585D-03 |
| P( 12) | 3 - 1 | 1184.36 | -1573.30 | 5.53034D-02 | 9.97050D-09 | -9.31599D-03 |
| R( 10) | 3 - 2 | 1948.27 | -809.40 | 1.01409D+01 | 1.65430D-06 | -3.57078D-01 |
| P( 12) | 3 - 2 | 1972.71 | -784.96 | 1.03452D+01 | 1.96995D-06 | -3.61554D-01 |
| R( 10) | 3 - 3 | 2746.08 | -11.59 | 6.84485D-04 | 9.99996D-01 | -1.71228D+00 |
| R( 11) | 3 - 0 | 432.30 | -2338.01 | 3.11480D-01 | 1.11514D-10 | 1.27240D-02 |
| P( 13) | 3 - 0 | 459.63 | -2310.68 | 3.25014D-01 | 1.26270D-10 | 1.27098D-02 |
| R( 11) | 3 - 1 | 1171.37 | -1598.94 | 4.77362D-02 | 1.02992D-08 | -8.80751D-03 |
| P( 13) | 3 - 1 | 1198.44 | -1571.87 | 5.57788D-02 | 1.16832D-08 | -9.38441D-03 |
| R( 11) | 3 - 2 | 1959.96 | -810.35 | 1.02059D+01 | 1.96901D-06 | -3.56940D-01 |
| P( 13) | 3 - 2 | 1986.52 | -783.79 | 1.02791D+01 | 2.31238D-06 | -3.61808D-01 |
| R( 11) | 3 - 3 | 2757.67 | -12.64 | 8.92101D-04 | 9.99995D-01 | -1.71273D+00 |
| R( 12) | 3 - 0 | 445.42 | -2338.58 | 3.19277D-01 | 1.30520D-10 | 1.28577D-02 |
| P( 14) | 3 - 0 | 474.93 | -2309.07 | 3.30189D-01 | 1.45619D-10 | 1.28423D-02 |
| R( 12) | 3 - 1 | 1184.36 | -1599.64 | 4.82248D-02 | 1.21013D-08 | -8.83306D-03 |
| P( 14) | 3 - 1 | 1213.60 | -1570.40 | 5.63245D-02 | 1.35283D-08 | -9.45689D-03 |
| R( 12) | 3 - 2 | 1972.71 | -811.29 | 1.02655D+01 | 2.31118D-06 | -3.56807D-01 |
| P( 14) | 3 - 2 | 2001.39 | -782.61 | 1.02181D+01 | 2.68234D-06 | -3.62066D-01 |
| R( 12) | 3 - 3 | 2770.31 | -13.69 | 1.13803D-03 | 9.99994D-01 | -1.71322D+00 |
| R( 13) | 3 - 0 | 459.63 | -2339.12 | 3.27546D-01 | 1.50913D-10 | 1.30014D-02 |
| P( 15) | 3 - 0 | 491.32 | -2307.43 | 3.36006D-01 | 1.66166D-10 | 1.29848D-02 |
| R( 13) | 3 - 1 | 1198.44 | -1600.31 | 4.87370D-02 | 1.40507D-08 | -8.86254D-03 |

| | | | | | | |
|---|---|---|---|---|---|---|
| P( 15) | 3 - 1 | 1229.84 | -1568.91 | 5.69365D-02 | 1.55050D-08 | -9.53347D-03 |
| R( 13) | 3 - 2 | 1986.52 | -812.22 | 1.03209D+01 | 2.68084D-06 | -3.56679D-01 |
| P( 15) | 3 - 2 | 2017.33 | -781.42 | 1.01613D+01 | 3.07987D-06 | -3.62330D-01 |
| R( 13) | 3 - 3 | 2784.00 | -14.75 | 1.42556D-03 | 9.99993D-01 | -1.71376D+00 |
| R( 14) | 3 - 0 | 474.93 | -2339.62 | 3.36322D-01 | 1.72660D-10 | 1.31551D-02 |
| P( 16) | 3 - 0 | 508.80 | -2305.74 | 3.42451D-01 | 1.87864D-10 | 1.31372D-02 |
| R( 14) | 3 - 1 | 1213.60 | -1600.95 | 4.92777D-02 | 1.61478D-08 | -8.89599D-03 |
| P( 16) | 3 - 1 | 1247.16 | -1567.38 | 5.76123D-02 | 1.76124D-08 | -9.61422D-03 |
| R( 14) | 3 - 2 | 2001.39 | -813.15 | 1.03728D+01 | 3.07803D-06 | -3.56556D-01 |
| P( 16) | 3 - 2 | 2034.33 | -780.22 | 1.01079D+01 | 3.50501D-06 | -3.62599D-01 |
| R( 14) | 3 - 3 | 2798.75 | -15.80 | 1.75797D-03 | 9.99992D-01 | -1.71433D+00 |
| R( 15) | 3 - 0 | 491.32 | -2340.07 | 3.45638D-01 | 1.95723D-10 | 1.33187D-02 |
| P( 17) | 3 - 0 | 527.37 | -2304.02 | 3.49517D-01 | 2.10665D-10 | 1.32995D-02 |
| R( 15) | 3 - 1 | 1229.84 | -1601.55 | 4.98509D-02 | 1.83930D-08 | -8.93347D-03 |
| P( 17) | 3 - 1 | 1265.56 | -1565.83 | 5.83504D-02 | 1.98498D-08 | -9.69920D-03 |
| R( 15) | 3 - 2 | 2017.33 | -814.06 | 1.04218D+01 | 3.50277D-06 | -3.56438D-01 |
| P( 17) | 3 - 2 | 2052.38 | -779.01 | 1.00571D+01 | 3.95779D-06 | -3.62874D-01 |
| R( 15) | 3 - 3 | 2814.54 | -16.85 | 2.13854D-03 | 9.99991D-01 | -1.71494D+00 |
| R( 16) | 3 - 0 | 508.80 | -2340.49 | 3.55523D-01 | 2.20063D-10 | 1.34922D-02 |
| P( 18) | 3 - 0 | 547.03 | -2302.25 | 3.57202D-01 | 2.34518D-10 | 1.34717D-02 |
| R( 16) | 3 - 1 | 1247.16 | -1602.13 | 5.04601D-02 | 2.07865D-08 | -8.97503D-03 |
| P( 18) | 3 - 1 | 1285.04 | -1564.25 | 5.91499D-02 | 2.22162D-08 | -9.78849D-03 |
| R( 16) | 3 - 2 | 2034.33 | -814.96 | 1.04686D+01 | 3.95511D-06 | -3.56324D-01 |
| P( 18) | 3 - 2 | 2071.50 | -777.79 | 1.00086D+01 | 4.43826D-06 | -3.63154D-01 |
| R( 16) | 3 - 3 | 2831.39 | -17.90 | 2.57059D-03 | 9.99990D-01 | -1.71559D+00 |
| R( 17) | 3 - 0 | 527.37 | -2340.86 | 3.66004D-01 | 2.45636D-10 | 1.36755D-02 |
| P( 19) | 3 - 0 | 567.78 | -2300.45 | 3.65506D-01 | 2.59367D-10 | 1.36537D-02 |
| R( 17) | 3 - 1 | 1265.56 | -1602.68 | 5.11087D-02 | 2.33287D-08 | -9.02073D-03 |
| P( 19) | 3 - 1 | 1305.60 | -1562.63 | 6.00107D-02 | 2.47107D-08 | -9.88216D-03 |

| | | | | | | | |
|---|---|---|---|---|---|---|---|
| R( 17) | 3 - 2 | 2052.38 | -815.85 | 1.05133D+01 | 4.43508D-06 | -3.56216D-01 |
| P( 19) | 3 - 2 | 2091.67 | -776.56 | 9.96197D+00 | 4.94647D-06 | -3.63439D-01 |
| R( 17) | 3 - 3 | 2849.29 | -18.95 | 3.05743D-03 | 9.99989D-01 | -1.71628D+00 |
| R( 18) | 3 - 0 | 547.03 | -2341.20 | 3.77106D-01 | 2.72398D-10 | 1.38685D-02 |
| P( 20) | 3 - 0 | 589.62 | -2298.61 | 3.74432D-01 | 2.85157D-10 | 1.38454D-02 |
| R( 18) | 3 - 1 | 1285.04 | -1603.19 | 5.17993D-02 | 2.60199D-08 | -9.07064D-03 |
| P( 20) | 3 - 1 | 1327.25 | -1560.99 | 6.09330D-02 | 2.73325D-08 | -9.98028D-03 |
| R( 18) | 3 - 2 | 2071.50 | -816.74 | 1.05563D+01 | 4.94272D-06 | -3.56113D-01 |
| P( 20) | 3 - 2 | 2112.91 | -775.32 | 9.91691D+00 | 5.48247D-06 | -3.63730D-01 |
| R( 18) | 3 - 3 | 2868.24 | -20.00 | 3.60238D-03 | 9.99988D-01 | -1.71701D+00 |
| R( 19) | 3 - 0 | 567.78 | -2341.50 | 3.88854D-01 | 3.00299D-10 | 1.40711D-02 |
| P( 21) | 3 - 0 | 612.55 | -2296.73 | 3.83986D-01 | 3.11828D-10 | 1.40467D-02 |
| R( 19) | 3 - 1 | 1305.60 | -1603.68 | 5.25348D-02 | 2.88603D-08 | -9.12481D-03 |
| P( 21) | 3 - 1 | 1349.97 | -1559.31 | 6.19174D-02 | 3.00804D-08 | -1.00829D-02 |
| R( 19) | 3 - 2 | 2091.67 | -817.61 | 1.05978D+01 | 5.47810D-06 | -3.56014D-01 |
| P( 21) | 3 - 2 | 2135.20 | -774.08 | 9.87318D+00 | 6.04631D-06 | -3.64027D-01 |
| R( 19) | 3 - 3 | 2888.23 | -21.05 | 4.20877D-03 | 9.99987D-01 | -1.71777D+00 |
| P( 1) | 4 - 0 | 361.22 | -3102.15 | 8.81591D+00 | 1.10358D-13 | 3.06859D-02 |
| P( 1) | 4 - 1 | 1100.96 | -2362.41 | 2.46894D-03 | 2.39909D-12 | 7.72720D-04 |
| P( 1) | 4 - 2 | 1890.87 | -1572.50 | 8.94714D-03 | 1.10278D-10 | -2.70867D-03 |
| P( 1) | 4 - 3 | 2689.17 | -774.20 | 2.82766D+01 | 1.94372D-08 | -4.40793D-01 |
| R( 0) | 4 - 0 | 360.13 | -3104.29 | 2.94330D+00 | 1.10548D-13 | 3.06785D-02 |
| P( 2) | 4 - 0 | 363.41 | -3101.01 | 5.86821D+00 | 4.40994D-13 | 3.06792D-02 |
| R( 0) | 4 - 1 | 1099.88 | -2364.54 | 8.38322D-04 | 2.40537D-12 | 7.78835D-04 |
| P( 2) | 4 - 1 | 1103.13 | -2361.29 | 1.64971D-03 | 9.58461D-12 | 7.74150D-04 |
| R( 0) | 4 - 2 | 1889.81 | -1574.61 | 2.85094D-03 | 1.10621D-10 | -2.64299D-03 |
| P( 2) | 4 - 2 | 1893.00 | -1571.42 | 6.11108D-03 | 4.40459D-10 | -2.74452D-03 |
| R( 0) | 4 - 3 | 2688.12 | -776.30 | 9.48200D+00 | 1.94357D-08 | -4.40318D-01 |
| P( 2) | 4 - 3 | 2691.28 | -773.14 | 1.87939D+01 | 7.77526D-08 | -4.41031D-01 |

| | | | | | | |
|---|---|---|---|---|---|---|
| R( 0) | 4 - 4 | 3463.37 | -1.05 | 3.68813D-07 | 1.00000D+00 | -1.75367D+00 |
| R( 1) | 4 - 0 | 361.22 | -3105.29 | 3.53210D+00 | 4.42477D-13 | 3.06643D-02 |
| P( 3) | 4 - 0 | 366.69 | -3099.82 | 5.27059D+00 | 9.91223D-13 | 3.06654D-02 |
| R( 1) | 4 - 1 | 1100.96 | -2365.55 | 1.02689D-03 | 9.63688D-12 | 7.86382D-04 |
| P( 3) | 4 - 1 | 1106.38 | -2360.13 | 1.49956D-03 | 2.15390D-11 | 7.78576D-04 |
| R( 1) | 4 - 2 | 1890.87 | -1575.64 | 3.35088D-03 | 4.43149D-10 | -2.61315D-03 |
| P( 3) | 4 - 2 | 1896.19 | -1570.32 | 5.64088D-03 | 9.89699D-10 | -2.78237D-03 |
| R( 1) | 4 - 3 | 2689.17 | -777.34 | 1.14118D+01 | 7.77441D-08 | -4.40080D-01 |
| P( 3) | 4 - 3 | 2694.44 | -772.07 | 1.68626D+01 | 1.74947D-07 | -4.41268D-01 |
| R( 1) | 4 - 4 | 3464.41 | -2.09 | 3.54067D-06 | 1.00000D+00 | -1.75373D+00 |
| R( 2) | 4 - 0 | 363.41 | -3106.24 | 3.78265D+00 | 9.96184D-13 | 3.06431D-02 |
| P( 4) | 4 - 0 | 371.06 | -3098.58 | 5.00684D+00 | 1.76017D-12 | 3.06447D-02 |
| R( 2) | 4 - 1 | 1103.13 | -2366.52 | 1.13133D-03 | 2.17173D-11 | 7.96921D-04 |
| P( 4) | 4 - 1 | 1110.71 | -2358.94 | 1.45330D-03 | 3.82494D-11 | 7.85996D-04 |
| R( 2) | 4 - 2 | 1893.00 | -1576.65 | 3.52091D-03 | 9.98718D-10 | -2.58531D-03 |
| P( 4) | 4 - 2 | 1900.44 | -1569.21 | 5.51547D-03 | 1.75711D-09 | -2.82220D-03 |
| R( 2) | 4 - 3 | 2691.28 | -778.37 | 1.22625D+01 | 1.74922D-07 | -4.39843D-01 |
| P( 4) | 4 - 3 | 2698.66 | -770.99 | 1.60099D+01 | 3.11028D-07 | -4.41506D-01 |
| R( 2) | 4 - 4 | 3466.51 | -3.14 | 1.28040D-05 | 1.00000D+00 | -1.75381D+00 |
| R( 3) | 4 - 0 | 366.69 | -3107.15 | 3.91895D+00 | 1.77193D-12 | 3.06149D-02 |
| P( 5) | 4 - 0 | 376.53 | -3097.30 | 4.85292D+00 | 2.74689D-12 | 3.06169D-02 |
| R( 3) | 4 - 1 | 1106.38 | -2367.46 | 1.21485D-03 | 3.86727D-11 | 8.10453D-04 |
| P( 5) | 4 - 1 | 1116.13 | -2357.71 | 1.44836D-03 | 5.97039D-11 | 7.96412D-04 |
| R( 3) | 4 - 2 | 1896.19 | -1577.65 | 3.58543D-03 | 1.77849D-09 | -2.55944D-03 |
| P( 5) | 4 - 2 | 1905.75 | -1568.08 | 5.51045D-03 | 2.74195D-09 | -2.86402D-03 |
| R( 3) | 4 - 3 | 2694.44 | -779.40 | 1.27532D+01 | 3.10970D-07 | -4.39605D-01 |
| P( 5) | 4 - 3 | 2703.93 | -769.91 | 1.55164D+01 | 4.86004D-07 | -4.41744D-01 |
| R( 3) | 4 - 4 | 3469.65 | -4.19 | 3.14763D-05 | 9.99999D-01 | -1.75394D+00 |
| R( 4) | 4 - 0 | 371.06 | -3108.00 | 4.00212D+00 | 2.76984D-12 | 3.05797D-02 |

| | | | | | | | | |
|---|---|---|---|---|---|---|---|---|
| P( 6) | 4 - 0 | 383.09 | -3095.97 | 4.74775D+00 | 3.95031D-12 | 3.05821D-02 |
| R( 4) | 4 - 1 | 1110.71 | -2368.36 | 1.29512D-03 | 6.05312D-11 | 8.26979D-04 |
| P( 6) | 4 - 1 | 1122.63 | -2356.44 | 1.46797D-03 | 8.58929D-11 | 8.09827D-04 |
| R( 4) | 4 - 2 | 1900.44 | -1578.63 | 3.60549D-03 | 2.78372D-09 | -2.53555D-03 |
| P( 6) | 4 - 2 | 1912.13 | -1566.94 | 5.56474D-03 | 3.94353D-09 | -2.90780D-03 |
| R( 4) | 4 - 3 | 2698.66 | -780.41 | 1.30800D+01 | 4.85890D-07 | -4.39367D-01 |
| P( 6) | 4 - 3 | 2710.25 | -768.82 | 1.51860D+01 | 6.99879D-07 | -4.41982D-01 |
| R( 4) | 4 - 4 | 3473.83 | -5.23 | 6.28800D-05 | 9.99999D-01 | -1.75410D+00 |
| R( 5) | 4 - 0 | 376.53 | -3108.82 | 4.05563D+00 | 3.98994D-12 | 3.05373D-02 |
| P( 7) | 4 - 0 | 390.75 | -3094.60 | 4.66785D+00 | 5.36923D-12 | 3.05403D-02 |
| R( 5) | 4 - 1 | 1116.13 | -2369.22 | 1.37937D-03 | 8.73232D-11 | 8.46500D-04 |
| P( 7) | 4 - 1 | 1130.21 | -2355.14 | 1.50599D-03 | 1.16809D-10 | 8.26243D-04 |
| R( 5) | 4 - 2 | 1905.75 | -1579.60 | 3.60447D-03 | 4.01572D-09 | -2.51361D-03 |
| P( 7) | 4 - 2 | 1919.57 | -1565.78 | 5.65496D-03 | 5.36121D-09 | -2.95353D-03 |
| R( 5) | 4 - 3 | 2703.93 | -781.42 | 1.33185D+01 | 6.99683D-07 | -4.39130D-01 |
| P( 7) | 4 - 3 | 2717.63 | -767.72 | 1.49433D+01 | 9.52664D-07 | -4.42220D-01 |
| R( 5) | 4 - 4 | 3479.07 | -6.28 | 1.10340D-04 | 9.99998D-01 | -1.75430D+00 |
| R( 6) | 4 - 0 | 383.09 | -3109.58 | 4.09045D+00 | 5.43212D-12 | 3.04880D-02 |
| P( 8) | 4 - 0 | 399.50 | -3093.18 | 4.60224D+00 | 7.00231D-12 | 3.04914D-02 |
| R( 6) | 4 - 1 | 1122.63 | -2370.05 | 1.47142D-03 | 1.19082D-10 | 8.69017D-04 |
| P( 8) | 4 - 1 | 1138.87 | -2353.80 | 1.55993D-03 | 1.52447D-10 | 8.45663D-04 |
| R( 6) | 4 - 2 | 1912.13 | -1580.54 | 3.59318D-03 | 5.47586D-09 | -2.49359D-03 |
| P( 8) | 4 - 2 | 1928.07 | -1564.60 | 5.77029D-03 | 6.99443D-09 | -3.00119D-03 |
| R( 6) | 4 - 3 | 2710.25 | -782.43 | 1.35038D+01 | 9.52352D-07 | -4.38892D-01 |
| P( 8) | 4 - 3 | 2726.06 | -766.62 | 1.47532D+01 | 1.24437D-06 | -4.42459D-01 |
| R( 6) | 4 - 4 | 3485.35 | -7.33 | 1.77185D-04 | 9.99998D-01 | -1.75453D+00 |
| R( 7) | 4 - 0 | 390.75 | -3110.30 | 4.11239D+00 | 7.09611D-12 | 3.04314D-02 |
| P( 9) | 4 - 0 | 409.34 | -3091.71 | 4.54515D+00 | 8.84809D-12 | 3.04354D-02 |
| R( 7) | 4 - 1 | 1130.21 | -2370.84 | 1.57378D-03 | 1.55841D-10 | 8.94533D-04 |

| | | | | | | |
|---|---|---|---|---|---|---|
| P( 9) | 4 - 1 | 1148.62 | -2352.43 | 1.62882D-03 | 1.92804D-10 | 8.68089D-04 |
| R( 7) | 4 - 2 | 1919.57 | -1581.48 | 3.57727D-03 | 7.16562D-09 | -2.47548D-03 |
| P( 9) | 4 - 2 | 1937.64 | -1563.41 | 5.90505D-03 | 8.84270D-09 | -3.05074D-03 |
| R( 7) | 4 - 3 | 2717.63 | -783.42 | 1.36545D+01 | 1.24390D-06 | -4.38654D-01 |
| P( 9) | 4 - 3 | 2735.54 | -765.51 | 1.45968D+01 | 1.57500D-06 | -4.42697D-01 |
| R( 7) | 4 - 4 | 3492.68 | -8.37 | 2.66748D-04 | 9.99997D-01 | -1.75480D+00 |
| R( 8) | 4 - 0 | 399.50 | -3110.97 | 4.12480D+00 | 8.98151D-12 | 3.03677D-02 |
| P( 10) | 4 - 0 | 420.27 | -3090.19 | 4.49322D+00 | 1.09049D-11 | 3.03722D-02 |
| R( 8) | 4 - 1 | 1138.87 | -2371.59 | 1.68835D-03 | 1.97639D-10 | 9.23051D-04 |
| P( 10) | 4 - 1 | 1159.45 | -2351.01 | 1.71249D-03 | 2.37878D-10 | 8.93526D-04 |
| R( 8) | 4 - 2 | 1928.07 | -1582.39 | 3.55991D-03 | 9.08651D-09 | -2.45925D-03 |
| P( 10) | 4 - 2 | 1948.27 | -1562.20 | 6.05603D-03 | 1.09056D-08 | -3.10217D-03 |
| R( 8) | 4 - 3 | 2726.06 | -784.41 | 1.37814D+01 | 1.57434D-06 | -4.38416D-01 |
| P( 10) | 4 - 3 | 2746.08 | -764.39 | 1.44636D+01 | 1.94457D-06 | -4.42936D-01 |
| R( 8) | 4 - 4 | 3501.05 | -9.42 | 3.82366D-04 | 9.99996D-01 | -1.75510D+00 |
| R( 9) | 4 - 0 | 409.34 | -3111.59 | 4.12977D+00 | 1.10878D-11 | 3.02968D-02 |
| P( 11) | 4 - 0 | 432.30 | -3088.63 | 4.44438D+00 | 1.31711D-11 | 3.03018D-02 |
| R( 9) | 4 - 1 | 1148.62 | -2372.31 | 1.81683D-03 | 2.44515D-10 | 9.54573D-04 |
| P( 11) | 4 - 1 | 1171.37 | -2349.57 | 1.81126D-03 | 2.87670D-10 | 9.21978D-04 |
| R( 9) | 4 - 2 | 1937.64 | -1583.29 | 3.54303D-03 | 1.12401D-08 | -2.44486D-03 |
| P( 11) | 4 - 2 | 1959.96 | -1560.97 | 6.22129D-03 | 1.31827D-08 | -3.15543D-03 |
| R( 9) | 4 - 3 | 2735.54 | -785.39 | 1.38913D+01 | 1.94366D-06 | -4.38178D-01 |
| P( 11) | 4 - 3 | 2757.67 | -763.27 | 1.43467D+01 | 2.35310D-06 | -4.43174D-01 |
| R( 9) | 4 - 4 | 3510.47 | -10.46 | 5.27382D-04 | 9.99996D-01 | -1.75544D+00 |
| R( 10) | 4 - 0 | 420.27 | -3112.17 | 4.12864D+00 | 1.34141D-11 | 3.02187D-02 |
| P( 12) | 4 - 0 | 445.42 | -3087.03 | 4.39729D+00 | 1.56447D-11 | 3.02242D-02 |
| R( 10) | 4 - 1 | 1159.45 | -2372.99 | 1.96082D-03 | 2.96509D-10 | 9.89102D-04 |
| P( 12) | 4 - 1 | 1184.36 | -2348.08 | 1.92571D-03 | 3.42181D-10 | 9.53451D-04 |
| R( 10) | 4 - 2 | 1948.27 | -1584.17 | 3.52781D-03 | 1.36282D-08 | -2.43229D-03 |

| | | | | | | | |
|---|---|---|---|---|---|---|---|
| P( 12) | 4 - 2 | 1972.71 | -1559.73 | 6.39958D-03 | 1.56738D-08 | -3.21050D-03 |
| R( 10) | 4 - 3 | 2746.08 | -786.37 | 1.39884D+01 | 2.35188D-06 | -4.37940D-01 |
| P( 12) | 4 - 3 | 2770.31 | -762.13 | 1.42419D+01 | 2.80058D-06 | -4.43413D-01 |
| R( 10) | 4 - 4 | 3520.93 | -11.51 | 7.05143D-04 | 9.99995D-01 | -1.75582D+00 |
| R( 11) | 4 - 0 | 432.30 | -3112.70 | 4.12235D+00 | 1.59597D-11 | 3.01332D-02 |
| P( 13) | 4 - 0 | 459.63 | -3085.37 | 4.35104D+00 | 1.83235D-11 | 3.01392D-02 |
| R( 11) | 4 - 1 | 1171.37 | -2373.63 | 2.12189D-03 | 3.53665D-10 | 1.02664D-03 |
| P( 13) | 4 - 1 | 1198.44 | -2346.56 | 2.05669D-03 | 4.01415D-10 | 9.87950D-04 |
| R( 11) | 4 - 2 | 1959.96 | -1585.04 | 3.51500D-03 | 1.62523D-08 | -2.42148D-03 |
| P( 13) | 4 - 2 | 1986.52 | -1558.48 | 6.59009D-03 | 1.83786D-08 | -3.26733D-03 |
| R( 11) | 4 - 3 | 2757.67 | -787.33 | 1.40758D+01 | 2.79901D-06 | -4.37701D-01 |
| P( 13) | 4 - 3 | 2784.00 | -761.00 | 1.41462D+01 | 3.28705D-06 | -4.43652D-01 |
| R( 11) | 4 - 4 | 3532.44 | -12.56 | 9.19004D-04 | 9.99994D-01 | -1.75623D+00 |
| R( 12) | 4 - 0 | 445.42 | -3113.18 | 4.11154D+00 | 1.87235D-11 | 3.00403D-02 |
| P( 14) | 4 - 0 | 474.93 | -3083.67 | 4.30499D+00 | 2.12052D-11 | 3.00470D-02 |
| R( 12) | 4 - 1 | 1184.36 | -2374.24 | 2.30170D-03 | 4.16027D-10 | 1.06720D-03 |
| P( 14) | 4 - 1 | 1213.60 | -2345.00 | 2.20522D-03 | 4.65377D-10 | 1.02548D-03 |
| R( 12) | 4 - 2 | 1972.71 | -1585.89 | 3.50509D-03 | 1.91145D-08 | -2.41240D-03 |
| P( 14) | 4 - 2 | 2001.39 | -1557.20 | 6.79227D-03 | 2.12970D-08 | -3.32588D-03 |
| R( 12) | 4 - 3 | 2770.31 | -788.29 | 1.41555D+01 | 3.28505D-06 | -4.37463D-01 |
| P( 14) | 4 - 3 | 2798.75 | -759.85 | 1.40575D+01 | 3.81251D-06 | -4.43892D-01 |
| R( 12) | 4 - 4 | 3545.00 | -13.60 | 1.17233D-03 | 9.99993D-01 | -1.75668D+00 |
| R( 13) | 4 - 0 | 459.63 | -3113.62 | 4.09669D+00 | 2.17041D-11 | 2.99400D-02 |
| P( 15) | 4 - 0 | 491.32 | -3081.93 | 4.25870D+00 | 2.42875D-11 | 2.99473D-02 |
| R( 13) | 4 - 1 | 1198.44 | -2374.81 | 2.50195D-03 | 4.83641D-10 | 1.11079D-03 |
| P( 15) | 4 - 1 | 1229.84 | -2343.41 | 2.37245D-03 | 5.34072D-10 | 1.06605D-03 |
| R( 13) | 4 - 2 | 1986.52 | -1586.72 | 3.49837D-03 | 2.22164D-08 | -2.40500D-03 |
| P( 15) | 4 - 2 | 2017.33 | -1555.91 | 7.00571D-03 | 2.44288D-08 | -3.38610D-03 |
| R( 13) | 4 - 3 | 2784.00 | -789.24 | 1.42289D+01 | 3.81001D-06 | -4.37224D-01 |

| | | | | | | | |
|---|---|---|---|---|---|---|---|
| P( 15) | 4 - 3 | 2814.54 | -758.70 | 1.39743D+01 | 4.37697D-06 | -4.44131D-01 |
| R( 13) | 4 - 4 | 3558.60 | -14.65 | 1.46848D-03 | 9.99991D-01 | -1.75717D+00 |
| R( 14) | 4 - 0 | 474.93 | -3114.01 | 4.07814D+00 | 2.49000D-11 | 2.98322D-02 |
| P( 16) | 4 - 0 | 508.80 | -3080.13 | 4.21182D+00 | 2.75675D-11 | 2.98401D-02 |
| R( 14) | 4 - 1 | 1213.60 | -2375.34 | 2.72442D-03 | 5.56555D-10 | 1.15740D-03 |
| P( 16) | 4 - 1 | 1247.16 | -2341.78 | 2.55969D-03 | 6.07508D-10 | 1.10967D-03 |
| R( 14) | 4 - 2 | 2001.39 | -1587.54 | 3.49502D-03 | 2.55602D-08 | -2.39923D-03 |
| P( 16) | 4 - 2 | 2034.33 | -1554.61 | 7.23012D-03 | 2.77740D-08 | -3.44795D-03 |
| R( 14) | 4 - 3 | 2798.75 | -790.19 | 1.42974D+01 | 4.37389D-06 | -4.36985D-01 |
| P( 16) | 4 - 3 | 2831.39 | -757.54 | 1.38955D+01 | 4.98045D-06 | -4.44371D-01 |
| R( 14) | 4 - 4 | 3573.24 | -15.69 | 1.81085D-03 | 9.99990D-01 | -1.75769D+00 |
| R( 15) | 4 - 0 | 491.32 | -3114.35 | 4.05617D+00 | 2.83094D-11 | 2.97168D-02 |
| P( 17) | 4 - 0 | 527.37 | -3078.30 | 4.16412D+00 | 3.10424D-11 | 2.97254D-02 |
| R( 15) | 4 - 1 | 1229.84 | -2375.83 | 2.97103D-03 | 6.34818D-10 | 1.20705D-03 |
| P( 17) | 4 - 1 | 1265.56 | -2340.11 | 2.76839D-03 | 6.85691D-10 | 1.15636D-03 |
| R( 15) | 4 - 2 | 2017.33 | -1588.34 | 3.49514D-03 | 2.91478D-08 | -2.39505D-03 |
| P( 17) | 4 - 2 | 2052.38 | -1553.29 | 7.46528D-03 | 3.13326D-08 | -3.51138D-03 |
| R( 15) | 4 - 3 | 2814.54 | -791.13 | 1.43616D+01 | 4.97671D-06 | -4.36746D-01 |
| P( 17) | 4 - 3 | 2849.29 | -756.38 | 1.38203D+01 | 5.62296D-06 | -4.44611D-01 |
| R( 15) | 4 - 4 | 3588.93 | -16.73 | 2.20282D-03 | 9.99989D-01 | -1.75825D+00 |
| R( 16) | 4 - 0 | 508.80 | -3114.65 | 4.03098D+00 | 3.19305D-11 | 2.95938D-02 |
| P( 18) | 4 - 0 | 547.03 | -3076.41 | 4.11541D+00 | 3.47089D-11 | 2.96030D-02 |
| R( 16) | 4 - 1 | 1247.16 | -2376.29 | 3.24376D-03 | 7.18479D-10 | 1.25975D-03 |
| P( 18) | 4 - 1 | 1285.04 | -2338.40 | 3.00010D-03 | 7.68630D-10 | 1.20611D-03 |
| R( 16) | 4 - 2 | 2034.33 | -1589.12 | 3.49877D-03 | 3.29813D-08 | -2.39239D-03 |
| P( 18) | 4 - 2 | 2071.50 | -1551.95 | 7.71098D-03 | 3.51047D-08 | -3.57632D-03 |
| R( 16) | 4 - 3 | 2831.39 | -792.06 | 1.44222D+01 | 5.61848D-06 | -4.36506D-01 |
| P( 18) | 4 - 3 | 2868.24 | -755.21 | 1.37480D+01 | 6.30452D-06 | -4.44851D-01 |
| R( 16) | 4 - 4 | 3605.67 | -17.78 | 2.64778D-03 | 9.99987D-01 | -1.75885D+00 |

| | | | | | | |
|---|---|---|---|---|---|---|
| R( 17) | 4 - 0 | 527.37 | -3114.89 | 4.00275D+00 | 3.57609D-11 | 2.94631D-02 |
| P( 19) | 4 - 0 | 567.78 | -3074.48 | 4.06555D+00 | 3.85637D-11 | 2.94730D-02 |
| R( 17) | 4 - 1 | 1265.56 | -2376.71 | 3.54474D-03 | 8.07589D-10 | 1.31550D-03 |
| P( 19) | 4 - 1 | 1305.60 | -2336.66 | 3.25650D-03 | 8.56333D-10 | 1.25894D-03 |
| R( 17) | 4 - 2 | 2052.38 | -1589.88 | 3.50589D-03 | 3.70629D-08 | -2.39119D-03 |
| P( 19) | 4 - 2 | 2091.67 | -1550.59 | 7.96706D-03 | 3.90905D-08 | -3.64272D-03 |
| R( 17) | 4 - 3 | 2849.29 | -792.98 | 1.44798D+01 | 6.29920D-06 | -4.36266D-01 |
| P( 19) | 4 - 3 | 2888.23 | -754.03 | 1.36780D+01 | 7.02514D-06 | -4.45091D-01 |
| R( 17) | 4 - 4 | 3623.45 | -18.82 | 3.14915D-03 | 9.99986D-01 | -1.75948D+00 |
| R( 18) | 4 - 0 | 547.03 | -3115.10 | 3.97161D+00 | 3.97981D-11 | 2.93245D-02 |
| P( 20) | 4 - 0 | 589.62 | -3072.51 | 4.01443D+00 | 4.26030D-11 | 2.93352D-02 |
| R( 18) | 4 - 1 | 1285.04 | -2377.09 | 3.87622D-03 | 9.02199D-10 | 1.37433D-03 |
| P( 20) | 4 - 1 | 1327.25 | -2334.89 | 3.53939D-03 | 9.48807D-10 | 1.31487D-03 |
| R( 18) | 4 - 2 | 2071.50 | -1590.63 | 3.51645D-03 | 4.13948D-08 | -2.39140D-03 |
| P( 20) | 4 - 2 | 2112.91 | -1549.22 | 8.23334D-03 | 4.32900D-08 | -3.71051D-03 |
| R( 18) | 4 - 3 | 2868.24 | -793.90 | 1.45347D+01 | 7.01888D-06 | -4.36026D-01 |
| P( 20) | 4 - 3 | 2909.28 | -752.85 | 1.36101D+01 | 7.78484D-06 | -4.45332D-01 |
| R( 18) | 4 - 4 | 3642.27 | -19.86 | 3.71035D-03 | 9.99984D-01 | -1.76015D+00 |
| R( 19) | 4 - 0 | 567.78 | -3115.25 | 3.93767D+00 | 4.40391D-11 | 2.91780D-02 |
| P( 21) | 4 - 0 | 612.55 | -3070.49 | 3.96198D+00 | 4.68229D-11 | 2.91894D-02 |
| R( 19) | 4 - 1 | 1305.60 | -2377.43 | 4.24055D-03 | 1.00236D-09 | 1.43623D-03 |
| P( 21) | 4 - 1 | 1349.97 | -2333.07 | 3.85067D-03 | 1.04606D-09 | 1.37391D-03 |
| R( 19) | 4 - 2 | 2091.67 | -1591.36 | 3.53037D-03 | 4.59794D-08 | -2.39294D-03 |
| P( 21) | 4 - 2 | 2135.20 | -1547.83 | 8.50965D-03 | 4.77036D-08 | -3.77964D-03 |
| R( 19) | 4 - 3 | 2888.23 | -794.80 | 1.45873D+01 | 7.77753D-06 | -4.35786D-01 |
| P( 21) | 4 - 3 | 2931.38 | -751.66 | 1.35439D+01 | 8.58362D-06 | -4.45573D-01 |
| R( 19) | 4 - 4 | 3662.13 | -20.91 | 4.33481D-03 | 9.99982D-01 | -1.76086D+00 |
| P( 1) | 5 - 0 | 361.22 | -3871.90 | 1.70399D+01 | 8.53069D-15 | -3.05946D-02 |
| P( 1) | 5 - 1 | 1100.96 | -3132.16 | 4.54829D+00 | 1.08342D-13 | 2.17248D-02 |

| | | | | | | | |
|---|---|---|---|---|---|---|---|
| P( 1) | 5 - 2 | 1890.87 | -2342.25 | 9.60080D-02 | 2.50885D-12 | -4.88093D-03 |
| P( 1) | 5 - 3 | 2689.17 | -1543.95 | 3.43748D-01 | 1.63519D-10 | 1.72571D-02 |
| P( 1) | 5 - 4 | 3464.41 | -768.71 | 3.67983D+01 | 2.40669D-08 | -5.08241D-01 |
| R( 0) | 5 - 0 | 360.13 | -3874.03 | 5.69148D+00 | 8.54843D-15 | -3.06004D-02 |
| P( 2) | 5 - 0 | 363.41 | -3870.75 | 1.13502D+01 | 3.41113D-14 | -3.05952D-02 |
| R( 0) | 5 - 1 | 1099.88 | -3134.28 | 1.51816D+00 | 1.08714D-13 | 2.17176D-02 |
| P( 2) | 5 - 1 | 1103.13 | -3131.03 | 3.02823D+00 | 4.32978D-13 | 2.17224D-02 |
| R( 0) | 5 - 2 | 1889.81 | -2344.35 | 3.20665D-02 | 2.51821D-12 | -4.87924D-03 |
| P( 2) | 5 - 2 | 1893.00 | -2341.16 | 6.36885D-02 | 1.00185D-11 | -4.87224D-03 |
| R( 0) | 5 - 3 | 2688.12 | -1546.04 | 1.16281D-01 | 1.64069D-10 | 1.73493D-02 |
| P( 2) | 5 - 3 | 2691.28 | -1542.88 | 2.27333D-01 | 6.52980D-10 | 1.72059D-02 |
| R( 0) | 5 - 4 | 3463.37 | -770.79 | 1.23393D+01 | 2.40648D-08 | -5.07692D-01 |
| P( 2) | 5 - 4 | 3466.51 | -767.65 | 2.44583D+01 | 9.62758D-08 | -5.08526D-01 |
| R( 0) | 5 - 5 | 4233.12 | -1.03 | 3.89516D-07 | 1.00000D+00 | -1.83359D+00 |
| R( 1) | 5 - 0 | 361.22 | -3875.01 | 6.83776D+00 | 3.42552D-14 | -3.06067D-02 |
| P( 3) | 5 - 0 | 366.69 | -3869.54 | 1.02074D+01 | 7.67574D-14 | -3.05979D-02 |
| R( 1) | 5 - 1 | 1100.96 | -3135.27 | 1.82189D+00 | 4.35676D-13 | 2.17079D-02 |
| P( 3) | 5 - 1 | 1106.38 | -3129.85 | 2.72071D+00 | 9.73720D-13 | 2.17160D-02 |
| R( 1) | 5 - 2 | 1890.87 | -2345.36 | 3.83657D-02 | 1.00951D-11 | -4.86886D-03 |
| P( 3) | 5 - 2 | 1896.19 | -2340.04 | 5.68845D-02 | 2.25037D-11 | -4.85719D-03 |
| R( 1) | 5 - 3 | 2689.17 | -1547.06 | 1.40474D-01 | 6.57318D-10 | 1.73903D-02 |
| P( 3) | 5 - 3 | 2694.44 | -1541.79 | 2.02871D-01 | 1.46686D-09 | 1.71513D-02 |
| R( 1) | 5 - 4 | 3464.41 | -771.81 | 1.48507D+01 | 9.62630D-08 | -5.07428D-01 |
| P( 3) | 5 - 4 | 3469.65 | -766.58 | 2.19457D+01 | 2.16637D-07 | -5.08817D-01 |
| R( 1) | 5 - 5 | 4234.16 | -2.07 | 3.73941D-06 | 1.00000D+00 | -1.83365D+00 |
| R( 2) | 5 - 0 | 363.41 | -3875.92 | 7.33547D+00 | 7.72456D-14 | -3.06153D-02 |
| P( 4) | 5 - 0 | 371.06 | -3868.27 | 9.71497D+00 | 1.36536D-13 | -3.06030D-02 |
| R( 2) | 5 - 1 | 1103.13 | -3136.21 | 1.95131D+00 | 9.82626D-13 | 2.16942D-02 |
| P( 4) | 5 - 1 | 1110.71 | -3128.62 | 2.58561D+00 | 1.73075D-12 | 2.17055D-02 |

| | | | | | | | |
|---|---|---|---|---|---|---|---|
| R( 2) | 5 - 2 | 1893.00 | -2346.33 | 4.08751D-02 | 2.27643D-11 | -4.85212D-03 |
| P( 4) | 5 - 2 | 1900.44 | -2338.89 | 5.36204D-02 | 3.99462D-11 | -4.83579D-03 |
| R( 2) | 5 - 3 | 2691.28 | -1548.05 | 1.51451D-01 | 1.48143D-09 | 1.74279D-02 |
| P( 4) | 5 - 3 | 2698.66 | -1540.68 | 1.91491D-01 | 2.60352D-09 | 1.70933D-02 |
| R( 2) | 5 - 4 | 3466.51 | -772.82 | 1.59579D+01 | 2.16599D-07 | -5.07170D-01 |
| P( 4) | 5 - 4 | 3473.83 | -765.50 | 2.08366D+01 | 3.85179D-07 | -5.09115D-01 |
| R( 2) | 5 - 5 | 4236.23 | -3.10 | 1.35225D-05 | 1.00000D+00 | -1.83373D+00 |
| R( 3) | 5 - 0 | 366.69 | -3876.78 | 7.61757D+00 | 1.37694D-13 | -3.06261D-02 |
| P( 5) | 5 - 0 | 376.53 | -3866.94 | 9.43988D+00 | 2.13560D-13 | -3.06103D-02 |
| R( 3) | 5 - 1 | 1106.38 | -3137.09 | 2.02199D+00 | 1.75176D-12 | 2.16765D-02 |
| P( 5) | 5 - 1 | 1116.13 | -3127.35 | 2.50736D+00 | 2.70481D-12 | 2.16910D-02 |
| R( 3) | 5 - 2 | 1896.19 | -2347.28 | 4.20376D-02 | 4.05642D-11 | -4.82904D-03 |
| P( 5) | 5 - 2 | 1905.75 | -2337.72 | 5.14567D-02 | 6.23293D-11 | -4.80804D-03 |
| R( 3) | 5 - 3 | 2694.44 | -1549.03 | 1.57976D-01 | 2.63805D-09 | 1.74621D-02 |
| P( 5) | 5 - 3 | 2703.93 | -1539.55 | 1.84429D-01 | 4.06142D-09 | 1.70318D-02 |
| R( 3) | 5 - 4 | 3469.65 | -773.82 | 1.65967D+01 | 3.85089D-07 | -5.06919D-01 |
| P( 5) | 5 - 4 | 3479.07 | -764.40 | 2.01952D+01 | 6.01930D-07 | -5.09420D-01 |
| R( 3) | 5 - 5 | 4239.33 | -4.14 | 3.32425D-05 | 9.99999D-01 | -1.83385D+00 |
| R( 4) | 5 - 0 | 371.06 | -3877.58 | 7.80214D+00 | 2.15824D-13 | -3.06391D-02 |
| P( 6) | 5 - 0 | 383.09 | -3865.55 | 9.26402D+00 | 3.07989D-13 | -3.06198D-02 |
| R( 4) | 5 - 1 | 1110.71 | -3137.94 | 2.06546D+00 | 2.74578D-12 | 2.16547D-02 |
| P( 6) | 5 - 1 | 1122.63 | -3126.02 | 2.45446D+00 | 3.89710D-12 | 2.16726D-02 |
| R( 4) | 5 - 2 | 1900.44 | -2348.21 | 4.25205D-02 | 6.35367D-11 | -4.79960D-03 |
| P( 6) | 5 - 2 | 1912.13 | -2336.51 | 4.97301D-02 | 8.96401D-11 | -4.77394D-03 |
| R( 4) | 5 - 3 | 2698.66 | -1549.99 | 1.62438D-01 | 4.12887D-09 | 1.74929D-02 |
| P( 6) | 5 - 3 | 2710.25 | -1538.40 | 1.79296D-01 | 5.83902D-09 | 1.69669D-02 |
| R( 4) | 5 - 4 | 3473.83 | -774.81 | 1.70225D+01 | 6.01754D-07 | -5.06674D-01 |
| P( 6) | 5 - 4 | 3485.35 | -763.30 | 1.97662D+01 | 8.66927D-07 | -5.09732D-01 |
| R( 4) | 5 - 5 | 4243.47 | -5.17 | 6.64074D-05 | 9.99999D-01 | -1.83401D+00 |

| | | | | | | |
|---|---|---|---|---|---|---|
| R( 5) | 5 - 0 | 376.53 | -3878.32 | 7.93457D+00 | 3.11905D-13 | -3.06543D-02 |
| P( 7) | 5 - 0 | 390.75 | -3864.10 | 9.14198D+00 | 4.20028D-13 | -3.06315D-02 |
| R( 5) | 5 - 1 | 1116.13 | -3138.73 | 2.09383D+00 | 3.96790D-12 | 2.16289D-02 |
| P( 7) | 5 - 1 | 1130.21 | -3124.64 | 2.41479D+00 | 5.30932D-12 | 2.16501D-02 |
| R( 5) | 5 - 2 | 1905.75 | -2349.10 | 4.25819D-02 | 9.17275D-11 | -4.76382D-03 |
| P( 7) | 5 - 2 | 1919.57 | -2335.28 | 4.81880D-02 | 1.21870D-10 | -4.73350D-03 |
| R( 5) | 5 - 3 | 2703.93 | -1550.93 | 1.65754D-01 | 5.95558D-09 | 1.75202D-02 |
| P( 7) | 5 - 3 | 2717.63 | -1537.23 | 1.75174D-01 | 7.93481D-09 | 1.68985D-02 |
| R( 5) | 5 - 4 | 3479.07 | -775.78 | 1.73334D+01 | 8.66623D-07 | -5.06436D-01 |
| P( 7) | 5 - 4 | 3492.68 | -762.18 | 1.94515D+01 | 1.18022D-06 | -5.10050D-01 |
| R( 5) | 5 - 5 | 4248.64 | -6.21 | 1.16528D-04 | 9.99998D-01 | -1.83419D+00 |
| R( 6) | 5 - 0 | 383.09 | -3879.00 | 8.03605D+00 | 4.26256D-13 | -3.06716D-02 |
| P( 8) | 5 - 0 | 399.50 | -3862.60 | 9.05254D+00 | 5.49931D-13 | -3.06454D-02 |
| R( 6) | 5 - 1 | 1122.63 | -3139.47 | 2.11277D+00 | 5.42182D-12 | 2.15992D-02 |
| P( 8) | 5 - 1 | 1138.87 | -3123.22 | 2.38269D+00 | 6.94363D-12 | 2.16237D-02 |
| R( 6) | 5 - 2 | 1912.13 | -2349.96 | 4.23437D-02 | 1.25186D-10 | -4.72169D-03 |
| P( 8) | 5 - 2 | 1928.07 | -2334.02 | 4.67146D-02 | 1.59013D-10 | -4.68671D-03 |
| R( 6) | 5 - 3 | 2710.25 | -1551.85 | 1.68354D-01 | 8.11992D-09 | 1.75442D-02 |
| P( 8) | 5 - 3 | 2726.06 | -1536.04 | 1.71635D-01 | 1.03473D-08 | 1.68267D-02 |
| R( 6) | 5 - 4 | 3485.35 | -776.75 | 1.75752D+01 | 1.17973D-06 | -5.06205D-01 |
| P( 8) | 5 - 4 | 3501.05 | -761.05 | 1.92051D+01 | 1.54185D-06 | -5.10376D-01 |
| R( 6) | 5 - 5 | 4254.85 | -7.24 | 1.87118D-04 | 9.99997D-01 | -1.83442D+00 |
| R( 7) | 5 - 0 | 390.75 | -3879.62 | 8.11776D+00 | 5.59243D-13 | -3.06911D-02 |
| P( 9) | 5 - 0 | 409.34 | -3861.03 | 8.98445D+00 | 6.97997D-13 | -3.06614D-02 |
| R( 7) | 5 - 1 | 1130.21 | -3140.16 | 2.12527D+00 | 7.11175D-12 | 2.15654D-02 |
| P( 9) | 5 - 1 | 1148.62 | -3121.75 | 2.35520D+00 | 8.80270D-12 | 2.15933D-02 |
| R( 7) | 5 - 2 | 1919.57 | -2350.80 | 4.18722D-02 | 1.63967D-10 | -4.67323D-03 |
| P( 9) | 5 - 2 | 1937.64 | -2332.73 | 4.52509D-02 | 2.01068D-10 | -4.63360D-03 |
| R( 7) | 5 - 3 | 2717.63 | -1552.75 | 1.70462D-01 | 1.06236D-08 | 1.75647D-02 |

| | | | | | | |
|---|---|---|---|---|---|---|
| P( 9) | 5 - 3 | 2735.54 | -1534.83 | 1.68454D-01 | 1.30749D-08 | 1.67514D-02 |
| R( 7) | 5 - 4 | 3492.68 | -777.70 | 1.77722D+01 | 1.54113D-06 | -5.05980D-01 |
| P( 9) | 5 - 4 | 3510.47 | -759.91 | 1.90030D+01 | 1.95189D-06 | -5.10708D-01 |
| R( 7) | 5 - 5 | 4262.10 | -8.28 | 2.81696D-04 | 9.99997D-01 | -1.83467D+00 |
| R( 8) | 5 - 0 | 399.50 | -3880.19 | 8.18620D+00 | 7.11279D-13 | -3.07126D-02 |
| P( 10) | 5 - 0 | 420.27 | -3859.41 | 8.93119D+00 | 8.64568D-13 | -3.06795D-02 |
| R( 8) | 5 - 1 | 1138.87 | -3140.81 | 2.13308D+00 | 9.04243D-12 | 2.15276D-02 |
| P( 10) | 5 - 1 | 1159.45 | -3120.23 | 2.33058D+00 | 1.08897D-11 | 2.15589D-02 |
| R( 8) | 5 - 2 | 1928.07 | -2351.61 | 4.12077D-02 | 2.08126D-10 | -4.61844D-03 |
| P( 10) | 5 - 2 | 1948.27 | -2331.42 | 4.37653D-02 | 2.48037D-10 | -4.57416D-03 |
| R( 8) | 5 - 3 | 2726.06 | -1553.63 | 1.72211D-01 | 1.34685D-08 | 1.75818D-02 |
| P( 10) | 5 - 3 | 2746.08 | -1533.61 | 1.65500D-01 | 1.61163D-08 | 1.66726D-02 |
| R( 8) | 5 - 4 | 3501.05 | -778.64 | 1.79385D+01 | 1.95086D-06 | -5.05761D-01 |
| P( 10) | 5 - 4 | 3520.93 | -758.75 | 1.88309D+01 | 2.41040D-06 | -5.11048D-01 |
| R( 8) | 5 - 5 | 4270.37 | -9.31 | 4.03781D-04 | 9.99996D-01 | -1.83496D+00 |
| R( 9) | 5 - 0 | 409.34 | -3880.69 | 8.24535D+00 | 8.82825D-13 | -3.07362D-02 |
| P( 11) | 5 - 0 | 432.30 | -3857.73 | 8.88871D+00 | 1.05003D-12 | -3.06997D-02 |
| R( 9) | 5 - 1 | 1148.62 | -3141.41 | 2.13727D+00 | 1.12191D-11 | 2.14858D-02 |
| P( 11) | 5 - 1 | 1171.37 | -3118.66 | 2.30777D+00 | 1.32081D-11 | 2.15207D-02 |
| R( 9) | 5 - 2 | 1937.64 | -2352.39 | 4.03768D-02 | 2.57726D-10 | -4.55733D-03 |
| P( 11) | 5 - 2 | 1959.96 | -2330.07 | 4.22404D-02 | 2.99926D-10 | -4.50840D-03 |
| R( 9) | 5 - 3 | 2735.54 | -1554.49 | 1.73679D-01 | 1.66563D-08 | 1.75955D-02 |
| P( 11) | 5 - 3 | 2757.67 | -1532.36 | 1.62692D-01 | 1.94700D-08 | 1.65902D-02 |
| R( 9) | 5 - 4 | 3510.47 | -779.56 | 1.80827D+01 | 2.40899D-06 | -5.05549D-01 |
| P( 11) | 5 - 4 | 3532.44 | -757.59 | 1.86803D+01 | 2.91746D-06 | -5.11394D-01 |
| R( 9) | 5 - 5 | 4279.68 | -10.34 | 5.56902D-04 | 9.99995D-01 | -1.83529D+00 |
| R( 10) | 5 - 0 | 420.27 | -3881.14 | 8.29780D+00 | 1.07439D-12 | -3.07617D-02 |
| P( 12) | 5 - 0 | 445.42 | -3855.99 | 8.85436D+00 | 1.25482D-12 | -3.07218D-02 |
| R( 10) | 5 - 1 | 1159.45 | -3141.96 | 2.13856D+00 | 1.36476D-11 | 2.14401D-02 |

| | | | | | | | | |
|---|---|---|---|---|---|---|---|---|
| P( 12) | 5 - 1 | 1184.36 | -3117.05 | 2.28609D+00 | 1.57622D-11 | 2.14785D-02 |
| R( 10) | 5 - 2 | 1948.27 | -2353.14 | 3.93991D-02 | 3.12834D-10 | -4.48991D-03 |
| P( 12) | 5 - 2 | 1972.71 | -2328.70 | 4.06671D-02 | 3.56745D-10 | -4.43633D-03 |
| R( 10) | 5 - 3 | 2746.08 | -1555.33 | 1.74920D-01 | 2.01889D-08 | 1.76056D-02 |
| P( 12) | 5 - 3 | 2770.31 | -1531.10 | 1.59979D-01 | 2.31346D-08 | 1.65043D-02 |
| R( 10) | 5 - 4 | 3520.93 | -780.48 | 1.82104D+01 | 2.91558D-06 | -5.05344D-01 |
| P( 12) | 5 - 4 | 3545.00 | -756.41 | 1.85455D+01 | 3.47315D-06 | -5.11747D-01 |
| R( 10) | 5 - 5 | 4290.03 | -11.38 | 7.44587D-04 | 9.99994D-01 | -1.83565D+00 |
| R( 11) | 5 - 0 | 432.30 | -3881.52 | 8.34531D+00 | 1.28652D-12 | -3.07891D-02 |
| P( 13) | 5 - 0 | 459.63 | -3854.19 | 8.82631D+00 | 1.47941D-12 | -3.07458D-02 |
| R( 11) | 5 - 1 | 1171.37 | -3142.45 | 2.13743D+00 | 1.63341D-11 | 2.13905D-02 |
| P( 13) | 5 - 1 | 1198.44 | -3115.38 | 2.26508D+00 | 1.85565D-11 | 2.14325D-02 |
| R( 11) | 5 - 2 | 1959.96 | -2353.86 | 3.82896D-02 | 3.73519D-10 | -4.41618D-03 |
| P( 13) | 5 - 2 | 1986.52 | -2327.30 | 3.90417D-02 | 4.18508D-10 | -4.35796D-03 |
| R( 11) | 5 - 3 | 2757.67 | -1556.15 | 1.75968D-01 | 2.40681D-08 | 1.76123D-02 |
| P( 13) | 5 - 3 | 2784.00 | -1529.82 | 1.57326D-01 | 2.71087D-08 | 1.64149D-02 |
| R( 11) | 5 - 4 | 3532.44 | -781.38 | 1.83256D+01 | 3.47071D-06 | -5.05144D-01 |
| P( 13) | 5 - 4 | 3558.60 | -755.22 | 1.84226D+01 | 4.07756D-06 | -5.12107D-01 |
| R( 11) | 5 - 5 | 4301.41 | -12.41 | 9.70375D-04 | 9.99992D-01 | -1.83604D+00 |
| R( 12) | 5 - 0 | 445.42 | -3881.85 | 8.38910D+00 | 1.51981D-12 | -3.08183D-02 |
| P( 14) | 5 - 0 | 474.93 | -3852.34 | 8.80328D+00 | 1.72432D-12 | -3.07718D-02 |
| R( 12) | 5 - 1 | 1184.36 | -3142.90 | 2.13421D+00 | 1.92856D-11 | 2.13369D-02 |
| P( 14) | 5 - 1 | 1213.60 | -3113.67 | 2.24442D+00 | 2.15961D-11 | 2.13826D-02 |
| R( 12) | 5 - 2 | 1972.71 | -2354.56 | 3.70613D-02 | 4.39856D-10 | -4.33616D-03 |
| P( 14) | 5 - 2 | 2001.39 | -2325.87 | 3.73638D-02 | 4.85232D-10 | -4.27331D-03 |
| R( 12) | 5 - 3 | 2770.31 | -1556.96 | 1.76849D-01 | 2.82958D-08 | 1.76155D-02 |
| P( 14) | 5 - 3 | 2798.75 | -1528.52 | 1.54709D-01 | 3.13909D-08 | 1.63218D-02 |
| R( 12) | 5 - 4 | 3545.00 | -782.27 | 1.84309D+01 | 4.07446D-06 | -5.04951D-01 |
| P( 14) | 5 - 4 | 3573.24 | -754.02 | 1.83089D+01 | 4.73078D-06 | -5.12474D-01 |

| | | | | | | | |
|---|---|---|---|---|---|---|---|
| R( 12) | 5 - 5 | 4313.82 | -13.45 | 1.23781D-03 | 9.99991D-01 | -1.83646D+00 |
| R( 13) | 5 - 0 | 459.63 | -3882.12 | 8.43003D+00 | 1.77492D-12 | -3.08493D-02 |
| P( 15) | 5 - 0 | 491.32 | -3850.43 | 8.78431D+00 | 1.99010D-12 | -3.07994D-02 |
| R( 13) | 5 - 1 | 1198.44 | -3143.31 | 2.12918D+00 | 2.25094D-11 | 2.12794D-02 |
| P( 15) | 5 - 1 | 1229.84 | -3111.91 | 2.22387D+00 | 2.48866D-11 | 2.13288D-02 |
| R( 13) | 5 - 2 | 1986.52 | -2355.22 | 3.57255D-02 | 5.11925D-10 | -4.24986D-03 |
| P( 15) | 5 - 2 | 2017.33 | -2324.41 | 3.56355D-02 | 5.56940D-10 | -4.18238D-03 |
| R( 13) | 5 - 3 | 2784.00 | -1557.74 | 1.77579D-01 | 3.28739D-08 | 1.76151D-02 |
| P( 15) | 5 - 3 | 2814.54 | -1527.20 | 1.52110D-01 | 3.59799D-08 | 1.62251D-02 |
| R( 13) | 5 - 4 | 3558.60 | -783.15 | 1.85284D+01 | 4.72691D-06 | -5.04765D-01 |
| P( 15) | 5 - 4 | 3588.93 | -752.81 | 1.82024D+01 | 5.43293D-06 | -5.12848D-01 |
| R( 13) | 5 - 5 | 4327.27 | -14.48 | 1.55043D-03 | 9.99990D-01 | -1.83692D+00 |
| R( 14) | 5 - 0 | 474.93 | -3882.33 | 8.46873D+00 | 2.05251D-12 | -3.08820D-02 |
| P( 16) | 5 - 0 | 508.80 | -3848.45 | 8.76868D+00 | 2.27735D-12 | -3.08289D-02 |
| R( 14) | 5 - 1 | 1213.60 | -3143.66 | 2.12251D+00 | 2.60134D-11 | 2.12181D-02 |
| P( 16) | 5 - 1 | 1247.16 | -3110.10 | 2.20328D+00 | 2.84340D-11 | 2.12713D-02 |
| R( 14) | 5 - 2 | 2001.39 | -2355.86 | 3.42928D-02 | 5.89811D-10 | -4.15730D-03 |
| P( 16) | 5 - 2 | 2034.33 | -2322.93 | 3.38606D-02 | 6.33659D-10 | -4.08520D-03 |
| R( 14) | 5 - 3 | 2798.75 | -1558.51 | 1.78172D-01 | 3.78045D-08 | 1.76113D-02 |
| P( 16) | 5 - 3 | 2831.39 | -1525.86 | 1.49518D-01 | 4.08744D-08 | 1.61247D-02 |
| R( 14) | 5 - 4 | 3573.24 | -784.01 | 1.86194D+01 | 5.42817D-06 | -5.04584D-01 |
| P( 16) | 5 - 4 | 3605.67 | -751.59 | 1.81017D+01 | 6.18412D-06 | -5.13229D-01 |
| R( 14) | 5 - 5 | 4341.74 | -15.51 | 1.91181D-03 | 9.99988D-01 | -1.83741D+00 |
| R( 15) | 5 - 0 | 491.32 | -3882.48 | 8.50567D+00 | 2.35333D-12 | -3.09162D-02 |
| P( 17) | 5 - 0 | 527.37 | -3846.43 | 8.75583D+00 | 2.58671D-12 | -3.08599D-02 |
| R( 15) | 5 - 1 | 1229.84 | -3143.96 | 2.11435D+00 | 2.98061D-11 | 2.11528D-02 |
| P( 17) | 5 - 1 | 1265.56 | -3108.24 | 2.18254D+00 | 3.22449D-11 | 2.12100D-02 |
| R( 15) | 5 - 2 | 2017.33 | -2356.47 | 3.27734D-02 | 6.73603D-10 | -4.05849D-03 |
| P( 17) | 5 - 2 | 2052.38 | -2321.42 | 3.20442D-02 | 7.15418D-10 | -3.98178D-03 |

| | | | | | | | |
|---|---|---|---|---|---|---|---|
| R( 15) | 5 - 3 | 2814.54 | -1559.25 | 1.78638D-01 | 4.30895D-08 | 1.76038D-02 |
| P( 17) | 5 - 3 | 2849.29 | -1524.51 | 1.46923D-01 | 4.60732D-08 | 1.60207D-02 |
| R( 15) | 5 - 4 | 3588.93 | -784.86 | 1.87050D+01 | 6.17833D-06 | -5.04410D-01 |
| P( 17) | 5 - 4 | 3623.45 | -750.35 | 1.80057D+01 | 6.98446D-06 | -5.13617D-01 |
| R( 15) | 5 - 5 | 4357.25 | -16.54 | 2.32551D-03 | 9.99986D-01 | -1.83794D+00 |
| R( 16) | 5 - 0 | 508.80 | -3882.57 | 8.54120D+00 | 2.67814D-12 | -3.09520D-02 |
| P( 18) | 5 - 0 | 547.03 | -3844.34 | 8.74533D+00 | 2.91883D-12 | -3.08924D-02 |
| R( 16) | 5 - 1 | 1247.16 | -3144.21 | 2.10483D+00 | 3.38966D-11 | 2.10838D-02 |
| P( 18) | 5 - 1 | 1285.04 | -3106.33 | 2.16154D+00 | 3.63264D-11 | 2.11450D-02 |
| R( 16) | 5 - 2 | 2034.33 | -2357.05 | 3.11773D-02 | 7.63396D-10 | -3.95345D-03 |
| P( 18) | 5 - 2 | 2071.50 | -2319.87 | 3.01926D-02 | 8.02253D-10 | -3.87213D-03 |
| R( 16) | 5 - 3 | 2831.39 | -1559.98 | 1.78982D-01 | 4.87310D-08 | 1.75928D-02 |
| P( 18) | 5 - 3 | 2868.24 | -1523.14 | 1.44319D-01 | 5.15750D-08 | 1.59129D-02 |
| R( 16) | 5 - 4 | 3605.67 | -785.70 | 1.87862D+01 | 6.97751D-06 | -5.04242D-01 |
| P( 18) | 5 - 4 | 3642.27 | -749.11 | 1.79135D+01 | 7.83408D-06 | -5.14012D-01 |
| R( 16) | 5 - 5 | 4373.80 | -17.57 | 2.79509D-03 | 9.99985D-01 | -1.83850D+00 |
| R( 17) | 5 - 0 | 527.37 | -3882.61 | 8.57556D+00 | 3.02773D-12 | -3.09892D-02 |
| P( 19) | 5 - 0 | 567.78 | -3842.19 | 8.73680D+00 | 3.27444D-12 | -3.09264D-02 |
| R( 17) | 5 - 1 | 1265.56 | -3144.42 | 2.09404D+00 | 3.82945D-11 | 2.10110D-02 |
| P( 19) | 5 - 1 | 1305.60 | -3104.38 | 2.14024D+00 | 4.06859D-11 | 2.10762D-02 |
| R( 17) | 5 - 2 | 2052.38 | -2357.60 | 2.95148D-02 | 8.59290D-10 | -3.84219D-03 |
| P( 19) | 5 - 2 | 2091.67 | -2318.30 | 2.83128D-02 | 8.94204D-10 | -3.75628D-03 |
| R( 17) | 5 - 3 | 2849.29 | -1560.69 | 1.79212D-01 | 5.47310D-08 | 1.75781D-02 |
| P( 19) | 5 - 3 | 2888.23 | -1521.74 | 1.41701D-01 | 5.73787D-08 | 1.58014D-02 |
| R( 17) | 5 - 4 | 3623.45 | -786.53 | 1.88635D+01 | 7.82583D-06 | -5.04080D-01 |
| P( 19) | 5 - 4 | 3662.13 | -747.85 | 1.78245D+01 | 8.73312D-06 | -5.14414D-01 |
| R( 17) | 5 - 5 | 4391.37 | -18.61 | 3.32414D-03 | 9.99983D-01 | -1.83909D+00 |
| R( 18) | 5 - 0 | 547.03 | -3882.58 | 8.60895D+00 | 3.40297D-12 | -3.10276D-02 |
| P( 20) | 5 - 0 | 589.62 | -3839.99 | 8.72994D+00 | 3.65427D-12 | -3.09618D-02 |

| | | | | | | | |
|---|---|---|---|---|---|---|---|
| R( 18) | 5 - 1 | 1285.04 | -3144.58 | 2.08207D+00 | 4.30098D-11 | 2.09343D-02 |
| P( 20) | 5 - 1 | 1327.25 | -3102.37 | 2.11857D+00 | 4.53316D-11 | 2.10038D-02 |
| R( 18) | 5 - 2 | 2071.50 | -2358.12 | 2.77959D-02 | 9.61390D-10 | -3.72475D-03 |
| P( 20) | 5 - 2 | 2112.91 | -2316.71 | 2.64127D-02 | 9.91315D-10 | -3.63426D-03 |
| R( 18) | 5 - 3 | 2868.24 | -1561.38 | 1.79331D-01 | 6.10918D-08 | 1.75598D-02 |
| P( 20) | 5 - 3 | 2909.28 | -1520.34 | 1.39065D-01 | 6.34830D-08 | 1.56861D-02 |
| R( 18) | 5 - 4 | 3642.27 | -787.35 | 1.89376D+01 | 8.72342D-06 | -5.03924D-01 |
| P( 20) | 5 - 4 | 3683.04 | -746.58 | 1.77382D+01 | 9.68172D-06 | -5.14822D-01 |
| R( 18) | 5 - 5 | 4409.98 | -19.64 | 3.91625D-03 | 9.99981D-01 | -1.83971D+00 |
| R( 19) | 5 - 0 | 567.78 | -3882.50 | 8.64150D+00 | 3.80472D-12 | -3.10673D-02 |
| P( 21) | 5 - 0 | 612.55 | -3837.74 | 8.72449D+00 | 4.05907D-12 | -3.09984D-02 |
| R( 19) | 5 - 1 | 1305.60 | -3144.68 | 2.06898D+00 | 4.80534D-11 | 2.08540D-02 |
| P( 21) | 5 - 1 | 1349.97 | -3100.32 | 2.09652D+00 | 5.02719D-11 | 2.09277D-02 |
| R( 19) | 5 - 2 | 2091.67 | -2358.61 | 2.60313D-02 | 1.06981D-09 | -3.60114D-03 |
| P( 21) | 5 - 2 | 2135.20 | -2315.08 | 2.45007D-02 | 1.09364D-09 | -3.50608D-03 |
| R( 19) | 5 - 3 | 2888.23 | -1562.05 | 1.79342D-01 | 6.78155D-08 | 1.75378D-02 |
| P( 21) | 5 - 3 | 2931.38 | -1518.91 | 1.36409D-01 | 6.98870D-08 | 1.55670D-02 |
| R( 19) | 5 - 4 | 3662.13 | -788.15 | 1.90087D+01 | 9.67039D-06 | -5.03774D-01 |
| P( 21) | 5 - 4 | 3704.99 | -745.30 | 1.76540D+01 | 1.06800D-05 | -5.15238D-01 |
| R( 19) | 5 - 5 | 4429.62 | -20.67 | 4.57501D-03 | 9.99979D-01 | -1.84037D+00 |
| Q( 0) | 0 - 0 | 360.13 | 0.00 | 0.00000D+00 | 1.00000D+00 | -1.42099D+00 |
| Q( 1) | 0 - 0 | 361.22 | -0.00 | 0.00000D+00 | 1.00000D+00 | -1.42102D+00 |
| Q( 2) | 0 - 0 | 363.41 | -0.00 | 0.00000D+00 | 1.00000D+00 | -1.42108D+00 |
| Q( 3) | 0 - 0 | 366.69 | -0.00 | 0.00000D+00 | 1.00000D+00 | -1.42117D+00 |
| Q( 4) | 0 - 0 | 371.06 | -0.00 | 0.00000D+00 | 1.00000D+00 | -1.42128D+00 |
| Q( 5) | 0 - 0 | 376.53 | -0.00 | 0.00000D+00 | 1.00000D+00 | -1.42143D+00 |
| Q( 6) | 0 - 0 | 383.09 | -0.00 | 0.00000D+00 | 1.00000D+00 | -1.42160D+00 |
| Q( 7) | 0 - 0 | 390.75 | -0.00 | 0.00000D+00 | 1.00000D+00 | -1.42180D+00 |
| Q( 8) | 0 - 0 | 399.50 | -0.00 | 0.00000D+00 | 1.00000D+00 | -1.42203D+00 |

| | | | | | | |
|---|---|---|---|---|---|---|
| Q( 9) | 0 - 0 | 409.34 | -0.00 | 0.00000D+00 | 1.00000D+00 | -1.42229D+00 |
| Q( 10) | 0 - 0 | 420.27 | -0.00 | 0.00000D+00 | 1.00000D+00 | -1.42258D+00 |
| Q( 11) | 0 - 0 | 432.30 | -0.00 | 0.00000D+00 | 1.00000D+00 | -1.42290D+00 |
| Q( 12) | 0 - 0 | 445.42 | -0.00 | 0.00000D+00 | 1.00000D+00 | -1.42325D+00 |
| Q( 13) | 0 - 0 | 459.63 | -0.00 | 0.00000D+00 | 1.00000D+00 | -1.42362D+00 |
| Q( 14) | 0 - 0 | 474.93 | -0.00 | 0.00000D+00 | 1.00000D+00 | -1.42403D+00 |
| Q( 15) | 0 - 0 | 491.32 | -0.00 | 0.00000D+00 | 1.00000D+00 | -1.42447D+00 |
| Q( 16) | 0 - 0 | 508.80 | -0.00 | 0.00000D+00 | 1.00000D+00 | -1.42493D+00 |
| Q( 17) | 0 - 0 | 527.37 | -0.00 | 0.00000D+00 | 1.00000D+00 | -1.42543D+00 |
| Q( 18) | 0 - 0 | 547.03 | -0.00 | 0.00000D+00 | 1.00000D+00 | -1.42595D+00 |
| Q( 19) | 0 - 0 | 567.78 | -0.00 | 0.00000D+00 | 1.00000D+00 | -1.42651D+00 |
| Q( 20) | 0 - 0 | 589.62 | -0.00 | 0.00000D+00 | 1.00000D+00 | -1.42710D+00 |
| Q( 0) | 1 - 0 | 360.13 | -739.75 | 0.00000D+00 | 1.70479D-21 | -1.83707D-01 |
| Q( 0) | 1 - 1 | 1099.88 | 0.00 | 0.00000D+00 | 1.00000D+00 | -1.55792D+00 |
| Q( 1) | 1 - 0 | 361.22 | -739.74 | 0.00000D+00 | 2.70065D-18 | -1.83723D-01 |
| Q( 1) | 1 - 1 | 1100.96 | -0.00 | 0.00000D+00 | 1.00000D+00 | -1.55794D+00 |
| Q( 2) | 1 - 0 | 363.41 | -739.72 | 0.00000D+00 | 2.75157D-28 | -1.83753D-01 |
| Q( 2) | 1 - 1 | 1103.13 | 0.00 | 0.00000D+00 | 1.00000D+00 | -1.55799D+00 |
| Q( 3) | 1 - 0 | 366.69 | -739.69 | 0.00000D+00 | 1.93180D-29 | -1.83799D-01 |
| Q( 3) | 1 - 1 | 1106.38 | 0.00 | 0.00000D+00 | 1.00000D+00 | -1.55807D+00 |
| Q( 4) | 1 - 0 | 371.06 | -739.65 | 0.00000D+00 | 1.32302D-27 | -1.83860D-01 |
| Q( 4) | 1 - 1 | 1110.71 | 0.00 | 0.00000D+00 | 1.00000D+00 | -1.55817D+00 |
| Q( 5) | 1 - 0 | 376.53 | -739.59 | 0.00000D+00 | 2.13922D-28 | -1.83937D-01 |
| Q( 5) | 1 - 1 | 1116.13 | 0.00 | 0.00000D+00 | 1.00000D+00 | -1.55830D+00 |
| Q( 6) | 1 - 0 | 383.09 | -739.53 | 0.00000D+00 | 2.02478D-27 | -1.84029D-01 |
| Q( 6) | 1 - 1 | 1122.63 | 0.00 | 0.00000D+00 | 1.00000D+00 | -1.55845D+00 |
| Q( 7) | 1 - 0 | 390.75 | -739.46 | 0.00000D+00 | 7.32015D-27 | -1.84136D-01 |
| Q( 7) | 1 - 1 | 1130.21 | 0.00 | 0.00000D+00 | 1.00000D+00 | -1.55863D+00 |
| Q( 8) | 1 - 0 | 399.50 | -739.38 | 0.00000D+00 | 1.64220D-26 | -1.84258D-01 |

| | | | | | | |
|---|---|---|---|---|---|---|
| Q( 8) | 1 - 1 | 1138.87 | 0.00 | 0.00000D+00 | 1.00000D+00 | -1.55884D+00 |
| Q( 9) | 1 - 0 | 409.34 | -739.28 | 0.00000D+00 | 5.21972D-26 | -1.84396D-01 |
| Q( 9) | 1 - 1 | 1148.62 | 0.00 | 0.00000D+00 | 1.00000D+00 | -1.55907D+00 |
| Q( 10) | 1 - 0 | 420.27 | -739.18 | 0.00000D+00 | 1.13861D-25 | -1.84549D-01 |
| Q( 10) | 1 - 1 | 1159.45 | 0.00 | 0.00000D+00 | 1.00000D+00 | -1.55933D+00 |
| Q( 11) | 1 - 0 | 432.30 | -739.07 | 0.00000D+00 | 2.39434D-25 | -1.84718D-01 |
| Q( 11) | 1 - 1 | 1171.37 | 0.00 | 0.00000D+00 | 1.00000D+00 | -1.55961D+00 |
| Q( 12) | 1 - 0 | 445.42 | -738.94 | 0.00000D+00 | 4.88558D-25 | -1.84902D-01 |
| Q( 12) | 1 - 1 | 1184.36 | 0.00 | 0.00000D+00 | 1.00000D+00 | -1.55992D+00 |
| Q( 13) | 1 - 0 | 459.63 | -738.81 | 0.00000D+00 | 9.09067D-25 | -1.85101D-01 |
| Q( 13) | 1 - 1 | 1198.44 | 0.00 | 0.00000D+00 | 1.00000D+00 | -1.56025D+00 |
| Q( 14) | 1 - 0 | 474.93 | -738.67 | 0.00000D+00 | 1.64529D-24 | -1.85316D-01 |
| Q( 14) | 1 - 1 | 1213.60 | 0.00 | 0.00000D+00 | 1.00000D+00 | -1.56061D+00 |
| Q( 15) | 1 - 0 | 491.32 | -738.52 | 0.00000D+00 | 2.79048D-24 | -1.85546D-01 |
| Q( 15) | 1 - 1 | 1229.84 | 0.00 | 0.00000D+00 | 1.00000D+00 | -1.56099D+00 |
| Q( 16) | 1 - 0 | 508.80 | -738.36 | 0.00000D+00 | 3.23756D-24 | -1.85792D-01 |
| Q( 16) | 1 - 1 | 1247.16 | 0.00 | 0.00000D+00 | 1.00000D+00 | -1.56140D+00 |
| Q( 17) | 1 - 0 | 527.37 | -738.19 | 0.00000D+00 | 5.61664D-24 | -1.86053D-01 |
| Q( 17) | 1 - 1 | 1265.56 | 0.00 | 0.00000D+00 | 1.00000D+00 | -1.56183D+00 |
| Q( 18) | 1 - 0 | 547.03 | -738.01 | 0.00000D+00 | 9.05449D-24 | -1.86329D-01 |
| Q( 18) | 1 - 1 | 1285.04 | 0.00 | 0.00000D+00 | 1.00000D+00 | -1.56229D+00 |
| Q( 19) | 1 - 0 | 567.78 | -737.82 | 0.00000D+00 | 1.46074D-23 | -1.86621D-01 |
| Q( 19) | 1 - 1 | 1305.60 | 0.00 | 0.00000D+00 | 1.00000D+00 | -1.56278D+00 |
| Q( 20) | 1 - 0 | 589.62 | -737.62 | 0.00000D+00 | 2.24334D-23 | -1.86928D-01 |
| Q( 20) | 1 - 1 | 1327.25 | 0.00 | 0.00000D+00 | 1.00000D+00 | -1.56329D+00 |
| Q( 0) | 2 - 0 | 360.13 | -1529.68 | 0.00000D+00 | 2.28982D-29 | -5.56371D-02 |
| Q( 0) | 2 - 1 | 1099.88 | -789.93 | 0.00000D+00 | 2.51547D-20 | -2.77277D-01 |
| Q( 0) | 2 - 2 | 1889.81 | 0.00 | 0.00000D+00 | 1.00000D+00 | -1.64304D+00 |
| Q( 1) | 2 - 0 | 361.22 | -1529.65 | 0.00000D+00 | 5.45389D-20 | -5.56393D-02 |

| | | | | | | |
|---|---|---|---|---|---|---|
| Q( 1) | 2 - 1 | 1100.96 | -789.91 | 0.00000D+00 | 2.38044D-18 | -2.77280D-01 |
| Q( 1) | 2 - 2 | 1890.87 | -0.00 | 0.00000D+00 | 1.00000D+00 | -1.64307D+00 |
| Q( 2) | 2 - 0 | 363.41 | -1529.59 | 0.00000D+00 | 2.65819D-29 | -5.56437D-02 |
| Q( 2) | 2 - 1 | 1103.13 | -789.87 | 0.00000D+00 | 2.51956D-20 | -2.77285D-01 |
| Q( 2) | 2 - 2 | 1893.00 | 0.00 | 0.00000D+00 | 1.00000D+00 | -1.64313D+00 |
| Q( 3) | 2 - 0 | 366.69 | -1529.50 | 0.00000D+00 | 1.63690D-30 | -5.56502D-02 |
| Q( 3) | 2 - 1 | 1106.38 | -789.81 | 0.00000D+00 | 2.52268D-20 | -2.77294D-01 |
| Q( 3) | 2 - 2 | 1896.19 | 0.00 | 0.00000D+00 | 1.00000D+00 | -1.64322D+00 |
| Q( 4) | 2 - 0 | 371.06 | -1529.37 | 0.00000D+00 | 8.15414D-30 | -5.56589D-02 |
| Q( 4) | 2 - 1 | 1110.71 | -789.73 | 0.00000D+00 | 2.52511D-20 | -2.77305D-01 |
| Q( 4) | 2 - 2 | 1900.44 | 0.00 | 0.00000D+00 | 1.00000D+00 | -1.64334D+00 |
| Q( 5) | 2 - 0 | 376.53 | -1529.22 | 0.00000D+00 | 3.06731D-29 | -5.56697D-02 |
| Q( 5) | 2 - 1 | 1116.13 | -789.63 | 0.00000D+00 | 2.52791D-20 | -2.77319D-01 |
| Q( 5) | 2 - 2 | 1905.75 | 0.00 | 0.00000D+00 | 1.00000D+00 | -1.64348D+00 |
| Q( 6) | 2 - 0 | 383.09 | -1529.04 | 0.00000D+00 | 1.59862D-28 | -5.56826D-02 |
| Q( 6) | 2 - 1 | 1122.63 | -789.51 | 0.00000D+00 | 2.53144D-20 | -2.77336D-01 |
| Q( 6) | 2 - 2 | 1912.13 | 0.00 | 0.00000D+00 | 1.00000D+00 | -1.64366D+00 |
| Q( 7) | 2 - 0 | 390.75 | -1528.82 | 0.00000D+00 | 1.45316D-28 | -5.56974D-02 |
| Q( 7) | 2 - 1 | 1130.21 | -789.36 | 0.00000D+00 | 2.53493D-20 | -2.77355D-01 |
| Q( 7) | 2 - 2 | 1919.57 | -0.00 | 0.00000D+00 | 1.00000D+00 | -1.64386D+00 |
| Q( 8) | 2 - 0 | 399.50 | -1528.58 | 0.00000D+00 | 7.50457D-28 | -5.57143D-02 |
| Q( 8) | 2 - 1 | 1138.87 | -789.20 | 0.00000D+00 | 2.53823D-20 | -2.77378D-01 |
| Q( 8) | 2 - 2 | 1928.07 | -0.00 | 0.00000D+00 | 1.00000D+00 | -1.64410D+00 |
| Q( 9) | 2 - 0 | 409.34 | -1528.30 | 0.00000D+00 | 1.11635D-27 | -5.57330D-02 |
| Q( 9) | 2 - 1 | 1148.62 | -789.02 | 0.00000D+00 | 2.54132D-20 | -2.77403D-01 |
| Q( 9) | 2 - 2 | 1937.64 | -0.00 | 0.00000D+00 | 1.00000D+00 | -1.64436D+00 |
| Q( 10) | 2 - 0 | 420.27 | -1527.99 | 0.00000D+00 | 3.50311D-27 | -5.57535D-02 |
| Q( 10) | 2 - 1 | 1159.45 | -788.81 | 0.00000D+00 | 2.54348D-20 | -2.77431D-01 |
| Q( 10) | 2 - 2 | 1948.27 | -0.00 | 0.00000D+00 | 1.00000D+00 | -1.64465D+00 |

| | | | | | | |
|---|---|---|---|---|---|---|
| Q( 11) | 2 - 0 | 432.30 | -1527.66 | 0.00000D+00 | 6.57891D-27 | -5.57758D-02 |
| Q( 11) | 2 - 1 | 1171.37 | -788.59 | 0.00000D+00 | 2.54664D-20 | -2.77462D-01 |
| Q( 11) | 2 - 2 | 1959.96 | -0.00 | 0.00000D+00 | 1.00000D+00 | -1.64498D+00 |
| Q( 12) | 2 - 0 | 445.42 | -1527.29 | 0.00000D+00 | 1.32541D-26 | -5.57996D-02 |
| Q( 12) | 2 - 1 | 1184.36 | -788.35 | 0.00000D+00 | 2.54768D-20 | -2.77496D-01 |
| Q( 12) | 2 - 2 | 1972.71 | -0.00 | 0.00000D+00 | 1.00000D+00 | -1.64533D+00 |
| Q( 13) | 2 - 0 | 459.63 | -1526.90 | 0.00000D+00 | 1.21084D-26 | -5.58250D-02 |
| Q( 13) | 2 - 1 | 1198.44 | -788.08 | 0.00000D+00 | 2.55789D-20 | -2.77533D-01 |
| Q( 13) | 2 - 2 | 1986.52 | -0.00 | 0.00000D+00 | 1.00000D+00 | -1.64571D+00 |
| Q( 14) | 2 - 0 | 474.93 | -1526.47 | 0.00000D+00 | 2.27904D-26 | -5.58519D-02 |
| Q( 14) | 2 - 1 | 1213.60 | -787.80 | 0.00000D+00 | 2.55815D-20 | -2.77573D-01 |
| Q( 14) | 2 - 2 | 2001.39 | -0.00 | 0.00000D+00 | 1.00000D+00 | -1.64612D+00 |
| Q( 15) | 2 - 0 | 491.32 | -1526.01 | 0.00000D+00 | 4.15581D-26 | -5.58800D-02 |
| Q( 15) | 2 - 1 | 1229.84 | -787.49 | 0.00000D+00 | 2.55653D-20 | -2.77616D-01 |
| Q( 15) | 2 - 2 | 2017.33 | -0.00 | 0.00000D+00 | 1.00000D+00 | -1.64656D+00 |
| Q( 16) | 2 - 0 | 508.80 | -1525.53 | 0.00000D+00 | 7.39400D-26 | -5.59092D-02 |
| Q( 16) | 2 - 1 | 1247.16 | -787.17 | 0.00000D+00 | 2.63266D-20 | -2.77663D-01 |
| Q( 16) | 2 - 2 | 2034.33 | -0.00 | 0.00000D+00 | 1.00000D+00 | -1.64702D+00 |
| Q( 17) | 2 - 0 | 527.37 | -1525.01 | 0.00000D+00 | 1.22172D-25 | -5.59395D-02 |
| Q( 17) | 2 - 1 | 1265.56 | -786.82 | 0.00000D+00 | 2.62696D-20 | -2.77712D-01 |
| Q( 17) | 2 - 2 | 2052.38 | -0.00 | 0.00000D+00 | 1.00000D+00 | -1.64752D+00 |
| Q( 18) | 2 - 0 | 547.03 | -1524.46 | 0.00000D+00 | 2.02273D-25 | -5.59707D-02 |
| Q( 18) | 2 - 1 | 1285.04 | -786.46 | 0.00000D+00 | 2.61790D-20 | -2.77764D-01 |
| Q( 18) | 2 - 2 | 2071.50 | -0.00 | 0.00000D+00 | 1.00000D+00 | -1.64805D+00 |
| Q( 19) | 2 - 0 | 567.78 | -1523.89 | 0.00000D+00 | 3.19140D-25 | -5.60025D-02 |
| Q( 19) | 2 - 1 | 1305.60 | -786.07 | 0.00000D+00 | 2.60573D-20 | -2.77820D-01 |
| Q( 19) | 2 - 2 | 2091.67 | -0.00 | 0.00000D+00 | 1.00000D+00 | -1.64860D+00 |
| Q( 20) | 2 - 0 | 589.62 | -1523.29 | 0.00000D+00 | 4.86247D-25 | -5.60350D-02 |
| Q( 20) | 2 - 1 | 1327.25 | -785.66 | 0.00000D+00 | 2.59046D-20 | -2.77879D-01 |

| | | | | | | |
|---|---|---|---|---|---|---|
| Q( 20) | 2 - 2 | 2112.91 | -0.00 | 0.00000D+00 | 1.00000D+00 | -1.64919D+00 |
| Q( 0) | 3 - 0 | 360.13 | -2327.99 | 0.00000D+00 | 6.99559D-26 | 1.19146D-02 |
| Q( 0) | 3 - 1 | 1099.88 | -1588.24 | 0.00000D+00 | 1.88383D-21 | -8.79512D-03 |
| Q( 0) | 3 - 2 | 1889.81 | -798.31 | 0.00000D+00 | 1.27606D-22 | -3.58903D-01 |
| Q( 0) | 3 - 3 | 2688.12 | 0.00 | 0.00000D+00 | 1.00000D+00 | -1.70989D+00 |
| Q( 1) | 3 - 0 | 361.22 | -2327.95 | 0.00000D+00 | 3.05375D-21 | 1.19250D-02 |
| Q( 1) | 3 - 1 | 1100.96 | -1588.21 | 0.00000D+00 | 1.14213D-19 | -8.79876D-03 |
| Q( 1) | 3 - 2 | 1890.87 | -798.30 | 0.00000D+00 | 6.26978D-18 | -3.58908D-01 |
| Q( 1) | 3 - 3 | 2689.17 | -0.00 | 0.00000D+00 | 1.00000D+00 | -1.70993D+00 |
| Q( 2) | 3 - 0 | 363.41 | -2327.87 | 0.00000D+00 | 2.46885D-29 | 1.19456D-02 |
| Q( 2) | 3 - 1 | 1103.13 | -1588.15 | 0.00000D+00 | 2.03817D-21 | -8.80604D-03 |
| Q( 2) | 3 - 2 | 1893.00 | -798.28 | 0.00000D+00 | 9.03247D-26 | -3.58918D-01 |
| Q( 2) | 3 - 3 | 2691.28 | 0.00 | 0.00000D+00 | 1.00000D+00 | -1.71001D+00 |
| Q( 3) | 3 - 0 | 366.69 | -2327.75 | 0.00000D+00 | 4.21816D-30 | 1.19766D-02 |
| Q( 3) | 3 - 1 | 1106.38 | -1588.06 | 0.00000D+00 | 2.03748D-21 | -8.81697D-03 |
| Q( 3) | 3 - 2 | 1896.19 | -798.25 | 0.00000D+00 | 6.72737D-26 | -3.58932D-01 |
| Q( 3) | 3 - 3 | 2694.44 | 0.00 | 0.00000D+00 | 1.00000D+00 | -1.71012D+00 |
| Q( 4) | 3 - 0 | 371.06 | -2327.59 | 0.00000D+00 | 1.06300D-28 | 1.20179D-02 |
| Q( 4) | 3 - 1 | 1110.71 | -1587.95 | 0.00000D+00 | 2.03421D-21 | -8.83156D-03 |
| Q( 4) | 3 - 2 | 1900.44 | -798.22 | 0.00000D+00 | 7.25383D-26 | -3.58951D-01 |
| Q( 4) | 3 - 3 | 2698.66 | 0.00 | 0.00000D+00 | 1.00000D+00 | -1.71028D+00 |
| Q( 5) | 3 - 0 | 376.53 | -2327.39 | 0.00000D+00 | 1.04462D-29 | 1.20695D-02 |
| Q( 5) | 3 - 1 | 1116.13 | -1587.80 | 0.00000D+00 | 2.03155D-21 | -8.84983D-03 |
| Q( 5) | 3 - 2 | 1905.75 | -798.17 | 0.00000D+00 | 5.32862D-26 | -3.58974D-01 |
| Q( 5) | 3 - 3 | 2703.93 | 0.00 | 0.00000D+00 | 1.00000D+00 | -1.71048D+00 |
| Q( 6) | 3 - 0 | 383.09 | -2327.15 | 0.00000D+00 | 9.61820D-31 | 1.21314D-02 |
| Q( 6) | 3 - 1 | 1122.63 | -1587.62 | 0.00000D+00 | 2.02720D-21 | -8.87180D-03 |
| Q( 6) | 3 - 2 | 1912.13 | -798.12 | 0.00000D+00 | 2.51578D-26 | -3.59003D-01 |
| Q( 6) | 3 - 3 | 2710.25 | 0.00 | 0.00000D+00 | 1.00000D+00 | -1.71072D+00 |

| | | | | | | |
|---|---|---|---|---|---|---|
| Q( 7) | 3 - 0 | 390.75 | -2326.88 | 0.00000D+00 | 1.39900D-28 | 1.22035D-02 |
| Q( 7) | 3 - 1 | 1130.21 | -1587.42 | 0.00000D+00 | 2.02231D-21 | -8.89749D-03 |
| Q( 7) | 3 - 2 | 1919.57 | -798.05 | 0.00000D+00 | 5.23505D-27 | -3.59036D-01 |
| Q( 7) | 3 - 3 | 2717.63 | 0.00 | 0.00000D+00 | 1.00000D+00 | -1.71100D+00 |
| Q( 8) | 3 - 0 | 399.50 | -2326.56 | 0.00000D+00 | 8.87805D-29 | 1.22859D-02 |
| Q( 8) | 3 - 1 | 1138.87 | -1587.18 | 0.00000D+00 | 2.01550D-21 | -8.92693D-03 |
| Q( 8) | 3 - 2 | 1928.07 | -797.98 | 0.00000D+00 | 5.61264D-28 | -3.59075D-01 |
| Q( 8) | 3 - 3 | 2726.06 | 0.00 | 0.00000D+00 | 1.00000D+00 | -1.71131D+00 |
| Q( 9) | 3 - 0 | 409.34 | -2326.20 | 0.00000D+00 | 1.03396D-28 | 1.23785D-02 |
| Q( 9) | 3 - 1 | 1148.62 | -1586.92 | 0.00000D+00 | 2.00688D-21 | -8.96015D-03 |
| Q( 9) | 3 - 2 | 1937.64 | -797.90 | 0.00000D+00 | 5.02768D-26 | -3.59118D-01 |
| Q( 9) | 3 - 3 | 2735.54 | 0.00 | 0.00000D+00 | 1.00000D+00 | -1.71167D+00 |
| Q( 10) | 3 - 0 | 420.27 | -2325.80 | 0.00000D+00 | 3.53976D-28 | 1.24813D-02 |
| Q( 10) | 3 - 1 | 1159.45 | -1586.62 | 0.00000D+00 | 1.99749D-21 | -8.99718D-03 |
| Q( 10) | 3 - 2 | 1948.27 | -797.81 | 0.00000D+00 | 2.17960D-25 | -3.59166D-01 |
| Q( 10) | 3 - 3 | 2746.08 | 0.00 | 0.00000D+00 | 1.00000D+00 | -1.71206D+00 |
| Q( 11) | 3 - 0 | 432.30 | -2325.37 | 0.00000D+00 | 5.90567D-28 | 1.25942D-02 |
| Q( 11) | 3 - 1 | 1171.37 | -1586.30 | 0.00000D+00 | 1.98717D-21 | -9.03807D-03 |
| Q( 11) | 3 - 2 | 1959.96 | -797.71 | 0.00000D+00 | 6.39597D-25 | -3.59218D-01 |
| Q( 11) | 3 - 3 | 2757.67 | 0.00 | 0.00000D+00 | 1.00000D+00 | -1.71250D+00 |
| Q( 12) | 3 - 0 | 445.42 | -2324.89 | 0.00000D+00 | 1.33826D-27 | 1.27173D-02 |
| Q( 12) | 3 - 1 | 1184.36 | -1585.95 | 0.00000D+00 | 1.97404D-21 | -9.08286D-03 |
| Q( 12) | 3 - 2 | 1972.71 | -797.60 | 0.00000D+00 | 1.49758D-24 | -3.59276D-01 |
| Q( 12) | 3 - 3 | 2770.31 | 0.00 | 0.00000D+00 | 1.00000D+00 | -1.71297D+00 |
| Q( 13) | 3 - 0 | 459.63 | -2324.37 | 0.00000D+00 | 2.28907D-27 | 1.28504D-02 |
| Q( 13) | 3 - 1 | 1198.44 | -1585.56 | 0.00000D+00 | 1.95753D-21 | -9.13160D-03 |
| Q( 13) | 3 - 2 | 1986.52 | -797.48 | 0.00000D+00 | 3.14595D-24 | -3.59339D-01 |
| Q( 13) | 3 - 3 | 2784.00 | 0.00 | 0.00000D+00 | 1.00000D+00 | -1.71349D+00 |
| Q( 14) | 3 - 0 | 474.93 | -2323.82 | 0.00000D+00 | 3.95068D-27 | 1.29935D-02 |

| | | | | | | | |
|---|---|---|---|---|---|---|---|
| Q( 14) | 3 - 1 | 1213.60 | -1585.15 | 0.00000D+00 | 1.93963D-21 | -9.18433D-03 |
| Q( 14) | 3 - 2 | 2001.39 | -797.35 | 0.00000D+00 | 5.98436D-24 | -3.59407D-01 |
| Q( 14) | 3 - 3 | 2798.75 | 0.00 | 0.00000D+00 | 1.00000D+00 | -1.71404D+00 |
| Q( 15) | 3 - 0 | 491.32 | -2323.22 | 0.00000D+00 | 4.94708D-27 | 1.31466D-02 |
| Q( 15) | 3 - 1 | 1229.84 | -1584.71 | 0.00000D+00 | 1.92764D-21 | -9.24111D-03 |
| Q( 15) | 3 - 2 | 2017.33 | -797.21 | 0.00000D+00 | 6.90823D-24 | -3.59480D-01 |
| Q( 15) | 3 - 3 | 2814.54 | 0.00 | 0.00000D+00 | 1.00000D+00 | -1.71463D+00 |
| Q( 16) | 3 - 0 | 508.80 | -2322.59 | 0.00000D+00 | 7.70153D-27 | 1.33096D-02 |
| Q( 16) | 3 - 1 | 1247.16 | -1584.23 | 0.00000D+00 | 2.14641D-21 | -9.30200D-03 |
| Q( 16) | 3 - 2 | 2034.33 | -797.06 | 0.00000D+00 | 1.28764D-23 | -3.59558D-01 |
| Q( 16) | 3 - 3 | 2831.39 | 0.00 | 0.00000D+00 | 1.00000D+00 | -1.71526D+00 |
| Q( 17) | 3 - 0 | 527.37 | -2321.92 | 0.00000D+00 | 1.37907D-26 | 1.34824D-02 |
| Q( 17) | 3 - 1 | 1265.56 | -1583.73 | 0.00000D+00 | 2.11920D-21 | -9.36706D-03 |
| Q( 17) | 3 - 2 | 2052.38 | -796.91 | 0.00000D+00 | 2.24617D-23 | -3.59641D-01 |
| Q( 17) | 3 - 3 | 2849.29 | 0.00 | 0.00000D+00 | 1.00000D+00 | -1.71593D+00 |
| Q( 18) | 3 - 0 | 547.03 | -2321.20 | 0.00000D+00 | 2.12604D-26 | 1.36650D-02 |
| Q( 18) | 3 - 1 | 1285.04 | -1583.19 | 0.00000D+00 | 2.08836D-21 | -9.43636D-03 |
| Q( 18) | 3 - 2 | 2071.50 | -796.74 | 0.00000D+00 | 3.74068D-23 | -3.59729D-01 |
| Q( 18) | 3 - 3 | 2868.24 | 0.00 | 0.00000D+00 | 1.00000D+00 | -1.71664D+00 |
| Q( 19) | 3 - 0 | 567.78 | -2320.45 | 0.00000D+00 | 3.44120D-26 | 1.38574D-02 |
| Q( 19) | 3 - 1 | 1305.60 | -1582.63 | 0.00000D+00 | 2.05353D-21 | -9.50996D-03 |
| Q( 19) | 3 - 2 | 2091.67 | -796.56 | 0.00000D+00 | 5.98364D-23 | -3.59823D-01 |
| Q( 19) | 3 - 3 | 2888.23 | 0.00 | 0.00000D+00 | 1.00000D+00 | -1.71739D+00 |
| Q( 20) | 3 - 0 | 589.62 | -2319.66 | 0.00000D+00 | 5.09072D-26 | 1.40594D-02 |
| Q( 20) | 3 - 1 | 1327.25 | -1582.04 | 0.00000D+00 | 2.01481D-21 | -9.58794D-03 |
| Q( 20) | 3 - 2 | 2112.91 | -796.37 | 0.00000D+00 | 9.20984D-23 | -3.59922D-01 |
| Q( 20) | 3 - 3 | 2909.28 | 0.00 | 0.00000D+00 | 1.00000D+00 | -1.71818D+00 |
| Q( 0) | 4 - 0 | 360.13 | -3103.24 | 0.00000D+00 | 6.82749D-30 | 3.06857D-02 |
| Q( 0) | 4 - 1 | 1099.88 | -2363.49 | 0.00000D+00 | 4.29999D-22 | 7.74281D-04 |

| | | | | | | |
|---|---|---|---|---|---|---|
| Q( 0) | 4 - 2 | 1889.81 | -1573.56 | 0.00000D+00 | 3.29629D-27 | -2.67483D-03 |
| Q( 0) | 4 - 3 | 2688.12 | -775.25 | 0.00000D+00 | 1.36474D-21 | -4.40555D-01 |
| Q( 0) | 4 - 4 | 3463.37 | 0.00 | 0.00000D+00 | 1.00000D+00 | -1.75365D+00 |
| Q( 1) | 4 - 0 | 361.22 | -3103.19 | 0.00000D+00 | 8.93177D-23 | 3.06787D-02 |
| Q( 1) | 4 - 1 | 1100.96 | -2363.45 | 0.00000D+00 | 8.13339D-21 | 7.77275D-04 |
| Q( 1) | 4 - 2 | 1890.87 | -1573.54 | 0.00000D+00 | 1.77342D-19 | -2.67681D-03 |
| Q( 1) | 4 - 3 | 2689.17 | -775.24 | 0.00000D+00 | 5.50891D-18 | -4.40555D-01 |
| Q( 1) | 4 - 4 | 3464.41 | -0.00 | 0.00000D+00 | 1.00000D+00 | -1.75369D+00 |
| Q( 2) | 4 - 0 | 363.41 | -3103.10 | 0.00000D+00 | 2.23731D-30 | 3.06647D-02 |
| Q( 2) | 4 - 1 | 1103.13 | -2363.38 | 0.00000D+00 | 4.31216D-22 | 7.83265D-04 |
| Q( 2) | 4 - 2 | 1893.00 | -1573.51 | 0.00000D+00 | 1.28413D-26 | -2.68076D-03 |
| Q( 2) | 4 - 3 | 2691.28 | -775.23 | 0.00000D+00 | 1.38860D-21 | -4.40555D-01 |
| Q( 2) | 4 - 4 | 3466.51 | 0.00 | 0.00000D+00 | 1.00000D+00 | -1.75376D+00 |
| Q( 3) | 4 - 0 | 366.69 | -3102.96 | 0.00000D+00 | 8.30022D-33 | 3.06438D-02 |
| Q( 3) | 4 - 1 | 1106.38 | -2363.27 | 0.00000D+00 | 4.32770D-22 | 7.92249D-04 |
| Q( 3) | 4 - 2 | 1896.19 | -1573.46 | 0.00000D+00 | 1.01449D-26 | -2.68667D-03 |
| Q( 3) | 4 - 3 | 2694.44 | -775.21 | 0.00000D+00 | 1.38830D-21 | -4.40556D-01 |
| Q( 3) | 4 - 4 | 3469.65 | 0.00 | 0.00000D+00 | 1.00000D+00 | -1.75387D+00 |
| Q( 4) | 4 - 0 | 371.06 | -3102.77 | 0.00000D+00 | 6.38857D-30 | 3.06158D-02 |
| Q( 4) | 4 - 1 | 1110.71 | -2363.13 | 0.00000D+00 | 4.34644D-22 | 8.04229D-04 |
| Q( 4) | 4 - 2 | 1900.44 | -1573.40 | 0.00000D+00 | 9.90305D-27 | -2.69454D-03 |
| Q( 4) | 4 - 3 | 2698.66 | -775.18 | 0.00000D+00 | 1.38846D-21 | -4.40556D-01 |
| Q( 4) | 4 - 4 | 3473.83 | 0.00 | 0.00000D+00 | 1.00000D+00 | -1.75401D+00 |
| Q( 5) | 4 - 0 | 376.53 | -3102.54 | 0.00000D+00 | 1.09451D-33 | 3.05808D-02 |
| Q( 5) | 4 - 1 | 1116.13 | -2362.94 | 0.00000D+00 | 4.37368D-22 | 8.19207D-04 |
| Q( 5) | 4 - 2 | 1905.75 | -1573.31 | 0.00000D+00 | 8.01221D-27 | -2.70435D-03 |
| Q( 5) | 4 - 3 | 2703.93 | -775.14 | 0.00000D+00 | 1.38825D-21 | -4.40556D-01 |
| Q( 5) | 4 - 4 | 3479.07 | 0.00 | 0.00000D+00 | 1.00000D+00 | -1.75419D+00 |
| Q( 6) | 4 - 0 | 383.09 | -3102.25 | 0.00000D+00 | 1.91750D-30 | 3.05387D-02 |

| | | | | | | | |
|---|---|---|---|---|---|---|---|
| Q( 6) | 4 - 1 | 1122.63 | -2362.72 | 0.00000D+00 | 4.40551D-22 | 8.37185D-04 |
| Q( 6) | 4 - 2 | 1912.13 | -1573.22 | 0.00000D+00 | 5.66053D-27 | -2.71608D-03 |
| Q( 6) | 4 - 3 | 2710.25 | -775.10 | 0.00000D+00 | 1.38589D-21 | -4.40556D-01 |
| Q( 6) | 4 - 4 | 3485.35 | 0.00 | 0.00000D+00 | 1.00000D+00 | -1.75441D+00 |
| Q( 7) | 4 - 0 | 390.75 | -3101.93 | 0.00000D+00 | 1.71282D-29 | 3.04896D-02 |
| Q( 7) | 4 - 1 | 1130.21 | -2362.47 | 0.00000D+00 | 4.44270D-22 | 8.58164D-04 |
| Q( 7) | 4 - 2 | 1919.57 | -1573.10 | 0.00000D+00 | 2.69217D-27 | -2.72971D-03 |
| Q( 7) | 4 - 3 | 2717.63 | -775.05 | 0.00000D+00 | 1.38198D-21 | -4.40556D-01 |
| Q( 7) | 4 - 4 | 3492.68 | 0.00 | 0.00000D+00 | 1.00000D+00 | -1.75466D+00 |
| Q( 8) | 4 - 0 | 399.50 | -3101.55 | 0.00000D+00 | 2.97834D-30 | 3.04333D-02 |
| Q( 8) | 4 - 1 | 1138.87 | -2362.17 | 0.00000D+00 | 4.48524D-22 | 8.82148D-04 |
| Q( 8) | 4 - 2 | 1928.07 | -1572.97 | 0.00000D+00 | 1.33293D-27 | -2.74522D-03 |
| Q( 8) | 4 - 3 | 2726.06 | -774.99 | 0.00000D+00 | 1.37433D-21 | -4.40557D-01 |
| Q( 8) | 4 - 4 | 3501.05 | -0.00 | 0.00000D+00 | 1.00000D+00 | -1.75494D+00 |
| Q( 9) | 4 - 0 | 409.34 | -3101.13 | 0.00000D+00 | 5.11245D-30 | 3.03698D-02 |
| Q( 9) | 4 - 1 | 1148.62 | -2361.84 | 0.00000D+00 | 4.53167D-22 | 9.09139D-04 |
| Q( 9) | 4 - 2 | 1937.64 | -1572.83 | 0.00000D+00 | 2.33606D-27 | -2.76258D-03 |
| Q( 9) | 4 - 3 | 2735.54 | -774.93 | 0.00000D+00 | 1.38422D-21 | -4.40557D-01 |
| Q( 9) | 4 - 4 | 3510.47 | -0.00 | 0.00000D+00 | 1.00000D+00 | -1.75527D+00 |
| Q( 10) | 4 - 0 | 420.27 | -3100.66 | 0.00000D+00 | 6.39806D-30 | 3.02992D-02 |
| Q( 10) | 4 - 1 | 1159.45 | -2361.48 | 0.00000D+00 | 4.58581D-22 | 9.39141D-04 |
| Q( 10) | 4 - 2 | 1948.27 | -1572.66 | 0.00000D+00 | 3.60113D-28 | -2.78175D-03 |
| Q( 10) | 4 - 3 | 2746.08 | -774.86 | 0.00000D+00 | 1.37383D-21 | -4.40557D-01 |
| Q( 10) | 4 - 4 | 3520.93 | -0.00 | 0.00000D+00 | 1.00000D+00 | -1.75563D+00 |
| Q( 11) | 4 - 0 | 432.30 | -3100.14 | 0.00000D+00 | 2.17039D-29 | 3.02213D-02 |
| Q( 11) | 4 - 1 | 1171.37 | -2361.08 | 0.00000D+00 | 4.64732D-22 | 9.72160D-04 |
| Q( 11) | 4 - 2 | 1959.96 | -1572.48 | 0.00000D+00 | 1.97661D-27 | -2.80269D-03 |
| Q( 11) | 4 - 3 | 2757.67 | -774.78 | 0.00000D+00 | 1.36145D-21 | -4.40557D-01 |
| Q( 11) | 4 - 4 | 3532.44 | -0.00 | 0.00000D+00 | 1.00000D+00 | -1.75602D+00 |

| | | | | | | | |
|---|---|---|---|---|---|---|---|
| Q( 12) | 4 - 0 | 445.42 | -3099.58 | 0.00000D+00 | 1.99792D-29 | 3.01361D-02 |
| Q( 12) | 4 - 1 | 1184.36 | -2360.64 | 0.00000D+00 | 4.71719D-22 | 1.00820D-03 |
| Q( 12) | 4 - 2 | 1972.71 | -1572.29 | 0.00000D+00 | 1.12817D-26 | -2.82538D-03 |
| Q( 12) | 4 - 3 | 2770.31 | -774.69 | 0.00000D+00 | 1.33995D-21 | -4.40558D-01 |
| Q( 12) | 4 - 4 | 3545.00 | -0.00 | 0.00000D+00 | 1.00000D+00 | -1.75645D+00 |
| Q( 13) | 4 - 0 | 459.63 | -3098.97 | 0.00000D+00 | 6.19189D-29 | 3.00435D-02 |
| Q( 13) | 4 - 1 | 1198.44 | -2360.16 | 0.00000D+00 | 4.79082D-22 | 1.04726D-03 |
| Q( 13) | 4 - 2 | 1986.52 | -1572.08 | 0.00000D+00 | 3.13503D-26 | -2.84976D-03 |
| Q( 13) | 4 - 3 | 2784.00 | -774.60 | 0.00000D+00 | 1.31369D-21 | -4.40558D-01 |
| Q( 13) | 4 - 4 | 3558.60 | -0.00 | 0.00000D+00 | 1.00000D+00 | -1.75692D+00 |
| Q( 14) | 4 - 0 | 474.93 | -3098.32 | 0.00000D+00 | 7.24474D-29 | 2.99435D-02 |
| Q( 14) | 4 - 1 | 1213.60 | -2359.65 | 0.00000D+00 | 4.87390D-22 | 1.08936D-03 |
| Q( 14) | 4 - 2 | 2001.39 | -1571.85 | 0.00000D+00 | 7.49098D-26 | -2.87580D-03 |
| Q( 14) | 4 - 3 | 2798.75 | -774.50 | 0.00000D+00 | 1.27690D-21 | -4.40558D-01 |
| Q( 14) | 4 - 4 | 3573.24 | -0.00 | 0.00000D+00 | 1.00000D+00 | -1.75743D+00 |
| Q( 15) | 4 - 0 | 491.32 | -3097.62 | 0.00000D+00 | 1.78160D-28 | 2.98361D-02 |
| Q( 15) | 4 - 1 | 1229.84 | -2359.10 | 0.00000D+00 | 4.96322D-22 | 1.13450D-03 |
| Q( 15) | 4 - 2 | 2017.33 | -1571.60 | 0.00000D+00 | 1.60083D-25 | -2.90343D-03 |
| Q( 15) | 4 - 3 | 2814.54 | -774.39 | 0.00000D+00 | 1.26939D-21 | -4.40558D-01 |
| Q( 15) | 4 - 4 | 3588.93 | -0.00 | 0.00000D+00 | 1.00000D+00 | -1.75797D+00 |
| Q( 16) | 4 - 0 | 508.80 | -3096.87 | 0.00000D+00 | 3.16913D-28 | 2.97210D-02 |
| Q( 16) | 4 - 1 | 1247.16 | -2358.51 | 0.00000D+00 | 4.59796D-22 | 1.18269D-03 |
| Q( 16) | 4 - 2 | 2034.33 | -1571.34 | 0.00000D+00 | 3.19165D-25 | -2.93262D-03 |
| Q( 16) | 4 - 3 | 2831.39 | -774.28 | 0.00000D+00 | 1.21305D-21 | -4.40559D-01 |
| Q( 16) | 4 - 4 | 3605.67 | -0.00 | 0.00000D+00 | 1.00000D+00 | -1.75855D+00 |
| Q( 17) | 4 - 0 | 527.37 | -3096.07 | 0.00000D+00 | 4.25002D-28 | 2.95983D-02 |
| Q( 17) | 4 - 1 | 1265.56 | -2357.89 | 0.00000D+00 | 4.70245D-22 | 1.23395D-03 |
| Q( 17) | 4 - 2 | 2052.38 | -1571.06 | 0.00000D+00 | 5.74817D-25 | -2.96329D-03 |
| Q( 17) | 4 - 3 | 2849.29 | -774.16 | 0.00000D+00 | 1.14543D-21 | -4.40559D-01 |

| | | | | | | |
|---|---|---|---|---|---|---|
| Q( 17) | 4 - 4 | 3623.45 | -0.00 | 0.00000D+00 | 1.00000D+00 | -1.75917D+00 |
| Q( 18) | 4 - 0 | 547.03 | -3095.23 | 0.00000D+00 | 7.10043D-28 | 2.94679D-02 |
| Q( 18) | 4 - 1 | 1285.04 | -2357.23 | 0.00000D+00 | 4.81794D-22 | 1.28827D-03 |
| Q( 18) | 4 - 2 | 2071.50 | -1570.77 | 0.00000D+00 | 9.73020D-25 | -2.99541D-03 |
| Q( 18) | 4 - 3 | 2868.24 | -774.03 | 0.00000D+00 | 1.06882D-21 | -4.40559D-01 |
| Q( 18) | 4 - 4 | 3642.27 | -0.00 | 0.00000D+00 | 1.00000D+00 | -1.75982D+00 |
| Q( 19) | 4 - 0 | 567.78 | -3094.35 | 0.00000D+00 | 7.26593D-28 | 2.93297D-02 |
| Q( 19) | 4 - 1 | 1305.60 | -2356.53 | 0.00000D+00 | 4.92969D-22 | 1.34567D-03 |
| Q( 19) | 4 - 2 | 2091.67 | -1570.46 | 0.00000D+00 | 1.14281D-24 | -3.02889D-03 |
| Q( 19) | 4 - 3 | 2888.23 | -773.90 | 0.00000D+00 | 1.04418D-21 | -4.40559D-01 |
| Q( 19) | 4 - 4 | 3662.13 | -0.00 | 0.00000D+00 | 1.00000D+00 | -1.76051D+00 |
| Q( 20) | 4 - 0 | 589.62 | -3093.42 | 0.00000D+00 | 1.16645D-27 | 2.91836D-02 |
| Q( 20) | 4 - 1 | 1327.25 | -2355.79 | 0.00000D+00 | 5.06524D-22 | 1.40617D-03 |
| Q( 20) | 4 - 2 | 2112.91 | -1570.13 | 0.00000D+00 | 1.84540D-24 | -3.06368D-03 |
| Q( 20) | 4 - 3 | 2909.28 | -773.76 | 0.00000D+00 | 9.44792D-22 | -4.40560D-01 |
| Q( 20) | 4 - 4 | 3683.04 | -0.00 | 0.00000D+00 | 1.00000D+00 | -1.76124D+00 |
| Q( 0) | 5 - 0 | 360.13 | -3873.00 | 0.00000D+00 | 3.55409D-29 | -3.05964D-02 |
| Q( 0) | 5 - 1 | 1099.88 | -3133.25 | 0.00000D+00 | 7.92257D-22 | 2.17232D-02 |
| Q( 0) | 5 - 2 | 1889.81 | -2343.31 | 0.00000D+00 | 1.56711D-28 | -4.88326D-03 |
| Q( 0) | 5 - 3 | 2688.12 | -1545.01 | 0.00000D+00 | 2.56721D-22 | 1.73049D-02 |
| Q( 0) | 5 - 4 | 3463.37 | -769.76 | 0.00000D+00 | 7.96835D-25 | -5.07963D-01 |
| Q( 0) | 5 - 5 | 4233.12 | 0.00 | 0.00000D+00 | 1.00000D+00 | -1.83358D+00 |
| Q( 1) | 5 - 0 | 361.22 | -3872.94 | 0.00000D+00 | 3.15125D-24 | -3.05987D-02 |
| Q( 1) | 5 - 1 | 1100.96 | -3133.20 | 0.00000D+00 | 1.79486D-21 | 2.17192D-02 |
| Q( 1) | 5 - 2 | 1890.87 | -2343.29 | 0.00000D+00 | 8.32358D-21 | -4.87690D-03 |
| Q( 1) | 5 - 3 | 2689.17 | -1544.99 | 0.00000D+00 | 2.07705D-19 | 1.73015D-02 |
| Q( 1) | 5 - 4 | 3464.41 | -769.74 | 0.00000D+00 | 5.69860D-18 | -5.07970D-01 |
| Q( 1) | 5 - 5 | 4234.16 | -0.00 | 0.00000D+00 | 1.00000D+00 | -1.83361D+00 |
| Q( 2) | 5 - 0 | 363.41 | -3872.82 | 0.00000D+00 | 1.71025D-29 | -3.06032D-02 |

| | | | | | | | |
|---|---|---|---|---|---|---|---|
| Q( 2) | 5 - 1 | 1103.13 | -3133.10 | 0.00000D+00 | 7.92103D-22 | 2.17111D-02 |
| Q( 2) | 5 - 2 | 1893.00 | -2343.23 | 0.00000D+00 | 1.71653D-28 | -4.86418D-03 |
| Q( 2) | 5 - 3 | 2691.28 | -1544.95 | 0.00000D+00 | 2.56498D-22 | 1.72948D-02 |
| Q( 2) | 5 - 4 | 3466.51 | -769.72 | 0.00000D+00 | 7.52787D-25 | -5.07983D-01 |
| Q( 2) | 5 - 5 | 4236.23 | -0.00 | 0.00000D+00 | 1.00000D+00 | -1.83368D+00 |
| Q( 3) | 5 - 0 | 366.69 | -3872.64 | 0.00000D+00 | 1.05431D-30 | -3.06100D-02 |
| Q( 3) | 5 - 1 | 1106.38 | -3132.96 | 0.00000D+00 | 7.92505D-22 | 2.16990D-02 |
| Q( 3) | 5 - 2 | 1896.19 | -2343.15 | 0.00000D+00 | 1.50190D-28 | -4.84511D-03 |
| Q( 3) | 5 - 3 | 2694.44 | -1544.89 | 0.00000D+00 | 2.56312D-22 | 1.72847D-02 |
| Q( 3) | 5 - 4 | 3469.65 | -769.68 | 0.00000D+00 | 7.51865D-25 | -5.08003D-01 |
| Q( 3) | 5 - 5 | 4239.33 | -0.00 | 0.00000D+00 | 1.00000D+00 | -1.83378D+00 |
| Q( 4) | 5 - 0 | 371.06 | -3872.41 | 0.00000D+00 | 2.35339D-29 | -3.06191D-02 |
| Q( 4) | 5 - 1 | 1110.71 | -3132.76 | 0.00000D+00 | 7.92502D-22 | 2.16829D-02 |
| Q( 4) | 5 - 2 | 1900.44 | -2343.03 | 0.00000D+00 | 2.17242D-28 | -4.81967D-03 |
| Q( 4) | 5 - 3 | 2698.66 | -1544.82 | 0.00000D+00 | 2.56504D-22 | 1.72712D-02 |
| Q( 4) | 5 - 4 | 3473.83 | -769.64 | 0.00000D+00 | 7.54896D-25 | -5.08030D-01 |
| Q( 4) | 5 - 5 | 4243.47 | -0.00 | 0.00000D+00 | 1.00000D+00 | -1.83392D+00 |
| Q( 5) | 5 - 0 | 376.53 | -3872.11 | 0.00000D+00 | 7.19903D-30 | -3.06303D-02 |
| Q( 5) | 5 - 1 | 1116.13 | -3132.52 | 0.00000D+00 | 7.92715D-22 | 2.16628D-02 |
| Q( 5) | 5 - 2 | 1905.75 | -2342.89 | 0.00000D+00 | 2.02419D-28 | -4.78789D-03 |
| Q( 5) | 5 - 3 | 2703.93 | -1544.72 | 0.00000D+00 | 2.56109D-22 | 1.72544D-02 |
| Q( 5) | 5 - 4 | 3479.07 | -769.58 | 0.00000D+00 | 6.86445D-25 | -5.08064D-01 |
| Q( 5) | 5 - 5 | 4248.64 | -0.00 | 0.00000D+00 | 1.00000D+00 | -1.83409D+00 |
| Q( 6) | 5 - 0 | 383.09 | -3871.76 | 0.00000D+00 | 4.67626D-31 | -3.06438D-02 |
| Q( 6) | 5 - 1 | 1122.63 | -3132.23 | 0.00000D+00 | 7.93005D-22 | 2.16387D-02 |
| Q( 6) | 5 - 2 | 1912.13 | -2342.72 | 0.00000D+00 | 2.29663D-28 | -4.74976D-03 |
| Q( 6) | 5 - 3 | 2710.25 | -1544.60 | 0.00000D+00 | 2.55921D-22 | 1.72341D-02 |
| Q( 6) | 5 - 4 | 3485.35 | -769.50 | 0.00000D+00 | 6.39923D-25 | -5.08104D-01 |
| Q( 6) | 5 - 5 | 4254.85 | -0.00 | 0.00000D+00 | 1.00000D+00 | -1.83430D+00 |

| | | | | | | |
|---|---|---|---|---|---|---|
| Q( 7) | 5 - 0 | 390.75 | -3871.35 | 0.00000D+00 | 8.67087D-30 | -3.06594D-02 |
| Q( 7) | 5 - 1 | 1130.21 | -3131.89 | 0.00000D+00 | 7.93340D-22 | 2.16106D-02 |
| Q( 7) | 5 - 2 | 1919.57 | -2342.52 | 0.00000D+00 | 3.99705D-28 | -4.70529D-03 |
| Q( 7) | 5 - 3 | 2717.63 | -1544.47 | 0.00000D+00 | 2.55327D-22 | 1.72104D-02 |
| Q( 7) | 5 - 4 | 3492.68 | -769.42 | 0.00000D+00 | 4.80409D-25 | -5.08151D-01 |
| Q( 7) | 5 - 5 | 4262.10 | -0.00 | 0.00000D+00 | 1.00000D+00 | -1.83454D+00 |
| Q( 8) | 5 - 0 | 399.50 | -3870.88 | 0.00000D+00 | 6.85783D-30 | -3.06771D-02 |
| Q( 8) | 5 - 1 | 1138.87 | -3131.50 | 0.00000D+00 | 7.93325D-22 | 2.15785D-02 |
| Q( 8) | 5 - 2 | 1928.07 | -2342.30 | 0.00000D+00 | 4.60137D-28 | -4.65447D-03 |
| Q( 8) | 5 - 3 | 2726.06 | -1544.32 | 0.00000D+00 | 2.54805D-22 | 1.71834D-02 |
| Q( 8) | 5 - 4 | 3501.05 | -769.33 | 0.00000D+00 | 3.89250D-25 | -5.08205D-01 |
| Q( 8) | 5 - 5 | 4270.37 | -0.00 | 0.00000D+00 | 1.00000D+00 | -1.83481D+00 |
| Q( 9) | 5 - 0 | 409.34 | -3870.35 | 0.00000D+00 | 2.26919D-31 | -3.06969D-02 |
| Q( 9) | 5 - 1 | 1148.62 | -3131.06 | 0.00000D+00 | 7.93508D-22 | 2.15424D-02 |
| Q( 9) | 5 - 2 | 1937.64 | -2342.04 | 0.00000D+00 | 8.20406D-28 | -4.59733D-03 |
| Q( 9) | 5 - 3 | 2735.54 | -1544.14 | 0.00000D+00 | 2.53578D-22 | 1.71528D-02 |
| Q( 9) | 5 - 4 | 3510.47 | -769.22 | 0.00000D+00 | 2.16953D-25 | -5.08265D-01 |
| Q( 9) | 5 - 5 | 4279.68 | -0.00 | 0.00000D+00 | 1.00000D+00 | -1.83512D+00 |
| Q( 10) | 5 - 0 | 420.27 | -3869.76 | 0.00000D+00 | 1.32376D-30 | -3.07188D-02 |
| Q( 10) | 5 - 1 | 1159.45 | -3130.58 | 0.00000D+00 | 7.93762D-22 | 2.15024D-02 |
| Q( 10) | 5 - 2 | 1948.27 | -2341.76 | 0.00000D+00 | 1.60761D-27 | -4.53386D-03 |
| Q( 10) | 5 - 3 | 2746.08 | -1543.95 | 0.00000D+00 | 2.52327D-22 | 1.71189D-02 |
| Q( 10) | 5 - 4 | 3520.93 | -769.10 | 0.00000D+00 | 6.56797D-26 | -5.08332D-01 |
| Q( 10) | 5 - 5 | 4290.03 | -0.00 | 0.00000D+00 | 1.00000D+00 | -1.83546D+00 |
| Q( 11) | 5 - 0 | 432.30 | -3869.11 | 0.00000D+00 | 3.55801D-31 | -3.07426D-02 |
| Q( 11) | 5 - 1 | 1171.37 | -3130.04 | 0.00000D+00 | 7.94172D-22 | 2.14585D-02 |
| Q( 11) | 5 - 2 | 1959.96 | -2341.45 | 0.00000D+00 | 2.36466D-27 | -4.46408D-03 |
| Q( 11) | 5 - 3 | 2757.67 | -1543.74 | 0.00000D+00 | 2.50666D-22 | 1.70814D-02 |
| Q( 11) | 5 - 4 | 3532.44 | -768.97 | 0.00000D+00 | 2.47369D-27 | -5.08406D-01 |

| | | | | | | | |
|---|---|---|---|---|---|---|---|
| Q( 11) | 5 - 5 | 4301.41 | -0.00 | 0.00000D+00 | 1.00000D+00 | -1.83584D+00 |
| Q( 12) | 5 - 0 | 445.42 | -3868.40 | 0.00000D+00 | 1.29294D-31 | -3.07683D-02 |
| Q( 12) | 5 - 1 | 1184.36 | -3129.46 | 0.00000D+00 | 7.94574D-22 | 2.14106D-02 |
| Q( 12) | 5 - 2 | 1972.71 | -2341.11 | 0.00000D+00 | 4.29499D-27 | -4.38800D-03 |
| Q( 12) | 5 - 3 | 2770.31 | -1543.51 | 0.00000D+00 | 2.48031D-22 | 1.70405D-02 |
| Q( 12) | 5 - 4 | 3545.00 | -768.82 | 0.00000D+00 | 1.70024D-25 | -5.08486D-01 |
| Q( 12) | 5 - 5 | 4313.82 | -0.00 | 0.00000D+00 | 1.00000D+00 | -1.83625D+00 |
| Q( 13) | 5 - 0 | 459.63 | -3867.64 | 0.00000D+00 | 8.75876D-33 | -3.07959D-02 |
| Q( 13) | 5 - 1 | 1198.44 | -3128.83 | 0.00000D+00 | 7.94877D-22 | 2.13589D-02 |
| Q( 13) | 5 - 2 | 1986.52 | -2340.74 | 0.00000D+00 | 6.73845D-27 | -4.30563D-03 |
| Q( 13) | 5 - 3 | 2784.00 | -1543.26 | 0.00000D+00 | 2.45378D-22 | 1.69961D-02 |
| Q( 13) | 5 - 4 | 3558.60 | -768.67 | 0.00000D+00 | 8.28637D-25 | -5.08573D-01 |
| Q( 13) | 5 - 5 | 4327.27 | -0.00 | 0.00000D+00 | 1.00000D+00 | -1.83669D+00 |
| Q( 14) | 5 - 0 | 474.93 | -3866.82 | 0.00000D+00 | 1.93701D-30 | -3.08252D-02 |
| Q( 14) | 5 - 1 | 1213.60 | -3128.15 | 0.00000D+00 | 7.95141D-22 | 2.13033D-02 |
| Q( 14) | 5 - 2 | 2001.39 | -2340.35 | 0.00000D+00 | 1.13179D-26 | -4.21697D-03 |
| Q( 14) | 5 - 3 | 2798.75 | -1543.00 | 0.00000D+00 | 2.41493D-22 | 1.69481D-02 |
| Q( 14) | 5 - 4 | 3573.24 | -768.50 | 0.00000D+00 | 2.21265D-24 | -5.08667D-01 |
| Q( 14) | 5 - 5 | 4341.74 | -0.00 | 0.00000D+00 | 1.00000D+00 | -1.83717D+00 |
| Q( 15) | 5 - 0 | 491.32 | -3865.94 | 0.00000D+00 | 6.26395D-30 | -3.08563D-02 |
| Q( 15) | 5 - 1 | 1229.84 | -3127.42 | 0.00000D+00 | 7.95737D-22 | 2.12438D-02 |
| Q( 15) | 5 - 2 | 2017.33 | -2339.92 | 0.00000D+00 | 1.79695D-26 | -4.12205D-03 |
| Q( 15) | 5 - 3 | 2814.54 | -1542.71 | 0.00000D+00 | 2.56458D-22 | 1.68966D-02 |
| Q( 15) | 5 - 4 | 3588.93 | -768.32 | 0.00000D+00 | 5.08088D-24 | -5.08767D-01 |
| Q( 15) | 5 - 5 | 4357.25 | -0.00 | 0.00000D+00 | 1.00000D+00 | -1.83768D+00 |
| Q( 16) | 5 - 0 | 508.80 | -3865.00 | 0.00000D+00 | 4.85646D-31 | -3.08889D-02 |
| Q( 16) | 5 - 1 | 1247.16 | -3126.64 | 0.00000D+00 | 8.50733D-22 | 2.11805D-02 |
| Q( 16) | 5 - 2 | 2034.33 | -2339.47 | 0.00000D+00 | 1.90487D-26 | -4.02088D-03 |
| Q( 16) | 5 - 3 | 2831.39 | -1542.41 | 0.00000D+00 | 2.56081D-22 | 1.68414D-02 |

| | | | | | | |
|---|---|---|---|---|---|---|
| Q( 16) | 5 - 4 | 3605.67 | -768.13 | 0.00000D+00 | 5.34801D-24 | -5.08873D-01 |
| Q( 16) | 5 - 5 | 4373.80 | -0.00 | 0.00000D+00 | 1.00000D+00 | -1.83822D+00 |
| Q( 17) | 5 - 0 | 527.37 | -3864.00 | 0.00000D+00 | 2.96118D-30 | -3.09231D-02 |
| Q( 17) | 5 - 1 | 1265.56 | -3125.81 | 0.00000D+00 | 8.51561D-22 | 2.11135D-02 |
| Q( 17) | 5 - 2 | 2052.38 | -2338.99 | 0.00000D+00 | 3.03952D-26 | -3.91349D-03 |
| Q( 17) | 5 - 3 | 2849.29 | -1542.08 | 0.00000D+00 | 2.49842D-22 | 1.67827D-02 |
| Q( 17) | 5 - 4 | 3623.45 | -767.93 | 0.00000D+00 | 1.08981D-23 | -5.08987D-01 |
| Q( 17) | 5 - 5 | 4391.37 | -0.00 | 0.00000D+00 | 1.00000D+00 | -1.83880D+00 |
| Q( 18) | 5 - 0 | 547.03 | -3862.95 | 0.00000D+00 | 1.52382D-31 | -3.09587D-02 |
| Q( 18) | 5 - 1 | 1285.04 | -3124.94 | 0.00000D+00 | 8.52463D-22 | 2.10427D-02 |
| Q( 18) | 5 - 2 | 2071.50 | -2338.48 | 0.00000D+00 | 4.85051D-26 | -3.79988D-03 |
| Q( 18) | 5 - 3 | 2868.24 | -1541.74 | 0.00000D+00 | 2.42387D-22 | 1.67203D-02 |
| Q( 18) | 5 - 4 | 3642.27 | -767.71 | 0.00000D+00 | 2.00228D-23 | -5.09106D-01 |
| Q( 18) | 5 - 5 | 4409.98 | -0.00 | 0.00000D+00 | 1.00000D+00 | -1.83941D+00 |
| Q( 19) | 5 - 0 | 567.78 | -3861.83 | 0.00000D+00 | 1.83003D-29 | -3.09956D-02 |
| Q( 19) | 5 - 1 | 1305.60 | -3124.01 | 0.00000D+00 | 8.53453D-22 | 2.09681D-02 |
| Q( 19) | 5 - 2 | 2091.67 | -2337.94 | 0.00000D+00 | 7.39130D-26 | -3.68009D-03 |
| Q( 19) | 5 - 3 | 2888.23 | -1541.38 | 0.00000D+00 | 2.33609D-22 | 1.66543D-02 |
| Q( 19) | 5 - 4 | 3662.13 | -767.49 | 0.00000D+00 | 3.43064D-23 | -5.09233D-01 |
| Q( 19) | 5 - 5 | 4429.62 | -0.00 | 0.00000D+00 | 1.00000D+00 | -1.84005D+00 |
| Q( 20) | 5 - 0 | 589.62 | -3860.66 | 0.00000D+00 | 1.79678D-29 | -3.10337D-02 |
| Q( 20) | 5 - 1 | 1327.25 | -3123.04 | 0.00000D+00 | 8.54341D-22 | 2.08899D-02 |
| Q( 20) | 5 - 2 | 2112.91 | -2337.38 | 0.00000D+00 | 1.16610D-25 | -3.55413D-03 |
| Q( 20) | 5 - 3 | 2909.28 | -1541.00 | 0.00000D+00 | 2.23760D-22 | 1.65845D-02 |
| Q( 20) | 5 - 4 | 3683.04 | -767.25 | 0.00000D+00 | 5.57298D-23 | -5.09365D-01 |
| Q( 20) | 5 - 5 | 4450.29 | -0.00 | 0.00000D+00 | 1.00000D+00 | -1.84073D+00 |
