# Supplementary material for: Ab initio spectroscopic studies of AlF and AlCl molecules
Source: arXiv:2303.08681 source file (2023-03-15)
Supplement: Supplementary file 8 [file AlF_triplet_pi_-_S8.pdf]

# AlF $a^3\Pi$: Rotational parameters

Note that (v',J') & (v",J") strictly label the upper and lower levels, resp., and E(lower)=E"

but E(2)-E(1) is: (energy of State-2 level) - (energy of State-1 level)

In the following table, E is expressed in $cm^{-1}$, A in $s^{-1}$ and transition dipole moment in debye.

| dJ(J") | Band v' v" | E(lower) | E(2)-E(1) | A(Einstein) | F-C Factor | <v'j'\|M\|v"j"> |
|---|---|---|---|---|---|---|
| R( 0) | 0 - 0 | 452.43 | -1.08 | 2.03384D-07 | 1.00000D+00 | -1.24135D+00 |
| R( 1) | 0 - 0 | 453.51 | -2.16 | 1.95204D-06 | 1.00000D+00 | -1.24123D+00 |
| R( 2) | 0 - 0 | 455.67 | -3.24 | 7.05614D-06 | 1.00000D+00 | -1.24103D+00 |
| R( 3) | 0 - 0 | 458.91 | -4.32 | 1.73363D-05 | 1.00000D+00 | -1.24075D+00 |
| R( 4) | 0 - 0 | 463.24 | -5.40 | 3.46066D-05 | 1.00000D+00 | -1.24039D+00 |
| R( 5) | 0 - 0 | 468.64 | -6.48 | 6.06714D-05 | 1.00000D+00 | -1.23995D+00 |
| R( 6) | 0 - 0 | 475.12 | -7.56 | 9.73216D-05 | 1.00000D+00 | -1.23943D+00 |
| R( 7) | 0 - 0 | 482.69 | -8.64 | 1.46333D-04 | 1.00000D+00 | -1.23883D+00 |
| R( 8) | 0 - 0 | 491.33 | -9.72 | 2.09461D-04 | 1.00000D+00 | -1.23815D+00 |
| R( 9) | 0 - 0 | 501.06 | -10.80 | 2.88442D-04 | 1.00000D+00 | -1.23739D+00 |
| R( 10) | 0 - 0 | 511.86 | -11.88 | 3.84988D-04 | 1.00000D+00 | -1.23654D+00 |
| R( 11) | 0 - 0 | 523.75 | -12.96 | 5.00784D-04 | 9.99999D-01 | -1.23561D+00 |
| R( 12) | 0 - 0 | 536.71 | -14.04 | 6.37483D-04 | 9.99999D-01 | -1.23460D+00 |
| R( 13) | 0 - 0 | 550.76 | -15.12 | 7.96710D-04 | 9.99999D-01 | -1.23351D+00 |
| R( 14) | 0 - 0 | 565.88 | -16.20 | 9.80052D-04 | 9.99999D-01 | -1.23233D+00 |
| R( 15) | 0 - 0 | 582.08 | -17.28 | 1.18906D-03 | 9.99999D-01 | -1.23107D+00 |
| R( 16) | 0 - 0 | 599.36 | -18.36 | 1.42524D-03 | 9.99999D-01 | -1.22972D+00 |
| R( 17) | 0 - 0 | 617.72 | -19.44 | 1.69006D-03 | 9.99999D-01 | -1.22829D+00 |
| R( 18) | 0 - 0 | 637.15 | -20.51 | 1.98493D-03 | 9.99999D-01 | -1.22677D+00 |

| | | | | | | |
|---|---|---|---|---|---|---|
| R( 19) | 0 - 0 | 657.67 | -21.59 | 2.31123D-03 | 9.99999D-01 | -1.22516D+00 |
| P( 1) | 1 - 0 | 453.51 | -883.22 | 1.08071D+02 | 3.54387D-09 | -7.07214D-01 |
| R( 0) | 1 - 0 | 452.43 | -885.37 | 3.63006D+01 | 3.54425D-09 | -7.07347D-01 |
| P( 2) | 1 - 0 | 455.67 | -882.12 | 7.17996D+01 | 1.41760D-08 | -7.07313D-01 |
| R( 0) | 1 - 1 | 1336.73 | -1.07 | 1.25825D-09 | 1.00000D+00 | 9.96983D-02 |
| R( 1) | 1 - 0 | 453.51 | -886.42 | 4.37445D+01 | 1.41763D-08 | -7.07577D-01 |
| P( 3) | 1 - 0 | 458.91 | -881.01 | 6.44137D+01 | 3.19002D-08 | -7.07521D-01 |
| R( 1) | 1 - 1 | 1337.79 | -2.13 | 1.20266D-08 | 1.00000D+00 | 9.94828D-02 |
| R( 2) | 1 - 0 | 455.67 | -887.45 | 4.70788D+01 | 3.18990D-08 | -7.07917D-01 |
| P( 4) | 1 - 0 | 463.24 | -879.89 | 6.11665D+01 | 5.67181D-08 | -7.07838D-01 |
| R( 2) | 1 - 1 | 1339.93 | -3.20 | 4.31735D-08 | 1.00000D+00 | 9.91236D-02 |
| R( 3) | 1 - 0 | 458.91 | -888.47 | 4.90534D+01 | 5.67153D-08 | -7.08366D-01 |
| P( 5) | 1 - 0 | 468.64 | -878.75 | 5.93080D+01 | 8.86352D-08 | -7.08265D-01 |
| R( 3) | 1 - 1 | 1343.12 | -4.26 | 1.05046D-07 | 1.00000D+00 | 9.86208D-02 |
| R( 4) | 1 - 0 | 463.24 | -889.48 | 5.04183D+01 | 8.86299D-08 | -7.08925D-01 |
| P( 6) | 1 - 0 | 475.12 | -877.59 | 5.80883D+01 | 1.27658D-07 | -7.08802D-01 |
| R( 4) | 1 - 1 | 1347.39 | -5.33 | 2.07072D-07 | 1.00000D+00 | 9.79742D-02 |
| R( 5) | 1 - 0 | 468.64 | -890.47 | 5.14622D+01 | 1.27649D-07 | -7.09594D-01 |
| P( 7) | 1 - 0 | 482.69 | -876.42 | 5.72188D+01 | 1.73794D-07 | -7.09449D-01 |
| R( 5) | 1 - 1 | 1352.72 | -6.39 | 3.57450D-07 | 1.00000D+00 | 9.71840D-02 |
| R( 6) | 1 - 0 | 475.12 | -891.45 | 5.23198D+01 | 1.73779D-07 | -7.10372D-01 |
| P( 8) | 1 - 0 | 491.33 | -875.24 | 5.65648D+01 | 2.27052D-07 | -7.10206D-01 |
| R( 6) | 1 - 1 | 1359.11 | -7.46 | 5.62877D-07 | 9.99999D-01 | 9.62502D-02 |
| R( 7) | 1 - 0 | 482.69 | -892.41 | 5.30626D+01 | 2.27030D-07 | -7.11260D-01 |
| P( 9) | 1 - 0 | 501.06 | -874.04 | 5.60549D+01 | 2.87442D-07 | -7.11073D-01 |
| R( 7) | 1 - 1 | 1366.57 | -8.53 | 8.28290D-07 | 9.99999D-01 | 9.51726D-02 |
| R( 8) | 1 - 0 | 491.33 | -893.35 | 5.37322D+01 | 2.87411D-07 | -7.12258D-01 |
| P( 10) | 1 - 0 | 511.86 | -872.82 | 5.56478D+01 | 3.54976D-07 | -7.12051D-01 |
| R( 8) | 1 - 1 | 1375.10 | -9.59 | 1.15664D-06 | 9.99999D-01 | 9.39514D-02 |

| | | | | | | |
|---|---|---|---|---|---|---|
| R( 9) | 1 - 0 | 501.06 | -894.28 | 5.43541D+01 | 3.54933D-07 | -7.13366D-01 |
| P( 11) | 1 - 0 | 523.75 | -871.59 | 5.53178D+01 | 4.29668D-07 | -7.13138D-01 |
| R( 9) | 1 - 1 | 1384.69 | -10.66 | 1.54872D-06 | 9.99999D-01 | 9.25864D-02 |
| R( 10) | 1 - 0 | 511.86 | -895.20 | 5.49454D+01 | 4.29611D-07 | -7.14584D-01 |
| P( 12) | 1 - 0 | 536.71 | -870.35 | 5.50480D+01 | 5.11532D-07 | -7.14337D-01 |
| R( 10) | 1 - 1 | 1395.34 | -11.72 | 2.00299D-06 | 9.99999D-01 | 9.10778D-02 |
| R( 11) | 1 - 0 | 523.75 | -896.10 | 5.55175D+01 | 5.11458D-07 | -7.15913D-01 |
| P( 13) | 1 - 0 | 550.76 | -869.09 | 5.48272D+01 | 6.00584D-07 | -7.15646D-01 |
| R( 11) | 1 - 1 | 1407.06 | -12.78 | 2.51550D-06 | 9.99998D-01 | 8.94256D-02 |
| R( 12) | 1 - 0 | 536.71 | -896.98 | 5.60787D+01 | 6.00490D-07 | -7.17352D-01 |
| P( 14) | 1 - 0 | 565.88 | -867.82 | 5.46473D+01 | 6.96842D-07 | -7.17067D-01 |
| R( 12) | 1 - 1 | 1419.85 | -13.85 | 3.07981D-06 | 9.99998D-01 | 8.76296D-02 |
| R( 13) | 1 - 0 | 550.76 | -897.85 | 5.66349D+01 | 6.96724D-07 | -7.18901D-01 |
| P( 15) | 1 - 0 | 582.08 | -866.53 | 5.45023D+01 | 8.00324D-07 | -7.18598D-01 |
| R( 13) | 1 - 1 | 1433.69 | -14.91 | 3.68701D-06 | 9.99998D-01 | 8.56899D-02 |
| R( 14) | 1 - 0 | 565.88 | -898.71 | 5.71908D+01 | 8.00178D-07 | -7.20562D-01 |
| P( 16) | 1 - 0 | 599.36 | -865.22 | 5.43879D+01 | 9.11050D-07 | -7.20242D-01 |
| R( 14) | 1 - 1 | 1448.61 | -15.98 | 4.32579D-06 | 9.99997D-01 | 8.36066D-02 |
| R( 15) | 1 - 0 | 582.08 | -899.54 | 5.77498D+01 | 9.10874D-07 | -7.22333D-01 |
| P( 17) | 1 - 0 | 617.72 | -863.91 | 5.43009D+01 | 1.02904D-06 | -7.21997D-01 |
| R( 15) | 1 - 1 | 1464.58 | -17.04 | 4.98253D-06 | 9.99997D-01 | 8.13796D-02 |
| R( 16) | 1 - 0 | 599.36 | -900.37 | 5.83147D+01 | 1.02883D-06 | -7.24215D-01 |
| P( 18) | 1 - 0 | 637.15 | -862.57 | 5.42385D+01 | 1.15433D-06 | -7.23863D-01 |
| R( 16) | 1 - 1 | 1481.62 | -18.10 | 5.64152D-06 | 9.99997D-01 | 7.90090D-02 |
| R( 17) | 1 - 0 | 617.72 | -901.17 | 5.88876D+01 | 1.15407D-06 | -7.26210D-01 |
| P( 19) | 1 - 0 | 657.67 | -861.23 | 5.41988D+01 | 1.28692D-06 | -7.25843D-01 |
| R( 17) | 1 - 1 | 1499.73 | -19.17 | 6.28525D-06 | 9.99996D-01 | 7.64947D-02 |
| R( 18) | 1 - 0 | 637.15 | -901.97 | 5.94706D+01 | 1.28663D-06 | -7.28315D-01 |
| P( 20) | 1 - 0 | 679.26 | -859.86 | 5.41801D+01 | 1.42686D-06 | -7.27935D-01 |

| | | | | | | | |
|---|---|---|---|---|---|---|---|
| R( 18) | 1 - 1 | 1518.89 | -20.23 | 6.89468D-06 | 9.99996D-01 | 7.38368D-02 |
| R( 19) | 1 - 0 | 657.67 | -902.74 | 6.00650D+01 | 1.42652D-06 | -7.30533D-01 |
| P( 21) | 1 - 0 | 701.93 | -858.49 | 5.41811D+01 | 1.57417D-06 | -7.30140D-01 |
| R( 19) | 1 - 1 | 1539.12 | -21.29 | 7.44975D-06 | 9.99996D-01 | 7.10353D-02 |
| P( 1) | 2 - 0 | 453.51 | -1740.60 | 4.76220D+02 | 1.69652D-11 | 5.36605D-01 |
| P( 1) | 2 - 1 | 1337.79 | -856.31 | 3.60663D+02 | 7.54668D-09 | 1.35332D+00 |
| R( 0) | 2 - 0 | 452.43 | -1742.74 | 1.59237D+02 | 1.70120D-11 | 5.36454D-01 |
| P( 2) | 2 - 0 | 455.67 | -1739.50 | 3.16980D+02 | 6.77718D-11 | 5.36692D-01 |
| R( 0) | 2 - 1 | 1336.73 | -858.44 | 1.21133D+02 | 7.54784D-09 | 1.35340D+00 |
| P( 2) | 2 - 1 | 1339.93 | -855.24 | 2.39573D+02 | 3.01867D-08 | 1.35341D+00 |
| R( 0) | 2 - 2 | 2194.11 | -1.06 | 3.51869D-08 | 1.00000D+00 | 5.31055D-01 |
| R( 1) | 2 - 0 | 453.51 | -1743.78 | 1.91381D+02 | 6.81189D-11 | 5.36390D-01 |
| P( 3) | 2 - 0 | 458.91 | -1738.38 | 2.84830D+02 | 1.52334D-10 | 5.36785D-01 |
| R( 1) | 2 - 1 | 1337.79 | -859.50 | 1.45932D+02 | 3.01880D-08 | 1.35356D+00 |
| P( 3) | 2 - 1 | 1343.12 | -854.17 | 2.14859D+02 | 6.79227D-08 | 1.35359D+00 |
| R( 1) | 2 - 2 | 2195.17 | -2.12 | 3.38011D-07 | 1.00000D+00 | 5.31238D-01 |
| R( 2) | 2 - 0 | 455.67 | -1744.80 | 2.05367D+02 | 1.53475D-10 | 5.36332D-01 |
| P( 4) | 2 - 0 | 463.24 | -1737.24 | 2.70834D+02 | 2.70519D-10 | 5.36886D-01 |
| R( 2) | 2 - 1 | 1339.93 | -860.55 | 1.56988D+02 | 6.79208D-08 | 1.35382D+00 |
| P( 4) | 2 - 1 | 1347.39 | -853.08 | 2.03931D+02 | 1.20751D-07 | 1.35385D+00 |
| R( 2) | 2 - 2 | 2197.29 | -3.18 | 1.22361D-06 | 1.00000D+00 | 5.31544D-01 |
| R( 3) | 2 - 0 | 458.91 | -1745.80 | 2.13299D+02 | 2.73225D-10 | 5.36281D-01 |
| P( 5) | 2 - 0 | 468.64 | -1736.07 | 2.62889D+02 | 4.22242D-10 | 5.36993D-01 |
| R( 3) | 2 - 1 | 1343.12 | -861.59 | 1.63478D+02 | 1.20744D-07 | 1.35416D+00 |
| P( 5) | 2 - 1 | 1352.72 | -852.00 | 1.97611D+02 | 1.88672D-07 | 1.35420D+00 |
| R( 3) | 2 - 2 | 2200.47 | -4.24 | 3.01241D-06 | 1.00000D+00 | 5.31973D-01 |
| R( 4) | 2 - 0 | 463.24 | -1746.78 | 2.18479D+02 | 4.27528D-10 | 5.36238D-01 |
| P( 6) | 2 - 0 | 475.12 | -1734.89 | 2.57693D+02 | 6.07416D-10 | 5.37108D-01 |
| R( 4) | 2 - 1 | 1347.39 | -862.63 | 1.67905D+02 | 1.88656D-07 | 1.35458D+00 |

| | | | | | | |
|---|---|---|---|---|---|---|
| P( 6) | 2 - 1 | 1359.11 | -850.91 | 1.93398D+02 | 2.71684D-07 | 1.35463D+00 |
| R( 4) | 2 - 2 | 2204.71 | -5.30 | 6.02913D-06 | 9.99999D-01 | 5.32524D-01 |
| R( 5) | 2 - 0 | 468.64 | -1747.74 | 2.22175D+02 | 6.16551D-10 | 5.36200D-01 |
| P( 7) | 2 - 0 | 482.69 | -1733.69 | 2.53976D+02 | 8.25962D-10 | 5.37230D-01 |
| R( 5) | 2 - 1 | 1352.72 | -863.66 | 1.71230D+02 | 2.71654D-07 | 1.35509D+00 |
| P( 7) | 2 - 1 | 1366.57 | -849.81 | 1.90327D+02 | 3.69785D-07 | 1.35515D+00 |
| R( 5) | 2 - 2 | 2210.02 | -6.36 | 1.06039D-05 | 9.99999D-01 | 5.33197D-01 |
| R( 6) | 2 - 0 | 475.12 | -1748.68 | 2.24981D+02 | 8.40471D-10 | 5.36170D-01 |
| P( 8) | 2 - 0 | 491.33 | -1732.47 | 2.51146D+02 | 1.07781D-09 | 5.37358D-01 |
| R( 6) | 2 - 1 | 1359.11 | -864.69 | 1.73905D+02 | 3.69734D-07 | 1.35568D+00 |
| P( 8) | 2 - 1 | 1375.10 | -848.71 | 1.87950D+02 | 4.82972D-07 | 1.35576D+00 |
| R( 6) | 2 - 2 | 2216.38 | -7.42 | 1.70738D-05 | 9.99999D-01 | 5.33992D-01 |
| R( 7) | 2 - 0 | 482.69 | -1749.60 | 2.27208D+02 | 1.09947D-09 | 5.36145D-01 |
| P( 9) | 2 - 0 | 501.06 | -1731.23 | 2.48889D+02 | 1.36290D-09 | 5.37493D-01 |
| R( 7) | 2 - 1 | 1366.57 | -865.72 | 1.76166D+02 | 4.82895D-07 | 1.35636D+00 |
| P( 9) | 2 - 1 | 1384.69 | -847.60 | 1.86028D+02 | 6.11244D-07 | 1.35645D+00 |
| R( 7) | 2 - 2 | 2223.80 | -8.48 | 2.57840D-05 | 9.99999D-01 | 5.34909D-01 |
| R( 8) | 2 - 0 | 491.33 | -1750.50 | 2.29040D+02 | 1.39376D-09 | 5.36127D-01 |
| P( 10) | 2 - 0 | 511.86 | -1729.97 | 2.47022D+02 | 1.68118D-09 | 5.37634D-01 |
| R( 8) | 2 - 1 | 1375.10 | -866.74 | 1.78152D+02 | 6.11132D-07 | 1.35712D+00 |
| P( 10) | 2 - 1 | 1395.34 | -846.49 | 1.84424D+02 | 7.54596D-07 | 1.35722D+00 |
| R( 8) | 2 - 2 | 2232.29 | -9.54 | 3.70894D-05 | 9.99998D-01 | 5.35948D-01 |
| R( 9) | 2 - 0 | 501.06 | -1751.38 | 2.30588D+02 | 1.72352D-09 | 5.36114D-01 |
| P( 11) | 2 - 0 | 523.75 | -1728.69 | 2.45435D+02 | 2.03260D-09 | 5.37781D-01 |
| R( 9) | 2 - 1 | 1384.69 | -867.75 | 1.79948D+02 | 7.54441D-07 | 1.35797D+00 |
| P( 11) | 2 - 1 | 1407.06 | -845.37 | 1.83052D+02 | 9.13027D-07 | 1.35808D+00 |
| R( 9) | 2 - 2 | 2241.83 | -10.60 | 5.13560D-05 | 9.99998D-01 | 5.37109D-01 |
| R( 10) | 2 - 0 | 511.86 | -1752.23 | 2.31924D+02 | 2.08897D-09 | 5.36107D-01 |
| P( 12) | 2 - 0 | 536.71 | -1727.38 | 2.44051D+02 | 2.41713D-09 | 5.37934D-01 |

| | | | | | | | |
|---|---|---|---|---|---|---|---|
| R( 10) | 2 - 1 | 1395.34 | -868.76 | 1.81609D+02 | 9.12818D-07 | 1.35890D+00 |
| P( 12) | 2 - 1 | 1419.85 | -844.25 | 1.81856D+02 | 1.08653D-06 | 1.35903D+00 |
| R( 10) | 2 - 2 | 2252.43 | -11.66 | 6.89623D-05 | 9.99997D-01 | 5.38391D-01 |
| R( 11) | 2 - 0 | 523.75 | -1753.07 | 2.33100D+02 | 2.49034D-09 | 5.36105D-01 |
| P( 13) | 2 - 0 | 550.76 | -1726.06 | 2.42823D+02 | 2.83473D-09 | 5.38093D-01 |
| R( 11) | 2 - 1 | 1407.06 | -869.76 | 1.83174D+02 | 1.08626D-06 | 1.35992D+00 |
| P( 13) | 2 - 1 | 1433.69 | -843.12 | 1.80798D+02 | 1.27511D-06 | 1.36006D+00 |
| R( 11) | 2 - 2 | 2264.10 | -12.72 | 9.03008D-05 | 9.99997D-01 | 5.39794D-01 |
| R( 12) | 2 - 0 | 536.71 | -1753.89 | 2.34148D+02 | 2.92785D-09 | 5.36108D-01 |
| P( 14) | 2 - 0 | 565.88 | -1724.72 | 2.41714D+02 | 3.28538D-09 | 5.38257D-01 |
| R( 12) | 2 - 1 | 1419.85 | -870.75 | 1.84669D+02 | 1.27476D-06 | 1.36102D+00 |
| P( 14) | 2 - 1 | 1448.61 | -841.99 | 1.79851D+02 | 1.47875D-06 | 1.36117D+00 |
| R( 12) | 2 - 2 | 2276.82 | -13.78 | 1.15780D-04 | 9.99996D-01 | 5.41319D-01 |
| R( 13) | 2 - 0 | 550.76 | -1754.68 | 2.35095D+02 | 3.40173D-09 | 5.36115D-01 |
| P( 15) | 2 - 0 | 582.08 | -1723.36 | 2.40698D+02 | 3.76906D-09 | 5.38426D-01 |
| R( 13) | 2 - 1 | 1433.69 | -871.74 | 1.86113D+02 | 1.47832D-06 | 1.36220D+00 |
| P( 15) | 2 - 1 | 1464.58 | -840.85 | 1.78996D+02 | 1.69746D-06 | 1.36237D+00 |
| R( 13) | 2 - 2 | 2290.60 | -14.84 | 1.45824D-04 | 9.99996D-01 | 5.42964D-01 |
| R( 14) | 2 - 0 | 565.88 | -1755.45 | 2.35958D+02 | 3.91224D-09 | 5.36127D-01 |
| P( 16) | 2 - 0 | 599.36 | -1721.97 | 2.39757D+02 | 4.28576D-09 | 5.38599D-01 |
| R( 14) | 2 - 1 | 1448.61 | -872.73 | 1.87522D+02 | 1.69692D-06 | 1.36346D+00 |
| P( 16) | 2 - 1 | 1481.62 | -839.71 | 1.78217D+02 | 1.93123D-06 | 1.36365D+00 |
| R( 14) | 2 - 2 | 2305.44 | -15.90 | 1.80876D-04 | 9.99995D-01 | 5.44730D-01 |
| R( 15) | 2 - 0 | 582.08 | -1756.21 | 2.36752D+02 | 4.45962D-09 | 5.36142D-01 |
| P( 17) | 2 - 0 | 617.72 | -1720.57 | 2.38875D+02 | 4.83549D-09 | 5.38777D-01 |
| R( 15) | 2 - 1 | 1464.58 | -873.70 | 1.88905D+02 | 1.93057D-06 | 1.36481D+00 |
| P( 17) | 2 - 1 | 1499.73 | -838.56 | 1.77505D+02 | 2.18006D-06 | 1.36501D+00 |
| R( 15) | 2 - 2 | 2321.33 | -16.95 | 2.21402D-04 | 9.99995D-01 | 5.46616D-01 |
| R( 16) | 2 - 0 | 599.36 | -1756.94 | 2.37487D+02 | 5.04414D-09 | 5.36159D-01 |

| | | | | | | | |
|---|---|---|---|---|---|---|---|
| P( 18) | 2 - 0 | 637.15 | -1719.14 | 2.38041D+02 | 5.41823D-09 | 5.38958D-01 |
| R( 16) | 2 - 1 | 1481.62 | -874.67 | 1.90271D+02 | 2.17927D-06 | 1.36624D+00 |
| P( 18) | 2 - 1 | 1518.89 | -837.40 | 1.76849D+02 | 2.44394D-06 | 1.36645D+00 |
| R( 16) | 2 - 2 | 2338.29 | -18.01 | 2.67885D-04 | 9.99994D-01 | 5.48622D-01 |
| R( 17) | 2 - 0 | 617.72 | -1757.65 | 2.38171D+02 | 5.66605D-09 | 5.36180D-01 |
| P( 19) | 2 - 0 | 657.67 | -1717.70 | 2.37247D+02 | 6.03399D-09 | 5.39142D-01 |
| R( 17) | 2 - 1 | 1499.73 | -875.64 | 1.91627D+02 | 2.44300D-06 | 1.36775D+00 |
| P( 19) | 2 - 1 | 1539.12 | -836.24 | 1.76243D+02 | 2.72288D-06 | 1.36798D+00 |
| R( 17) | 2 - 2 | 2356.30 | -19.07 | 3.20834D-04 | 9.99993D-01 | 5.50748D-01 |
| R( 18) | 2 - 0 | 637.15 | -1758.34 | 2.38811D+02 | 6.32564D-09 | 5.36203D-01 |
| P( 20) | 2 - 0 | 679.26 | -1716.23 | 2.36485D+02 | 6.68279D-09 | 5.39329D-01 |
| R( 18) | 2 - 1 | 1518.89 | -876.60 | 1.92978D+02 | 2.72176D-06 | 1.36933D+00 |
| P( 20) | 2 - 1 | 1560.41 | -835.08 | 1.75682D+02 | 3.01686D-06 | 1.36959D+00 |
| R( 18) | 2 - 2 | 2375.37 | -20.12 | 3.80783D-04 | 9.99992D-01 | 5.52993D-01 |
| R( 19) | 2 - 0 | 657.67 | -1759.00 | 2.39411D+02 | 7.02317D-09 | 5.36227D-01 |
| P( 21) | 2 - 0 | 701.93 | -1714.74 | 2.35748D+02 | 7.36464D-09 | 5.39519D-01 |
| R( 19) | 2 - 1 | 1539.12 | -877.55 | 1.94329D+02 | 3.01556D-06 | 1.37100D+00 |
| P( 21) | 2 - 1 | 1582.76 | -833.91 | 1.75162D+02 | 3.32588D-06 | 1.37128D+00 |
| R( 19) | 2 - 2 | 2395.49 | -21.18 | 4.48292D-04 | 9.99992D-01 | 5.55357D-01 |
| P( 1) | 3 - 0 | 453.51 | -2551.22 | 1.75855D+01 | 1.49483D-13 | 5.81104D-02 |
| P( 1) | 3 - 1 | 1337.79 | -1666.94 | 4.98153D+02 | 3.60492D-11 | -5.85599D-01 |
| P( 1) | 3 - 2 | 2195.17 | -809.57 | 4.08148D+02 | 1.33058D-08 | -1.56614D+00 |
| R( 0) | 3 - 0 | 452.43 | -2553.37 | 5.89928D+00 | 1.50291D-13 | 5.82223D-02 |
| P( 2) | 3 - 0 | 455.67 | -2550.12 | 1.17188D+01 | 5.96780D-13 | 5.81359D-02 |
| R( 0) | 3 - 1 | 1336.73 | -1669.07 | 1.66502D+02 | 3.61621D-11 | -5.85274D-01 |
| P( 2) | 3 - 1 | 1339.93 | -1665.87 | 3.31553D+02 | 1.43944D-10 | -5.85679D-01 |
| R( 0) | 3 - 2 | 2194.11 | -811.69 | 1.37121D+02 | 1.33064D-08 | -1.56613D+00 |
| P( 2) | 3 - 2 | 2197.29 | -808.51 | 2.71059D+02 | 5.32201D-08 | -1.56622D+00 |
| R( 0) | 3 - 3 | 3004.73 | -1.06 | 7.84045D-08 | 1.00000D+00 | -7.92342D-01 |

| | | | | | | | |
|---|---|---|---|---|---|---|---|
| R( 1) | 3 - 0 | 453.51 | -2554.41 | 7.12130D+00 | 6.02299D-13 | 5.83597D-02 |
| P( 3) | 3 - 0 | 458.91 | -2549.00 | 1.05620D+01 | 1.34200D-12 | 5.82158D-02 |
| R( 1) | 3 - 1 | 1337.79 | -1670.12 | 2.00014D+02 | 1.44887D-10 | -5.85027D-01 |
| P( 3) | 3 - 1 | 1343.12 | -1664.79 | 2.97845D+02 | 3.23450D-10 | -5.85704D-01 |
| R( 1) | 3 - 2 | 2195.17 | -812.75 | 1.65208D+02 | 5.32189D-08 | -1.56621D+00 |
| P( 3) | 3 - 2 | 2200.47 | -807.45 | 2.43036D+02 | 1.19742D-07 | -1.56635D+00 |
| R( 1) | 3 - 3 | 3005.79 | -2.12 | 7.52864D-07 | 1.00000D+00 | -7.92461D-01 |
| R( 2) | 3 - 0 | 455.67 | -2555.43 | 7.68940D+00 | 1.35966D-12 | 5.85515D-02 |
| P( 4) | 3 - 0 | 463.24 | -2547.86 | 1.00920D+01 | 2.38435D-12 | 5.83501D-02 |
| R( 2) | 3 - 1 | 1339.93 | -1671.17 | 2.14484D+02 | 3.26631D-10 | -5.84726D-01 |
| P( 4) | 3 - 1 | 1347.39 | -1663.71 | 2.83080D+02 | 5.74258D-10 | -5.85673D-01 |
| R( 2) | 3 - 2 | 2197.29 | -813.81 | 1.77732D+02 | 1.19732D-07 | -1.56634D+00 |
| P( 4) | 3 - 2 | 2204.71 | -806.39 | 2.30607D+02 | 2.12857D-07 | -1.56653D+00 |
| R( 2) | 3 - 3 | 3007.92 | -3.18 | 2.72357D-06 | 1.00000D+00 | -7.92659D-01 |
| R( 3) | 3 - 0 | 458.91 | -2556.43 | 8.05083D+00 | 2.42625D-12 | 5.87976D-02 |
| P( 5) | 3 - 0 | 468.64 | -2546.70 | 9.86172D+00 | 3.72501D-12 | 5.85388D-02 |
| R( 3) | 3 - 1 | 1343.12 | -1672.22 | 2.22574D+02 | 5.81854D-10 | -5.84368D-01 |
| P( 5) | 3 - 1 | 1352.72 | -1662.63 | 2.74598D+02 | 8.96184D-10 | -5.85586D-01 |
| R( 3) | 3 - 2 | 2200.47 | -814.87 | 1.85080D+02 | 2.12832D-07 | -1.56652D+00 |
| P( 5) | 3 - 2 | 2210.02 | -805.33 | 2.23387D+02 | 3.32550D-07 | -1.56677D+00 |
| R( 3) | 3 - 3 | 3011.10 | -4.24 | 6.69897D-06 | 9.99999D-01 | -7.92936D-01 |
| R( 4) | 3 - 0 | 463.24 | -2557.41 | 8.32775D+00 | 3.80693D-12 | 5.90980D-02 |
| P( 6) | 3 - 0 | 475.12 | -2545.52 | 9.74945D+00 | 5.36565D-12 | 5.87819D-02 |
| R( 4) | 3 - 1 | 1347.39 | -1673.26 | 2.27735D+02 | 9.11072D-10 | -5.83955D-01 |
| P( 6) | 3 - 1 | 1359.11 | -1661.54 | 2.68945D+02 | 1.28907D-09 | -5.85444D-01 |
| R( 4) | 3 - 2 | 2204.71 | -815.93 | 1.90084D+02 | 3.32503D-07 | -1.56675D+00 |
| P( 6) | 3 - 2 | 2216.38 | -804.27 | 2.18543D+02 | 4.78802D-07 | -1.56706D+00 |
| R( 4) | 3 - 3 | 3015.34 | -5.30 | 1.33915D-05 | 9.99999D-01 | -7.93293D-01 |
| R( 5) | 3 - 0 | 468.64 | -2558.37 | 8.56737D+00 | 5.50742D-12 | 5.94528D-02 |

| | | | | | | | |
|---|---|---|---|---|---|---|---|
| P( 7) | 3 - 0 | 482.69 | -2544.33 | 9.70842D+00 | 7.30876D-12 | 5.90795D-02 |
| R( 5) | 3 - 1 | 1352.72 | -1674.30 | 2.31297D+02 | 1.31484D-09 | -5.83486D-01 |
| P( 7) | 3 - 1 | 1366.57 | -1660.44 | 2.64793D+02 | 1.75279D-09 | -5.85246D-01 |
| R( 5) | 3 - 2 | 2210.02 | -817.00 | 1.93833D+02 | 4.78721D-07 | -1.56703D+00 |
| P( 7) | 3 - 2 | 2223.80 | -803.21 | 2.14984D+02 | 6.51589D-07 | -1.56740D+00 |
| R( 5) | 3 - 3 | 3020.65 | -6.37 | 2.35185D-05 | 9.99999D-01 | -7.93727D-01 |
| R( 6) | 3 - 0 | 475.12 | -2559.32 | 8.79193D+00 | 7.53424D-12 | 5.98621D-02 |
| P( 8) | 3 - 0 | 491.33 | -2543.11 | 9.71694D+00 | 9.55761D-12 | 5.94316D-02 |
| R( 6) | 3 - 1 | 1359.11 | -1675.33 | 2.33878D+02 | 1.79377D-09 | -5.82961D-01 |
| P( 8) | 3 - 1 | 1375.10 | -1659.34 | 2.61524D+02 | 2.28727D-09 | -5.84993D-01 |
| R( 6) | 3 - 2 | 2216.38 | -818.06 | 1.96836D+02 | 6.51460D-07 | -1.56737D+00 |
| P( 8) | 3 - 2 | 2232.29 | -802.15 | 2.12203D+02 | 8.50883D-07 | -1.56780D+00 |
| R( 6) | 3 - 3 | 3027.01 | -7.43 | 3.78032D-05 | 9.99998D-01 | -7.94241D-01 |
| R( 7) | 3 - 0 | 482.69 | -2560.24 | 9.01341D+00 | 9.89481D-12 | 6.03257D-02 |
| P( 9) | 3 - 0 | 501.06 | -2541.87 | 9.76367D+00 | 1.21162D-11 | 5.98383D-02 |
| R( 7) | 3 - 1 | 1366.57 | -1676.36 | 2.35806D+02 | 2.34851D-09 | -5.82380D-01 |
| P( 9) | 3 - 1 | 1384.69 | -1658.24 | 2.58809D+02 | 2.89248D-09 | -5.84683D-01 |
| R( 7) | 3 - 2 | 2223.80 | -819.12 | 1.99363D+02 | 8.50690D-07 | -1.56775D+00 |
| P( 9) | 3 - 2 | 2241.83 | -801.09 | 2.09930D+02 | 1.07665D-06 | -1.56824D+00 |
| R( 7) | 3 - 3 | 3034.44 | -8.49 | 5.69756D-05 | 9.99998D-01 | -7.94832D-01 |
| R( 8) | 3 - 0 | 491.33 | -2561.14 | 9.23898D+00 | 1.25974D-11 | 6.08439D-02 |
| P( 10) | 3 - 0 | 511.86 | -2540.61 | 9.84218D+00 | 1.49895D-11 | 6.02996D-02 |
| R( 8) | 3 - 1 | 1375.10 | -1677.38 | 2.37270D+02 | 2.97974D-09 | -5.81741D-01 |
| P( 10) | 3 - 1 | 1395.34 | -1657.13 | 2.56458D+02 | 3.56844D-09 | -5.84317D-01 |
| R( 8) | 3 - 2 | 2232.29 | -820.18 | 2.01568D+02 | 1.07638D-06 | -1.56819D+00 |
| P( 10) | 3 - 2 | 2252.43 | -800.04 | 2.08008D+02 | 1.32885D-06 | -1.56874D+00 |
| R( 8) | 3 - 3 | 3042.93 | -9.55 | 8.17744D-05 | 9.99997D-01 | -7.95502D-01 |
| R( 9) | 3 - 0 | 501.06 | -2562.02 | 9.47329D+00 | 1.56511D-11 | 6.14166D-02 |
| P( 11) | 3 - 0 | 523.75 | -2539.33 | 9.94864D+00 | 1.81831D-11 | 6.08157D-02 |

| | | | | | | |
|---|---|---|---|---|---|---|
| R( 9) | 3 - 1 | 1384.69 | -1678.39 | 2.38388D+02 | 3.68821D-09 | -5.81046D-01 |
| P( 11) | 3 - 1 | 1407.06 | -1656.02 | 2.54354D+02 | 4.31519D-09 | -5.83895D-01 |
| R( 9) | 3 - 2 | 2241.83 | -821.25 | 2.03549D+02 | 1.32848D-06 | -1.56868D+00 |
| P( 11) | 3 - 2 | 2264.10 | -798.98 | 2.06342D+02 | 1.60745D-06 | -1.56929D+00 |
| R( 9) | 3 - 3 | 3052.47 | -10.61 | 1.12947D-04 | 9.99997D-01 | -7.96249D-01 |
| R( 10) | 3 - 0 | 511.86 | -2562.88 | 9.71960D+00 | 1.90659D-11 | 6.20438D-02 |
| P( 12) | 3 - 0 | 536.71 | -2538.03 | 1.00807D+01 | 2.17033D-11 | 6.13865D-02 |
| R( 10) | 3 - 1 | 1395.34 | -1679.40 | 2.39236D+02 | 4.47469D-09 | -5.80294D-01 |
| P( 12) | 3 - 1 | 1419.85 | -1654.90 | 2.52420D+02 | 5.13283D-09 | -5.83415D-01 |
| R( 10) | 3 - 2 | 2252.43 | -822.31 | 2.05369D+02 | 1.60695D-06 | -1.56921D+00 |
| P( 12) | 3 - 2 | 2276.82 | -797.92 | 2.04868D+02 | 1.91240D-06 | -1.56988D+00 |
| R( 10) | 3 - 3 | 3063.08 | -11.66 | 1.51253D-04 | 9.99996D-01 | -7.97074D-01 |
| R( 11) | 3 - 0 | 523.75 | -2563.72 | 9.98035D+00 | 2.28526D-11 | 6.27257D-02 |
| P( 13) | 3 - 0 | 550.76 | -2536.71 | 1.02370D+01 | 2.55573D-11 | 6.20122D-02 |
| R( 11) | 3 - 1 | 1407.06 | -1680.40 | 2.39866D+02 | 5.34001D-09 | -5.79484D-01 |
| P( 13) | 3 - 1 | 1433.69 | -1653.77 | 2.50604D+02 | 6.02149D-09 | -5.82879D-01 |
| R( 11) | 3 - 2 | 2264.10 | -823.37 | 2.07069D+02 | 1.91174D-06 | -1.56980D+00 |
| P( 13) | 3 - 2 | 2290.60 | -796.87 | 2.03544D+02 | 2.24364D-06 | -1.57053D+00 |
| R( 11) | 3 - 3 | 3074.74 | -12.72 | 1.97461D-04 | 9.99995D-01 | -7.97975D-01 |
| R( 12) | 3 - 0 | 536.71 | -2564.54 | 1.02575D+01 | 2.70231D-11 | 6.34623D-02 |
| P( 14) | 3 - 0 | 565.88 | -2535.37 | 1.04166D+01 | 2.97531D-11 | 6.26928D-02 |
| R( 12) | 3 - 1 | 1419.85 | -1681.40 | 2.40314D+02 | 6.28504D-09 | -5.78617D-01 |
| P( 14) | 3 - 1 | 1448.61 | -1652.64 | 2.48871D+02 | 6.98135D-09 | -5.82285D-01 |
| R( 12) | 3 - 2 | 2276.82 | -824.43 | 2.08681D+02 | 2.24281D-06 | -1.57043D+00 |
| P( 14) | 3 - 2 | 2305.44 | -795.81 | 2.02337D+02 | 2.60113D-06 | -1.57123D+00 |
| R( 12) | 3 - 3 | 3087.47 | -13.78 | 2.52353D-04 | 9.99994D-01 | -7.98953D-01 |
| R( 13) | 3 - 0 | 550.76 | -2565.33 | 1.05526D+01 | 3.15899D-11 | 6.42537D-02 |
| P( 15) | 3 - 0 | 582.08 | -2534.01 | 1.06191D+01 | 3.42994D-11 | 6.34284D-02 |
| R( 13) | 3 - 1 | 1433.69 | -1682.39 | 2.40606D+02 | 7.31069D-09 | -5.77691D-01 |

| | | | | | | | |
|---|---|---|---|---|---|---|---|
| P( 15) | 3 - 1 | 1464.58 | -1651.51 | 2.47192D+02 | 8.01262D-09 | -5.81634D-01 |
| R( 13) | 3 - 2 | 2290.60 | -825.49 | 2.10225D+02 | 2.60009D-06 | -1.57111D+00 |
| P( 15) | 3 - 2 | 2321.33 | -794.76 | 2.01227D+02 | 2.98480D-06 | -1.57197D+00 |
| R( 13) | 3 - 3 | 3101.25 | -14.84 | 3.16728D-04 | 9.99993D-01 | -8.00007D-01 |
| R( 14) | 3 - 0 | 565.88 | -2566.11 | 1.08672D+01 | 3.65665D-11 | 6.50999D-02 |
| P( 16) | 3 - 0 | 599.36 | -2532.63 | 1.08443D+01 | 3.92057D-11 | 6.42191D-02 |
| R( 14) | 3 - 1 | 1448.61 | -1683.38 | 2.40762D+02 | 8.41791D-09 | -5.76706D-01 |
| P( 16) | 3 - 1 | 1481.62 | -1650.36 | 2.45550D+02 | 9.11556D-09 | -5.80925D-01 |
| R( 14) | 3 - 2 | 2305.44 | -826.55 | 2.11719D+02 | 2.98353D-06 | -1.57184D+00 |
| P( 16) | 3 - 2 | 2338.29 | -793.70 | 2.00198D+02 | 3.39460D-06 | -1.57276D+00 |
| R( 14) | 3 - 3 | 3116.09 | -15.90 | 3.91396D-04 | 9.99992D-01 | -8.01136D-01 |
| R( 15) | 3 - 0 | 582.08 | -2566.86 | 1.12026D+01 | 4.19673D-11 | 6.60010D-02 |
| P( 17) | 3 - 0 | 617.72 | -2531.23 | 1.10924D+01 | 4.44820D-11 | 6.50650D-02 |
| R( 15) | 3 - 1 | 1464.58 | -1684.36 | 2.40796D+02 | 9.60771D-09 | -5.75663D-01 |
| P( 17) | 3 - 1 | 1499.73 | -1649.22 | 2.43928D+02 | 1.02905D-08 | -5.80157D-01 |
| R( 15) | 3 - 2 | 2321.33 | -827.61 | 2.13173D+02 | 3.39306D-06 | -1.57262D+00 |
| P( 17) | 3 - 2 | 2356.30 | -792.65 | 1.99235D+02 | 3.83047D-06 | -1.57360D+00 |
| R( 15) | 3 - 3 | 3131.99 | -16.96 | 4.77184D-04 | 9.99991D-01 | -8.02339D-01 |
| R( 16) | 3 - 0 | 599.36 | -2567.60 | 1.15600D+01 | 4.78075D-11 | 6.69571D-02 |
| P( 18) | 3 - 0 | 637.15 | -2529.80 | 1.13635D+01 | 5.01395D-11 | 6.59663D-02 |
| R( 16) | 3 - 1 | 1481.62 | -1685.33 | 2.40719D+02 | 1.08811D-08 | -5.74560D-01 |
| P( 18) | 3 - 1 | 1518.89 | -1648.06 | 2.42315D+02 | 1.15377D-08 | -5.79330D-01 |
| R( 16) | 3 - 2 | 2338.29 | -828.67 | 2.14598D+02 | 3.82861D-06 | -1.57344D+00 |
| P( 18) | 3 - 2 | 2375.37 | -791.59 | 1.98331D+02 | 4.29232D-06 | -1.57449D+00 |
| R( 16) | 3 - 3 | 3148.94 | -18.01 | 5.74937D-04 | 9.99990D-01 | -8.03617D-01 |
| R( 17) | 3 - 0 | 617.72 | -2568.31 | 1.19406D+01 | 5.41034D-11 | 6.79683D-02 |
| P( 19) | 3 - 0 | 657.67 | -2528.36 | 1.16579D+01 | 5.61897D-11 | 6.69229D-02 |
| R( 17) | 3 - 1 | 1499.73 | -1686.30 | 2.40539D+02 | 1.22392D-08 | -5.73396D-01 |
| P( 19) | 3 - 1 | 1539.12 | -1646.90 | 2.40703D+02 | 1.28575D-08 | -5.78444D-01 |

| | | | | | | | |
|---|---|---|---|---|---|---|---|
| R( 17) | 3 - 2 | 2356.30 | -829.73 | 2.16001D+02 | 4.29011D-06 | -1.57430D+00 |
| P( 19) | 3 - 2 | 2395.49 | -790.54 | 1.97476D+02 | 4.78009D-06 | -1.57542D+00 |
| R( 17) | 3 - 3 | 3166.96 | -19.07 | 6.85517D-04 | 9.99989D-01 | -8.04969D-01 |
| R( 18) | 3 - 0 | 637.15 | -2569.00 | 1.23457D+01 | 6.08720D-11 | 6.90346D-02 |
| P( 20) | 3 - 0 | 679.26 | -2526.89 | 1.19761D+01 | 6.26452D-11 | 6.79351D-02 |
| R( 18) | 3 - 1 | 1518.89 | -1687.26 | 2.40264D+02 | 1.36831D-08 | -5.72172D-01 |
| P( 20) | 3 - 1 | 1560.41 | -1645.74 | 2.39085D+02 | 1.42505D-08 | -5.77498D-01 |
| R( 18) | 3 - 2 | 2375.37 | -830.78 | 2.17387D+02 | 4.77750D-06 | -1.57521D+00 |
| P( 20) | 3 - 2 | 2416.67 | -789.48 | 1.96665D+02 | 5.29371D-06 | -1.57640D+00 |
| R( 18) | 3 - 3 | 3186.03 | -20.12 | 8.09806D-04 | 9.99988D-01 | -8.06393D-01 |
| R( 19) | 3 - 0 | 657.67 | -2569.66 | 1.27764D+01 | 6.81313D-11 | 7.01562D-02 |
| P( 21) | 3 - 0 | 701.93 | -2525.40 | 1.23187D+01 | 6.95189D-11 | 6.90029D-02 |
| R( 19) | 3 - 1 | 1539.12 | -1688.21 | 2.39899D+02 | 1.52140D-08 | -5.70887D-01 |
| P( 21) | 3 - 1 | 1582.76 | -1644.57 | 2.37454D+02 | 1.57170D-08 | -5.76492D-01 |
| R( 19) | 3 - 2 | 2395.49 | -831.84 | 2.18761D+02 | 5.29068D-06 | -1.57616D+00 |
| P( 21) | 3 - 2 | 2438.90 | -788.43 | 1.95892D+02 | 5.83309D-06 | -1.57742D+00 |
| R( 19) | 3 - 3 | 3206.15 | -21.18 | 9.48703D-04 | 9.99986D-01 | -8.07890D-01 |
| P( 1) | 4 - 0 | 453.51 | -3322.60 | 3.71504D+02 | 5.21117D-15 | -1.79706D-01 |
| P( 1) | 4 - 1 | 1337.79 | -2438.32 | 2.87251D+02 | 5.47352D-14 | -2.51359D-01 |
| P( 1) | 4 - 2 | 2195.17 | -1580.94 | 3.22216D+02 | 5.92386D-11 | 5.09914D-01 |
| P( 1) | 4 - 3 | 3005.79 | -770.32 | 3.36216D+02 | 2.06422D-08 | 1.53145D+00 |
| R( 0) | 4 - 0 | 452.43 | -3324.75 | 1.24033D+02 | 5.18445D-15 | -1.79676D-01 |
| P( 2) | 4 - 0 | 455.67 | -3321.51 | 2.47478D+02 | 2.08570D-14 | -1.79726D-01 |
| R( 0) | 4 - 1 | 1336.73 | -2440.45 | 9.61281D+01 | 5.54042D-14 | -2.51524D-01 |
| P( 2) | 4 - 1 | 1339.93 | -2437.25 | 1.91290D+02 | 2.17488D-13 | -2.51386D-01 |
| R( 0) | 4 - 2 | 2194.11 | -1583.07 | 1.07634D+02 | 5.95147D-11 | 5.09430D-01 |
| P( 2) | 4 - 2 | 2197.29 | -1579.89 | 2.14456D+02 | 2.36452D-10 | 5.10005D-01 |
| R( 0) | 4 - 3 | 3004.73 | -772.44 | 1.12991D+02 | 2.06435D-08 | 1.53137D+00 |
| P( 2) | 4 - 3 | 3007.92 | -769.26 | 2.23236D+02 | 8.25623D-08 | 1.53150D+00 |

| | | | | | | | |
|---|---|---|---|---|---|---|---|
| R( 0) | 4 - 4 | 3776.11 | -1.06 | 8.06086D-08 | 1.00000D+00 | 7.99500D-01 |
| R( 1) | 4 - 0 | 453.51 | -3325.80 | 1.48963D+02 | 2.07072D-14 | -1.79665D-01 |
| P( 3) | 4 - 0 | 458.91 | -3320.39 | 2.22562D+02 | 4.68244D-14 | -1.79748D-01 |
| R( 1) | 4 - 1 | 1337.79 | -2441.51 | 1.15681D+02 | 2.23233D-13 | -2.51716D-01 |
| P( 3) | 4 - 1 | 1343.12 | -2436.18 | 1.72071D+02 | 4.88321D-13 | -2.51485D-01 |
| R( 1) | 4 - 2 | 2195.17 | -1584.14 | 1.29223D+02 | 2.38531D-10 | 5.09036D-01 |
| P( 3) | 4 - 2 | 2200.47 | -1578.83 | 1.92618D+02 | 5.31104D-10 | 5.09995D-01 |
| R( 1) | 4 - 3 | 3005.79 | -773.51 | 1.36148D+02 | 8.25603D-08 | 1.53135D+00 |
| P( 3) | 4 - 3 | 3011.10 | -768.21 | 2.00102D+02 | 1.85755D-07 | 1.53155D+00 |
| R( 1) | 4 - 4 | 3777.18 | -2.13 | 7.73912D-07 | 1.00000D+00 | 7.99566D-01 |
| R( 2) | 4 - 0 | 455.67 | -3326.83 | 1.59738D+02 | 4.63833D-14 | -1.79658D-01 |
| P( 4) | 4 - 0 | 463.24 | -3319.26 | 2.11807D+02 | 8.30390D-14 | -1.79773D-01 |
| R( 2) | 4 - 1 | 1339.93 | -2442.57 | 1.24367D+02 | 5.07630D-13 | -2.51981D-01 |
| P( 4) | 4 - 1 | 1347.39 | -2435.11 | 1.63887D+02 | 8.66579D-13 | -2.51658D-01 |
| R( 2) | 4 - 2 | 2197.29 | -1585.21 | 1.38465D+02 | 5.37991D-10 | 5.08542D-01 |
| P( 4) | 4 - 2 | 2204.71 | -1577.79 | 1.83000D+02 | 9.42512D-10 | 5.09884D-01 |
| R( 2) | 4 - 3 | 3007.92 | -774.58 | 1.46476D+02 | 1.85736D-07 | 1.53133D+00 |
| P( 4) | 4 - 3 | 3015.34 | -767.16 | 1.89808D+02 | 3.30184D-07 | 1.53162D+00 |
| R( 2) | 4 - 4 | 3779.31 | -3.19 | 2.79903D-06 | 1.00000D+00 | 7.99676D-01 |
| R( 3) | 4 - 0 | 458.91 | -3327.84 | 1.65797D+02 | 8.19950D-14 | -1.79653D-01 |
| P( 5) | 4 - 0 | 468.64 | -3318.12 | 2.05775D+02 | 1.29281D-13 | -1.79802D-01 |
| R( 3) | 4 - 1 | 1343.12 | -2443.63 | 1.29488D+02 | 9.13181D-13 | -2.52319D-01 |
| P( 5) | 4 - 1 | 1352.72 | -2434.04 | 1.59435D+02 | 1.35370D-12 | -2.51904D-01 |
| R( 3) | 4 - 2 | 2200.47 | -1586.29 | 1.43549D+02 | 9.58839D-10 | 5.07946D-01 |
| P( 5) | 4 - 2 | 2210.02 | -1576.74 | 1.77416D+02 | 1.47023D-09 | 5.09673D-01 |
| R( 3) | 4 - 3 | 3011.10 | -775.66 | 1.52531D+02 | 3.30138D-07 | 1.53131D+00 |
| P( 5) | 4 - 3 | 3020.65 | -766.11 | 1.83798D+02 | 5.15816D-07 | 1.53169D+00 |
| R( 3) | 4 - 4 | 3782.50 | -4.26 | 6.88221D-06 | 9.99999D-01 | 7.99829D-01 |
| R( 4) | 4 - 0 | 463.24 | -3328.84 | 1.69713D+02 | 1.27245D-13 | -1.79650D-01 |

| | | | | | | | |
|---|---|---|---|---|---|---|---|
| P( 6) | 4 - 0 | 475.12 | -3316.96 | 2.01891D+02 | 1.85278D-13 | -1.79832D-01 |
| R( 4) | 4 - 1 | 1347.39 | -2444.69 | 1.33035D+02 | 1.44567D-12 | -2.52730D-01 |
| P( 6) | 4 - 1 | 1359.11 | -2432.97 | 1.56725D+02 | 1.95177D-12 | -2.52223D-01 |
| R( 4) | 4 - 2 | 2204.71 | -1587.37 | 1.46708D+02 | 1.50211D-09 | 5.07250D-01 |
| P( 6) | 4 - 2 | 2216.38 | -1575.70 | 1.73632D+02 | 2.11383D-09 | 5.09360D-01 |
| R( 4) | 4 - 3 | 3015.34 | -776.74 | 1.56647D+02 | 5.15726D-07 | 1.53131D+00 |
| P( 6) | 4 - 3 | 3027.01 | -765.07 | 1.79738D+02 | 7.42602D-07 | 1.53176D+00 |
| R( 4) | 4 - 4 | 3786.76 | -5.32 | 1.37518D-05 | 9.99999D-01 | 8.00025D-01 |
| R( 5) | 4 - 0 | 468.64 | -3329.83 | 1.72476D+02 | 1.81768D-13 | -1.79650D-01 |
| P( 7) | 4 - 0 | 482.69 | -3315.78 | 1.99164D+02 | 2.50691D-13 | -1.79866D-01 |
| R( 5) | 4 - 1 | 1352.72 | -2445.75 | 1.35774D+02 | 2.11196D-12 | -2.53213D-01 |
| P( 7) | 4 - 1 | 1366.57 | -2431.89 | 1.54991D+02 | 2.66384D-12 | -2.52614D-01 |
| R( 5) | 4 - 2 | 2210.02 | -1588.45 | 1.48801D+02 | 2.16894D-09 | 5.06452D-01 |
| P( 7) | 4 - 2 | 2223.80 | -1574.66 | 1.70789D+02 | 2.87300D-09 | 5.08946D-01 |
| R( 5) | 4 - 3 | 3020.65 | -777.82 | 1.59722D+02 | 7.42446D-07 | 1.53131D+00 |
| P( 7) | 4 - 3 | 3034.44 | -764.03 | 1.76730D+02 | 1.01048D-06 | 1.53185D+00 |
| R( 5) | 4 - 4 | 3792.08 | -6.39 | 2.41382D-05 | 9.99998D-01 | 8.00265D-01 |
| R( 6) | 4 - 0 | 475.12 | -3330.79 | 1.74549D+02 | 2.45130D-13 | -1.79653D-01 |
| P( 8) | 4 - 0 | 491.33 | -3314.58 | 1.97133D+02 | 3.25111D-13 | -1.79902D-01 |
| R( 6) | 4 - 1 | 1359.11 | -2446.80 | 1.38064D+02 | 2.92005D-12 | -2.53768D-01 |
| P( 8) | 4 - 1 | 1375.10 | -2430.82 | 1.53875D+02 | 3.49393D-12 | -2.53078D-01 |
| R( 6) | 4 - 2 | 2216.38 | -1589.53 | 1.50227D+02 | 2.96052D-09 | 5.05552D-01 |
| P( 8) | 4 - 2 | 2232.29 | -1573.63 | 1.68488D+02 | 3.74747D-09 | 5.08430D-01 |
| R( 6) | 4 - 3 | 3027.01 | -778.90 | 1.62174D+02 | 1.01024D-06 | 1.53131D+00 |
| P( 8) | 4 - 3 | 3042.93 | -762.99 | 1.74356D+02 | 1.31939D-06 | 1.53194D+00 |
| R( 6) | 4 - 4 | 3798.46 | -7.45 | 3.87745D-05 | 9.99997D-01 | 8.00548D-01 |
| R( 7) | 4 - 0 | 482.69 | -3331.74 | 1.76175D+02 | 3.16834D-13 | -1.79657D-01 |
| P( 9) | 4 - 0 | 501.06 | -3313.37 | 1.95552D+02 | 4.08065D-13 | -1.79940D-01 |
| R( 7) | 4 - 1 | 1366.57 | -2447.86 | 1.40094D+02 | 3.87910D-12 | -2.54396D-01 |

| | | | | | | | |
|---|---|---|---|---|---|---|---|
| P( 9) | 4 - 1 | 1384.69 | -2429.74 | 1.53189D+02 | 4.44704D-12 | -2.53615D-01 |
| R( 7) | 4 - 2 | 2223.80 | -1590.62 | 1.51201D+02 | 3.87812D-09 | 5.04550D-01 |
| P( 9) | 4 - 2 | 2241.83 | -1572.60 | 1.66515D+02 | 4.73706D-09 | 5.07813D-01 |
| R( 7) | 4 - 3 | 3034.44 | -779.99 | 1.64225D+02 | 1.31902D-06 | 1.53132D+00 |
| P( 9) | 4 - 3 | 3052.47 | -761.96 | 1.72393D+02 | 1.66924D-06 | 1.53203D+00 |
| R( 7) | 4 - 4 | 3805.91 | -8.51 | 5.83968D-05 | 9.99997D-01 | 8.00873D-01 |
| R( 8) | 4 - 0 | 491.33 | -3332.67 | 1.77495D+02 | 3.96320D-13 | -1.79663D-01 |
| P( 10) | 4 - 0 | 511.86 | -3312.14 | 1.94279D+02 | 4.99018D-13 | -1.79981D-01 |
| R( 8) | 4 - 1 | 1375.10 | -2448.91 | 1.41976D+02 | 4.99946D-12 | -2.55095D-01 |
| P( 10) | 4 - 1 | 1395.34 | -2428.66 | 1.52822D+02 | 5.52913D-12 | -2.54225D-01 |
| R( 8) | 4 - 2 | 2232.29 | -1591.71 | 1.51843D+02 | 4.92311D-09 | 5.03446D-01 |
| P( 10) | 4 - 2 | 2252.43 | -1571.57 | 1.64750D+02 | 5.84167D-09 | 5.07093D-01 |
| R( 8) | 4 - 3 | 3042.93 | -781.08 | 1.66002D+02 | 1.66871D-06 | 1.53134D+00 |
| P( 10) | 4 - 3 | 3063.08 | -760.93 | 1.70714D+02 | 2.05994D-06 | 1.53213D+00 |
| R( 8) | 4 - 4 | 3814.43 | -9.58 | 8.37446D-05 | 9.99996D-01 | 8.01241D-01 |
| R( 9) | 4 - 0 | 501.06 | -3333.58 | 1.78597D+02 | 4.82965D-13 | -1.79671D-01 |
| P( 11) | 4 - 0 | 523.75 | -3310.89 | 1.93226D+02 | 5.97371D-13 | -1.80023D-01 |
| R( 9) | 4 - 1 | 1384.69 | -2449.96 | 1.43776D+02 | 6.29278D-12 | -2.55867D-01 |
| P( 11) | 4 - 1 | 1407.06 | -2427.58 | 1.52707D+02 | 6.74721D-12 | -2.54906D-01 |
| R( 9) | 4 - 2 | 2241.83 | -1592.81 | 1.52229D+02 | 6.09692D-09 | 5.02240D-01 |
| P( 11) | 4 - 2 | 2264.10 | -1570.54 | 1.63115D+02 | 7.06128D-09 | 5.06272D-01 |
| R( 9) | 4 - 3 | 3052.47 | -782.17 | 1.67586D+02 | 2.05922D-06 | 1.53135D+00 |
| P( 11) | 4 - 3 | 3074.74 | -759.90 | 1.69238D+02 | 2.49140D-06 | 1.53224D+00 |
| R( 9) | 4 - 4 | 3824.00 | -10.64 | 1.15561D-04 | 9.99995D-01 | 8.01651D-01 |
| R( 10) | 4 - 0 | 511.86 | -3334.48 | 1.79536D+02 | 5.76092D-13 | -1.79680D-01 |
| P( 12) | 4 - 0 | 536.71 | -3309.63 | 1.92335D+02 | 7.02468D-13 | -1.80066D-01 |
| R( 10) | 4 - 1 | 1395.34 | -2451.00 | 1.45540D+02 | 7.77200D-12 | -2.56710D-01 |
| P( 12) | 4 - 1 | 1419.85 | -2426.50 | 1.52799D+02 | 8.10921D-12 | -2.55660D-01 |
| R( 10) | 4 - 2 | 2252.43 | -1593.91 | 1.52410D+02 | 7.40106D-09 | 5.00931D-01 |

| | | | | | | | |
|---|---|---|---|---|---|---|---|
| P( 12) | 4 - 2 | 2276.82 | -1569.52 | 1.61563D+02 | 8.39592D-09 | 5.05348D-01 |
| R( 10) | 4 - 3 | 3063.08 | -783.27 | 1.69028D+02 | 2.49043D-06 | 1.53138D+00 |
| P( 12) | 4 - 3 | 3087.47 | -758.88 | 1.67914D+02 | 2.96349D-06 | 1.53235D+00 |
| R( 10) | 4 - 4 | 3834.64 | -11.70 | 1.54595D-04 | 9.99994D-01 | 8.02101D-01 |
| R( 11) | 4 - 0 | 523.75 | -3335.36 | 1.80352D+02 | 6.74968D-13 | -1.79690D-01 |
| P( 13) | 4 - 0 | 550.76 | -3308.35 | 1.91567D+02 | 8.13598D-13 | -1.80111D-01 |
| R( 11) | 4 - 1 | 1407.06 | -2452.04 | 1.47300D+02 | 9.45144D-12 | -2.57625D-01 |
| P( 13) | 4 - 1 | 1433.69 | -2425.41 | 1.53070D+02 | 9.62446D-12 | -2.56486D-01 |
| R( 11) | 4 - 2 | 2264.10 | -1595.01 | 1.52418D+02 | 8.83711D-09 | 4.99519D-01 |
| P( 13) | 4 - 2 | 2290.60 | -1568.51 | 1.60059D+02 | 9.84573D-09 | 5.04321D-01 |
| R( 11) | 4 - 3 | 3074.74 | -784.36 | 1.70363D+02 | 2.96223D-06 | 1.53140D+00 |
| P( 13) | 4 - 3 | 3101.25 | -757.86 | 1.66705D+02 | 3.47610D-06 | 1.53247D+00 |
| R( 11) | 4 - 4 | 3846.34 | -12.76 | 2.01597D-04 | 9.99993D-01 | 8.02593D-01 |
| R( 12) | 4 - 0 | 536.71 | -3336.22 | 1.81070D+02 | 7.78810D-13 | -1.79701D-01 |
| P( 14) | 4 - 0 | 565.88 | -3307.05 | 1.90894D+02 | 9.29999D-13 | -1.80157D-01 |
| R( 12) | 4 - 1 | 1419.85 | -2453.08 | 1.49077D+02 | 1.13470D-11 | -2.58610D-01 |
| P( 14) | 4 - 1 | 1448.61 | -2424.32 | 1.53497D+02 | 1.13031D-11 | -2.57384D-01 |
| R( 12) | 4 - 2 | 2276.82 | -1596.11 | 1.52278D+02 | 1.04068D-08 | 4.98003D-01 |
| P( 14) | 4 - 2 | 2305.44 | -1567.49 | 1.58580D+02 | 1.14109D-08 | 5.03191D-01 |
| R( 12) | 4 - 3 | 3087.47 | -785.46 | 1.71616D+02 | 3.47450D-06 | 1.53143D+00 |
| P( 14) | 4 - 3 | 3116.09 | -756.84 | 1.65588D+02 | 4.02910D-06 | 1.53258D+00 |
| R( 12) | 4 - 4 | 3859.11 | -13.82 | 2.57327D-04 | 9.99991D-01 | 8.03125D-01 |
| R( 13) | 4 - 0 | 550.76 | -3337.06 | 1.81710D+02 | 8.86789D-13 | -1.79712D-01 |
| P( 15) | 4 - 0 | 582.08 | -3305.74 | 1.90295D+02 | 1.05086D-12 | -1.80204D-01 |
| R( 13) | 4 - 1 | 1433.69 | -2454.12 | 1.50887D+02 | 1.34757D-11 | -2.59667D-01 |
| P( 15) | 4 - 1 | 1464.58 | -2423.23 | 1.54067D+02 | 1.31564D-11 | -2.58353D-01 |
| R( 13) | 4 - 2 | 2290.60 | -1597.22 | 1.52005D+02 | 1.21117D-08 | 4.96383D-01 |
| P( 15) | 4 - 2 | 2321.33 | -1566.48 | 1.57111D+02 | 1.30917D-08 | 5.01957D-01 |
| R( 13) | 4 - 3 | 3101.25 | -786.57 | 1.72803D+02 | 4.02710D-06 | 1.53146D+00 |

| | | | | | | |
|---|---|---|---|---|---|---|
| P( 15) | 4 - 3 | 3131.99 | -755.83 | 1.64544D+02 | 4.62234D-06 | 1.53271D+00 |
| R( 13) | 4 - 4 | 3872.93 | -14.89 | 3.22546D-04 | 9.99990D-01 | 8.03696D-01 |
| R( 14) | 4 - 0 | 565.88 | -3337.88 | 1.82286D+02 | 9.98031D-13 | -1.79723D-01 |
| P( 16) | 4 - 0 | 599.36 | -3304.40 | 1.89754D+02 | 1.17532D-12 | -1.80250D-01 |
| R( 14) | 4 - 1 | 1448.61 | -2455.15 | 1.52743D+02 | 1.58565D-11 | -2.60794D-01 |
| P( 16) | 4 - 1 | 1481.62 | -2422.14 | 1.54766D+02 | 1.51970D-11 | -2.59394D-01 |
| R( 14) | 4 - 2 | 2305.44 | -1598.32 | 1.51614D+02 | 1.39538D-08 | 4.94659D-01 |
| P( 16) | 4 - 2 | 2338.29 | -1565.47 | 1.55637D+02 | 1.48884D-08 | 5.00619D-01 |
| R( 14) | 4 - 3 | 3116.09 | -787.67 | 1.73940D+02 | 4.61989D-06 | 1.53149D+00 |
| P( 16) | 4 - 3 | 3148.94 | -754.82 | 1.63559D+02 | 5.25569D-06 | 1.53283D+00 |
| R( 14) | 4 - 4 | 3887.82 | -15.95 | 3.98024D-04 | 9.99988D-01 | 8.04307D-01 |
| R( 15) | 4 - 0 | 582.08 | -3338.69 | 1.82807D+02 | 1.11163D-12 | -1.79733D-01 |
| P( 17) | 4 - 0 | 617.72 | -3303.05 | 1.89259D+02 | 1.30250D-12 | -1.80297D-01 |
| R( 15) | 4 - 1 | 1464.58 | -2456.18 | 1.54655D+02 | 1.85100D-11 | -2.61991D-01 |
| P( 17) | 4 - 1 | 1499.73 | -2421.04 | 1.55588D+02 | 1.74387D-11 | -2.60506D-01 |
| R( 15) | 4 - 2 | 2321.33 | -1599.43 | 1.51113D+02 | 1.59350D-08 | 4.92830D-01 |
| P( 17) | 4 - 2 | 2356.30 | -1564.47 | 1.54151D+02 | 1.68016D-08 | 4.99176D-01 |
| R( 15) | 4 - 3 | 3131.99 | -788.78 | 1.75034D+02 | 5.25270D-06 | 1.53152D+00 |
| P( 17) | 4 - 3 | 3166.96 | -753.81 | 1.62623D+02 | 5.92897D-06 | 1.53296D+00 |
| R( 15) | 4 - 4 | 3903.76 | -17.01 | 4.84536D-04 | 9.99987D-01 | 8.04956D-01 |
| R( 16) | 4 - 0 | 599.36 | -3339.47 | 1.83281D+02 | 1.22663D-12 | -1.79742D-01 |
| P( 18) | 4 - 0 | 637.15 | -3301.68 | 1.88802D+02 | 1.43145D-12 | -1.80342D-01 |
| R( 16) | 4 - 1 | 1481.62 | -2457.21 | 1.56629D+02 | 2.14583D-11 | -2.63258D-01 |
| P( 18) | 4 - 1 | 1518.89 | -2419.94 | 1.56526D+02 | 1.98964D-11 | -2.61688D-01 |
| R( 16) | 4 - 2 | 2338.29 | -1600.54 | 1.50510D+02 | 1.80572D-08 | 4.90895D-01 |
| P( 18) | 4 - 2 | 2375.37 | -1563.47 | 1.52645D+02 | 1.88316D-08 | 4.97629D-01 |
| R( 16) | 4 - 3 | 3148.94 | -789.89 | 1.76094D+02 | 5.92539D-06 | 1.53156D+00 |
| P( 18) | 4 - 3 | 3186.03 | -752.81 | 1.61729D+02 | 6.64203D-06 | 1.53308D+00 |
| R( 16) | 4 - 4 | 3920.77 | -18.06 | 5.82861D-04 | 9.99985D-01 | 8.05642D-01 |

| | | | | | | |
|---|---|---|---|---|---|---|
| R( 17) | 4 - 0 | 617.72 | -3340.24 | 1.83714D+02 | 1.34208D-12 | -1.79750D-01 |
| P( 19) | 4 - 0 | 657.67 | -3300.29 | 1.88373D+02 | 1.56122D-12 | -1.80387D-01 |
| R( 17) | 4 - 1 | 1499.73 | -2458.23 | 1.58672D+02 | 2.47255D-11 | -2.64594D-01 |
| P( 19) | 4 - 1 | 1539.12 | -2418.83 | 1.57575D+02 | 2.25867D-11 | -2.62941D-01 |
| R( 17) | 4 - 2 | 2356.30 | -1601.66 | 1.49810D+02 | 2.03224D-08 | 4.88854D-01 |
| P( 19) | 4 - 2 | 2395.49 | -1562.47 | 1.51114D+02 | 2.09790D-08 | 4.95975D-01 |
| R( 17) | 4 - 3 | 3166.96 | -791.00 | 1.77126D+02 | 6.63777D-06 | 1.53158D+00 |
| P( 19) | 4 - 3 | 3206.15 | -751.80 | 1.60868D+02 | 7.39469D-06 | 1.53321D+00 |
| R( 17) | 4 - 4 | 3938.83 | -19.12 | 6.93789D-04 | 9.99983D-01 | 8.06365D-01 |
| R( 18) | 4 - 0 | 637.15 | -3340.98 | 1.84111D+02 | 1.45698D-12 | -1.79756D-01 |
| P( 20) | 4 - 0 | 679.26 | -3298.88 | 1.87968D+02 | 1.69083D-12 | -1.80430D-01 |
| R( 18) | 4 - 1 | 1518.89 | -2459.24 | 1.60790D+02 | 2.83375D-11 | -2.66000D-01 |
| P( 20) | 4 - 1 | 1560.41 | -2417.72 | 1.58732D+02 | 2.55273D-11 | -2.64264D-01 |
| R( 18) | 4 - 2 | 2375.37 | -1602.77 | 1.49019D+02 | 2.27327D-08 | 4.86707D-01 |
| P( 20) | 4 - 2 | 2416.67 | -1561.47 | 1.49554D+02 | 2.32445D-08 | 4.94215D-01 |
| R( 18) | 4 - 3 | 3186.03 | -792.11 | 1.78133D+02 | 7.38968D-06 | 1.53161D+00 |
| P( 20) | 4 - 3 | 3227.33 | -750.81 | 1.60038D+02 | 8.18677D-06 | 1.53333D+00 |
| R( 18) | 4 - 4 | 3957.95 | -20.18 | 8.18111D-04 | 9.99982D-01 | 8.07123D-01 |
| R( 19) | 4 - 0 | 657.67 | -3341.71 | 1.84473D+02 | 1.57032D-12 | -1.79759D-01 |
| P( 21) | 4 - 0 | 701.93 | -3297.45 | 1.87580D+02 | 1.81926D-12 | -1.80471D-01 |
| R( 19) | 4 - 1 | 1539.12 | -2460.25 | 1.62987D+02 | 3.23223D-11 | -2.67474D-01 |
| P( 21) | 4 - 1 | 1582.76 | -2416.61 | 1.59992D+02 | 2.87373D-11 | -2.65657D-01 |
| R( 19) | 4 - 2 | 2395.49 | -1603.88 | 1.48139D+02 | 2.52904D-08 | 4.84452D-01 |
| P( 21) | 4 - 2 | 2438.90 | -1560.47 | 1.47962D+02 | 2.56286D-08 | 4.92349D-01 |
| R( 19) | 4 - 3 | 3206.15 | -793.22 | 1.79120D+02 | 8.18092D-06 | 1.53163D+00 |
| P( 21) | 4 - 3 | 3249.56 | -749.81 | 1.59233D+02 | 9.01808D-06 | 1.53345D+00 |
| R( 19) | 4 - 4 | 3978.14 | -21.24 | 9.56629D-04 | 9.99980D-01 | 8.07916D-01 |
| P( 1) | 5 - 0 | 453.51 | -4053.07 | 2.63499D+00 | 4.64656D-15 | -1.12334D-02 |
| P( 1) | 5 - 1 | 1337.79 | -3168.78 | 6.55629D+02 | 4.27065D-14 | 2.56324D-01 |

| | | | | | | | |
|---|---|---|---|---|---|---|---|
| P( 1) | 5 - 2 | 2195.17 | -2311.41 | 7.08010D+02 | 3.80057D-16 | 4.27566D-01 |
| P( 1) | 5 - 3 | 3005.79 | -1500.78 | 1.29610D+02 | 8.84547D-11 | -3.49655D-01 |
| P( 1) | 5 - 4 | 3777.18 | -729.40 | 2.27643D+02 | 3.07154D-08 | -1.36765D+00 |
| R( 0) | 5 - 0 | 452.43 | -4055.22 | 8.89212D-01 | 4.64644D-15 | -1.12938D-02 |
| P( 2) | 5 - 0 | 455.67 | -4051.98 | 1.76166D+00 | 1.85838D-14 | -1.12539D-02 |
| R( 0) | 5 - 1 | 1336.73 | -3170.92 | 2.18820D+02 | 4.22370D-14 | 2.56226D-01 |
| P( 2) | 5 - 1 | 1339.93 | -3167.73 | 4.36721D+02 | 1.70507D-13 | 2.56345D-01 |
| R( 0) | 5 - 2 | 2194.11 | -2313.55 | 2.36880D+02 | 5.04406D-16 | 4.27766D-01 |
| P( 2) | 5 - 2 | 2197.29 | -2310.36 | 4.71460D+02 | 1.36094D-15 | 4.27609D-01 |
| R( 0) | 5 - 3 | 3004.73 | -1502.92 | 4.32354D+01 | 8.89518D-11 | -3.49041D-01 |
| P( 2) | 5 - 3 | 3007.92 | -1499.74 | 8.62740D+01 | 3.52887D-10 | -3.49754D-01 |
| R( 0) | 5 - 4 | 3776.11 | -731.54 | 7.65366D+01 | 3.07176D-08 | -1.36753D+00 |
| P( 2) | 5 - 4 | 3779.31 | -728.35 | 1.51111D+02 | 1.22847D-07 | -1.36768D+00 |
| R( 0) | 5 - 5 | 4506.58 | -1.07 | 5.71475D-08 | 1.00000D+00 | -6.64354D-01 |
| R( 1) | 5 - 0 | 453.51 | -4056.29 | 1.08324D+00 | 1.85998D-14 | -1.13747D-02 |
| P( 3) | 5 - 0 | 458.91 | -4050.89 | 1.59953D+00 | 4.17846D-14 | -1.13082D-02 |
| R( 1) | 5 - 1 | 1337.79 | -3172.01 | 2.62697D+02 | 1.69275D-13 | 2.56150D-01 |
| P( 3) | 5 - 1 | 1343.12 | -3166.68 | 3.92669D+02 | 3.83000D-13 | 2.56348D-01 |
| R( 1) | 5 - 2 | 2195.17 | -2314.63 | 2.84980D+02 | 2.24778D-15 | 4.28009D-01 |
| P( 3) | 5 - 2 | 2200.47 | -2309.33 | 4.24019D+02 | 2.92635D-15 | 4.27747D-01 |
| R( 1) | 5 - 3 | 3005.79 | -1504.01 | 5.18414D+01 | 3.56733D-10 | -3.48524D-01 |
| P( 3) | 5 - 3 | 3011.10 | -1498.70 | 7.74677D+01 | 7.92289D-10 | -3.49713D-01 |
| R( 1) | 5 - 4 | 3777.18 | -732.62 | 9.22394D+01 | 1.22843D-07 | -1.36743D+00 |
| P( 3) | 5 - 4 | 3782.50 | -727.30 | 1.35415D+02 | 2.76370D-07 | -1.36768D+00 |
| R( 1) | 5 - 5 | 4507.65 | -2.15 | 5.48585D-07 | 1.00000D+00 | -6.64366D-01 |
| R( 2) | 5 - 0 | 455.67 | -4057.35 | 1.18506D+00 | 4.18558D-14 | -1.14893D-02 |
| P( 4) | 5 - 0 | 463.24 | -4049.79 | 1.54593D+00 | 7.42485D-14 | -1.13963D-02 |
| R( 2) | 5 - 1 | 1339.93 | -3173.10 | 2.81544D+02 | 3.80526D-13 | 2.56056D-01 |
| P( 4) | 5 - 1 | 1347.39 | -3165.64 | 3.73558D+02 | 6.80032D-13 | 2.56334D-01 |

| | | | | | | |
|---|---|---|---|---|---|---|
| R( 2) | 5 - 2 | 2197.29 | -2315.73 | 3.06256D+02 | 5.90641D-15 | 4.28348D-01 |
| P( 4) | 5 - 2 | 2204.71 | -2308.31 | 4.03733D+02 | 4.99782D-15 | 4.27981D-01 |
| R( 2) | 5 - 3 | 3007.92 | -1505.11 | 5.54570D+01 | 8.05110D-10 | -3.47869D-01 |
| P( 4) | 5 - 3 | 3015.34 | -1497.68 | 7.35519D+01 | 1.40547D-09 | -3.49532D-01 |
| R( 2) | 5 - 4 | 3779.31 | -733.72 | 9.92532D+01 | 2.76338D-07 | -1.36731D+00 |
| P( 4) | 5 - 4 | 3786.76 | -726.26 | 1.28413D+02 | 4.91203D-07 | -1.36767D+00 |
| R( 2) | 5 - 5 | 4509.80 | -3.22 | 1.98362D-06 | 9.99999D-01 | -6.64387D-01 |
| R( 3) | 5 - 0 | 458.91 | -4058.40 | 1.26189D+00 | 7.44170D-14 | -1.16377D-02 |
| P( 5) | 5 - 0 | 468.64 | -4048.68 | 1.53405D+00 | 1.15952D-13 | -1.15182D-02 |
| R( 3) | 5 - 1 | 1343.12 | -3174.19 | 2.92017D+02 | 6.75339D-13 | 2.55944D-01 |
| P( 5) | 5 - 1 | 1352.72 | -3164.60 | 3.62732D+02 | 1.06092D-12 | 2.56301D-01 |
| R( 3) | 5 - 2 | 2200.47 | -2316.85 | 3.18701D+02 | 1.23558D-14 | 4.28781D-01 |
| P( 5) | 5 - 2 | 2210.02 | -2307.30 | 3.92608D+02 | 7.72077D-15 | 4.28310D-01 |
| R( 3) | 5 - 3 | 3011.10 | -1506.22 | 5.73754D+01 | 1.43590D-09 | -3.47073D-01 |
| P( 5) | 5 - 3 | 3020.65 | -1496.67 | 7.12338D+01 | 2.19163D-09 | -3.49212D-01 |
| R( 3) | 5 - 4 | 3782.50 | -734.82 | 1.03372D+02 | 4.91126D-07 | -1.36717D+00 |
| P( 5) | 5 - 4 | 3792.08 | -725.24 | 1.24309D+02 | 7.67258D-07 | -1.36762D+00 |
| R( 3) | 5 - 5 | 4513.02 | -4.30 | 4.87569D-06 | 9.99999D-01 | -6.64417D-01 |
| R( 4) | 5 - 0 | 463.24 | -4059.45 | 1.33231D+00 | 1.16280D-13 | -1.18199D-02 |
| P( 6) | 5 - 0 | 475.12 | -4047.56 | 1.54587D+00 | 1.66873D-13 | -1.16739D-02 |
| R( 4) | 5 - 1 | 1347.39 | -3175.30 | 2.98660D+02 | 1.05281D-12 | 2.55812D-01 |
| P( 6) | 5 - 1 | 1359.11 | -3163.58 | 3.55648D+02 | 1.52486D-12 | 2.56249D-01 |
| R( 4) | 5 - 2 | 2204.71 | -2317.97 | 3.27224D+02 | 2.28302D-14 | 4.29310D-01 |
| P( 6) | 5 - 2 | 2216.38 | -2306.31 | 3.85735D+02 | 1.13175D-14 | 4.28735D-01 |
| R( 4) | 5 - 3 | 3015.34 | -1507.34 | 5.84946D+01 | 2.25109D-09 | -3.46139D-01 |
| P( 6) | 5 - 3 | 3027.01 | -1495.67 | 6.96156D+01 | 3.15010D-09 | -3.48753D-01 |
| R( 4) | 5 - 4 | 3786.76 | -735.93 | 1.06175D+02 | 7.67105D-07 | -1.36700D+00 |
| P( 6) | 5 - 4 | 3798.46 | -724.22 | 1.21525D+02 | 1.10441D-06 | -1.36756D+00 |
| R( 4) | 5 - 5 | 4517.32 | -5.37 | 9.73832D-06 | 9.99998D-01 | -6.64454D-01 |

| | | | | | | | |
|---|---|---|---|---|---|---|---|
| R( 5) | 5 - 0 | 468.64 | -4060.49 | 1.40375D+00 | 1.67438D-13 | -1.20357D-02 |
| P( 7) | 5 - 0 | 482.69 | -4046.44 | 1.57466D+00 | 2.26986D-13 | -1.18633D-02 |
| R( 5) | 5 - 1 | 1352.72 | -3176.41 | 3.03217D+02 | 1.51182D-12 | 2.55662D-01 |
| P( 7) | 5 - 1 | 1366.57 | -3162.56 | 3.50558D+02 | 2.07081D-12 | 2.56179D-01 |
| R( 5) | 5 - 2 | 2210.02 | -2319.11 | 3.33714D+02 | 3.89853D-14 | 4.29932D-01 |
| P( 7) | 5 - 2 | 2223.80 | -2305.32 | 3.81226D+02 | 1.61313D-14 | 4.29255D-01 |
| R( 5) | 5 - 3 | 3020.65 | -1508.48 | 5.91601D+01 | 3.25288D-09 | -3.45065D-01 |
| P( 7) | 5 - 3 | 3034.44 | -1494.69 | 6.83523D+01 | 4.28033D-09 | -3.48155D-01 |
| R( 5) | 5 - 4 | 3792.08 | -737.05 | 1.08271D+02 | 1.10415D-06 | -1.36680D+00 |
| P( 7) | 5 - 4 | 3805.91 | -723.21 | 1.19451D+02 | 1.50251D-06 | -1.36746D+00 |
| R( 5) | 5 - 5 | 4522.69 | -6.44 | 1.70847D-05 | 9.99997D-01 | -6.64500D-01 |
| R( 6) | 5 - 0 | 475.12 | -4061.52 | 1.47995D+00 | 2.27878D-13 | -1.22853D-02 |
| P( 8) | 5 - 0 | 491.33 | -4045.31 | 1.61755D+00 | 2.96261D-13 | -1.20865D-02 |
| R( 6) | 5 - 1 | 1359.11 | -3177.53 | 3.06505D+02 | 2.05104D-12 | 2.55493D-01 |
| P( 8) | 5 - 1 | 1375.10 | -3161.55 | 3.46647D+02 | 2.69755D-12 | 2.56091D-01 |
| R( 6) | 5 - 2 | 2216.38 | -2320.26 | 3.39053D+02 | 6.29902D-14 | 4.30649D-01 |
| P( 8) | 5 - 2 | 2232.29 | -2304.35 | 3.78200D+02 | 2.26522D-14 | 4.29869D-01 |
| R( 6) | 5 - 3 | 3027.01 | -1509.63 | 5.95332D+01 | 4.44358D-09 | -3.43851D-01 |
| P( 8) | 5 - 3 | 3042.93 | -1493.72 | 6.72832D+01 | 5.58197D-09 | -3.47417D-01 |
| R( 6) | 5 - 4 | 3798.46 | -738.18 | 1.09942D+02 | 1.50209D-06 | -1.36659D+00 |
| P( 8) | 5 - 4 | 3814.43 | -722.22 | 1.17804D+02 | 1.96139D-06 | -1.36735D+00 |
| R( 6) | 5 - 5 | 4529.13 | -7.51 | 2.74273D-05 | 9.99996D-01 | -6.64553D-01 |
| R( 7) | 5 - 0 | 482.69 | -4062.54 | 1.56318D+00 | 2.97585D-13 | -1.25686D-02 |
| P( 9) | 5 - 0 | 501.06 | -4044.17 | 1.67323D+00 | 3.74664D-13 | -1.23434D-02 |
| R( 7) | 5 - 1 | 1366.57 | -3178.66 | 3.08954D+02 | 2.66890D-12 | 2.55305D-01 |
| P( 9) | 5 - 1 | 1384.69 | -3160.54 | 3.43482D+02 | 3.40361D-12 | 2.55983D-01 |
| R( 7) | 5 - 2 | 2223.80 | -2321.42 | 3.43707D+02 | 9.76308D-14 | 4.31460D-01 |
| P( 9) | 5 - 2 | 2241.83 | -2303.40 | 3.76190D+02 | 3.15538D-14 | 4.30578D-01 |
| R( 7) | 5 - 3 | 3034.44 | -1510.79 | 5.96994D+01 | 5.82570D-09 | -3.42497D-01 |

| | | | | | | | |
|---|---|---|---|---|---|---|---|
| P( 9) | 5 - 3 | 3052.47 | -1492.76 | 6.63236D+01 | 7.05480D-09 | -3.46539D-01 |
| R( 7) | 5 - 4 | 3805.91 | -739.32 | 1.11340D+02 | 1.96076D-06 | -1.36634D+00 |
| P( 9) | 5 - 4 | 3824.00 | -721.23 | 1.16434D+02 | 2.48084D-06 | -1.36721D+00 |
| R( 7) | 5 - 5 | 4536.64 | -8.59 | 4.12782D-05 | 9.99995D-01 | -6.64613D-01 |
| R( 8) | 5 - 0 | 491.33 | -4063.56 | 1.65506D+00 | 3.76535D-13 | -1.28855D-02 |
| P( 10) | 5 - 0 | 511.86 | -4043.03 | 1.74123D+00 | 4.62155D-13 | -1.26341D-02 |
| R( 8) | 5 - 1 | 1375.10 | -3179.79 | 3.10813D+02 | 3.36364D-12 | 2.55097D-01 |
| P( 10) | 5 - 1 | 1395.34 | -3159.55 | 3.40814D+02 | 4.18736D-12 | 2.55857D-01 |
| R( 8) | 5 - 2 | 2232.29 | -2322.60 | 3.47947D+02 | 1.46424D-13 | 4.32364D-01 |
| P( 10) | 5 - 2 | 2252.43 | -2302.45 | 3.74926D+02 | 4.37413D-14 | 4.31382D-01 |
| R( 8) | 5 - 3 | 3042.93 | -1511.96 | 5.97082D+01 | 7.40188D-09 | -3.41004D-01 |
| P( 10) | 5 - 3 | 3063.08 | -1491.81 | 6.54246D+01 | 8.69877D-09 | -3.45522D-01 |
| R( 8) | 5 - 4 | 3814.43 | -740.46 | 1.12550D+02 | 2.47993D-06 | -1.36607D+00 |
| P( 10) | 5 - 4 | 3834.64 | -720.25 | 1.15255D+02 | 3.06062D-06 | -1.36704D+00 |
| R( 8) | 5 - 5 | 4545.23 | -9.66 | 5.91483D-05 | 9.99994D-01 | -6.64681D-01 |
| R( 9) | 5 - 0 | 501.06 | -4064.56 | 1.75688D+00 | 4.64703D-13 | -1.32361D-02 |
| P( 11) | 5 - 0 | 523.75 | -4041.87 | 1.82149D+00 | 5.58690D-13 | -1.29584D-02 |
| R( 9) | 5 - 1 | 1384.69 | -3180.93 | 3.12235D+02 | 4.13328D-12 | 2.54869D-01 |
| P( 11) | 5 - 1 | 1407.06 | -3158.56 | 3.38486D+02 | 5.04691D-12 | 2.55711D-01 |
| R( 9) | 5 - 2 | 2241.83 | -2323.79 | 3.51942D+02 | 2.13740D-13 | 4.33361D-01 |
| P( 11) | 5 - 2 | 2264.10 | -2301.52 | 3.74240D+02 | 6.04101D-14 | 4.32279D-01 |
| R( 9) | 5 - 3 | 3052.47 | -1513.15 | 5.95905D+01 | 9.17495D-09 | -3.39371D-01 |
| P( 11) | 5 - 3 | 3074.74 | -1490.88 | 6.45563D+01 | 1.05140D-08 | -3.44365D-01 |
| R( 9) | 5 - 4 | 3824.00 | -741.62 | 1.13627D+02 | 3.05938D-06 | -1.36578D+00 |
| P( 11) | 5 - 4 | 3846.34 | -719.28 | 1.14211D+02 | 3.70049D-06 | -1.36685D+00 |
| R( 9) | 5 - 5 | 4554.89 | -10.73 | 8.15476D-05 | 9.99992D-01 | -6.64755D-01 |
| R( 10) | 5 - 0 | 511.86 | -4065.56 | 1.86979D+00 | 5.62051D-13 | -1.36202D-02 |
| P( 12) | 5 - 0 | 536.71 | -4040.71 | 1.91426D+00 | 6.64216D-13 | -1.33164D-02 |
| R( 10) | 5 - 1 | 1395.34 | -3182.08 | 3.13321D+02 | 4.97561D-12 | 2.54621D-01 |

| | | | | | | | |
|---|---|---|---|---|---|---|---|
| P( 12) | 5 - 1 | 1419.85 | -3157.58 | 3.36398D+02 | 5.98024D-12 | 2.55545D-01 |
| R( 10) | 5 - 2 | 2252.43 | -2324.99 | 3.55801D+02 | 3.04943D-13 | 4.34450D-01 |
| P( 12) | 5 - 2 | 2276.82 | -2300.60 | 3.74023D+02 | 8.31147D-14 | 4.33270D-01 |
| R( 10) | 5 - 3 | 3063.08 | -1514.34 | 5.93665D+01 | 1.11479D-08 | -3.37598D-01 |
| P( 12) | 5 - 3 | 3087.47 | -1489.96 | 6.36994D+01 | 1.25007D-08 | -3.43068D-01 |
| R( 10) | 5 - 4 | 3834.64 | -742.78 | 1.14604D+02 | 3.69883D-06 | -1.36545D+00 |
| P( 12) | 5 - 4 | 3859.11 | -718.32 | 1.13268D+02 | 4.40017D-06 | -1.36664D+00 |
| R( 10) | 5 - 5 | 4565.62 | -11.80 | 1.08985D-04 | 9.99991D-01 | -6.64835D-01 |
| R( 11) | 5 - 0 | 523.75 | -4066.55 | 1.99490D+00 | 6.68539D-13 | -1.40378D-02 |
| P( 13) | 5 - 0 | 550.76 | -4039.54 | 2.01999D+00 | 7.78675D-13 | -1.37080D-02 |
| R( 11) | 5 - 1 | 1407.06 | -3183.23 | 3.14138D+02 | 5.88823D-12 | 2.54353D-01 |
| P( 13) | 5 - 1 | 1433.69 | -3156.60 | 3.34479D+02 | 6.98499D-12 | 2.55360D-01 |
| R( 11) | 5 - 2 | 2264.10 | -2326.20 | 3.59600D+02 | 4.26525D-13 | 4.35631D-01 |
| P( 13) | 5 - 2 | 2290.60 | -2299.70 | 3.74201D+02 | 1.13847D-13 | 4.34354D-01 |
| R( 11) | 5 - 3 | 3074.74 | -1515.55 | 5.90501D+01 | 1.33238D-08 | -3.35685D-01 |
| P( 13) | 5 - 3 | 3101.25 | -1489.05 | 6.28411D+01 | 1.46593D-08 | -3.41631D-01 |
| R( 11) | 5 - 4 | 3846.34 | -743.95 | 1.15507D+02 | 4.39801D-06 | -1.36510D+00 |
| P( 13) | 5 - 4 | 3872.93 | -717.36 | 1.12403D+02 | 5.15935D-06 | -1.36639D+00 |
| R( 11) | 5 - 5 | 4577.42 | -12.87 | 1.41967D-04 | 9.99989D-01 | -6.64920D-01 |
| R( 12) | 5 - 0 | 536.71 | -4067.52 | 2.13328D+00 | 7.84114D-13 | -1.44890D-02 |
| P( 14) | 5 - 0 | 565.88 | -4038.36 | 2.13925D+00 | 9.02000D-13 | -1.41332D-02 |
| R( 12) | 5 - 1 | 1419.85 | -3184.39 | 3.14734D+02 | 6.86845D-12 | 2.54063D-01 |
| P( 14) | 5 - 1 | 1448.61 | -3155.63 | 3.32682D+02 | 8.05871D-12 | 2.55154D-01 |
| R( 12) | 5 - 2 | 2276.82 | -2327.42 | 3.63391D+02 | 5.86271D-13 | 4.36903D-01 |
| P( 14) | 5 - 2 | 2305.44 | -2298.80 | 3.74720D+02 | 1.55127D-13 | 4.35530D-01 |
| R( 12) | 5 - 3 | 3087.47 | -1516.77 | 5.86513D+01 | 1.57059D-08 | -3.33632D-01 |
| P( 14) | 5 - 3 | 3116.09 | -1488.15 | 6.19727D+01 | 1.69904D-08 | -3.40054D-01 |
| R( 12) | 5 - 4 | 3859.11 | -745.13 | 1.16350D+02 | 5.15660D-06 | -1.36472D+00 |
| P( 14) | 5 - 4 | 3887.82 | -716.42 | 1.11597D+02 | 5.97769D-06 | -1.36612D+00 |

| | | | | | | |
|---|---|---|---|---|---|---|
| R( 12) | 5 - 5 | 4590.29 | -13.94 | 1.81000D-04 | 9.99987D-01 | -6.65011D-01 |
| R( 13) | 5 - 0 | 550.76 | -4068.49 | 2.28603D+00 | 9.08716D-13 | -1.49735D-02 |
| P( 15) | 5 - 0 | 582.08 | -4037.17 | 2.27274D+00 | 1.03412D-12 | -1.45919D-02 |
| R( 13) | 5 - 1 | 1433.69 | -3185.55 | 3.15141D+02 | 7.91354D-12 | 2.53752D-01 |
| P( 15) | 5 - 1 | 1464.58 | -3154.67 | 3.30969D+02 | 9.19872D-12 | 2.54927D-01 |
| R( 13) | 5 - 2 | 2290.60 | -2328.65 | 3.67214D+02 | 7.93409D-13 | 4.38265D-01 |
| P( 15) | 5 - 2 | 2321.33 | -2297.92 | 3.75544D+02 | 2.10096D-13 | 4.36799D-01 |
| R( 13) | 5 - 3 | 3101.25 | -1518.00 | 5.81773D+01 | 1.82978D-08 | -3.31438D-01 |
| P( 15) | 5 - 3 | 3131.99 | -1487.26 | 6.10881D+01 | 1.94946D-08 | -3.38337D-01 |
| R( 13) | 5 - 4 | 3872.93 | -746.32 | 1.17147D+02 | 5.97426D-06 | -1.36431D+00 |
| P( 15) | 5 - 4 | 3903.76 | -715.49 | 1.10839D+02 | 6.85486D-06 | -1.36582D+00 |
| R( 13) | 5 - 5 | 4604.24 | -15.01 | 2.26588D-04 | 9.99985D-01 | -6.65106D-01 |
| R( 14) | 5 - 0 | 565.88 | -4069.45 | 2.45428D+00 | 1.04227D-12 | -1.54914D-02 |
| P( 16) | 5 - 0 | 599.36 | -4035.97 | 2.42127D+00 | 1.17494D-12 | -1.50841D-02 |
| R( 14) | 5 - 1 | 1448.61 | -3186.72 | 3.15385D+02 | 9.02040D-12 | 2.53419D-01 |
| P( 16) | 5 - 1 | 1481.62 | -3153.71 | 3.29315D+02 | 1.04021D-11 | 2.54679D-01 |
| R( 14) | 5 - 2 | 2305.44 | -2329.89 | 3.71097D+02 | 1.05879D-12 | 4.39717D-01 |
| P( 16) | 5 - 2 | 2338.29 | -2297.04 | 3.76643D+02 | 2.82627D-13 | 4.38158D-01 |
| R( 14) | 5 - 3 | 3116.09 | -1519.24 | 5.76340D+01 | 2.11028D-08 | -3.29104D-01 |
| P( 16) | 5 - 3 | 3148.94 | -1486.39 | 6.01830D+01 | 2.21728D-08 | -3.36480D-01 |
| R( 14) | 5 - 4 | 3887.82 | -747.51 | 1.17906D+02 | 6.85063D-06 | -1.36387D+00 |
| P( 16) | 5 - 4 | 3920.77 | -714.56 | 1.10119D+02 | 7.79047D-06 | -1.36549D+00 |
| R( 14) | 5 - 5 | 4619.25 | -16.08 | 2.79230D-04 | 9.99983D-01 | -6.65205D-01 |
| R( 15) | 5 - 0 | 582.08 | -4070.40 | 2.63920D+00 | 1.18471D-12 | -1.60427D-02 |
| P( 17) | 5 - 0 | 617.72 | -4034.76 | 2.58571D+00 | 1.32437D-12 | -1.56097D-02 |
| R( 15) | 5 - 1 | 1464.58 | -3187.89 | 3.15484D+02 | 1.01858D-11 | 2.53063D-01 |
| P( 17) | 5 - 1 | 1499.73 | -3152.75 | 3.27699D+02 | 1.16659D-11 | 2.54410D-01 |
| R( 15) | 5 - 2 | 2321.33 | -2331.15 | 3.75062D+02 | 1.39505D-12 | 4.41259D-01 |
| P( 17) | 5 - 2 | 2356.30 | -2296.18 | 3.77997D+02 | 3.77432D-13 | 4.39609D-01 |

| | | | | | | |
|---|---|---|---|---|---|---|
| R( 15) | 5 - 3 | 3131.99 | -1520.49 | 5.70258D+01 | 2.41249D-08 | -3.26630D-01 |
| P( 17) | 5 - 3 | 3166.96 | -1485.52 | 5.92544D+01 | 2.50259D-08 | -3.34482D-01 |
| R( 15) | 5 - 4 | 3903.76 | -748.72 | 1.18634D+02 | 7.78534D-06 | -1.36340D+00 |
| P( 17) | 5 - 4 | 3938.83 | -713.65 | 1.09431D+02 | 8.78414D-06 | -1.36514D+00 |
| R( 15) | 5 - 5 | 4635.33 | -17.15 | 3.39427D-04 | 9.99981D-01 | -6.65307D-01 |
| R( 16) | 5 - 0 | 599.36 | -4071.33 | 2.84201D+00 | 1.33592D-12 | -1.66271D-02 |
| P( 18) | 5 - 0 | 637.15 | -4033.54 | 2.76703D+00 | 1.48230D-12 | -1.61687D-02 |
| R( 16) | 5 - 1 | 1481.62 | -3189.07 | 3.15451D+02 | 1.14062D-11 | 2.52684D-01 |
| P( 18) | 5 - 1 | 1518.89 | -3151.80 | 3.26104D+02 | 1.29866D-11 | 2.54118D-01 |
| R( 16) | 5 - 2 | 2338.29 | -2332.41 | 3.79127D+02 | 1.81683D-12 | 4.42888D-01 |
| P( 18) | 5 - 2 | 2375.37 | -2295.33 | 3.79588D+02 | 5.00191D-13 | 4.41149D-01 |
| R( 16) | 5 - 3 | 3148.94 | -1521.75 | 5.63564D+01 | 2.73677D-08 | -3.24015D-01 |
| P( 18) | 5 - 3 | 3186.03 | -1484.67 | 5.83003D+01 | 2.80551D-08 | -3.32344D-01 |
| R( 16) | 5 - 4 | 3920.77 | -749.93 | 1.19334D+02 | 8.77798D-06 | -1.36289D+00 |
| P( 18) | 5 - 4 | 3957.95 | -712.74 | 1.08768D+02 | 9.83543D-06 | -1.36475D+00 |
| R( 16) | 5 - 5 | 4652.48 | -18.22 | 4.07675D-04 | 9.99978D-01 | -6.65411D-01 |
| R( 17) | 5 - 0 | 617.72 | -4072.26 | 3.06399D+00 | 1.49580D-12 | -1.72447D-02 |
| P( 19) | 5 - 0 | 657.67 | -4032.31 | 2.96626D+00 | 1.64861D-12 | -1.67609D-02 |
| R( 17) | 5 - 1 | 1499.73 | -3190.25 | 3.15297D+02 | 1.26780D-11 | 2.52282D-01 |
| P( 19) | 5 - 1 | 1539.12 | -3150.86 | 3.24517D+02 | 1.43609D-11 | 2.53804D-01 |
| R( 17) | 5 - 2 | 2356.30 | -2333.68 | 3.83305D+02 | 2.34090D-12 | 4.44605D-01 |
| P( 19) | 5 - 2 | 2395.49 | -2294.49 | 3.81404D+02 | 6.57673D-13 | 4.42779D-01 |
| R( 17) | 5 - 3 | 3166.96 | -1523.02 | 5.56288D+01 | 3.08354D-08 | -3.21258D-01 |
| P( 19) | 5 - 3 | 3206.15 | -1483.83 | 5.73195D+01 | 3.12615D-08 | -3.30065D-01 |
| R( 17) | 5 - 4 | 3938.83 | -751.15 | 1.20012D+02 | 9.82812D-06 | -1.36236D+00 |
| P( 19) | 5 - 4 | 3978.14 | -711.84 | 1.08128D+02 | 1.09439D-05 | -1.36432D+00 |
| R( 17) | 5 - 5 | 4670.69 | -19.28 | 4.84464D-04 | 9.99976D-01 | -6.65517D-01 |
| R( 18) | 5 - 0 | 637.15 | -4073.17 | 3.30647D+00 | 1.66422D-12 | -1.78952D-02 |
| P( 20) | 5 - 0 | 679.26 | -4031.07 | 3.18450D+00 | 1.82316D-12 | -1.73863D-02 |

| | | | | | | | |
|---|---|---|---|---|---|---|---|
| R( 18) | 5 - 1 | 1518.89 | -3191.43 | 3.15029D+02 | 1.39973D-11 | 2.51856D-01 |
| P( 20) | 5 - 1 | 1560.41 | -3149.91 | 3.22928D+02 | 1.57852D-11 | 2.53467D-01 |
| R( 18) | 5 - 2 | 2375.37 | -2334.96 | 3.87608D+02 | 2.98643D-12 | 4.46408D-01 |
| P( 20) | 5 - 2 | 2416.67 | -2293.65 | 3.83433D+02 | 8.57872D-13 | 4.44497D-01 |
| R( 18) | 5 - 3 | 3186.03 | -1524.30 | 5.48457D+01 | 3.45319D-08 | -3.18361D-01 |
| P( 20) | 5 - 3 | 3227.33 | -1482.99 | 5.63110D+01 | 3.46466D-08 | -3.27645D-01 |
| R( 18) | 5 - 4 | 3957.95 | -752.37 | 1.20670D+02 | 1.09353D-05 | -1.36178D+00 |
| P( 20) | 5 - 4 | 3999.37 | -710.95 | 1.07506D+02 | 1.21092D-05 | -1.36387D+00 |
| R( 18) | 5 - 5 | 4689.98 | -20.35 | 5.70284D-04 | 9.99973D-01 | -6.65624D-01 |
| R( 19) | 5 - 0 | 657.67 | -4074.07 | 3.57081D+00 | 1.84105D-12 | -1.85788D-02 |
| P( 21) | 5 - 0 | 701.93 | -4029.81 | 3.42290D+00 | 2.00581D-12 | -1.80448D-02 |
| R( 19) | 5 - 1 | 1539.12 | -3192.62 | 3.14655D+02 | 1.53601D-11 | 2.51405D-01 |
| P( 21) | 5 - 1 | 1582.76 | -3148.97 | 3.21328D+02 | 1.72554D-11 | 2.53106D-01 |
| R( 19) | 5 - 2 | 2395.49 | -2336.25 | 3.92044D+02 | 3.77514D-12 | 4.48296D-01 |
| P( 21) | 5 - 2 | 2438.90 | -2292.83 | 3.85668D+02 | 1.11015D-12 | 4.46303D-01 |
| R( 19) | 5 - 3 | 3206.15 | -1525.59 | 5.40095D+01 | 3.84617D-08 | -3.15323D-01 |
| P( 21) | 5 - 3 | 3249.56 | -1482.17 | 5.52746D+01 | 3.82118D-08 | -3.25084D-01 |
| R( 19) | 5 - 4 | 3978.14 | -753.60 | 1.21311D+02 | 1.20991D-05 | -1.36117D+00 |
| P( 21) | 5 - 4 | 4021.67 | -710.07 | 1.06899D+02 | 1.33307D-05 | -1.36338D+00 |
| R( 19) | 5 - 5 | 4710.32 | -21.41 | 6.65620D-04 | 9.99970D-01 | -6.65730D-01 |
| Q( 0) | 0 - 0 | 452.43 | 0.00 | 0.00000D+00 | 1.00000D+00 | -1.24139D+00 |
| Q( 1) | 0 - 0 | 453.51 | -0.00 | 0.00000D+00 | 1.00000D+00 | -1.24131D+00 |
| Q( 2) | 0 - 0 | 455.67 | 0.00 | 0.00000D+00 | 1.00000D+00 | -1.24115D+00 |
| Q( 3) | 0 - 0 | 458.91 | 0.00 | 0.00000D+00 | 1.00000D+00 | -1.24091D+00 |
| Q( 4) | 0 - 0 | 463.24 | 0.00 | 0.00000D+00 | 1.00000D+00 | -1.24059D+00 |
| Q( 5) | 0 - 0 | 468.64 | 0.00 | 0.00000D+00 | 1.00000D+00 | -1.24019D+00 |
| Q( 6) | 0 - 0 | 475.12 | 0.00 | 0.00000D+00 | 1.00000D+00 | -1.23971D+00 |
| Q( 7) | 0 - 0 | 482.69 | 0.00 | 0.00000D+00 | 1.00000D+00 | -1.23915D+00 |
| Q( 8) | 0 - 0 | 491.33 | 0.00 | 0.00000D+00 | 1.00000D+00 | -1.23851D+00 |

| | | | | | | |
|---|---|---|---|---|---|---|
| Q( 9) | 0 - 0 | 501.06 | 0.00 | 0.00000D+00 | 1.00000D+00 | -1.23779D+00 |
| Q( 10) | 0 - 0 | 511.86 | 0.00 | 0.00000D+00 | 1.00000D+00 | -1.23698D+00 |
| Q( 11) | 0 - 0 | 523.75 | 0.00 | 0.00000D+00 | 1.00000D+00 | -1.23610D+00 |
| Q( 12) | 0 - 0 | 536.71 | -0.00 | 0.00000D+00 | 1.00000D+00 | -1.23513D+00 |
| Q( 13) | 0 - 0 | 550.76 | -0.00 | 0.00000D+00 | 1.00000D+00 | -1.23408D+00 |
| Q( 14) | 0 - 0 | 565.88 | -0.00 | 0.00000D+00 | 1.00000D+00 | -1.23294D+00 |
| Q( 15) | 0 - 0 | 582.08 | -0.00 | 0.00000D+00 | 1.00000D+00 | -1.23172D+00 |
| Q( 16) | 0 - 0 | 599.36 | -0.00 | 0.00000D+00 | 1.00000D+00 | -1.23042D+00 |
| Q( 17) | 0 - 0 | 617.72 | -0.00 | 0.00000D+00 | 1.00000D+00 | -1.22903D+00 |
| Q( 18) | 0 - 0 | 637.15 | -0.00 | 0.00000D+00 | 1.00000D+00 | -1.22755D+00 |
| Q( 19) | 0 - 0 | 657.67 | -0.00 | 0.00000D+00 | 1.00000D+00 | -1.22599D+00 |
| Q( 20) | 0 - 0 | 679.26 | -0.00 | 0.00000D+00 | 1.00000D+00 | -1.22434D+00 |
| Q( 0) | 1 - 0 | 452.43 | -884.30 | 0.00000D+00 | 6.68700D-19 | -7.07226D-01 |
| Q( 0) | 1 - 1 | 1336.73 | 0.00 | 0.00000D+00 | 1.00000D+00 | 9.97701D-02 |
| Q( 1) | 1 - 0 | 453.51 | -884.29 | 0.00000D+00 | 7.50251D-18 | -7.07335D-01 |
| Q( 1) | 1 - 1 | 1337.79 | -0.00 | 0.00000D+00 | 1.00000D+00 | 9.96265D-02 |
| Q( 2) | 1 - 0 | 455.67 | -884.26 | 0.00000D+00 | 2.49260D-24 | -7.07554D-01 |
| Q( 2) | 1 - 1 | 1339.93 | 0.00 | 0.00000D+00 | 1.00000D+00 | 9.93391D-02 |
| Q( 3) | 1 - 0 | 458.91 | -884.21 | 0.00000D+00 | 2.49549D-24 | -7.07883D-01 |
| Q( 3) | 1 - 1 | 1343.12 | 0.00 | 0.00000D+00 | 1.00000D+00 | 9.89081D-02 |
| Q( 4) | 1 - 0 | 463.24 | -884.15 | 0.00000D+00 | 2.62813D-24 | -7.08321D-01 |
| Q( 4) | 1 - 1 | 1347.39 | 0.00 | 0.00000D+00 | 1.00000D+00 | 9.83335D-02 |
| Q( 5) | 1 - 0 | 468.64 | -884.08 | 0.00000D+00 | 2.60992D-24 | -7.08869D-01 |
| Q( 5) | 1 - 1 | 1352.72 | 0.00 | 0.00000D+00 | 1.00000D+00 | 9.76152D-02 |
| Q( 6) | 1 - 0 | 475.12 | -883.99 | 0.00000D+00 | 2.70087D-24 | -7.09527D-01 |
| Q( 6) | 1 - 1 | 1359.11 | 0.00 | 0.00000D+00 | 1.00000D+00 | 9.67532D-02 |
| Q( 7) | 1 - 0 | 482.69 | -883.88 | 0.00000D+00 | 2.82613D-24 | -7.10294D-01 |
| Q( 7) | 1 - 1 | 1366.57 | 0.00 | 0.00000D+00 | 1.00000D+00 | 9.57475D-02 |
| Q( 8) | 1 - 0 | 491.33 | -883.76 | 0.00000D+00 | 3.02784D-24 | -7.11172D-01 |

| | | | | | | |
|---|---|---|---|---|---|---|
| Q( 8) | 1 - 1 | 1375.10 | 0.00 | 0.00000D+00 | 1.00000D+00 | 9.45982D-02 |
| Q( 9) | 1 - 0 | 501.06 | -883.63 | 0.00000D+00 | 3.33329D-24 | -7.12160D-01 |
| Q( 9) | 1 - 1 | 1384.69 | 0.00 | 0.00000D+00 | 1.00000D+00 | 9.33052D-02 |
| Q( 10) | 1 - 0 | 511.86 | -883.48 | 0.00000D+00 | 3.64441D-24 | -7.13257D-01 |
| Q( 10) | 1 - 1 | 1395.34 | 0.00 | 0.00000D+00 | 1.00000D+00 | 9.18685D-02 |
| Q( 11) | 1 - 0 | 523.75 | -883.31 | 0.00000D+00 | 4.23703D-24 | -7.14466D-01 |
| Q( 11) | 1 - 1 | 1407.06 | 0.00 | 0.00000D+00 | 1.00000D+00 | 9.02881D-02 |
| Q( 12) | 1 - 0 | 536.71 | -883.13 | 0.00000D+00 | 4.99135D-24 | -7.15785D-01 |
| Q( 12) | 1 - 1 | 1419.85 | 0.00 | 0.00000D+00 | 1.00000D+00 | 8.85641D-02 |
| Q( 13) | 1 - 0 | 550.76 | -882.94 | 0.00000D+00 | 8.77991D-24 | -7.17214D-01 |
| Q( 13) | 1 - 1 | 1433.69 | 0.00 | 0.00000D+00 | 1.00000D+00 | 8.66964D-02 |
| Q( 14) | 1 - 0 | 565.88 | -882.73 | 0.00000D+00 | 1.07542D-23 | -7.18755D-01 |
| Q( 14) | 1 - 1 | 1448.61 | 0.00 | 0.00000D+00 | 1.00000D+00 | 8.46850D-02 |
| Q( 15) | 1 - 0 | 582.08 | -882.50 | 0.00000D+00 | 1.36817D-23 | -7.20406D-01 |
| Q( 15) | 1 - 1 | 1464.58 | 0.00 | 0.00000D+00 | 1.00000D+00 | 8.25300D-02 |
| Q( 16) | 1 - 0 | 599.36 | -882.26 | 0.00000D+00 | 1.75504D-23 | -7.22169D-01 |
| Q( 16) | 1 - 1 | 1481.62 | 0.00 | 0.00000D+00 | 1.00000D+00 | 8.02313D-02 |
| Q( 17) | 1 - 0 | 617.72 | -882.01 | 0.00000D+00 | 2.26683D-23 | -7.24044D-01 |
| Q( 17) | 1 - 1 | 1499.73 | 0.00 | 0.00000D+00 | 1.00000D+00 | 7.77889D-02 |
| Q( 18) | 1 - 0 | 637.15 | -881.74 | 0.00000D+00 | 2.92335D-23 | -7.26030D-01 |
| Q( 18) | 1 - 1 | 1518.89 | 0.00 | 0.00000D+00 | 1.00000D+00 | 7.52030D-02 |
| Q( 19) | 1 - 0 | 657.67 | -881.45 | 0.00000D+00 | 3.79420D-23 | -7.28129D-01 |
| Q( 19) | 1 - 1 | 1539.12 | 0.00 | 0.00000D+00 | 1.00000D+00 | 7.24734D-02 |
| Q( 20) | 1 - 0 | 679.26 | -881.15 | 0.00000D+00 | 4.90395D-23 | -7.30340D-01 |
| Q( 20) | 1 - 1 | 1560.41 | 0.00 | 0.00000D+00 | 1.00000D+00 | 6.96002D-02 |
| Q( 0) | 2 - 0 | 452.43 | -1741.68 | 0.00000D+00 | 3.89693D-26 | 5.36526D-01 |
| Q( 0) | 2 - 1 | 1336.73 | -857.38 | 0.00000D+00 | 5.76721D-18 | 1.35332D+00 |
| Q( 0) | 2 - 2 | 2194.11 | 0.00 | 0.00000D+00 | 1.00000D+00 | 5.30993D-01 |
| Q( 1) | 2 - 0 | 453.51 | -1741.66 | 0.00000D+00 | 3.00540D-19 | 5.36534D-01 |

| | | | | | | | |
|---|---|---|---|---|---|---|---|
| Q( 1) | 2 - 1 | 1337.79 | -857.37 | 0.00000D+00 | 2.69460D-17 | 1.35340D+00 |
| Q( 1) | 2 - 2 | 2195.17 | -0.00 | 0.00000D+00 | 1.00000D+00 | 5.31116D-01 |
| Q( 2) | 2 - 0 | 455.67 | -1741.62 | 0.00000D+00 | 1.13854D-26 | 5.36548D-01 |
| Q( 2) | 2 - 1 | 1339.93 | -857.36 | 0.00000D+00 | 5.74999D-18 | 1.35357D+00 |
| Q( 2) | 2 - 2 | 2197.29 | 0.00 | 0.00000D+00 | 1.00000D+00 | 5.31361D-01 |
| Q( 3) | 2 - 0 | 458.91 | -1741.56 | 0.00000D+00 | 1.07968D-26 | 5.36569D-01 |
| Q( 3) | 2 - 1 | 1343.12 | -857.35 | 0.00000D+00 | 5.74047D-18 | 1.35383D+00 |
| Q( 3) | 2 - 2 | 2200.47 | 0.00 | 0.00000D+00 | 1.00000D+00 | 5.31728D-01 |
| Q( 4) | 2 - 0 | 463.24 | -1741.48 | 0.00000D+00 | 1.03040D-26 | 5.36598D-01 |
| Q( 4) | 2 - 1 | 1347.39 | -857.33 | 0.00000D+00 | 5.72794D-18 | 1.35418D+00 |
| Q( 4) | 2 - 2 | 2204.71 | 0.00 | 0.00000D+00 | 1.00000D+00 | 5.32218D-01 |
| Q( 5) | 2 - 0 | 468.64 | -1741.38 | 0.00000D+00 | 8.60695D-27 | 5.36633D-01 |
| Q( 5) | 2 - 1 | 1352.72 | -857.30 | 0.00000D+00 | 5.71257D-18 | 1.35460D+00 |
| Q( 5) | 2 - 2 | 2210.02 | 0.00 | 0.00000D+00 | 1.00000D+00 | 5.32830D-01 |
| Q( 6) | 2 - 0 | 475.12 | -1741.26 | 0.00000D+00 | 6.97295D-27 | 5.36675D-01 |
| Q( 6) | 2 - 1 | 1359.11 | -857.27 | 0.00000D+00 | 5.69408D-18 | 1.35512D+00 |
| Q( 6) | 2 - 2 | 2216.38 | 0.00 | 0.00000D+00 | 1.00000D+00 | 5.33564D-01 |
| Q( 7) | 2 - 0 | 482.69 | -1741.12 | 0.00000D+00 | 5.24643D-27 | 5.36724D-01 |
| Q( 7) | 2 - 1 | 1366.57 | -857.23 | 0.00000D+00 | 5.67287D-18 | 1.35572D+00 |
| Q( 7) | 2 - 2 | 2223.80 | 0.00 | 0.00000D+00 | 1.00000D+00 | 5.34420D-01 |
| Q( 8) | 2 - 0 | 491.33 | -1740.95 | 0.00000D+00 | 2.07555D-27 | 5.36779D-01 |
| Q( 8) | 2 - 1 | 1375.10 | -857.19 | 0.00000D+00 | 5.64908D-18 | 1.35640D+00 |
| Q( 8) | 2 - 2 | 2232.29 | 0.00 | 0.00000D+00 | 1.00000D+00 | 5.35398D-01 |
| Q( 9) | 2 - 0 | 501.06 | -1740.77 | 0.00000D+00 | 2.37644D-28 | 5.36841D-01 |
| Q( 9) | 2 - 1 | 1384.69 | -857.15 | 0.00000D+00 | 5.62272D-18 | 1.35717D+00 |
| Q( 9) | 2 - 2 | 2241.83 | 0.00 | 0.00000D+00 | 1.00000D+00 | 5.36498D-01 |
| Q( 10) | 2 - 0 | 511.86 | -1740.57 | 0.00000D+00 | 7.23525D-28 | 5.36908D-01 |
| Q( 10) | 2 - 1 | 1395.34 | -857.09 | 0.00000D+00 | 5.59392D-18 | 1.35803D+00 |
| Q( 10) | 2 - 2 | 2252.43 | 0.00 | 0.00000D+00 | 1.00000D+00 | 5.37719D-01 |

| | | | | | | | |
|---|---|---|---|---|---|---|---|
| Q( 11) | 2 - 0 | 523.75 | -1740.35 | 0.00000D+00 | 4.06867D-26 | 5.36981D-01 |
| Q( 11) | 2 - 1 | 1407.06 | -857.04 | 0.00000D+00 | 5.56576D-18 | 1.35896D+00 |
| Q( 11) | 2 - 2 | 2264.10 | 0.00 | 0.00000D+00 | 1.00000D+00 | 5.39062D-01 |
| Q( 12) | 2 - 0 | 536.71 | -1740.11 | 0.00000D+00 | 8.49747D-26 | 5.37059D-01 |
| Q( 12) | 2 - 1 | 1419.85 | -856.97 | 0.00000D+00 | 5.71431D-18 | 1.35999D+00 |
| Q( 12) | 2 - 2 | 2276.82 | -0.00 | 0.00000D+00 | 1.00000D+00 | 5.40526D-01 |
| Q( 13) | 2 - 0 | 550.76 | -1739.84 | 0.00000D+00 | 1.64662D-25 | 5.37143D-01 |
| Q( 13) | 2 - 1 | 1433.69 | -856.90 | 0.00000D+00 | 5.67922D-18 | 1.36109D+00 |
| Q( 13) | 2 - 2 | 2290.60 | -0.00 | 0.00000D+00 | 1.00000D+00 | 5.42111D-01 |
| Q( 14) | 2 - 0 | 565.88 | -1739.56 | 0.00000D+00 | 2.86050D-25 | 5.37231D-01 |
| Q( 14) | 2 - 1 | 1448.61 | -856.83 | 0.00000D+00 | 5.64259D-18 | 1.36228D+00 |
| Q( 14) | 2 - 2 | 2305.44 | -0.00 | 0.00000D+00 | 1.00000D+00 | 5.43816D-01 |
| Q( 15) | 2 - 0 | 582.08 | -1739.25 | 0.00000D+00 | 4.75225D-25 | 5.37323D-01 |
| Q( 15) | 2 - 1 | 1464.58 | -856.75 | 0.00000D+00 | 5.60457D-18 | 1.36355D+00 |
| Q( 15) | 2 - 2 | 2321.33 | -0.00 | 0.00000D+00 | 1.00000D+00 | 5.45642D-01 |
| Q( 16) | 2 - 0 | 599.36 | -1738.93 | 0.00000D+00 | 7.74006D-25 | 5.37419D-01 |
| Q( 16) | 2 - 1 | 1481.62 | -856.66 | 0.00000D+00 | 5.56552D-18 | 1.36491D+00 |
| Q( 16) | 2 - 2 | 2338.29 | -0.00 | 0.00000D+00 | 1.00000D+00 | 5.47588D-01 |
| Q( 17) | 2 - 0 | 617.72 | -1738.58 | 0.00000D+00 | 1.14786D-24 | 5.37518D-01 |
| Q( 17) | 2 - 1 | 1499.73 | -856.57 | 0.00000D+00 | 5.52581D-18 | 1.36634D+00 |
| Q( 17) | 2 - 2 | 2356.30 | -0.00 | 0.00000D+00 | 1.00000D+00 | 5.49654D-01 |
| Q( 18) | 2 - 0 | 637.15 | -1738.21 | 0.00000D+00 | 1.77183D-24 | 5.37621D-01 |
| Q( 18) | 2 - 1 | 1518.89 | -856.47 | 0.00000D+00 | 5.48544D-18 | 1.36786D+00 |
| Q( 18) | 2 - 2 | 2375.37 | -0.00 | 0.00000D+00 | 1.00000D+00 | 5.51840D-01 |
| Q( 19) | 2 - 0 | 657.67 | -1737.82 | 0.00000D+00 | 2.66288D-24 | 5.37726D-01 |
| Q( 19) | 2 - 1 | 1539.12 | -856.37 | 0.00000D+00 | 5.44490D-18 | 1.36946D+00 |
| Q( 19) | 2 - 2 | 2395.49 | -0.00 | 0.00000D+00 | 1.00000D+00 | 5.54144D-01 |
| Q( 20) | 2 - 0 | 679.26 | -1737.41 | 0.00000D+00 | 3.90058D-24 | 5.37832D-01 |
| Q( 20) | 2 - 1 | 1560.41 | -856.26 | 0.00000D+00 | 5.40435D-18 | 1.37114D+00 |

| | | | | | | |
|---|---|---|---|---|---|---|
| Q( 20) | 2 - 2 | 2416.67 | -0.00 | 0.00000D+00 | 1.00000D+00 | 5.56567D-01 |
| Q( 0) | 3 - 0 | 452.43 | -2552.31 | 0.00000D+00 | 1.30000D-22 | 5.81392D-02 |
| Q( 0) | 3 - 1 | 1336.73 | -1668.01 | 0.00000D+00 | 4.67760D-19 | -5.85464D-01 |
| Q( 0) | 3 - 2 | 2194.11 | -810.63 | 0.00000D+00 | 6.21413D-20 | -1.56611D+00 |
| Q( 0) | 3 - 3 | 3004.73 | 0.00 | 0.00000D+00 | 1.00000D+00 | -7.92303D-01 |
| Q( 1) | 3 - 0 | 453.51 | -2552.29 | 0.00000D+00 | 3.53127D-20 | 5.81935D-02 |
| Q( 1) | 3 - 1 | 1337.79 | -1668.00 | 0.00000D+00 | 1.36437D-20 | -5.85409D-01 |
| Q( 1) | 3 - 2 | 2195.17 | -810.63 | 0.00000D+00 | 1.53365D-17 | -1.56616D+00 |
| Q( 1) | 3 - 3 | 3005.79 | -0.00 | 0.00000D+00 | 1.00000D+00 | -7.92382D-01 |
| Q( 2) | 3 - 0 | 455.67 | -2552.25 | 0.00000D+00 | 1.48768D-25 | 5.83022D-02 |
| Q( 2) | 3 - 1 | 1339.93 | -1667.99 | 0.00000D+00 | 5.41993D-19 | -5.85298D-01 |
| Q( 2) | 3 - 2 | 2197.29 | -810.63 | 0.00000D+00 | 1.88007D-23 | -1.56626D+00 |
| Q( 2) | 3 - 3 | 3007.92 | 0.00 | 0.00000D+00 | 1.00000D+00 | -7.92541D-01 |
| Q( 3) | 3 - 0 | 458.91 | -2552.19 | 0.00000D+00 | 1.46458D-25 | 5.84652D-02 |
| Q( 3) | 3 - 1 | 1343.12 | -1667.98 | 0.00000D+00 | 5.40257D-19 | -5.85132D-01 |
| Q( 3) | 3 - 2 | 2200.47 | -810.63 | 0.00000D+00 | 1.89513D-23 | -1.56642D+00 |
| Q( 3) | 3 - 3 | 3011.10 | 0.00 | 0.00000D+00 | 1.00000D+00 | -7.92778D-01 |
| Q( 4) | 3 - 0 | 463.24 | -2552.11 | 0.00000D+00 | 1.49904D-25 | 5.86826D-02 |
| Q( 4) | 3 - 1 | 1347.39 | -1667.96 | 0.00000D+00 | 5.37934D-19 | -5.84910D-01 |
| Q( 4) | 3 - 2 | 2204.71 | -810.63 | 0.00000D+00 | 1.92372D-23 | -1.56663D+00 |
| Q( 4) | 3 - 3 | 3015.34 | 0.00 | 0.00000D+00 | 1.00000D+00 | -7.93095D-01 |
| Q( 5) | 3 - 0 | 468.64 | -2552.01 | 0.00000D+00 | 1.46138D-25 | 5.89544D-02 |
| Q( 5) | 3 - 1 | 1352.72 | -1667.93 | 0.00000D+00 | 5.35076D-19 | -5.84632D-01 |
| Q( 5) | 3 - 2 | 2210.02 | -810.63 | 0.00000D+00 | 1.97271D-23 | -1.56689D+00 |
| Q( 5) | 3 - 3 | 3020.65 | 0.00 | 0.00000D+00 | 1.00000D+00 | -7.93490D-01 |
| Q( 6) | 3 - 0 | 475.12 | -2551.89 | 0.00000D+00 | 1.41490D-25 | 5.92807D-02 |
| Q( 6) | 3 - 1 | 1359.11 | -1667.90 | 0.00000D+00 | 5.31634D-19 | -5.84299D-01 |
| Q( 6) | 3 - 2 | 2216.38 | -810.63 | 0.00000D+00 | 2.04501D-23 | -1.56720D+00 |
| Q( 6) | 3 - 3 | 3027.01 | 0.00 | 0.00000D+00 | 1.00000D+00 | -7.93964D-01 |

| | | | | | | | |
|---|---|---|---|---|---|---|---|
| Q( 7) | 3 - 0 | 482.69 | -2551.75 | 0.00000D+00 | 1.35971D-25 | 5.96614D-02 |
| Q( 7) | 3 - 1 | 1366.57 | -1667.87 | 0.00000D+00 | 5.27656D-19 | -5.83909D-01 |
| Q( 7) | 3 - 2 | 2223.80 | -810.64 | 0.00000D+00 | 2.15572D-23 | -1.56757D+00 |
| Q( 7) | 3 - 3 | 3034.44 | 0.00 | 0.00000D+00 | 1.00000D+00 | -7.94517D-01 |
| Q( 8) | 3 - 0 | 491.33 | -2551.59 | 0.00000D+00 | 1.28225D-25 | 6.00967D-02 |
| Q( 8) | 3 - 1 | 1375.10 | -1667.83 | 0.00000D+00 | 5.23141D-19 | -5.83464D-01 |
| Q( 8) | 3 - 2 | 2232.29 | -810.64 | 0.00000D+00 | 2.36764D-23 | -1.56799D+00 |
| Q( 8) | 3 - 3 | 3042.93 | 0.00 | 0.00000D+00 | 1.00000D+00 | -7.95148D-01 |
| Q( 9) | 3 - 0 | 501.06 | -2551.41 | 0.00000D+00 | 1.19427D-25 | 6.05865D-02 |
| Q( 9) | 3 - 1 | 1384.69 | -1667.79 | 0.00000D+00 | 5.18112D-19 | -5.82961D-01 |
| Q( 9) | 3 - 2 | 2241.83 | -810.64 | 0.00000D+00 | 2.61220D-23 | -1.56845D+00 |
| Q( 9) | 3 - 3 | 3052.47 | 0.00 | 0.00000D+00 | 1.00000D+00 | -7.95856D-01 |
| Q( 10) | 3 - 0 | 511.86 | -2551.21 | 0.00000D+00 | 1.04520D-25 | 6.11309D-02 |
| Q( 10) | 3 - 1 | 1395.34 | -1667.74 | 0.00000D+00 | 5.12572D-19 | -5.82403D-01 |
| Q( 10) | 3 - 2 | 2252.43 | -810.64 | 0.00000D+00 | 2.95360D-23 | -1.56897D+00 |
| Q( 10) | 3 - 3 | 3063.08 | 0.00 | 0.00000D+00 | 1.00000D+00 | -7.96642D-01 |
| Q( 11) | 3 - 0 | 523.75 | -2550.99 | 0.00000D+00 | 9.50031D-26 | 6.17300D-02 |
| Q( 11) | 3 - 1 | 1407.06 | -1667.68 | 0.00000D+00 | 5.06531D-19 | -5.81787D-01 |
| Q( 11) | 3 - 2 | 2264.10 | -810.65 | 0.00000D+00 | 3.44449D-23 | -1.56953D+00 |
| Q( 11) | 3 - 3 | 3074.74 | 0.00 | 0.00000D+00 | 1.00000D+00 | -7.97505D-01 |
| Q( 12) | 3 - 0 | 536.71 | -2550.75 | 0.00000D+00 | 7.87450D-26 | 6.23839D-02 |
| Q( 12) | 3 - 1 | 1419.85 | -1667.62 | 0.00000D+00 | 5.59368D-19 | -5.81114D-01 |
| Q( 12) | 3 - 2 | 2276.82 | -810.65 | 0.00000D+00 | 4.17896D-23 | -1.57015D+00 |
| Q( 12) | 3 - 3 | 3087.47 | 0.00 | 0.00000D+00 | 1.00000D+00 | -7.98445D-01 |
| Q( 13) | 3 - 0 | 550.76 | -2550.49 | 0.00000D+00 | 3.63695D-26 | 6.30926D-02 |
| Q( 13) | 3 - 1 | 1433.69 | -1667.55 | 0.00000D+00 | 5.51434D-19 | -5.80383D-01 |
| Q( 13) | 3 - 2 | 2290.60 | -810.65 | 0.00000D+00 | 6.81214D-23 | -1.57082D+00 |
| Q( 13) | 3 - 3 | 3101.25 | 0.00 | 0.00000D+00 | 1.00000D+00 | -7.99461D-01 |
| Q( 14) | 3 - 0 | 565.88 | -2550.21 | 0.00000D+00 | 1.69825D-26 | 6.38562D-02 |

| | | | | | | | |
|---|---|---|---|---|---|---|---|
| Q( 14) | 3 - 1 | 1448.61 | -1667.48 | 0.00000D+00 | 5.43354D-19 | -5.79595D-01 |
| Q( 14) | 3 - 2 | 2305.44 | -810.65 | 0.00000D+00 | 8.73087D-23 | -1.57153D+00 |
| Q( 14) | 3 - 3 | 3116.09 | 0.00 | 0.00000D+00 | 1.00000D+00 | -8.00552D-01 |
| Q( 15) | 3 - 0 | 582.08 | -2549.91 | 0.00000D+00 | 5.06874D-27 | 6.46747D-02 |
| Q( 15) | 3 - 1 | 1464.58 | -1667.40 | 0.00000D+00 | 5.34819D-19 | -5.78748D-01 |
| Q( 15) | 3 - 2 | 2321.33 | -810.66 | 0.00000D+00 | 1.12460D-22 | -1.57229D+00 |
| Q( 15) | 3 - 3 | 3131.99 | 0.00 | 0.00000D+00 | 1.00000D+00 | -8.01719D-01 |
| Q( 16) | 3 - 0 | 599.36 | -2549.58 | 0.00000D+00 | 1.63916D-29 | 6.55484D-02 |
| Q( 16) | 3 - 1 | 1481.62 | -1667.32 | 0.00000D+00 | 5.25855D-19 | -5.77842D-01 |
| Q( 16) | 3 - 2 | 2338.29 | -810.66 | 0.00000D+00 | 1.46471D-22 | -1.57310D+00 |
| Q( 16) | 3 - 3 | 3148.94 | 0.00 | 0.00000D+00 | 1.00000D+00 | -8.02960D-01 |
| Q( 17) | 3 - 0 | 617.72 | -2549.24 | 0.00000D+00 | 7.38208D-27 | 6.64772D-02 |
| Q( 17) | 3 - 1 | 1499.73 | -1667.23 | 0.00000D+00 | 5.16480D-19 | -5.76877D-01 |
| Q( 17) | 3 - 2 | 2356.30 | -810.66 | 0.00000D+00 | 1.91979D-22 | -1.57395D+00 |
| Q( 17) | 3 - 3 | 3166.96 | 0.00 | 0.00000D+00 | 1.00000D+00 | -8.04275D-01 |
| Q( 18) | 3 - 0 | 637.15 | -2548.87 | 0.00000D+00 | 3.72861D-26 | 6.74612D-02 |
| Q( 18) | 3 - 1 | 1518.89 | -1667.13 | 0.00000D+00 | 5.06732D-19 | -5.75852D-01 |
| Q( 18) | 3 - 2 | 2375.37 | -810.66 | 0.00000D+00 | 2.53965D-22 | -1.57485D+00 |
| Q( 18) | 3 - 3 | 3186.03 | 0.00 | 0.00000D+00 | 1.00000D+00 | -8.05663D-01 |
| Q( 19) | 3 - 0 | 657.67 | -2548.48 | 0.00000D+00 | 9.63440D-26 | 6.85006D-02 |
| Q( 19) | 3 - 1 | 1539.12 | -1667.03 | 0.00000D+00 | 4.96613D-19 | -5.74767D-01 |
| Q( 19) | 3 - 2 | 2395.49 | -810.66 | 0.00000D+00 | 3.36208D-22 | -1.57579D+00 |
| Q( 19) | 3 - 3 | 3206.15 | 0.00 | 0.00000D+00 | 1.00000D+00 | -8.07124D-01 |
| Q( 20) | 3 - 0 | 679.26 | -2548.07 | 0.00000D+00 | 2.02148D-25 | 6.95954D-02 |
| Q( 20) | 3 - 1 | 1560.41 | -1666.92 | 0.00000D+00 | 4.86147D-19 | -5.73621D-01 |
| Q( 20) | 3 - 2 | 2416.67 | -810.66 | 0.00000D+00 | 4.47062D-22 | -1.57678D+00 |
| Q( 20) | 3 - 3 | 3227.33 | 0.00 | 0.00000D+00 | 1.00000D+00 | -8.08656D-01 |
| Q( 0) | 4 - 0 | 452.43 | -3323.68 | 0.00000D+00 | 3.55240D-23 | -1.79690D-01 |
| Q( 0) | 4 - 1 | 1336.73 | -2439.38 | 0.00000D+00 | 4.61170D-20 | -2.51405D-01 |

| | | | | | | | |
|---|---|---|---|---|---|---|---|
| Q( 0) | 4 - 2 | 2194.11 | -1582.01 | 0.00000D+00 | 1.19282D-20 | 5.09722D-01 |
| Q( 0) | 4 - 3 | 3004.73 | -771.38 | 0.00000D+00 | 1.24678D-18 | 1.53141D+00 |
| Q( 0) | 4 - 4 | 3776.11 | 0.00 | 0.00000D+00 | 1.00000D+00 | 7.99478D-01 |
| Q( 1) | 4 - 0 | 453.51 | -3323.67 | 0.00000D+00 | 4.35047D-21 | -1.79693D-01 |
| Q( 1) | 4 - 1 | 1337.79 | -2439.38 | 0.00000D+00 | 4.37117D-21 | -2.51478D-01 |
| Q( 1) | 4 - 2 | 2195.17 | -1582.01 | 0.00000D+00 | 1.55966D-18 | 5.09622D-01 |
| Q( 1) | 4 - 3 | 3005.79 | -771.38 | 0.00000D+00 | 3.68784D-17 | 1.53142D+00 |
| Q( 1) | 4 - 4 | 3777.18 | -0.00 | 0.00000D+00 | 1.00000D+00 | 7.99522D-01 |
| Q( 2) | 4 - 0 | 455.67 | -3323.64 | 0.00000D+00 | 1.40197D-26 | -1.79698D-01 |
| Q( 2) | 4 - 1 | 1339.93 | -2439.38 | 0.00000D+00 | 5.87574D-20 | -2.51624D-01 |
| Q( 2) | 4 - 2 | 2197.29 | -1582.02 | 0.00000D+00 | 3.08355D-24 | 5.09420D-01 |
| Q( 2) | 4 - 3 | 3007.92 | -771.39 | 0.00000D+00 | 4.01002D-19 | 1.53143D+00 |
| Q( 2) | 4 - 4 | 3779.31 | 0.00 | 0.00000D+00 | 1.00000D+00 | 7.99610D-01 |
| Q( 3) | 4 - 0 | 458.91 | -3323.59 | 0.00000D+00 | 1.40420D-26 | -1.79707D-01 |
| Q( 3) | 4 - 1 | 1343.12 | -2439.38 | 0.00000D+00 | 5.88997D-20 | -2.51843D-01 |
| Q( 3) | 4 - 2 | 2200.47 | -1582.03 | 0.00000D+00 | 3.04638D-24 | 5.09117D-01 |
| Q( 3) | 4 - 3 | 3011.10 | -771.40 | 0.00000D+00 | 4.00187D-19 | 1.53145D+00 |
| Q( 3) | 4 - 4 | 3782.50 | 0.00 | 0.00000D+00 | 1.00000D+00 | 7.99741D-01 |
| Q( 4) | 4 - 0 | 463.24 | -3323.52 | 0.00000D+00 | 1.41489D-26 | -1.79719D-01 |
| Q( 4) | 4 - 1 | 1347.39 | -2439.37 | 0.00000D+00 | 5.90852D-20 | -2.52135D-01 |
| Q( 4) | 4 - 2 | 2204.71 | -1582.04 | 0.00000D+00 | 3.03289D-24 | 5.08714D-01 |
| Q( 4) | 4 - 3 | 3015.34 | -771.41 | 0.00000D+00 | 3.99091D-19 | 1.53148D+00 |
| Q( 4) | 4 - 4 | 3786.76 | 0.00 | 0.00000D+00 | 1.00000D+00 | 7.99916D-01 |
| Q( 5) | 4 - 0 | 468.64 | -3323.44 | 0.00000D+00 | 1.40072D-26 | -1.79733D-01 |
| Q( 5) | 4 - 1 | 1352.72 | -2439.36 | 0.00000D+00 | 5.93193D-20 | -2.52499D-01 |
| Q( 5) | 4 - 2 | 2210.02 | -1582.06 | 0.00000D+00 | 2.91361D-24 | 5.08209D-01 |
| Q( 5) | 4 - 3 | 3020.65 | -771.43 | 0.00000D+00 | 3.97799D-19 | 1.53151D+00 |
| Q( 5) | 4 - 4 | 3792.08 | 0.00 | 0.00000D+00 | 1.00000D+00 | 8.00135D-01 |
| Q( 6) | 4 - 0 | 475.12 | -3323.34 | 0.00000D+00 | 1.43343D-26 | -1.79750D-01 |

| | | | | | | |
|---|---|---|---|---|---|---|
| Q( 6) | 4 - 1 | 1359.11 | -2439.35 | 0.00000D+00 | 5.95976D-20 | -2.52937D-01 |
| Q( 6) | 4 - 2 | 2216.38 | -1582.08 | 0.00000D+00 | 2.74903D-24 | 5.07603D-01 |
| Q( 6) | 4 - 3 | 3027.01 | -771.45 | 0.00000D+00 | 3.96291D-19 | 1.53156D+00 |
| Q( 6) | 4 - 4 | 3798.46 | 0.00 | 0.00000D+00 | 1.00000D+00 | 8.00396D-01 |
| Q( 7) | 4 - 0 | 482.69 | -3323.23 | 0.00000D+00 | 1.54222D-26 | -1.79769D-01 |
| Q( 7) | 4 - 1 | 1366.57 | -2439.34 | 0.00000D+00 | 5.99218D-20 | -2.53447D-01 |
| Q( 7) | 4 - 2 | 2223.80 | -1582.11 | 0.00000D+00 | 2.53293D-24 | 5.06895D-01 |
| Q( 7) | 4 - 3 | 3034.44 | -771.47 | 0.00000D+00 | 3.94639D-19 | 1.53160D+00 |
| Q( 7) | 4 - 4 | 3805.91 | 0.00 | 0.00000D+00 | 1.00000D+00 | 8.00700D-01 |
| Q( 8) | 4 - 0 | 491.33 | -3323.09 | 0.00000D+00 | 1.60457D-26 | -1.79790D-01 |
| Q( 8) | 4 - 1 | 1375.10 | -2439.33 | 0.00000D+00 | 6.02897D-20 | -2.54029D-01 |
| Q( 8) | 4 - 2 | 2232.29 | -1582.14 | 0.00000D+00 | 2.30071D-24 | 5.06086D-01 |
| Q( 8) | 4 - 3 | 3042.93 | -771.50 | 0.00000D+00 | 3.92851D-19 | 1.53166D+00 |
| Q( 8) | 4 - 4 | 3814.43 | 0.00 | 0.00000D+00 | 1.00000D+00 | 8.01047D-01 |
| Q( 9) | 4 - 0 | 501.06 | -3322.94 | 0.00000D+00 | 1.72952D-26 | -1.79814D-01 |
| Q( 9) | 4 - 1 | 1384.69 | -2439.32 | 0.00000D+00 | 6.07048D-20 | -2.54684D-01 |
| Q( 9) | 4 - 2 | 2241.83 | -1582.17 | 0.00000D+00 | 1.92972D-24 | 5.05174D-01 |
| Q( 9) | 4 - 3 | 3052.47 | -771.53 | 0.00000D+00 | 3.90978D-19 | 1.53171D+00 |
| Q( 9) | 4 - 4 | 3824.00 | 0.00 | 0.00000D+00 | 1.00000D+00 | 8.01436D-01 |
| Q( 10) | 4 - 0 | 511.86 | -3322.78 | 0.00000D+00 | 1.85982D-26 | -1.79839D-01 |
| Q( 10) | 4 - 1 | 1395.34 | -2439.30 | 0.00000D+00 | 6.11588D-20 | -2.55410D-01 |
| Q( 10) | 4 - 2 | 2252.43 | -1582.21 | 0.00000D+00 | 1.53554D-24 | 5.04160D-01 |
| Q( 10) | 4 - 3 | 3063.08 | -771.56 | 0.00000D+00 | 3.89104D-19 | 1.53178D+00 |
| Q( 10) | 4 - 4 | 3834.64 | 0.00 | 0.00000D+00 | 1.00000D+00 | 8.01866D-01 |
| Q( 11) | 4 - 0 | 523.75 | -3322.59 | 0.00000D+00 | 2.19054D-26 | -1.79865D-01 |
| Q( 11) | 4 - 1 | 1407.06 | -2439.28 | 0.00000D+00 | 6.16533D-20 | -2.56209D-01 |
| Q( 11) | 4 - 2 | 2264.10 | -1582.25 | 0.00000D+00 | 1.06499D-24 | 5.03044D-01 |
| Q( 11) | 4 - 3 | 3074.74 | -771.60 | 0.00000D+00 | 3.87210D-19 | 1.53184D+00 |
| Q( 11) | 4 - 4 | 3846.34 | 0.00 | 0.00000D+00 | 1.00000D+00 | 8.02338D-01 |

| | | | | | | | |
|---|---|---|---|---|---|---|---|
| Q( 12) | 4 - 0 | 536.71 | -3322.39 | 0.00000D+00 | 2.52658D-26 | -1.79893D-01 |
| Q( 12) | 4 - 1 | 1419.85 | -2439.26 | 0.00000D+00 | 5.27852D-20 | -2.57080D-01 |
| Q( 12) | 4 - 2 | 2276.82 | -1582.29 | 0.00000D+00 | 6.16225D-25 | 5.01824D-01 |
| Q( 12) | 4 - 3 | 3087.47 | -771.64 | 0.00000D+00 | 3.85447D-19 | 1.53192D+00 |
| Q( 12) | 4 - 4 | 3859.11 | 0.00 | 0.00000D+00 | 1.00000D+00 | 8.02850D-01 |
| Q( 13) | 4 - 0 | 550.76 | -3322.17 | 0.00000D+00 | 3.61861D-26 | -1.79921D-01 |
| Q( 13) | 4 - 1 | 1433.69 | -2439.24 | 0.00000D+00 | 5.33453D-20 | -2.58021D-01 |
| Q( 13) | 4 - 2 | 2290.60 | -1582.33 | 0.00000D+00 | 2.59432D-26 | 5.00501D-01 |
| Q( 13) | 4 - 3 | 3101.25 | -771.68 | 0.00000D+00 | 3.85380D-19 | 1.53199D+00 |
| Q( 13) | 4 - 4 | 3872.93 | 0.00 | 0.00000D+00 | 1.00000D+00 | 8.03402D-01 |
| Q( 14) | 4 - 0 | 565.88 | -3321.94 | 0.00000D+00 | 4.46383D-26 | -1.79950D-01 |
| Q( 14) | 4 - 1 | 1448.61 | -2439.21 | 0.00000D+00 | 5.39770D-20 | -2.59034D-01 |
| Q( 14) | 4 - 2 | 2305.44 | -1582.38 | 0.00000D+00 | 4.55928D-26 | 4.99074D-01 |
| Q( 14) | 4 - 3 | 3116.09 | -771.73 | 0.00000D+00 | 3.93813D-19 | 1.53207D+00 |
| Q( 14) | 4 - 4 | 3887.82 | 0.00 | 0.00000D+00 | 1.00000D+00 | 8.03993D-01 |
| Q( 15) | 4 - 0 | 582.08 | -3321.68 | 0.00000D+00 | 5.65584D-26 | -1.79978D-01 |
| Q( 15) | 4 - 1 | 1464.58 | -2439.18 | 0.00000D+00 | 5.46498D-20 | -2.60118D-01 |
| Q( 15) | 4 - 2 | 2321.33 | -1582.43 | 0.00000D+00 | 5.41059D-25 | 4.97543D-01 |
| Q( 15) | 4 - 3 | 3131.99 | -771.77 | 0.00000D+00 | 3.92853D-19 | 1.53214D+00 |
| Q( 15) | 4 - 4 | 3903.76 | 0.00 | 0.00000D+00 | 1.00000D+00 | 8.04623D-01 |
| Q( 16) | 4 - 0 | 599.36 | -3321.41 | 0.00000D+00 | 7.32176D-26 | -1.80007D-01 |
| Q( 16) | 4 - 1 | 1481.62 | -2439.14 | 0.00000D+00 | 5.53601D-20 | -2.61273D-01 |
| Q( 16) | 4 - 2 | 2338.29 | -1582.48 | 0.00000D+00 | 1.85807D-24 | 4.95907D-01 |
| Q( 16) | 4 - 3 | 3148.94 | -771.82 | 0.00000D+00 | 3.92321D-19 | 1.53222D+00 |
| Q( 16) | 4 - 4 | 3920.77 | 0.00 | 0.00000D+00 | 1.00000D+00 | 8.05291D-01 |
| Q( 17) | 4 - 0 | 617.72 | -3321.11 | 0.00000D+00 | 1.02336D-25 | -1.80034D-01 |
| Q( 17) | 4 - 1 | 1499.73 | -2439.10 | 0.00000D+00 | 5.61091D-20 | -2.62498D-01 |
| Q( 17) | 4 - 2 | 2356.30 | -1582.53 | 0.00000D+00 | 4.45395D-24 | 4.94166D-01 |
| Q( 17) | 4 - 3 | 3166.96 | -771.88 | 0.00000D+00 | 3.92278D-19 | 1.53230D+00 |

| | | | | | | |
|---|---|---|---|---|---|---|
| Q( 17) | 4 - 4 | 3938.83 | 0.00 | 0.00000D+00 | 1.00000D+00 | 8.05996D-01 |
| Q( 18) | 4 - 0 | 637.15 | -3320.80 | 0.00000D+00 | 1.32750D-25 | -1.80060D-01 |
| Q( 18) | 4 - 1 | 1518.89 | -2439.06 | 0.00000D+00 | 5.68925D-20 | -2.63793D-01 |
| Q( 18) | 4 - 2 | 2375.37 | -1582.59 | 0.00000D+00 | 8.78143D-24 | 4.92319D-01 |
| Q( 18) | 4 - 3 | 3186.03 | -771.93 | 0.00000D+00 | 3.92815D-19 | 1.53238D+00 |
| Q( 18) | 4 - 4 | 3957.95 | 0.00 | 0.00000D+00 | 1.00000D+00 | 8.06737D-01 |
| Q( 19) | 4 - 0 | 657.67 | -3320.47 | 0.00000D+00 | 1.69612D-25 | -1.80084D-01 |
| Q( 19) | 4 - 1 | 1539.12 | -2439.01 | 0.00000D+00 | 5.77126D-20 | -2.65158D-01 |
| Q( 19) | 4 - 2 | 2395.49 | -1582.65 | 0.00000D+00 | 1.59215D-23 | 4.90365D-01 |
| Q( 19) | 4 - 3 | 3206.15 | -771.99 | 0.00000D+00 | 3.94018D-19 | 1.53245D+00 |
| Q( 19) | 4 - 4 | 3978.14 | 0.00 | 0.00000D+00 | 1.00000D+00 | 8.07513D-01 |
| Q( 20) | 4 - 0 | 679.26 | -3320.12 | 0.00000D+00 | 2.23243D-25 | -1.80106D-01 |
| Q( 20) | 4 - 1 | 1560.41 | -2438.96 | 0.00000D+00 | 5.85628D-20 | -2.66591D-01 |
| Q( 20) | 4 - 2 | 2416.67 | -1582.71 | 0.00000D+00 | 2.65657D-23 | 4.88304D-01 |
| Q( 20) | 4 - 3 | 3227.33 | -772.04 | 0.00000D+00 | 3.96021D-19 | 1.53253D+00 |
| Q( 20) | 4 - 4 | 3999.37 | 0.00 | 0.00000D+00 | 1.00000D+00 | 8.08324D-01 |
| Q( 0) | 5 - 0 | 452.43 | -4054.15 | 0.00000D+00 | 2.26978D-24 | -1.12467D-02 |
| Q( 0) | 5 - 1 | 1336.73 | -3169.85 | 0.00000D+00 | 2.16204D-19 | 2.56284D-01 |
| Q( 0) | 5 - 2 | 2194.11 | -2312.47 | 0.00000D+00 | 8.33739D-22 | 4.27618D-01 |
| Q( 0) | 5 - 3 | 3004.73 | -1501.85 | 0.00000D+00 | 3.28427D-20 | -3.49418D-01 |
| Q( 0) | 5 - 4 | 3776.11 | -730.47 | 0.00000D+00 | 2.88521D-18 | -1.36760D+00 |
| Q( 0) | 5 - 5 | 4506.58 | 0.00 | 0.00000D+00 | 1.00000D+00 | -6.64349D-01 |
| Q( 1) | 5 - 0 | 453.51 | -4054.14 | 0.00000D+00 | 3.54351D-22 | -1.12805D-02 |
| Q( 1) | 5 - 1 | 1337.79 | -3169.86 | 0.00000D+00 | 3.06353D-19 | 2.56266D-01 |
| Q( 1) | 5 - 2 | 2195.17 | -2312.49 | 0.00000D+00 | 1.65286D-19 | 4.27714D-01 |
| Q( 1) | 5 - 3 | 3005.79 | -1501.86 | 0.00000D+00 | 1.68861D-18 | -3.49278D-01 |
| Q( 1) | 5 - 4 | 3777.18 | -730.48 | 0.00000D+00 | 6.65891D-17 | -1.36758D+00 |
| Q( 1) | 5 - 5 | 4507.65 | -0.00 | 0.00000D+00 | 1.00000D+00 | -6.64358D-01 |
| Q( 2) | 5 - 0 | 455.67 | -4054.13 | 0.00000D+00 | 3.53343D-26 | -1.13481D-02 |

| | | | | | | | |
|---|---|---|---|---|---|---|---|
| Q( 2) | 5 - 1 | 1339.93 | -3169.87 | 0.00000D+00 | 2.09594D-19 | 2.56230D-01 |
| Q( 2) | 5 - 2 | 2197.29 | -2312.51 | 0.00000D+00 | 1.52182D-26 | 4.27905D-01 |
| Q( 2) | 5 - 3 | 3007.92 | -1501.88 | 0.00000D+00 | 8.61198D-20 | -3.49000D-01 |
| Q( 2) | 5 - 4 | 3779.31 | -730.49 | 0.00000D+00 | 1.45246D-18 | -1.36753D+00 |
| Q( 2) | 5 - 5 | 4509.80 | 0.00 | 0.00000D+00 | 1.00000D+00 | -6.64375D-01 |
| Q( 3) | 5 - 0 | 458.91 | -4054.11 | 0.00000D+00 | 3.50780D-26 | -1.14495D-02 |
| Q( 3) | 5 - 1 | 1343.12 | -3169.90 | 0.00000D+00 | 2.09219D-19 | 2.56175D-01 |
| Q( 3) | 5 - 2 | 2200.47 | -2312.55 | 0.00000D+00 | 1.55951D-26 | 4.28191D-01 |
| Q( 3) | 5 - 3 | 3011.10 | -1501.92 | 0.00000D+00 | 8.58336D-20 | -3.48582D-01 |
| Q( 3) | 5 - 4 | 3782.50 | -730.52 | 0.00000D+00 | 1.44903D-18 | -1.36746D+00 |
| Q( 3) | 5 - 5 | 4513.02 | 0.00 | 0.00000D+00 | 1.00000D+00 | -6.64400D-01 |
| Q( 4) | 5 - 0 | 463.24 | -4054.08 | 0.00000D+00 | 3.61646D-26 | -1.15846D-02 |
| Q( 4) | 5 - 1 | 1347.39 | -3169.93 | 0.00000D+00 | 2.08722D-19 | 2.56102D-01 |
| Q( 4) | 5 - 2 | 2204.71 | -2312.60 | 0.00000D+00 | 1.88832D-26 | 4.28572D-01 |
| Q( 4) | 5 - 3 | 3015.34 | -1501.97 | 0.00000D+00 | 8.54594D-20 | -3.48024D-01 |
| Q( 4) | 5 - 4 | 3786.76 | -730.56 | 0.00000D+00 | 1.44443D-18 | -1.36737D+00 |
| Q( 4) | 5 - 5 | 4517.32 | 0.00 | 0.00000D+00 | 1.00000D+00 | -6.64434D-01 |
| Q( 5) | 5 - 0 | 468.64 | -4054.05 | 0.00000D+00 | 3.61020D-26 | -1.17535D-02 |
| Q( 5) | 5 - 1 | 1352.72 | -3169.97 | 0.00000D+00 | 2.08106D-19 | 2.56011D-01 |
| Q( 5) | 5 - 2 | 2210.02 | -2312.67 | 0.00000D+00 | 1.97886D-26 | 4.29049D-01 |
| Q( 5) | 5 - 3 | 3020.65 | -1502.04 | 0.00000D+00 | 8.49912D-20 | -3.47327D-01 |
| Q( 5) | 5 - 4 | 3792.08 | -730.61 | 0.00000D+00 | 1.43881D-18 | -1.36725D+00 |
| Q( 5) | 5 - 5 | 4522.69 | 0.00 | 0.00000D+00 | 1.00000D+00 | -6.64475D-01 |
| Q( 6) | 5 - 0 | 475.12 | -4054.00 | 0.00000D+00 | 3.57868D-26 | -1.19562D-02 |
| Q( 6) | 5 - 1 | 1359.11 | -3170.02 | 0.00000D+00 | 2.07369D-19 | 2.55901D-01 |
| Q( 6) | 5 - 2 | 2216.38 | -2312.75 | 0.00000D+00 | 2.47893D-26 | 4.29620D-01 |
| Q( 6) | 5 - 3 | 3027.01 | -1502.11 | 0.00000D+00 | 8.44195D-20 | -3.46491D-01 |
| Q( 6) | 5 - 4 | 3798.46 | -730.66 | 0.00000D+00 | 1.43233D-18 | -1.36711D+00 |
| Q( 6) | 5 - 5 | 4529.13 | 0.00 | 0.00000D+00 | 1.00000D+00 | -6.64525D-01 |

| | | | | | | |
|---|---|---|---|---|---|---|
| Q( 7) | 5 - 0 | 482.69 | -4053.95 | 0.00000D+00 | 3.70388D-26 | -1.21926D-02 |
| Q( 7) | 5 - 1 | 1366.57 | -3170.07 | 0.00000D+00 | 2.06513D-19 | 2.55772D-01 |
| Q( 7) | 5 - 2 | 2223.80 | -2312.84 | 0.00000D+00 | 3.44117D-26 | 4.30286D-01 |
| Q( 7) | 5 - 3 | 3034.44 | -1502.20 | 0.00000D+00 | 8.37512D-20 | -3.45515D-01 |
| Q( 7) | 5 - 4 | 3805.91 | -730.73 | 0.00000D+00 | 1.42516D-18 | -1.36694D+00 |
| Q( 7) | 5 - 5 | 4536.64 | 0.00 | 0.00000D+00 | 1.00000D+00 | -6.64582D-01 |
| Q( 8) | 5 - 0 | 491.33 | -4053.90 | 0.00000D+00 | 3.73270D-26 | -1.24627D-02 |
| Q( 8) | 5 - 1 | 1375.10 | -3170.13 | 0.00000D+00 | 2.05553D-19 | 2.55624D-01 |
| Q( 8) | 5 - 2 | 2232.29 | -2312.94 | 0.00000D+00 | 4.77341D-26 | 4.31046D-01 |
| Q( 8) | 5 - 3 | 3042.93 | -1502.30 | 0.00000D+00 | 8.29769D-20 | -3.44399D-01 |
| Q( 8) | 5 - 4 | 3814.43 | -730.80 | 0.00000D+00 | 1.41735D-18 | -1.36675D+00 |
| Q( 8) | 5 - 5 | 4545.23 | 0.00 | 0.00000D+00 | 1.00000D+00 | -6.64646D-01 |
| Q( 9) | 5 - 0 | 501.06 | -4053.83 | 0.00000D+00 | 3.86889D-26 | -1.27665D-02 |
| Q( 9) | 5 - 1 | 1384.69 | -3170.20 | 0.00000D+00 | 2.04478D-19 | 2.55457D-01 |
| Q( 9) | 5 - 2 | 2241.83 | -2313.06 | 0.00000D+00 | 6.97510D-26 | 4.31900D-01 |
| Q( 9) | 5 - 3 | 3052.47 | -1502.42 | 0.00000D+00 | 8.20951D-20 | -3.43144D-01 |
| Q( 9) | 5 - 4 | 3824.00 | -730.89 | 0.00000D+00 | 1.40904D-18 | -1.36653D+00 |
| Q( 9) | 5 - 5 | 4554.89 | 0.00 | 0.00000D+00 | 1.00000D+00 | -6.64717D-01 |
| Q( 10) | 5 - 0 | 511.86 | -4053.76 | 0.00000D+00 | 3.82604D-26 | -1.31040D-02 |
| Q( 10) | 5 - 1 | 1395.34 | -3170.28 | 0.00000D+00 | 2.03300D-19 | 2.55270D-01 |
| Q( 10) | 5 - 2 | 2252.43 | -2313.19 | 0.00000D+00 | 1.10448D-25 | 4.32847D-01 |
| Q( 10) | 5 - 3 | 3063.08 | -1502.54 | 0.00000D+00 | 8.11124D-20 | -3.41749D-01 |
| Q( 10) | 5 - 4 | 3834.64 | -730.98 | 0.00000D+00 | 1.40056D-18 | -1.36629D+00 |
| Q( 10) | 5 - 5 | 4565.62 | 0.00 | 0.00000D+00 | 1.00000D+00 | -6.64794D-01 |
| Q( 11) | 5 - 0 | 523.75 | -4053.67 | 0.00000D+00 | 4.14079D-26 | -1.34751D-02 |
| Q( 11) | 5 - 1 | 1407.06 | -3170.36 | 0.00000D+00 | 2.02020D-19 | 2.55063D-01 |
| Q( 11) | 5 - 2 | 2264.10 | -2313.32 | 0.00000D+00 | 1.77806D-25 | 4.33887D-01 |
| Q( 11) | 5 - 3 | 3074.74 | -1502.68 | 0.00000D+00 | 8.00052D-20 | -3.40214D-01 |
| Q( 11) | 5 - 4 | 3846.34 | -731.08 | 0.00000D+00 | 1.39213D-18 | -1.36602D+00 |

| | | | | | | | |
|---|---|---|---|---|---|---|---|
| Q( 11) | 5 - 5 | 4577.42 | 0.00 | 0.00000D+00 | 1.00000D+00 | -6.64877D-01 |
| Q( 12) | 5 - 0 | 536.71 | -4053.58 | 0.00000D+00 | 4.41334D-26 | -1.38797D-02 |
| Q( 12) | 5 - 1 | 1419.85 | -3170.45 | 0.00000D+00 | 2.08647D-19 | 2.54836D-01 |
| Q( 12) | 5 - 2 | 2276.82 | -2313.48 | 0.00000D+00 | 2.90058D-25 | 4.35020D-01 |
| Q( 12) | 5 - 3 | 3087.47 | -1502.83 | 0.00000D+00 | 7.87871D-20 | -3.38539D-01 |
| Q( 12) | 5 - 4 | 3859.11 | -731.19 | 0.00000D+00 | 1.38388D-18 | -1.36572D+00 |
| Q( 12) | 5 - 5 | 4590.29 | 0.00 | 0.00000D+00 | 1.00000D+00 | -6.64966D-01 |
| Q( 13) | 5 - 0 | 550.76 | -4053.48 | 0.00000D+00 | 4.67616D-26 | -1.43179D-02 |
| Q( 13) | 5 - 1 | 1433.69 | -3170.54 | 0.00000D+00 | 2.07199D-19 | 2.54589D-01 |
| Q( 13) | 5 - 2 | 2290.60 | -2313.64 | 0.00000D+00 | 4.65231D-25 | 4.36245D-01 |
| Q( 13) | 5 - 3 | 3101.25 | -1502.99 | 0.00000D+00 | 7.74356D-20 | -3.36724D-01 |
| Q( 13) | 5 - 4 | 3872.93 | -731.31 | 0.00000D+00 | 1.40774D-18 | -1.36540D+00 |
| Q( 13) | 5 - 5 | 4604.24 | 0.00 | 0.00000D+00 | 1.00000D+00 | -6.65059D-01 |
| Q( 14) | 5 - 0 | 565.88 | -4053.37 | 0.00000D+00 | 5.13414D-26 | -1.47896D-02 |
| Q( 14) | 5 - 1 | 1448.61 | -3170.64 | 0.00000D+00 | 2.05694D-19 | 2.54320D-01 |
| Q( 14) | 5 - 2 | 2305.44 | -2313.81 | 0.00000D+00 | 1.03755D-24 | 4.37560D-01 |
| Q( 14) | 5 - 3 | 3116.09 | -1503.16 | 0.00000D+00 | 8.10772D-20 | -3.34769D-01 |
| Q( 14) | 5 - 4 | 3887.82 | -731.43 | 0.00000D+00 | 1.40396D-18 | -1.36504D+00 |
| Q( 14) | 5 - 5 | 4619.25 | 0.00 | 0.00000D+00 | 1.00000D+00 | -6.65157D-01 |
| Q( 15) | 5 - 0 | 582.08 | -4053.25 | 0.00000D+00 | 5.85210D-26 | -1.52947D-02 |
| Q( 15) | 5 - 1 | 1464.58 | -3170.75 | 0.00000D+00 | 2.04093D-19 | 2.54029D-01 |
| Q( 15) | 5 - 2 | 2321.33 | -2314.00 | 0.00000D+00 | 1.56912D-24 | 4.38967D-01 |
| Q( 15) | 5 - 3 | 3131.99 | -1503.34 | 0.00000D+00 | 7.93750D-20 | -3.32674D-01 |
| Q( 15) | 5 - 4 | 3903.76 | -731.57 | 0.00000D+00 | 1.39818D-18 | -1.36466D+00 |
| Q( 15) | 5 - 5 | 4635.33 | 0.00 | 0.00000D+00 | 1.00000D+00 | -6.65257D-01 |
| Q( 16) | 5 - 0 | 599.36 | -4053.12 | 0.00000D+00 | 6.46109D-26 | -1.58331D-02 |
| Q( 16) | 5 - 1 | 1481.62 | -3170.85 | 0.00000D+00 | 2.02425D-19 | 2.53717D-01 |
| Q( 16) | 5 - 2 | 2338.29 | -2314.19 | 0.00000D+00 | 2.37554D-24 | 4.40463D-01 |
| Q( 16) | 5 - 3 | 3148.94 | -1503.53 | 0.00000D+00 | 7.75187D-20 | -3.30438D-01 |

| | | | | | | |
|---|---|---|---|---|---|---|
| Q( 16) | 5 - 4 | 3920.77 | -731.71 | 0.00000D+00 | 1.39380D-18 | -1.36425D+00 |
| Q( 16) | 5 - 5 | 4652.48 | 0.00 | 0.00000D+00 | 1.00000D+00 | -6.65361D-01 |
| Q( 17) | 5 - 0 | 617.72 | -4052.98 | 0.00000D+00 | 7.39970D-26 | -1.64049D-02 |
| Q( 17) | 5 - 1 | 1499.73 | -3170.97 | 0.00000D+00 | 2.00693D-19 | 2.53381D-01 |
| Q( 17) | 5 - 2 | 2356.30 | -2314.40 | 0.00000D+00 | 3.55665D-24 | 4.42048D-01 |
| Q( 17) | 5 - 3 | 3166.96 | -1503.74 | 0.00000D+00 | 7.55157D-20 | -3.28061D-01 |
| Q( 17) | 5 - 4 | 3938.83 | -731.86 | 0.00000D+00 | 1.39120D-18 | -1.36380D+00 |
| Q( 17) | 5 - 5 | 4670.69 | 0.00 | 0.00000D+00 | 1.00000D+00 | -6.65467D-01 |
| Q( 18) | 5 - 0 | 637.15 | -4052.82 | 0.00000D+00 | 8.32344D-26 | -1.70098D-02 |
| Q( 18) | 5 - 1 | 1518.89 | -3171.08 | 0.00000D+00 | 1.98907D-19 | 2.53023D-01 |
| Q( 18) | 5 - 2 | 2375.37 | -2314.61 | 0.00000D+00 | 5.29593D-24 | 4.43721D-01 |
| Q( 18) | 5 - 3 | 3186.03 | -1503.95 | 0.00000D+00 | 7.33639D-20 | -3.25543D-01 |
| Q( 18) | 5 - 4 | 3957.95 | -732.02 | 0.00000D+00 | 1.39071D-18 | -1.36332D+00 |
| Q( 18) | 5 - 5 | 4689.98 | 0.00 | 0.00000D+00 | 1.00000D+00 | -6.65573D-01 |
| Q( 19) | 5 - 0 | 657.67 | -4052.66 | 0.00000D+00 | 1.03308D-25 | -1.76478D-02 |
| Q( 19) | 5 - 1 | 1539.12 | -3171.20 | 0.00000D+00 | 1.97106D-19 | 2.52641D-01 |
| Q( 19) | 5 - 2 | 2395.49 | -2314.83 | 0.00000D+00 | 8.66393D-24 | 4.45483D-01 |
| Q( 19) | 5 - 3 | 3206.15 | -1504.17 | 0.00000D+00 | 7.07613D-20 | -3.22885D-01 |
| Q( 19) | 5 - 4 | 3978.14 | -732.19 | 0.00000D+00 | 1.39750D-18 | -1.36281D+00 |
| Q( 19) | 5 - 5 | 4710.32 | 0.00 | 0.00000D+00 | 1.00000D+00 | -6.65680D-01 |
| Q( 20) | 5 - 0 | 679.26 | -4052.48 | 0.00000D+00 | 1.22179D-25 | -1.83189D-02 |
| Q( 20) | 5 - 1 | 1560.41 | -3171.32 | 0.00000D+00 | 1.95236D-19 | 2.52235D-01 |
| Q( 20) | 5 - 2 | 2416.67 | -2315.07 | 0.00000D+00 | 1.23391D-23 | 4.47330D-01 |
| Q( 20) | 5 - 3 | 3227.33 | -1504.41 | 0.00000D+00 | 6.82763D-20 | -3.20085D-01 |
| Q( 20) | 5 - 4 | 3999.37 | -732.36 | 0.00000D+00 | 1.40259D-18 | -1.36226D+00 |
| Q( 20) | 5 - 5 | 4731.74 | 0.00 | 0.00000D+00 | 1.00000D+00 | -6.65786D-01 |
