# Supplementary material for: Ab initio spectroscopic studies of AlF and AlCl molecules
Source: arXiv:2303.08681 source file (2023-03-15)
Supplement: Supplementary file 9 [file AlF_triplet_sigma_-_S10.pdf]

# AlF $b^3\Sigma$: Rotational parameters

Note that (v',J') & (v",J") strictly label the upper and lower levels, resp., and E(lower)=E"

but E(2)-E(1) is: (energy of State-2 level) - (energy of State-1 level)

In the following table, E is expressed in $cm^{-1}$, A in $s^{-1}$ and transition dipole moment in debye.

| dJ(J") | Band v' v" | E(lower) | E(2)-E(1) | A(Einstein) | F-C Factor | <v'j'\|M\|v"j"> |
|---|---|---|---|---|---|---|
| R( 0) | 0 - 0 | 360.72 | -1.09 | 4.02402D-07 | 1.00000D+00 | -1.71343D+00 |
| R( 1) | 0 - 0 | 361.81 | -2.19 | 3.86292D-06 | 1.00000D+00 | -1.71345D+00 |
| R( 2) | 0 - 0 | 364.00 | -3.28 | 1.39681D-05 | 1.00000D+00 | -1.71347D+00 |
| R( 3) | 0 - 0 | 367.29 | -4.38 | 3.43342D-05 | 1.00000D+00 | -1.71351D+00 |
| R( 4) | 0 - 0 | 371.66 | -5.47 | 6.85787D-05 | 1.00000D+00 | -1.71356D+00 |
| R( 5) | 0 - 0 | 377.14 | -6.57 | 1.20318D-04 | 1.00000D+00 | -1.71362D+00 |
| R( 6) | 0 - 0 | 383.70 | -7.66 | 1.93166D-04 | 1.00000D+00 | -1.71369D+00 |
| R( 7) | 0 - 0 | 391.36 | -8.75 | 2.90733D-04 | 1.00000D+00 | -1.71377D+00 |
| R( 8) | 0 - 0 | 400.12 | -9.85 | 4.16627D-04 | 9.99999D-01 | -1.71387D+00 |
| R( 9) | 0 - 0 | 409.96 | -10.94 | 5.74452D-04 | 9.99999D-01 | -1.71397D+00 |
| R( 10) | 0 - 0 | 420.90 | -12.03 | 7.67807D-04 | 9.99999D-01 | -1.71408D+00 |
| R( 11) | 0 - 0 | 432.94 | -13.13 | 1.00028D-03 | 9.99999D-01 | -1.71421D+00 |
| R( 12) | 0 - 0 | 446.06 | -14.22 | 1.27548D-03 | 9.99999D-01 | -1.71435D+00 |
| R( 13) | 0 - 0 | 460.28 | -15.31 | 1.59696D-03 | 9.99999D-01 | -1.71450D+00 |
| R( 14) | 0 - 0 | 475.59 | -16.40 | 1.96832D-03 | 9.99998D-01 | -1.71465D+00 |
| R( 15) | 0 - 0 | 491.99 | -17.49 | 2.39311D-03 | 9.99998D-01 | -1.71482D+00 |
| R( 16) | 0 - 0 | 509.48 | -18.58 | 2.87490D-03 | 9.99998D-01 | -1.71501D+00 |
| R( 17) | 0 - 0 | 528.06 | -19.67 | 3.41725D-03 | 9.99998D-01 | -1.71520D+00 |
| R( 18) | 0 - 0 | 547.74 | -20.76 | 4.02370D-03 | 9.99998D-01 | -1.71540D+00 |

| | | | | | | |
|---|---|---|---|---|---|---|
| R( 19) | 0 - 0 | 568.50 | -21.85 | 4.69778D-03 | 9.99997D-01 | -1.71562D+00 |
| P( 1) | 1 - 0 | 361.81 | -724.30 | 5.35099D-01 | 6.67517D-09 | 6.70092D-02 |
| R( 0) | 1 - 0 | 360.72 | -726.48 | 1.78466D-01 | 6.67557D-09 | 6.67273D-02 |
| P( 2) | 1 - 0 | 364.00 | -723.19 | 3.56622D-01 | 2.67013D-08 | 6.71531D-02 |
| R( 0) | 1 - 1 | 1086.12 | -1.08 | 3.99772D-07 | 1.00000D+00 | 1.74370D+00 |
| R( 1) | 1 - 0 | 361.81 | -727.54 | 2.14213D-01 | 2.67015D-08 | 6.65893D-02 |
| P( 3) | 1 - 0 | 367.29 | -722.07 | 3.20855D-01 | 6.00863D-08 | 6.72990D-02 |
| R( 1) | 1 - 1 | 1087.20 | -2.16 | 3.83769D-06 | 1.00000D+00 | 1.74371D+00 |
| R( 2) | 1 - 0 | 364.00 | -728.59 | 2.29567D-01 | 6.00835D-08 | 6.64532D-02 |
| P( 4) | 1 - 0 | 371.66 | -720.93 | 3.05470D-01 | 1.06835D-07 | 6.74469D-02 |
| R( 2) | 1 - 1 | 1089.36 | -3.24 | 1.38769D-05 | 1.00000D+00 | 1.74374D+00 |
| R( 3) | 1 - 0 | 367.29 | -729.63 | 2.38121D-01 | 1.06828D-07 | 6.63191D-02 |
| P( 5) | 1 - 0 | 377.14 | -719.78 | 2.96876D-01 | 1.66958D-07 | 6.75968D-02 |
| R( 3) | 1 - 1 | 1092.59 | -4.32 | 3.41102D-05 | 1.00000D+00 | 1.74378D+00 |
| R( 4) | 1 - 0 | 371.66 | -730.64 | 2.43581D-01 | 1.66945D-07 | 6.61869D-02 |
| P( 6) | 1 - 0 | 383.70 | -718.61 | 2.91365D-01 | 2.40470D-07 | 6.77488D-02 |
| R( 4) | 1 - 1 | 1096.91 | -5.40 | 6.81318D-05 | 1.00000D+00 | 1.74383D+00 |
| R( 5) | 1 - 0 | 377.14 | -731.65 | 2.47372D-01 | 2.40448D-07 | 6.60566D-02 |
| P( 7) | 1 - 0 | 391.36 | -717.42 | 2.87513D-01 | 3.27388D-07 | 6.79027D-02 |
| R( 5) | 1 - 1 | 1102.31 | -6.48 | 1.19535D-04 | 9.99999D-01 | 1.74389D+00 |
| R( 6) | 1 - 0 | 383.70 | -732.64 | 2.50161D-01 | 3.27353D-07 | 6.59283D-02 |
| P( 8) | 1 - 0 | 400.12 | -716.22 | 2.84653D-01 | 4.27730D-07 | 6.80588D-02 |
| R( 6) | 1 - 1 | 1108.78 | -7.55 | 1.91910D-04 | 9.99999D-01 | 1.74396D+00 |
| R( 7) | 1 - 0 | 391.36 | -733.61 | 2.52299D-01 | 4.27678D-07 | 6.58018D-02 |
| P( 9) | 1 - 0 | 409.96 | -715.01 | 2.82433D-01 | 5.41519D-07 | 6.82168D-02 |
| R( 7) | 1 - 1 | 1116.34 | -8.63 | 2.88847D-04 | 9.99999D-01 | 1.74404D+00 |
| R( 8) | 1 - 0 | 400.12 | -734.57 | 2.53991D-01 | 5.41445D-07 | 6.56773D-02 |
| P( 10) | 1 - 0 | 420.90 | -713.78 | 2.80650D-01 | 6.68781D-07 | 6.83770D-02 |
| R( 8) | 1 - 1 | 1124.97 | -9.71 | 4.13930D-04 | 9.99998D-01 | 1.74413D+00 |

| | | | | | | | |
|---|---|---|---|---|---|---|---|
| R( 9) | 1 - 0 | 409.96 | -735.51 | 2.55363D-01 | 6.68679D-07 | 6.55546D-02 |
| P( 11) | 1 - 0 | 432.94 | -712.54 | 2.79177D-01 | 8.09544D-07 | 6.85392D-02 |
| R( 9) | 1 - 1 | 1134.68 | -10.79 | 5.70742D-04 | 9.99998D-01 | 1.74424D+00 |
| R( 10) | 1 - 0 | 420.90 | -736.44 | 2.56497D-01 | 8.09408D-07 | 6.54338D-02 |
| P( 12) | 1 - 0 | 446.06 | -711.28 | 2.77931D-01 | 9.63839D-07 | 6.87036D-02 |
| R( 10) | 1 - 1 | 1145.47 | -11.87 | 7.62860D-04 | 9.99998D-01 | 1.74435D+00 |
| R( 11) | 1 - 0 | 432.94 | -737.35 | 2.57449D-01 | 9.63663D-07 | 6.53148D-02 |
| P( 13) | 1 - 0 | 460.28 | -710.01 | 2.76857D-01 | 1.13170D-06 | 6.88700D-02 |
| R( 11) | 1 - 1 | 1157.34 | -12.95 | 9.93858D-04 | 9.99997D-01 | 1.74448D+00 |
| R( 12) | 1 - 0 | 446.06 | -738.25 | 2.58259D-01 | 1.13148D-06 | 6.51977D-02 |
| P( 14) | 1 - 0 | 475.59 | -708.72 | 2.75916D-01 | 1.31316D-06 | 6.90385D-02 |
| R( 12) | 1 - 1 | 1170.29 | -14.02 | 1.26731D-03 | 9.99997D-01 | 1.74461D+00 |
| R( 13) | 1 - 0 | 460.28 | -739.13 | 2.58955D-01 | 1.31289D-06 | 6.50825D-02 |
| P( 15) | 1 - 0 | 491.99 | -707.42 | 2.75078D-01 | 1.50827D-06 | 6.92092D-02 |
| R( 13) | 1 - 1 | 1184.31 | -15.10 | 1.58677D-03 | 9.99996D-01 | 1.74476D+00 |
| R( 14) | 1 - 0 | 475.59 | -740.00 | 2.59559D-01 | 1.50793D-06 | 6.49691D-02 |
| P( 16) | 1 - 0 | 509.48 | -706.10 | 2.74323D-01 | 1.71707D-06 | 6.93821D-02 |
| R( 14) | 1 - 1 | 1199.41 | -16.18 | 1.95579D-03 | 9.99996D-01 | 1.74492D+00 |
| R( 15) | 1 - 0 | 491.99 | -740.85 | 2.60087D-01 | 1.71665D-06 | 6.48575D-02 |
| P( 17) | 1 - 0 | 528.06 | -704.77 | 2.73634D-01 | 1.93959D-06 | 6.95570D-02 |
| R( 15) | 1 - 1 | 1215.59 | -17.25 | 2.37795D-03 | 9.99995D-01 | 1.74509D+00 |
| R( 16) | 1 - 0 | 509.48 | -741.69 | 2.60550D-01 | 1.93909D-06 | 6.47478D-02 |
| P( 18) | 1 - 0 | 547.74 | -703.43 | 2.72999D-01 | 2.17590D-06 | 6.97342D-02 |
| R( 16) | 1 - 1 | 1232.84 | -18.33 | 2.85676D-03 | 9.99994D-01 | 1.74527D+00 |
| R( 17) | 1 - 0 | 528.06 | -742.51 | 2.60960D-01 | 2.17530D-06 | 6.46398D-02 |
| P( 19) | 1 - 0 | 568.50 | -702.07 | 2.72409D-01 | 2.42604D-06 | 6.99135D-02 |
| R( 17) | 1 - 1 | 1251.17 | -19.40 | 3.39578D-03 | 9.99994D-01 | 1.74546D+00 |
| R( 18) | 1 - 0 | 547.74 | -743.31 | 2.61323D-01 | 2.42534D-06 | 6.45337D-02 |
| P( 20) | 1 - 0 | 590.35 | -700.70 | 2.71855D-01 | 2.69007D-06 | 7.00950D-02 |

| | | | | | | | |
|---|---|---|---|---|---|---|---|
| R( 18) | 1 - 1 | 1270.57 | -20.48 | 3.99854D-03 | 9.99993D-01 | 1.74567D+00 |
| R( 19) | 1 - 0 | 568.50 | -744.10 | 2.61647D-01 | 2.68925D-06 | 6.44293D-02 |
| P( 21) | 1 - 0 | 613.29 | -699.31 | 2.71332D-01 | 2.96803D-06 | 7.02788D-02 |
| R( 19) | 1 - 1 | 1291.05 | -21.55 | 4.66855D-03 | 9.99992D-01 | 1.74588D+00 |
| P( 1) | 2 - 0 | 361.81 | -1451.59 | 4.95130D-05 | 2.98427D-11 | -2.27193D-04 |
| P( 1) | 2 - 1 | 1087.20 | -726.20 | 1.14303D+00 | 1.26877D-08 | -9.75532D-02 |
| R( 0) | 2 - 0 | 360.72 | -1453.75 | 1.70945D-05 | 2.99509D-11 | -2.30703D-04 |
| P( 2) | 2 - 0 | 364.00 | -1450.46 | 3.25154D-05 | 1.19154D-10 | -2.25750D-04 |
| R( 0) | 2 - 1 | 1086.12 | -728.35 | 3.81298D-01 | 1.26882D-08 | -9.71588D-02 |
| P( 2) | 2 - 1 | 1089.36 | -725.11 | 7.61740D-01 | 5.07518D-08 | -9.77555D-02 |
| R( 0) | 2 - 2 | 1813.40 | -1.07 | 4.00853D-07 | 1.00000D+00 | -1.77572D+00 |
| R( 1) | 2 - 0 | 361.81 | -1454.79 | 2.09268D-05 | 1.19967D-10 | -2.32766D-04 |
| P( 3) | 2 - 0 | 367.29 | -1449.32 | 2.88759D-05 | 2.67683D-10 | -2.24516D-04 |
| R( 1) | 2 - 1 | 1087.20 | -729.40 | 4.57734D-01 | 5.07505D-08 | -9.69668D-02 |
| P( 3) | 2 - 1 | 1092.59 | -724.01 | 6.85317D-01 | 1.14204D-07 | -9.79613D-02 |
| R( 1) | 2 - 2 | 1814.47 | -2.13 | 3.84807D-06 | 1.00000D+00 | -1.77574D+00 |
| R( 2) | 2 - 0 | 364.00 | -1455.80 | 2.29088D-05 | 2.70369D-10 | -2.35037D-04 |
| P( 4) | 2 - 0 | 371.66 | -1448.14 | 2.71848D-05 | 4.75074D-10 | -2.23494D-04 |
| R( 2) | 2 - 1 | 1089.36 | -730.45 | 4.90622D-01 | 1.14194D-07 | -9.67781D-02 |
| P( 4) | 2 - 1 | 1096.91 | -722.89 | 6.52449D-01 | 2.03050D-07 | -9.81705D-02 |
| R( 2) | 2 - 2 | 1816.60 | -3.20 | 1.39145D-05 | 1.00000D+00 | -1.77577D+00 |
| R( 3) | 2 - 0 | 367.29 | -1456.79 | 2.43099D-05 | 4.81441D-10 | -2.37513D-04 |
| P( 5) | 2 - 0 | 377.14 | -1446.94 | 2.61739D-05 | 7.41038D-10 | -2.22687D-04 |
| R( 3) | 2 - 1 | 1092.59 | -731.48 | 5.08997D-01 | 2.03026D-07 | -9.65929D-02 |
| P( 5) | 2 - 1 | 1102.31 | -721.76 | 6.34102D-01 | 3.17305D-07 | -9.83832D-02 |
| R( 3) | 2 - 2 | 1819.80 | -4.27 | 3.42027D-05 | 9.99999D-01 | -1.77582D+00 |
| R( 4) | 2 - 0 | 371.66 | -1457.75 | 2.54777D-05 | 7.53475D-10 | -2.40197D-04 |
| P( 6) | 2 - 0 | 383.70 | -1445.71 | 2.54971D-05 | 1.06526D-09 | -2.22098D-04 |
| R( 4) | 2 - 1 | 1096.91 | -732.50 | 5.20776D-01 | 3.17258D-07 | -9.64110D-02 |

| | | | | | | | | |
|---|---|---|---|---|---|---|---|---|
| P( 6) | 2 - 1 | 1108.78 | -720.63 | 6.22355D-01 | 4.56988D-07 | -9.85994D-02 |
| R( 4) | 2 - 2 | 1824.07 | -5.34 | 6.83169D-05 | 9.99999D-01 | -1.77588D+00 |
| R( 5) | 2 - 0 | 377.14 | -1458.68 | 2.65473D-05 | 1.08676D-09 | -2.43090D-04 |
| P( 7) | 2 - 0 | 391.36 | -1444.45 | 2.50218D-05 | 1.44744D-09 | -2.21731D-04 |
| R( 5) | 2 - 1 | 1102.31 | -733.50 | 5.29007D-01 | 4.56907D-07 | -9.62325D-02 |
| P( 7) | 2 - 1 | 1116.34 | -719.47 | 6.14164D-01 | 6.22120D-07 | -9.88191D-02 |
| R( 5) | 2 - 2 | 1829.41 | -6.40 | 1.19860D-04 | 9.99999D-01 | -1.77595D+00 |
| R( 6) | 2 - 0 | 383.70 | -1459.58 | 2.75832D-05 | 1.48158D-09 | -2.46193D-04 |
| P( 8) | 2 - 0 | 400.12 | -1443.17 | 2.46861D-05 | 1.88725D-09 | -2.21590D-04 |
| R( 6) | 2 - 1 | 1108.78 | -734.50 | 5.35110D-01 | 6.21991D-07 | -9.60574D-02 |
| P( 8) | 2 - 1 | 1124.97 | -718.31 | 6.08108D-01 | 8.12727D-07 | -9.90424D-02 |
| R( 6) | 2 - 2 | 1835.81 | -7.47 | 1.92434D-04 | 9.99998D-01 | -1.77603D+00 |
| R( 7) | 2 - 0 | 391.36 | -1460.46 | 2.86210D-05 | 1.93822D-09 | -2.49510D-04 |
| P( 9) | 2 - 0 | 409.96 | -1441.86 | 2.44580D-05 | 2.38438D-09 | -2.21681D-04 |
| R( 7) | 2 - 1 | 1116.34 | -735.48 | 5.39839D-01 | 8.12534D-07 | -9.58856D-02 |
| P( 9) | 2 - 1 | 1134.68 | -717.14 | 6.03433D-01 | 1.02884D-06 | -9.92691D-02 |
| R( 7) | 2 - 2 | 1843.28 | -8.54 | 2.89637D-04 | 9.99998D-01 | -1.77613D+00 |
| R( 8) | 2 - 0 | 400.12 | -1461.31 | 2.96827D-05 | 2.45697D-09 | -2.53043D-04 |
| P( 10) | 2 - 0 | 420.90 | -1440.52 | 2.43191D-05 | 2.93849D-09 | -2.22009D-04 |
| R( 8) | 2 - 1 | 1124.97 | -736.45 | 5.43628D-01 | 1.02856D-06 | -9.57172D-02 |
| P( 10) | 2 - 1 | 1145.47 | -715.95 | 5.99703D-01 | 1.27049D-06 | -9.94995D-02 |
| R( 8) | 2 - 2 | 1851.82 | -9.60 | 4.15066D-04 | 9.99997D-01 | -1.77623D+00 |
| R( 9) | 2 - 0 | 409.96 | -1462.13 | 3.07833D-05 | 3.03809D-09 | -2.56795D-04 |
| P( 11) | 2 - 0 | 432.94 | -1439.16 | 2.42588D-05 | 3.54927D-09 | -2.22579D-04 |
| R( 9) | 2 - 1 | 1134.68 | -737.41 | 5.46749D-01 | 1.27011D-06 | -9.55522D-02 |
| P( 11) | 2 - 1 | 1157.34 | -714.75 | 5.96650D-01 | 1.53771D-06 | -9.97334D-02 |
| R( 9) | 2 - 2 | 1861.42 | -10.67 | 5.72313D-04 | 9.99997D-01 | -1.77636D+00 |
| R( 10) | 2 - 0 | 420.90 | -1462.92 | 3.19342D-05 | 3.68188D-09 | -2.60772D-04 |
| P( 12) | 2 - 0 | 446.06 | -1437.77 | 2.42708D-05 | 4.21639D-09 | -2.23399D-04 |

| | | | | | | |
|---|---|---|---|---|---|---|
| R( 10) | 2 - 1 | 1145.47 | -738.35 | 5.49376D-01 | 1.53721D-06 | -9.53905D-02 |
| P( 12) | 2 - 1 | 1170.29 | -713.54 | 5.94097D-01 | 1.83055D-06 | -9.99708D-02 |
| R( 10) | 2 - 2 | 1872.09 | -11.74 | 7.64968D-04 | 9.99996D-01 | -1.77649D+00 |
| R( 11) | 2 - 0 | 432.94 | -1463.69 | 3.31445D-05 | 4.38860D-09 | -2.64978D-04 |
| P( 13) | 2 - 0 | 460.28 | -1436.35 | 2.43515D-05 | 4.93950D-09 | -2.24476D-04 |
| R( 11) | 2 - 1 | 1157.34 | -739.29 | 5.51630D-01 | 1.82990D-06 | -9.52321D-02 |
| P( 13) | 2 - 1 | 1184.31 | -712.32 | 5.91924D-01 | 2.14905D-06 | -1.00212D-01 |
| R( 11) | 2 - 2 | 1883.83 | -12.80 | 9.96616D-04 | 9.99995D-01 | -1.77664D+00 |
| R( 12) | 2 - 0 | 446.06 | -1464.43 | 3.44224D-05 | 5.15853D-09 | -2.69417D-04 |
| P( 14) | 2 - 0 | 475.59 | -1434.91 | 2.44991D-05 | 5.71827D-09 | -2.25817D-04 |
| R( 12) | 2 - 1 | 1170.29 | -740.21 | 5.53595D-01 | 2.14822D-06 | -9.50771D-02 |
| P( 14) | 2 - 1 | 1199.41 | -711.08 | 5.90047D-01 | 2.49326D-06 | -1.00457D-01 |
| R( 12) | 2 - 2 | 1896.63 | -13.87 | 1.27084D-03 | 9.99995D-01 | -1.77680D+00 |
| R( 13) | 2 - 0 | 460.28 | -1465.15 | 3.57750D-05 | 5.99192D-09 | -2.74096D-04 |
| P( 15) | 2 - 0 | 491.99 | -1433.43 | 2.47133D-05 | 6.55235D-09 | -2.27431D-04 |
| R( 13) | 2 - 1 | 1184.31 | -741.11 | 5.55333D-01 | 2.49222D-06 | -9.49255D-02 |
| P( 15) | 2 - 1 | 1215.59 | -709.84 | 5.88405D-01 | 2.86322D-06 | -1.00705D-01 |
| R( 13) | 2 - 2 | 1910.49 | -14.93 | 1.59121D-03 | 9.99994D-01 | -1.77697D+00 |
| R( 14) | 2 - 0 | 475.59 | -1465.83 | 3.72097D-05 | 6.88906D-09 | -2.79021D-04 |
| P( 16) | 2 - 0 | 509.48 | -1431.94 | 2.49944D-05 | 7.44139D-09 | -2.29327D-04 |
| R( 14) | 2 - 1 | 1199.41 | -742.01 | 5.56888D-01 | 2.86195D-06 | -9.47772D-02 |
| P( 16) | 2 - 1 | 1232.84 | -708.58 | 5.86953D-01 | 3.25901D-06 | -1.00957D-01 |
| R( 14) | 2 - 2 | 1925.42 | -16.00 | 1.96130D-03 | 9.99993D-01 | -1.77716D+00 |
| R( 15) | 2 - 0 | 491.99 | -1466.49 | 3.87336D-05 | 7.85020D-09 | -2.84198D-04 |
| P( 17) | 2 - 0 | 528.06 | -1430.41 | 2.53440D-05 | 8.38503D-09 | -2.31513D-04 |
| R( 15) | 2 - 1 | 1215.59 | -742.89 | 5.58296D-01 | 3.25746D-06 | -9.46322D-02 |
| P( 17) | 2 - 1 | 1251.17 | -707.31 | 5.85655D-01 | 3.68068D-06 | -1.01213D-01 |
| R( 15) | 2 - 2 | 1941.42 | -17.06 | 2.38467D-03 | 9.99992D-01 | -1.77736D+00 |
| R( 16) | 2 - 0 | 509.48 | -1467.12 | 4.03537D-05 | 8.87559D-09 | -2.89635D-04 |

| | | | | | | |
|---|---|---|---|---|---|---|
| P( 18) | 2 - 0 | 547.74 | -1428.86 | 2.57641D-05 | 9.38291D-09 | -2.34001D-04 |
| R( 16) | 2 - 1 | 1232.84 | -743.76 | 5.59582D-01 | 3.67882D-06 | -9.44906D-02 |
| P( 18) | 2 - 1 | 1270.57 | -706.03 | 5.84487D-01 | 4.12829D-06 | -1.01473D-01 |
| R( 16) | 2 - 2 | 1958.48 | -18.12 | 2.86489D-03 | 9.99991D-01 | -1.77757D+00 |
| R( 17) | 2 - 0 | 528.06 | -1467.72 | 4.20777D-05 | 9.96550D-09 | -2.95341D-04 |
| P( 19) | 2 - 0 | 568.50 | -1427.29 | 2.62574D-05 | 1.04346D-08 | -2.36799D-04 |
| R( 17) | 2 - 1 | 1251.17 | -744.62 | 5.60768D-01 | 4.12608D-06 | -9.43524D-02 |
| P( 19) | 2 - 1 | 1291.05 | -704.74 | 5.83425D-01 | 4.60191D-06 | -1.01736D-01 |
| R( 17) | 2 - 2 | 1976.60 | -19.19 | 3.40550D-03 | 9.99990D-01 | -1.77779D+00 |
| R( 18) | 2 - 0 | 547.74 | -1468.30 | 4.39133D-05 | 1.11202D-08 | -3.01322D-04 |
| P( 20) | 2 - 0 | 590.35 | -1425.69 | 2.68273D-05 | 1.15399D-08 | -2.39921D-04 |
| R( 18) | 2 - 1 | 1270.57 | -745.47 | 5.61871D-01 | 4.59931D-06 | -9.42175D-02 |
| P( 20) | 2 - 1 | 1312.60 | -703.43 | 5.82456D-01 | 5.10162D-06 | -1.02003D-01 |
| R( 18) | 2 - 2 | 1995.79 | -20.25 | 4.01006D-03 | 9.99988D-01 | -1.77803D+00 |
| R( 19) | 2 - 0 | 568.50 | -1468.85 | 4.58690D-05 | 1.23398D-08 | -3.07588D-04 |
| P( 21) | 2 - 0 | 613.29 | -1424.06 | 2.74777D-05 | 1.26982D-08 | -2.43377D-04 |
| R( 19) | 2 - 1 | 1291.05 | -746.30 | 5.62903D-01 | 5.09858D-06 | -9.40859D-02 |
| P( 21) | 2 - 1 | 1335.23 | -702.12 | 5.81564D-01 | 5.62749D-06 | -1.02274D-01 |
| R( 19) | 2 - 2 | 2016.04 | -21.31 | 4.68209D-03 | 9.99987D-01 | -1.77828D+00 |
| P( 1) | 3 - 0 | 361.81 | -2169.91 | 1.73576D-04 | 5.76417D-13 | 2.32746D-04 |
| P( 1) | 3 - 1 | 1087.20 | -1444.52 | 1.68515D-02 | 7.73225D-11 | 4.22214D-03 |
| P( 1) | 3 - 2 | 1814.47 | -717.25 | 1.86478D+00 | 1.90238D-08 | 1.26942D-01 |
| R( 0) | 3 - 0 | 360.72 | -2172.06 | 5.72726D-05 | 5.78999D-13 | 2.31221D-04 |
| P( 2) | 3 - 0 | 364.00 | -2168.77 | 1.17030D-04 | 2.30060D-12 | 2.34246D-04 |
| R( 0) | 3 - 1 | 1086.12 | -1446.66 | 5.65153D-03 | 7.76090D-11 | 4.22566D-03 |
| P( 2) | 3 - 1 | 1089.36 | -1443.42 | 1.12038D-02 | 3.08729D-10 | 4.22122D-03 |
| R( 0) | 3 - 2 | 1813.40 | -719.38 | 6.22296D-01 | 1.90242D-08 | 1.26452D-01 |
| P( 2) | 3 - 2 | 1816.60 | -716.17 | 1.24250D+00 | 7.60974D-08 | 1.27194D-01 |
| R( 0) | 3 - 3 | 2531.72 | -1.06 | 4.03637D-07 | 1.00000D+00 | 1.81048D+00 |

| | | | | | | | |
|---|---|---|---|---|---|---|---|
| R( 1) | 3 - 0 | 361.81 | -2173.07 | 6.88091D-05 | 2.31902D-12 | 2.31196D-04 |
| P( 3) | 3 - 0 | 367.29 | -2167.60 | 1.06953D-04 | 5.16850D-12 | 2.36239D-04 |
| R( 1) | 3 - 1 | 1087.20 | -1447.69 | 6.80471D-03 | 3.10916D-10 | 4.22825D-03 |
| P( 3) | 3 - 1 | 1092.59 | -1442.29 | 1.00581D-02 | 6.93555D-10 | 4.22086D-03 |
| R( 1) | 3 - 2 | 1814.47 | -720.42 | 7.47194D-01 | 7.60933D-08 | 1.26214D-01 |
| P( 3) | 3 - 2 | 1819.80 | -715.08 | 1.11766D+00 | 1.71237D-07 | 1.27451D-01 |
| R( 1) | 3 - 3 | 2532.78 | -2.11 | 3.87482D-06 | 1.00000D+00 | 1.81050D+00 |
| R( 2) | 3 - 0 | 364.00 | -2174.05 | 7.41219D-05 | 5.22814D-12 | 2.31662D-04 |
| P( 4) | 3 - 0 | 371.66 | -2166.39 | 1.03840D-04 | 9.17176D-12 | 2.38723D-04 |
| R( 2) | 3 - 1 | 1089.36 | -1448.70 | 7.31692D-03 | 7.00816D-10 | 4.23140D-03 |
| P( 4) | 3 - 1 | 1096.91 | -1441.14 | 9.55715D-03 | 1.23095D-09 | 4.22106D-03 |
| R( 2) | 3 - 2 | 1816.60 | -721.45 | 8.01046D-01 | 1.71216D-07 | 1.25981D-01 |
| P( 4) | 3 - 2 | 1824.07 | -713.98 | 1.06388D+00 | 3.04452D-07 | 1.27713D-01 |
| R( 2) | 3 - 3 | 2534.89 | -3.17 | 1.40113D-05 | 1.00000D+00 | 1.81054D+00 |
| R( 3) | 3 - 0 | 367.29 | -2174.99 | 7.76050D-05 | 9.31316D-12 | 2.32621D-04 |
| P( 5) | 3 - 0 | 377.14 | -2165.14 | 1.03311D-04 | 1.43052D-11 | 2.41701D-04 |
| R( 3) | 3 - 1 | 1092.59 | -1449.68 | 7.61675D-03 | 1.24816D-09 | 4.23511D-03 |
| P( 5) | 3 - 1 | 1102.31 | -1439.97 | 9.27237D-03 | 1.92022D-09 | 4.22182D-03 |
| R( 3) | 3 - 2 | 1819.80 | -722.48 | 8.31225D-01 | 3.04401D-07 | 1.25752D-01 |
| P( 5) | 3 - 2 | 1829.41 | -712.87 | 1.03380D+00 | 4.75764D-07 | 1.27979D-01 |
| R( 3) | 3 - 3 | 2538.06 | -4.22 | 3.44409D-05 | 9.99999D-01 | 1.81059D+00 |
| R( 4) | 3 - 0 | 371.66 | -2175.90 | 8.04612D-05 | 1.45815D-11 | 2.34070D-04 |
| P( 6) | 3 - 0 | 383.70 | -2163.86 | 1.04181D-04 | 2.05632D-11 | 2.45172D-04 |
| R( 4) | 3 - 1 | 1096.91 | -1450.65 | 7.82110D-03 | 1.95384D-09 | 4.23937D-03 |
| P( 6) | 3 - 1 | 1108.78 | -1438.78 | 9.08685D-03 | 2.76067D-09 | 4.22315D-03 |
| R( 4) | 3 - 2 | 1824.07 | -723.49 | 8.50652D-01 | 4.75664D-07 | 1.25528D-01 |
| P( 6) | 3 - 2 | 1835.81 | -711.75 | 1.01450D+00 | 6.85199D-07 | 1.28250D-01 |
| R( 4) | 3 - 3 | 2542.28 | -5.28 | 6.87934D-05 | 9.99999D-01 | 1.81065D+00 |
| R( 5) | 3 - 0 | 377.14 | -2176.76 | 8.31590D-05 | 2.10407D-11 | 2.36012D-04 |

| | | | | | | | |
|---|---|---|---|---|---|---|---|
| P( 7) | 3 - 0 | 391.36 | -2162.53 | 1.06003D-04 | 2.79402D-11 | 2.49136D-04 |
| R( 5) | 3 - 1 | 1102.31 | -1451.59 | 7.97496D-03 | 2.81879D-09 | 4.24419D-03 |
| P( 7) | 3 - 1 | 1116.34 | -1437.56 | 8.95562D-03 | 3.75162D-09 | 4.22505D-03 |
| R( 5) | 3 - 2 | 1829.41 | -724.49 | 8.64296D-01 | 6.85026D-07 | 1.25309D-01 |
| P( 7) | 3 - 2 | 1843.28 | -710.61 | 1.00101D+00 | 9.32787D-07 | 1.28526D-01 |
| R( 5) | 3 - 3 | 2547.56 | -6.34 | 1.20698D-04 | 9.99998D-01 | 1.81072D+00 |
| R( 6) | 3 - 0 | 383.70 | -2177.58 | 8.59237D-05 | 2.86985D-11 | 2.38446D-04 |
| P( 8) | 3 - 0 | 400.12 | -2161.17 | 1.08580D-04 | 3.64309D-11 | 2.53594D-04 |
| R( 6) | 3 - 1 | 1108.78 | -1452.50 | 8.09931D-03 | 3.84393D-09 | 4.24956D-03 |
| P( 8) | 3 - 1 | 1124.97 | -1436.31 | 8.85770D-03 | 4.89241D-09 | 4.22752D-03 |
| R( 6) | 3 - 2 | 1835.81 | -725.47 | 8.74477D-01 | 9.32512D-07 | 1.25094D-01 |
| P( 8) | 3 - 2 | 1851.82 | -709.47 | 9.91006D-01 | 1.21856D-06 | 1.28807D-01 |
| R( 6) | 3 - 3 | 2553.90 | -7.39 | 1.93781D-04 | 9.99998D-01 | 1.81081D+00 |
| R( 7) | 3 - 0 | 391.36 | -2178.37 | 8.88816D-05 | 3.75631D-11 | 2.41372D-04 |
| P( 9) | 3 - 0 | 409.96 | -2159.77 | 1.11815D-04 | 4.60300D-11 | 2.58548D-04 |
| R( 7) | 3 - 1 | 1116.34 | -1453.39 | 8.20530D-03 | 5.03024D-09 | 4.25550D-03 |
| P( 9) | 3 - 1 | 1134.68 | -1435.05 | 8.78199D-03 | 6.18242D-09 | 4.23056D-03 |
| R( 7) | 3 - 2 | 1843.28 | -726.45 | 8.82422D-01 | 1.21815D-06 | 1.24884D-01 |
| P( 9) | 3 - 2 | 1861.42 | -708.31 | 9.83264D-01 | 1.54257D-06 | 1.29093D-01 |
| R( 7) | 3 - 3 | 2561.29 | -8.45 | 2.91670D-04 | 9.99997D-01 | 1.81091D+00 |
| R( 8) | 3 - 0 | 400.12 | -2179.12 | 9.21136D-05 | 4.76425D-11 | 2.44790D-04 |
| P( 10) | 3 - 0 | 420.90 | -2158.33 | 1.15665D-04 | 5.67326D-11 | 2.63996D-04 |
| R( 8) | 3 - 1 | 1124.97 | -1454.26 | 8.29936D-03 | 6.37872D-09 | 4.26199D-03 |
| P( 10) | 3 - 1 | 1145.47 | -1433.76 | 8.72205D-03 | 7.62103D-09 | 4.23418D-03 |
| R( 8) | 3 - 2 | 1851.82 | -727.42 | 8.88842D-01 | 1.54198D-06 | 1.24679D-01 |
| P( 10) | 3 - 2 | 1872.09 | -707.14 | 9.77073D-01 | 1.90485D-06 | 1.29383D-01 |
| R( 8) | 3 - 3 | 2569.73 | -9.50 | 4.17988D-04 | 9.99996D-01 | 1.81103D+00 |
| R( 9) | 3 - 0 | 409.96 | -2179.83 | 9.56776D-05 | 5.89452D-11 | 2.48702D-04 |
| P( 11) | 3 - 0 | 432.94 | -2156.86 | 1.20110D-04 | 6.85338D-11 | 2.69941D-04 |

| | | | | | | |
|---|---|---|---|---|---|---|
| R( 9) | 3 - 1 | 1134.68 | -1455.11 | 8.38550D-03 | 7.89040D-09 | 4.26904D-03 |
| P( 11) | 3 - 1 | 1157.34 | -1432.45 | 8.67390D-03 | 9.20765D-09 | 4.23838D-03 |
| R( 9) | 3 - 2 | 1861.42 | -728.37 | 8.94179D-01 | 1.90404D-06 | 1.24478D-01 |
| P( 11) | 3 - 2 | 1883.83 | -705.96 | 9.71992D-01 | 2.30545D-06 | 1.29679D-01 |
| R( 9) | 3 - 3 | 2579.24 | -10.56 | 5.76354D-04 | 9.99996D-01 | 1.81116D+00 |
| R( 10) | 3 - 0 | 420.90 | -2180.50 | 9.96199D-05 | 7.14797D-11 | 2.53108D-04 |
| P( 12) | 3 - 0 | 446.06 | -2155.34 | 1.25149D-04 | 8.14287D-11 | 2.76383D-04 |
| R( 10) | 3 - 1 | 1145.47 | -1455.93 | 8.46634D-03 | 9.56631D-09 | 4.27665D-03 |
| P( 12) | 3 - 1 | 1170.29 | -1431.12 | 8.63496D-03 | 1.09417D-08 | 4.24316D-03 |
| R( 10) | 3 - 2 | 1872.09 | -729.31 | 8.98719D-01 | 2.30438D-06 | 1.24282D-01 |
| P( 12) | 3 - 2 | 1896.63 | -704.78 | 9.67733D-01 | 2.74444D-06 | 1.29979D-01 |
| R( 10) | 3 - 3 | 2589.79 | -11.61 | 7.70389D-04 | 9.99995D-01 | 1.81131D+00 |
| R( 11) | 3 - 0 | 432.94 | -2181.13 | 1.03981D-04 | 8.52547D-11 | 2.58007D-04 |
| P( 13) | 3 - 0 | 460.28 | -2153.79 | 1.30791D-04 | 9.54128D-11 | 2.83322D-04 |
| R( 11) | 3 - 1 | 1157.34 | -1456.73 | 8.54367D-03 | 1.14075D-08 | 4.28482D-03 |
| P( 13) | 3 - 1 | 1184.31 | -1429.76 | 8.60346D-03 | 1.28227D-08 | 4.24854D-03 |
| R( 11) | 3 - 2 | 1883.83 | -730.24 | 9.02658D-01 | 2.74305D-06 | 1.24091D-01 |
| P( 13) | 3 - 2 | 1910.49 | -703.58 | 9.64103D-01 | 3.22187D-06 | 1.30284D-01 |
| R( 11) | 3 - 3 | 2601.40 | -12.67 | 1.00370D-03 | 9.99994D-01 | 1.81146D+00 |
| R( 12) | 3 - 0 | 446.06 | -2181.73 | 1.08797D-04 | 1.00279D-10 | 2.63400D-04 |
| P( 14) | 3 - 0 | 475.59 | -2152.20 | 1.37052D-04 | 1.10481D-10 | 2.90760D-04 |
| R( 12) | 3 - 1 | 1170.29 | -1457.50 | 8.61877D-03 | 1.34152D-08 | 4.29356D-03 |
| P( 14) | 3 - 1 | 1199.41 | -1428.38 | 8.57817D-03 | 1.48500D-08 | 4.25450D-03 |
| R( 12) | 3 - 2 | 1896.63 | -731.16 | 9.06133D-01 | 3.22009D-06 | 1.23904D-01 |
| P( 14) | 3 - 2 | 1925.42 | -702.37 | 9.60963D-01 | 3.73780D-06 | 1.30595D-01 |
| R( 12) | 3 - 3 | 2614.07 | -13.72 | 1.27991D-03 | 9.99993D-01 | 1.81163D+00 |
| R( 13) | 3 - 0 | 460.28 | -2182.28 | 1.14105D-04 | 1.16562D-10 | 2.69289D-04 |
| P( 15) | 3 - 0 | 491.99 | -2150.57 | 1.43953D-04 | 1.26630D-10 | 2.98697D-04 |
| R( 13) | 3 - 1 | 1184.31 | -1458.25 | 8.69255D-03 | 1.55904D-08 | 4.30287D-03 |

| | | | | | | | |
|---|---|---|---|---|---|---|---|
| P( 15) | 3 - 1 | 1215.59 | -1426.98 | 8.55819D-03 | 1.70231D-08 | 4.26106D-03 |
| R( 13) | 3 - 2 | 1910.49 | -732.07 | 9.09245D-01 | 3.73558D-06 | 1.23722D-01 |
| P( 15) | 3 - 2 | 1941.42 | -701.14 | 9.58213D-01 | 4.29230D-06 | 1.30910D-01 |
| R( 13) | 3 - 3 | 2627.79 | -14.77 | 1.60262D-03 | 9.99991D-01 | 1.81182D+00 |
| R( 14) | 3 - 0 | 475.59 | -2182.80 | 1.19940D-04 | 1.34112D-10 | 2.75673D-04 |
| P( 16) | 3 - 0 | 509.48 | -2148.91 | 1.51521D-04 | 1.43854D-10 | 3.07134D-04 |
| R( 14) | 3 - 1 | 1199.41 | -1458.98 | 8.76572D-03 | 1.79343D-08 | 4.31274D-03 |
| P( 16) | 3 - 1 | 1232.84 | -1425.55 | 8.54286D-03 | 1.93417D-08 | 4.26822D-03 |
| R( 14) | 3 - 2 | 1925.42 | -732.97 | 9.12069D-01 | 4.28958D-06 | 1.23544D-01 |
| P( 16) | 3 - 2 | 1958.48 | -699.91 | 9.55780D-01 | 4.88546D-06 | 1.31230D-01 |
| R( 14) | 3 - 3 | 2642.56 | -15.83 | 1.97543D-03 | 9.99990D-01 | 1.81202D+00 |
| R( 15) | 3 - 0 | 491.99 | -2183.28 | 1.26340D-04 | 1.52938D-10 | 2.82554D-04 |
| P( 17) | 3 - 0 | 528.06 | -2147.21 | 1.59784D-04 | 1.62149D-10 | 3.16073D-04 |
| R( 15) | 3 - 1 | 1215.59 | -1459.68 | 8.83881D-03 | 2.04481D-08 | 4.32319D-03 |
| P( 17) | 3 - 1 | 1251.17 | -1424.10 | 8.53170D-03 | 2.18051D-08 | 4.27599D-03 |
| R( 15) | 3 - 2 | 1941.42 | -733.85 | 9.14659D-01 | 4.88216D-06 | 1.23371D-01 |
| P( 17) | 3 - 2 | 1976.60 | -698.67 | 9.53608D-01 | 5.51735D-06 | 1.31555D-01 |
| R( 15) | 3 - 3 | 2658.39 | -16.88 | 2.40194D-03 | 9.99989D-01 | 1.81223D+00 |
| R( 16) | 3 - 0 | 509.48 | -2183.72 | 1.33341D-04 | 1.73050D-10 | 2.89931D-04 |
| P( 18) | 3 - 0 | 547.74 | -2145.47 | 1.68775D-04 | 1.81510D-10 | 3.25513D-04 |
| R( 16) | 3 - 1 | 1232.84 | -1460.36 | 8.91226D-03 | 2.31330D-08 | 4.33421D-03 |
| P( 18) | 3 - 1 | 1270.57 | -1422.63 | 8.52431D-03 | 2.44130D-08 | 4.28437D-03 |
| R( 16) | 3 - 2 | 1958.48 | -734.72 | 9.17060D-01 | 5.51338D-06 | 1.23203D-01 |
| P( 18) | 3 - 2 | 1995.79 | -697.42 | 9.51653D-01 | 6.18805D-06 | 1.31886D-01 |
| R( 16) | 3 - 3 | 2675.27 | -17.93 | 2.88575D-03 | 9.99987D-01 | 1.81246D+00 |
| R( 17) | 3 - 0 | 528.06 | -2184.12 | 1.40984D-04 | 1.94458D-10 | 2.97805D-04 |
| P( 19) | 3 - 0 | 568.50 | -2143.69 | 1.78530D-04 | 2.01933D-10 | 3.35456D-04 |
| R( 17) | 3 - 1 | 1251.17 | -1461.02 | 8.98639D-03 | 2.59902D-08 | 4.34582D-03 |
| P( 19) | 3 - 1 | 1291.05 | -1421.14 | 8.52042D-03 | 2.71648D-08 | 4.29337D-03 |

| | | | | | | | |
|---|---|---|---|---|---|---|---|
| R( 17) | 3 - 2 | 1976.60 | -735.59 | 9.19307D-01 | 6.18334D-06 | 1.23039D-01 |
| P( 19) | 3 - 2 | 2016.04 | -696.15 | 9.49882D-01 | 6.89766D-06 | 1.32221D-01 |
| R( 17) | 3 - 3 | 2693.20 | -18.98 | 3.43043D-03 | 9.99986D-01 | 1.81270D+00 |
| R( 18) | 3 - 0 | 547.74 | -2184.49 | 1.49310D-04 | 2.17169D-10 | 3.06178D-04 |
| P( 20) | 3 - 0 | 590.35 | -2141.88 | 1.89085D-04 | 2.23414D-10 | 3.45902D-04 |
| R( 18) | 3 - 1 | 1270.57 | -1461.65 | 9.06149D-03 | 2.90210D-08 | 4.35800D-03 |
| P( 20) | 3 - 1 | 1312.60 | -1419.62 | 8.51978D-03 | 3.00602D-08 | 4.30300D-03 |
| R( 18) | 3 - 2 | 1995.79 | -736.44 | 9.21426D-01 | 6.89211D-06 | 1.22880D-01 |
| P( 20) | 3 - 2 | 2037.35 | -694.88 | 9.48267D-01 | 7.64626D-06 | 1.32562D-01 |
| R( 18) | 3 - 3 | 2712.19 | -20.04 | 4.03958D-03 | 9.99984D-01 | 1.81296D+00 |
| R( 19) | 3 - 0 | 568.50 | -2184.81 | 1.58361D-04 | 2.41194D-10 | 3.15049D-04 |
| P( 21) | 3 - 0 | 613.29 | -2140.02 | 2.00481D-04 | 2.45946D-10 | 3.56854D-04 |
| R( 19) | 3 - 1 | 1291.05 | -1462.26 | 9.13779D-03 | 3.22267D-08 | 4.37077D-03 |
| P( 21) | 3 - 1 | 1335.23 | -1418.08 | 8.52223D-03 | 3.30989D-08 | 4.31325D-03 |
| R( 19) | 3 - 2 | 2016.04 | -737.28 | 9.23440D-01 | 7.63979D-06 | 1.22725D-01 |
| P( 21) | 3 - 2 | 2059.72 | -693.59 | 9.46787D-01 | 8.43396D-06 | 1.32908D-01 |
| R( 19) | 3 - 3 | 2732.22 | -21.09 | 4.71677D-03 | 9.99982D-01 | 1.81323D+00 |
| P( 1) | 4 - 0 | 361.81 | -2884.73 | 1.49149D-02 | 1.53087D-14 | -1.40751D-03 |
| P( 1) | 4 - 1 | 1087.20 | -2159.34 | 4.10992D-03 | 1.51220D-12 | -1.14086D-03 |
| P( 1) | 4 - 2 | 1814.47 | -1432.07 | 7.44933D-02 | 1.44043D-10 | -8.99310D-03 |
| P( 1) | 4 - 3 | 2532.78 | -713.77 | 2.77628D+00 | 2.47834D-08 | -1.56026D-01 |
| R( 0) | 4 - 0 | 360.72 | -2886.87 | 4.98318D-03 | 1.54032D-14 | -1.40758D-03 |
| P( 2) | 4 - 0 | 364.00 | -2883.58 | 9.92966D-03 | 6.10662D-14 | -1.40739D-03 |
| R( 0) | 4 - 1 | 1086.12 | -2161.47 | 1.36646D-03 | 1.51973D-12 | -1.13772D-03 |
| P( 2) | 4 - 1 | 1089.36 | -2158.23 | 2.74600D-03 | 6.03403D-12 | -1.14301D-03 |
| R( 0) | 4 - 2 | 1813.40 | -1434.19 | 2.49530D-02 | 1.44579D-10 | -8.99525D-03 |
| P( 2) | 4 - 2 | 1816.60 | -1430.98 | 4.95562D-02 | 5.75100D-10 | -8.99377D-03 |
| R( 0) | 4 - 3 | 2531.72 | -715.87 | 9.26834D-01 | 2.47833D-08 | -1.55458D-01 |
| P( 2) | 4 - 3 | 2534.89 | -712.70 | 1.84949D+00 | 9.91379D-08 | -1.56319D-01 |

| | | | | | | | |
|---|---|---|---|---|---|---|---|
| R( 0) | 4 - 4 | 3246.54 | -1.04 | 4.07146D-07 | 1.00000D+00 | -1.84911D+00 |
| R( 1) | 4 - 0 | 361.81 | -2887.86 | 5.98550D-03 | 6.16774D-14 | -1.40752D-03 |
| P( 3) | 4 - 0 | 367.29 | -2882.39 | 8.92321D-03 | 1.37261D-13 | -1.40720D-03 |
| R( 1) | 4 - 1 | 1087.20 | -2162.48 | 1.63916D-03 | 6.08882D-12 | -1.13672D-03 |
| P( 3) | 4 - 1 | 1092.59 | -2157.08 | 2.47837D-03 | 1.35519D-11 | -1.14553D-03 |
| R( 1) | 4 - 2 | 1814.47 | -1435.21 | 3.00265D-02 | 5.79235D-10 | -8.99807D-03 |
| P( 3) | 4 - 2 | 1819.80 | -1429.87 | 4.45148D-02 | 1.29183D-09 | -8.99561D-03 |
| R( 1) | 4 - 3 | 2532.78 | -716.90 | 1.11307D+00 | 9.91294D-08 | -1.55183D-01 |
| P( 3) | 4 - 3 | 2538.06 | -711.62 | 1.66334D+00 | 2.23087D-07 | -1.56618D-01 |
| R( 1) | 4 - 4 | 3247.59 | -2.09 | 3.90851D-06 | 1.00000D+00 | -1.84913D+00 |
| R( 2) | 4 - 0 | 364.00 | -2888.80 | 6.41823D-03 | 1.39163D-13 | -1.40740D-03 |
| P( 4) | 4 - 0 | 371.66 | -2881.14 | 8.48428D-03 | 2.43633D-13 | -1.40695D-03 |
| R( 2) | 4 - 1 | 1089.36 | -2163.45 | 1.75670D-03 | 1.37307D-11 | -1.13610D-03 |
| P( 4) | 4 - 1 | 1096.91 | -2155.90 | 2.36845D-03 | 2.40421D-11 | -1.14844D-03 |
| R( 2) | 4 - 2 | 1816.60 | -1436.21 | 3.22669D-02 | 1.30561D-09 | -9.00204D-03 |
| P( 4) | 4 - 2 | 1824.07 | -1428.73 | 4.23223D-02 | 2.29258D-09 | -8.99861D-03 |
| R( 2) | 4 - 3 | 2534.89 | -717.92 | 1.19352D+00 | 2.23049D-07 | -1.54913D-01 |
| P( 4) | 4 - 3 | 2542.28 | -710.53 | 1.58300D+00 | 3.96645D-07 | -1.56923D-01 |
| R( 2) | 4 - 4 | 3249.67 | -3.13 | 1.41332D-05 | 9.99999D-01 | -1.84917D+00 |
| R( 3) | 4 - 0 | 367.29 | -2889.70 | 6.66039D-03 | 2.48145D-13 | -1.40722D-03 |
| P( 5) | 4 - 0 | 377.14 | -2879.85 | 8.23384D-03 | 3.80154D-13 | -1.40664D-03 |
| R( 3) | 4 - 1 | 1092.59 | -2164.39 | 1.82337D-03 | 2.44659D-11 | -1.13586D-03 |
| P( 5) | 4 - 1 | 1102.31 | -2154.68 | 2.31194D-03 | 3.74883D-11 | -1.15173D-03 |
| R( 3) | 4 - 2 | 1819.80 | -1437.18 | 3.35684D-02 | 2.32524D-09 | -9.00717D-03 |
| P( 5) | 4 - 2 | 1829.41 | -1427.57 | 4.10848D-02 | 3.57593D-09 | -9.00279D-03 |
| R( 3) | 4 - 3 | 2538.06 | -718.93 | 1.23873D+00 | 3.96557D-07 | -1.54650D-01 |
| P( 5) | 4 - 3 | 2547.56 | -709.42 | 1.53796D+00 | 6.19848D-07 | -1.57235D-01 |
| R( 3) | 4 - 4 | 3252.81 | -4.18 | 3.47407D-05 | 9.99999D-01 | -1.84922D+00 |
| R( 4) | 4 - 0 | 371.66 | -2890.54 | 6.81534D-03 | 3.88970D-13 | -1.40697D-03 |

| | | | | | | | |
|---|---|---|---|---|---|---|---|
| P( 6) | 4 - 0 | 383.70 | -2878.50 | 8.06850D-03 | 5.46781D-13 | -1.40626D-03 |
| R( 4) | 4 - 1 | 1096.91 | -2165.29 | 1.86761D-03 | 3.83162D-11 | -1.13600D-03 |
| P( 6) | 4 - 1 | 1108.78 | -2153.42 | 2.28043D-03 | 5.38735D-11 | -1.15541D-03 |
| R( 4) | 4 - 2 | 1824.07 | -1438.13 | 3.44476D-02 | 3.63973D-09 | -9.01346D-03 |
| P( 6) | 4 - 2 | 1835.81 | -1426.39 | 4.02856D-02 | 5.14041D-09 | -9.00815D-03 |
| R( 4) | 4 - 3 | 2542.28 | -719.93 | 1.26793D+00 | 6.19676D-07 | -1.54393D-01 |
| P( 6) | 4 - 3 | 2553.90 | -708.31 | 1.50896D+00 | 8.92733D-07 | -1.57552D-01 |
| R( 4) | 4 - 4 | 3256.98 | -5.22 | 6.93925D-05 | 9.99999D-01 | -1.84929D+00 |
| R( 5) | 4 - 0 | 377.14 | -2891.33 | 6.92281D-03 | 5.62024D-13 | -1.40666D-03 |
| P( 7) | 4 - 0 | 391.36 | -2877.11 | 7.94849D-03 | 7.43511D-13 | -1.40582D-03 |
| R( 5) | 4 - 1 | 1102.31 | -2166.16 | 1.90037D-03 | 5.53044D-11 | -1.13652D-03 |
| P( 7) | 4 - 1 | 1116.34 | -2152.13 | 2.26297D-03 | 7.31807D-11 | -1.15946D-03 |
| R( 5) | 4 - 2 | 1829.41 | -1439.06 | 3.51033D-02 | 5.25067D-09 | -9.02090D-03 |
| P( 7) | 4 - 2 | 1843.28 | -1425.19 | 3.97260D-02 | 6.98458D-09 | -9.01469D-03 |
| R( 5) | 4 - 3 | 2547.56 | -720.91 | 1.28853D+00 | 8.92435D-07 | -1.54141D-01 |
| P( 7) | 4 - 3 | 2561.29 | -707.18 | 1.48861D+00 | 1.21535D-06 | -1.57875D-01 |
| R( 5) | 4 - 4 | 3262.21 | -6.27 | 1.21750D-04 | 9.99998D-01 | -1.84937D+00 |
| R( 6) | 4 - 0 | 383.70 | -2892.08 | 7.00135D-03 | 7.67735D-13 | -1.40628D-03 |
| P( 8) | 4 - 0 | 400.12 | -2875.66 | 7.85526D-03 | 9.70376D-13 | -1.40531D-03 |
| R( 6) | 4 - 1 | 1108.78 | -2167.00 | 1.92675D-03 | 7.54534D-11 | -1.13742D-03 |
| P( 8) | 4 - 1 | 1124.97 | -2150.81 | 2.25446D-03 | 9.53939D-11 | -1.16391D-03 |
| R( 6) | 4 - 2 | 1835.81 | -1439.97 | 3.56282D-02 | 7.15971D-09 | -9.02949D-03 |
| P( 8) | 4 - 2 | 1851.82 | -1423.96 | 3.93132D-02 | 9.10700D-09 | -9.02240D-03 |
| R( 6) | 4 - 3 | 2553.90 | -721.88 | 1.30396D+00 | 1.21487D-06 | -1.53896D-01 |
| P( 8) | 4 - 3 | 2569.73 | -706.05 | 1.47346D+00 | 1.58774D-06 | -1.58205D-01 |
| R( 6) | 4 - 4 | 3268.47 | -7.31 | 1.95472D-04 | 9.99997D-01 | -1.84946D+00 |
| R( 7) | 4 - 0 | 391.36 | -2892.77 | 7.06075D-03 | 1.00657D-12 | -1.40583D-03 |
| P( 9) | 4 - 0 | 409.96 | -2874.17 | 7.77897D-03 | 1.22745D-12 | -1.40474D-03 |
| R( 7) | 4 - 1 | 1116.34 | -2167.79 | 1.94948D-03 | 9.87873D-11 | -1.13870D-03 |

| | | | | | | | |
|---|---|---|---|---|---|---|---|
| P( 9) | 4 - 1 | 1134.68 | -2149.45 | 2.25223D-03 | 1.20497D-10 | -1.16874D-03 |
| R( 7) | 4 - 2 | 1843.28 | -1440.85 | 3.60714D-02 | 9.36848D-09 | -9.03924D-03 |
| P( 9) | 4 - 2 | 1861.42 | -1422.71 | 3.89983D-02 | 1.15063D-08 | -9.03130D-03 |
| R( 7) | 4 - 3 | 2561.29 | -722.85 | 1.31607D+00 | 1.58704D-06 | -1.53656D-01 |
| P( 9) | 4 - 3 | 2579.24 | -704.90 | 1.46168D+00 | 2.00999D-06 | -1.58540D-01 |
| R( 7) | 4 - 4 | 3275.78 | -8.35 | 2.94218D-04 | 9.99996D-01 | -1.84957D+00 |
| R( 8) | 4 - 0 | 400.12 | -2893.41 | 7.10669D-03 | 1.27903D-12 | -1.40531D-03 |
| P( 10) | 4 - 0 | 420.90 | -2872.63 | 7.71392D-03 | 1.51483D-12 | -1.40409D-03 |
| R( 8) | 4 - 1 | 1124.97 | -2168.56 | 1.97011D-03 | 1.25331D-10 | -1.14037D-03 |
| P( 10) | 4 - 1 | 1145.47 | -2148.06 | 2.25470D-03 | 1.48476D-10 | -1.17396D-03 |
| R( 8) | 4 - 2 | 1851.82 | -1441.71 | 3.64614D-02 | 1.18787D-08 | -9.05013D-03 |
| P( 10) | 4 - 2 | 1872.09 | -1421.44 | 3.87527D-02 | 1.41809D-08 | -9.04139D-03 |
| R( 8) | 4 - 3 | 2569.73 | -723.80 | 1.32591D+00 | 2.00898D-06 | -1.53422D-01 |
| P( 10) | 4 - 3 | 2589.79 | -703.74 | 1.45221D+00 | 2.48214D-06 | -1.58882D-01 |
| R( 8) | 4 - 4 | 3284.13 | -9.40 | 4.21644D-04 | 9.99995D-01 | -1.84970D+00 |
| R( 9) | 4 - 0 | 409.96 | -2894.01 | 7.14265D-03 | 1.58568D-12 | -1.40472D-03 |
| P( 11) | 4 - 0 | 432.94 | -2871.03 | 7.65656D-03 | 1.83267D-12 | -1.40337D-03 |
| R( 9) | 4 - 1 | 1134.68 | -2169.28 | 1.98964D-03 | 1.55108D-10 | -1.14241D-03 |
| P( 11) | 4 - 1 | 1157.34 | -2146.63 | 2.26092D-03 | 1.79316D-10 | -1.17956D-03 |
| R( 9) | 4 - 2 | 1861.42 | -1442.55 | 3.68159D-02 | 1.46919D-08 | -9.06217D-03 |
| P( 11) | 4 - 2 | 1883.83 | -1420.14 | 3.85589D-02 | 1.71297D-08 | -9.05267D-03 |
| R( 9) | 4 - 3 | 2579.24 | -724.73 | 1.33414D+00 | 2.48076D-06 | -1.53194D-01 |
| P( 11) | 4 - 3 | 2601.40 | -702.56 | 1.44439D+00 | 3.00429D-06 | -1.59230D-01 |
| R( 9) | 4 - 4 | 3293.53 | -10.44 | 5.81403D-04 | 9.99994D-01 | -1.84984D+00 |
| R( 10) | 4 - 0 | 420.90 | -2894.55 | 7.17090D-03 | 1.92709D-12 | -1.40405D-03 |
| P( 12) | 4 - 0 | 446.06 | -2869.39 | 7.60458D-03 | 2.18114D-12 | -1.40257D-03 |
| R( 10) | 4 - 1 | 1145.47 | -2169.98 | 2.00871D-03 | 1.88146D-10 | -1.14483D-03 |
| P( 12) | 4 - 1 | 1170.29 | -2145.16 | 2.27028D-03 | 2.13002D-10 | -1.18555D-03 |
| R( 10) | 4 - 2 | 1872.09 | -1443.36 | 3.71465D-02 | 1.78100D-08 | -9.07536D-03 |

| | | | | | | | |
|---|---|---|---|---|---|---|---|
| P( 12) | 4 - 2 | 1896.63 | -1418.82 | 3.84053D-02 | 2.03510D-08 | -9.06515D-03 |
| R( 10) | 4 - 3 | 2589.79 | -725.66 | 1.34118D+00 | 3.00246D-06 | -1.52972D-01 |
| P( 12) | 4 - 3 | 2614.07 | -701.38 | 1.43780D+00 | 3.57652D-06 | -1.59584D-01 |
| R( 10) | 4 - 4 | 3303.97 | -11.48 | 7.77148D-04 | 9.99993D-01 | -1.84999D+00 |
| R( 11) | 4 - 0 | 432.94 | -2895.04 | 7.19297D-03 | 2.30389D-12 | -1.40330D-03 |
| P( 13) | 4 - 0 | 460.28 | -2867.70 | 7.55641D-03 | 2.56046D-12 | -1.40170D-03 |
| R( 11) | 4 - 1 | 1157.34 | -2170.63 | 2.02775D-03 | 2.24472D-10 | -1.14764D-03 |
| P( 13) | 4 - 1 | 1184.31 | -2143.67 | 2.28236D-03 | 2.49523D-10 | -1.19194D-03 |
| R( 11) | 4 - 2 | 1883.83 | -1444.15 | 3.74609D-02 | 2.12346D-08 | -9.08969D-03 |
| P( 13) | 4 - 2 | 1910.49 | -1417.48 | 3.82841D-02 | 2.38437D-08 | -9.07883D-03 |
| R( 11) | 4 - 3 | 2601.40 | -726.57 | 1.34733D+00 | 3.57413D-06 | -1.52756D-01 |
| P( 13) | 4 - 3 | 2627.79 | -700.19 | 1.43214D+00 | 4.19891D-06 | -1.59945D-01 |
| R( 11) | 4 - 4 | 3315.45 | -12.53 | 1.01253D-03 | 9.99992D-01 | -1.85016D+00 |
| R( 12) | 4 - 0 | 446.06 | -2895.48 | 7.20994D-03 | 2.71677D-12 | -1.40247D-03 |
| P( 14) | 4 - 0 | 475.59 | -2865.96 | 7.51091D-03 | 2.97088D-12 | -1.40074D-03 |
| R( 12) | 4 - 1 | 1170.29 | -2171.26 | 2.04708D-03 | 2.64111D-10 | -1.15083D-03 |
| P( 14) | 4 - 1 | 1199.41 | -2142.13 | 2.29688D-03 | 2.88864D-10 | -1.19871D-03 |
| R( 12) | 4 - 2 | 1896.63 | -1444.92 | 3.77647D-02 | 2.49674D-08 | -9.10518D-03 |
| P( 14) | 4 - 2 | 1925.42 | -1416.12 | 3.81899D-02 | 2.76063D-08 | -9.09371D-03 |
| R( 12) | 4 - 3 | 2614.07 | -727.47 | 1.35279D+00 | 4.19588D-06 | -1.52545D-01 |
| P( 14) | 4 - 3 | 2642.56 | -698.98 | 1.42722D+00 | 4.87158D-06 | -1.60311D-01 |
| R( 12) | 4 - 4 | 3327.98 | -13.57 | 1.29118D-03 | 9.99991D-01 | -1.85035D+00 |
| R( 13) | 4 - 0 | 460.28 | -2895.87 | 7.22255D-03 | 3.16642D-12 | -1.40155D-03 |
| P( 15) | 4 - 0 | 491.99 | -2864.16 | 7.46726D-03 | 3.41269D-12 | -1.39970D-03 |
| R( 13) | 4 - 1 | 1184.31 | -2171.84 | 2.06694D-03 | 3.07094D-10 | -1.15440D-03 |
| P( 15) | 4 - 1 | 1215.59 | -2140.57 | 2.31362D-03 | 3.31014D-10 | -1.20588D-03 |
| R( 13) | 4 - 2 | 1910.49 | -1445.66 | 3.80620D-02 | 2.90103D-08 | -9.12180D-03 |
| P( 15) | 4 - 2 | 1941.42 | -1414.73 | 3.81186D-02 | 3.16375D-08 | -9.10980D-03 |
| R( 13) | 4 - 3 | 2627.79 | -728.36 | 1.35771D+00 | 4.86779D-06 | -1.52341D-01 |

| | | | | | | | |
|---|---|---|---|---|---|---|---|
| P( 15) | 4 - 3 | 2658.39 | -697.76 | 1.42287D+00 | 5.59462D-06 | -1.60684D-01 |
| R( 13) | 4 - 4 | 3341.54 | -14.61 | 1.61676D-03 | 9.99989D-01 | -1.85054D+00 |
| R( 14) | 4 - 0 | 475.59 | -2896.22 | 7.23137D-03 | 3.65361D-12 | -1.40055D-03 |
| P( 16) | 4 - 0 | 509.48 | -2862.32 | 7.42486D-03 | 3.88620D-12 | -1.39858D-03 |
| R( 14) | 4 - 1 | 1199.41 | -2172.39 | 2.08751D-03 | 3.53447D-10 | -1.15835D-03 |
| P( 16) | 4 - 1 | 1232.84 | -2138.97 | 2.33245D-03 | 3.75961D-10 | -1.21345D-03 |
| R( 14) | 4 - 2 | 1925.42 | -1446.38 | 3.83558D-02 | 3.33651D-08 | -9.13957D-03 |
| P( 16) | 4 - 2 | 1958.48 | -1413.33 | 3.80674D-02 | 3.59359D-08 | -9.12710D-03 |
| R( 14) | 4 - 3 | 2642.56 | -729.24 | 1.36220D+00 | 5.58996D-06 | -1.52142D-01 |
| P( 16) | 4 - 3 | 2675.27 | -696.53 | 1.41900D+00 | 6.36816D-06 | -1.61064D-01 |
| R( 14) | 4 - 4 | 3356.15 | -15.65 | 1.99290D-03 | 9.99987D-01 | -1.85076D+00 |
| R( 15) | 4 - 0 | 491.99 | -2896.51 | 7.23680D-03 | 4.17914D-12 | -1.39945D-03 |
| P( 17) | 4 - 0 | 528.06 | -2860.43 | 7.38321D-03 | 4.39177D-12 | -1.39735D-03 |
| R( 15) | 4 - 1 | 1215.59 | -2172.91 | 2.10892D-03 | 4.03202D-10 | -1.16269D-03 |
| P( 17) | 4 - 1 | 1251.17 | -2137.33 | 2.35326D-03 | 4.23695D-10 | -1.22140D-03 |
| R( 15) | 4 - 2 | 1941.42 | -1447.08 | 3.86484D-02 | 3.80335D-08 | -9.15849D-03 |
| P( 17) | 4 - 2 | 1976.60 | -1411.90 | 3.80339D-02 | 4.05003D-08 | -9.14562D-03 |
| R( 15) | 4 - 3 | 2658.39 | -730.11 | 1.36635D+00 | 6.36251D-06 | -1.51949D-01 |
| P( 17) | 4 - 3 | 2693.20 | -695.29 | 1.41552D+00 | 7.19232D-06 | -1.61449D-01 |
| R( 15) | 4 - 4 | 3371.80 | -16.69 | 2.42324D-03 | 9.99986D-01 | -1.85099D+00 |
| R( 16) | 4 - 0 | 509.48 | -2896.75 | 7.23914D-03 | 4.74384D-12 | -1.39825D-03 |
| P( 18) | 4 - 0 | 547.74 | -2858.49 | 7.34195D-03 | 4.92979D-12 | -1.39604D-03 |
| R( 16) | 4 - 1 | 1232.84 | -2173.39 | 2.13129D-03 | 4.56389D-10 | -1.16741D-03 |
| P( 18) | 4 - 1 | 1270.57 | -2135.66 | 2.37598D-03 | 4.74205D-10 | -1.22976D-03 |
| R( 16) | 4 - 2 | 1958.48 | -1447.75 | 3.89417D-02 | 4.30175D-08 | -9.17855D-03 |
| P( 18) | 4 - 2 | 1995.79 | -1410.44 | 3.80165D-02 | 4.53293D-08 | -9.16535D-03 |
| R( 16) | 4 - 3 | 2675.27 | -730.96 | 1.37021D+00 | 7.18553D-06 | -1.51761D-01 |
| P( 18) | 4 - 3 | 2712.19 | -694.04 | 1.41236D+00 | 8.06722D-06 | -1.61841D-01 |
| R( 16) | 4 - 4 | 3388.50 | -17.73 | 2.91140D-03 | 9.99984D-01 | -1.85123D+00 |

| | | | | | | | |
|---|---|---|---|---|---|---|---|
| R( 17) | 4 - 0 | 528.06 | -2896.94 | 7.23862D-03 | 5.34860D-12 | -1.39695D-03 |
| P( 19) | 4 - 0 | 568.50 | -2856.51 | 7.30078D-03 | 5.50069D-12 | -1.39462D-03 |
| R( 17) | 4 - 1 | 1251.17 | -2173.84 | 2.15472D-03 | 5.13039D-10 | -1.17251D-03 |
| P( 19) | 4 - 1 | 1291.05 | -2133.96 | 2.40055D-03 | 5.27482D-10 | -1.23851D-03 |
| R( 17) | 4 - 2 | 1976.60 | -1448.40 | 3.92369D-02 | 4.83188D-08 | -9.19976D-03 |
| P( 19) | 4 - 2 | 2016.04 | -1408.97 | 3.80138D-02 | 5.04216D-08 | -9.18631D-03 |
| R( 17) | 4 - 3 | 2693.20 | -731.80 | 1.37384D+00 | 8.05916D-06 | -1.51580D-01 |
| P( 19) | 4 - 3 | 2732.22 | -692.78 | 1.40947D+00 | 8.99301D-06 | -1.62240D-01 |
| R( 17) | 4 - 4 | 3406.23 | -18.77 | 3.46101D-03 | 9.99982D-01 | -1.85149D+00 |
| R( 18) | 4 - 0 | 547.74 | -2897.08 | 7.23541D-03 | 5.99433D-12 | -1.39555D-03 |
| P( 20) | 4 - 0 | 590.35 | -2854.47 | 7.25944D-03 | 6.10492D-12 | -1.39309D-03 |
| R( 18) | 4 - 1 | 1270.57 | -2174.25 | 2.17928D-03 | 5.73185D-10 | -1.17801D-03 |
| P( 20) | 4 - 1 | 1312.60 | -2132.22 | 2.42694D-03 | 5.83517D-10 | -1.24766D-03 |
| R( 18) | 4 - 2 | 1995.79 | -1449.03 | 3.95354D-02 | 5.39394D-08 | -9.22211D-03 |
| P( 20) | 4 - 2 | 2037.35 | -1407.47 | 3.80247D-02 | 5.57760D-08 | -9.20850D-03 |
| R( 18) | 4 - 3 | 2712.19 | -732.63 | 1.37729D+00 | 8.98353D-06 | -1.51404D-01 |
| P( 20) | 4 - 3 | 2753.31 | -691.51 | 1.40681D+00 | 9.96984D-06 | -1.62644D-01 |
| R( 18) | 4 - 4 | 3425.01 | -19.81 | 4.07569D-03 | 9.99980D-01 | -1.85176D+00 |
| R( 19) | 4 - 0 | 568.50 | -2897.18 | 7.22964D-03 | 6.68201D-12 | -1.39403D-03 |
| P( 21) | 4 - 0 | 613.29 | -2852.39 | 7.21773D-03 | 6.74298D-12 | -1.39145D-03 |
| R( 19) | 4 - 1 | 1291.05 | -2174.62 | 2.20505D-03 | 6.36860D-10 | -1.18388D-03 |
| P( 21) | 4 - 1 | 1335.23 | -2130.45 | 2.45511D-03 | 6.42301D-10 | -1.25722D-03 |
| R( 19) | 4 - 2 | 2016.04 | -1449.64 | 3.98380D-02 | 5.98813D-08 | -9.24560D-03 |
| P( 21) | 4 - 2 | 2059.72 | -1405.96 | 3.80484D-02 | 6.13912D-08 | -9.23193D-03 |
| R( 19) | 4 - 3 | 2732.22 | -733.45 | 1.38057D+00 | 9.95877D-06 | -1.51234D-01 |
| P( 21) | 4 - 3 | 2775.45 | -690.22 | 1.40436D+00 | 1.09979D-05 | -1.63056D-01 |
| R( 19) | 4 - 4 | 3444.82 | -20.85 | 4.75907D-03 | 9.99978D-01 | -1.85205D+00 |
| P( 1) | 5 - 0 | 361.81 | -3595.83 | 4.88684D-03 | 9.84277D-17 | -5.78915D-04 |
| P( 1) | 5 - 1 | 1087.20 | -2870.44 | 1.40430D-02 | 4.91437D-14 | 1.37596D-03 |

| | | | | | | | |
|---|---|---|---|---|---|---|---|
| P( 1) | 5 - 2 | 1814.47 | -2143.17 | 1.57728D-02 | 3.50675D-12 | 2.26030D-03 |
| P( 1) | 5 - 3 | 2532.78 | -1424.87 | 1.74031D-01 | 2.31610D-10 | 1.38501D-02 |
| P( 1) | 5 - 4 | 3247.59 | -710.06 | 3.83520D+00 | 3.03343D-08 | 1.84822D-01 |
| R( 0) | 5 - 0 | 360.72 | -3597.96 | 1.63426D-03 | 1.00611D-16 | -5.79343D-04 |
| P( 2) | 5 - 0 | 364.00 | -3594.67 | 3.25595D-03 | 3.90032D-16 | -5.79021D-04 |
| R( 0) | 5 - 1 | 1086.12 | -2872.56 | 4.69079D-03 | 4.94649D-14 | 1.37588D-03 |
| P( 2) | 5 - 1 | 1089.36 | -2869.32 | 9.34977D-03 | 1.95941D-13 | 1.37587D-03 |
| R( 0) | 5 - 2 | 1813.40 | -2145.27 | 5.24632D-03 | 3.52399D-12 | 2.25456D-03 |
| P( 2) | 5 - 2 | 1816.60 | -2142.07 | 1.05291D-02 | 1.39923D-11 | 2.26355D-03 |
| R( 0) | 5 - 3 | 2531.72 | -1426.96 | 5.82673D-02 | 2.32465D-10 | 1.38502D-02 |
| P( 2) | 5 - 3 | 2534.89 | -1423.79 | 1.15787D-01 | 9.24745D-10 | 1.38518D-02 |
| R( 0) | 5 - 4 | 3246.54 | -712.13 | 1.28076D+00 | 3.03338D-08 | 1.84183D-01 |
| P( 2) | 5 - 4 | 3249.67 | -709.00 | 2.55452D+00 | 1.21342D-07 | 1.85152D-01 |
| R( 0) | 5 - 5 | 3957.64 | -1.03 | 4.12076D-07 | 1.00000D+00 | 1.88861D+00 |
| R( 1) | 5 - 0 | 361.81 | -3598.93 | 1.96633D-03 | 4.01795D-16 | -5.79878D-04 |
| P( 3) | 5 - 0 | 367.29 | -3593.46 | 2.93062D-03 | 8.77804D-16 | -5.79341D-04 |
| R( 1) | 5 - 1 | 1087.20 | -2873.55 | 5.63335D-03 | 1.98046D-13 | 1.37570D-03 |
| P( 3) | 5 - 1 | 1092.59 | -2868.15 | 8.40234D-03 | 4.40115D-13 | 1.37569D-03 |
| R( 1) | 5 - 2 | 1814.47 | -2146.28 | 6.29044D-03 | 1.41187D-11 | 2.25207D-03 |
| P( 3) | 5 - 2 | 1819.80 | -2140.94 | 9.49037D-03 | 3.14211D-11 | 2.26704D-03 |
| R( 1) | 5 - 3 | 2532.78 | -1427.97 | 7.00889D-02 | 9.31326D-10 | 1.38521D-02 |
| P( 3) | 5 - 3 | 2538.06 | -1422.69 | 1.04012D-01 | 2.07726D-09 | 1.38548D-02 |
| R( 1) | 5 - 4 | 3247.59 | -713.16 | 1.53836D+00 | 1.21328D-07 | 1.83874D-01 |
| P( 3) | 5 - 4 | 3252.81 | -707.94 | 2.29705D+00 | 2.73049D-07 | 1.85489D-01 |
| R( 1) | 5 - 5 | 3958.68 | -2.07 | 3.95584D-06 | 1.00000D+00 | 1.88863D+00 |
| R( 2) | 5 - 0 | 364.00 | -3599.84 | 2.11382D-03 | 9.11436D-16 | -5.80626D-04 |
| P( 4) | 5 - 0 | 371.66 | -3592.18 | 2.79323D-03 | 1.55514D-15 | -5.79875D-04 |
| R( 2) | 5 - 1 | 1089.36 | -2874.49 | 6.03940D-03 | 4.46710D-13 | 1.37545D-03 |
| P( 4) | 5 - 1 | 1096.91 | -2866.93 | 7.98899D-03 | 7.80492D-13 | 1.37543D-03 |

| | | | | | | | |
|---|---|---|---|---|---|---|---|
| R( 2) | 5 - 2 | 1816.60 | -2147.24 | 6.73539D-03 | 3.18352D-11 | 2.24982D-03 |
| P( 4) | 5 - 2 | 1824.07 | -2139.77 | 9.05346D-03 | 5.57344D-11 | 2.27078D-03 |
| R( 2) | 5 - 3 | 2534.89 | -1428.96 | 7.52854D-02 | 2.09919D-09 | 1.38552D-02 |
| P( 4) | 5 - 3 | 2542.28 | -1421.56 | 9.88851D-02 | 3.68654D-09 | 1.38590D-02 |
| R( 2) | 5 - 4 | 3249.67 | -714.17 | 1.64984D+00 | 2.72993D-07 | 1.83571D-01 |
| P( 4) | 5 - 4 | 3256.98 | -706.86 | 2.18578D+00 | 4.85472D-07 | 1.85832D-01 |
| R( 2) | 5 - 5 | 3960.74 | -3.10 | 1.43043D-05 | 9.99999D-01 | 1.88867D+00 |
| R( 3) | 5 - 0 | 367.29 | -3600.69 | 2.20094D-03 | 1.63486D-15 | -5.81588D-04 |
| P( 5) | 5 - 0 | 377.14 | -3590.84 | 2.71960D-03 | 2.42343D-15 | -5.80622D-04 |
| R( 3) | 5 - 1 | 1092.59 | -2875.38 | 6.26577D-03 | 7.96125D-13 | 1.37510D-03 |
| P( 5) | 5 - 1 | 1102.31 | -2865.67 | 7.75286D-03 | 1.21650D-12 | 1.37508D-03 |
| R( 3) | 5 - 2 | 1819.80 | -2148.18 | 6.98151D-03 | 5.67162D-11 | 2.24781D-03 |
| P( 5) | 5 - 2 | 1829.41 | -2138.57 | 8.81805D-03 | 8.68881D-11 | 2.27476D-03 |
| R( 3) | 5 - 3 | 2538.06 | -1429.92 | 7.82813D-02 | 3.73852D-09 | 1.38596D-02 |
| P( 5) | 5 - 3 | 2547.56 | -1420.42 | 9.59819D-02 | 5.75031D-09 | 1.38645D-02 |
| R( 3) | 5 - 4 | 3252.81 | -715.17 | 1.71262D+00 | 4.85339D-07 | 1.83276D-01 |
| P( 5) | 5 - 4 | 3262.21 | -705.77 | 2.12327D+00 | 7.58645D-07 | 1.86183D-01 |
| R( 3) | 5 - 5 | 3963.84 | -4.14 | 3.51614D-05 | 9.99999D-01 | 1.88873D+00 |
| R( 4) | 5 - 0 | 371.66 | -3601.48 | 2.26155D-03 | 2.57934D-15 | -5.82761D-04 |
| P( 6) | 5 - 0 | 383.70 | -3589.45 | 2.67586D-03 | 3.48326D-15 | -5.81581D-04 |
| R( 4) | 5 - 1 | 1096.91 | -2876.24 | 6.40979D-03 | 1.24704D-12 | 1.37466D-03 |
| P( 6) | 5 - 1 | 1108.78 | -2864.36 | 7.59663D-03 | 1.74744D-12 | 1.37464D-03 |
| R( 4) | 5 - 2 | 1824.07 | -2149.08 | 7.13796D-03 | 8.88058D-11 | 2.24605D-03 |
| P( 6) | 5 - 2 | 1835.81 | -2137.34 | 8.67495D-03 | 1.24834D-10 | 2.27900D-03 |
| R( 4) | 5 - 3 | 2542.28 | -1430.87 | 8.02835D-02 | 5.85184D-09 | 1.38651D-02 |
| P( 6) | 5 - 3 | 2553.90 | -1419.25 | 9.40958D-02 | 8.26625D-09 | 1.38712D-02 |
| R( 4) | 5 - 4 | 3256.98 | -716.16 | 1.75330D+00 | 7.58385D-07 | 1.82987D-01 |
| P( 6) | 5 - 4 | 3268.47 | -704.68 | 2.08294D+00 | 1.09261D-06 | 1.86540D-01 |
| R( 4) | 5 - 5 | 3967.98 | -5.17 | 7.02330D-05 | 9.99998D-01 | 1.88880D+00 |

| | | | | | | | |
|---|---|---|---|---|---|---|---|
| R( 5) | 5 - 0 | 377.14 | -3602.21 | 2.30868D-03 | 3.75323D-15 | -5.84147D-04 |
| P( 7) | 5 - 0 | 391.36 | -3587.99 | 2.64898D-03 | 4.73619D-15 | -5.82752D-04 |
| R( 5) | 5 - 1 | 1102.31 | -2877.04 | 6.50887D-03 | 1.80021D-12 | 1.37413D-03 |
| P( 7) | 5 - 1 | 1116.34 | -2863.01 | 7.48286D-03 | 2.37258D-12 | 1.37411D-03 |
| R( 5) | 5 - 2 | 1829.41 | -2149.94 | 7.24674D-03 | 1.28148D-10 | 2.24454D-03 |
| P( 7) | 5 - 2 | 1843.28 | -2136.07 | 8.58215D-03 | 1.69522D-10 | 2.28348D-03 |
| R( 5) | 5 - 3 | 2547.56 | -1431.79 | 8.17561D-02 | 8.44173D-09 | 1.38719D-02 |
| P( 7) | 5 - 3 | 2561.29 | -1418.06 | 9.27625D-02 | 1.12321D-08 | 1.38792D-02 |
| R( 5) | 5 - 4 | 3262.21 | -717.15 | 1.78209D+00 | 1.09216D-06 | 1.82705D-01 |
| P( 7) | 5 - 4 | 3275.78 | -703.57 | 2.05457D+00 | 1.48741D-06 | 1.86905D-01 |
| R( 5) | 5 - 5 | 3973.15 | -6.20 | 1.23225D-04 | 9.99998D-01 | 1.88889D+00 |
| R( 6) | 5 - 0 | 383.70 | -3602.88 | 2.34842D-03 | 5.16605D-15 | -5.85744D-04 |
| P( 8) | 5 - 0 | 400.12 | -3586.47 | 2.63287D-03 | 6.18474D-15 | -5.84135D-04 |
| R( 6) | 5 - 1 | 1108.78 | -2877.80 | 6.58047D-03 | 2.45639D-12 | 1.37351D-03 |
| P( 8) | 5 - 1 | 1124.97 | -2861.61 | 7.39409D-03 | 3.09124D-12 | 1.37349D-03 |
| R( 6) | 5 - 2 | 1835.81 | -2150.77 | 7.32743D-03 | 1.74785D-10 | 2.24326D-03 |
| P( 8) | 5 - 2 | 1851.82 | -2134.77 | 8.52005D-03 | 2.20903D-10 | 2.28820D-03 |
| R( 6) | 5 - 3 | 2553.90 | -1432.69 | 8.29158D-02 | 1.15108D-08 | 1.38799D-02 |
| P( 8) | 5 - 3 | 2569.73 | -1416.85 | 9.17656D-02 | 1.46455D-08 | 1.38884D-02 |
| R( 6) | 5 - 4 | 3268.47 | -718.12 | 1.80377D+00 | 1.48669D-06 | 1.82429D-01 |
| P( 8) | 5 - 4 | 3284.13 | -702.45 | 2.03338D+00 | 1.94310D-06 | 1.87276D-01 |
| R( 6) | 5 - 5 | 3979.35 | -7.24 | 1.97840D-04 | 9.99997D-01 | 1.88900D+00 |
| R( 7) | 5 - 0 | 391.36 | -3603.49 | 2.38400D-03 | 6.82847D-15 | -5.87552D-04 |
| P( 9) | 5 - 0 | 409.96 | -3584.89 | 2.62432D-03 | 7.83246D-15 | -5.85728D-04 |
| R( 7) | 5 - 1 | 1116.34 | -2878.52 | 6.63383D-03 | 3.21635D-12 | 1.37280D-03 |
| P( 9) | 5 - 1 | 1134.68 | -2860.17 | 7.32105D-03 | 3.90271D-12 | 1.37278D-03 |
| R( 7) | 5 - 2 | 1843.28 | -2151.57 | 7.39040D-03 | 2.28760D-10 | 2.24222D-03 |
| P( 9) | 5 - 2 | 1861.42 | -2133.43 | 8.47826D-03 | 2.78927D-10 | 2.29317D-03 |
| R( 7) | 5 - 3 | 2561.29 | -1433.57 | 8.38772D-02 | 1.50616D-08 | 1.38890D-02 |

| | | | | | | |
|---|---|---|---|---|---|---|
| P( 9) | 5 - 3 | 2579.24 | -1415.62 | 9.09902D-02 | 1.85042D-08 | 1.38989D-02 |
| R( 7) | 5 - 4 | 3275.78 | -719.08 | 1.82085D+00 | 1.94203D-06 | 1.82160D-01 |
| P( 9) | 5 - 4 | 3293.53 | -701.33 | 2.01685D+00 | 2.45974D-06 | 1.87654D-01 |
| R( 7) | 5 - 5 | 3986.59 | -8.27 | 2.97783D-04 | 9.99996D-01 | 1.88912D+00 |
| R( 8) | 5 - 0 | 400.12 | -3604.04 | 2.41730D-03 | 8.75244D-15 | -5.89569D-04 |
| P( 10) | 5 - 0 | 420.90 | -3583.25 | 2.62145D-03 | 9.68392D-15 | -5.87530D-04 |
| R( 8) | 5 - 1 | 1124.97 | -2879.19 | 6.67426D-03 | 4.08088D-12 | 1.37199D-03 |
| P( 10) | 5 - 1 | 1145.47 | -2858.68 | 7.25839D-03 | 4.80630D-12 | 1.37198D-03 |
| R( 8) | 5 - 2 | 1851.82 | -2152.34 | 7.44164D-03 | 2.90115D-10 | 2.24142D-03 |
| P( 10) | 5 - 2 | 1872.09 | -2132.07 | 8.45075D-03 | 3.43544D-10 | 2.29838D-03 |
| R( 8) | 5 - 3 | 2569.73 | -1434.42 | 8.47068D-02 | 1.90968D-08 | 1.38994D-02 |
| P( 10) | 5 - 3 | 2589.79 | -1414.37 | 9.03701D-02 | 2.28060D-08 | 1.39106D-02 |
| R( 8) | 5 - 4 | 3284.13 | -720.02 | 1.83480D+00 | 2.45822D-06 | 1.81898D-01 |
| P( 10) | 5 - 4 | 3303.97 | -700.19 | 2.00351D+00 | 3.03740D-06 | 1.88039D-01 |
| R( 8) | 5 - 5 | 3994.86 | -9.30 | 4.26754D-04 | 9.99995D-01 | 1.88926D+00 |
| R( 9) | 5 - 0 | 409.96 | -3604.53 | 2.44946D-03 | 1.09512D-14 | -5.91794D-04 |
| P( 11) | 5 - 0 | 432.94 | -3581.56 | 2.62313D-03 | 1.17448D-14 | -5.89541D-04 |
| R( 9) | 5 - 1 | 1134.68 | -2879.81 | 6.70509D-03 | 5.05074D-12 | 1.37109D-03 |
| P( 11) | 5 - 1 | 1157.34 | -2857.15 | 7.20279D-03 | 5.80133D-12 | 1.37108D-03 |
| R( 9) | 5 - 2 | 1861.42 | -2153.07 | 7.48485D-03 | 3.58891D-10 | 2.24085D-03 |
| P( 11) | 5 - 2 | 1883.83 | -2130.66 | 8.43380D-03 | 4.14700D-10 | 2.30383D-03 |
| R( 9) | 5 - 3 | 2579.24 | -1435.26 | 8.54459D-02 | 2.36192D-08 | 1.39110D-02 |
| P( 11) | 5 - 3 | 2601.40 | -1413.09 | 8.98642D-02 | 2.75488D-08 | 1.39236D-02 |
| R( 9) | 5 - 4 | 3293.53 | -720.96 | 1.84654D+00 | 3.03532D-06 | 1.81643D-01 |
| P( 11) | 5 - 4 | 3315.45 | -699.04 | 1.99247D+00 | 3.67617D-06 | 1.88432D-01 |
| R( 9) | 5 - 5 | 4004.16 | -10.33 | 5.88451D-04 | 9.99993D-01 | 1.88942D+00 |
| R( 10) | 5 - 0 | 420.90 | -3604.96 | 2.48126D-03 | 1.34395D-14 | -5.94227D-04 |
| P( 12) | 5 - 0 | 446.06 | -3579.80 | 2.62858D-03 | 1.40218D-14 | -5.91759D-04 |
| R( 10) | 5 - 1 | 1145.47 | -2880.39 | 6.72844D-03 | 6.12674D-12 | 1.37009D-03 |

| | | | | | | | |
|---|---|---|---|---|---|---|---|
| P( 12) | 5 - 1 | 1170.29 | -2855.57 | 7.15207D-03 | 6.88712D-12 | 1.37009D-03 |
| R( 10) | 5 - 2 | 1872.09 | -2153.77 | 7.52244D-03 | 4.35129D-10 | 2.24051D-03 |
| P( 12) | 5 - 2 | 1896.63 | -2129.23 | 8.42496D-03 | 4.92345D-10 | 2.30952D-03 |
| R( 10) | 5 - 3 | 2589.79 | -1436.07 | 8.61212D-02 | 2.86314D-08 | 1.39239D-02 |
| P( 12) | 5 - 3 | 2614.07 | -1411.79 | 8.94455D-02 | 3.27301D-08 | 1.39379D-02 |
| R( 10) | 5 - 4 | 3303.97 | -721.89 | 1.85664D+00 | 3.67340D-06 | 1.81394D-01 |
| P( 12) | 5 - 4 | 3327.98 | -697.88 | 1.98313D+00 | 4.37611D-06 | 1.88831D-01 |
| R( 10) | 5 - 5 | 4014.49 | -11.37 | 7.86571D-04 | 9.99992D-01 | 1.88959D+00 |
| R( 11) | 5 - 0 | 432.94 | -3605.32 | 2.51321D-03 | 1.62333D-14 | -5.96865D-04 |
| P( 13) | 5 - 0 | 460.28 | -3577.98 | 2.63730D-03 | 1.65228D-14 | -5.94183D-04 |
| R( 11) | 5 - 1 | 1157.34 | -2880.92 | 6.74577D-03 | 7.30969D-12 | 1.36898D-03 |
| P( 13) | 5 - 1 | 1184.31 | -2853.95 | 7.10476D-03 | 8.06303D-12 | 1.36900D-03 |
| R( 11) | 5 - 2 | 1883.83 | -2154.43 | 7.55604D-03 | 5.18870D-10 | 2.24040D-03 |
| P( 13) | 5 - 2 | 1910.49 | -2127.76 | 8.42256D-03 | 5.76427D-10 | 2.31544D-03 |
| R( 11) | 5 - 3 | 2601.40 | -1436.85 | 8.67510D-02 | 3.41361D-08 | 1.39379D-02 |
| P( 13) | 5 - 3 | 2627.79 | -1410.47 | 8.90959D-02 | 3.83480D-08 | 1.39534D-02 |
| R( 11) | 5 - 4 | 3315.45 | -722.81 | 1.86551D+00 | 4.37251D-06 | 1.81152D-01 |
| P( 13) | 5 - 4 | 3341.54 | -696.71 | 1.97508D+00 | 5.13734D-06 | 1.89238D-01 |
| R( 11) | 5 - 5 | 4025.86 | -12.40 | 1.02481D-03 | 9.99990D-01 | 1.88978D+00 |
| R( 12) | 5 - 0 | 446.06 | -3605.63 | 2.54568D-03 | 1.93504D-14 | -5.99708D-04 |
| P( 14) | 5 - 0 | 475.59 | -3576.10 | 2.64893D-03 | 1.92571D-14 | -5.96812D-04 |
| R( 12) | 5 - 1 | 1170.29 | -2881.40 | 6.75808D-03 | 8.60041D-12 | 1.36778D-03 |
| P( 14) | 5 - 1 | 1199.41 | -2852.28 | 7.05981D-03 | 9.32838D-12 | 1.36781D-03 |
| R( 12) | 5 - 2 | 1896.63 | -2155.06 | 7.58678D-03 | 6.10153D-10 | 2.24052D-03 |
| P( 14) | 5 - 2 | 1925.42 | -2126.26 | 8.42542D-03 | 6.66890D-10 | 2.32159D-03 |
| R( 12) | 5 - 3 | 2614.07 | -1437.62 | 8.73484D-02 | 4.01362D-08 | 1.39531D-02 |
| P( 14) | 5 - 3 | 2642.56 | -1409.13 | 8.88027D-02 | 4.44002D-08 | 1.39703D-02 |
| R( 12) | 5 - 4 | 3327.98 | -723.71 | 1.87344D+00 | 5.13276D-06 | 1.80917D-01 |
| P( 14) | 5 - 4 | 3356.15 | -695.54 | 1.96805D+00 | 5.95993D-06 | 1.89651D-01 |

| | | | | | | | |
|---|---|---|---|---|---|---|---|
| R( 12) | 5 - 5 | 4038.26 | -13.43 | 1.30685D-03 | 9.99989D-01 | 1.88999D+00 |
| R( 13) | 5 - 0 | 460.28 | -3605.87 | 2.57895D-03 | 2.28102D-14 | -6.02753D-04 |
| P( 15) | 5 - 0 | 491.99 | -3574.16 | 2.66320D-03 | 2.22350D-14 | -5.99643D-04 |
| R( 13) | 5 - 1 | 1184.31 | -2881.84 | 6.76611D-03 | 9.99972D-12 | 1.36646D-03 |
| P( 15) | 5 - 1 | 1215.59 | -2850.57 | 7.01646D-03 | 1.06826D-11 | 1.36652D-03 |
| R( 13) | 5 - 2 | 1910.49 | -2155.66 | 7.61550D-03 | 7.09018D-10 | 2.24085D-03 |
| P( 15) | 5 - 2 | 1941.42 | -2124.73 | 8.43267D-03 | 7.63682D-10 | 2.32798D-03 |
| R( 13) | 5 - 3 | 2627.79 | -1438.36 | 8.79226D-02 | 4.66344D-08 | 1.39695D-02 |
| P( 15) | 5 - 3 | 2658.39 | -1407.76 | 8.85564D-02 | 5.08845D-08 | 1.39884D-02 |
| R( 13) | 5 - 4 | 3341.54 | -724.61 | 1.88063D+00 | 5.95422D-06 | 1.80688D-01 |
| P( 15) | 5 - 4 | 3371.80 | -694.35 | 1.96183D+00 | 6.84402D-06 | 1.90072D-01 |
| R( 13) | 5 - 5 | 4051.69 | -14.46 | 1.63639D-03 | 9.99987D-01 | 1.89021D+00 |
| R( 14) | 5 - 0 | 475.59 | -3606.06 | 2.61321D-03 | 2.66338D-14 | -6.06000D-04 |
| P( 16) | 5 - 0 | 509.48 | -3572.16 | 2.67992D-03 | 2.54682D-14 | -6.02675D-04 |
| R( 14) | 5 - 1 | 1199.41 | -2882.24 | 6.77038D-03 | 1.15085D-11 | 1.36504D-03 |
| P( 16) | 5 - 1 | 1232.84 | -2848.81 | 6.97414D-03 | 1.21249D-11 | 1.36512D-03 |
| R( 14) | 5 - 2 | 1925.42 | -2156.22 | 7.64277D-03 | 8.15503D-10 | 2.24140D-03 |
| P( 16) | 5 - 2 | 1958.48 | -2123.17 | 8.44367D-03 | 8.66749D-10 | 2.33458D-03 |
| R( 14) | 5 - 3 | 2642.56 | -1439.08 | 8.84806D-02 | 5.36336D-08 | 1.39872D-02 |
| P( 16) | 5 - 3 | 2675.27 | -1406.38 | 8.83502D-02 | 5.77988D-08 | 1.40079D-02 |
| R( 14) | 5 - 4 | 3356.15 | -725.49 | 1.88722D+00 | 6.83698D-06 | 1.80467D-01 |
| P( 16) | 5 - 4 | 3388.50 | -693.15 | 1.95627D+00 | 7.78970D-06 | 1.90500D-01 |
| R( 14) | 5 - 5 | 4066.15 | -15.49 | 2.01710D-03 | 9.99985D-01 | 1.89045D+00 |
| R( 15) | 5 - 0 | 491.99 | -3606.18 | 2.64862D-03 | 3.08442D-14 | -6.09445D-04 |
| P( 17) | 5 - 0 | 528.06 | -3570.11 | 2.69893D-03 | 2.89701D-14 | -6.05907D-04 |
| R( 15) | 5 - 1 | 1215.59 | -2882.58 | 6.77128D-03 | 1.31276D-11 | 1.36351D-03 |
| P( 17) | 5 - 1 | 1251.17 | -2847.00 | 6.93240D-03 | 1.36549D-11 | 1.36361D-03 |
| R( 15) | 5 - 2 | 1941.42 | -2156.75 | 7.66906D-03 | 9.29646D-10 | 2.24216D-03 |
| P( 17) | 5 - 2 | 1976.60 | -2121.57 | 8.45791D-03 | 9.76034D-10 | 2.34141D-03 |

| | | | | | | | |
|---|---|---|---|---|---|---|---|
| R( 15) | 5 - 3 | 2658.39 | -1439.78 | 8.90278D-02 | 6.11366D-08 | 1.40060D-02 |
| P( 17) | 5 - 3 | 2693.20 | -1404.97 | 8.81790D-02 | 6.51410D-08 | 1.40286D-02 |
| R( 15) | 5 - 4 | 3371.80 | -726.37 | 1.89335D+00 | 7.78116D-06 | 1.80251D-01 |
| P( 17) | 5 - 4 | 3406.23 | -691.94 | 1.95125D+00 | 8.79712D-06 | 1.90935D-01 |
| R( 15) | 5 - 5 | 4081.65 | -16.52 | 2.45267D-03 | 9.99983D-01 | 1.89070D+00 |
| R( 16) | 5 - 0 | 509.48 | -3606.24 | 2.68530D-03 | 3.54665D-14 | -6.13087D-04 |
| P( 18) | 5 - 0 | 547.74 | -3567.99 | 2.72013D-03 | 3.27553D-14 | -6.09335D-04 |
| R( 16) | 5 - 1 | 1232.84 | -2882.89 | 6.76912D-03 | 1.48579D-11 | 1.36186D-03 |
| P( 18) | 5 - 1 | 1270.57 | -2845.15 | 6.89092D-03 | 1.52718D-11 | 1.36200D-03 |
| R( 16) | 5 - 2 | 1958.48 | -2157.25 | 7.69469D-03 | 1.05149D-09 | 2.24313D-03 |
| P( 18) | 5 - 2 | 1995.79 | -2119.94 | 8.47499D-03 | 1.09148D-09 | 2.34845D-03 |
| R( 16) | 5 - 3 | 2675.27 | -1440.45 | 8.95682D-02 | 6.91464D-08 | 1.40261D-02 |
| P( 18) | 5 - 3 | 2712.19 | -1403.54 | 8.80387D-02 | 7.29089D-08 | 1.40507D-02 |
| R( 16) | 5 - 4 | 3388.50 | -727.23 | 1.89909D+00 | 8.78687D-06 | 1.80043D-01 |
| P( 18) | 5 - 4 | 3425.01 | -690.72 | 1.94668D+00 | 9.86639D-06 | 1.91378D-01 |
| R( 16) | 5 - 5 | 4098.17 | -17.55 | 2.94677D-03 | 9.99980D-01 | 1.89098D+00 |
| R( 17) | 5 - 0 | 528.06 | -3606.25 | 2.72334D-03 | 4.05280D-14 | -6.16924D-04 |
| P( 19) | 5 - 0 | 568.50 | -3565.81 | 2.74341D-03 | 3.68402D-14 | -6.12958D-04 |
| R( 17) | 5 - 1 | 1251.17 | -2883.14 | 6.76412D-03 | 1.67004D-11 | 1.36010D-03 |
| P( 19) | 5 - 1 | 1291.05 | -2843.26 | 6.84941D-03 | 1.69752D-11 | 1.36027D-03 |
| R( 17) | 5 - 2 | 1976.60 | -2157.71 | 7.71992D-03 | 1.18106D-09 | 2.24430D-03 |
| P( 19) | 5 - 2 | 2016.04 | -2118.27 | 8.49462D-03 | 1.21304D-09 | 2.35571D-03 |
| R( 17) | 5 - 3 | 2693.20 | -1441.11 | 9.01052D-02 | 7.76657D-08 | 1.40473D-02 |
| P( 19) | 5 - 3 | 2732.22 | -1402.08 | 8.79261D-02 | 8.11004D-08 | 1.40741D-02 |
| R( 17) | 5 - 4 | 3406.23 | -728.08 | 1.90451D+00 | 9.85421D-06 | 1.79841D-01 |
| P( 19) | 5 - 4 | 3444.82 | -689.49 | 1.94249D+00 | 1.09977D-05 | 1.91827D-01 |
| R( 17) | 5 - 5 | 4115.72 | -18.58 | 3.50307D-03 | 9.99978D-01 | 1.89127D+00 |
| R( 18) | 5 - 0 | 547.74 | -3606.19 | 2.76283D-03 | 4.60582D-14 | -6.20954D-04 |
| P( 20) | 5 - 0 | 590.35 | -3563.57 | 2.76871D-03 | 4.12427D-14 | -6.16774D-04 |

| | | | | | | | |
|---|---|---|---|---|---|---|---|
| R( 18) | 5 - 1 | 1270.57 | -2883.35 | 6.75644D-03 | 1.86560D-11 | 1.35821D-03 |
| P( 20) | 5 - 1 | 1312.60 | -2841.32 | 6.80765D-03 | 1.87644D-11 | 1.35842D-03 |
| R( 18) | 5 - 2 | 1995.79 | -2158.14 | 7.74494D-03 | 1.31840D-09 | 2.24567D-03 |
| P( 20) | 5 - 2 | 2037.35 | -2116.58 | 8.51651D-03 | 1.34064D-09 | 2.36317D-03 |
| R( 18) | 5 - 3 | 2712.19 | -1441.74 | 9.06412D-02 | 8.66977D-08 | 1.40698D-02 |
| P( 20) | 5 - 3 | 2753.31 | -1400.61 | 8.78388D-02 | 8.97133D-08 | 1.40988D-02 |
| R( 18) | 5 - 4 | 3425.01 | -728.92 | 1.90968D+00 | 1.09833D-05 | 1.79646D-01 |
| P( 20) | 5 - 4 | 3465.67 | -688.25 | 1.93863D+00 | 1.21911D-05 | 1.92284D-01 |
| R( 18) | 5 - 5 | 4134.31 | -19.61 | 4.12524D-03 | 9.99976D-01 | 1.89157D+00 |
| R( 19) | 5 - 0 | 568.50 | -3606.07 | 2.80382D-03 | 5.20892D-14 | -6.25173D-04 |
| P( 21) | 5 - 0 | 613.29 | -3561.28 | 2.79596D-03 | 4.59828D-14 | -6.20779D-04 |
| R( 19) | 5 - 1 | 1291.05 | -2883.52 | 6.74622D-03 | 2.07256D-11 | 1.35619D-03 |
| P( 21) | 5 - 1 | 1335.23 | -2839.34 | 6.76547D-03 | 2.06391D-11 | 1.35645D-03 |
| R( 19) | 5 - 2 | 2016.04 | -2158.53 | 7.76990D-03 | 1.46355D-09 | 2.24722D-03 |
| P( 21) | 5 - 2 | 2059.72 | -2114.85 | 8.54046D-03 | 1.47424D-09 | 2.37084D-03 |
| R( 19) | 5 - 3 | 2732.22 | -1442.34 | 9.11786D-02 | 9.62453D-08 | 1.40935D-02 |
| P( 21) | 5 - 3 | 2775.45 | -1399.12 | 8.77748D-02 | 9.87456D-08 | 1.41249D-02 |
| R( 19) | 5 - 4 | 3444.82 | -729.75 | 1.91464D+00 | 1.21744D-05 | 1.79457D-01 |
| P( 21) | 5 - 4 | 3487.57 | -687.00 | 1.93505D+00 | 1.34468D-05 | 1.92749D-01 |
| R( 19) | 5 - 5 | 4153.92 | -20.64 | 4.81695D-03 | 9.99973D-01 | 1.89189D+00 |
| Q( 0) | 0 - 0 | 360.72 | 0.00 | 0.00000D+00 | 1.00000D+00 | -1.71342D+00 |
| Q( 1) | 0 - 0 | 361.81 | -0.00 | 0.00000D+00 | 1.00000D+00 | -1.71343D+00 |
| Q( 2) | 0 - 0 | 364.00 | 0.00 | 0.00000D+00 | 1.00000D+00 | -1.71346D+00 |
| Q( 3) | 0 - 0 | 367.29 | 0.00 | 0.00000D+00 | 1.00000D+00 | -1.71349D+00 |
| Q( 4) | 0 - 0 | 371.66 | 0.00 | 0.00000D+00 | 1.00000D+00 | -1.71353D+00 |
| Q( 5) | 0 - 0 | 377.14 | 0.00 | 0.00000D+00 | 1.00000D+00 | -1.71359D+00 |
| Q( 6) | 0 - 0 | 383.70 | 0.00 | 0.00000D+00 | 1.00000D+00 | -1.71365D+00 |
| Q( 7) | 0 - 0 | 391.36 | 0.00 | 0.00000D+00 | 1.00000D+00 | -1.71373D+00 |
| Q( 8) | 0 - 0 | 400.12 | 0.00 | 0.00000D+00 | 1.00000D+00 | -1.71382D+00 |

| | | | | | | | |
|---|---|---|---|---|---|---|---|
| Q( 9) | 0 - 0 | 409.96 | 0.00 | 0.00000D+00 | 1.00000D+00 | -1.71392D+00 |
| Q( 10) | 0 - 0 | 420.90 | 0.00 | 0.00000D+00 | 1.00000D+00 | -1.71403D+00 |
| Q( 11) | 0 - 0 | 432.94 | 0.00 | 0.00000D+00 | 1.00000D+00 | -1.71415D+00 |
| Q( 12) | 0 - 0 | 446.06 | 0.00 | 0.00000D+00 | 1.00000D+00 | -1.71428D+00 |
| Q( 13) | 0 - 0 | 460.28 | -0.00 | 0.00000D+00 | 1.00000D+00 | -1.71442D+00 |
| Q( 14) | 0 - 0 | 475.59 | -0.00 | 0.00000D+00 | 1.00000D+00 | -1.71457D+00 |
| Q( 15) | 0 - 0 | 491.99 | -0.00 | 0.00000D+00 | 1.00000D+00 | -1.71474D+00 |
| Q( 16) | 0 - 0 | 509.48 | -0.00 | 0.00000D+00 | 1.00000D+00 | -1.71491D+00 |
| Q( 17) | 0 - 0 | 528.06 | -0.00 | 0.00000D+00 | 1.00000D+00 | -1.71510D+00 |
| Q( 18) | 0 - 0 | 547.74 | -0.00 | 0.00000D+00 | 1.00000D+00 | -1.71530D+00 |
| Q( 19) | 0 - 0 | 568.50 | -0.00 | 0.00000D+00 | 1.00000D+00 | -1.71551D+00 |
| Q( 20) | 0 - 0 | 590.35 | -0.00 | 0.00000D+00 | 1.00000D+00 | -1.71573D+00 |
| Q( 0) | 1 - 0 | 360.72 | -725.40 | 0.00000D+00 | 5.65695D-23 | 6.68672D-02 |
| Q( 0) | 1 - 1 | 1086.12 | 0.00 | 0.00000D+00 | 1.00000D+00 | 1.74369D+00 |
| Q( 1) | 1 - 0 | 361.81 | -725.38 | 0.00000D+00 | 9.50332D-18 | 6.68692D-02 |
| Q( 1) | 1 - 1 | 1087.20 | -0.00 | 0.00000D+00 | 1.00000D+00 | 1.74370D+00 |
| Q( 2) | 1 - 0 | 364.00 | -725.35 | 0.00000D+00 | 5.52257D-23 | 6.68731D-02 |
| Q( 2) | 1 - 1 | 1089.36 | 0.00 | 0.00000D+00 | 1.00000D+00 | 1.74372D+00 |
| Q( 3) | 1 - 0 | 367.29 | -725.31 | 0.00000D+00 | 5.52937D-23 | 6.68791D-02 |
| Q( 3) | 1 - 1 | 1092.59 | 0.00 | 0.00000D+00 | 1.00000D+00 | 1.74376D+00 |
| Q( 4) | 1 - 0 | 371.66 | -725.25 | 0.00000D+00 | 5.52145D-23 | 6.68869D-02 |
| Q( 4) | 1 - 1 | 1096.91 | 0.00 | 0.00000D+00 | 1.00000D+00 | 1.74380D+00 |
| Q( 5) | 1 - 0 | 377.14 | -725.17 | 0.00000D+00 | 5.64869D-23 | 6.68968D-02 |
| Q( 5) | 1 - 1 | 1102.31 | -0.00 | 0.00000D+00 | 1.00000D+00 | 1.74385D+00 |
| Q( 6) | 1 - 0 | 383.70 | -725.08 | 0.00000D+00 | 5.70601D-23 | 6.69086D-02 |
| Q( 6) | 1 - 1 | 1108.78 | -0.00 | 0.00000D+00 | 1.00000D+00 | 1.74392D+00 |
| Q( 7) | 1 - 0 | 391.36 | -724.98 | 0.00000D+00 | 5.86005D-23 | 6.69224D-02 |
| Q( 7) | 1 - 1 | 1116.34 | -0.00 | 0.00000D+00 | 1.00000D+00 | 1.74400D+00 |
| Q( 8) | 1 - 0 | 400.12 | -724.86 | 0.00000D+00 | 6.28518D-23 | 6.69382D-02 |

| | | | | | | | |
|---|---|---|---|---|---|---|---|
| Q( 8) | 1 - 1 | 1124.97 | -0.00 | 0.00000D+00 | 1.00000D+00 | 1.74408D+00 |
| Q( 9) | 1 - 0 | 409.96 | -724.72 | 0.00000D+00 | 6.62003D-23 | 6.69559D-02 |
| Q( 9) | 1 - 1 | 1134.68 | -0.00 | 0.00000D+00 | 1.00000D+00 | 1.74418D+00 |
| Q( 10) | 1 - 0 | 420.90 | -724.57 | 0.00000D+00 | 7.02501D-23 | 6.69756D-02 |
| Q( 10) | 1 - 1 | 1145.47 | -0.00 | 0.00000D+00 | 1.00000D+00 | 1.74429D+00 |
| Q( 11) | 1 - 0 | 432.94 | -724.41 | 0.00000D+00 | 7.62390D-23 | 6.69973D-02 |
| Q( 11) | 1 - 1 | 1157.34 | -0.00 | 0.00000D+00 | 1.00000D+00 | 1.74441D+00 |
| Q( 12) | 1 - 0 | 446.06 | -724.23 | 0.00000D+00 | 8.47455D-23 | 6.70210D-02 |
| Q( 12) | 1 - 1 | 1170.29 | -0.00 | 0.00000D+00 | 1.00000D+00 | 1.74454D+00 |
| Q( 13) | 1 - 0 | 460.28 | -724.03 | 0.00000D+00 | 9.54579D-23 | 6.70466D-02 |
| Q( 13) | 1 - 1 | 1184.31 | -0.00 | 0.00000D+00 | 1.00000D+00 | 1.74469D+00 |
| Q( 14) | 1 - 0 | 475.59 | -723.82 | 0.00000D+00 | 1.11173D-22 | 6.70743D-02 |
| Q( 14) | 1 - 1 | 1199.41 | -0.00 | 0.00000D+00 | 1.00000D+00 | 1.74484D+00 |
| Q( 15) | 1 - 0 | 491.99 | -723.60 | 0.00000D+00 | 1.50402D-22 | 6.71039D-02 |
| Q( 15) | 1 - 1 | 1215.59 | -0.00 | 0.00000D+00 | 1.00000D+00 | 1.74501D+00 |
| Q( 16) | 1 - 0 | 509.48 | -723.36 | 0.00000D+00 | 1.80900D-22 | 6.71355D-02 |
| Q( 16) | 1 - 1 | 1232.84 | -0.00 | 0.00000D+00 | 1.00000D+00 | 1.74518D+00 |
| Q( 17) | 1 - 0 | 528.06 | -723.10 | 0.00000D+00 | 2.25851D-22 | 6.71691D-02 |
| Q( 17) | 1 - 1 | 1251.17 | -0.00 | 0.00000D+00 | 1.00000D+00 | 1.74537D+00 |
| Q( 18) | 1 - 0 | 547.74 | -722.83 | 0.00000D+00 | 2.79445D-22 | 6.72047D-02 |
| Q( 18) | 1 - 1 | 1270.57 | -0.00 | 0.00000D+00 | 1.00000D+00 | 1.74557D+00 |
| Q( 19) | 1 - 0 | 568.50 | -722.55 | 0.00000D+00 | 3.50439D-22 | 6.72423D-02 |
| Q( 19) | 1 - 1 | 1291.05 | -0.00 | 0.00000D+00 | 1.00000D+00 | 1.74578D+00 |
| Q( 20) | 1 - 0 | 590.35 | -722.25 | 0.00000D+00 | 4.43931D-22 | 6.72819D-02 |
| Q( 20) | 1 - 1 | 1312.60 | -0.00 | 0.00000D+00 | 1.00000D+00 | 1.74600D+00 |
| Q( 0) | 2 - 0 | 360.72 | -1452.68 | 0.00000D+00 | 8.80413D-23 | -2.28844D-04 |
| Q( 0) | 2 - 1 | 1086.12 | -727.28 | 0.00000D+00 | 2.31299D-21 | -9.73543D-02 |
| Q( 0) | 2 - 2 | 1813.40 | 0.00 | 0.00000D+00 | 1.00000D+00 | -1.77572D+00 |
| Q( 1) | 2 - 0 | 361.81 | -1452.65 | 0.00000D+00 | 6.18634D-19 | -2.29036D-04 |

| | | | | | | | |
|---|---|---|---|---|---|---|---|
| Q( 1) | 2 - 1 | 1087.20 | -727.27 | 0.00000D+00 | 1.42461D-17 | -9.73577D-02 |
| Q( 1) | 2 - 2 | 1814.47 | -0.00 | 0.00000D+00 | 1.00000D+00 | -1.77573D+00 |
| Q( 2) | 2 - 0 | 364.00 | -1452.60 | 0.00000D+00 | 3.51176D-25 | -2.29417D-04 |
| Q( 2) | 2 - 1 | 1089.36 | -727.25 | 0.00000D+00 | 6.47941D-26 | -9.73646D-02 |
| Q( 2) | 2 - 2 | 1816.60 | 0.00 | 0.00000D+00 | 1.00000D+00 | -1.77576D+00 |
| Q( 3) | 2 - 0 | 367.29 | -1452.52 | 0.00000D+00 | 3.32465D-25 | -2.29992D-04 |
| Q( 3) | 2 - 1 | 1092.59 | -727.21 | 0.00000D+00 | 8.37006D-26 | -9.73748D-02 |
| Q( 3) | 2 - 2 | 1819.80 | 0.00 | 0.00000D+00 | 1.00000D+00 | -1.77579D+00 |
| Q( 4) | 2 - 0 | 371.66 | -1452.41 | 0.00000D+00 | 3.09932D-25 | -2.30761D-04 |
| Q( 4) | 2 - 1 | 1096.91 | -727.16 | 0.00000D+00 | 9.86970D-26 | -9.73885D-02 |
| Q( 4) | 2 - 2 | 1824.07 | 0.00 | 0.00000D+00 | 1.00000D+00 | -1.77585D+00 |
| Q( 5) | 2 - 0 | 377.14 | -1452.27 | 0.00000D+00 | 2.96968D-25 | -2.31727D-04 |
| Q( 5) | 2 - 1 | 1102.31 | -727.10 | 0.00000D+00 | 1.41223D-25 | -9.74057D-02 |
| Q( 5) | 2 - 2 | 1829.41 | 0.00 | 0.00000D+00 | 1.00000D+00 | -1.77591D+00 |
| Q( 6) | 2 - 0 | 383.70 | -1452.11 | 0.00000D+00 | 2.75625D-25 | -2.32891D-04 |
| Q( 6) | 2 - 1 | 1108.78 | -727.03 | 0.00000D+00 | 1.96384D-25 | -9.74262D-02 |
| Q( 6) | 2 - 2 | 1835.81 | 0.00 | 0.00000D+00 | 1.00000D+00 | -1.77599D+00 |
| Q( 7) | 2 - 0 | 391.36 | -1451.92 | 0.00000D+00 | 2.44227D-25 | -2.34257D-04 |
| Q( 7) | 2 - 1 | 1116.34 | -726.94 | 0.00000D+00 | 3.49808D-25 | -9.74502D-02 |
| Q( 7) | 2 - 2 | 1843.28 | 0.00 | 0.00000D+00 | 1.00000D+00 | -1.77608D+00 |
| Q( 8) | 2 - 0 | 400.12 | -1451.70 | 0.00000D+00 | 3.07727D-25 | -2.35829D-04 |
| Q( 8) | 2 - 1 | 1124.97 | -726.85 | 0.00000D+00 | 6.33954D-25 | -9.74777D-02 |
| Q( 8) | 2 - 2 | 1851.82 | 0.00 | 0.00000D+00 | 1.00000D+00 | -1.77618D+00 |
| Q( 9) | 2 - 0 | 409.96 | -1451.46 | 0.00000D+00 | 2.38371D-25 | -2.37611D-04 |
| Q( 9) | 2 - 1 | 1134.68 | -726.74 | 0.00000D+00 | 1.08737D-24 | -9.75086D-02 |
| Q( 9) | 2 - 2 | 1861.42 | 0.00 | 0.00000D+00 | 1.00000D+00 | -1.77629D+00 |
| Q( 10) | 2 - 0 | 420.90 | -1451.19 | 0.00000D+00 | 1.59919D-25 | -2.39608D-04 |
| Q( 10) | 2 - 1 | 1145.47 | -726.62 | 0.00000D+00 | 1.94071D-24 | -9.75429D-02 |
| Q( 10) | 2 - 2 | 1872.09 | 0.00 | 0.00000D+00 | 1.00000D+00 | -1.77642D+00 |

| | | | | | | | |
|---|---|---|---|---|---|---|---|
| Q( 11) | 2 - 0 | 432.94 | -1450.89 | 0.00000D+00 | 8.47945D-26 | -2.41825D-04 |
| Q( 11) | 2 - 1 | 1157.34 | -726.49 | 0.00000D+00 | 3.48743D-24 | -9.75807D-02 |
| Q( 11) | 2 - 2 | 1883.83 | 0.00 | 0.00000D+00 | 1.00000D+00 | -1.77656D+00 |
| Q( 12) | 2 - 0 | 446.06 | -1450.57 | 0.00000D+00 | 2.16708D-27 | -2.44268D-04 |
| Q( 12) | 2 - 1 | 1170.29 | -726.34 | 0.00000D+00 | 1.21624D-23 | -9.76220D-02 |
| Q( 12) | 2 - 2 | 1896.63 | 0.00 | 0.00000D+00 | 1.00000D+00 | -1.77672D+00 |
| Q( 13) | 2 - 0 | 460.28 | -1450.21 | 0.00000D+00 | 6.81751D-26 | -2.46944D-04 |
| Q( 13) | 2 - 1 | 1184.31 | -726.18 | 0.00000D+00 | 1.91955D-23 | -9.76668D-02 |
| Q( 13) | 2 - 2 | 1910.49 | 0.00 | 0.00000D+00 | 1.00000D+00 | -1.77689D+00 |
| Q( 14) | 2 - 0 | 475.59 | -1449.84 | 0.00000D+00 | 2.55146D-25 | -2.49859D-04 |
| Q( 14) | 2 - 1 | 1199.41 | -726.01 | 0.00000D+00 | 3.02308D-23 | -9.77151D-02 |
| Q( 14) | 2 - 2 | 1925.42 | 0.00 | 0.00000D+00 | 1.00000D+00 | -1.77707D+00 |
| Q( 15) | 2 - 0 | 491.99 | -1449.43 | 0.00000D+00 | 6.43892D-25 | -2.53020D-04 |
| Q( 15) | 2 - 1 | 1215.59 | -725.83 | 0.00000D+00 | 4.71878D-23 | -9.77669D-02 |
| Q( 15) | 2 - 2 | 1941.42 | 0.00 | 0.00000D+00 | 1.00000D+00 | -1.77726D+00 |
| Q( 16) | 2 - 0 | 509.48 | -1449.00 | 0.00000D+00 | 1.33485D-24 | -2.56437D-04 |
| Q( 16) | 2 - 1 | 1232.84 | -725.64 | 0.00000D+00 | 7.20199D-23 | -9.78222D-02 |
| Q( 16) | 2 - 2 | 1958.48 | 0.00 | 0.00000D+00 | 1.00000D+00 | -1.77747D+00 |
| Q( 17) | 2 - 0 | 528.06 | -1448.54 | 0.00000D+00 | 2.13794D-24 | -2.60117D-04 |
| Q( 17) | 2 - 1 | 1251.17 | -725.43 | 0.00000D+00 | 1.07864D-22 | -9.78810D-02 |
| Q( 17) | 2 - 2 | 1976.60 | 0.00 | 0.00000D+00 | 1.00000D+00 | -1.77768D+00 |
| Q( 18) | 2 - 0 | 547.74 | -1448.05 | 0.00000D+00 | 3.78758D-24 | -2.64069D-04 |
| Q( 18) | 2 - 1 | 1270.57 | -725.22 | 0.00000D+00 | 1.59528D-22 | -9.79434D-02 |
| Q( 18) | 2 - 2 | 1995.79 | 0.00 | 0.00000D+00 | 1.00000D+00 | -1.77792D+00 |
| Q( 19) | 2 - 0 | 568.50 | -1447.54 | 0.00000D+00 | 6.29987D-24 | -2.68304D-04 |
| Q( 19) | 2 - 1 | 1291.05 | -724.99 | 0.00000D+00 | 2.34797D-22 | -9.80093D-02 |
| Q( 19) | 2 - 2 | 2016.04 | 0.00 | 0.00000D+00 | 1.00000D+00 | -1.77816D+00 |
| Q( 20) | 2 - 0 | 590.35 | -1447.00 | 0.00000D+00 | 1.00201D-23 | -2.72832D-04 |
| Q( 20) | 2 - 1 | 1312.60 | -724.74 | 0.00000D+00 | 3.37383D-22 | -9.80788D-02 |

| | | | | | | | |
|---|---|---|---|---|---|---|---|
| Q( 20) | 2 - 2 | 2037.35 | 0.00 | 0.00000D+00 | 1.00000D+00 | -1.77842D+00 |
| Q( 0) | 3 - 0 | 360.72 | -2171.00 | 0.00000D+00 | 2.57059D-24 | 2.31738D-04 |
| Q( 0) | 3 - 1 | 1086.12 | -1445.60 | 0.00000D+00 | 7.95061D-25 | 4.22362D-03 |
| Q( 0) | 3 - 2 | 1813.40 | -718.32 | 0.00000D+00 | 1.52188D-20 | 1.26695D-01 |
| Q( 0) | 3 - 3 | 2531.72 | 0.00 | 0.00000D+00 | 1.00000D+00 | 1.81048D+00 |
| Q( 1) | 3 - 0 | 361.81 | -2170.96 | 0.00000D+00 | 6.08506D-20 | 2.32231D-04 |
| Q( 1) | 3 - 1 | 1087.20 | -1445.58 | 0.00000D+00 | 9.94393D-19 | 4.22415D-03 |
| Q( 1) | 3 - 2 | 1814.47 | -718.31 | 0.00000D+00 | 1.58523D-17 | 1.26699D-01 |
| Q( 1) | 3 - 3 | 2532.78 | -0.00 | 0.00000D+00 | 1.00000D+00 | 1.81049D+00 |
| Q( 2) | 3 - 0 | 364.00 | -2170.88 | 0.00000D+00 | 3.40218D-24 | 2.33217D-04 |
| Q( 2) | 3 - 1 | 1089.36 | -1445.53 | 0.00000D+00 | 3.99774D-27 | 4.22521D-03 |
| Q( 2) | 3 - 2 | 1816.60 | -718.29 | 0.00000D+00 | 1.42834D-20 | 1.26709D-01 |
| Q( 2) | 3 - 3 | 2534.89 | 0.00 | 0.00000D+00 | 1.00000D+00 | 1.81052D+00 |
| Q( 3) | 3 - 0 | 367.29 | -2170.77 | 0.00000D+00 | 3.37353D-24 | 2.34697D-04 |
| Q( 3) | 3 - 1 | 1092.59 | -1445.46 | 0.00000D+00 | 4.38640D-27 | 4.22680D-03 |
| Q( 3) | 3 - 2 | 1819.80 | -718.25 | 0.00000D+00 | 1.42547D-20 | 1.26723D-01 |
| Q( 3) | 3 - 3 | 2538.06 | 0.00 | 0.00000D+00 | 1.00000D+00 | 1.81056D+00 |
| Q( 4) | 3 - 0 | 371.66 | -2170.62 | 0.00000D+00 | 3.33812D-24 | 2.36670D-04 |
| Q( 4) | 3 - 1 | 1096.91 | -1445.37 | 0.00000D+00 | 1.62492D-27 | 4.22893D-03 |
| Q( 4) | 3 - 2 | 1824.07 | -718.21 | 0.00000D+00 | 1.42252D-20 | 1.26742D-01 |
| Q( 4) | 3 - 3 | 2542.28 | 0.00 | 0.00000D+00 | 1.00000D+00 | 1.81061D+00 |
| Q( 5) | 3 - 0 | 377.14 | -2170.42 | 0.00000D+00 | 3.33943D-24 | 2.39137D-04 |
| Q( 5) | 3 - 1 | 1102.31 | -1445.25 | 0.00000D+00 | 1.37571D-27 | 4.23159D-03 |
| Q( 5) | 3 - 2 | 1829.41 | -718.15 | 0.00000D+00 | 1.41897D-20 | 1.26765D-01 |
| Q( 5) | 3 - 3 | 2547.56 | 0.00 | 0.00000D+00 | 1.00000D+00 | 1.81068D+00 |
| Q( 6) | 3 - 0 | 383.70 | -2170.19 | 0.00000D+00 | 3.31309D-24 | 2.42099D-04 |
| Q( 6) | 3 - 1 | 1108.78 | -1445.11 | 0.00000D+00 | 1.46981D-28 | 4.23478D-03 |
| Q( 6) | 3 - 2 | 1835.81 | -718.08 | 0.00000D+00 | 1.41469D-20 | 1.26794D-01 |
| Q( 6) | 3 - 3 | 2553.90 | 0.00 | 0.00000D+00 | 1.00000D+00 | 1.81077D+00 |

| | | | | | | |
|---|---|---|---|---|---|---|
| Q( 7) | 3 - 0 | 391.36 | -2169.92 | 0.00000D+00 | 3.26234D-24 | 2.45555D-04 |
| Q( 7) | 3 - 1 | 1116.34 | -1444.95 | 0.00000D+00 | 1.17862D-27 | 4.23851D-03 |
| Q( 7) | 3 - 2 | 1843.28 | -718.00 | 0.00000D+00 | 1.41085D-20 | 1.26827D-01 |
| Q( 7) | 3 - 3 | 2561.29 | 0.00 | 0.00000D+00 | 1.00000D+00 | 1.81086D+00 |
| Q( 8) | 3 - 0 | 400.12 | -2169.62 | 0.00000D+00 | 3.24212D-24 | 2.49505D-04 |
| Q( 8) | 3 - 1 | 1124.97 | -1444.76 | 0.00000D+00 | 4.86429D-27 | 4.24278D-03 |
| Q( 8) | 3 - 2 | 1851.82 | -717.91 | 0.00000D+00 | 1.44517D-20 | 1.26864D-01 |
| Q( 8) | 3 - 3 | 2569.73 | 0.00 | 0.00000D+00 | 1.00000D+00 | 1.81097D+00 |
| Q( 9) | 3 - 0 | 409.96 | -2169.27 | 0.00000D+00 | 3.17142D-24 | 2.53951D-04 |
| Q( 9) | 3 - 1 | 1134.68 | -1444.55 | 0.00000D+00 | 2.26127D-26 | 4.24758D-03 |
| Q( 9) | 3 - 2 | 1861.42 | -717.81 | 0.00000D+00 | 1.44168D-20 | 1.26907D-01 |
| Q( 9) | 3 - 3 | 2579.24 | 0.00 | 0.00000D+00 | 1.00000D+00 | 1.81110D+00 |
| Q( 10) | 3 - 0 | 420.90 | -2168.89 | 0.00000D+00 | 3.05635D-24 | 2.58894D-04 |
| Q( 10) | 3 - 1 | 1145.47 | -1444.32 | 0.00000D+00 | 5.24514D-26 | 4.25293D-03 |
| Q( 10) | 3 - 2 | 1872.09 | -717.70 | 0.00000D+00 | 1.43995D-20 | 1.26954D-01 |
| Q( 10) | 3 - 3 | 2589.79 | 0.00 | 0.00000D+00 | 1.00000D+00 | 1.81123D+00 |
| Q( 11) | 3 - 0 | 432.94 | -2168.47 | 0.00000D+00 | 2.93990D-24 | 2.64332D-04 |
| Q( 11) | 3 - 1 | 1157.34 | -1444.06 | 0.00000D+00 | 1.23377D-25 | 4.25883D-03 |
| Q( 11) | 3 - 2 | 1883.83 | -717.58 | 0.00000D+00 | 1.43925D-20 | 1.27006D-01 |
| Q( 11) | 3 - 3 | 2601.40 | 0.00 | 0.00000D+00 | 1.00000D+00 | 1.81139D+00 |
| Q( 12) | 3 - 0 | 446.06 | -2168.01 | 0.00000D+00 | 2.54077D-24 | 2.70268D-04 |
| Q( 12) | 3 - 1 | 1170.29 | -1443.78 | 0.00000D+00 | 6.78358D-25 | 4.26527D-03 |
| Q( 12) | 3 - 2 | 1896.63 | -717.44 | 0.00000D+00 | 1.47204D-20 | 1.27063D-01 |
| Q( 12) | 3 - 3 | 2614.07 | 0.00 | 0.00000D+00 | 1.00000D+00 | 1.81155D+00 |
| Q( 13) | 3 - 0 | 460.28 | -2167.51 | 0.00000D+00 | 2.31815D-24 | 2.76702D-04 |
| Q( 13) | 3 - 1 | 1184.31 | -1443.48 | 0.00000D+00 | 1.14524D-24 | 4.27226D-03 |
| Q( 13) | 3 - 2 | 1910.49 | -717.30 | 0.00000D+00 | 1.48168D-20 | 1.27125D-01 |
| Q( 13) | 3 - 3 | 2627.79 | -0.00 | 0.00000D+00 | 1.00000D+00 | 1.81173D+00 |
| Q( 14) | 3 - 0 | 475.59 | -2166.97 | 0.00000D+00 | 2.11936D-24 | 2.83634D-04 |

| | | | | | | | |
|---|---|---|---|---|---|---|---|
| Q( 14) | 3 - 1 | 1199.41 | -1443.15 | 0.00000D+00 | 1.86821D-24 | 4.27980D-03 |
| Q( 14) | 3 - 2 | 1925.42 | -717.14 | 0.00000D+00 | 1.49497D-20 | 1.27191D-01 |
| Q( 14) | 3 - 3 | 2642.56 | -0.00 | 0.00000D+00 | 1.00000D+00 | 1.81192D+00 |
| Q( 15) | 3 - 0 | 491.99 | -2166.40 | 0.00000D+00 | 1.83169D-24 | 2.91065D-04 |
| Q( 15) | 3 - 1 | 1215.59 | -1442.80 | 0.00000D+00 | 2.89151D-24 | 4.28791D-03 |
| Q( 15) | 3 - 2 | 1941.42 | -716.97 | 0.00000D+00 | 1.51332D-20 | 1.27262D-01 |
| Q( 15) | 3 - 3 | 2658.39 | -0.00 | 0.00000D+00 | 1.00000D+00 | 1.81213D+00 |
| Q( 16) | 3 - 0 | 509.48 | -2165.79 | 0.00000D+00 | 1.53553D-24 | 2.98997D-04 |
| Q( 16) | 3 - 1 | 1232.84 | -1442.43 | 0.00000D+00 | 4.48564D-24 | 4.29657D-03 |
| Q( 16) | 3 - 2 | 1958.48 | -716.79 | 0.00000D+00 | 1.53697D-20 | 1.27338D-01 |
| Q( 16) | 3 - 3 | 2675.27 | -0.00 | 0.00000D+00 | 1.00000D+00 | 1.81235D+00 |
| Q( 17) | 3 - 0 | 528.06 | -2165.14 | 0.00000D+00 | 1.26082D-24 | 3.07429D-04 |
| Q( 17) | 3 - 1 | 1251.17 | -1442.04 | 0.00000D+00 | 6.76469D-24 | 4.30580D-03 |
| Q( 17) | 3 - 2 | 1976.60 | -716.60 | 0.00000D+00 | 1.60595D-20 | 1.27419D-01 |
| Q( 17) | 3 - 3 | 2693.20 | -0.00 | 0.00000D+00 | 1.00000D+00 | 1.81259D+00 |
| Q( 18) | 3 - 0 | 547.74 | -2164.45 | 0.00000D+00 | 9.54128D-25 | 3.16363D-04 |
| Q( 18) | 3 - 1 | 1270.57 | -1441.62 | 0.00000D+00 | 1.00827D-23 | 4.31560D-03 |
| Q( 18) | 3 - 2 | 1995.79 | -716.40 | 0.00000D+00 | 1.64524D-20 | 1.27505D-01 |
| Q( 18) | 3 - 3 | 2712.19 | -0.00 | 0.00000D+00 | 1.00000D+00 | 1.81284D+00 |
| Q( 19) | 3 - 0 | 568.50 | -2163.73 | 0.00000D+00 | 6.44098D-25 | 3.25798D-04 |
| Q( 19) | 3 - 1 | 1291.05 | -1441.18 | 0.00000D+00 | 1.45964D-23 | 4.32597D-03 |
| Q( 19) | 3 - 2 | 2016.04 | -716.19 | 0.00000D+00 | 1.69194D-20 | 1.27595D-01 |
| Q( 19) | 3 - 3 | 2732.22 | -0.00 | 0.00000D+00 | 1.00000D+00 | 1.81310D+00 |
| Q( 20) | 3 - 0 | 590.35 | -2162.96 | 0.00000D+00 | 3.69212D-25 | 3.35737D-04 |
| Q( 20) | 3 - 1 | 1312.60 | -1440.71 | 0.00000D+00 | 2.11291D-23 | 4.33693D-03 |
| Q( 20) | 3 - 2 | 2037.35 | -715.97 | 0.00000D+00 | 1.75136D-20 | 1.27691D-01 |
| Q( 20) | 3 - 3 | 2753.31 | -0.00 | 0.00000D+00 | 1.00000D+00 | 1.81338D+00 |
| Q( 0) | 4 - 0 | 360.72 | -2885.82 | 0.00000D+00 | 6.22750D-25 | -1.40758D-03 |
| Q( 0) | 4 - 1 | 1086.12 | -2160.42 | 0.00000D+00 | 2.77350D-24 | -1.13910D-03 |

| | | | | | | |
|---|---|---|---|---|---|---|
| Q( 0) | 4 - 2 | 1813.40 | -1433.14 | 0.00000D+00 | 1.55022D-21 | -8.99359D-03 |
| Q( 0) | 4 - 3 | 2531.72 | -714.82 | 0.00000D+00 | 7.17202D-22 | -1.55739D-01 |
| Q( 0) | 4 - 4 | 3246.54 | 0.00 | 0.00000D+00 | 1.00000D+00 | -1.84910D+00 |
| Q( 1) | 4 - 0 | 361.81 | -2885.77 | 0.00000D+00 | 9.29180D-21 | -1.40751D-03 |
| Q( 1) | 4 - 1 | 1087.20 | -2160.39 | 0.00000D+00 | 1.37288D-19 | -1.13948D-03 |
| Q( 1) | 4 - 2 | 1814.47 | -1433.12 | 0.00000D+00 | 1.27178D-18 | -8.99472D-03 |
| Q( 1) | 4 - 3 | 2532.78 | -714.81 | 0.00000D+00 | 1.61085D-17 | -1.55745D-01 |
| Q( 1) | 4 - 4 | 3247.59 | -0.00 | 0.00000D+00 | 1.00000D+00 | -1.84912D+00 |
| Q( 2) | 4 - 0 | 364.00 | -2885.67 | 0.00000D+00 | 1.22631D-25 | -1.40739D-03 |
| Q( 2) | 4 - 1 | 1089.36 | -2160.32 | 0.00000D+00 | 7.66597D-28 | -1.14025D-03 |
| Q( 2) | 4 - 2 | 1816.60 | -1433.07 | 0.00000D+00 | 1.99385D-21 | -8.99697D-03 |
| Q( 2) | 4 - 3 | 2534.89 | -714.79 | 0.00000D+00 | 7.10778D-23 | -1.55757D-01 |
| Q( 2) | 4 - 4 | 3249.67 | 0.00 | 0.00000D+00 | 1.00000D+00 | -1.84915D+00 |
| Q( 3) | 4 - 0 | 367.29 | -2885.52 | 0.00000D+00 | 1.20908D-25 | -1.40720D-03 |
| Q( 3) | 4 - 1 | 1092.59 | -2160.21 | 0.00000D+00 | 1.08486D-27 | -1.14140D-03 |
| Q( 3) | 4 - 2 | 1819.80 | -1433.00 | 0.00000D+00 | 1.98640D-21 | -9.00034D-03 |
| Q( 3) | 4 - 3 | 2538.06 | -714.75 | 0.00000D+00 | 7.07407D-23 | -1.55775D-01 |
| Q( 3) | 4 - 4 | 3252.81 | 0.00 | 0.00000D+00 | 1.00000D+00 | -1.84919D+00 |
| Q( 4) | 4 - 0 | 371.66 | -2885.32 | 0.00000D+00 | 1.18246D-25 | -1.40696D-03 |
| Q( 4) | 4 - 1 | 1096.91 | -2160.07 | 0.00000D+00 | 4.26316D-28 | -1.14294D-03 |
| Q( 4) | 4 - 2 | 1824.07 | -1432.91 | 0.00000D+00 | 1.97666D-21 | -9.00484D-03 |
| Q( 4) | 4 - 3 | 2542.28 | -714.70 | 0.00000D+00 | 7.11336D-23 | -1.55799D-01 |
| Q( 4) | 4 - 4 | 3256.98 | 0.00 | 0.00000D+00 | 1.00000D+00 | -1.84925D+00 |
| Q( 5) | 4 - 0 | 377.14 | -2885.07 | 0.00000D+00 | 1.17528D-25 | -1.40664D-03 |
| Q( 5) | 4 - 1 | 1102.31 | -2159.90 | 0.00000D+00 | 6.08966D-28 | -1.14486D-03 |
| Q( 5) | 4 - 2 | 1829.41 | -1432.80 | 0.00000D+00 | 1.96352D-21 | -9.01046D-03 |
| Q( 5) | 4 - 3 | 2547.56 | -714.65 | 0.00000D+00 | 7.18418D-23 | -1.55829D-01 |
| Q( 5) | 4 - 4 | 3262.21 | 0.00 | 0.00000D+00 | 1.00000D+00 | -1.84933D+00 |
| Q( 6) | 4 - 0 | 383.70 | -2884.77 | 0.00000D+00 | 1.16784D-25 | -1.40626D-03 |

| | | | | | | |
|---|---|---|---|---|---|---|
| Q( 6) | 4 - 1 | 1108.78 | -2159.69 | 0.00000D+00 | 2.85322D-28 | -1.14716D-03 |
| Q( 6) | 4 - 2 | 1835.81 | -1432.66 | 0.00000D+00 | 1.94771D-21 | -9.01722D-03 |
| Q( 6) | 4 - 3 | 2553.90 | -714.58 | 0.00000D+00 | 7.25822D-23 | -1.55864D-01 |
| Q( 6) | 4 - 4 | 3268.47 | 0.00 | 0.00000D+00 | 1.00000D+00 | -1.84941D+00 |
| Q( 7) | 4 - 0 | 391.36 | -2884.42 | 0.00000D+00 | 1.16710D-25 | -1.40582D-03 |
| Q( 7) | 4 - 1 | 1116.34 | -2159.44 | 0.00000D+00 | 2.99748D-29 | -1.14985D-03 |
| Q( 7) | 4 - 2 | 1843.28 | -1432.50 | 0.00000D+00 | 1.92812D-21 | -9.02510D-03 |
| Q( 7) | 4 - 3 | 2561.29 | -714.49 | 0.00000D+00 | 7.43655D-23 | -1.55906D-01 |
| Q( 7) | 4 - 4 | 3275.78 | 0.00 | 0.00000D+00 | 1.00000D+00 | -1.84952D+00 |
| Q( 8) | 4 - 0 | 400.12 | -2884.02 | 0.00000D+00 | 1.78382D-25 | -1.40530D-03 |
| Q( 8) | 4 - 1 | 1124.97 | -2159.16 | 0.00000D+00 | 5.74269D-27 | -1.15293D-03 |
| Q( 8) | 4 - 2 | 1851.82 | -1432.31 | 0.00000D+00 | 2.05379D-21 | -9.03410D-03 |
| Q( 8) | 4 - 3 | 2569.73 | -714.40 | 0.00000D+00 | 8.95120D-23 | -1.55954D-01 |
| Q( 8) | 4 - 4 | 3284.13 | 0.00 | 0.00000D+00 | 1.00000D+00 | -1.84964D+00 |
| Q( 9) | 4 - 0 | 409.96 | -2883.57 | 0.00000D+00 | 1.81848D-25 | -1.40472D-03 |
| Q( 9) | 4 - 1 | 1134.68 | -2158.85 | 0.00000D+00 | 1.42749D-26 | -1.15639D-03 |
| Q( 9) | 4 - 2 | 1861.42 | -1432.11 | 0.00000D+00 | 2.02031D-21 | -9.04424D-03 |
| Q( 9) | 4 - 3 | 2579.24 | -714.29 | 0.00000D+00 | 9.70298D-23 | -1.56008D-01 |
| Q( 9) | 4 - 4 | 3293.53 | 0.00 | 0.00000D+00 | 1.00000D+00 | -1.84977D+00 |
| Q( 10) | 4 - 0 | 420.90 | -2883.07 | 0.00000D+00 | 1.86405D-25 | -1.40406D-03 |
| Q( 10) | 4 - 1 | 1145.47 | -2158.49 | 0.00000D+00 | 2.82679D-26 | -1.16024D-03 |
| Q( 10) | 4 - 2 | 1872.09 | -1431.88 | 0.00000D+00 | 1.98364D-21 | -9.05551D-03 |
| Q( 10) | 4 - 3 | 2589.79 | -714.18 | 0.00000D+00 | 1.06452D-22 | -1.56068D-01 |
| Q( 10) | 4 - 4 | 3303.97 | 0.00 | 0.00000D+00 | 1.00000D+00 | -1.84992D+00 |
| Q( 11) | 4 - 0 | 432.94 | -2882.52 | 0.00000D+00 | 1.94929D-25 | -1.40332D-03 |
| Q( 11) | 4 - 1 | 1157.34 | -2158.11 | 0.00000D+00 | 5.10094D-26 | -1.16447D-03 |
| Q( 11) | 4 - 2 | 1883.83 | -1431.62 | 0.00000D+00 | 1.94146D-21 | -9.06791D-03 |
| Q( 11) | 4 - 3 | 2601.40 | -714.05 | 0.00000D+00 | 1.21841D-22 | -1.56134D-01 |
| Q( 11) | 4 - 4 | 3315.45 | 0.00 | 0.00000D+00 | 1.00000D+00 | -1.85008D+00 |

| | | | | | | |
|---|---|---|---|---|---|---|
| Q( 12) | 4 - 0 | 446.06 | -2881.91 | 0.00000D+00 | 2.05224D-25 | -1.40251D-03 |
| Q( 12) | 4 - 1 | 1170.29 | -2157.69 | 0.00000D+00 | 8.45941D-26 | -1.16910D-03 |
| Q( 12) | 4 - 2 | 1896.63 | -1431.35 | 0.00000D+00 | 1.89389D-21 | -9.08144D-03 |
| Q( 12) | 4 - 3 | 2614.07 | -713.91 | 0.00000D+00 | 1.38733D-22 | -1.56206D-01 |
| Q( 12) | 4 - 4 | 3327.98 | 0.00 | 0.00000D+00 | 1.00000D+00 | -1.85026D+00 |
| Q( 13) | 4 - 0 | 460.28 | -2881.26 | 0.00000D+00 | 2.20158D-25 | -1.40161D-03 |
| Q( 13) | 4 - 1 | 1184.31 | -2157.23 | 0.00000D+00 | 1.44858D-25 | -1.17411D-03 |
| Q( 13) | 4 - 2 | 1910.49 | -1431.05 | 0.00000D+00 | 1.84195D-21 | -9.09611D-03 |
| Q( 13) | 4 - 3 | 2627.79 | -713.75 | 0.00000D+00 | 1.60023D-22 | -1.56284D-01 |
| Q( 13) | 4 - 4 | 3341.54 | 0.00 | 0.00000D+00 | 1.00000D+00 | -1.85045D+00 |
| Q( 14) | 4 - 0 | 475.59 | -2880.56 | 0.00000D+00 | 2.40381D-25 | -1.40062D-03 |
| Q( 14) | 4 - 1 | 1199.41 | -2156.74 | 0.00000D+00 | 2.31693D-25 | -1.17951D-03 |
| Q( 14) | 4 - 2 | 1925.42 | -1430.73 | 0.00000D+00 | 1.78262D-21 | -9.11191D-03 |
| Q( 14) | 4 - 3 | 2642.56 | -713.59 | 0.00000D+00 | 1.88235D-22 | -1.56368D-01 |
| Q( 14) | 4 - 4 | 3356.15 | 0.00 | 0.00000D+00 | 1.00000D+00 | -1.85066D+00 |
| Q( 15) | 4 - 0 | 491.99 | -2879.82 | 0.00000D+00 | 2.60687D-25 | -1.39955D-03 |
| Q( 15) | 4 - 1 | 1215.59 | -2156.22 | 0.00000D+00 | 3.63605D-25 | -1.18531D-03 |
| Q( 15) | 4 - 2 | 1941.42 | -1430.39 | 0.00000D+00 | 1.71869D-21 | -9.12886D-03 |
| Q( 15) | 4 - 3 | 2658.39 | -713.41 | 0.00000D+00 | 2.25493D-22 | -1.56458D-01 |
| Q( 15) | 4 - 4 | 3371.80 | 0.00 | 0.00000D+00 | 1.00000D+00 | -1.85088D+00 |
| Q( 16) | 4 - 0 | 509.48 | -2879.02 | 0.00000D+00 | 2.90222D-25 | -1.39839D-03 |
| Q( 16) | 4 - 1 | 1232.84 | -2155.66 | 0.00000D+00 | 5.56418D-25 | -1.19149D-03 |
| Q( 16) | 4 - 2 | 1958.48 | -1430.02 | 0.00000D+00 | 1.64786D-21 | -9.14694D-03 |
| Q( 16) | 4 - 3 | 2675.27 | -713.23 | 0.00000D+00 | 2.73583D-22 | -1.56554D-01 |
| Q( 16) | 4 - 4 | 3388.50 | 0.00 | 0.00000D+00 | 1.00000D+00 | -1.85112D+00 |
| Q( 17) | 4 - 0 | 528.06 | -2878.17 | 0.00000D+00 | 4.03704D-25 | -1.39712D-03 |
| Q( 17) | 4 - 1 | 1251.17 | -2155.06 | 0.00000D+00 | 8.44130D-25 | -1.19807D-03 |
| Q( 17) | 4 - 2 | 1976.60 | -1429.63 | 0.00000D+00 | 1.72027D-21 | -9.16617D-03 |
| Q( 17) | 4 - 3 | 2693.20 | -713.03 | 0.00000D+00 | 3.36610D-22 | -1.56656D-01 |

| | | | | | | | |
|---|---|---|---|---|---|---|---|
| Q( 17) | 4 - 4 | 3406.23 | 0.00 | 0.00000D+00 | 1.00000D+00 | -1.85137D+00 |
| Q( 18) | 4 - 0 | 547.74 | -2877.27 | 0.00000D+00 | 4.57516D-25 | -1.39576D-03 |
| Q( 18) | 4 - 1 | 1270.57 | -2154.43 | 0.00000D+00 | 1.25146D-24 | -1.20504D-03 |
| Q( 18) | 4 - 2 | 1995.79 | -1429.22 | 0.00000D+00 | 1.63134D-21 | -9.18654D-03 |
| Q( 18) | 4 - 3 | 2712.19 | -712.82 | 0.00000D+00 | 4.18698D-22 | -1.56764D-01 |
| Q( 18) | 4 - 4 | 3425.01 | 0.00 | 0.00000D+00 | 1.00000D+00 | -1.85164D+00 |
| Q( 19) | 4 - 0 | 568.50 | -2876.32 | 0.00000D+00 | 5.25519D-25 | -1.39428D-03 |
| Q( 19) | 4 - 1 | 1291.05 | -2153.77 | 0.00000D+00 | 1.80549D-24 | -1.21241D-03 |
| Q( 19) | 4 - 2 | 2016.04 | -1428.78 | 0.00000D+00 | 1.53591D-21 | -9.20805D-03 |
| Q( 19) | 4 - 3 | 2732.22 | -712.59 | 0.00000D+00 | 5.28659D-22 | -1.56878D-01 |
| Q( 19) | 4 - 4 | 3444.82 | 0.00 | 0.00000D+00 | 1.00000D+00 | -1.85192D+00 |
| Q( 20) | 4 - 0 | 590.35 | -2875.32 | 0.00000D+00 | 6.22337D-25 | -1.39270D-03 |
| Q( 20) | 4 - 1 | 1312.60 | -2153.07 | 0.00000D+00 | 2.60418D-24 | -1.22018D-03 |
| Q( 20) | 4 - 2 | 2037.35 | -1428.33 | 0.00000D+00 | 1.43374D-21 | -9.23071D-03 |
| Q( 20) | 4 - 3 | 2753.31 | -712.36 | 0.00000D+00 | 6.68805D-22 | -1.56999D-01 |
| Q( 20) | 4 - 4 | 3465.67 | -0.00 | 0.00000D+00 | 1.00000D+00 | -1.85222D+00 |
| Q( 0) | 5 - 0 | 360.72 | -3596.92 | 0.00000D+00 | 2.30381D-24 | -5.79022D-04 |
| Q( 0) | 5 - 1 | 1086.12 | -2871.52 | 0.00000D+00 | 4.01644D-24 | 1.37596D-03 |
| Q( 0) | 5 - 2 | 1813.40 | -2144.24 | 0.00000D+00 | 2.50171D-25 | 2.25731D-03 |
| Q( 0) | 5 - 3 | 2531.72 | -1425.92 | 0.00000D+00 | 1.57271D-22 | 1.38495D-02 |
| Q( 0) | 5 - 4 | 3246.54 | -711.10 | 0.00000D+00 | 7.90841D-21 | 1.84499D-01 |
| Q( 0) | 5 - 5 | 3957.64 | 0.00 | 0.00000D+00 | 1.00000D+00 | 1.88860D+00 |
| Q( 1) | 5 - 0 | 361.81 | -3596.86 | 0.00000D+00 | 2.08647D-21 | -5.79236D-04 |
| Q( 1) | 5 - 1 | 1087.20 | -2871.48 | 0.00000D+00 | 2.92448D-20 | 1.37587D-03 |
| Q( 1) | 5 - 2 | 1814.47 | -2144.21 | 0.00000D+00 | 2.55688D-19 | 2.25756D-03 |
| Q( 1) | 5 - 3 | 2532.78 | -1425.90 | 0.00000D+00 | 1.95142D-18 | 1.38507D-02 |
| Q( 1) | 5 - 4 | 3247.59 | -711.09 | 0.00000D+00 | 1.96743D-17 | 1.84506D-01 |
| Q( 1) | 5 - 5 | 3958.68 | -0.00 | 0.00000D+00 | 1.00000D+00 | 1.88861D+00 |
| Q( 2) | 5 - 0 | 364.00 | -3596.74 | 0.00000D+00 | 1.01049D-24 | -5.79663D-04 |

| | | | | | | | |
|---|---|---|---|---|---|---|---|
| Q( 2) | 5 - 1 | 1089.36 | -2871.39 | 0.00000D+00 | 1.97367D-27 | 1.37570D-03 |
| Q( 2) | 5 - 2 | 1816.60 | -2144.14 | 0.00000D+00 | 2.90161D-23 | 2.25807D-03 |
| Q( 2) | 5 - 3 | 2534.89 | -1425.86 | 0.00000D+00 | 1.22991D-23 | 1.38530D-02 |
| Q( 2) | 5 - 4 | 3249.67 | -711.07 | 0.00000D+00 | 1.47813D-21 | 1.84520D-01 |
| Q( 2) | 5 - 5 | 3960.74 | 0.00 | 0.00000D+00 | 1.00000D+00 | 1.88865D+00 |
| Q( 3) | 5 - 0 | 367.29 | -3596.56 | 0.00000D+00 | 1.00584D-24 | -5.80304D-04 |
| Q( 3) | 5 - 1 | 1092.59 | -2871.25 | 0.00000D+00 | 2.45902D-27 | 1.37543D-03 |
| Q( 3) | 5 - 2 | 1819.80 | -2144.04 | 0.00000D+00 | 2.92040D-23 | 2.25882D-03 |
| Q( 3) | 5 - 3 | 2538.06 | -1425.79 | 0.00000D+00 | 1.22003D-23 | 1.38566D-02 |
| Q( 3) | 5 - 4 | 3252.81 | -711.04 | 0.00000D+00 | 1.47816D-21 | 1.84540D-01 |
| Q( 3) | 5 - 5 | 3963.84 | 0.00 | 0.00000D+00 | 1.00000D+00 | 1.88870D+00 |
| Q( 4) | 5 - 0 | 371.66 | -3596.32 | 0.00000D+00 | 1.00051D-24 | -5.81158D-04 |
| Q( 4) | 5 - 1 | 1096.91 | -2871.07 | 0.00000D+00 | 2.54167D-27 | 1.37508D-03 |
| Q( 4) | 5 - 2 | 1824.07 | -2143.91 | 0.00000D+00 | 2.94081D-23 | 2.25983D-03 |
| Q( 4) | 5 - 3 | 2542.28 | -1425.70 | 0.00000D+00 | 1.18289D-23 | 1.38613D-02 |
| Q( 4) | 5 - 4 | 3256.98 | -711.00 | 0.00000D+00 | 1.48051D-21 | 1.84568D-01 |
| Q( 4) | 5 - 5 | 3967.98 | 0.00 | 0.00000D+00 | 1.00000D+00 | 1.88876D+00 |
| Q( 5) | 5 - 0 | 377.14 | -3596.01 | 0.00000D+00 | 9.99809D-25 | -5.82224D-04 |
| Q( 5) | 5 - 1 | 1102.31 | -2870.84 | 0.00000D+00 | 3.35968D-27 | 1.37464D-03 |
| Q( 5) | 5 - 2 | 1829.41 | -2143.74 | 0.00000D+00 | 2.96645D-23 | 2.26108D-03 |
| Q( 5) | 5 - 3 | 2547.56 | -1425.59 | 0.00000D+00 | 1.14579D-23 | 1.38672D-02 |
| Q( 5) | 5 - 4 | 3262.21 | -710.94 | 0.00000D+00 | 1.48799D-21 | 1.84602D-01 |
| Q( 5) | 5 - 5 | 3973.15 | 0.00 | 0.00000D+00 | 1.00000D+00 | 1.88885D+00 |
| Q( 6) | 5 - 0 | 383.70 | -3595.65 | 0.00000D+00 | 1.00573D-24 | -5.83502D-04 |
| Q( 6) | 5 - 1 | 1108.78 | -2870.57 | 0.00000D+00 | 3.98366D-27 | 1.37411D-03 |
| Q( 6) | 5 - 2 | 1835.81 | -2143.54 | 0.00000D+00 | 2.99580D-23 | 2.26259D-03 |
| Q( 6) | 5 - 3 | 2553.90 | -1425.46 | 0.00000D+00 | 1.10042D-23 | 1.38742D-02 |
| Q( 6) | 5 - 4 | 3268.47 | -710.88 | 0.00000D+00 | 1.49650D-21 | 1.84643D-01 |
| Q( 6) | 5 - 5 | 3979.35 | 0.00 | 0.00000D+00 | 1.00000D+00 | 1.88894D+00 |

| | | | | | | |
|---|---|---|---|---|---|---|
| Q( 7) | 5 - 0 | 391.36 | -3595.22 | 0.00000D+00 | 1.01183D-24 | -5.84992D-04 |
| Q( 7) | 5 - 1 | 1116.34 | -2870.25 | 0.00000D+00 | 5.00979D-27 | 1.37348D-03 |
| Q( 7) | 5 - 2 | 1843.28 | -2143.30 | 0.00000D+00 | 3.02391D-23 | 2.26434D-03 |
| Q( 7) | 5 - 3 | 2561.29 | -1425.30 | 0.00000D+00 | 1.03915D-23 | 1.38825D-02 |
| Q( 7) | 5 - 4 | 3275.78 | -710.81 | 0.00000D+00 | 1.50867D-21 | 1.84691D-01 |
| Q( 7) | 5 - 5 | 3986.59 | 0.00 | 0.00000D+00 | 1.00000D+00 | 1.88906D+00 |
| Q( 8) | 5 - 0 | 400.12 | -3594.74 | 0.00000D+00 | 1.02737D-24 | -5.86692D-04 |
| Q( 8) | 5 - 1 | 1124.97 | -2869.88 | 0.00000D+00 | 7.66206D-27 | 1.37276D-03 |
| Q( 8) | 5 - 2 | 1851.82 | -2143.04 | 0.00000D+00 | 1.90791D-23 | 2.26633D-03 |
| Q( 8) | 5 - 3 | 2569.73 | -1425.12 | 0.00000D+00 | 9.57335D-24 | 1.38919D-02 |
| Q( 8) | 5 - 4 | 3284.13 | -710.72 | 0.00000D+00 | 1.52672D-21 | 1.84745D-01 |
| Q( 8) | 5 - 5 | 3994.86 | 0.00 | 0.00000D+00 | 1.00000D+00 | 1.88919D+00 |
| Q( 9) | 5 - 0 | 409.96 | -3594.20 | 0.00000D+00 | 1.03204D-24 | -5.88601D-04 |
| Q( 9) | 5 - 1 | 1134.68 | -2869.47 | 0.00000D+00 | 1.00162D-26 | 1.37195D-03 |
| Q( 9) | 5 - 2 | 1861.42 | -2142.73 | 0.00000D+00 | 1.92937D-23 | 2.26857D-03 |
| Q( 9) | 5 - 3 | 2579.24 | -1424.92 | 0.00000D+00 | 8.69092D-24 | 1.39025D-02 |
| Q( 9) | 5 - 4 | 3293.53 | -710.63 | 0.00000D+00 | 1.54842D-21 | 1.84807D-01 |
| Q( 9) | 5 - 5 | 4004.16 | 0.00 | 0.00000D+00 | 1.00000D+00 | 1.88934D+00 |
| Q( 10) | 5 - 0 | 420.90 | -3593.59 | 0.00000D+00 | 1.02966D-24 | -5.90719D-04 |
| Q( 10) | 5 - 1 | 1145.47 | -2869.02 | 0.00000D+00 | 1.45185D-26 | 1.37105D-03 |
| Q( 10) | 5 - 2 | 1872.09 | -2142.40 | 0.00000D+00 | 1.95463D-23 | 2.27105D-03 |
| Q( 10) | 5 - 3 | 2589.79 | -1424.70 | 0.00000D+00 | 7.59827D-24 | 1.39143D-02 |
| Q( 10) | 5 - 4 | 3303.97 | -710.52 | 0.00000D+00 | 1.61753D-21 | 1.84875D-01 |
| Q( 10) | 5 - 5 | 4014.49 | 0.00 | 0.00000D+00 | 1.00000D+00 | 1.88951D+00 |
| Q( 11) | 5 - 0 | 432.94 | -3592.92 | 0.00000D+00 | 1.03939D-24 | -5.93043D-04 |
| Q( 11) | 5 - 1 | 1157.34 | -2868.52 | 0.00000D+00 | 2.21037D-26 | 1.37004D-03 |
| Q( 11) | 5 - 2 | 1883.83 | -2142.03 | 0.00000D+00 | 1.96767D-23 | 2.27376D-03 |
| Q( 11) | 5 - 3 | 2601.40 | -1424.46 | 0.00000D+00 | 7.08791D-24 | 1.39273D-02 |
| Q( 11) | 5 - 4 | 3315.45 | -710.41 | 0.00000D+00 | 1.65498D-21 | 1.84950D-01 |

| | | | | | | |
|---|---|---|---|---|---|---|
| Q( 11) | 5 - 5 | 4025.86 | 0.00 | 0.00000D+00 | 1.00000D+00 | 1.88969D+00 |
| Q( 12) | 5 - 0 | 446.06 | -3592.20 | 0.00000D+00 | 1.05668D-24 | -5.95574D-04 |
| Q( 12) | 5 - 1 | 1170.29 | -2867.97 | 0.00000D+00 | 3.22055D-26 | 1.36893D-03 |
| Q( 12) | 5 - 2 | 1896.63 | -2141.63 | 0.00000D+00 | 1.97133D-23 | 2.27671D-03 |
| Q( 12) | 5 - 3 | 2614.07 | -1424.19 | 0.00000D+00 | 5.64146D-24 | 1.39415D-02 |
| Q( 12) | 5 - 4 | 3327.98 | -710.28 | 0.00000D+00 | 1.71209D-21 | 1.85032D-01 |
| Q( 12) | 5 - 5 | 4038.26 | 0.00 | 0.00000D+00 | 1.00000D+00 | 1.88989D+00 |
| Q( 13) | 5 - 0 | 460.28 | -3591.41 | 0.00000D+00 | 1.05994D-24 | -5.98309D-04 |
| Q( 13) | 5 - 1 | 1184.31 | -2867.38 | 0.00000D+00 | 4.65851D-26 | 1.36773D-03 |
| Q( 13) | 5 - 2 | 1910.49 | -2141.20 | 0.00000D+00 | 1.96720D-23 | 2.27989D-03 |
| Q( 13) | 5 - 3 | 2627.79 | -1423.90 | 0.00000D+00 | 4.14211D-24 | 1.39568D-02 |
| Q( 13) | 5 - 4 | 3341.54 | -710.15 | 0.00000D+00 | 1.77801D-21 | 1.85121D-01 |
| Q( 13) | 5 - 5 | 4051.69 | 0.00 | 0.00000D+00 | 1.00000D+00 | 1.89011D+00 |
| Q( 14) | 5 - 0 | 475.59 | -3590.56 | 0.00000D+00 | 1.09142D-24 | -6.01247D-04 |
| Q( 14) | 5 - 1 | 1199.41 | -2866.74 | 0.00000D+00 | 6.79440D-26 | 1.36641D-03 |
| Q( 14) | 5 - 2 | 1925.42 | -2140.73 | 0.00000D+00 | 1.94262D-23 | 2.28330D-03 |
| Q( 14) | 5 - 3 | 2642.56 | -1423.59 | 0.00000D+00 | 2.68294D-24 | 1.39734D-02 |
| Q( 14) | 5 - 4 | 3356.15 | -710.00 | 0.00000D+00 | 1.86813D-21 | 1.85217D-01 |
| Q( 14) | 5 - 5 | 4066.15 | 0.00 | 0.00000D+00 | 1.00000D+00 | 1.89034D+00 |
| Q( 15) | 5 - 0 | 491.99 | -3589.66 | 0.00000D+00 | 1.10281D-24 | -6.04385D-04 |
| Q( 15) | 5 - 1 | 1215.59 | -2866.06 | 0.00000D+00 | 1.02013D-25 | 1.36499D-03 |
| Q( 15) | 5 - 2 | 1941.42 | -2140.23 | 0.00000D+00 | 1.90021D-23 | 2.28693D-03 |
| Q( 15) | 5 - 3 | 2658.39 | -1423.26 | 0.00000D+00 | 1.32713D-24 | 1.39912D-02 |
| Q( 15) | 5 - 4 | 3371.80 | -709.84 | 0.00000D+00 | 1.97818D-21 | 1.85320D-01 |
| Q( 15) | 5 - 5 | 4081.65 | 0.00 | 0.00000D+00 | 1.00000D+00 | 1.89059D+00 |
| Q( 16) | 5 - 0 | 509.48 | -3588.69 | 0.00000D+00 | 1.12771D-24 | -6.07723D-04 |
| Q( 16) | 5 - 1 | 1232.84 | -2865.33 | 0.00000D+00 | 1.47950D-25 | 1.36346D-03 |
| Q( 16) | 5 - 2 | 1958.48 | -2139.69 | 0.00000D+00 | 1.83860D-23 | 2.29078D-03 |
| Q( 16) | 5 - 3 | 2675.27 | -1422.90 | 0.00000D+00 | 3.32892D-25 | 1.40102D-02 |

| | | | | | | | |
|---|---|---|---|---|---|---|---|
| Q( 16) | 5 - 4 | 3388.50 | -709.67 | 0.00000D+00 | 2.11439D-21 | 1.85430D-01 |
| Q( 16) | 5 - 5 | 4098.17 | 0.00 | 0.00000D+00 | 1.00000D+00 | 1.89085D+00 |
| Q( 17) | 5 - 0 | 528.06 | -3587.66 | 0.00000D+00 | 1.17827D-24 | -6.11257D-04 |
| Q( 17) | 5 - 1 | 1251.17 | -2864.56 | 0.00000D+00 | 2.11869D-25 | 1.36182D-03 |
| Q( 17) | 5 - 2 | 1976.60 | -2139.12 | 0.00000D+00 | 9.42780D-24 | 2.29485D-03 |
| Q( 17) | 5 - 3 | 2693.20 | -1422.52 | 0.00000D+00 | 1.04181D-26 | 1.40304D-02 |
| Q( 17) | 5 - 4 | 3406.23 | -709.49 | 0.00000D+00 | 2.28760D-21 | 1.85547D-01 |
| Q( 17) | 5 - 5 | 4115.72 | 0.00 | 0.00000D+00 | 1.00000D+00 | 1.89114D+00 |
| Q( 18) | 5 - 0 | 547.74 | -3586.57 | 0.00000D+00 | 1.31788D-24 | -6.14986D-04 |
| Q( 18) | 5 - 1 | 1270.57 | -2863.74 | 0.00000D+00 | 5.09233D-25 | 1.36006D-03 |
| Q( 18) | 5 - 2 | 1995.79 | -2138.52 | 0.00000D+00 | 6.06072D-24 | 2.29912D-03 |
| Q( 18) | 5 - 3 | 2712.19 | -1422.12 | 0.00000D+00 | 4.80699D-24 | 1.40518D-02 |
| Q( 18) | 5 - 4 | 3425.01 | -709.30 | 0.00000D+00 | 2.96518D-21 | 1.85670D-01 |
| Q( 18) | 5 - 5 | 4134.31 | 0.00 | 0.00000D+00 | 1.00000D+00 | 1.89144D+00 |
| Q( 19) | 5 - 0 | 568.50 | -3585.43 | 0.00000D+00 | 1.37641D-24 | -6.18908D-04 |
| Q( 19) | 5 - 1 | 1291.05 | -2862.87 | 0.00000D+00 | 7.08643D-25 | 1.35818D-03 |
| Q( 19) | 5 - 2 | 2016.04 | -2137.89 | 0.00000D+00 | 5.07684D-24 | 2.30361D-03 |
| Q( 19) | 5 - 3 | 2732.22 | -1421.70 | 0.00000D+00 | 9.63246D-24 | 1.40745D-02 |
| Q( 19) | 5 - 4 | 3444.82 | -709.10 | 0.00000D+00 | 3.29239D-21 | 1.85801D-01 |
| Q( 19) | 5 - 5 | 4153.92 | 0.00 | 0.00000D+00 | 1.00000D+00 | 1.89175D+00 |
| Q( 20) | 5 - 0 | 590.35 | -3584.22 | 0.00000D+00 | 1.46378D-24 | -6.23019D-04 |
| Q( 20) | 5 - 1 | 1312.60 | -2861.97 | 0.00000D+00 | 9.54298D-25 | 1.35617D-03 |
| Q( 20) | 5 - 2 | 2037.35 | -2137.22 | 0.00000D+00 | 3.99254D-24 | 2.30829D-03 |
| Q( 20) | 5 - 3 | 2753.31 | -1421.25 | 0.00000D+00 | 1.85033D-23 | 1.40983D-02 |
| Q( 20) | 5 - 4 | 3465.67 | -708.89 | 0.00000D+00 | 3.69607D-21 | 1.85938D-01 |
| Q( 20) | 5 - 5 | 4174.57 | 0.00 | 0.00000D+00 | 1.00000D+00 | 1.89209D+00 |
