# Supplementary material for: Ab initio spectroscopic studies of AlF and AlCl molecules
Source: arXiv:2303.08681 source file (2023-03-15)
Supplement: Supplementary file 10 [file Plots_PQR_Einstein_coefficients_PS1.pdf]

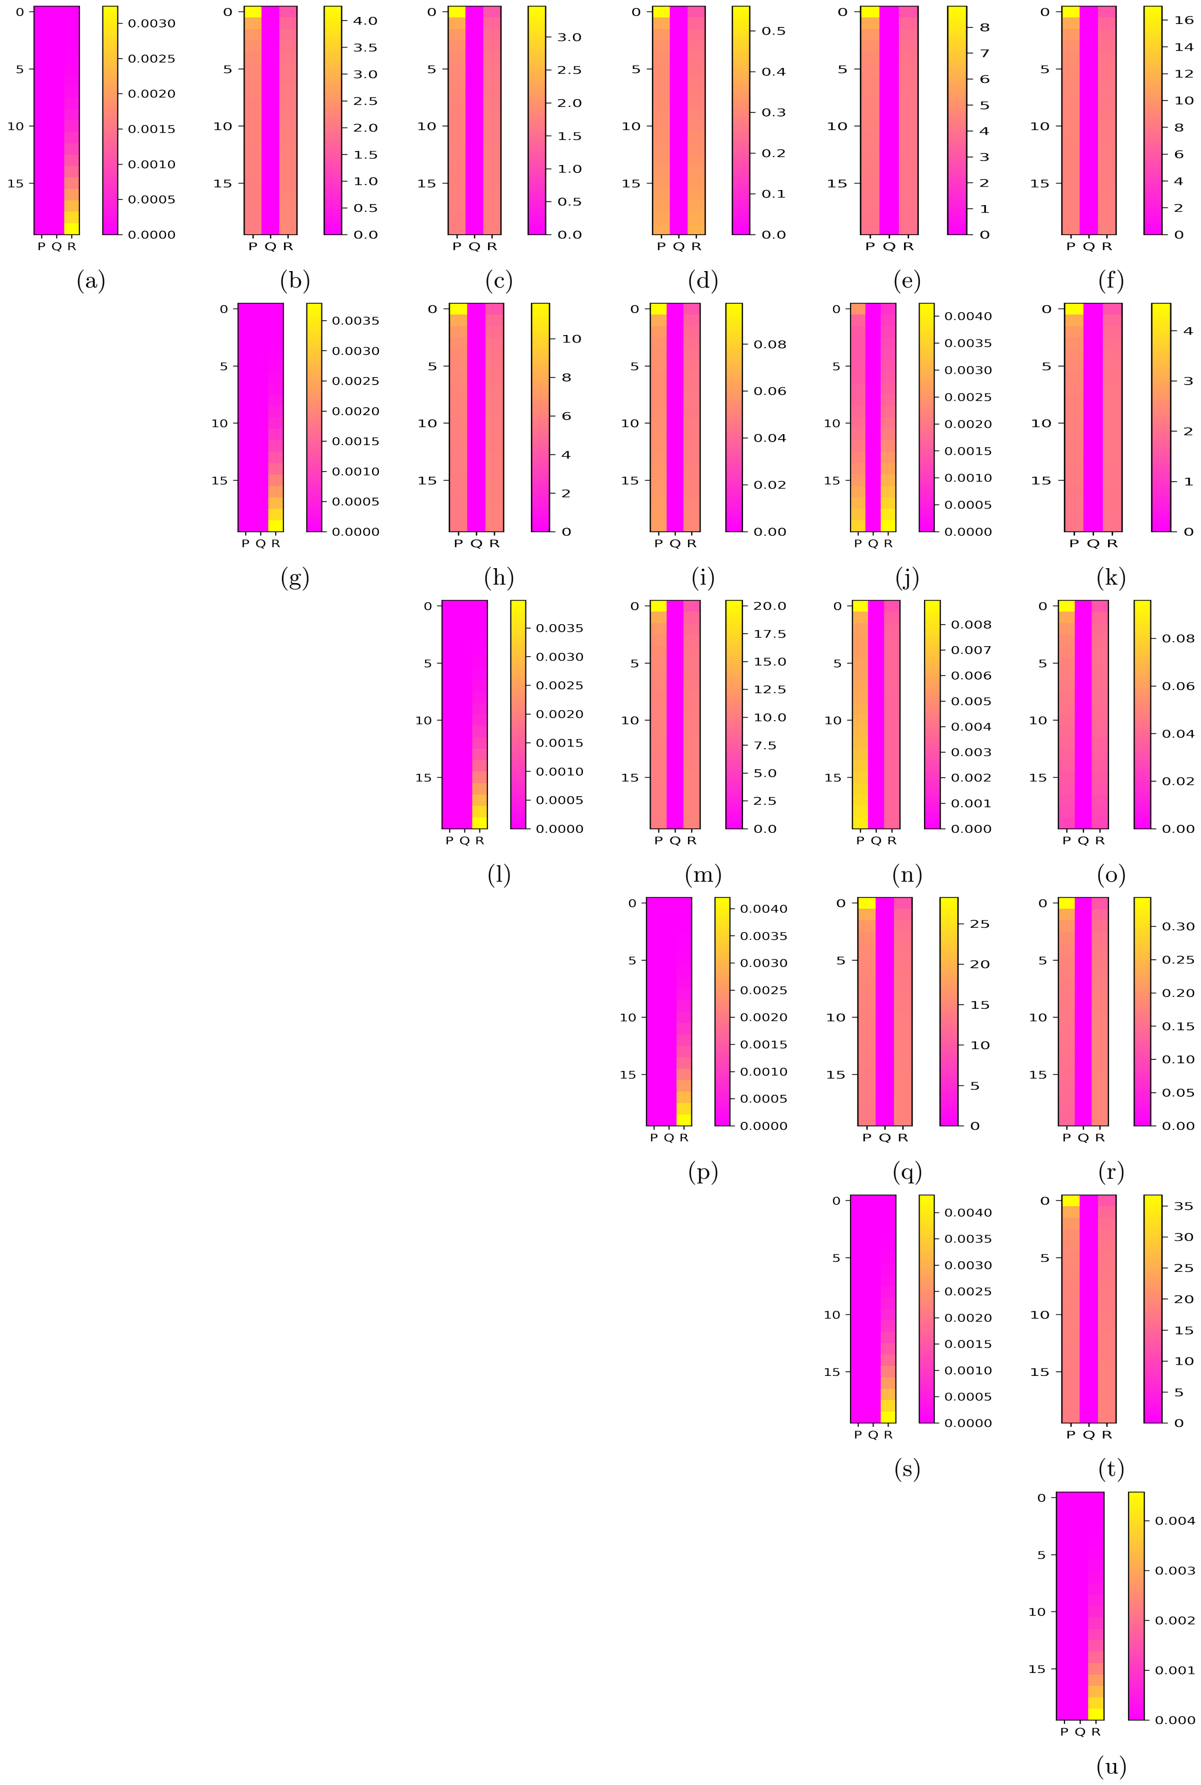


FIG. 1: Einstein A coefficients for the $^1\Sigma$ ground electronic state of AlF. Each subfigure gives the values of the A coefficients (colour coded) for the $P$, $Q$, and $R$ branches (x-axis) of a given $v" \to v$ transition for values of $J$ ranging from 0 to 20 (y-axis). Subfigure (a), for instance, considers the transitions $v" = 0 \to v' = 0$, whereas (b) shows data for $v" = 0 \to v' = 1$, and so on. Therefore, Row1 provides our results with $v" = 0$ and $v'$ going from 0 to 5, while row 2 considers $v" = 1$ and $v'$ going from 1 to 5, and so on.

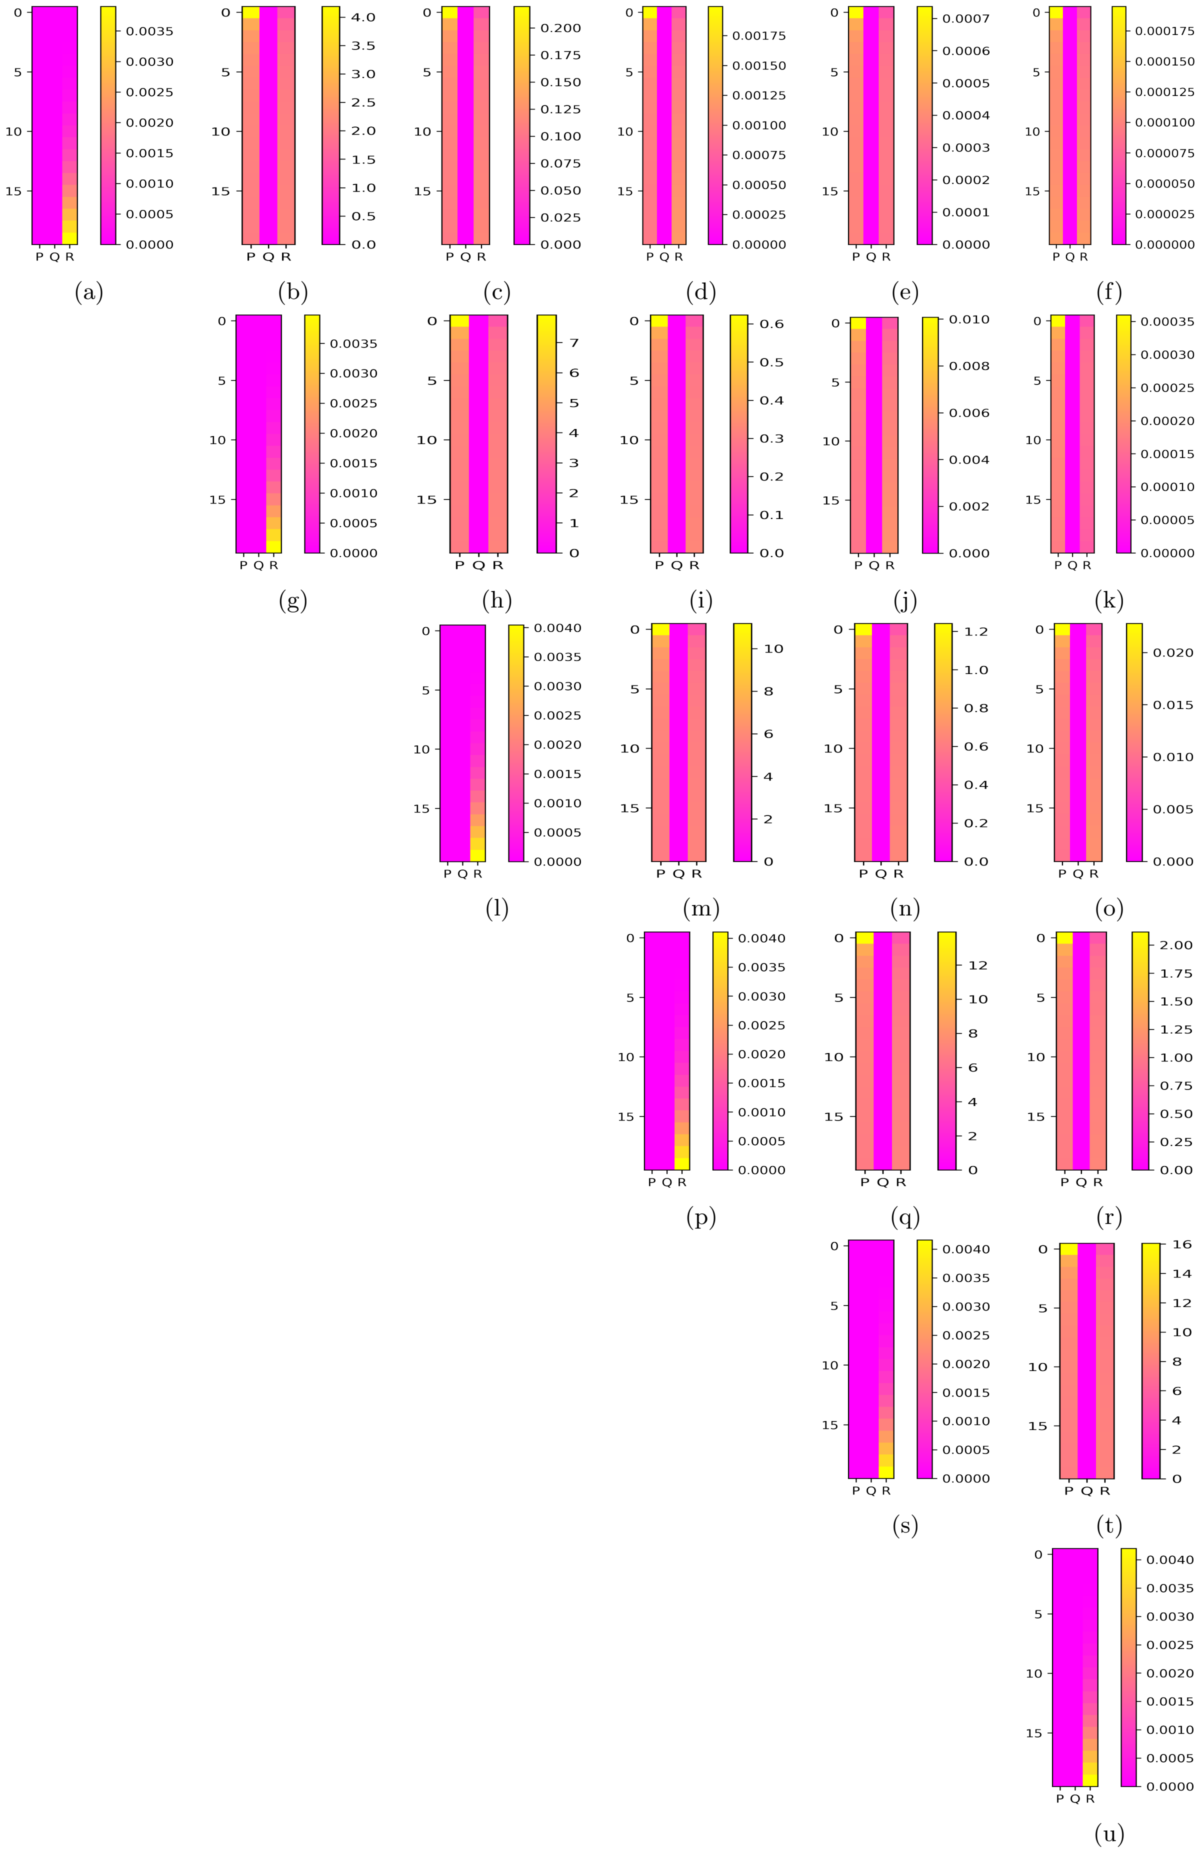


FIG. 2: Einstein A coefficients for the $^1\Pi$ electronic state of AlF. The notation utilized in this Figure is identical to that of Figure 1.

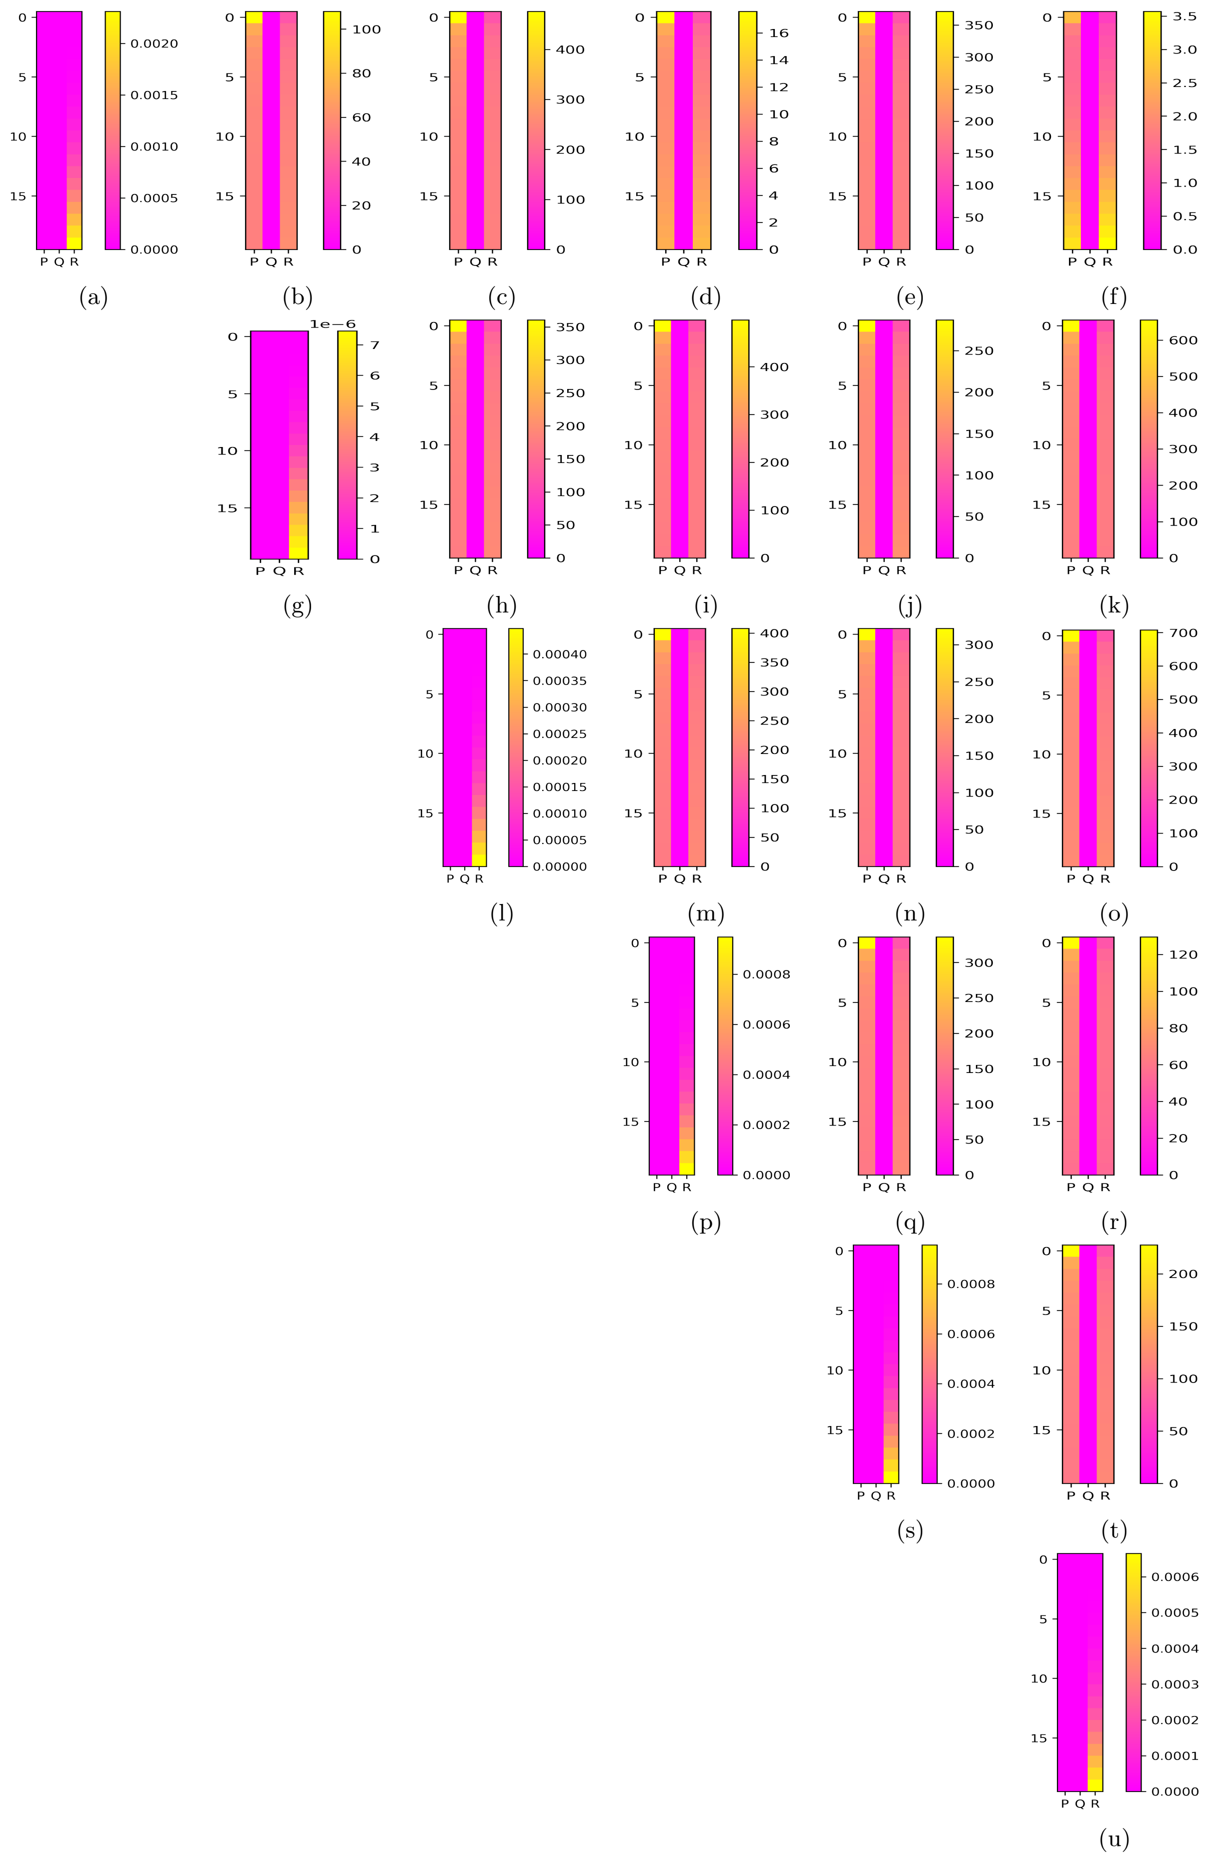


FIG. 3: Einstein A coefficients for the $^3\Pi$ electronic state of AlF. Both this Figure and Figure A1 use the same notation.

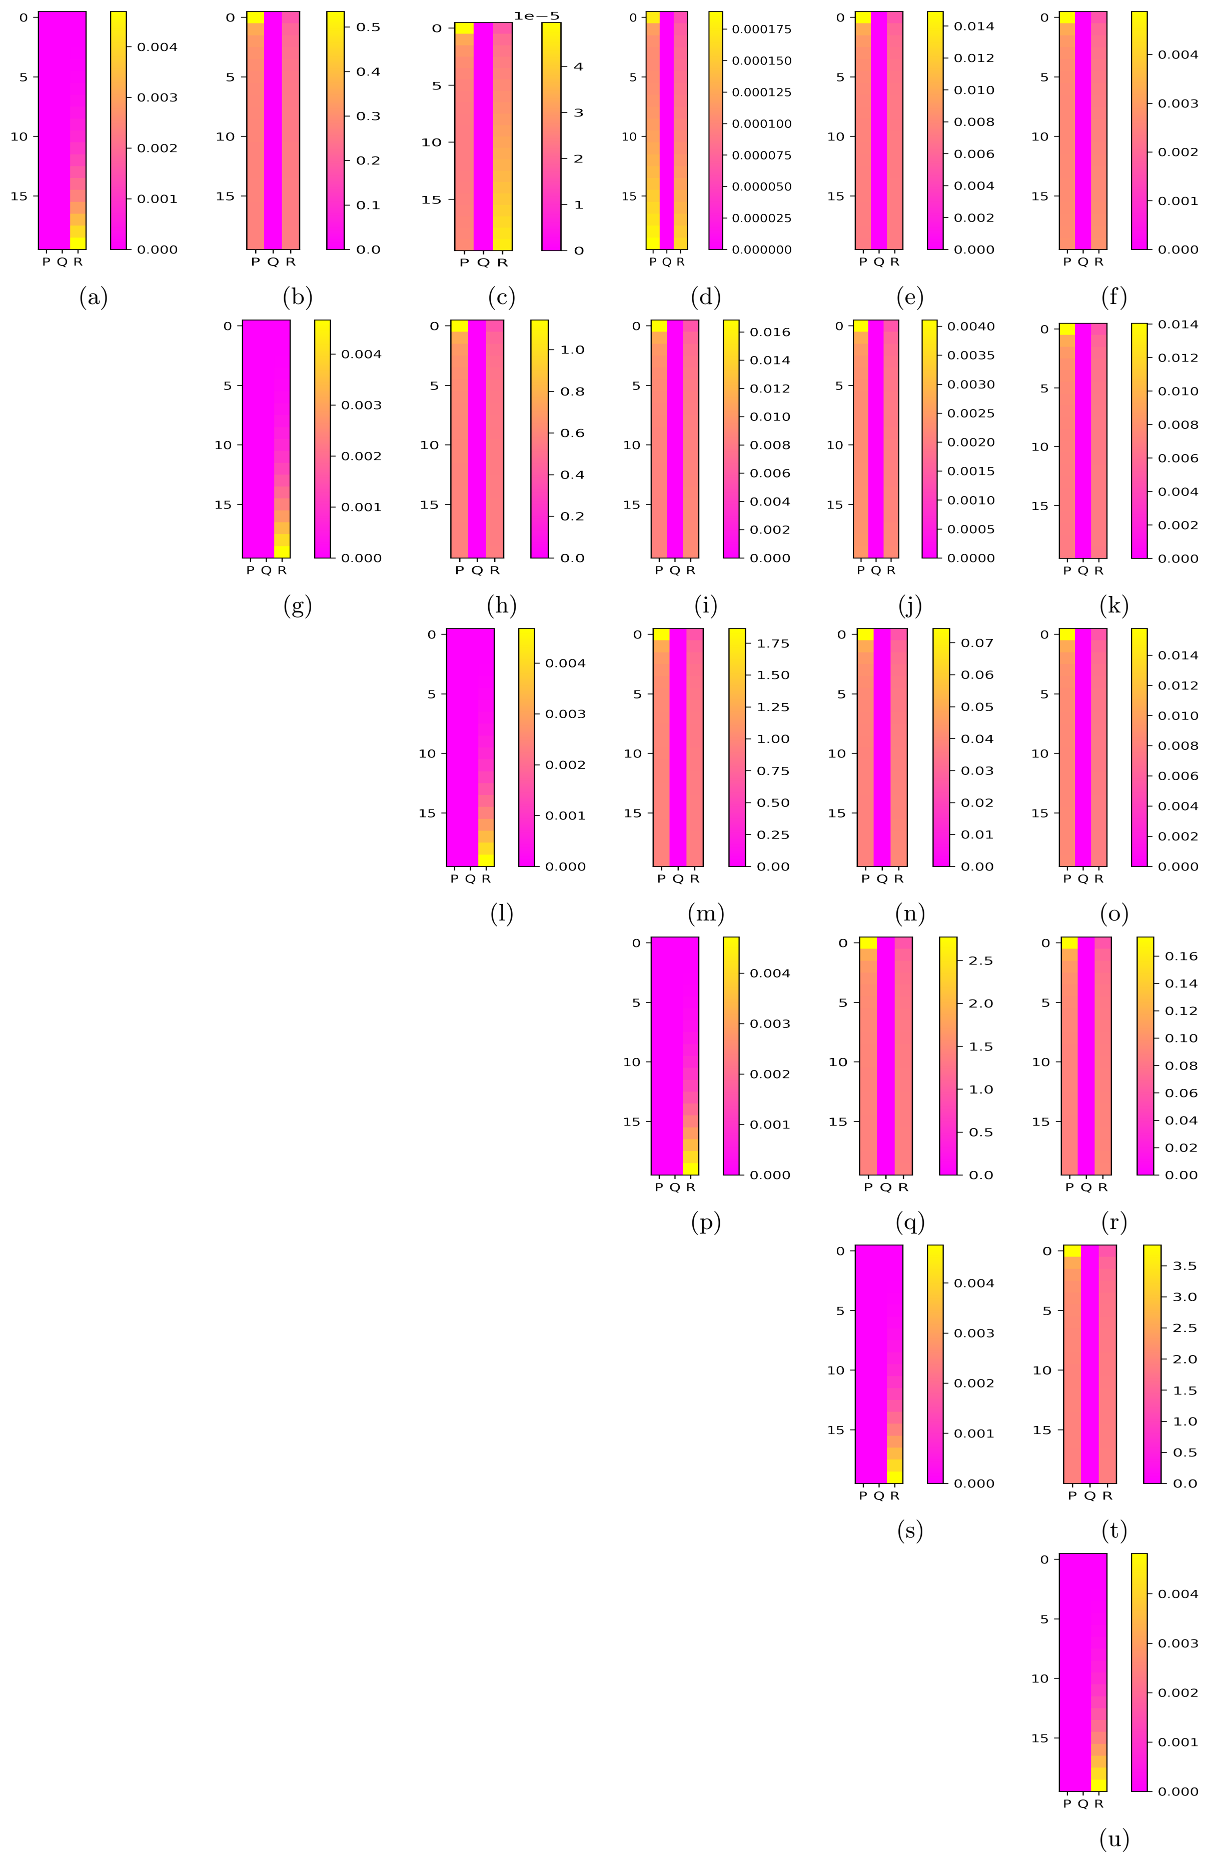


FIG. 4: Einstein A coefficients for the $^3\Sigma$ electronic state of AlF. Figure 1 and this Figure employ the same notation.

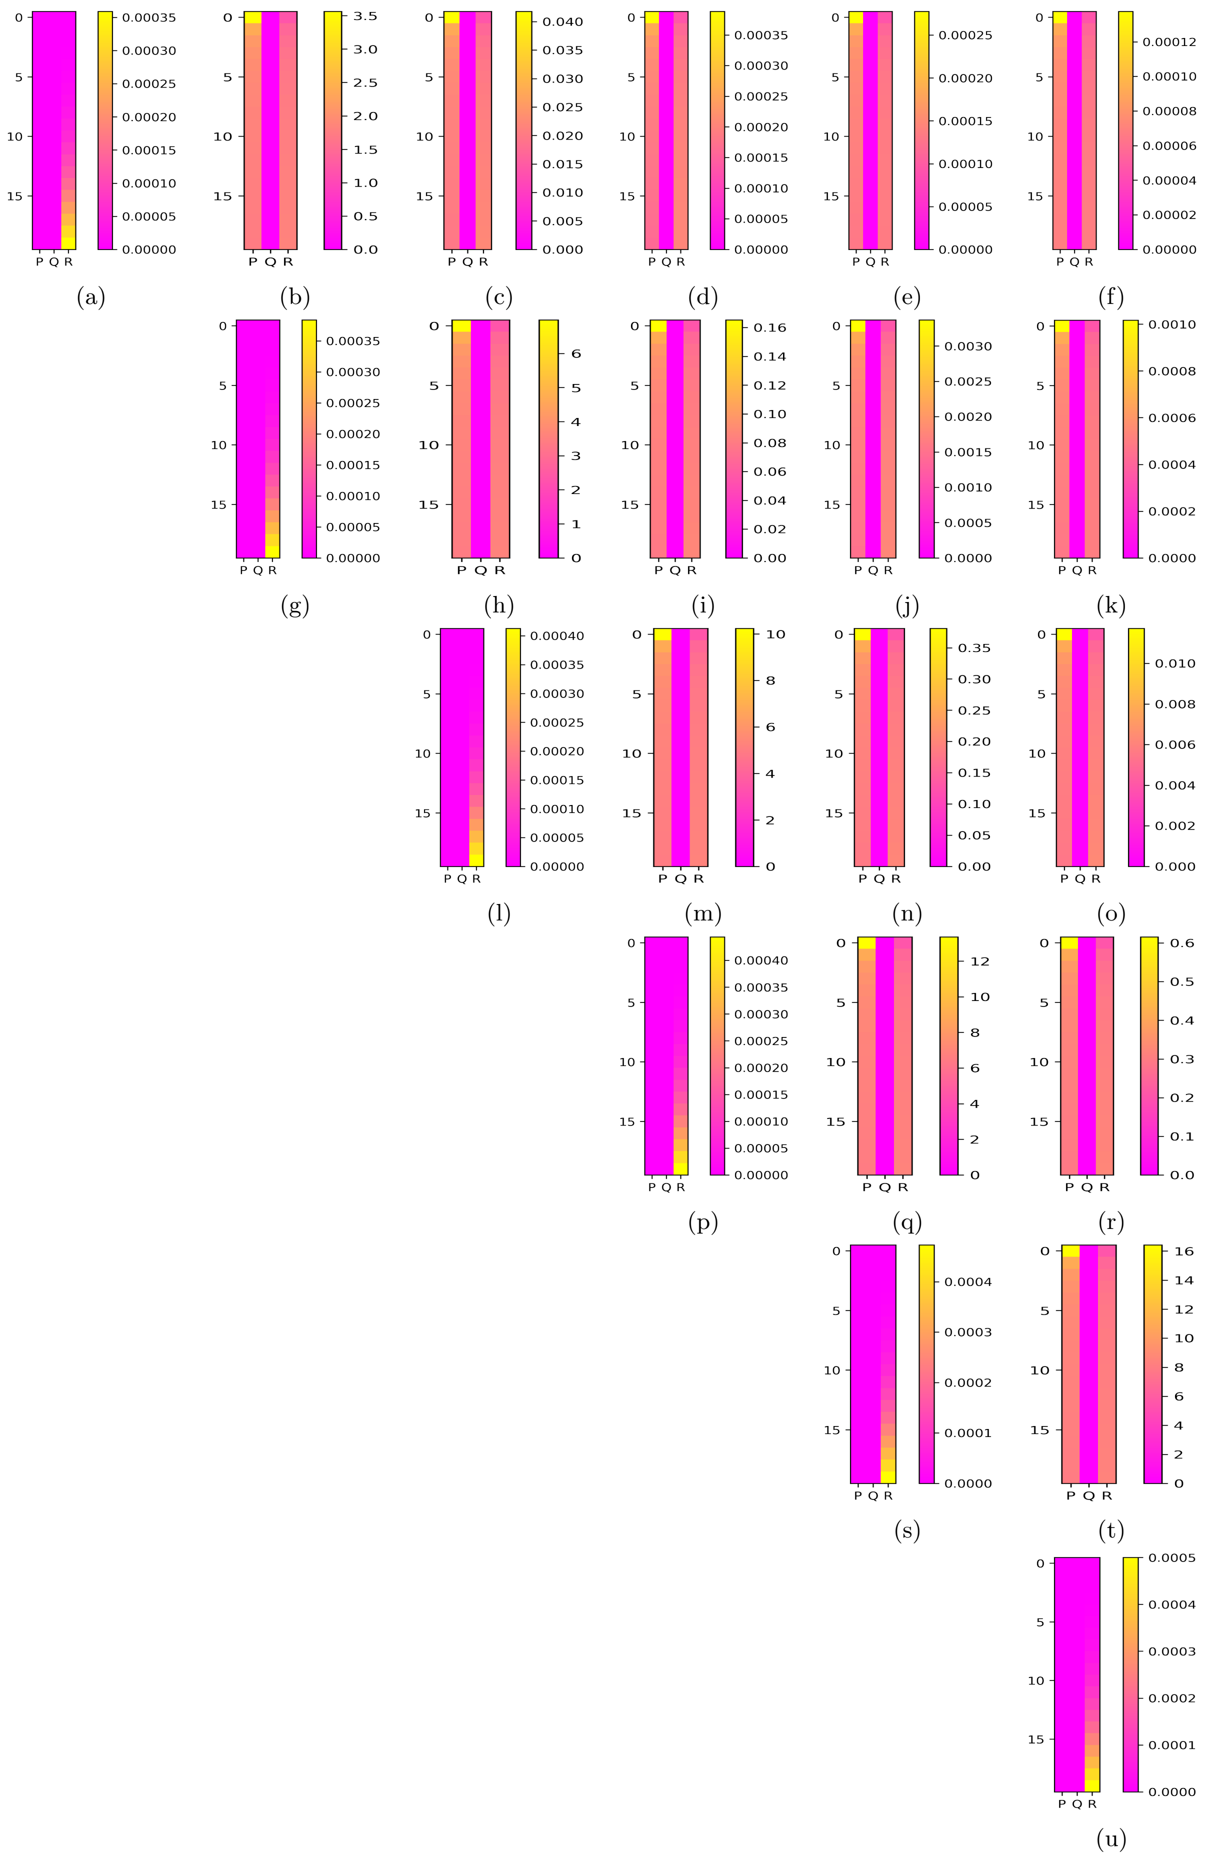


FIG. 5: Einstein A coefficients for the $^1\Sigma$ ground electronic state of AlCl. This Figure follows the same notation as Figure 1.

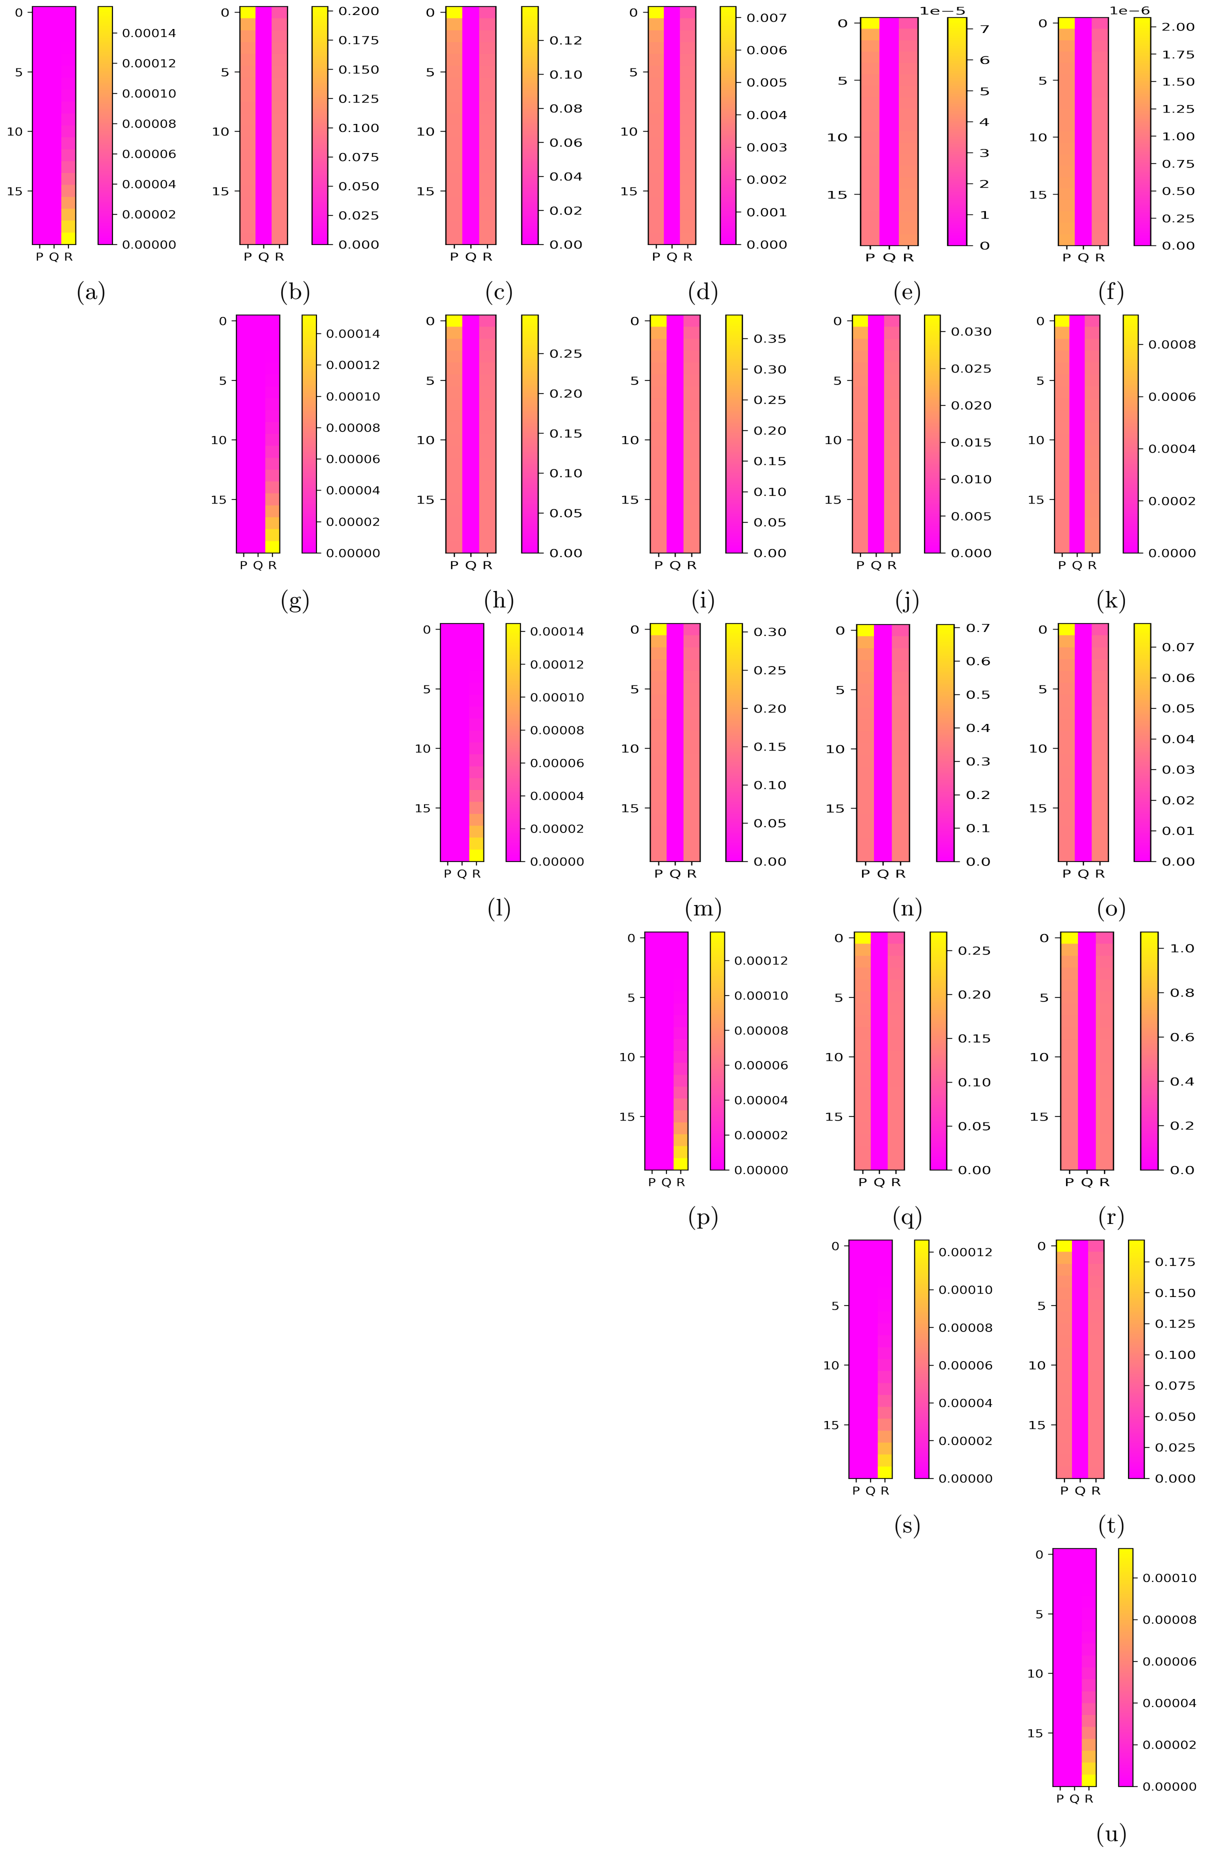


FIG. 6: Einstein A coefficients for the $^1\Pi$ excited electronic state of AlCl. The notation in this Figure is identical to that of Figure A1.

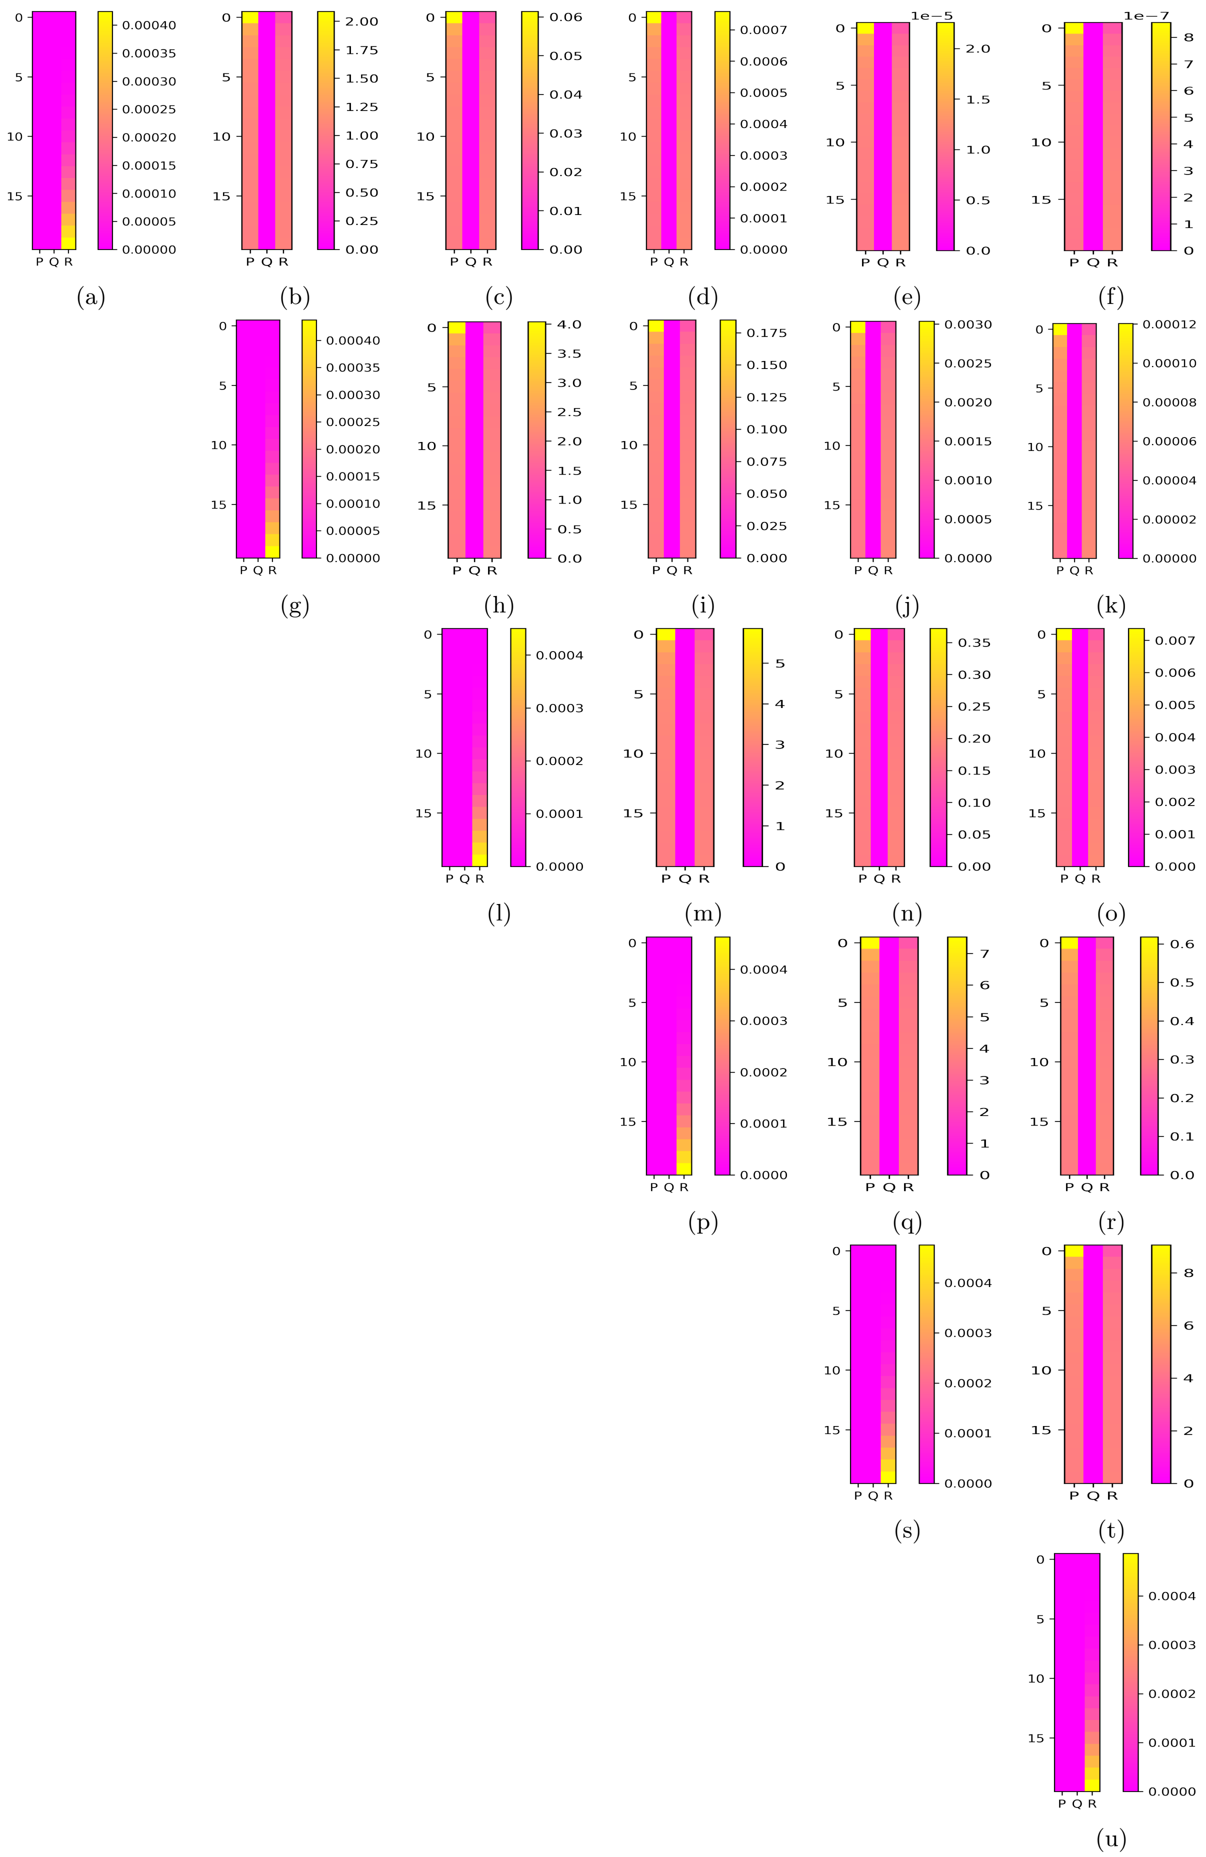


FIG. 7: Einstein A coefficients for the $^3\Pi$ excited electronic state of AlCl. The notation used in this Figure is the same as Figure 1's.
