# Supplementary material for: Ab initio spectroscopic studies of AlF and AlCl molecules
Source: arXiv:2303.08681 source file (2023-03-15)
Supplement: Supplementary file 11 [file AlCl_a3Pi_S12.pdf]

$\text{AlCl a}^3\Pi \rightarrow \text{Centrifugal distortion constants (in cm}^{-1}\text{)}$

| v  | Dv             | Hv             | Lv             | Mv             | Nv             | Ov             |
|----|----------------|----------------|----------------|----------------|----------------|----------------|
| 0  | -2.2412995D-07 | -3.9085225D-14 | -3.9662354D-20 | -1.3106268D-24 | -5.9463888D-30 | 2.2347952D-35  |
| 1  | -2.2378308D-07 | -5.3814000D-14 | -1.0581446D-19 | -1.0930926D-24 | -5.9117291D-29 | 8.4157746D-34  |
| 2  | -2.2371075D-07 | -6.9718216D-14 | -5.3513888D-19 | 1.0294819D-23  | -3.5173602D-29 | 1.1223025D-33  |
| 3  | -2.2452388D-07 | -4.3282687D-14 | -8.9677912D-19 | 2.9534187D-23  | 1.7003069D-28  | -8.0831316D-33 |
| 4  | -2.2584289D-07 | 6.1795944D-14  | -8.0680236D-19 | -3.3712631D-24 | 4.0795856D-28  | -9.1717344D-33 |
| 5  | -2.2706549D-07 | 1.4385379D-13  | -1.3757761D-19 | -8.0326282D-23 | -1.0976835D-28 | 2.7606916D-32  |
| 6  | -2.2816468D-07 | 6.6546324D-14  | 1.5206102D-19  | -4.5153221D-23 | -1.1052027D-27 | 1.3313597D-33  |
| 7  | -2.2981976D-07 | -7.8569366D-14 | -1.6015532D-18 | -6.8709140D-24 | -3.1136510D-28 | -3.5220257D-32 |
| 8  | -2.3375528D-07 | -2.3275422D-13 | -3.7637262D-18 | -4.0304717D-23 | 2.7915697D-27  | 3.7255476D-32  |
| 9  | -2.4124659D-07 | -4.0071575D-13 | -5.1071876D-20 | 3.7486023D-23  | 2.2190205D-27  | 6.4314969D-32  |
| 10 | -2.4865166D-07 | -4.3343730D-13 | 8.5698772D-18  | 1.9573654D-22  | -1.5082611D-27 | 5.4459922D-32  |
| 11 | -2.4928990D-07 | -1.9561768D-13 | 1.6419629D-17  | 4.4168848D-22  | 4.2480617D-28  | -2.5004122D-31 |
| 12 | -2.3752565D-07 | 4.5102335D-13  | 2.2544833D-17  | 1.3435102D-22  | -1.2080709D-26 | -3.3162967D-31 |
| 13 | -2.1100898D-07 | 1.0585619D-12  | 6.3474033D-18  | -6.6806490D-22 | -6.1378963D-27 | 5.5150352D-31  |
| 14 | -1.8216032D-07 | 9.1449891D-13  | -1.6764528D-17 | -3.6629318D-22 | 1.3603923D-26  | 2.4140812D-31  |
| 15 | -1.6495567D-07 | 4.2392254D-13  | -1.7322698D-17 | 2.4012420D-22  | -1.9315494D-27 | -5.4018979D-31 |
| 16 | -1.5850902D-07 | 1.3143771D-13  | -1.8850305D-17 | -1.2051458D-22 | -4.6779893D-27 | 1.9321938D-31  |
| 17 | -1.6200678D-07 | -2.8578020D-13 | -2.7531826D-17 | -7.6838298D-23 | 1.0237427D-26  | 2.7785918D-31  |
| 18 | -1.7877655D-07 | -7.5603595D-13 | -2.2276581D-17 | 3.6260971D-22  | -1.5257061D-27 | -2.7938784D-31 |
| 19 | -2.0477359D-07 | -9.1701839D-13 | -1.6136826D-17 | 2.2298514D-22  | -1.3330425D-26 | -5.0003750D-31 |
| 20 | -2.3510680D-07 | -9.5572702D-13 | -2.7241826D-17 | -3.9585714D-22 | 1.0307546D-26  | 5.2913821D-31  |
| 21 | -2.7333277D-07 | -1.2470125D-12 | -2.9020831D-17 | 1.4871832D-22  | 4.4727940D-26  | 3.9120184D-31  |
| 22 | -3.1827668D-07 | -1.1425929D-12 | 1.4411514D-17  | 1.1306835D-21  | 3.5853126D-26  | -3.5903222D-31 |
| 23 | -3.4997607D-07 | 1.5325712D-13  | 8.0170581D-17  | 5.2758644D-22  | -6.4820749D-26 | -2.9896585D-30 |
| 24 | -3.4614341D-07 | 1.8535321D-12  | 6.1704369D-17  | -3.5311269D-21 | -5.5186298D-26 | 5.3510976D-30  |
| 25 | -3.2261292D-07 | 1.5694273D-12  | 2.6776983D-18  | -1.1433015D-21 | 1.0221701D-25  | -9.6780881D-31 |
| 26 | -3.0560920D-07 | 7.6569466D-13  | 2.9594838D-17  | -6.6617664D-22 | -1.3429784D-25 | 2.3914289D-31  |
| 27 | -2.9162872D-07 | -3.0096661D-13 | -1.4385150D-17 | -8.6078859D-22 | 7.6654627D-27  | 3.9418663D-30  |
| 28 | -2.9318328D-07 | -1.9271660D-12 | -2.1943462D-17 | 2.9241969D-21  | 1.6295867D-27  | -2.5163114D-30 |
| 29 | -3.0805978D-07 | -2.4826936D-12 | 1.1120981D-17  | 4.6210647D-21  | -6.1085705D-26 | -1.0545158D-29 |
| 30 | -3.1832223D-07 | -1.6767512D-12 | -1.5941960D-17 | -1.0791842D-21 | -8.8567287D-26 | 9.1283948D-30  |
| 31 | -3.2726859D-07 | -1.9519337D-12 | -9.0713227D-17 | 3.6839656D-21  | 3.8361274D-25  | -9.2058857D-30 |
| 32 | -3.4641907D-07 | -1.0570085D-12 | 6.1965331D-19  | 1.2463119D-22  | -2.7489491D-25 | -2.6329394D-30 |
| 33 | -3.5446051D-07 | -2.1147519D-13 | -8.8681448D-17 | -3.4405732D-21 | 3.8679111D-25  | 7.6048656D-30  |
| 34 | -3.7062907D-07 | -3.2611898D-13 | -3.9936859D-17 | -2.4153345D-21 | -6.6864944D-26 | 2.4010071D-30  |
| 35 | -3.9046724D-07 | -4.4436557D-13 | -1.8755556D-17 | -1.9179873D-21 | 1.7118635D-25  | -6.5654027D-30 |
| 36 | -4.1098242D-07 | -3.5824513D-13 | 2.5583764D-17  | -8.0939218D-21 | -2.7558990D-25 | 3.5991138D-29  |
| 37 | -4.3198777D-07 | -1.6405571D-12 | 2.2651948D-17  | 2.7827077D-21  | 1.0641959D-25  | -3.5226284D-29 |
| 38 | -4.5540300D-07 | -1.7576537D-12 | 7.2904386D-17  | -7.3049932D-21 | -5.6336701D-25 | 6.0682981D-29  |
| 39 | -4.7684105D-07 | -3.3192244D-12 | 2.8758469D-17  | 8.4557082D-21  | -1.9104759D-25 | -7.9158687D-29 |
| 40 | -5.0179378D-07 | -3.7466141D-12 | -2.4629331D-17 | -2.2752697D-21 | 1.5813143D-25  | 6.2137612D-29  |
| 41 | -5.3315821D-07 | -4.9305357D-12 | -1.2250984D-17 | 6.1103486D-21  | -9.5901528D-25 | -5.5771801D-29 |
| 42 | -5.6905926D-07 | -6.0736737D-12 | -1.7979964D-16 | 7.2617653D-21  | 1.0412424D-24  | -6.3007604D-29 |
| 43 | -6.2031178D-07 | -6.9410683D-12 | -2.0366148D-16 | -9.6220417D-21 | -3.9349133D-25 | 1.1310092D-28  |

|    |                |                |                |                |                |                |
|----|----------------|----------------|----------------|----------------|----------------|----------------|
| 44 | -6.8880948D-07 | -9.6180302D-12 | -3.1555808D-16 | 2.4275150D-21  | -6.2274791D-25 | -1.9034487D-28 |
| 45 | -7.8410919D-07 | -1.3081562D-11 | -6.3431986D-16 | -2.4401641D-20 | 8.1329693D-25  | 9.0588942D-30  |
| 46 | -9.3260553D-07 | -2.0595619D-11 | -1.0619741D-15 | -7.2733400D-20 | -5.4757202D-24 | -1.9947967D-28 |
| 47 | -1.1844294D-06 | -4.0078900D-11 | -2.9140843D-15 | -2.5293707D-19 | -2.8497043D-23 | -3.7646279D-27 |
| 48 | -1.7538404D-06 | -1.1658337D-10 | -1.6874856D-14 | -3.3614203D-18 | -8.5632375D-22 | -2.6624730D-25 |
| 49 | -2.8819756D-05 | 1.5937312D-07  | -8.0935569D-10 | 3.5359032D-12  | -1.1758231D-14 | 1.3457528D-17  |
