# Supplementary material for: Ab initio spectroscopic studies of AlF and AlCl molecules
Source: arXiv:2303.08681 source file (2023-03-15)
Supplement: Supplementary file 12 [file AlF_a3Pi_S2.pdf]

AlF a<sup>3</sup>Pi --> Centrifugal distortion constants (in cm<sup>-1</sup>)

| v  | Dv             | Hv             | Lv             | Mv             | Nv             | Ov             |
|----|----------------|----------------|----------------|----------------|----------------|----------------|
| 0  | -7.9096679D-07 | -1.9992810D-12 | -3.3141288D-17 | 1.0304719D-21  | -1.0306608D-27 | 6.0605367D-32  |
| 1  | -8.4932871D-07 | 4.6839744D-12  | -1.4852851D-16 | 1.1520425D-21  | -2.8719719D-26 | 1.2858964D-30  |
| 2  | -1.0950384D-06 | 9.5072081D-12  | -1.3344603D-16 | 3.3983116D-21  | -2.3010943D-25 | 8.1387649D-30  |
| 3  | -1.3027540D-06 | 1.3845491D-11  | -5.0544072D-16 | 2.2711875D-20  | -5.4205079D-25 | 4.9099178D-31  |
| 4  | -1.6455873D-06 | 3.1047346D-11  | -9.5359827D-16 | 7.3977306D-22  | 1.6924958D-24  | -1.0984760D-28 |
| 5  | -2.0887595D-06 | 3.0316392D-11  | 6.1027112D-16  | -9.7878780D-20 | 4.3640426D-24  | -4.1340669D-29 |
| 6  | -2.1653580D-06 | -3.2434864D-12 | 2.6164549D-15  | -9.9291077D-20 | -4.3586471D-24 | 6.9876500D-28  |
| 7  | -1.8199946D-06 | -4.3631325D-11 | 1.9968848D-15  | 1.8513736D-19  | -1.4355897D-23 | -6.6417512D-28 |
| 8  | -1.3333341D-06 | -3.4626970D-11 | -2.3653632D-15 | 1.2025270D-19  | 1.8530284D-23  | -4.9871131D-28 |
| 9  | -1.2364569D-06 | -4.9192115D-12 | -6.8860222D-16 | -1.6066262D-19 | -1.5656491D-24 | 1.0795305D-27  |
| 10 | -1.2220717D-06 | -1.1130711D-11 | 3.4512336D-16  | 4.4289535D-20  | -5.6517850D-24 | -6.0948305D-28 |
| 11 | -1.1650013D-06 | -7.2421491D-12 | -3.0531438D-16 | -1.5807271D-20 | 3.5187730D-24  | 2.4964618D-28  |
| 12 | -1.1412622D-06 | -7.0839737D-12 | 1.6561367D-16  | 2.2081962D-20  | -4.6675435D-24 | -2.1103123D-28 |
| 13 | -1.0906300D-06 | -4.5521737D-12 | -7.0881522D-16 | 1.3381634D-20  | 7.6457619D-24  | -1.8511353D-28 |
| 14 | -1.0998244D-06 | 1.0758394D-12  | 8.8400287D-17  | -8.8212052D-20 | -2.4073171D-24 | 8.3070284D-28  |
| 15 | -1.1019911D-06 | -5.1388225D-12 | 5.7202479D-16  | 5.5201592D-20  | -8.1062287D-24 | -6.5872284D-28 |
| 16 | -1.0585583D-06 | -4.6727863D-12 | -5.6827071D-16 | 4.0878016D-20  | 8.8675489D-24  | -3.3973151D-28 |
| 17 | -1.0555624D-06 | 4.6465806D-13  | -1.4233993D-16 | -7.0660830D-20 | 2.9603049D-25  | 8.6418994D-28  |
| 18 | -1.0592702D-06 | -2.2000407D-12 | 3.6112273D-16  | 1.9626524D-20  | -7.0245612D-24 | -3.9461922D-28 |
| 19 | -1.0379411D-06 | -2.7241852D-12 | -3.0207899D-16 | 3.1860113D-20  | 6.0299559D-24  | -4.1555807D-28 |
| 20 | -1.0357028D-06 | 2.1820205D-13  | -4.7517999D-17 | -5.5393322D-20 | 7.7224646D-25  | 8.0425682D-28  |
| 21 | -1.0361488D-06 | -1.9821940D-12 | 3.7000929D-16  | 1.1803392D-20  | -7.8295194D-24 | -1.7392403D-28 |
| 22 | -1.0177371D-06 | -3.6017356D-12 | -2.0394244D-16 | 6.5418973D-20  | 3.6782054D-24  | -9.3010334D-28 |
| 23 | -1.0075389D-06 | 6.5546360D-14  | -4.4053728D-16 | -4.2013466D-20 | 8.2784133D-24  | 6.4317515D-28  |
| 24 | -1.0165683D-06 | 7.9179173D-13  | 2.6936572D-16  | -6.0634275D-20 | -6.3123856D-24 | 8.4298247D-28  |
| 25 | -1.0144146D-06 | -2.5189537D-12 | 3.6009740D-16  | 4.4749820D-20  | -7.5064675D-24 | -7.6605625D-28 |
| 26 | -9.9922202D-07 | -3.0821092D-12 | -2.6657501D-16 | 5.6612676D-20  | 6.4238035D-24  | -8.3723803D-28 |
| 27 | -9.9398865D-07 | -2.0794960D-13 | -3.4187574D-16 | -4.4328128D-20 | 7.0320400D-24  | 8.4315878D-28  |
| 28 | -1.0005660D-06 | 2.8058662D-14  | 2.1289399D-16  | -4.6233225D-20 | -6.5061467D-24 | 7.3427517D-28  |
| 29 | -9.9960279D-07 | -2.2258836D-12 | 2.2111494D-16  | 3.9163622D-20  | -5.8135701D-24 | -8.0280641D-28 |
| 30 | -9.9235150D-07 | -2.3974965D-12 | -2.1597905D-16 | 4.0049067D-20  | 5.7067252D-24  | -7.3211252D-28 |
| 31 | -9.9180633D-07 | -6.1512847D-13 | -2.5862857D-16 | -3.6290898D-20 | 6.5475169D-24  | 7.3284069D-28  |
| 32 | -9.9900951D-07 | -4.1545733D-13 | 1.7362459D-16  | -4.9708415D-20 | -5.3868225D-24 | 9.6614842D-28  |
| 33 | -1.0022979D-06 | -2.4739445D-12 | 2.8315755D-16  | 3.0963380D-20  | -8.5186235D-24 | -6.4016607D-28 |
| 34 | -9.9913989D-07 | -3.3276604D-12 | -1.4363481D-16 | 6.1871677D-20  | 3.3570274D-24  | -1.2280168D-27 |
| 35 | -9.9993305D-07 | -1.8619763D-12 | -3.9240993D-16 | -5.8115817D-21 | 1.0085718D-23  | 1.5226972D-28  |
| 36 | -1.0095723D-06 | -5.9958814D-13 | -1.1907534D-16 | -6.6507253D-20 | 2.1876822D-24  | 1.3428879D-27  |
| 37 | -1.0223650D-06 | -1.4867559D-12 | 2.7960272D-16  | -3.7675310D-20 | -9.3027709D-24 | 7.1992040D-28  |
| 38 | -1.0310240D-06 | -3.5969619D-12 | 2.5966463D-16  | 4.3982372D-20  | -8.6146760D-24 | -1.0194290D-27 |
| 39 | -1.0363670D-06 | -4.4445963D-12 | -1.5703260D-16 | 6.6172338D-20  | 4.1042020D-24  | -1.4409460D-27 |
| 40 | -1.0460220D-06 | -3.4677369D-12 | -4.0519253D-16 | 7.9324370D-22  | 1.1103206D-23  | 9.5599369D-29  |
| 41 | -1.0638207D-06 | -2.5781346D-12 | -2.1143676D-16 | -6.0458267D-20 | 3.8814485D-24  | 1.4275988D-27  |
| 42 | -1.0865052D-06 | -3.2672392D-12 | 1.1735649D-16  | -4.7846607D-20 | -7.1965946D-24 | 1.0162201D-27  |
| 43 | -1.1098703D-06 | -5.1015481D-12 | 1.9376450D-16  | 1.4337304D-20  | -9.7710043D-24 | -5.0706718D-28 |

|    |                |                |                |                |                |                |
|----|----------------|----------------|----------------|----------------|----------------|----------------|
| 44 | -1.1338361D-06 | -6.7041406D-12 | -5.1802571D-17 | 5.6275031D-20  | -1.6469905D-24 | -1.5226168D-27 |
| 45 | -1.1624429D-06 | -7.2745440D-12 | -3.6338617D-16 | 3.2914965D-20  | 8.5579932D-24  | -8.9633545D-28 |
| 46 | -1.2003749D-06 | -7.3807200D-12 | -4.3603344D-16 | -3.1402627D-20 | 9.5772497D-24  | 7.9549084D-28  |
| 47 | -1.2495904D-06 | -8.3485953D-12 | -2.4951538D-16 | -6.8446751D-20 | 6.9853824D-26  | 1.7124553D-27  |
| 48 | -1.3099062D-06 | -1.0910642D-11 | -7.6714684D-17 | -4.4132468D-20 | -9.9243503D-24 | 8.8778377D-28  |
| 49 | -1.3827831D-06 | -1.4778168D-11 | -1.7187115D-16 | 9.6530386D-21  | -1.1005195D-23 | -7.9496949D-28 |
| 50 | -1.4741002D-06 | -1.9442902D-11 | -5.5229176D-16 | 3.8998016D-20  | -3.2333833D-24 | -1.8167293D-27 |
| 51 | -1.5940325D-06 | -2.4978375D-11 | -1.0514683D-15 | 1.9849265D-20  | 6.6486208D-24  | -1.4708551D-27 |
| 52 | -1.7546603D-06 | -3.1939790D-11 | -1.4719411D-15 | -3.4783715D-20 | 1.1249967D-23  | -1.9147356D-28 |
